# Supplementary material for: 3 mm Spectroscopic Observations of Massive Star-Forming Regions with IRAM 30-m
Source: arXiv:2412.09823 source file (2024-12-13)
Supplement: Supplementary file 1 [file IRAM_supplement.pdf]

doi: 10.1093/pasj/xxx000

# 3 mm Spectroscopic Observations of Massive Star-Forming Regions with IRAM 30-m

**Xuefang Xu[1,2], Junzhi Wang[3], Qian Gou[1,2], Juan Li[4,5], Donghui Quan[6], Di Li[7,8], Fei Li[9], Chunguo Duan[1,2], and Juncheng Lei[1,2]**

[1]School of Chemistry and Chemical Engineering, Chongqing University, Chongqing 401331, China
[2]Chongqing Key Laboratory of Chemical Theory and Mechanism, Chongqing 401331, China
[3]Guangxi Key Laboratory for Relativistic Astrophysics, Department of Physics, Guangxi University, Nanning 530004, China
[4]Shanghai Astronomical Observatory, Chinese Academy of Sciences, 80 Nandan Road, Shanghai 200030, China
[5]Key Laboratory of Radio Astronomy, Chinese Academy of Sciences, China
[6]Research Center for Intelligent Computing Platforms, Zhejiang Laboratory, Hangzhou 311100, China
[7]Department of Astronomy, Tsinghua University, Beijing 100084, China
[8]National Astronomical Observatories, Chinese Academy of Sciences, Beijing 100012, China
[9]School of Astronomy and Space Science, Nanjing University, Nanjing 210093, China

*E-mail: junzhiwang@gxu.edu.cn, qian.gou@cqu.edu.cn

Received ; Accepted

## Abstract

Broadband spectroscopic observations with high sensitivity provide an unbiased way to detect emissions of molecules in space. We present deep observations from ∼105.8 GHz to 113.6 GHz toward 50 Galactic massive star-forming regions using IRAM 30-m millimeter telescope, with noise levels ranging from 6 to 29 mK at frequency channel spacing of 195 kHz, which corresponds to $\sim$ 0.54 km s$^{-1}$ at 110 GHz. Totally, 27 molecular species have been identified, of which 16 are complex organic molecules. The related parameters, such as peak temperature, integrated intensity, and line width of the identified molecular lines were obtained. This provides a useful dataset for investigating astro-chemical evolution of molecules in massive star-forming cores.

**Key words:** key word$astrochemistry_1$ — key word$line: identification_2$ — key word$ISM: clouds_3$ — . . . — key word$ISM: molecules_4$

## Appendix. Supplementary material

© 2018. Astronomical Society of Japan.

**Table A1.** Rotational temperatures and column densities of detected molecules using in Weeds

| Source | Species | Rotational Temperature (K) | Column Density ($cm^{-2}$) | Velocity offset (km $s^{-1}$) |
|---|---|---|---|---|
| (1) | (2) | (3) | (4) | (5) |
| | $NH_2CHO$ | 45 | $1.8\times10^{15}$ | 0.2 |
| | CCS | 45 | $2.5\times10^{14}$ | 0.5 |
| | $C_2H_5CN$ | 45 | $2.0\times10^{14}$ | 0. |
| | $HC_5N$ | 45 | $8.5\times10^{13}$ | 0. |
| | $C_2H_3CN$ | 45 | $8.0\times10^{14}$ | 0.5 |
| | $C_2H_5OH$ | 45 | $3.5\times10^{15}$ | 0. |
| | $CH_3OCH_3$ | 45 | $9.0\times10^{15}$ | 0. |
| | $OC^{34}S$ | 45 | $1.5\times10^{15}$ | 0. |
| | $CH_3OH$ | 45 | $3.3\times10^{16}$ | -2.0 |
| | $CH_3C^{15}N$ | 45 | $8.5\times10^{13}$ | -2.0 |
| | $^{13}CH_3CN$ | 45 | $1.0\times10^{14}$ | 0. |
| | $CH_3SH$ | 45 | $4.5\times10^{15}$ | 0. |
| | $CH_3OCHO$ | 45 | $1.0\times10^{16}$ | 0. |
| G000.67−00.03 | $SO_2$ | 45 | $1.6\times10^{16}$ | -2.0 |
| | t-HCOOH | 45 | $1.5\times10^{15}$ | 0. |
| | SiS | 45 | $9.0\times10^{14}$ | 0. |
| | $HC_3N$ | 45 | $4.0\times10^{15}$ | 0. |
| | SO | 45 | $1.2\times10^{16}$ | 0. |
| | $HC_3N$, $v_7$=1 | 45 | $1.0\times10^{17}$ | 0. |
| | OCS | 45 | $1.3\times10^{16}$ | 0. |
| | HNCO | 45 | $1.2\times10^{15}$ | 0. |
| | $C^{18}O$ | 45 | $5.1\times10^{17}$ | 3.0 |
| | $^{13}CO$ | 85 | $8.0\times10^{18}$ | 3.0 |
| | $CH_3{}^{13}CN$ | 45 | $1.2\times10^{14}$ | 0. |
| | $CH_3CN$ | 45 | $1.5\times10^{15}$ | 0. |
| | $CH_3CHO$ | 45 | $2.6\times10^{15}$ | 0. |
| | $C^{17}O$ | 45 | $1.6\times10^{17}$ | 3.5 |
| | CN | 85 | $1.0\times10^{15}$ | -2.0 |
| | CCS | 45 | $5.2\times10^{13}$ | 0. |
| | $HC_5N$ | 45 | $9.5\times10^{13}$ | -0.5 |
| | $C_2H_3CN$ | 45 | $1.1\times10^{14}$ | -0.5 |
| | $CH_3OH$ | 45 | $6.5\times10^{15}$ | 0.5 |
| | $SO_2$ | 45 | $1.0\times10^{18}$ | 0. |
| | $CH_3C_3N$ | 45 | $7.0\times10^{13}$ | 0. |
| | $^{13}CN$ | 45 | $3.2\times10^{14}$ | -0.7 |
| | $HC_3N$ | 85 | $8.5\times10^{15}$ | 0. |
| | SO | 45 | $1.0\times10^{16}$ | 0. |
| G005.88−00.39 | $HC_3N$, $v_7$=1 | 85 | $1.5\times10^{15}$ | 0.5 |
| | OCS | 45 | $3.0\times10^{15}$ | 0.5 |
| | $C^{18}O$ | 85 | $4.3\times10^{17}$ | 0. |
| | HNCO | 45 | $2.5\times10^{14}$ | 0. |
| | $C^{15}N$ | 45 | $8.5\times10^{13}$ | 0. |
| | $^{13}CO$ | 85 | $9.2\times10^{18}$ | 0. |
| | $CH_3CN$ | 45 | $7.5\times10^{14}$ | 0. |
| | $CH_3OCHO$ | 45 | $3.4\times10^{14}$ | -0.5 |
| | $CH_3OCH_3$ | 45 | $1.0\times10^{15}$ | 1.0 |
| | $C^{17}O$ | 45 | $5.5\times10^{16}$ | 0. |
| | CN | 85 | $3.0\times10^{16}$ | 0. |
| | $NH_2CHO$ | 45 | $7.0\times10^{13}$ | 1.0 |
| | CCS | 45 | $2.5\times10^{13}$ | 1.5 |
| | $HC_5N$ | 45 | $2.0\times10^{13}$ | 1.5 |
| | $C_2H_5OH$ | 45 | $4.1\times10^{14}$ | 2.0 |
| | $^{34}SO$ | 45 | $1.1\times10^{14}$ | 3.0 |
| | $CH_3OCH_3$ | 45 | $1.0\times10^{15}$ | 1.0 |
| | $OC^{34}S$ | 45 | $2.3\times10^{14}$ | 2.0 |
| | $CH_3OH$ | 85 | $1.2\times10^{16}$ | 2.5 |
| | $C_2H_5CN$ | 45 | $7.3\times10^{13}$ | 3.0 |
| | $^{13}CH_3CN$ | 45 | $5.5\times10^{12}$ | 2.0 |
| | $CH_3OCHO$ | 45 | $1.3\times10^{15}$ | 2.0 |
| | t-HCOOH | 45 | $6.7\times10^{13}$ | 1.5 |
| G009.62+00.19 | $^{13}CN$ | 45 | $1.2\times10^{14}$ | 2.3 |
| | $HC_3N$ | 85 | $9.2\times10^{14}$ | 2.0 |
| | SO | 45 | $2.0\times10^{15}$ | 2.5 |
| | $HC_3N$, $v_7$=1 | 85 | $6.5\times10^{14}$ | 1.0 |
| | OCS | 45 | $2.7\times10^{15}$ | 2.5 |
| | HNCO | 45 | $1.2\times10^{14}$ | 2.0 |
| | $C^{18}O$ | 85 | $4.3\times10^{17}$ | 2.0 |
| | $C^{15}N$ | 45 | $1.5\times10^{12}$ | 2.5 |
| | $^{13}CO$ | 85 | $8.5\times10^{18}$ | 2.5 |
| | $CH_3CN$ | 45 | $2.0\times10^{14}$ | 2.0 |
| | $C_2H_3CN$ | 45 | $1.1\times10^{13}$ | 2.5 |
| | $CH_3CHO$ | 45 | $1.4\times10^{14}$ | 2.0 |
| | $C^{17}O$ | 45 | $7.0\times10^{13}$ | 1.5 |
| | CN | 85 | $1.0\times10^{16}$ | 2.2 |
| | $SO_2$, $v_2$=1 | 85 | $1.5\times10^{18}$ | -2.0 |
| | $NH_2CHO$ | 45 | $1.3\times10^{15}$ | -2.0 |
| | $CH_3OCHO$ | 45 | $7.0\times10^{15}$ | -2.0 |
| | $^{13}CH_3CH_2CN$ | 45 | $1.2\times10^{14}$ | -2.0 |
| | CCS | 45 | $2.7\times10^{13}$ | -2.0 |
| | $C_2H_5OH$ | 45 | $3.0\times10^{15}$ | -2.0 |
| | HCOCN | 45 | $1.0\times10^{14}$ | -5.0 |
| | $HC_5N$ | 45 | $3.0\times10^{13}$ | -2.0 |
| | $C_2H_5{}^{13}CN$ | 45 | $5.5\times10^{13}$ | -3.0 |
| | $C_2H_5CN$ | 45 | $5.5\times10^{16}$ | -2.0 |
| | $C_2H_3CN$ | 45 | $7.5\times10^{14}$ | -2.0 |
| | $^{34}SO$ | 45 | $5.0\times10^{14}$ | -2.0 |
| | $CH_3OCH_3$ | 45 | $1.5\times10^{16}$ | -2.0 |
| | $OC^{34}S$ | 45 | $1.8\times10^{15}$ | -3.0 |
| | CCS | 45 | $2.0\times10^{13}$ | 1.0 |
| | $HC_5N$ | 45 | $1.5\times10^{13}$ | 1.0 |
| | $^{34}SO$ | 45 | $3.7\times10^{13}$ | -0.5 |
| | $CH_3OH$ | 85 | $2.2\times10^{15}$ | 0. |
| | t-HCOOH | 85 | $1.2\times10^{14}$ | 1.0 |
| | $^{13}CN$ | 85 | $1.0\times10^{14}$ | 1.0 |
| | $HC_3N$ | 85 | $3.0\times10^{14}$ | 1.0 |
| G035.02+00.34 | SO | 45 | $1.5\times10^{15}$ | 0.5 |
| | OCS | 45 | $4.7\times10^{14}$ | 0.5 |
| | $C^{18}O$ | 85 | $2.2\times10^{17}$ | 0. |
| | HNCO | 45 | $7.5\times10^{13}$ | 1.0 |
| | $^{13}CO$ | 85 | $1.7\times10^{18}$ | 0. |
| | $CH_3CN$ | 45 | $3.8\times10^{13}$ | 0. |
| | $CH_3CHO$ | 45 | $1.7\times10^{14}$ | 0. |
| | $C^{17}O$ | 45 | $3.3\times10^{16}$ | 0.2 |
| | CN | 45 | $3.5\times10^{15}$ | 1.0 |
| | $NH_2CHO$ | 45 | $2.3\times10^{13}$ | 3.0 |
| | CCS | 45 | $2.7\times10^{13}$ | 4.0 |
| | $HC_5N$ | 45 | $2.2\times10^{13}$ | 4.5 |
| | $^{34}SO$ | 45 | $4.5\times10^{13}$ | 2.0 |
| | $CH_3OCH_3$ | 45 | $1.5\times10^{15}$ | 2.0 |
| | $OC^{34}S$ | 45 | $1.0\times10^{14}$ | 2.0 |
| | $CH_3OH$ | 85 | $2.7\times10^{16}$ | 1.5 |
| | $CH_3OCHO$ | 85 | $1.2\times10^{15}$ | 3.0 |
| | $SO_2$ | 85 | $1.7\times10^{15}$ | 1.0 |
| | t-HCOOH | 85 | $3.0\times10^{14}$ | 4.0 |
| G035.19−00.74 | $^{13}CN$ | 85 | $2.0\times10^{14}$ | 4.0 |
| | $HC_3N$ | 85 | $6.0\times10^{14}$ | 4.0 |
| | SO | 45 | $1.8\times10^{15}$ | 4.0 |
| | OCS | 45 | $1.3\times10^{15}$ | 4.0 |
| | $C^{18}O$ | 85 | $2.0\times10^{17}$ | 4.0 |
| | HNCO | 45 | $2.5\times10^{14}$ | 4.0 |
| | $C^{15}N$ | 45 | $3.0\times10^{13}$ | 4.0 |
| | $^{13}CO$ | 85 | $3.0\times10^{18}$ | 4.0 |
| | $CH_3CN$ | 45 | $1.7\times10^{14}$ | 3.5 |
| | $CH_3CHO$ | 45 | $5.2\times10^{14}$ | 4.0 |
| | $C^{17}O$ | 45 | $2.3\times10^{16}$ | 4.0 |
| | CN | 45 | $3.0\times10^{15}$ | 4.0 |
| | CCS | 45 | $8.5\times10^{12}$ | 2.0 |
| | $CH_3OH$ | 85 | $1.0\times10^{15}$ | 1.5 |
| | t-HCOOH | 85 | $1.0\times10^{14}$ | 2.0 |
| | $^{13}CN$ | 85 | $1.2\times10^{14}$ | 2.0 |
| | $HC_3N$ | 85 | $1.5\times10^{14}$ | 2.0 |
| | SO | 45 | $1.0\times10^{15}$ | 2.0 |
| | OCS | 45 | $4.0\times10^{14}$ | 2.0 |
| G035.20−01.73 | $C^{18}O$ | 85 | $1.1\times10^{17}$ | 2.0 |
| | HNCO | 45 | $4.5\times10^{13}$ | 2.0 |
| | $C^{15}N$ | 45 | $4.0\times10^{13}$ | 2.0 |
| | $^{13}CO$ | 85 | $1.7\times10^{18}$ | 2.0 |
| | $CH_3CN$ | 45 | $4.1\times10^{13}$ | 2.0 |
| | $CH_3CHO$ | 45 | $1.0\times10^{14}$ | 2.0 |
| | $C^{17}O$ | 45 | $2.0\times10^{16}$ | 2.0 |
| | CN | 45 | $3.0\times10^{15}$ | 1.0 |
| | CCS | 45 | $1.7\times10^{13}$ | 3.0 |
| | $HC_5N$ | 45 | $1.2\times10^{13}$ | 3.5 |
| | $^{34}SO$ | 45 | $3.3\times10^{13}$ | 2.0 |
| | $CH_3OH$ | 85 | $4.0\times10^{15}$ | 2.5 |
| | $CH_3OCHO$ | 45 | $4.7\times10^{14}$ | 3.5 |
| | $SO_2$ | 85 | $4.5\times10^{14}$ | 3.0 |
| | t-HCOOH | 85 | $1.5\times10^{14}$ | 3.0 |
| | $^{13}CN$ | 85 | $1.0\times10^{14}$ | 2.5 |
| | $HC_3N$ | 85 | $1.7\times10^{14}$ | 3.0 |
| G037.43+01.51 | SO | 45 | $1.3\times10^{15}$ | 3.0 |
| | OCS | 45 | $4.7\times10^{14}$ | 3.0 |
| | HNCO | 45 | $7.0\times10^{13}$ | 2.5 |
| | $C^{18}O$ | 85 | $1.9\times10^{17}$ | 3.0 |
| | $C^{15}N$ | 45 | $1.0\times10^{13}$ | 2.5 |
| | $^{13}CO$ | 85 | $4.4\times10^{18}$ | 3.0 |
| | $CH_3CN$ | 45 | $5.0\times10^{13}$ | 3.0 |
| | $CH_3OCH_3$ | 45 | $1.0\times10^{15}$ | 3.0 |
| | $CH_3CHO$ | 45 | $1.3\times10^{14}$ | 3.0 |
| | $C^{17}O$ | 45 | $2.6\times10^{16}$ | 3.0 |
| | CN | 85 | $1.0\times10^{15}$ | 3.0 |
| | $SO_2$, $v_2$=1 | 85 | $2.0\times10^{18}$ | 0. |
| | CCS | 45 | $2.5\times10^{13}$ | -2.0 |
| | $^{34}SO$ | 45 | $4.5\times10^{15}$ | 2.0 |
| | $CH_3OH$ | 85 | $5.7\times10^{15}$ | 2.0 |
| | $SO_2$ | 85 | $7.0\times10^{16}$ | 1.0 |
| | $C_2H_5CN$ | 45 | $7.0\times10^{13}$ | 2.0 |
| | $^{33}SO$ | 85 | $1.0\times10^{15}$ | 0. |
| | t-HCOOH | 85 | $1.5\times10^{15}$ | -2.0 |
| | $HC_3N$ | 85 | $1.5\times10^{14}$ | 0. |
| | SO | 85 | $5.1\times10^{16}$ | -2.0 |
| G043.16+00.01 | $HC_3N$, v7=1 | 85 | $1.5\times10^{15}$ | 0. |
| | OCS | 45 | $4.1\times10^{15}$ | -0.5 |
| | HNCO | 45 | $3.0\times10^{14}$ | 0. |
| | $C^{18}O$ | 85 | $4.1\times10^{17}$ | 0. |
| | $^{13}CO$ | 85 | $9.1\times10^{18}$ | 0. |

**Table A1.** (Continued)

| Source (1) | Species (2) | Rotational Temperature (K) (3) | Column Density ($cm^{-2}$) (4) | Velocity offset ($km\ s^{-1}$) (5) |
|---|---|---|---|---|
| | $CH_3COCH_3$ | 45 | $1.5\times10^{15}$ | -2.0 |
| | $C_2H_5CN$, $v_{12}$=1−A | 85 | $1.0\times10^{18}$ | -2.0 |
| | aGg'−$(CH_2OH)_2$ | 45 | $3.5\times10^{14}$ | -4.0 |
| | $HOCO^+$ | 45 | $1.5\times10^{13}$ | 0. |
| | $CH_3OCH_2OH$ | 45 | $6.5\times10^{16}$ | -2.0 |
| | $CH_3{}^{13}CH_2CN$ | 45 | $2.0\times10^{13}$ | -2.0 |
| | $CH_3OH$ | 85 | $7.5\times10^{16}$ | -2.0 |
| | $SO_2$ | 85 | $1.8\times10^{17}$ | -2.0 |
| | $C_2H_5CN$, $v_{20}$=1−A | 85 | $2.5\times10^{17}$ | -2.0 |
| | $^{13}CH_3CN$ | 85 | $2.5\times10^{14}$ | -2.0 |
| G010.47+00.02 | $CH_3C_3N$ | 85 | $2.5\times10^{13}$ | -3.0 |
| | $OC^{33}S$ | 45 | $3.5\times10^{14}$ | -2.0 |
| | t-HCOOH | 85 | $1.0\times10^{15}$ | -2.0 |
| | $^{13}CN$ | 85 | $1.0\times10^{14}$ | -2.0 |
| | SiS | 85 | $2.0\times10^{13}$ | -1.0 |
| | $HC_3N$, $v_4$=1 | 85 | $4.0\times10^{19}$ | -1.0 |
| | $HC_3N$ | 85 | $1.4\times10^{15}$ | -2.0 |
| | $O^{13}CS$ | 85 | $5.5\times10^{14}$ | -2.0 |
| | $HC_3N$, $v_5$=1/$v_7$=3 | 85 | $3.0\times10^{18}$ | -2.0 |
| | SO | 45 | $6.2\times10^{15}$ | -2.0 |
| | $HC_3N$, $v_6$=1 | 85 | $3.2\times10^{17}$ | -2.0 |
| | $HC_3N$, $v_7$=1 | 85 | $6.5\times10^{15}$ | -2.0 |
| | OCS | 45 | $9.2\times10^{15}$ | -2.0 |
| | HNCO | 45 | $1.1\times10^{15}$ | -2.0 |
| | $HC_3N$, $v_6$=$v_7$=1 | 85 | $7.2\times10^{18}$ | -2.0 |
| | $C^{18}O$ | 85 | $4.3\times10^{17}$ | -2.0 |
| | $HC_3N$, $v_7$=2 | 85 | $1.0\times10^{17}$ | -2.0 |
| | $^{13}CO$ | 85 | $6.5\times10^{19}$ | -2.5 |
| | $CH_3{}^{13}CN$ | 85 | $2.0\times10^{14}$ | -2.0 |
| | $CH_3CN$ | 85 | $1.2\times10^{15}$ | -2.0 |
| | $CH_3CN$, $v_8$=1 | 85 | $1.2\times10^{17}$ | -2.0 |
| | $^{13}CH_2CHCN$ | 85 | $1.2\times10^{13}$ | -2.0 |
| | $CH_3COOH$ | 45 | $1.5\times10^{16}$ | -2.0 |
| | $CH_3CHO$ | 45 | $6.5\times10^{14}$ | -2.0 |
| | $C^{17}O$ | 45 | $5.5\times10^{16}$ | -2.0 |
| | CN | 45 | $6.3\times10^{15}$ | -2.3 |
| | $NH_2CHO$ | 45 | $1.0\times10^{14}$ | 0. |
| | CCS | 45 | $9.0\times10^{13}$ | 0. |
| | $HC_5N$ | 45 | $5.0\times10^{13}$ | 0. |
| | $CH_3SH$ | 45 | $1.7\times10^{15}$ | 0. |
| | $C_2H_3CN$ | 45 | $4.5\times10^{13}$ | -0.5 |
| | $C_2H_5OH$ | 45 | $4.1\times10^{14}$ | 0. |
| | $OC^{34}S$ | 45 | $1.8\times10^{14}$ | 0. |
| | $CH_3OH$ | 45 | $1.3\times10^{14}$ | -1.0 |
| | $SO_2$ | 45 | $3.5\times10^{17}$ | 3.0 |
| | $^{13}CH_3CN$ | 45 | $5.5\times10^{12}$ | 2.0 |
| | $^{13}C^{17}O$ | 45 | $3.1\times10^{15}$ | 1.5 |
| | $C_2H_5CN$ | 45 | $5.0\times10^{13}$ | -1.0 |
| | t-HCOOH | 45 | $3.7\times10^{14}$ | 0. |
| | $^{13}CN$ | 45 | $3.2\times10^{14}$ | 0. |
| G010.62−00.38 | SiS | 45 | $1.0\times10^{14}$ | -1.0 |
| | $HC_3N$ | 85 | $1.7\times10^{15}$ | 0. |
| | SO | 45 | $5.2\times10^{15}$ | 0.5 |
| | $HC_3N$, $v_7$=1 | 85 | $3.0\times10^{14}$ | 0. |
| | OCS | 45 | $3.5\times10^{15}$ | 0. |
| | $C^{18}O$ | 85 | $1.7\times10^{18}$ | 0. |
| | HNCO | 45 | $4.3\times10^{14}$ | -0.5 |
| | $C^{15}N$ | 45 | $2.5\times10^{12}$ | -1.5 |
| | $^{13}CO$ | 85 | $1.8\times10^{19}$ | 0. |
| | $CH_3CN$ | 45 | $2.0\times10^{14}$ | -1.0 |
| | $CH_3OCHO$ | 45 | $1.0\times10^{15}$ | -1.0 |
| | $CH_3OCH_3$ | 45 | $3.0\times10^{15}$ | -1.0 |
| | $CH_3CHO$ | 45 | $1.1\times10^{15}$ | 0. |
| | $C^{17}O$ | 85 | $2.0\times10^{17}$ | 0. |
| | CN | 85 | $2.0\times10^{16}$ | 0. |
| | $CH_3OH$ | 85 | $5.3\times10^{15}$ | -20 |
| | $^{13}CN$ | 45 | $5.2\times10^{13}$ | -0.5 |
| | $HC_3N$ | 85 | $1.4\times10^{14}$ | -0.5 |
| | SO | 45 | $3.2\times10^{14}$ | -0.5 |
| G011.49−01.48 | $C^{18}O$ | 85 | $1.7\times10^{16}$ | -0.5 |
| | $^{13}CO$ | 85 | $1.7\times10^{19}$ | -1.0 |
| | $CH_3CN$ | 45 | $2.0\times10^{13}$ | -1.0 |
| | $C^{17}O$ | 45 | $8.5\times10^{15}$ | -1.0 |
| | CN | 85 | $5.0\times10^{15}$ | -1.0 |
| | $NH_2CHO$ | 45 | $4.6\times10^{13}$ | -1.0 |
| | CCS | 45 | $1.7\times10^{13}$ | -1.0 |
| | $HC_5N$ | 45 | $3.0\times10^{13}$ | -1.0 |
| | $C_2H_3CN$ | 45 | $4.5\times10^{13}$ | -1.0 |
| | $CH_3OH$ | 85 | $1.5\times10^{15}$ | 0. |
| | $C_2H_5CN$ | 45 | $7.0\times10^{13}$ | -0.5 |
| | $CH_3OCHO$ | 45 | $3.0\times10^{14}$ | -1.0 |
| | t-HCOOH | 85 | $1.2\times10^{14}$ | 0. |
| | $^{13}CN$ | 45 | $1.0\times10^{14}$ | -1.0 |
| | $HC_3N$ | 85 | $3.2\times10^{14}$ | -1.0 |
| G011.91−00.61 | SO | 45 | $6.1\times10^{14}$ | -0.5 |
| | $HC_3N$, $v_7$=1 | 85 | $1.0\times10^{14}$ | -1.0 |
| | OCS | 45 | $1.0\times10^{15}$ | -1.0 |
| | $C^{18}O$ | 85 | $9.0\times10^{16}$ | -0.5 |
| | $CH_3CN$ | 45 | $2.0\times10^{14}$ | 0. |
| | $CH_3OCHO$ | 45 | $4.3\times10^{14}$ | 0. |
| | $CH_3OCH_3$ | 45 | $1.5\times10^{15}$ | 0. |
| | $CH_3CHO$ | 45 | $6.0\times10^{14}$ | -4.0 |
| | $C^{17}O$ | 45 | $8.0\times10^{16}$ | -1.5 |
| | CN | 45 | $5.7\times10^{15}$ | -4.0 |
| | $NH_2CHO$ | 45 | $1.6\times10^{13}$ | -1.0 |
| | CCS | 45 | $1.3\times10^{13}$ | -0.5 |
| | $^{34}SO$ | 45 | $7.0\times10^{13}$ | -0.5 |
| | $OC^{34}S$ | 45 | $7.2\times10^{13}$ | -0.5 |
| | $CH_3OH$ | 85 | $4.3\times10^{15}$ | -0.5 |
| | $^{13}C^{17}O$ | 85 | $4.8\times10^{15}$ | -0.5 |
| | $SO_2$ | 85 | $3.1\times10^{15}$ | -0.5 |
| | $CH_3OCHO$ | 85 | $5.0\times10^{14}$ | -1.0 |
| | $C_2H_5CN$ | 85 | $5.0\times10^{13}$ | -4.0 |
| | t-HCOOH | 85 | $2.0\times10^{14}$ | -0.5 |
| | $^{13}CN$ | 85 | $7.0\times10^{13}$ | -0.5 |
| G043.79−00.12 | $HC_3N$ | 85 | $2.4\times10^{14}$ | 0. |
| | SO | 45 | $2.1\times10^{15}$ | 0. |
| | $HC_3N$, $v_7$=1 | 85 | $2.5\times10^{14}$ | 0. |
| | OCS | 45 | $9.1\times10^{14}$ | -0.5 |
| | HNCO | 45 | $4.0\times10^{13}$ | -1.0 |
| | $C^{18}O$ | 85 | $2.3\times10^{17}$ | 0. |
| | $C^{15}N$ | 45 | $3.5\times10^{13}$ | -1.0 |
| | $^{13}CO$ | 85 | $4.4\times10^{18}$ | 0. |
| | $CH_3CN$ | 45 | $8.0\times10^{13}$ | -1.0 |
| | $CH_3OCH_3$ | 45 | $8.0\times10^{14}$ | -1.0 |
| | $CH_3CHO$ | 45 | $1.5\times10^{14}$ | -0.5 |
| | $C^{17}O$ | 45 | $4.5\times10^{16}$ | 0. |
| | CN | 45 | $4.0\times10^{15}$ | 0. |
| | $SO_2$, $v_2$=1 | 85 | $2.1\times10^{18}$ | 4.0 |
| | $NH_2CHO$ | 45 | $2.5\times10^{14}$ | 3.0 |
| | $CH_3SH$ | 45 | $1.5\times10^{15}$ | 4.0 |
| | $CH_3COCH_3$ | 45 | $2.2\times10^{15}$ | 3.0 |
| | CCS | 45 | $1.0\times10^{13}$ | 5.5 |
| | $HC_5N$ | 85 | $5.0\times10^{13}$ | 5.0 |
| | $C_2H_3CN$ | 45 | $4.0\times10^{13}$ | 5.0 |
| | $C_2H_5OH$ | 45 | $2.5\times10^{15}$ | 4.0 |
| | $CH_3OH$ | 45 | $1.8\times10^{16}$ | 4.0 |
| | $C_2H_5CN$ | 45 | $3.5\times10^{14}$ | 4.0 |
| | $SO_2$ | 45 | $4.1\times10^{18}$ | 4.0 |
| | $^{13}CH_3CN$ | 45 | $2.5\times10^{13}$ | 4.0 |
| | $^{13}C^{17}O$ | 45 | $3.5\times10^{15}$ | 4.0 |
| | $CH_3OCHO$ | 45 | $5.3\times10^{15}$ | 4.0 |
| | t-HCOOH | 45 | $1.4\times10^{15}$ | 4.0 |
| G049.48−00.36 | $^{13}CN$ | 45 | $3.7\times10^{13}$ | 4.0 |
| | $HC_3N$ | 45 | $9.4\times10^{14}$ | 4.5 |
| | SO | 45 | $7.7\times10^{15}$ | 5.0 |
| | $HC_3N$, $v_7$=1 | 45 | $4.3\times10^{16}$ | 4.5 |
| | OCS | 45 | $3.5\times10^{15}$ | 4.0 |
| | HNCO | 45 | $5.0\times10^{14}$ | 4.0 |
| | $CH_3OCH_3$ | 45 | $4.0\times10^{15}$ | 2.0 |
| | $C^{18}O$ | 85 | $2.7\times10^{17}$ | 5.0 |
| | $C^{15}N$ | 45 | $2.0\times10^{13}$ | 6.0 |
| | $^{13}CO$ | 85 | $8.5\times10^{18}$ | 4.0 |
| | $CH_3{}^{13}CN$ | 45 | $8.0\times10^{13}$ | 4.0 |
| | $CH_3CN$ | 45 | $4.1\times10^{14}$ | 4.0 |
| | $CH_3CN$, $v_8$=1 | 45 | $4.0\times10^{18}$ | 4.0 |
| | $CH_3COOH$, vt=0 | 45 | $7.0\times10^{16}$ | 3.0 |
| | $CH_3CHO$ | 45 | $3.5\times10^{14}$ | 3.0 |
| | $C^{17}O$ | 45 | $5.5\times10^{16}$ | 5.5 |
| | CN | 45 | $1.3\times10^{16}$ | 4.0 |
| | $SO_2$, $v_2$=1 | 85 | $2.3\times10^{18}$ | 0. |
| | $NH_2CHO$ | 45 | $7.8\times10^{14}$ | -1.0 |
| | $CH_3OCHO$ | 45 | $2.0\times10^{16}$ | -2.0 |
| | $CH_3COCH_3$ | 45 | $2.4\times10^{14}$ | -1.0 |
| | CCS | 45 | $5.5\times10^{13}$ | -1.5 |
| | $HC_5N$ | 45 | $1.3\times10^{13}$ | -0.5 |
| | $C_2H_3CN$ | 45 | $1.0\times10^{14}$ | 0.5 |
| | $C_2H_5OH$ | 45 | $4.5\times10^{15}$ | -1.0 |
| | $^{34}SO$ | 45 | $9.0\times10^{14}$ | -1.0 |
| | $CH_3OCH_3$ | 45 | $4.3\times10^{16}$ | -2.0 |
| | $OC^{34}S$ | 45 | $1.8\times10^{15}$ | -1.0 |
| | aGg'−$(CH_2OH)_2$ | 45 | $1.5\times10^{14}$ | -2.0 |
| | $HOCO^+$ | 45 | $4.5\times10^{12}$ | 0. |
| | $CH_3OH$ | 45 | $9.5\times10^{16}$ | -1.5 |
| | $C_2H_5CN$ | 45 | $5.0\times10^{14}$ | 0. |
| | $SO_2$ | 45 | $2.5\times10^{18}$ | 0. |
| | $^{13}CH_3CN$ | 45 | $2.0\times10^{13}$ | 0. |
| G049.48−00.38 | $OC^{33}S$ | 45 | $5.0\times10^{13}$ | -1.0 |
| | t-HCOOH | 45 | $1.2\times10^{15}$ | -1.0 |
| | $^{13}CN$ | 45 | $2.5\times10^{14}$ | -1.0 |
| | SiS | 45 | $2.7\times10^{13}$ | 0. |
| | $O^{13}CS$ | 45 | $3.0\times10^{14}$ | -2.0 |
| | $HC_3N$ | 45 | $2.8\times10^{15}$ | -1.8 |
| | SO | 45 | $2.3\times10^{16}$ | -1.0 |
| | $HC_3N$, $v_7$=1 | 85 | $1.0\times10^{17}$ | 2.0 |
| | OCS | 45 | $1.6\times10^{16}$ | -1.5 |

**Table A1.** (Continued)

| Source (1) | Species (2) | Rotational Temperature (K) (3) | Column Density ($cm^{-2}$) (4) | Velocity offset (km $s^{-1}$) (5) |
|---|---|---|---|---|
| | HNCO | 45 | $5.2\times10^{14}$ | -1.0 |
| | $C^{15}N$ | 45 | $7.5\times10^{12}$ | 0. |
| | $^{13}CO$ | 85 | $3.7\times10^{17}$ | -1.5 |
| | $CH_3CN$ | 45 | $1.7\times10^{14}$ | -1.0 |
| | $CH_3OCH_3$ | 45 | $1.0\times10^{14}$ | -1.0 |
| | $CH_3CHO$ | 45 | $3.6\times10^{14}$ | -1.0 |
| | $C^{17}O$ | 45 | $2.5\times10^{16}$ | 0. |
| | CN | 85 | $4.0\times10^{15}$ | -3.0 |
| | $NH_2CHO$ | 45 | $2.6\times10^{13}$ | 2.0 |
| | CCS | 45 | $4.5\times10^{13}$ | 1.0 |
| | $HC_5N$ | 45 | $5.0\times10^{13}$ | 2.0 |
| | $CH_3SH$ | 45 | $1.0\times10^{15}$ | 3.0 |
| | $C_2H_3CN$ | 45 | $4.5\times10^{13}$ | 1.0 |
| | $^{13}C^{17}O$ | 45 | $3.1\times10^{15}$ | 1.0 |
| | $CH_3C_3N$ | 45 | $2.0\times10^{13}$ | 1.0 |
| | $^{13}CN$ | 45 | $1.0\times10^{14}$ | 2.0 |
| | $CH_3OH$ | 85 | $4.3\times10^{16}$ | 2.0 |
| | $HC_3N$ | 85 | $1.1\times10^{15}$ | 1.5 |
| G012.80−00.20 | SO | 45 | $2.6\times10^{15}$ | 2.0 |
| | OCS | 45 | $1.6\times10^{15}$ | 2.0 |
| | $C^{18}O$ | 85 | $8.6\times10^{17}$ | 1.5 |
| | HNCO | 45 | $3.2\times10^{14}$ | 2.0 |
| | $^{13}CO$ | 85 | $1.0\times10^{19}$ | 1.5 |
| | $CH_3CN$ | 45 | $1.2\times10^{14}$ | 1.5 |
| | t-HCOOH | 45 | $1.5\times10^{14}$ | 1.0 |
| | $CH_3OCH_3$ | 45 | $1.0\times10^{15}$ | 2.0 |
| | $CH_3CHO$ | 85 | $1.5\times10^{15}$ | 1.5 |
| | $C^{17}O$ | 45 | $1.6\times10^{17}$ | 1.0 |
| | CN | 85 | $6.0\times10^{15}$ | 2.0 |
| | $NH_2CHO$ | 45 | $3.6\times10^{13}$ | 1.0 |
| | CCS | 45 | $2.2\times10^{13}$ | 2.0 |
| | $HC_5N$ | 45 | $2.0\times10^{13}$ | 2.0 |
| | $C_2H_3CN$ | 45 | $4.5\times10^{13}$ | 2.0 |
| | $C_2H_5OH$ | 45 | $5.0\times10^{14}$ | 2.0 |
| | $^{34}SO$ | 45 | $5.5\times10^{13}$ | 2.0 |
| | $CH_3OCH_3$ | 45 | $4.0\times10^{15}$ | 2.0 |
| | $OC^{34}S$ | 45 | $2.3\times10^{14}$ | 2.5 |
| | $CH_3OH$ | 85 | $1.3\times10^{16}$ | 2.0 |
| | $C_2H_5CN$ | 45 | $1.0\times10^{14}$ | 2.5 |
| | $^{13}CH_3CN$ | 45 | $1.0\times10^{13}$ | 2.0 |
| | $^{13}C^{17}O$ | 45 | $4.5\times10^{15}$ | 2.0 |
| | $CH_3OCHO$ | 45 | $1.5\times10^{15}$ | 2.0 |
| | $SO_2$ | 45 | $2.2\times10^{15}$ | 2.0 |
| G012.88+00.48 | t-HCOOH | 85 | $3.2\times10^{14}$ | 1.0 |
| | $^{13}CN$ | 45 | $1.0\times10^{14}$ | 2.0 |
| | $O^{13}CS$ | 85 | $7.5\times10^{13}$ | 2.0 |
| | $HC_3N$ | 85 | $3.2\times10^{14}$ | 2.0 |
| | SO | 45 | $1.8\times10^{15}$ | 2.0 |
| | $HC_3N$, $v_7$=1 | 85 | $4.0\times10^{14}$ | 3.0 |
| | OCS | 45 | $1.7\times10^{15}$ | 2.0 |
| | HNCO | 45 | $7.0\times10^{13}$ | 2.0 |
| | $C^{18}O$ | 85 | $4.7\times10^{17}$ | 2.5 |
| | $C^{15}N$ | 45 | $7.5\times10^{12}$ | 2.0 |
| | $^{13}CO$ | 85 | $2.1\times10^{18}$ | 3.0 |
| | $CH_3CN$ | 45 | $1.7\times10^{14}$ | 2.0 |
| | $CH_3CHO$ | 45 | $1.5\times10^{14}$ | 2.0 |
| | $C^{17}O$ | 45 | $9.0\times10^{16}$ | 2.5 |
| | CN | 85 | $3.0\times10^{15}$ | 3.5 |
| | $CH_3OH$ | 85 | $7.5\times10^{15}$ | 1.0 |
| | $HC_3N$ | 85 | $4.5\times10^{13}$ | 0.5 |
| | SO | 45 | $1.7\times10^{14}$ | 0.5 |
| | OCS | 45 | $1.5\times10^{14}$ | 1.5 |
| G012.90−00.24 | $C^{18}O$ | 85 | $3.4\times10^{17}$ | 0.5 |
| | HNCO | 45 | $5.0\times10^{13}$ | -1.5 |
| | $^{13}CO$ | 85 | $1.9\times10^{18}$ | 0. |
| | $CH_3CN$ | 45 | $1.7\times10^{13}$ | 0. |
| | $C^{17}O$ | 45 | $5.0\times10^{16}$ | 0. |
| | CN | 85 | $1.2\times10^{15}$ | 1.5 |
| | $NH_2CHO$ | 45 | $3.6\times10^{13}$ | -0.5 |
| | CCS | 45 | $2.0\times10^{13}$ | -2.0 |
| | $^{34}SO$ | 45 | $5.5\times10^{13}$ | -2.0 |
| | $CH_3OCH_3$ | 45 | $4.0\times10^{13}$ | -2.0 |
| | $OC^{34}S$ | 45 | $1.3\times10^{14}$ | -1.0 |
| | $CH_3OH$ | 85 | $2.0\times10^{16}$ | -0.5 |
| | $C_2H_5CN$ | 85 | $7.0\times10^{13}$ | -1.0 |
| | $CH_3OCHO$ | 85 | $3.0\times10^{15}$ | -1.0 |
| | $SO_2$ | 85 | $2.3\times10^{15}$ | -1.0 |
| | $^{13}CN$ | 85 | $2.2\times10^{14}$ | -1.0 |
| G012.90−00.26 | $HC_3N$ | 85 | $5.0\times10^{14}$ | -2.0 |
| | SO | 45 | $1.3\times10^{15}$ | -1.5 |
| | $HC_3N$, $v_7$=1 | 85 | $4.7\times10^{14}$ | -1.5 |
| | OCS | 45 | $1.5\times10^{15}$ | -1.0 |
| | HNCO | 45 | $7.0\times10^{13}$ | -0.5 |
| | $C^{18}O$ | 85 | $4.2\times10^{17}$ | -3.0 |
| | $^{13}CO$ | 45 | $7.0\times10^{13}$ | -3.0 |
| | $CH_3CN$ | 85 | $3.0\times10^{18}$ | -1.0 |
| | $CH_3CHO$ | 85 | $7.0\times10^{14}$ | -2.0 |
| | $C^{17}O$ | 45 | $6.5\times10^{16}$ | -3.0 |
| | HNCO | 45 | $1.2\times10^{15}$ | -1.0 |
| | $C^{18}O$ | 85 | $6.2\times10^{17}$ | -1.0 |
| | $^{13}CO$ | 85 | $1.9\times10^{19}$ | -1.0 |
| | $CH_3{}^{13}CN$ | 45 | $1.0\times10^{14}$ | -2.0 |
| | $CH_3CN$ | 45 | $1.2\times10^{15}$ | -2.0 |
| | $CH_3CN$, $v_8$=1 | 45 | $5.0\times10^{18}$ | 0. |
| | $CH_3COOH$, vt=0 | 45 | $1.3\times10^{17}$ | 0. |
| | $CH_3CHO$ | 45 | $2.3\times10^{14}$ | 0. |
| | $C^{17}O$ | 45 | $1.2\times10^{17}$ | -1.5 |
| | CN | 45 | $1.7\times10^{16}$ | -3.0 |
| | CCS | 45 | $1.6\times10^{13}$ | -2.5 |
| | $HC_5N$ | 45 | $7.1\times10^{12}$ | -2.5 |
| | $CH_3OH$ | 85 | $1.7\times10^{15}$ | -4.0 |
| | t-HCOOH | 85 | $2.2\times10^{14}$ | -3.0 |
| | $^{13}CN$ | 45 | $3.0\times10^{13}$ | -3.0 |
| | $HC_3N$ | 85 | $2.0\times10^{14}$ | -2.5 |
| | SO | 45 | $1.4\times10^{15}$ | -2.0 |
| G059.78+00.06 | OCS | 45 | $2.8\times10^{14}$ | -2.0 |
| | $C^{15}N$ | 45 | $5.3\times10^{13}$ | -1.5 |
| | $C^{18}O$ | 85 | $6.6\times10^{16}$ | -2.2 |
| | HNCO | 45 | $7.0\times10^{13}$ | -1.7 |
| | $^{13}CO$ | 85 | $2.7\times10^{18}$ | -1.2 |
| | $CH_3CN$ | 45 | $2.0\times10^{13}$ | -2.7 |
| | $CH_3CHO$ | 45 | $5.0\times10^{13}$ | -3.0 |
| | $C^{17}O$ | 45 | $9.0\times10^{15}$ | -2.0 |
| | CN | 45 | $4.8\times10^{15}$ | -2.5 |
| | CCS | 45 | $1.5\times10^{13}$ | -0.5 |
| | $HC_5N$ | 45 | $1.0\times10^{13}$ | -0.2 |
| | $CH_3OH$ | 45 | $2.0\times10^{15}$ | -0.5 |
| | $CH_3OCHO$ | 45 | $2.0\times10^{14}$ | 1.5 |
| | $SO_2$ | 45 | $6.0\times10^{14}$ | -2.5 |
| | t-HCOOH | 85 | $2.0\times10^{14}$ | -1.0 |
| | $^{13}CN$ | 85 | $2.5\times10^{14}$ | -1.3 |
| | $HC_3N$ | 85 | $2.7\times10^{14}$ | -0.5 |
| | SO | 45 | $1.5\times10^{15}$ | -1.0 |
| G069.54−00.97 | OCS | 45 | $7.0\times10^{14}$ | -0.7 |
| | $C^{18}O$ | 85 | $2.0\times10^{17}$ | -1.0 |
| | HNCO | 45 | $1.0\times10^{14}$ | -1.0 |
| | $C^{15}N$ | 45 | $1.0\times10^{13}$ | -1.0 |
| | $^{13}CO$ | 85 | $3.5\times10^{18}$ | -0.5 |
| | $CH_3CN$ | 45 | $6.7\times10^{13}$ | -0.3 |
| | $CH_3OCH_3$ | 45 | $1.0\times10^{14}$ | -1.0 |
| | $CH_3CHO$ | 45 | $1.7\times10^{14}$ | -0.5 |
| | $C^{17}O$ | 45 | $3.5\times10^{16}$ | -1.0 |
| | CN | 45 | $5.4\times10^{15}$ | -0.5 |
| | CCS | 45 | $1.7\times10^{13}$ | 7.5 |
| | $HC_5N$ | 45 | $1.2\times10^{13}$ | 6.8 |
| | $C_2H_5OH$ | 45 | $4.2\times10^{14}$ | 4.7 |
| | $CH_3OH$ | 45 | $1.1\times10^{15}$ | 6.5 |
| | t-HCOOH | 85 | $1.5\times10^{14}$ | 7.0 |
| | $^{13}CN$ | 85 | $1.3\times10^{14}$ | 7.0 |
| | $HC_3N$ | 85 | $3.1\times10^{14}$ | 7.0 |
| | SO | 45 | $1.1\times10^{15}$ | 7.5 |
| G075.76+00.33 | OCS | 45 | $3.1\times10^{14}$ | 7.3 |
| | $C^{18}O$ | 85 | $8.2\times10^{16}$ | 7.3 |
| | HNCO | 45 | $8.5\times10^{13}$ | 7.0 |
| | $C^{15}N$ | 45 | $4.0\times10^{13}$ | 7.0 |
| | $^{13}CO$ | 85 | $2.1\times10^{18}$ | 7.0 |
| | $CH_3CN$ | 45 | $5.0\times10^{13}$ | 7.0 |
| | $CH_3CHO$ | 45 | $2.7\times10^{14}$ | 7.3 |
| | $C^{17}O$ | 45 | $1.5\times10^{16}$ | 7.3 |
| | CN | 45 | $4.5\times10^{15}$ | 7.3 |
| | $NH_2CHO$ | 45 | $5.0\times10^{13}$ | 3.0 |
| | CCS | 45 | $1.3\times10^{13}$ | 0. |
| | $CH_3OH$ | 45 | $3.0\times10^{15}$ | 0. |
| | $^{13}CN$ | 45 | $1.0\times10^{14}$ | 0. |
| | $HC_3N$ | 85 | $2.9\times10^{14}$ | 0. |
| | SO | 45 | $5.2\times10^{14}$ | 0. |
| | $HC_3N$, $v_7$=1 | 85 | $2.5\times10^{14}$ | 1.0 |
| G078.12+03.63 | OCS | 45 | $4.3\times10^{14}$ | 0. |
| | HNCO | 45 | $6.5\times10^{13}$ | 0. |
| | $C^{18}O$ | 85 | $6.0\times10^{16}$ | 0.8 |
| | $C^{15}N$ | 45 | $2.5\times10^{13}$ | 1.0 |
| | $^{13}CO$ | 85 | $2.2\times10^{18}$ | 0. |
| | $CH_3CN$ | 45 | $6.0\times10^{13}$ | 0. |
| | $C^{17}O$ | 45 | $7.0\times10^{15}$ | 1.0 |
| | CN | 45 | $6.5\times10^{15}$ | 0.5 |
| | CCS | 45 | $2.3\times10^{13}$ | -1.0 |
| | $HC_5N$ | 45 | $1.5\times10^{13}$ | -1.0 |
| | $CH_3OH$ | 45 | $4.0\times10^{14}$ | -3.0 |
| | t-HCOOH | 85 | $2.0\times10^{14}$ | -1.0 |
| | $^{13}CN$ | 85 | $3.0\times10^{14}$ | -1.0 |
| | $HC_3N$ | 85 | $4.1\times10^{14}$ | -1.0 |
| | SO | 45 | $1.4\times10^{15}$ | -1.0 |
| G081.75+00.59 | OCS | 45 | $2.8\times10^{14}$ | -1.0 |
| | $C^{18}O$ | 85 | $1.9\times10^{17}$ | -1.0 |
| | HNCO | 45 | $1.3\times10^{14}$ | -1.0 |
| | $C^{15}N$ | 45 | $4.5\times10^{13}$ | -1.0 |

**Table A1.** (Continued)

| Source | Species | Rotational Temperature (K) | Column Density ($cm^{-2}$) | Velocity offset ($km\ s^{-1}$) |
|---|---|---|---|---|
| (1) | (2) | (3) | (4) | (5) |
| | CN | 45 | $2.0\times10^{15}$ | -1.5 |
| | $NH_2CHO$ | 45 | $5.0\times10^{13}$ | -1.0 |
| | CCS | 45 | $1.8\times10^{13}$ | 0. |
| | $HC_5N$ | 85 | $6.4\times10^{12}$ | 0. |
| | $CH_3OCH_3$ | 45 | $2.5\times10^{15}$ | 0. |
| | $OC^{34}S$ | 85 | $1.6\times10^{14}$ | 0. |
| | $CH_3OH$ | 85 | $8.0\times10^{15}$ | 0.5 |
| | $CH_3OCHO$ | 85 | $2.0\times10^{15}$ | 0. |
| | t-HCOOH | 85 | $5.0\times10^{14}$ | -0.5 |
| | $^{13}CN$ | 85 | $1.0\times10^{14}$ | -0.5 |
| G014.33−00.64 | $HC_3N$ | 85 | $7.0\times10^{14}$ | 0. |
| | SO | 45 | $3.2\times10^{15}$ | 0.5 |
| | OCS | 85 | $2.2\times10^{15}$ | 0.5 |
| | $C^{18}O$ | 85 | $1.1\times10^{17}$ | 0.5 |
| | HNCO | 45 | $2.0\times10^{14}$ | 0.3 |
| | $C^{15}N$ | 45 | $5.0\times10^{13}$ | 0. |
| | $^{13}CO$ | 85 | $1.0\times10^{18}$ | 0.5 |
| | $CH_3CN$ | 45 | $1.3\times10^{14}$ | 0. |
| | $CH_3CHO$ | 45 | $5.0\times10^{14}$ | 0. |
| | $C^{17}O$ | 45 | $2.0\times10^{16}$ | 1.0 |
| | CN | 45 | $2.5\times10^{15}$ | 0.5 |
| | CCS | 45 | $1.1\times10^{13}$ | -2.0 |
| | $HC_5N$ | 85 | $6.4\times10^{12}$ | -3.0 |
| | $CH_3OH$ | 85 | $5.0\times10^{15}$ | -2.0 |
| | $^{13}CN$ | 85 | $1.0\times10^{14}$ | -3.0 |
| | $HC_3N$ | 85 | $4.0\times10^{14}$ | -3.0 |
| | SO | 45 | $3.8\times10^{14}$ | -2.5 |
| G015.03−00.67 | OCS | 45 | $1.5\times10^{14}$ | -2.0 |
| | $C^{18}O$ | 85 | $6.0\times10^{16}$ | -2.5 |
| | HNCO | 45 | $2.5\times10^{13}$ | -2.0 |
| | $C^{15}N$ | 45 | $2.5\times10^{13}$ | -2.0 |
| | $^{13}CO$ | 85 | $1.6\times10^{18}$ | -2.5 |
| | $CH_3CN$ | 45 | $5.0\times10^{13}$ | -2.0 |
| | $C^{17}O$ | 45 | $1.2\times10^{16}$ | -2.0 |
| | CN | 45 | $6.8\times10^{15}$ | -2.5 |
| | CCS | 45 | $1.3\times10^{13}$ | -1.0 |
| | $OC^{34}S$ | 85 | $1.0\times10^{14}$ | 0. |
| | $CH_3OH$ | 85 | $5.7\times10^{15}$ | -0.5 |
| | $^{13}C^{17}O$ | 85 | $5.5\times10^{15}$ | 0. |
| | $C_2H_5CN$ | 45 | $1.0\times10^{13}$ | 0. |
| | $^{13}CN$ | 85 | $1.2\times10^{14}$ | 0. |
| | $O^{13}CS$ | 85 | $3.0\times10^{13}$ | 1.0 |
| | $HC_3N$ | 85 | $2.5\times10^{14}$ | 0. |
| | SO | 45 | $7.1\times10^{14}$ | -0.5 |
| G016.58−00.05 | OCS | 45 | $8.0\times10^{14}$ | -0.5 |
| | $C^{18}O$ | 85 | $3.4\times10^{17}$ | -1.0 |
| | HNCO | 45 | $1.5\times10^{14}$ | -0.5 |
| | $CH_3CN$ | 45 | $8.0\times10^{13}$ | -0.5 |
| | $CH_3OCHO$ | 45 | $3.3\times10^{14}$ | -0.5 |
| | $CH_3OCH_3$ | 45 | $9.0\times10^{14}$ | -0.5 |
| | $CH_3CHO$ | 45 | $2.5\times10^{14}$ | -0.5 |
| | $C^{17}O$ | 45 | $6.2\times10^{16}$ | -0.5 |
| | CN | 45 | $2.5\times10^{15}$ | -0.5 |
| | $NH_2CHO$ | 45 | $4.5\times10^{13}$ | -3.0 |
| | CCS | 45 | $1.2\times10^{13}$ | -3.0 |
| | $HC_5N$ | 45 | $1.5\times10^{13}$ | -3.0 |
| | $CH_3OH$ | 85 | $1.8\times10^{16}$ | -3.5 |
| | $C_2H_5CN$ | 85 | $7.0\times10^{13}$ | -1.0 |
| | $^{13}CN$ | 85 | $2.0\times10^{14}$ | -2.0 |
| | $HC_3N$ | 85 | $2.2\times10^{14}$ | -3.0 |
| | SO | 45 | $7.5\times10^{14}$ | -3.0 |
| | $HC_3N$, $v_7$=1 | 85 | $5.0\times10^{14}$ | 0. |
| G023.00−00.41 | OCS | 45 | $1.7\times10^{15}$ | -2.0 |
| | HNCO | 45 | $1.0\times10^{14}$ | -2.5 |
| | $C^{18}O$ | 85 | $1.7\times10^{17}$ | -3.5 |
| | $^{13}CO$ | 85 | $3.2\times10^{18}$ | -6.0 |
| | $CH_3CN$ | 45 | $8.0\times10^{13}$ | -2.5 |
| | $CH_3OCHO$ | 45 | $1.0\times10^{14}$ | -2.0 |
| | $C_2H_3CN$ | 45 | $3.0\times10^{13}$ | -2.1 |
| | $CH_3OCH_3$ | 85 | $2.0\times10^{15}$ | -3.0 |
| | $CH_3CHO$ | 85 | $3.0\times10^{14}$ | -3.0 |
| | $C^{17}O$ | 45 | $4.2\times10^{16}$ | -4.0 |
| | CN | 45 | $3.0\times10^{15}$ | -3.0 |
| | $NH_2CHO$ | 45 | $4.0\times10^{13}$ | 4.5 |
| | CCS | 45 | $1.5\times10^{13}$ | 4.5 |
| | $OC^{34}S$ | 45 | $1.0\times10^{14}$ | 5.0 |
| | $CH_3OH$ | 85 | $2.5\times10^{15}$ | 5.5 |
| | $^{13}C^{17}O$ | 85 | $4.0\times10^{15}$ | 4.5 |
| | $CH_3OCHO$ | 45 | $3.0\times10^{14}$ | 4.5 |
| | t-HCOOH | 85 | $2.4\times10^{14}$ | 4.0 |
| | $^{13}CN$ | 85 | $2.0\times10^{14}$ | 4.0 |
| | $HC_3N$ | 85 | $3.0\times10^{14}$ | 4.5 |
| G023.44−00.18 | SO | 45 | $8.2\times10^{14}$ | 4.5 |
| | OCS | 45 | $1.3\times10^{15}$ | 4.0 |
| | $C^{18}O$ | 85 | $3.0\times10^{17}$ | 4.5 |
| | HNCO | 45 | $5.3\times10^{14}$ | 4.5 |
| | $^{13}CO$ | 85 | $3.3\times10^{18}$ | 4.5 |
| | $CH_3CN$ | 45 | $1.5\times10^{14}$ | 4.5 |
| | $^{13}CO$ | 85 | $3.3\times10^{18}$ | -1.0 |
| | $CH_3CN$ | 45 | $4.0\times10^{13}$ | -1.0 |
| | $CH_3CHO$ | 45 | $2.5\times10^{14}$ | -1.0 |
| | $C^{17}O$ | 45 | $3.3\times10^{16}$ | -1.0 |
| | CN | 45 | $5.5\times10^{15}$ | -1.0 |
| | $NH_2CHO$ | 45 | $3.0\times10^{13}$ | 2.5 |
| | CCS | 45 | $1.4\times10^{13}$ | 2.5 |
| | $C_2H_5OH$ | 45 | $3.0\times10^{14}$ | 2.0 |
| | $^{34}SO$ | 45 | $2.2\times10^{14}$ | 2.5 |
| | $CH_3OCH_3$ | 45 | $3.0\times10^{15}$ | 2.0 |
| | $OC^{34}S$ | 45 | $1.0\times10^{14}$ | 2.0 |
| | $HOCO^+$ | 45 | $5.0\times10^{12}$ | 2.0 |
| | $CH_3OH$ | 85 | $2.5\times10^{16}$ | 2.0 |
| | $SO_2$ | 85 | $1.0\times10^{16}$ | 2.0 |
| | $C_2H_5CN$ | 45 | $4.5\times10^{13}$ | 2.0 |
| | $CH_3OCHO$ | 45 | $1.5\times10^{15}$ | 2.0 |
| | t-HCOOH | 85 | $4.6\times10^{14}$ | 2.5 |
| G081.87+00.78 | $^{13}CN$ | 85 | $1.0\times10^{14}$ | 2.5 |
| | $HC_3N$ | 85 | $5.5\times10^{14}$ | 2.5 |
| | SO | 45 | $7.5\times10^{15}$ | 2.5 |
| | $HC_3N$, $v_7$=1 | 85 | $5.0\times10^{14}$ | 2.0 |
| | OCS | 45 | $2.0\times10^{15}$ | 2.5 |
| | HNCO | 45 | $1.5\times10^{14}$ | 2.5 |
| | $C^{15}N$ | 45 | $3.5\times10^{13}$ | 2.5 |
| | $^{13}CO$ | 85 | $6.2\times10^{18}$ | 2.5 |
| | $C^{18}O$ | 85 | $2.5\times10^{17}$ | 2.5 |
| | $CH_3CN$ | 45 | $2.2\times10^{14}$ | 2.5 |
| | $CH_3CHO$ | 45 | $3.8\times10^{14}$ | 2.5 |
| | $C^{17}O$ | 45 | $3.8\times10^{16}$ | 2.5 |
| | CN | 45 | $6.5\times10^{15}$ | 2.5 |
| | CCS | 45 | $1.2\times10^{13}$ | -1.0 |
| | $^{34}SO$ | 45 | $2.0\times10^{13}$ | -2.0 |
| | $CH_3OH$ | 85 | $5.0\times10^{15}$ | -1.5 |
| | t-HCOOH | 85 | $1.8\times10^{14}$ | -1.0 |
| | $^{13}CN$ | 45 | $5.0\times10^{13}$ | -1.0 |
| | $HC_3N$ | 85 | $3.5\times10^{14}$ | -1.0 |
| | SO | 45 | $1.3\times10^{15}$ | -1.0 |
| | OCS | 45 | $5.4\times10^{14}$ | -1.0 |
| G092.67+03.07 | $C^{18}O$ | 85 | $6.0\times10^{16}$ | -1.0 |
| | HNCO | 45 | $6.7\times10^{13}$ | -1.0 |
| | $C^{15}N$ | 45 | $1.5\times10^{13}$ | -1.0 |
| | $^{13}CO$ | 85 | $2.5\times10^{18}$ | -1.0 |
| | $CH_3CN$ | 45 | $7.2\times10^{13}$ | -1.0 |
| | $CH_3OCH_3$ | 45 | $7.5\times10^{13}$ | -1.0 |
| | $CH_3CHO$ | 45 | $2.0\times10^{14}$ | -1.0 |
| | $C^{17}O$ | 45 | $1.3\times10^{16}$ | -1.0 |
| | CN | 45 | $3.5\times10^{15}$ | -1.0 |
| | $HC_5N$ | 45 | $1.2\times10^{13}$ | -3.5 |
| | $^{34}SO$ | 45 | $8.5\times10^{13}$ | -4.0 |
| | $CH_3C^{15}N$ | 45 | $7.5\times10^{14}$ | -3.5 |
| | $CH_3OH$ | 85 | $1.3\times10^{15}$ | -4.0 |
| | $SO_2$ | 85 | $1.1\times10^{16}$ | -2.0 |
| | t-HCOOH | 85 | $2.5\times10^{14}$ | -4.0 |
| | $^{13}CN$ | 45 | $1.7\times10^{14}$ | -4.0 |
| | $HC_3N$ | 85 | $3.6\times10^{14}$ | -4.0 |
| G109.87+02.11 | SO | 45 | $3.3\times10^{15}$ | -4.0 |
| | $HC_3N$, $v_7$=1 | 85 | $2.5\times10^{14}$ | -4.0 |
| | OCS | 45 | $3.1\times10^{14}$ | -4.0 |
| | HNCO | 45 | $2.3\times10^{13}$ | -3.0 |
| | $C^{18}O$ | 85 | $2.8\times10^{17}$ | -4.0 |
| | $C^{15}N$ | 45 | $7.0\times10^{13}$ | -3.0 |
| | $^{13}CO$ | 85 | $5.1\times10^{18}$ | -4.0 |
| | $CH_3CN$ | 45 | $6.0\times10^{13}$ | -4.0 |
| | $CH_3CHO$ | 45 | $1.0\times10^{14}$ | -4.0 |
| | $C^{17}O$ | 45 | $4.1\times10^{16}$ | -4.0 |
| | CN | 45 | $5.5\times10^{15}$ | -4.0 |
| | $NH_2CHO$ | 45 | $1.0\times10^{13}$ | -1.0 |
| | CCS | 45 | $1.2\times10^{13}$ | 0. |
| | $C_2H_5OH$ | 45 | $4.0\times10^{14}$ | -0.5 |
| | $CH_3OCH_3$ | 45 | $1.5\times10^{15}$ | -1.0 |
| | $CH_3OH$ | 45 | $4.0\times10^{16}$ | -1.0 |
| | $CH_3OCHO$ | 45 | $6.0\times10^{14}$ | -1.5 |
| | $SO_2$ | 45 | $8.0\times10^{14}$ | 5.0 |
| | t-HCOOH | 85 | $2.0\times10^{14}$ | -1.5 |
| | $^{13}CN$ | 45 | $3.5\times10^{13}$ | 0. |
| | $HC_3N$ | 85 | $1.7\times10^{14}$ | 0. |
| G111.54+00.77 | SO | 45 | $1.7\times10^{15}$ | 0. |
| | $HC_3N$, $v_7$=1 | 85 | $2.5\times10^{14}$ | 7.0 |
| | OCS | 45 | $6.0\times10^{14}$ | -0.6 |
| | HNCO | 45 | $1.3\times10^{13}$ | -2.0 |
| | $C^{18}O$ | 85 | $1.4\times10^{17}$ | 0. |
| | $C^{15}N$ | 45 | $1.3\times10^{13}$ | 0. |
| | $^{13}CO$ | 85 | $3.6\times10^{18}$ | 0. |
| | $CH_3CN$ | 45 | $6.0\times10^{13}$ | -1.0 |
| | $CH_3CHO$ | 45 | $1.3\times10^{14}$ | 0. |
| | $C^{17}O$ | 45 | $2.3\times10^{16}$ | 0. |
| | CN | 45 | $3.5\times10^{15}$ | -0.5 |
| | CCS | 45 | $2.0\times10^{13}$ | 5.5 |

**Table A1.** (Continued)

| Source (1) | Species (2) | Rotational Temperature (K) (3) | Column Density ($cm^{-2}$) (4) | Velocity offset (km $s^{-1}$) (5) |
|---|---|---|---|---|
| | $CH_3OCH_3$ | 45 | $1.5\times10^{15}$ | 4.5 |
| | $CH_3CHO$ | 45 | $5.5\times10^{14}$ | 4.5 |
| | $C^{17}O$ | 45 | $6.7\times10^{16}$ | 4.0 |
| | CN | 45 | $3.0\times10^{15}$ | 6.0 |
| | $NH_2CHO$ | 45 | $5.0\times10^{13}$ | 0.5 |
| | CCS | 45 | $1.1\times10^{13}$ | 0. |
| | $C_2H_5CN$ | 45 | $8.0\times10^{13}$ | 1.0 |
| | $HC_5N$ | 45 | $1.5\times10^{13}$ | 0.5 |
| | $C_2H_5OH$ | 45 | $5.0\times10^{14}$ | 1.5 |
| | $CH_3COCH_3$ | 45 | $6.0\times10^{14}$ | 1.0 |
| | $CH_3OCH_3$ | 45 | $6.0\times10^{15}$ | 1.5 |
| | $OC^{34}S$ | 45 | $3.0\times10^{14}$ | 1.5 |
| | $CH_3OH$ | 45 | $7.0\times10^{15}$ | 1.0 |
| | $^{13}CH_3CN$ | 45 | $2.5\times10^{13}$ | 1.0 |
| | $^{13}C^{17}O$ | 45 | $2.5\times10^{15}$ | -1.0 |
| | $CH_3OCHO$ | 45 | $2.0\times10^{15}$ | 0.5 |
| | $OC^{33}S$ | 85 | $1.0\times10^{14}$ | 1.5 |
| | t-HCOOH | 85 | $3.0\times10^{14}$ | 0. |
| G027.36−00.16 | $^{13}CN$ | 85 | $2.0\times10^{14}$ | -1.0 |
| | $O^{13}CS$ | 85 | $1.0\times10^{14}$ | 0.5 |
| | $HC_3N$ | 85 | $4.0\times10^{14}$ | 0. |
| | SO | 45 | $1.2\times10^{15}$ | 0.5 |
| | $HC_3N$, $v_7$=1 | 85 | $2.0\times10^{14}$ | 1.0 |
| | OCS | 45 | $2.2\times10^{15}$ | 1.0 |
| | $C^{18}O$ | 85 | $1.9\times10^{17}$ | -1.0 |
| | HNCO | 45 | $5.3\times10^{14}$ | 1.0 |
| | $^{13}CO$ | 85 | $3.5\times10^{18}$ | -0.5 |
| | $CH_3{}^{13}CN$ | 45 | $2.0\times10^{13}$ | 0.5 |
| | $CH_3CN$ | 45 | $2.0\times10^{14}$ | 0.5 |
| | $C_2H_3CN$ | 45 | $1.0\times10^{14}$ | 1.0 |
| | $CH_3CHO$ | 45 | $6.0\times10^{14}$ | 0.5 |
| | $C^{17}O$ | 45 | $3.3\times10^{16}$ | -0.5 |
| | CN | 45 | $6.0\times10^{15}$ | -0.5 |
| | $NH_2CHO$ | 45 | $1.5\times10^{13}$ | 3.0 |
| | CCS | 45 | $2.3\times10^{13}$ | 3.0 |
| | $HC_5N$ | 45 | $1.0\times10^{13}$ | 3.0 |
| | $CH_3OH$ | 45 | $2.2\times10^{15}$ | 3.5 |
| | $^{13}C^{17}O$ | 45 | $1.5\times10^{15}$ | 3.5 |
| | $C_2H_5CN$ | 45 | $1.0\times10^{13}$ | 3.5 |
| | $SO_2$ | 45 | $1.0\times10^{15}$ | 5.0 |
| | t-HCOOH | 85 | $1.2\times10^{14}$ | 3.0 |
| | $^{13}CN$ | 45 | $1.0\times10^{14}$ | 3.0 |
| | $HC_3N$ | 85 | $2.1\times10^{14}$ | 3.5 |
| G028.86+00.06 | SO | 45 | $1.1\times10^{15}$ | 3.5 |
| | $HC_3N$, $v_7$=1 | 85 | $2.0\times10^{14}$ | 4.0 |
| | OCS | 45 | $1.1\times10^{15}$ | 3.0 |
| | $C^{18}O$ | 85 | $2.0\times10^{17}$ | 3.5 |
| | HNCO | 45 | $1.3\times10^{14}$ | 3.5 |
| | $C^{15}N$ | 45 | $1.3\times10^{13}$ | 3.5 |
| | $^{13}CO$ | 85 | $1.5\times10^{13}$ | 3.5 |
| | $CH_3CN$ | 45 | $8.5\times10^{13}$ | 3.5 |
| | $CH_3OCH_3$ | 45 | $1.2\times10^{14}$ | 3.0 |
| | $CH_3CHO$ | 45 | $1.5\times10^{14}$ | 3.0 |
| | $C^{17}O$ | 45 | $3.3\times10^{16}$ | 3.5 |
| | CN | 45 | $4.0\times10^{15}$ | 4.0 |
| | $NH_2CHO$ | 45 | $7.0\times10^{13}$ | 0. |
| | CCS | 45 | $3.8\times10^{13}$ | -0.5 |
| | $HC_5N$ | 45 | $3.0\times10^{13}$ | -0.5 |
| | $C_2H_3CN$ | 45 | $7.1\times10^{13}$ | 0. |
| | $CH_3OCH_3$ | 45 | $3.0\times10^{15}$ | -3.0 |
| | $OC^{34}S$ | 45 | $3.0\times10^{14}$ | -0.5 |
| | $CH_3OH$ | 45 | $8.3\times10^{15}$ | 0. |
| | $C_2H_5CN$ | 45 | $2.0\times10^{14}$ | -0.5 |
| | t-HCOOH | 85 | $2.0\times10^{14}$ | 0. |
| | $^{13}CN$ | 85 | $1.8\times10^{13}$ | 0. |
| | $HC_3N$ | 85 | $5.5\times10^{14}$ | -0.5 |
| G029.95−00.01 | SO | 45 | $2.0\times10^{15}$ | -0.5 |
| | $HC_3N$, $v_7$=1 | 85 | $1.8\times10^{15}$ | 0. |
| | OCS | 45 | $2.7\times10^{15}$ | 0. |
| | HNCO | 45 | $2.5\times10^{14}$ | -0.5 |
| | $C^{18}O$ | 85 | $3.5\times10^{17}$ | -0.5 |
| | $^{13}CO$ | 85 | $5.8\times10^{18}$ | -0.5 |
| | $CH_3{}^{13}CN$ | 45 | $2.0\times10^{13}$ | -0.5 |
| | $CH_3CN$ | 45 | $2.0\times10^{14}$ | -0.5 |
| | $CH_3OCHO$ | 45 | $5.0\times10^{14}$ | -0.5 |
| | $CH_3CHO$ | 45 | $1.6\times10^{14}$ | -0.5 |
| | $C^{17}O$ | 45 | $5.3\times10^{16}$ | -0.5 |
| | CN | 45 | $8.0\times10^{15}$ | -1.0 |
| | $NH_2CHO$ | 45 | $2.0\times10^{13}$ | 0. |
| | CCS | 45 | $2.1\times10^{13}$ | 0. |
| | $C_2H_3CN$ | 45 | $1.7\times10^{13}$ | 0. |
| | $CH_3OCH_3$ | 45 | $2.0\times10^{15}$ | 0. |
| | $OC^{34}S$ | 45 | $6.2\times10^{13}$ | 0. |
| | $CH_3OH$ | 85 | $1.8\times10^{16}$ | 0. |
| | $^{13}C^{17}O$ | 85 | $3.8\times10^{15}$ | -0.5 |
| | $CH_3OCHO$ | 45 | $1.0\times10^{15}$ | 0. |
| | t-HCOOH | 85 | $2.2\times10^{14}$ | 0. |
| | $^{13}CN$ | 85 | $3.0\times10^{14}$ | 0. |
| | $HC_5N$ | 45 | $1.1\times10^{13}$ | 5.5 |
| | $^{34}SO$ | 45 | $1.9\times10^{13}$ | 5.0 |
| | $CH_3OH$ | 85 | $2.5\times10^{15}$ | 5.5 |
| | $CH_3OCHO$ | 45 | $5.9\times10^{13}$ | 5.0 |
| | t-HCOOH | 85 | $1.0\times10^{14}$ | 5.5 |
| | $^{13}CN$ | 45 | $1.9\times10^{13}$ | 5.0 |
| | $HC_3N$ | 85 | $1.8\times10^{14}$ | 5.5 |
| G121.29+00.65 | SO | 45 | $8.2\times10^{14}$ | 5.7 |
| | OCS | 45 | $3.4\times10^{14}$ | 5.5 |
| | $C^{18}O$ | 85 | $9.0\times10^{16}$ | 5.5 |
| | HNCO | 45 | $1.0\times10^{12}$ | 5.0 |
| | $C^{15}N$ | 45 | $1.5\times10^{13}$ | 5.5 |
| | $^{13}CO$ | 85 | $2.0\times10^{18}$ | 5.5 |
| | $CH_3CN$ | 45 | $3.0\times10^{13}$ | 5.5 |
| | $CH_3CHO$ | 45 | $1.4\times10^{14}$ | 5.0 |
| | $C^{17}O$ | 45 | $1.6\times10^{16}$ | 5.0 |
| | CN | 45 | $3.2\times10^{15}$ | 5.5 |
| | CCS | 45 | $1.4\times10^{13}$ | -0.5 |
| | $HC_5N$ | 45 | $7.0\times10^{12}$ | -1.0 |
| | $^{34}SO$ | 45 | $3.2\times10^{13}$ | -1.0 |
| | $CH_3OH$ | 45 | $2.3\times10^{15}$ | -0.4 |
| | $CH_3OCHO$ | 45 | $1.8\times10^{14}$ | -0.4 |
| | t-HCOOH | 85 | $1.2\times10^{14}$ | 0. |
| | $^{13}CN$ | 85 | $2.5\times10^{13}$ | -0.5 |
| | $HC_3N$ | 85 | $2.6\times10^{14}$ | -0.7 |
| | SO | 45 | $1.4\times10^{15}$ | -0.5 |
| G123.06−06.30 | OCS | 45 | $5.6\times10^{14}$ | -0.5 |
| | HNCO | 45 | $2.0\times10^{13}$ | -1.0 |
| | $C^{18}O$ | 85 | $6.8\times10^{16}$ | 0. |
| | $C^{15}N$ | 45 | $1.3\times10^{13}$ | -0.5 |
| | $^{13}CO$ | 85 | $2.5\times10^{18}$ | 0. |
| | $CH_3CN$ | 45 | $6.3\times10^{13}$ | -0.5 |
| | $CH_3OCH_3$ | 45 | $2.0\times10^{14}$ | -0.5 |
| | $CH_3CHO$ | 45 | $3.0\times10^{14}$ | -0.5 |
| | $C^{17}O$ | 45 | $1.1\times10^{16}$ | 0. |
| | CN | 45 | $3.7\times10^{15}$ | -0.5 |
| | CCS | 45 | $1.7\times10^{13}$ | 0. |
| | $CH_3OCH_3$ | 45 | $3.3\times10^{15}$ | -0.5 |
| | $OC^{34}S$ | 45 | $5.4\times10^{14}$ | -0.3 |
| | $HOCO^+$ | 45 | $4.0\times10^{12}$ | 0. |
| | $CH_3OH$ | 85 | $3.5\times10^{16}$ | 0.5 |
| | $C_2H_5CN$ | 45 | $1.0\times10^{14}$ | 0. |
| | $CH_3OCHO$ | 45 | $1.5\times10^{15}$ | 0. |
| | $SO_2$ | 45 | $4.5\times10^{15}$ | -1.0 |
| | $OC^{33}S$ | 45 | $1.5\times10^{14}$ | -1.0 |
| | t-HCOOH | 85 | $3.0\times10^{14}$ | 1.0 |
| G133.94+01.06 | $^{13}CN$ | 85 | $1.2\times10^{14}$ | 0. |
| | $HC_3N$ | 85 | $3.9\times10^{14}$ | -0.5 |
| | SO | 45 | $6.4\times10^{15}$ | -0.5 |
| | $HC_3N$, $v_7$=1 | 85 | $6.0\times10^{14}$ | 0. |
| | OCS | 45 | $3.3\times10^{15}$ | -0.5 |
| | HNCO | 45 | $3.0\times10^{13}$ | 0. |
| | $C^{18}O$ | 85 | $1.8\times10^{17}$ | -0.5 |
| | $^{13}CO$ | 85 | $4.5\times10^{18}$ | -0.5 |
| | $CH_3CN$ | 45 | $1.7\times10^{14}$ | -0.5 |
| | $CH_3CHO$ | 45 | $3.3\times10^{14}$ | -0.5 |
| | $C^{17}O$ | 45 | $3.0\times10^{16}$ | -0.3 |
| | CN | 45 | $4.0\times10^{15}$ | -0.5 |
| | $CH_3OH$ | 85 | $2.8\times10^{15}$ | 1.5 |
| | $HC_3N$ | 45 | $6.3\times10^{12}$ | 1.5 |
| | SO | 45 | $6.5\times10^{14}$ | 2.0 |
| G168.06+00.82 | $C^{18}O$ | 85 | $3.0\times10^{16}$ | 1.5 |
| | $^{13}CO$ | 85 | $1.3\times10^{18}$ | 1.5 |
| | $C^{17}O$ | 45 | $5.5\times10^{15}$ | 1.5 |
| | CN | 45 | $3.0\times10^{14}$ | 1.5 |
| | CCS | 45 | $1.3\times10^{13}$ | -1.0 |
| | $^{13}CN$ | 45 | $3.0\times10^{13}$ | -1.0 |
| | $CH_3OH$ | 85 | $6.1\times10^{15}$ | -1.2 |
| | $HC_3N$ | 85 | $7.6\times10^{13}$ | -1.3 |
| | SO | 45 | $4.4\times10^{14}$ | -1.0 |
| | OCS | 45 | $7.9\times10^{13}$ | -1.5 |
| | $C^{18}O$ | 85 | $5.3\times10^{16}$ | -0.5 |
| G176.51+00.20 | HNCO | 45 | $2.3\times10^{13}$ | -1.0 |
| | $C^{15}N$ | 45 | $1.3\times10^{13}$ | -1.0 |
| | $^{13}CO$ | 85 | $1.4\times10^{18}$ | -1.0 |
| | $CH_3CN$ | 45 | $3.3\times10^{12}$ | -1.0 |
| | $CH_3OCH_3$ | 45 | $7.3\times10^{13}$ | -1.0 |
| | $CH_3CHO$ | 45 | $9.4\times10^{13}$ | -1.3 |
| | $C^{17}O$ | 45 | $7.0\times10^{15}$ | 0. |
| | CN | 45 | $1.6\times10^{15}$ | -1.0 |
| | CCS | 45 | $1.3\times10^{13}$ | -0.8 |
| | $HOCO^+$ | 45 | $4.4\times10^{12}$ | -1.0 |
| | $CH_3OH$ | 45 | $2.4\times10^{14}$ | -0.5 |
| | $^{13}CN$ | 45 | $3.8\times10^{13}$ | -0.5 |
| | $HC_3N$ | 85 | $1.0\times10^{14}$ | -1.0 |
| | SO | 45 | $2.5\times10^{14}$ | -0.8 |
| | OCS | 45 | $1.2\times10^{14}$ | -1.0 |
| G183.72−03.66 | $C^{18}O$ | 85 | $2.0\times10^{16}$ | -1.0 |

**Table A1.** (Continued)

| Source | Species | Rotational Temperature (K) | Column Density ($cm^{-2}$) | Velocity offset ($km\ s^{-1}$) |
|---|---|---|---|---|
| (1) | (2) | (3) | (4) | (5) |
| G031.28+00.06 | $HC_3N$ | 85 | $3.5\times10^{14}$ | 0. |
| | SO | 45 | $1.5\times10^{15}$ | 0. |
| | OCS | 45 | $1.7\times10^{15}$ | 0. |
| | $C^{18}O$ | 85 | $2.5\times10^{17}$ | 0. |
| | HNCO | 45 | $3.8\times10^{14}$ | 0. |
| | $C^{15}N$ | 45 | $3.0\times10^{13}$ | 0.5 |
| | $^{13}CO$ | 85 | $7.4\times10^{18}$ | 0. |
| | $CH_3CN$ | 45 | $1.3\times10^{14}$ | 0. |
| | $CH_3CHO$ | 45 | $2.6\times10^{14}$ | 0. |
| | $C^{17}O$ | 45 | $4.0\times10^{16}$ | 0. |
| | CN | 45 | $2.0\times10^{15}$ | 0. |
| | CCS | 45 | $2.4\times10^{13}$ | 0. |
| | $HC_5N$ | 45 | $1.4\times10^{13}$ | 0.5 |
| | $CH_3OH$ | 85 | $4.6\times10^{15}$ | 0.5 |
| | $CH_3OCHO$ | 85 | $4.0\times10^{14}$ | 0.5 |
| | $C_2H_3CN$ | 45 | $6.8\times10^{13}$ | -1.0 |
| | $^{13}CN$ | 85 | $1.5\times10^{14}$ | 0. |
| | $HC_3N$ | 85 | $3.0\times10^{14}$ | 0. |
| | SO | 45 | $1.3\times10^{15}$ | 0. |
| G031.58+00.07 | OCS | 45 | $1.5\times10^{15}$ | 0. |
| | $C^{18}O$ | 85 | $2.4\times10^{17}$ | 0. |
| | HNCO | 45 | $2.3\times10^{14}$ | 0. |
| | $^{13}CO$ | 85 | $3.2\times10^{18}$ | 0. |
| | $CH_3CN$ | 45 | $7.3\times10^{13}$ | 0. |
| | $CH_3OCH_3$ | 45 | $7.5\times10^{14}$ | 0. |
| | $CH_3CHO$ | 45 | $2.5\times10^{14}$ | 0. |
| | $C^{17}O$ | 45 | $3.7\times10^{16}$ | 0.5 |
| | CN | 45 | $3.0\times10^{15}$ | 0. |
| | $NH_2CHO$ | 45 | $3.0\times10^{13}$ | -1.0 |
| | CCS | 45 | $1.0\times10^{13}$ | -1.0 |
| | $HC_5N$ | 45 | $1.1\times10^{13}$ | -1.0 |
| | $^{34}SO$ | 45 | $3.2\times10^{13}$ | -1.0 |
| | $CH_3OCH_3$ | 45 | $1.5\times10^{15}$ | -1.0 |
| | $OC^{34}S$ | 45 | $1.0\times10^{14}$ | -1.0 |
| | $CH_3OH$ | 85 | $5.2\times10^{15}$ | -1.0 |
| | $C_2H_5CN$ | 85 | $5.0\times10^{13}$ | -1.0 |
| | $^{13}CH_3CN$ | 85 | $1.0\times10^{13}$ | -1.0 |
| | $CH_3OCHO$ | 45 | $3.0\times10^{14}$ | -1.0 |
| G032.04+00.05 | t-HCOOH | 85 | $2.2\times10^{14}$ | -1.0 |
| | $^{13}CN$ | 85 | $2.6\times10^{14}$ | -1.0 |
| | $HC_3N$ | 85 | $3.1\times10^{14}$ | -1.0 |
| | SO | 45 | $1.2\times10^{15}$ | -1.0 |
| | OCS | 45 | $1.4\times10^{15}$ | -1.0 |
| | HNCO | 45 | $8.5\times10^{13}$ | -1.0 |
| | $C^{18}O$ | 85 | $2.3\times10^{17}$ | -1.0 |
| | $^{13}CO$ | 85 | $3.3\times10^{18}$ | -1.5 |
| | $CH_3CN$ | 45 | $1.4\times10^{14}$ | -1.0 |
| | $CH_3CHO$ | 45 | $3.7\times10^{14}$ | -2.0 |
| | $C^{17}O$ | 45 | $3.0\times10^{16}$ | -1.0 |
| | CN | 45 | $3.0\times10^{15}$ | -2.0 |
| | $NH_2CHO$ | 45 | $2.0\times10^{13}$ | 1.0 |
| | CCS | 45 | $1.0\times10^{13}$ | 0. |
| | $HC_5N$ | 45 | $1.1\times10^{13}$ | 0. |
| | $CH_3OCHO$ | 45 | $3.0\times10^{14}$ | 0. |
| | t-HCOOH | 85 | $1.6\times10^{14}$ | 2.0 |
| | $^{13}CN$ | 85 | $1.7\times10^{14}$ | 1.0 |
| | $CH_3OH$ | 85 | $5.2\times10^{15}$ | 0. |
| | SiS | 85 | $7.0\times10^{12}$ | 0. |
| | $HC_3N$ | 85 | $1.8\times10^{14}$ | 0. |
| G034.39+00.22 | SO | 45 | $4.5\times10^{14}$ | 0. |
| | OCS | 45 | $4.8\times10^{14}$ | 0. |
| | $C^{18}O$ | 85 | $1.7\times10^{17}$ | 0.5 |
| | HNCO | 45 | $2.1\times10^{14}$ | 0. |
| | $^{13}CO$ | 85 | $2.0\times10^{18}$ | 0. |
| | $CH_3CN$ | 45 | $4.8\times10^{13}$ | 0. |
| | $CH_3OCH_3$ | 45 | $1.0\times10^{14}$ | 0. |
| | $CH_3CHO$ | 45 | $2.0\times10^{14}$ | 0. |
| | $C^{17}O$ | 45 | $2.7\times10^{16}$ | 0. |
| | CN | 45 | $2.0\times10^{15}$ | 0. |
| | HNCO | 45 | $2.7\times10^{13}$ | -0.7 |
| | $C^{15}N$ | 45 | $1.0\times10^{13}$ | -0.7 |
| | $^{13}CO$ | 85 | $4.7\times10^{17}$ | -1.0 |
| | $CH_3CN$ | 45 | $8.5\times10^{12}$ | -1.0 |
| | $CH_3OCH_3$ | 45 | $5.7\times10^{13}$ | -0.5 |
| | $CH_3CHO$ | 45 | $3.7\times10^{13}$ | -0.5 |
| | $C^{17}O$ | 45 | $3.0\times10^{15}$ | -0.5 |
| | CN | 45 | $2.1\times10^{15}$ | -1.0 |
| | CCS | 45 | $1.0\times10^{13}$ | -4.6 |
| | $^{34}SO$ | 45 | $3.3\times10^{13}$ | -5.2 |
| | $CH_3OH$ | 45 | $6.0\times10^{14}$ | -5.0 |
| | t-HCOOH | 85 | $1.2\times10^{14}$ | -5.0 |
| | $^{13}CN$ | 85 | $5.0\times10^{13}$ | -5.0 |
| | $HC_3N$ | 85 | $1.3\times10^{14}$ | -4.7 |
| | SO | 45 | $1.4\times10^{15}$ | -4.6 |
| G188.94+00.88 | OCS | 45 | $3.3\times10^{14}$ | -4.7 |
| | $C^{18}O$ | 85 | $6.0\times10^{16}$ | -5.0 |
| | HNCO | 45 | $5.4\times10^{13}$ | -4.8 |
| | $C^{15}N$ | 45 | $7.4\times10^{12}$ | -4.8 |
| | $^{13}CO$ | 85 | $2.3\times10^{18}$ | -5.0 |
| | $CH_3CN$ | 45 | $1.4\times10^{13}$ | -4.8 |
| | $CH_3CHO$ | 45 | $7.4\times10^{13}$ | -4.8 |
| | $C^{17}O$ | 45 | $7.7\times10^{15}$ | -5.0 |
| | CN | 45 | $2.4\times10^{15}$ | -4.8 |
| | $NH_2CHO$ | 45 | $3.5\times10^{13}$ | -0.5 |
| | $CH_3OCHO$ | 45 | $2.5\times10^{15}$ | 1.0 |
| | CCS | 45 | $9.2\times10^{12}$ | 1.5 |
| | $^{34}SO$ | 45 | $4.5\times10^{13}$ | 0.3 |
| | $CH_3OH$ | 85 | $2.2\times10^{17}$ | -0.5 |
| | $SO_2$ | 45 | $1.1\times10^{15}$ | 0.5 |
| | t-HCOOH | 85 | $4.1\times10^{14}$ | -0.5 |
| | $^{13}CN$ | 85 | $4.1\times10^{13}$ | 0.7 |
| | $C_2H_5OH$ | 85 | $8.1\times10^{14}$ | -0.5 |
| G192.60−00.04 | $HC_3N$ | 85 | $1.9\times10^{14}$ | 1.2 |
| | SO | 45 | $2.3\times10^{15}$ | 1.3 |
| | OCS | 45 | $5.0\times10^{14}$ | 1.5 |
| | HNCO | 45 | $1.1\times10^{13}$ | -1.0 |
| | $C^{18}O$ | 85 | $9.0\times10^{16}$ | 1.5 |
| | $^{13}CO$ | 85 | $3.8\times10^{18}$ | 1.3 |
| | $CH_3CN$ | 45 | $4.0\times10^{13}$ | 0.5 |
| | $CH_3CHO$ | 45 | $1.2\times10^{14}$ | 0.5 |
| | $C^{17}O$ | 45 | $1.3\times10^{16}$ | 1.3 |
| | CN | 45 | $5.2\times10^{15}$ | 1.5 |
| | CCS | 45 | $5.0\times10^{12}$ | 5.7 |
| | $CH_3OH$ | 45 | $1.6\times10^{15}$ | 5.0 |
| | $C_2H_5CN$ | 45 | $3.0\times10^{13}$ | 4.0 |
| | $CH_3OCHO$ | 45 | $1.9\times10^{14}$ | 5.0 |
| | $SO_2$ | 45 | $1.7\times10^{15}$ | 4.0 |
| | $^{13}CN$ | 45 | $3.7\times10^{13}$ | 5.3 |
| | $HC_3N$ | 85 | $8.3\times10^{13}$ | 5.5 |
| | SO | 45 | $6.4\times10^{14}$ | 5.5 |
| G209.00−19.38 | OCS | 45 | $2.7\times10^{14}$ | 5.5 |
| | $C^{18}O$ | 85 | $2.2\times10^{1}$ | 6.0 |
| | HNCO | 45 | $2.2\times10^{13}$ | 5.5 |
| | $C^{15}N$ | 45 | $2.0\times10^{13}$ | 5.5 |
| | $^{13}CO$ | 85 | $1.5\times10^{18}$ | 6.0 |
| | $CH_3CN$ | 45 | $3.7\times10^{13}$ | 5.5 |
| | $CH_3OCH_3$ | 45 | $2.0\times10^{14}$ | 5.0 |
| | $CH_3CHO$ | 45 | $3.0\times10^{13}$ | 5.5 |
| | $C^{17}O$ | 45 | $5.0\times10^{15}$ | 6.0 |
| | CN | 45 | $2.6\times10^{15}$ | 6.0 |
| | CCS | 45 | $9.0\times10^{12}$ | -4.0 |
| | $^{34}SO$ | 45 | $2.2\times10^{13}$ | -5.0 |
| | $CH_3OH$ | 45 | $5.1\times10^{13}$ | -3.0 |
| | $^{13}CN$ | 45 | $8.4\times10^{12}$ | -4.0 |
| | $HC_3N$ | 45 | $7.4\times10^{13}$ | -4.0 |
| | SO | 45 | $7.1\times10^{14}$ | -4.0 |
| G232.62+00.99 | OCS | 45 | $5.2\times10^{13}$ | -4.2 |
| | $C^{18}O$ | 45 | $3.2\times10^{16}$ | -4.4 |
| | HNCO | 45 | $8.0\times10^{12}$ | -4.5 |
| | $^{13}CO$ | 85 | $1.3\times10^{18}$ | -4.3 |
| | $CH_3CN$ | 45 | $1.1\times10^{13}$ | -4.0 |
| | $C^{17}O$ | 45 | $2.5\times10^{15}$ | -4.5 |
| | CN | 85 | $3.5\times10^{15}$ | -4.0 |

**Table A2.** Detected lines and their parameters in each sources

| Species | Transitions | Rest Freq. (MHz) | $E_u$ (K) | $\mu^2S$ ($D^2$) | $T_{mb}$ (mK) | $V_{LSR}$ (km $s^{-1}$) | $\Delta V$ (km $s^{-1}$) | $\int T_{mb}$ dv (mK km $s^{-1}$) |
|---|---|---|---|---|---|---|---|---|
| | | | | G000.67−00.03 | | | | |
| $NH_2CHO$ | 5(2, 4) − 4(2, 3) | 105972.665(37e-3) | 27.2 | 54.915 | 611 | 62.5(0.1) | 13.2 (0.3) | 8594(140) |
| $NH_2CHO$ | 5(4, 1) − 4(4, 0) | 106107.870(88e-3) | 63.0 | 23.537 | 239 | 62.5(0.3) | 9.3(0.7) | 2360(138) |
| $NH_2CHO$ | 5(3, 3) − 4(3, 2) | 106134.468(55e-3) | 42.1 | 41.845 | 391 | 62.5(0.5) | 12.8(0.5) | 5319(171) |
| $NH_2CHO$ | 5(3, 2) − 4(3, 1) | 106141.442(55e-3) | 42.1 | 41.84 | 375 | 62.5(0.5) | 12.0(0.5) | 4791(160) |
| $NH_2CHO$ | 5(2, 3) − 4(2, 2) | 106541.773(37e-3) | 27.2 | 54.915 | 598 | 62.5(0.1) | 12.8(0.3) | 8163(172) |
| CCS | 8(9) − 7(8) | 106347.726(2e-2) | 25.0 | 74.425 | 340 | 62.0(0.2) | 17.4(0.6) | 6309(164) |
| $C_2H_5CN$ | 15(3, 12) − 15(2, 13) | 106375.033(5e-2) | 61.7 | 13.244 | 46 | 62.0(1.1) | 9.2 (3.1) | 453(110) |
| $HC_5N$ | 40 − 39 | 106498.910(7e-3) | 104.8 | 2249.7 | 90 | 62.0(0.1) | 18.7(0.5) | 1802(77) |
| $C_2H_3CN$ | 11(1, 10) − 10(1, 9) | 106641.383(1e-3) | 32.9 | 476.24 | 204 | 62.5(0.3) | 12.6(0.8) | 2745(168) |
| $C_2H_5OH$ | 13(1, 12) − 13(0, 13) | 106649.479(5e-2) | 79.4 | 10.463 | 42 | 62.0(1.8) | 16.1(10.3) | 719(265) |
| $C_2H_5OH$ | 6(1, 5) − 5(1, 4) | 106676.542(5e-2) | 76.1 | 9.325 | 40 | 62.0(1.5) | 8.1(2.4) | 345(109) |
| $C_2H_5OH$ | 9(2, 8) − 9(1, 9) | 106723.558(5e-2) | 42.7 | 7.9044 | 108 | 62.0(0.5) | 18.0(0.5) | 2078(66) |
| Hα | H (39) α | 106737.357(0) | – | – | 265 | 55.6(0.6) | 40.8(1.4) | 10701 (294) |
| $C_2H_5OH$ | 6(1, 5) − 5(1, 4) | 106767.234(5e-2) | 80.7 | 9.6466 | 56 | 62.0(1.5) | 21.9(6.3) | 1890(350) |
| $CH_3OCH_3$ | 9(1, 8) − 8(2, 7) | 106777.344(9e-3) | 43.4 | 58.573 | 89 | 62.0(0.9) | 10.7(1.8) | 1006(159) |
| $OC^{34}S$ | 9 − 8 | 106787.390(2e-3) | 25.6 | 4.601 | 146 | 62.0(0.5) | 10.6(1.1) | 1643(147) |
| $CH_3OH$, vt=0-2 | $3(1)^+ - 4(0)^+$, vt=0 | 107013.831(1e-2) | 28.3 | 12.036 | 1321 | 60.0(0.) | 11.8(0.1) | 16553(143) |
| $C_2H_5CN$ | 12(2, 11) − 11(2, 10) | 107043.527(5e-2) | 37.9 | 172.86 | 248 | 62.0(0.3) | 12.1(0.7) | 3182(148) |
| $CH_3C^{15}N$ | 6(3) − 5(3) | 107043.140(6e-2) | 82.4 | 277.350 | blended | – | – | – |
| $CH_3C^{15}N$ | 6(0) − 5(0) | 107061.410(6e-2) | 18.0 | 184.936 | 139 | 61.8(0.5) | 15.2(1.3) | 2250(165) |
| $CH_3OH$, vt=0-2 | 15(-2) − 15(1) E2, vt=0 | 107159.906(14e-3) | 304.7 | 10.421 | 180 | 60.0(0.5) | 33.5(1.3) | 6402(205) |
| $^{13}CH_3CN$ | 6(2) − 5(2) | 107188.500(1e-1) | 46.6 | 164.068 | 231 | 61.5 (0.5) | 14.5(1.1) | 3552(240) |
| $^{13}CH_3CN$ | 6(1) − 5(1) | 107194.550(1e-1) | 25.2 | 179.427 | 134 | 61.5(0.7) | 10.1(2.0) | 1435(231) |
| $^{13}CH_3CN$ | 6(0) − 5(0) | 107196.570(1e-1) | 18.0 | 184.590 | 120 | 61.5(0.5) | 15.3(2.3) | 1959(184) |
| $C_2H_5CN$ | 12(7, 5) − 11(7, 4) | 107485.160(5e-2) | 88.0 | 117.36 | 272 | 62.0(0.5) | 16.7(0.5) | 4830(59) |
| $C_2H_5CN$ | 12(6, 6) − 11(6, 5) | 107486.949(5e-2) | 73.6 | 133.42 | 160 | 62.0(0.5) | 11.0(0.5) | 1866(59) |
| $C_2H_5CN$ | 12(5, 7) − 11(5, 6) | 107502.432(5e-2) | 61.3 | 146.99 | 241 | 62.0(0.5) | 16.1(0.5) | 4140(59) |
| $C_2H_5CN$ | 12(10, 2) − 11(10, 1) | 107519.861(5e-2) | 144.6 | 54.355 | 130 | 62.0(0.5) | 10.6(0.5) | 1466(59) |
| $CH_3OCHO$ | 9( 2, 8) − 8( 2, 7) E | 107537.258(1e-2) | 28.8 | 22.60702 | 159 | 62.0(0.5) | 13.2(0.5) | 2218(59) |
| $CH_3OCHO$ | 9( 2, 8) − 8( 2, 7) A | 107543.711(1e-2) | 28.8 | 22.61344 | blended | – | – | – |
| $C_2H_5CN$ | 12(4, 9) − 11(4, 8) | 107544.042(5e-2) | 51.3 | 158.12 | 302 | 62.0(0.5) | 10.1(0.5) | 3251(59) |
| $C_2H_5CN$ | 12(4, 8) − 11(4, 7) | 107547.460(5e-2) | 51.3 | 158.11 | 183 | 62.0(0.5) | 10.5(0.5) | 2046(59) |
| $C_2H_5CN$ | 12(3, 10) − 11(3, 9) | 107594.056(5e-2) | 43.6 | 166.77 | 213 | 62.0(0.5) | 16.6(0.5) | 3770(59) |
| $CH_3OCHO$ | 23( 6,17) − 23( 5,18) E | 107604.366(1e-2) | 189.0 | 7.68978 | 68 | 62.0(0.5) | 8.6(0.5) | 626(59) |
| $C_2H_5CN$ | 12(3, 9) − 11(3, 8) | 107734.723(5e-2) | 43.6 | 166.76 | 221 | 62.0(0.5) | 26.9(1.8) | 6317(271) |
| $CH_3OCH_3$ | 47(18, 30) − 48(17, 32) | 107770.696(68) | 1479.8 | 24.31526 | 68 | 62.0(0.7) | 6.7(1.4) | 479(97) |
| $SO_2$ | 12(4, 8) − 13(3, 11) | 107843.470(2e-3) | 111.0 | 4.5354 | 175 | 60.0(0.5) | 16.6 (1.0) | 3096(163) |
| t-HCOOH | 5(1, 5) − 4(1, 4) | 108126.720(3e-3) | 18.8 | 9.6966 | 114 | 62.0(0.6) | 13.4(1.5) | 1636(151) |
| $CH_3SH$, v=0-2 | 4(-1, 4) − 4(0, 4) A, vt=0 | 108379.758(1e-3) | 17.3 | 0.3856 | 51 | 62.0(1.2) | 4.4(2.1) | 237(121) |
| $CH_3OH$, vt=0-2 | 0(0) − 1(-1) E2, vt=0 | 108893.945(12e-3) | 13.1 | 3.9134 | 860 | 62.0(0.) | 11.7(0.2) | 10689(171) |
| SiS | 6(0) − 5(0) | 108924.301(1e-2) | 18.3 | 5.62 | 138 | 62.0(0.6) | 17.2(2.0) | 2530(200) |
| $C_2H_5CN$ | 12(2, 10) − 11(2, 9) | 108940.554(5e-2) | 38.2 | 172.93 | blended | – | – | – |
| $C_2H_5CN$ | 11(3, 9) − 12(0, 12) | 108940.696(4e-3) | 38.4 | 0.042598 | 246 | 62.0(0.3) | 15.2(1.2) | 3999(206) |
| $HC_3N$ | 12 − 11 | 109173.634(1e-2) | 34.1 | 167.1 | 5943 | 62.0(0.5) | 17.0(0.5) | 107590(914) |
| SO | 3(2) − 2(1) | 109252.220(1e-1) | 21.1 | 3.5585 | 2083 | 62.0(0.) | 20.4(0.1) | 45302(340) |
| $HC_3N$, $v_7$=1 | 12(-1) − 11(1) | 109442.013(2e-2) | 355.0 | 165.12 | 136 | 62.0(0.7) | 25.7(2.0) | 3725(228) |
| OCS | 9 − 8 | 109463.063(5e-3) | 26.3 | 4.6034 | 1574 | 62.0(0.) | 11.2(0.3) | 18740(647) |
| HNCO | 5(1, 5) − 4(1, 4) | 109495.996(6e-3) | 59.0 | 11.847 | 409 | 62.0(0.3) | 16.2(0.9) | 7058(298) |
| $CH_3OCH_3$ | 8( 2, 7) − 8( 1, 8) AA | 109576.778(11e-3) | 38.3 | 59.869 | 97 | 62.0(1.4) | 33.8(5.2) | 3505(370) |
| $HC_3N$, $v_7$=1 | 12(-1) − 11(1) | 109442.013(2e-2) | 355.0 | 165.12 | 172 | 62.0(0.8) | 27.8(2.8) | 6910(366) |
| $C_2H_5CN$ | 12(1, 11) − 11(1, 10) | 109650.263(5e-2) | 53.4 | 176.49 | 246 | 62.0(0.4) | 19.4(1.5) | 5084(274) |
| $NH_2CHO$ | 5(1, 4) − 4(1, 3) | 109753.549(25e-3) | 18.8 | 62.756 | 687 | 62.5(0.5) | 15.1(0.5) | 11021(454) |
| $C^{18}O$ | 1 − 0 | 109782.173(6e-3) | 5.3 | 0.01221 | 3271 | 62.0(0.5) | 11.2(0.5) | 72371(454) |
| HNCO | 5(0, 5) − 4(0, 4) | 109905.749(7e-3) | 15.8 | 12.482 | 4931 | 62.0(0.) | 22.6(0.1) | 118770(478) |
| $^{13}CO$ | 1 − 0 | 110201.35(0) | 5.3 | 0.01220 | 10745 | 63.0(0.5) | 20.1(0.9) | 229350(11600) |
| HNCO | 5(1, 4) − 4(1, 3) | 110298.089(5e-3) | 59.2 | 11.847 | 425 | 62.0(0.5) | 18.3(0.5) | 8291(430) |
| $CH_3{}^{13}CN$ | 6(2) − 5(2) | 110320.400(1e-1) | 47.1 | 164.054 | 146 | 62.2(0.5) | 14.2(0.5) | 2210(430) |
| $CH_3{}^{13}CN$ | 6(1) − 5(1) | 110326.770(1e-1) | 25.7 | 179.434 | 170 | 62.1(0.5) | 16.0(0.5) | 2890(430) |
| $CH_3{}^{13}CN$ | 6(0) − 5(0) | 110328.870(1e-1) | 18.5 | 184.563 | 330 | 62.2(0.5) | 19.4(0.5) | 6808(430) |
| $CH_3CN$ | 6(5, 0) − 5(5, 0) | 110330.345(0) | 197.1 | 56.399 | blended | – | – | – |
| $CH_3CN$ | 6(4, 0) − 5(4, 0) | 110349.471(0) | 132.8 | 102.54 | 455 | 62.0(0.5) | 24.1(0.5) | 11703(430) |
| $CH_3CN$ | 6(3, 0) − 5(-3, 0) | 110364.354(0) | 82.8 | 138.45 | 1485 | 62.0(0.5) | 18.1(0.5) | 28546(430) |
| $CH_3CN$ | 6(-3, 0) − 5(3, 0) | 110364.354(0) | 82.8 | 138.45 | blended | – | – | – |
| $CH_3CN$ | 6(2, 0) − 5(2, 0) | 110374.989(0) | 47.1 | 164.06 | 1800 | 62.0(0.5) | 15.0(0.5) | 28663(430) |
| $CH_3CN$ | 6(1, 0) − 5(1, 0) | 110381.372(0) | 25.7 | 179.45 | 3010 | 62.0(0.5) | 17.8(0.5) | 57045(430) |
| $CH_3OCHO$ | 9( 7, 3) − 8( 7, 2) E | 110536.003(1e-2) | 59.1 | 9.46692 | 89 | 62.0(0.8) | 10.2(2.9) | 974(186) |
| $CH_3OCHO$ | 9( 6, 3) − 8( 6, 2) E | 110652.813(1e-2) | 50.5 | 13.30853 | 74 | 62.0(1.5) | 25.6(4.7) | 2003(283) |
| $CH_3OCHO$ | 9( 6, 3) − 8( 6, 2) A | 110663.429(1e-2) | 50.4 | 13.31127 | 191 | 62.0(0.6) | 13.0(1.0) | 2648(205) |
| $CH_3OCHO$ | 9( 6, 4) − 8( 6, 3) A | 110663.273(1e-2) | 50.4 | 13.3112 | blended | – | – | – |
| $CH_3OCHO$ | 10( 1, 10) − 9( 1, 9) A | 110790.526(1e-2) | 30.3 | 16.17539 | 236 | 62.0(0.2) | 5.4(0.2) | 1351(17) |
| $C_2H_3CN$ | 12( 1, 12) − 11( 1, 11) | 110839.968 (1e-3) | 36.8 | 520.3 | 174 | 62.5(0.2) | 6.0(0.2) | 1116(17) |
| $CH_3OCHO$ | 9( 5, 4) − 8( 5, 3) E | 110873.955(1e-2) | 43.2 | 16.55225 | 97 | 62.0(0.2) | 4.3(0.2) | 448(17) |
| $CH_3OCHO$ | 9( 5, 5) − 8( 5, 4) E | 110882.331(1e-2) | 43.2 | 16.55225 | 212 | 62.0(0.2) | 5.5(0.2) | 1247(17) |
| $CH_3OCHO$ | 9( 3, 7) − 8( 3, 6) A | 110887.092(1e-2) | 32.6 | 21.25577 | 144 | 62.0(0.2) | 6.5(0.2) | 995(17) |
| $CH_3OCHO$ | 9( 4, 6) − 8( 4, 5) E | 111223.491(1e-2) | 37.2 | 18.18412 | 108 | 62.0(0.7) | 9.7(2.4) | 1116(184) |
| $CH_3OH$, vt=0-2 | $7(2)^+ - 8(1)^+$, vt=0 | 111289.453(13e-3) | 102.7 | 9.3425 | 368 | 60.0(0.2) | 11.7(0.5) | 4601(169) |
| $CH_3OCHO$ | 9( 4, 5) − 8( 4, 4) E | 111408.412(1e-2) | 37.3 | 18.18412 | 91 | 62.0(0.) | 8.8(1.2) | 857(84) |
| $CH_3OCHO$ | 9( 4, 5) − 8( 4, 4) A | 111453.300(1e-2) | 37.2 | 19.21778 | 129 | 62.0(0.5) | 10.3(1.4) | 1420(156) |
| $CH_3OCHO$ | 9( 1, 8) − 8( 1, 7) E | 111674.131(1e-2) | 28.1 | 23.18984 | 169 | 62.0(0.8) | 17.3(2.8) | 2941(333) |
| $CH_3OCHO$ | 9( 1, 8) − 8( 1, 7) A | 111682.189(1e-2) | 28.1 | 23.19587 | 166 | 62.0(0.8) | 14.1(1.9) | 2494(306) |
| t-HCOOH | 5(0, 5) − 4(0, 4) | 111746.784(3e-3) | 16.1 | 10.092 | 153 | 62.0(0.7) | 18.3(2.0) | 2988(255) |
| $CH_3OCH_3$ | 19( 3,16) − 19( 2,17) AA | 111744.238(29e-3) | 187.5 | 259.8 | blended | – | – | – |
| $CH_3OCH_3$ | 7( 0, 7) − 6( 1, 6) AA | 111782.562(8e-3) | 25.2 | 68.047 | 328 | 62.0(0.2) | 11.6(0.6) | 4067(196) |
| $CH_3OCH_3$ | 18( 3,15) − 18( 2,16) EE | 111813.668(21e-3) | 169.8 | 386.29 | 69 | 62.0(1.5) | 15.1(3.7) | 1100(230) |
| $HC_5N$ | 42 − 41 | 111823.024(0) | 115.4 | 2362.2 | 102 | 62.0(1.0) | 10.9(2.3) | 1180(203) |
| Hβ | H (48) β | 111885.070(0) | – | – | 56 | 64.1(1.9) | 14.8(3.7) | 881(208) |
| $CH_3CHO$ | 6( 1, 6) − 5( 1, 5) A, vt=0 | 112248.716(3e-3) | 21.1 | 73.76807 | 385 | 62.0(0.5) | 27.4(0.5) | 11227(131) |
| $CH_3CHO$ | 6( 1, 6) − 5( 1, 5) A, vt=1 | 112254.508(3e-3) | 21.2 | 73.79585 | 279 | 62.0(0.5) | 18.8(0.5) | 5577(131) |
| t-HCOOH | 5(2, 4) − 4(2, 3) | 112287.145(3e-3) | 28.9 | 8.4851 | 65 | 62.0(1.0) | 5.2(2.3) | 360(139) |
| $CH_3OCHO$ | 25( 5,20) − 25( 4,21) A | 112310.915(1e-2) | 214.4 | 7.80962 | 106 | 62.0(0.4) | 2.4(0.9) | 276(92) |
| $C^{17}O$ | 1 − 0 | 112359.284(1e-3) | 5.4 | 0.01217 | 1141 | 61.8(0.5) | 24.1(0.5) | 29315(135) |
| $CH_3COCH_3$ | 6( 5, 1) − 5( 4, 1) EE | 112375.101(8e-3) | 18.4 | 70.65642 | 104 | 62.0(0.5) | 16.7(0.5) | 1843(135) |
| t-HCOOH | 5(4, 1) − 4(4, 0) | 112432.319(3e-3) | 67.1 | 3.6372 | 64 | 62.0(0.5) | 5.0(0.5) | 337(135) |
| t-HCOOH | 5(4, 2) − 4(4, 1) | 112432.292(3e-3) | 67.1 | 3.6372 | blended | – | – | – |
| t-HCOOH | 5(3, 3) − 4(3, 2) | 112459.621(3e-3) | 67.1 | 6.4662 | 27 | 62.0(0.5) | 14.2(0.5) | 402(135) |
| t-HCOOH | 5(3, 2) − 4(3, 1) | 112467.007(3e-3) | 44.8 | 6.4654 | 62 | 62.0(0.5) | 13.8(0.5) | 905(135) |
| $C_2H_5CN$ | 13( 1, 13) − 12( 1, 12) | 112646.350(9e-2) | 39.0 | 191.45 | 293 | 62.0(0.4) | 14.1(1.1) | 4390(258) |
| $C_2H_5OH$ | 2( 2, 1) − 1( 1, 0) | 112807.174(5e-2) | 7.5 | 3.2057 | 198 | 62.0(0.5) | 20.2(0.5) | 4262(59) |
| $C_2H_3CN$ | 12( 0,12) −11( 0,11) | 112840.637(1e-3) | 35.3 | 523.56 | 245 | 62.5(0.5) | 14.0(0.5) | 2660(59) |

**Table A2.** (Continued)

| Species | Transitions | Rest Freq. (MHz) | $E_u$ (K) | $\mu^2$S ($D^2$) | $T_{mb}$ (mK) | $V_{LSR}$ (km $s^{-1}$) | ΔV (km $s^{-1}$) | $\int T_{mb}$ dv (mK km $s^{-1}$) |
|---|---|---|---|---|---|---|---|---|
| t-HCOOH | 5(2, 3) − 4(2, 2) | 112891.443(3e-3) | 28.9 | 8.4849 | 134 | 62.0(0.5) | 7.9(0.5) | 1124(59) |
| $CH_3OCH_3$ | 17( 3,14) − 17( 2,15) AA | 113061.072(22e-3) | 153.1 | 221.33 | 89 | 62.0(0.5) | 13.4(0.5) | 1270(123) |
| $C_2H_5OH$ | 10( 2, 9) − 10 ( 1, 10) | 113098.078(5e-2) | 51.0 | 8.3566 | 99 | 62.0(0.5) | 20.4(0.5) | 2140(123) |
| CN | N= 1-0, J=1/2-1/2, F=1/2-1/2 | 113123.370(6e-3) | 5.4 | 0.15271 | blended | – | – | – |
| CN | N= 1-0, J=1/2-1/2, F=1/2-3/2 | 113144.157(6e-3) | 5.4 | 1.2492 | 275 | 60.0(0.5) | 13.2(0.5) | 3874(117) |
| CN | N= 1-0, J=1/2-1/2, F=3/2-1/2 | 113170.492(4e-3) | 5.4 | 1.2199 | 609 | 59.3(0.6) | 9.6(1.3) | 6273(683) |
| CN | N= 1-0, J=1/2-1/2, F=3/2-3/2 | 113191.279(3e-3) | 5.4 | 1.5836 | 252 | 59.6(0.5) | 12.3(0.5) | 3303(117) |
| CCS | 9(8) − 8(7) | 113410.186(2e-2) | 33.6 | 65.427 | 178 | 62.8(0.5) | 12.8(0.5) | 2434(191) |
| CN | N= 1-0, J=3/2-1/2, F=3/2-1/2 | 113488.120(3e-3) | 5.4 | 1.5838 | 272 | 60.3(0.8) | 7.8(2.3) | 2258(502) |
| CN | N= 1-0, J=3/2-1/2, F=5/2-3/2 | 113490.970(2e-3) | 5.4 | 4.205 | 186 | 60.0(1.3) | 7.0(3.0) | 1375(467) |
| CN | N= 1-0, J=3/2-1/2, F=1/2-1/2 | 113499.644(3e-3) | 5.4 | 1.2491 | 168 | 60.0(1.3) | 7.1(2.6) | 1263(429) |
| CN | N= 1-0, J=3/2-1/2, F=3/2-3/2 | 113508.907(3e-3) | 5.4 | 1.2196 | 123 | 59.8(1.5) | 4.5(3.3) | 585(356) |
| CN | N= 1-0, J=3/2-1/2, F=1/2-3/2 | 113520.432(4e-3) | 5.4 | 0.15263 | 260 | 60.1(0.9) | 6.6(2.3) | 1815(471) |
| | | | | G005.88−00.39 | | | | |
| CCS | 8(9) − 7(8) | 106347.726(2e-2) | 25.0 | 74.425 | 328 | 9.0(0.) | 4.3(0.3) | 1513(72) |
| $HC_5N$ | 40 − 39 | 106498.910(7e-3) | 104.8 | 2249.7 | 334 | 8.7(0.) | 4.4(0.2) | 1556(62) |
| $C_2H_3CN$ | 11(1, 10) − 10(1, 9) | 106641.395(1e-3) | 32.9 | 476.24 | 181 | 8.5(0.2) | 4.0 (0.3) | 773(53) |
| Hα | H (39) α | 106737.357(0) | – | – | 1081 | 6.9(0.2) | 59.1(0.6) | 67990(543) |
| $CH_3OH$, vt=0-2 | $3(1)^+ − 4( 0)^+$, vt=0 | 107013.831(1e-2) | 28.3 | 12.036 | 847 | 9.5(0.) | 6.0(0.1) | 5437(96) |
| $SO_2$ | 27(3, 25) − 26(4, 22) | 107060.208(2e-3) | 369.4 | 8.2723 | 175 | 9.0(0.2) | 6.7(0.5) | 1240(80) |
| $CH_3C_3N$ | 26(2) − 25(2) | 107407.677(4e-3) | 99.5 | 116.3 | 55 | 9.0(0.6) | 3.3(0.9) | 193(47) |
| $CH_3C_3N$ | 26(1) − 25(1) | 107410.776(4e-3) | 77.1 | 1171.5 | 41 | 9.0(0.2) | 3.9(1.0) | 169(47) |
| $CH_3C_3N$ | 26(0) − 25(0) | 107411.809(4e-3) | 69.6 | 1173.3 | 157 | 8.9(0.2) | 5.0(0.4) | 845(56) |
| $SO_2$ | 12(4, 8) − 13(3, 11) | 107843.470(2e-3) | 111.0 | 4.5354 | 443 | 9.0(0.) | 7.1(0.2) | 33304(87) |
| $^{13}CN$ | 1(1, 0) − 0(1, 1), F = 1 − 2 | 108426.889(5e-2) | 5.2 | 1.267 | 121 | 8.1 (0.2) | 2.7(0.5) | 350(52) |
| $^{13}CN$ | 1(1, 1) − 0(1, 0), F = 0 − 1 | 108631.121(5e-2) | 5.2 | 0.642 | 75 | 8.3(0.5) | 5.5(0.5) | 434(47) |
| $^{13}CN$ | 1(1, 1) − 0(1, 0), F = 1 − 1 | 108636.923(5e-2) | 5.2 | 1.932 | 204 | 8.6(0.5) | 3.3(0.5) | 723(47) |
| $^{13}CN$ | 1(2, 1) − 0(1, 1), F = 1 − 0 | 108638.212(5e-2) | 5.2 | 0.722 | 68 | 8.7(0.5) | 3.9(0.5) | 277(47) |
| $^{13}CN$ | 1(2, 1) − 0(1, 1), F = 2 − 1 | 108643.590(5e-2) | 5.2 | 0.856 | 128 | 8.8(0.5) | 2.8(0.5) | 385(47) |
| $^{13}CN$ | 1(2, 1) − 0(1, 1), F = 0 − 1 | 108644.346(5e-2) | 5.2 | 0.642 | 116 | 8.7(0.5) | 2.9(0.5) | 364(47) |
| $^{13}CN$ | 1(2, 1) − 0(1, 1), F = 1 − 1 | 108645.064(5e-2) | 5.2 | 0.551 | blended | – | – | – |
| $^{13}CN$ | 1(1, 1) − 0(1, 0), F = 2 − 1 | 108651.297(5e-2) | 5.2 | 3.276 | 316 | 8.9(0.5) | 2.8(0.5) | 959(47) |
| $^{13}CN$ | 1(2, 1) − 0(1, 1), F = 2 − 2 | 108657.646(5e-2) | 5.2 | 2.420 | 206 | 9.0(0.5) | 4.5(0.5) | 978(47) |
| $^{13}CN$ | 1(2, 1) − 0(1, 1), F = 1 − 2 | 108658.948(5e-2) | 5.2 | 0.669 | blended | – | – | – |
| $^{13}CN$ | 1(2, 2) − 0(1, 1), F = 3 − 2 | 108780.201(5e-2) | 5.2 | 4.905 | 463 | 8.6(0.1) | 3.2(0.2) | 1595(73) |
| $^{13}CN$ | 1(2, 2) − 0(1, 1), F = 2 − 1 | 108782.374(5e-2) | 5.2 | 2.586 | 211 | 8.6(0.2) | 3.5(0.4) | 786(77) |
| $^{13}CN$ | 1(2, 2) − 0(1, 1), F = 1 − 0 | 108786.982(5e-2) | 5.2 | 1.144 | 133 | 8.6(0.2) | 2.4(0.4) | 336(57) |
| $^{13}CN$ | 1(2, 2) − 0(1, 1), F = 1 − 1 | 108793.753(5e-2) | 5.2 | 0.894 | 106 | 8.5(0.3) | 3.2(0.7) | 360(68) |
| $^{13}CN$ | 1(2, 2) − 0(1, 1), F = 2 − 2 | 108796.400(5e-2) | 5.2 | 0.918 | 90 | 8.5(0.4) | 3.1(1.4) | 291(85) |
| $CH_3OH$, vt=0-2 | 0(0) − 1(-1) E2, vt=0 | 108893.945(12e-3) | 13.1 | 3.9134 | 747 | 9.5(0.) | 2.2(0.1) | 1736(55) |
| $HC_5N$ | 41 − 40 | 109160.973(7e-3) | 110.0 | 2306 | 291 | 8.5(0.1) | 4.9(0.3) | 1533(78) |
| $HC_3N$ | 12 − 11 | 109173.634(1e-2) | 34.1 | 167.1 | 13456 | 9.0(0.) | 4.5(0.1) | 64643(771) |
| SO | 3(2) − 2(1) | 109252.220(1e-1) | 21.1 | 3.5585 | 2709 | 9.3(0.0) | 8.0(0.1) | 23053(292) |
| $HC_3N$, $v_7$=1 | 12(-1) − 11(1) | 109442.013(2e-2) | 355.0 | 165.12 | 198 | 9.5(0.2) | 5.0(0.6) | 1047(94) |
| OCS | 9 − 8 | 109463.063(5e-3) | 26.3 | 4.6034 | 815 | 9.5(0.1) | 5.3(0.1) | 4634(97) |
| Hγ | H (55) γ | 109536.001(1e-3) | – | – | 71 | 9.3(1.8) | 33.3(3.5) | 2518(260) |
| $HC_3N$, $v_7$=1 | 12(1) − 11(-1) | 109598.818(2e-2) | 355.0 | 165.12 | 168 | 9.5(0.2) | 4.2(0.5) | 749(75) |
| $C^{18}O$ | 1 − 0 | 109782.173(6e-3) | 5.3 | 0.01221 | 5448 | 9.0(0.1) | 4.1(0.1) | 23710(359) |
| HNCO | 5(0, 5) − 4(0, 4) | 109905.749(7e-3) | 15.8 | 12.482 | 557 | 9.0(0.1) | 6.5(0.3) | 3840(122) |
| $C^{15}N$ | 1(2, 1) − 0(1, 0) | 110023.540(1e-1) | 5.3 | 1.386 | 84 | 7.1(0.5) | 4.4(1.3) | 389(98) |
| $C^{15}N$ | 1(2, 2) − 0(1, 1) | 110024.590(1e-1) | 5.3 | 3.504 | 90 | 7.5(0.2) | 1.1(0.6) | 107(57) |
| $^{13}CO$ | 1 − 0 | 110201.35(0) | 5.3 | 0.01220 | 22621 | 9.2(0.1) | 4.0(0.1) | 96974(1520) |
| HNCO | 5(1, 4) − 4(1, 3) | 110298.089(5e-3) | 59.2 | 11.847 | 57 | 9.0(1.5) | 22.0(3.7) | 1331(187) |
| $CH_3CN$ | 6(5, 0) − 5(5, 0) | 110330.345(0) | 197.1 | 56.399 | 100 | 9.0(0.5) | 10.3(0.5) | 1100(257) |
| $CH_3CN$ | 6(4, 0) − 5(4, 0) | 110349.471(0) | 132.8 | 102.54 | 229 | 9.0(0.5) | 5.4(0.5) | 1325(257) |
| $CH_3CN$ | 6(3, 0) − 5(-3, 0) | 110364.354(0) | 82.8 | 138.45 | 1116 | 9.0(0.5) | 5.5(0.5) | 6487(257) |
| $CH_3CN$ | 6(-3, 0) − 5(3, 0) | 110364.354(0) | 82.8 | 138.45 | blended | – | – | – |
| $CH_3CN$ | 6(2, 0) − 5(2, 0) | 110374.989(0) | 47.1 | 164.06 | 1252 | 9.0(0.5) | 5.4(0.5) | 7253(257) |
| $CH_3CN$ | 6(1, 0) − 5(1, 0) | 110381.372(0) | 25.7 | 179.45 | 2197 | 9.0(0.5) | 5.3(0.5) | 12296(257) |
| $CH_3CN$ | 6(0, 0) − 5(0, 0) | 110383.500(0) | 18.5 | 184.58 | 2300 | 9.0(0.5) | 4.3(0.5) | 10501(257) |
| $CH_3OCHO$ | 10(1, 10) − 9(1, 9) E | 110788.664(1e-2) | 30.3 | 26.16584 | 101 | 8.5(0.5) | 4.0(0.5) | 433(27) |
| $CH_3OCHO$ | 10(1, 10) − 9(1, 9) A | 110790.526(1e-2) | 30.3 | 16.17539 | 82 | 8.5(0.5) | 1.8(0.5) | 157(27) |
| $C_2H_3CN$ | 12( 1, 12) − 11( 1, 11) | 110839.968 (1e-3) | 36.8 | 520.3 | 117 | 8.5(0.4) | 5.1(0.8) | 631(94) |
| $CH_3OH$, vt=0-2 | $7(2)^+ − 8( 1)^+$, vt=0 | 111289.453(13e-3) | 102.7 | 9.3425 | 163 | 9.5(0.5) | 3.6(0.5) | 620(34) |
| $CH_3C_3N$ | 27(2) − 26(2) | 111538.207(4e-3) | 104.9 | 1211.5 | 53 | 8.0(0.6) | 2.7(1.1) | 154(61) |
| $CH_3C_3N$ | 27(1) − 26(1) | 111541.424(4e-3) | 82.4 | 1216.7 | 50 | 8.0(0.9) | 2.0(0.9) | 333(106) |
| $CH_3C_3N$ | 27(0) − 26(0) | 111542.497(4e-3) | 74.9 | 1218.5 | 182 | 8.0(0.2) | 4.4(0.5) | 846(88) |
| $CH_3OCH_3$ | 7( 0, 7) − 6( 1, 6) AA | 111782.600 (1e-3) | 25.2 | 68.047 | 151 | 10.0(0.3) | 4.8(0.9) | 774(108) |
| $HC_5N$ | 42 − 41 | 111823.024(0) | 115.4 | 2362.2 | 339 | 8.5(0.5) | 4.1(0.5) | 1476(66) |
| Hβ | H (48) β | 111885.070(0) | – | – | 242 | 10.6(0.8) | 56.7 (1.7) | 14611(400) |
| $C^{17}O$ | 1 − 0 | 112359.284(1e-3) | 5.4 | 0.01217 | 1220 | 9.1(0.1) | 6.0(0.1) | 7729(152) |
| $C_2H_3CN$ | 12(0, 12) − 11(0, 11) | 112840.637 (1e-3) | 35.3 | 157.45337 | 218 | 8.5(0.2) | 3.6(0.5) | 835(104) |
| CN | N= 1-0, J=1/2-1/2, F=1/2-1/2 | 113123.370(6e-3) | 5.4 | 0.15271 | 1473 | 9.0(0.1) | 3.4(0.3) | 5362(330) |
| CN | N= 1-0, J=1/2-1/2, F=1/2-3/2 | 113144.157(6e-3) | 5.4 | 1.2492 | 3687 | 9.0(0.) | 4.4(0.1) | 17079(381) |
| CN | N= 1-0, J=1/2-1/2, F=3/2-1/2 | 113170.492(4e-3) | 5.4 | 1.2199 | 5444 | 9.0(0.) | 4.1(0.1) | 24001(374) |
| CN | N= 1-0, J=1/2-1/2, F=3/2-3/2 | 113191.279(3e-3) | 5.4 | 1.5836 | 4413 | 9.0(0.) | 4.4(0.1) | 20617(381) |
| CN | N= 1-0, J=3/2-1/2, F=3/2-1/2 | 113488.120(3e-3) | 5.4 | 1.5838 | 5259 | 9.0(0.5) | 2.0(0.5) | 11442(965) |
| CN | N= 1-0, J=3/2-1/2, F=5/2-3/2 | 113490.970(2e-3) | 5.4 | 4.205 | 11501 | 9.0(0.5) | 4.1(0.5) | 50691(965) |
| CN | N= 1-0, J=3/2-1/2, F=1/2-1/2 | 113499.644(3e-3) | 5.4 | 1.2491 | 2280 | 9.0(0.5) | 4.2(0.5) | 10242(965) |
| CN | N= 1-0, J=3/2-1/2, F=3/2-3/2 | 113508.907(3e-3) | 5.4 | 1.2196 | 3305 | 9.0(0.5) | 3.8(0.5) | 13342(965) |
| CN | N= 1-0, J=3/2-1/2, F=1/2-3/2 | 113520.432(4e-3) | 5.4 | 0.15263 | 864 | 9.0(0.5) | 1.1(0.5) | 1035(965) |
| | | | | G009.62+00.19 | | | | |
| $NH_2CHO$ | 5(2, 4) − 4(2, 3) | 105972.665(37e-3) | 27.2 | 54.915 | 33 | 3.1(0.8) | 8.5(1.3) | 302(51) |
| $NH_2CHO$ | 5(4, 1) − 4(4, 0) | 106107.870(88e-3) | 63.0 | 23.537 | 31 | 3.0(1.0) | 9.3(1.7) | 310(58) |
| $NH_2CHO$ | 5(3, 3) − 4(3, 2) | 106134.468(55e-3) | 42.1 | 41.845 | 29 | 2.8(1.0) | 8.8(2.7) | 272(68) |
| $NH_2CHO$ | 5(3, 2) − 4(3, 1) | 106141.442(55e-3) | 42.1 | 41.84 | 26 | 3.1(1.2) | 10.8(2.8) | 297(69) |
| CCS | 8(9) − 7(8) | 106347.726(2e-2) | 25.0 | 74.425 | 145 | 3.5(0.1) | 4.6(0.4) | 717(49) |
| $HC_5N$ | 40 − 39 | 106498.910(7e-3) | 104.8 | 2249.7 | 70 | 3.5(0.2) | 3.8(0.6) | 279(37) |
| $NH_2CHO$ | 5(2, 3) − 4(2, 2) | 106541.773(37e-3) | 27.2 | 54.915 | 37 | 3.0(0.7) | 4.5(1.0) | 180(35) |
| $C_2H_5OH$ | 9(2, 8) − 9(1, 9) | 106723.558(5e-2) | 42.7 | 7.904 | 52 | 4.(0.3) | 2.2(0.6) | 122(30) |
| Hα | H (39) α | 106737.357(0) | – | – | 65 | 8.1(0.7) | 19.1(1.1) | 1317(26) |
| $^{34}SO$ | 3(2) − 2(1) | 106743.244(7e-20 | 20.9 | 3.557 | 51 | 4.8(0.5) | 8.4(1.5) | 461(76) |
| $C_2H_5OH$ | 6(1, 5) − 5(1, 4) | 106767.234(5e-2) | 80.7 | 9.6466 | 44 | 4.0(0.5) | 1.1(1.2) | 50(33) |
| $CH_3OCH_3$ | 9(1, 8) − 8(2, 7) AA | 106775.679(2e-3) | 43.4 | 36.60122 | blended | – | – | – |
| $CH_3OCH_3$ | 9(1, 8) − 8(2, 7) EE | 106777.372(1e-3) | 43.4 | 58.57089 | blended | – | – | – |
| $CH_3OCH_3$ | 9(1, 8) − 8(2, 7) AE | 106779.069(2e-3) | 43.3 | 17.39008 | blended | – | – | – |

**Table A2.** (Continued)

| Species | Transitions | Rest Freq. (MHz) | $E_u$ (K) | $\mu^2S$ ($D^2$) | $T_{mb}$ (mK) | $V_{LSR}$ (km $s^{-1}$) | $\Delta V$ (km $s^{-1}$) | $\int T_{mb}$ dv (mK km $s^{-1}$) |
|---|---|---|---|---|---|---|---|---|
| $OC^{34}S$ | 9 − 8 | 106787.390(2e-3) | 25.6 | 4.601 | 84 | 3.7(0.3) | 6.0(0.7) | 533(52) |
| He$\alpha$ | He (39) $\alpha$ | 106780.85240 (0.) | − | − | 33 | 8.2(1.0) | 9.2(1.8) | 319(63) |
| $CH_3OH$, vt=0-2 | $3(1)^+ − 4(0)^+$, vt=0 | 107013.831(1e-2) | 28.3 | 12.036 | 664 | 4.5(0.5) | 5.0(0.5) | 3539(477) |
| $C_2H_5CN$ | 12(2, 11) − 11(2, 10) | 107043.527(5e-2) | 37.9 | 172.86 | 69 | 5.0(0.5) | 1.3(0.5) | 93(22) |
| $CH_3OH$, vt=0-2 | 15(-2) − 15(1) E2, vt=0 | 107159.906(14e-3) | 304.7 | 10.421 | 62 | 3.8(0.4) | 7.4(1.0) | 489(53) |
| $^{13}CH_3CN$ | 6(4) − 5(4) | 107164.310(0) | 132.5 | 102.548 | 21 | 4.4(1.1) | 7.9(3.0) | 177(50) |
| $^{13}CH_3CN$ | 6(3) − 5(3) | 107178.424(0) | 82.4 | 276.826 | 32 | 4.8(0.6) | 7.6(1.3) | 260(42) |
| $^{13}CH_3CN$ | 6(2) − 5(2) | 107188.500(1e-1) | 46.6 | 164.068 | 22 | 5.6(0.7) | 5.2(1.5) | 124(39) |
| $^{13}CH_3CN$ | 6(1) − 5(1) | 107194.550(1e-1) | 25.2 | 179.427 | 41 | 4.0(2.2) | 5.1(1.7) | 260(128) |
| $^{13}CH_3CN$ | 6(0) − 5(0) | 107196.570(1e-1) | 18.0 | 184.590 | 45 | 5.1(2.2) | 5.6(2.2) | 266(47) |
| $C_2H_5CN$ | 12(7, 5) − 11(7, 4) | 107485.160(5e-2) | 88.0 | 117.36 | 106 | 5.0(0.3) | 10.0(0.7) | 1126(70) |
| $C_2H_5CN$ | 12(6, 6) − 11(6, 5) | 107486.949(5e-2) | 73.6 | 133.42 | 68 | 5.2(0.3) | 4.9(0.7) | 359(48) |
| $C_2H_5CN$ | 12(5, 7) − 11(5, 6) | 107502.432(5e-2) | 61.3 | 146.99 | 118 | 5.0(0.2) | 7.1(0.5) | 886(59) |
| $C_2H_5OH$ | 8( 2, 7) − 7( 3, 5), vt=1-0 | 107498.091(5e-2) | 96.3 | 1.1723 | 57 | 4.0(0.2) | 0.9(0.3) | 55(20) |
| $CH_3OCHO$ | 9( 2, 8) − 8( 2, 7) E | 107537.258(1e-2) | 28.8 | 22.60702 | 46 | 4.0(0.6) | 8.4(1.5) | 414(63) |
| $CH_3OCHO$ | 9( 2, 8) − 8( 2, 7) A | 107543.711(1e-2) | 28.8 | 22.61344 | 110 | 4.0(0.2) | 7.0(0.7) | 818(67) |
| $C_2H_5CN$ | 12(4, 9) − 11(4, 8) | 107544.042(5e-2) | 51.3 | 158.12 | blended | − | − | − |
| $C_2H_5CN$ | 12(4, 8) − 11(4, 7) | 107547.460(5e-2) | 51.3 | 158.11 | 73 | 4.8(0.4) | 5.5(0.9) | 430(61) |
| $C_2H_5CN$ | 12(3, 10) − 11(3, 9) | 107594.056(5e-2) | 43.6 | 166.77 | 72 | 5.0(0.4) | 8.3(0.9) | 675(62) |
| $C_2H_5CN$ | 12(3, 9) − 11(3, 8) | 107734.723(5e-2) | 43.6 | 166.76 | 70 | 5.0(0.4) | 9.3(1.0) | 688(61) |
| t-HCOOH | 5(1, 5) − 4(1, 4) | 108126.720(3e-3) | 18.8 | 9.6966 | 37 | 3.6(0.4) | 2.9(1.1) | 116(33) |
| $^{13}CN$ | 1(1, 1) − 0(1, 0), F = 0 − 1 | 108631.121(5e-2) | 5.2 | 0.642 | 20 | 3.4(0.5) | 3.8(0.5) | 82(23) |
| $^{13}CN$ | 1(1, 1) − 0(1, 0), F = 1 − 1 | 108636.923(5e-2) | 5.2 | 1.932 | 55 | 3.4(0.5) | 4.2(0.5) | 247(23) |
| $^{13}CN$ | 1(2, 1) − 0(1, 1), F = 1 − 0 | 108638.212(5e-2) | 5.2 | 0.722 | 31 | 3.6(0.5) | 5.5(0.5) | 181(23) |
| $^{13}CN$ | 1(2, 1) − 0(1, 1), F = 2 − 1 | 108643.590(5e-2) | 5.2 | 0.856 | 38 | 3.5(0.5) | 3.3(0.5) | 133(23) |
| $^{13}CN$ | 1(2, 1) − 0(1, 1), F = 0 − 1 | 108644.346(5e-2) | 5.2 | 0.642 | 48 | 3.8(0.5) | 3.6(0.5) | 181(23) |
| $^{13}CN$ | 1(2, 1) − 0(1, 1), F = 1 − 1 | 108645.064(5e-2) | 5.2 | 0.551 | 43 | 4.0(0.5) | 2.5(0.5) | 113(23) |
| $^{13}CN$ | 1(1, 1) − 0(1, 0), F = 2 − 1 | 108651.297(5e-2) | 5.2 | 3.276 | 129 | 3.6(0.5) | 4.2(0.5) | 576(23) |
| $^{13}CN$ | 1(2, 1) − 0(1, 1), F = 2 − 2 | 108657.646(5e-2) | 5.2 | 2.420 | 96 | 3.2(0.5) | 4.6(0.5) | 471(23) |
| $^{13}CN$ | 1(2, 1) − 0(1, 1), F = 1 − 2 | 108658.948(5e-2) | 5.2 | 0.669 | 13 | 3.8(0.5) | 7.4(0.5) | 105(23) |
| $^{13}CN$ | 1(2, 2) − 0(1, 1), F = 3 − 2 | 108780.201(5e-2) | 5.2 | 4.905 | 157 | 4.1(0.5) | 5.4(0.5) | 904(31) |
| $^{13}CN$ | 1(2, 2) − 0(1, 1), F = 2 − 1 | 108782.374(5e-2) | 5.2 | 2.586 | 77 | 4.7(0.5) | 5.0(0.5) | 410(31) |
| $^{13}CN$ | 1(2, 2) − 0(1, 1), F = 1 − 0 | 108786.982(5e-2) | 5.2 | 1.144 | 63 | 4.2(0.5) | 2.5(0.5) | 171(31) |
| $^{13}CN$ | 1(2, 2) − 0(1, 1), F = 1 − 1 | 108793.753(5e-2) | 5.2 | 0.894 | 25 | 3.8(0.5) | 4.4(0.5) | 116(31) |
| $^{13}CN$ | 1(2, 2) − 0(1, 1), F = 2 − 2 | 108796.400(5e-2) | 5.2 | 0.918 | 20 | 4.0(0.5) | 2.6(0.5) | 56(31) |
| $CH_3OH$, vt=0-2 | 0(0) − 1(-1) E2, vt=0 | 108893.945(12e-3) | 13.1 | 3.913 | 871 | 4.1(0.) | 8.2(0.1) | 7604(104) |
| $C_2H_5CN$ | 12(2, 10) − 11(2, 9) | 108940.554(5e-2) | 38.2 | 172.93 | 70 | 5.0(0.7) | 3.8(1.3) | 281(85) |
| $C_2H_5CN$ | 11(3, 9) − 12(0, 12) | 108940.696(4e-3) | 38.4 | 0.042598 | 36 | 5.0(0.5) | 3.5(2.2) | 133(109) |
| $CH_3OH$, vt=0-2 | 26(0) − 26(-1) E2, vt=0 | 109137.011(18e-3) | 821.5 | 12.31 | 67 | 4.5(0.5) | 4.5(0.5) | 324(291) |
| $CH_3OH$, vt=0-2 | 14(5) − 15(4) E1, vt=0 | 109138.783(15e-3) | 379.7 | 13.593 | 60 | 4.3(0.5) | 1.7(0.5) | 112(291) |
| $CH_3OH$, vt=0-2 | 16(-2) − 16(1) E2, vt=0 | 109153.184(14e-3) | 342.0 | 14.726 | 71 | 4.1(0.5) | 6.5(0.5) | 491(291) |
| $HC_5N$ | 41 − 40 | 109160.973(7e-3) | 110.0 | 2306 | 79 | 3.0(0.5) | 6.2(0.5) | 520(291) |
| $HC_3N$ | 12 − 11 | 109173.634(1e-2) | 34.1 | 167.1 | 2956 | 3.7(0.5) | 5.5(0.5) | 17224(291) |
| SO | 3(2) − 2(1) | 109252.220(1e-1) | 21.1 | 3.5585 | 718 | 4.6(0.) | 6.8(0.1) | 5230(81) |
| $HC_3N$, $v_7$=1 | 12(-1) − 11(1) | 109442.013(2e-2) | 355.0 | 165.12 | 82 | 3.2(0.5) | 9.1(1.4) | 789(127) |
| OCS | 9 − 8 | 109463.063(5e-3) | 26.3 | 4.6034 | 717 | 4.5(0.) | 7.1(0.1) | 5406(93) |
| HNCO | 5(1, 5) − 4(1, 4) | 109495.996(6e-3) | 59.0 | 11.847 | 63 | 3.8(0.) | 7.0(1.9) | 470(103) |
| $HC_3N$, $v_7$=1 | 12(1) − 11(-1) | 109598.818(2e-2) | 355.0 | 165.12 | 99 | 3.0(0.5) | 7.8(0.5) | 822(25) |
| $C^{18}O$ | 1 − 0 | 109782.173(6e-3) | 5.3 | 0.01221 | 422 | 4.2(0.5) | 8.8(0.5) | 3947(915) |
| HNCO | 5(2, 4) − 4(2, 3) | 109872.337(3e-2) | 186.1 | 10.013 | 72 | 4.0(0.4) | 0.5(0.1) | 42(28) |
| HNCO | 5(2, 3) − 4(2, 2) | 109872.765(3e-2) | 186.1 | 10.012 | 27 | 4.0(0.9) | 1.5(0.2) | 45(58) |
| HNCO | 5(0, 5) − 4(0, 4) | 109905.749(7e-3) | 15.8 | 12.482 | 716 | 4.0(0.) | 6.7(0.2) | 5092(115) |
| $C^{15}N$ | 1(2, 1) − 0(1, 0) | 110023.540(1e-1) | 5.3 | 1.386 | 17 | 4.8(1.0) | 0.5(0.1) | 98(26) |
| $C^{15}N$ | 1(2, 2) − 0(1, 1) | 110024.590(1e-1) | 5.3 | 3.504 | 81 | 4.3(0.2) | 0.5(0.2) | 47(42) |
| $^{13}CO$ | 1 − 0 | 110201.35(0) | 5.3 | 0.01220 | 15946 | 4.5(0.1) | 6.7(0.2) | 114280(2560) |
| HNCO | 5(1, 4) − 4(1, 3) | 110298.089(5e-3) | 59.2 | 11.847 | 31 | 4.0(1.3) | 3.0(1.1) | 99(85) |
| $CH_3CN$ | 6(5, 0) − 5(5, 0) | 110330.345(0) | 197.1 | 56.399 | 100 | 3.8(0.6) | 6.7(1.6) | 710(124) |
| $CH_3CN$ | 6(4, 0) − 5(4, 0) | 110349.471(0) | 132.8 | 102.54 | 209 | 4.0(0.) | 5.8(0.5) | 1290(99) |
| $CH_3CN$ | 6(3, 0) − 5(-3, 0) | 110364.354(0) | 82.8 | 138.45 | 568 | 4.0(0.) | 6.3(0.2) | 3788(108) |
| $CH_3CN$ | 6(-3, 0) − 5(3, 0) | 110364.354(0) | 82.8 | 138.45 | blended | − | − | − |
| $CH_3CN$ | 6(2, 0) − 5(2, 0) | 110374.989(0) | 47.1 | 164.06 | 586 | 4.0(0.) | 6.5(0.2) | 4073(114) |
| $CH_3CN$ | 6(1, 0) − 5(1, 0) | 110381.372(0) | 25.7 | 179.45 | 92 | 4.2(0.2) | 7.5(0.3) | 7297(359) |
| $CH_3CN$ | 6(0, 0) − 5(0, 0) | 110383.500(0) | 18.5 | 184.58 | 793 | 3.9(0.1) | 5.3(0.2) | 4434(325) |
| $CH_3OCHO$ | 9(6, 4) − 8(6, 3) E | 110662.315(1e-2) | 50.4 | 13.30855 | 47 | 4.0(0.8) | 3.7(1.5) | 182(77) |
| $CH_3OCHO$ | 10(1,10) − 9(1, 9) E | 110788.664(1e-2) | 30.3 | 26.16584 | 63 | 4.0(1.0) | 4.7(1.6) | 318(121) |
| $CH_3OCHO$ | 10(1, 10) − 9(1, 9) A | 110790.526(1e-2) | 30.3 | 26.17539 | 25 | 4.0(0.6) | 1.2(1.4) | 33(81) |
| $C_2H_3CN$ | 12(1, 12) − 11(1, 11) | 110839.968(1e-3) | 36.8 | 520.3 | 26 | 4.6(1.2) | 1.7(2.5) | 46(62) |
| $CH_3OCHO$ | 9(5, 5) − 8(5, 4) A | 110880.447(1e-2) | 43.2 | 16.56015 | 61 | 4.0(0.2) | 0.8(0.7) | 51(25) |
| $CH_3OCHO$ | 9(5, 5) − 8(5, 4) E | 110882.331(1e-2) | 43.2 | 16.55225 | 42 | 4.0(0.) | 3.0(1.1) | 132(38) |
| $CH_3OCHO$ | 10(0, 10) − 9(0, 9) E | 111169.903(1e-2) | 30.2 | 26.18776 | 45 | 4.0(0.7) | 1.7(1.3) | 80(60) |
| $CH_3OCHO$ | 10(0, 10) − 9(0, 9) A | 111171.634(1e-2) | 30.2 | 26.19136 | 86 | 4.0(0.3) | 1.1(0.6) | 105(51) |
| $CH_3OH$, vt=0-2 | $7( 2)^+ − 8( 1)^+$, vt=0 | 111289.453(13e-3) | 102.7 | 9.3425 | 190 | 4.5(0.5) | 5.1(0.5) | 1023(41) |
| $CH_3OCH_3$ | 7(0, 7) − 6(1, 6) AA | 111782.600(1e-3) | 25.2 | 68.047 | 139 | 3.0(0.3) | 5.2(0.6) | 770(94) |
| $CH_3OCH_3$ | 18(3, 15) − 18( 2, 16) EE | 111813.812(1e-3) | 169.8 | 386.29 | 60 | 3.0(0.4) | 1.6(0.6) | 105(43) |
| $HC_5N$ | 42 − 41 | 111823.024(0) | 115.4 | 2362.2 | 82 | 3.3(0.3) | 1.2(0.5) | 107(40) |
| $CH_3CHO$ | 6(1, 6) − 5(1, 5) A, vt=0 | 112248.716(3e-3) | 21.1 | 73.76807 | 66 | 4.0(0.6) | 3.8(1.0) | 267(76) |
| $CH_3CHO$ | 6(1, 6) − 5(1, 5) E, vt=0 | 112254.508(3e-3) | 21.2 | 73.79585 | 108 | 4.0(0.3) | 3.4(0.6) | 392(64) |
| $C^{17}O$ | 1 − 0 | 112359.284(1e-3) | 5.4 | 0.01217 | 1765 | 3.5(0.1) | 5.9(0.1) | 11092(111) |
| $C_2H_5CN$ | 13(1, 13) − 12(1, 12) | 112646.350(9e-2) | 39.0 | 191.45 | 90 | 5.0(0.4) | 5.3(0.8) | 512(79) |
| $C_2H_3CN$ | 12(0, 12) − 11( 0, 11) | 112840.637(1e-3) | 35.3 | 523.56 | 78 | 4.6(0.4) | 1.7(0.8) | 140(52) |
| $C_2H_3CN$ | 47(7, 41) − 48( 6, 42) | 113092.551(6e-3) | 948.3 | 6.7184 | 185 | 4.5(0.2) | 2.3(0.7) | 445(93) |
| $C_2H_3CN$ | 20(4, 17) − 421(3, 18) | 113093.970(1e-3) | 130.3 | 8.493 | 124 | 4.5(0.) | 0.9(0.4) | 114(54) |
| CN | N= 1-0, J=1/2-1/2, F=1/2-1/2 | 113123.370(6e-3) | 5.4 | 0.15271 | 570 | 4.2(0.5) | 5.4(0.5) | 3288(252) |
| CN | N= 1-0, J=1/2-1/2, F=1/2-3/2 | 113144.157(6e-3) | 5.4 | 1.2492 | 1621 | 4.2(0.5) | 4.2(0.5) | 7267(252) |
| CN | N= 1-0, J=1/2-1/2, F=3/2-1/2 | 113170.492(4e-3) | 5.4 | 1.2199 | 2194 | 4.2(0.5) | 4.1(0.5) | 9558(252) |
| CN | N= 1-0, J=1/2-1/2, F=3/2-3/2 | 113191.279(3e-3) | 5.4 | 1.5836 | 1802 | 4.2(0.5) | 4.1(0.5) | 7796(252) |
| CN | N= 1-0, J=3/2-1/2, F=3/2-1/2 | 113488.120(3e-3) | 5.4 | 1.5838 | 1781 | 4.2(0.5) | 4.3(0.5) | 8208(447) |
| CN | N= 1-0, J=3/2-1/2, F=5/2-3/2 | 113490.970(2e-3) | 5.4 | 4.205 | 4345 | 4.2(0.5) | 3.9(0.5) | 17967(447) |
| CN | N= 1-0, J=3/2-1/2, F=1/2-1/2 | 113499.644(3e-3) | 5.4 | 1.2491 | 927 | 4.2(0.5) | 4.2(0.5) | 4177(447) |
| CN | N= 1-0, J=3/2-1/2, F=3/2-3/2 | 113508.907(3e-3) | 5.4 | 1.2196 | 1402 | 4.2(0.5) | 4.9(0.5) | 7296(545) |
| CN | N= 1-0, J=3/2-1/2, F=1/2-3/2 | 113520.432(4e-3) | 5.4 | 0.15263 | 269 | 4.2(0.5) | 5.4(0.5) | 1556(447) |
| G010.47+00.02 | | | | | | | | |
| $SO_2$, $v_2$=1 | 10(1, 9) − 10(0, 10) | 105956.755(0) | 799.9 | 17.868 | 35 | 67.2(1.4) | 12.4(2.8) | 469(96) |
| $NH_2CHO$ | 5(2, 4) − 4(2, 3) | 105972.665(37e-3) | 27.2 | 54.915 | 473 | 67.0(0.) | 9.1(0.2) | 4559(99) |
| $CH_3OCHO$ | 3(3, 1) − 2(2, 0) A | 105977.940(1e-2) | 9.5 | 1.13661 | 52 | 67.0(0.9) | 9.6(2.3) | 532(103) |
| $CH_3OCHO$ | 3(3, 1) − 2(2, 1) E | 106018.879(1e-2) | 9.5 | 0.96781 | 65 | 67.0(0.5) | 5.7(0.5) | 67 (37) |
| $CH_3OCHO$ | 3(3, 0) − 2(2, 0) E | 106031.705(1e-2) | 9.5 | 0.96583 | 26 | 67.0(2.1) | 6.4(1.5) | 91(41) |
| $NH_2CHO$ | 5(4, 1) − 4(4, 0) | 106107.870(88e-3) | 63.0 | 23.537 | 411 | 66.8(0.2) | 9.7(0.4) | 4227(136) |

**Table A2.** (Continued)

| Species | Transitions | Rest Freq. | $E_u$ | $\mu^2S$ | $T_{mb}$ | $V_{LSR}$ | $\Delta V$ | $\int T_{mb}$ dv |
|---|---|---|---|---|---|---|---|---|
| | | (MHz) | (K) | ($D^2$) | (mK) | (km $s^{-1}$) | (km $s^{-1}$) | (mK km $s^{-1}$) |
| $NH_2CHO$ | 5(4, 2) − 4(4, 1) | 106107.845(88e-3) | 63.0 | 23.537 | blended | – | – | – |
| $CH_3OCHO$ | 3(3, 0) − 2(2, 1) A | 106125.344(1e-2) | 9.5 | 1.13527 | 24 | 67.0(0.5) | 4.7(0.5) | 122(54) |
| $NH_2CHO$ | 5(3, 3) − 4(3, 2) | 106134.468(55e-3) | 42.1 | 41.845 | 417 | 67.0(0.) | 9.8(0.2) | 4335(85) |
| $NH_2CHO$ | 5(3, 2) − 4(3, 1) | 106141.442(55e-3) | 42.1 | 41.84 | 418 | 67.4(0.) | 10.1(0.2) | 4499(87) |
| $^{13}CH_3CH_2CN$ | 12(2, 10) − 11(2, 9) | 106257.434(2e-3) | 37.4 | 169.890 | 53 | 67.1(0.5) | 4.8(2.0) | 269(73) |
| CCS | 8(9) − 7(8) | 106347.726(2e-2) | 25.0 | 74.425 | 97 | 67.0(0.3) | 7.5(0.6) | 780(61) |
| $C_2H_5OH$ | 22(5, 17) − 21(6, 16) | 106375.782(5e-2) | 244.6 | 6.3338 | 158 | 67.0(0.2) | 7.1(0.4) | 1191(59) |
| HCOCN | 11(3, 9) − 10(3, 8) | 106392.645(4e-3) | 57.7 | 22.91014 | 540 | 64.1(0.3) | 0.8(0.3) | 430(20) |
| HCOCN | 11(3, 8) − 10(3, 7) | 106397.716(4e-3) | 57.7 | 22.90799 | 410 | 64.0(0.5) | 1.5(0.5) | 310(18) |
| HCOCN | 11(4, 8) − 10(4, 7) | 106397.763(4e-3) | 78.6 | 21.47650 | blended | – | – | – |
| HCOCN | 11(4, 7) − 10(4, 6) | 106397.792(4e-3) | 78.6 | 21.47649 | blended | – | – | – |
| HCOCN | 11(5, 6) − 10(5, 5) | 106417.668(4e-3) | 105.6 | 19.63758 | 390 | 64.0(0.5) | 5.5(0.1) | 230(28) |
| HCOCN | 11(6, 5) − 10(6, 4) | 106447.709(4e-3) | 138.4 | 17.386 | 128 | 64.0(0.5) | 9.4(0.5) | 1271(20) |
| HCOCN | 11(7, 4) − 10(7, 3) | 106485.698(4e-3) | 177.1 | 14.727 | 52 | 64.1(0.5) | 5.6(0.5) | 313(20) |
| $HC_5N$ | 40 − 39 | 106498.910(7e-3) | 104.8 | 2249.7 | 64 | 67.0(0.5) | 8.7(0.5) | 591(20) |
| $C_2H_5{}^{13}CN$ | 15(3, 12) − 15(2, 13) | 106469.905(2e-3) | 61.4 | 13.330 | blended | – | – | – |
| $C_2H_5{}^{13}CN$ | 12(2, 11) − 11(2, 10) | 106514.253(1e-3) | 37.7 | 169.810 | 49 | 65.9(1.9) | 6.1(3.5) | 315(181) |
| $NH_2CHO$ | 5(2, 3) − 4(2, 2) | 106541.773(37e-3) | 27.2 | 54.915 | 465 | 67.0(0.1) | 9.4(0.1) | 4634(62) |
| $C_2H_5CN$ | 27(3, 24) − 26(4, 23) | 106562.916(5e-2) | 174.1 | 7.2384 | 47 | 67.0(0.5) | 5.2(0.9) | 263(43) |
| $CH_3OCHO$ | 14(4, 11) − 14(3, 12) E | 106632.804(1e-2) | 72.9 | 3.49007 | 62 | 66.9(0.5) | 7.2(0.5) | 479(40) |
| $C_2H_3CN$ | 11(1, 10) − 10(1, 9) | 106641.389(1e-3) | 32.9 | 476.24 | 360 | 67.0(0.5) | 10.7(0.5) | 4108(40) |
| $CH_3OCHO$ | 9(2, 8) − 8(2, 7) | 106648.754(1e-2) | 216.4 | 22.54 | blended | – | – | – |
| $C_2H_5OH$ | 13(1, 12) − 13(0, 13) | 106649.479(5e-2) | 79.4 | 10.463 | 126 | 66.7(0.5) | 8.7(0.5) | 1163(40) |
| $CH_3OCHO$ | 14(4, 11) − 14(3, 12) A | 106668.134(1e-2) | 72.9 | 3.48762 | 25 | 67.0(0.5) | 6.0(0.5) | 161(40) |
| $C_2H_5OH$ | 6(1, 5) − 5(1, 4) | 106676.542(5e-2) | 76.1 | 9.325 | 75 | 67.1(0.5) | 11.5(0.5) | 919(40) |
| $C_2H_5OH$ | 9(2, 8) − 9(1, 9) | 106723.558(5e-2) | 42.7 | 7.9044 | 113 | 67.0(0.5) | 10.8(0.5) | 1294(41) |
| $C_2H_5OH$ | 6(1, 5) − 5(1, 4) | 106767.234(5e-2) | 80.7 | 9.6466 | 72 | 66.8(0.5) | 7.9(0.5) | 1199(41) |
| $^{34}SO$ | 3(2) − 2(1) | 106743.244(7e-2) | 20.9 | 3.557 | 189 | 67.0(0.5) | 14.1(0.5) | 2839(41) |
| $CH_3OCH_3$ | 9(1, 8) − 8(2, 7) AA | 106775.602(14e-3) | 43.4 | 36.603 | 63 | 67.0(0.5) | 8.4(0.5) | 562(82) |
| $CH_3OCH_3$ | 9(1, 8) − 8(2, 7) EE | 106777.344(9e-3) | 43.4 | 58.573 | 129 | 67.4(0.5) | 9.8(0.5) | 1360(82) |
| $CH_3OCH_3$ | 9(1, 8) − 8(2, 7) EA | 106779.091(11e-3) | 43.4 | 21.963 | 91 | 67.2(0.5) | 7.8(0.5) | 1495(82) |
| $CH_3OCH_3$ | 9(1, 8) − 8(2, 7) AE | 106779.083(11e-3) | 43.4 | 14.645 | blended | – | – | – |
| $OC^{34}S$ | 9 − 8 | 106787.390(2e-3) | 25.6 | 4.601 | 407 | 66.0(0.5) | 9.1(0.5) | 3941(82) |
| $CH_3COCH_3$ | 18(6, 12) − 18(5, 13) EE | 106873.162(18e-3) | 121.8 | 877.18596 | 19 | 67.6(3.0) | 6.8(4.5) | 138(85) |
| $CH_3COCH_3$ | 18(7, 12) − 18(6, 13) EE | 106873.359(18e-3) | 121.8 | 877.18275 | blended | – | – | – |
| $C_2H_5CN$, $v_{12}$=1−A | 12(2, 11) − 11(2, 10) | 106890.807(5e-2) | 806.8 | 169.79 | 43 | 67.2(0.5) | 1.5(1.2) | 68(44) |
| $C_2H_5CN$ | 4(2, 2) − 3(1, 3) | 106905.507(2e-1) | 8.8 | 2.6677 | 42 | 67.0(2.3) | 6.5(3.9) | 297(173) |
| aGg'−$(CH_2OH)_2$ | 12(1, 12) v=0 − 11(1, 11) v=1 | 106907.385(2e-3) | 36.3 | 467.50155 | 38 | 65.2(1.9) | 3.4(3.3) | 143(137) |
| $HOCO^+$ | 5(0, 5) − 4(0, 4) | 106913.545(3e-3) | 15.4 | 36.454 | 68 | 67.0(0.9) | 4.1(1.8) | 296(121) |
| $C_2H_5OH$ | 19(2, 18) − 19(1, 18) | 106931.232(5e-2) | 222.5 | 25.014 | 37 | 67.0(1.5) | 3.4(2.6) | 133(107) |
| $CH_3OCH_2OH$ | 10(2, 8) − 9(2, 7) A | 106951.984(3e-3) | 30.3 | 1.8613 | 83 | 67.0(0.9) | 6.7(1.7) | 590(152) |
| $CH_3OCH_2OH$ | 10(2, 8) − 9(2, 7) E | 106950.381(3e-3) | 30.3 | 1.8613 | blended | – | – | – |
| $CH_3{}^{13}CH_2CN$ | 12(7, 5) − 11(7, 4) | 106956.706(2e-3) | 86.4 | 115.279 | 77 | 67.0(0.9) | 4.8(1.9) | 392(136) |
| $CH_3{}^{13}CH_2CN$ | 12(6, 7) − 11(6, 6) | 106960.569(2e-3) | 72.4 | 131.054 | 87 | 67.0(0.8) | 5.0(1.6) | 465(137) |
| $CH_3{}^{13}CH_2CN$ | 12(6, 6) − 11(6, 5) | 106960.570(2e-3) | 72.4 | 131.054 | blended | – | – | – |
| $C_2H_5{}^{13}CN$ | 12(5, 8) − 11(5, 7) | 106966.128(1e-3) | 61.2 | 144.406 | 42 | 66.0(1.9) | 6.3(4.0) | 284(158) |
| $C_2H_5{}^{13}CN$ | 12(5, 7) − 11(5, 6) | 106966.174(1e-3) | 61.2 | 144.405 | blended | – | – | – |
| $CH_3{}^{13}CH_2CN$ | 12(5, 8) − 11(5, 7) | 106978.873(2e-3) | 60.5 | 144.398 | 53 | 67.1(1.2) | 4.4(2.2) | 246(124) |
| $CH_3{}^{13}CH_2CN$ | 12(5, 7) − 11(5, 6) | 106978.933(2e-3) | 60.5 | 144.398 | blended | – | – | – |
| $C_2H_5{}^{13}CN$ | 12(10, 2) − 11(10, 1) | 106985.100(1e-3) | 144.4 | 54.351 | 101 | 66.2(1.1) | 5.8(1.1) | 631(292) |
| $CH_3COCH_3$ | 18(6, 12) − 18(5, 13) AA | 107006.295(22e-3) | 121.8 | 329.26249 | 49 | 67.5(1.1) | 9.4(1.1) | 1019(292) |
| $CH_3COCH_3$ | 18(7, 12) − 18(6, 13) AA | 107006.496(22e-3) | 121.8 | 548.83353 | blended | – | – | – |
| $CH_3OH$, vt=0-2 | $3(1)^+$ − $4(0)^+$, vt=0 | 107013.831(1e-2) | 28.3 | 12.036 | 1915 | 67.2(1.1) | 9.0(1.1) | 18348(292) |
| $CH_3{}^{13}CH_2CN$ | 12(4, 9) − 11(4, 8) | 107024.745(2e-3) | 50.7 | 155.341 | 78 | 67.1(1.1) | 9.4(1.1) | 778(292) |
| $CH_3{}^{13}CH_2CN$ | 12(4, 8) − 11(4, 7) | 107029.120(2e-3) | 50.7 | 155.328 | 41 | 67.0(1.1) | 7.8(1.1) | 344(292) |
| aGg'−$(CH_2OH)_2$ | 10(2, 9) v=1 − 9(2, 8) v=0 | 107040.005(2e-3) | 29.0 | 305.75751 | blended | – | – | – |
| $C_2H_5CN$ | 12(2, 11) − 11(2, 10) | 107043.527(5e-2) | 37.9 | 172.86 | 574 | 67.0(1.1) | 9.5(1.1) | 5815(292) |
| $SO_2$ | 27(3, 25) − 26(4, 22) | 107060.208(2e-3) | 369.4 | 8.2723 | 224 | 66.5(1.1) | 11.2(1.1) | 2665(292) |
| aGg'−$(CH_2OH)_2$ | 10(3, 7) v=1 − 9(3, 7) v=1 | 107073.219(1e-3) | 32.0 | 3.03815 | 34 | 65.3(1.1) | 7.8(1.1) | 277(252) |
| $CH_3{}^{13}CH_2CN$ | 12(3, 10) − 11(3, 9) | 107076.464(2e-3) | 43.1 | 163.832 | 16 | 67.0(1.1) | 4.7(1.1) | 79(29) |
| $CH_3OCH_2OH$ | 15(5, 10) − 15(4, 12) A | 107088.892(7e-3) | 74.4 | 0.41998 | 234 | 67.0(1.1) | 6.0(1.1) | 1492(126) |
| $C_2H_5CN$, $v_{20}$=1−A | 12(2, 11) − 11(2, 10) | 107131.971(5e-2) | 574.5 | 169.83 | 74 | 0. | 3.4(1.1) | 270(126) |
| $^{13}CH_3CN$ | 6(5) − 5(5) | 107146.173(0) | 196.9 | 56.399 | 12 | 67.0(1.1) | 2.9(1.1) | 38(12) |
| $CH_3OH$, vt=0-2 | 15(-2) − 15(1) E2, vt=0 | 107159.906(14e-3) | 304.7 | 10.421 | 546 | 67.6(1.1) | 9.9(1.1) | 5727(126) |
| $^{13}CH_3CN$ | 6(4) − 5(4) | 107164.310(0) | 132.5 | 102.548 | 32 | 67.2(1.1) | 2.6(1.1) | 433(126) |
| $^{13}CH_3CN$ | 6(3) − 5(3) | 107178.424(0) | 82.4 | 276.826 | 279 | 67.3(1.1) | 6.9(1.1) | 2047(126) |
| $^{13}CH_3CN$ | 6(2) − 5(2) | 107188.500(1e-1) | 46.6 | 164.068 | 227 | 67.2(1.1) | 6.5(1.1) | 1574(126) |
| $^{13}CH_3CN$ | 6(1) − 5(1) | 107194.550(1e-1) | 25.2 | 179.427 | 308 | 67.0(1.1) | 8.6(1.1) | 2819(126) |
| $^{13}CH_3CN$ | 6(0) − 5(0) | 107196.570(1e-1) | 18.0 | 184.590 | 231 | 67.0(1.1) | 6.7(1.1) | 1638(126) |
| $CH_3COCH_3$ | 11(9, 3) − 10(10, 0) AE | 107225.457(56e-3) | 57.6 | 1.5476 | 36 | 67.0(0.8) | 4.2(1.8) | 164(57) |
| $CH_3{}^{13}CH_2CN$ | 12(3, 9) − 11(3, 8) | 107235.511(2e-3) | 43.2 | 163.806 | 54 | 67.0(0.8) | 4.7(1.1) | 269(57) |
| $CH_3OCH_2OH$ | 18(5, 13) − 18(4, 15) A | 107250.247(7e-3) | 100.0 | 0.47916 | 203 | 67.0(0.2) | 7.9(0.5) | 1706(93) |
| $CH_3OCH_2OH$ | 14(5, 9) − 14(4, 11) A | 107251.507(7e-3) | 66.9 | 0.39439 | blended | – | – | – |
| $CH_3OCH_2OH$ | 14(5, 9) − 14(4, 11) E | 107256.688(11e-3) | 66.9 | 0.35702 | 42 | 67.2(0.7) | 6.8(3.6) | 302(112) |
| $CH_3OCH_2OH$ | 12(5, 8) − 12(4, 8) E | 107288.292(21e-6) | 53.4 | 0.23167 | 27 | 67.0(1.3) | 4.3(2.1) | 123(81) |
| $HOCO^+$ | 5(1, 4) − 4(1, 3) | 107315.356(2e-3) | 52.8 | 34.996 | 42 | 66.7(1.3) | 5.8(2.4) | 257(107) |
| $CH_3OCH_2OH$ | 12(5, 8) − 12(4, 8) A | 107315.268(7e-3) | 53.4 | 0.33693 | blended | – | – | – |
| $CH_3OCH_2OH$ | 12(5, 7) − 12(4, 8) A | 107325.807(7e-3) | 53.4 | 0.15131 | blended | – | – | – |
| $C_2H_5CN$, $v_{12}$=1−A | 12(7, 5) − 11(7, 4) | 107326.120(5e-2) | 857.8 | 115.27 | blended | – | – | – |
| $C_2H_5CN$, $v_{12}$=1−A | 12(6, 6) − 11(6, 5) | 107327.264(2e-3) | 843.1 | 131.05 | 67 | 67.0(0.8) | 5.5(1.9) | 391(113) |
| $C_2H_5CN$, $v_{12}$=1−A | 12(8, 4) − 11(8, 3) | 107333.138(5e-2) | 874.8 | 97.074 | 38 | 67.0(1.5) | 5.9(2.4) | 238(106) |
| $C_2H_5CN$, $v_{12}$=1−A | 12(5, 7) − 11(5, 6) | 107341.894(5e-2) | 830.7 | 144.41 | 136 | 67.2(0.4) | 5.8(1.0) | 845(126) |
| $CH_3OCH_2OH$ | 12(5, 7) − 12(4, 8) E | 107339.848(13e-3) | 53.4 | 0.2566 | blended | – | – | – |
| $C_2H_5CN$, $v_{12}$=1−A | 12(9, 3) − 11(9, 2) | 107345.941(5e-2) | 894.0 | 76.452 | 23 | 67.0(3.0) | 6.2(4.8) | 155(116) |
| $C_2H_5CN$, $v_{12}$=1−A | 12(4, 9) − 11(4, 8) | 107382.151(2e-3) | 820.5 | 155.32 | 61 | 67.0(1.0) | 5.3(2.0) | 341(131) |
| $C_2H_5CN$, $v_{12}$=1−A | 12(11, 1) − 11(11, 0) | 107383.258(3e-3) | 939.1 | 27.905 | blended | – | – | – |
| $C_2H_5CN$, $v_{12}$=1−A | 12(4, 8) − 11(4, 7) | 107385.550(5e-2) | 820.5 | 155.31 | 36 | 66.5(2.2) | 7.1(3.6) | 272(138) |
| $CH_3C_3N$ | 26(3) − 25(3) | 107402.512(3e-3) | 137.0 | 2315.4 | 52 | 66.0(0.6) | 4.3(1.2) | 239(63) |
| $CH_3C_3N$ | 26(2) − 25(2) | 107407.677(4e-3) | 99.5 | 1166.3 | 27 | 66.3(1.4) | 3.9(2.5) | 110(61) |
| $CH_3C_3N$ | 26(1) − 25(1) | 107410.776(4e-3) | 77.1 | 1171.5 | blended | – | – | – |
| $CH_3C_3N$ | 26(0) − 25(0) | 107411.809(4e-3) | 69.6 | 1173.5 | 53 | 66.0(0.6) | 5.4(1.5) | 307(74) |
| $CH_3OCH_2OH$ | 13(5, 9) − 13(4, 10) A | 107419.686(7e-3) | 59.9 | 0.16816 | 165 | 67.0(0.2) | 7.3(0.6) | 1283(87) |
| $C_2H_5CN$, $v_{12}$=1−A | 12(3, 10) − 11(3, 9) | 107432.075(5e-2) | 812.6 | 163.82 | 90 | 67.0(2.2) | 2.7(2.0) | 31(19) |
| $C_2H_5CN$ | 12(7, 5) − 11(7, 4) | 107485.160(5e-2) | 88.0 | 117.36 | blended | – | – | – |
| $C_2H_5CN$ | 12(6, 6) − 11(6, 5) | 107486.949(5e-2) | 73.6 | 133.42 | 698 | 67.0(1.1) | 12.4(1.1) | 9246(296) |
| $C_2H_5CN$ | 12(8, 4) − 11(8, 3) | 107491.574(5e-2) | 104.6 | 98.829 | 459 | 66.8(1.1) | 7.0(1.1) | 3429(296) |
| $C_2H_5CN$ | 12(5, 7) − 11(5, 6) | 107502.432(5e-2) | 61.3 | 146.99 | 720 | 66.7(1.1) | 11.0(1.1) | 8401(296) |
| $C_2H_5CN$ | 12(10, 2) − 11(10, 1) | 107519.861(5e-2) | 144.6 | 54.355 | 416 | 67.0(1.1) | 9.7(1.1) | 4277(296) |
| $CH_3OCHO$ | 9( 2, 8) − 8( 2, 7) E | 107537.258(1e-2) | 28.8 | 22.60702 | 309 | 67.0(1.1) | 16.7(1.1) | 5470(296) |
| $CH_3OCHO$ | 9( 2, 8) − 8( 2, 7) A | 107543.711(1e-2) | 28.8 | 22.61344 | 652 | 67.0(1.1) | 7.2(1.1) | 5008(296) |

**Table A2.** (Continued)

| Species | Transitions | Rest Freq. | $E_u$ | $\mu^2 S$ | $T_{mb}$ | $V_{LSR}$ | $\Delta V$ | $\int T_{mb}\,dv$ |
|---|---|---|---|---|---|---|---|---|
| | | (MHz) | (K) | ($D^2$) | (mK) | (km $s^{-1}$) | (km $s^{-1}$) | (mK km $s^{-1}$) |
| $C_2H_5CN$ | 12(4, 9) − 11(4, 8) | 1107544.042(5e-2) | 51.3 | 158.12 | blended | – | – | – |
| $C_2H_5CN$ | 12(4, 8) − 11(4, 7) | 1107547.460(5e-2) | 51.3 | 158.11 | 522 | 67.2(1.1) | 8.3(1.1) | 4600(296) |
| $C_2H_5CN$, $v_{12}$=1−A | 12(3, 9) − 11(3, 8) | 107567.469(5e-2) | 812.6 | 163.79 | 37 | 67.2(1.1) | 7.2(1.1) | 279(181) |
| $C_2H_5CN$, $v_{20}$=1−A | 12(7, 5) − 11(7, 4) | 107569.684(2e-3) | 624.2 | 115.29 | 118 | 67.1(1.1) | 8.2(1.1) | 1027(181) |
| $C_2H_5CN$, $v_{20}$=1−A | 12(7, 6) − 11(7, 5) | 107569.674(5e-2) | 624.2 | 115.29 | blended | – | – | – |
| $C_2H_5CN$, $v_{20}$=1−A | 12(6, 6) − 11(6, 5) | 107571.583(5e-2) | 609.8 | 131.06 | blended | – | – | – |
| $C_2H_5CN$, $v_{20}$=1−A | 12(6, 7) − 11(6, 6) | 107571.556(2e-3) | 609.8 | 131.06 | blended | – | – | – |
| $C_2H_5CN$, $v_{20}$=1−A | 12(8, 4) − 11(8, 3) | 107575.996(5e-2) | 640.6 | 97.077 | 96 | 67.2(1.1) | 8.5(1.1) | 872(181) |
| $C_2H_5CN$, $v_{20}$=1−A | 12(8, 5) − 11(8, 4) | 107575.909(3e-3) | 640.6 | 97.077 | blended | – | – | – |
| $C_2H_5CN$, $v_{20}$=1−A | 12(5, 7) − 11(5, 6) | 107587.030(2e-3) | 597.7 | 144.42 | 132 | 67.1(1.1) | 10.1(1.1) | 1417(181) |
| $C_2H_5CN$, $v_{20}$=1−A | 12(5, 8) − 11(5, 7) | 107587.007(5e-2) | 597.7 | 144.42 | blended | – | – | – |
| $C_2H_5CN$, $v_{20}$=1−A | 12(9, 3) − 11(9, 2) | 107587.703(3e-3) | 659.3 | 76.448 | blended | – | – | – |
| $C_2H_5CN$ | 12(3, 10) − 11(3, 9) | 107594.056(5e-2) | 43.6 | 166.77 | 547 | 67.0(1.1) | 14.7(1.1) | 8537(181) |
| $CH_3OCHO$ | 23(6, 17) − 23(5, 18) E | 107604.366(1e-2) | 189.0 | 7.68978 | 308 | 67.2(1.1) | 9.7(1.1) | 3184(181) |
| $C_2H_5CN$, $v_{20}$=1−A | 12(10, 2) − 11(10, 1) | 107603.761(3e-3) | 680.2 | 53.387 | blended | – | – | – |
| $C_2H_5CN$, $v_{20}$=1−A | 12(4, 9) − 11(4, 8) | 107628.215(2e-3) | 587.8 | 155.33 | 95 | 67.2(1.1) | 6.7(1.1) | 1072(101) |
| $C_2H_5CN$, $v_{20}$=1−A | 12(4, 8) − 11(4, 7) | 107631.866(2e-3) | 587.8 | 155.31 | 188 | 67.2(1.1) | 7.7(1.1) | 2956(101) |
| $CH_3OCH_2OH$ | 12(5, 7) − 12(4, 9) A | 107636.401(7e-3) | 53.4 | 0.33662 | 241 | 67.0(1.1) | 6.7(1.1) | 1724(101) |
| $C_2H_5CN$, $v_{20}$=1−A | 12(3, 10) − 11(3, 9) | 107677.884(5e-2) | 580.1 | 163.79 | 65 | 67.6(2.6) | 6.8(6.6) | 458(377) |
| $C_2H_5CN$ | 34(3, 31) − 34(2, 32) | 107702.174(5e-2) | 269.4 | 37.448 | 150 | 67.3(1.5) | 11.8(3.4) | 1884(482) |
| $C_2H_5CN$ | 12(3, 9) − 11(3, 8) | 107734.723(5e-2) | 43.6 | 166.76 | 565 | 67.0(0.2) | 9.8(0.3) | 5895(200) |
| $CH_3OCH_2OH$ | 11(5, 7) − 11(4, 8) E | 107782.910(17e-3) | 47.4 | 0.26913 | 77 | 67.0(0.6) | 11.6(1.4) | 956(103) |
| $CH_3COCH_3$ | 16(4, 12) − 16(3, 13) EE | 107797.721(13e-3) | 90.8 | 602.22608 | 21 | 67.0(2.0) | 8.6(3.4) | 193(81) |
| $C_2H_5CN$, $v_{20}$=1−A | 10(5, 6) − 11(4, 7) | 107816.736(103e-3) | 587.8 | 1.4633 | 110 | 67.2(0.3) | 6.0(0.6) | 703(54) |
| $C_2H_5CN$, $v_{20}$=1−A | 12(3, 9) − 11(3, 8) | 107817.517(54e-2) | 580.2 | 163.83 | blended | – | – | – |
| $SO_2$ | 12(4, 8) − 13(3, 11) | 107843.470(2e-3) | 111.0 | 4.5354 | 300 | 67.0(0.) | 9.1(0.5) | 2896(65) |
| $CH_3OCH_2OH$ | 10(5, 6) − 10(4, 6) A | 107889.384(7e-3) | 41.9 | 0.27111 | blended | – | – | – |
| $CH_3OCH_2OH$ | 10(5, 5) − 10(4, 6) A | 107891.030(7e-3) | 41.9 | 0.11731 | 51 | 67.2(0.2) | 4.0(1.0) | 220(53) |
| $CH_3COCH_3$ | 15(7, 8) − 14(10, 5) AE | 107919.101(98e-3) | 93.0 | 4.0077 | 198 | 67.0(0.2) | 8.1(0.4) | 1708(71) |
| $CH_3OCH_2OH$ | 31(4, 27) − 31(3, 28) E | 107986.564(22e-3) | 261.8 | 0.44014 | 86 | 67.4(0.4) | 8.8(1.1) | 802(79) |
| $CH_3OCHO$ | 15(5, 10) − 15(4, 11) E | 108045.959(1e-2) | 87.9 | 4.11041 | 50 | 66.5(1.1) | 1.1(1.1) | 58(24) |
| $CH_3OCHO$ | 15(5, 10) − 15(4, 11) A | 108050.939(1e-2) | 87.9 | 4.11748 | 23 | 66.7(1.1) | 9.5(1.1) | 233(24) |
| $CH_3OH$, vt=0-2 | 18(-1) − 19(-2) E2, vt=1 | 108058.877(31e-3) | 809.1 | 10.162 | 40 | 67.0(1.1) | 7.7(1.1) | 327(24) |
| $OC^{33}S$ | 9 − 8 | 108084.784(2e-3) | 25.9 | 4.605 | 103 | 67.5(1.1) | 5.8(1.1) | 631(24) |
| t-HCOOH | 5(1, 5) − 4(1, 4) | 108126.720(3e-3) | 18.8 | 9.6966 | 87 | 67.6(0.6) | 7.8(1.3) | 726(108) |
| $CH_3COCH_3$ | 15(3, 12) − 15(2,13) EE | 108147.056(13e-3) | 76.7 | 460.37793 | 34 | 66.7(1.5) | 7.1(3.5) | 255(104) |
| $CH_3COCH_3$ | 15(4, 12) − 15(3,13) EE | 108147.057(13e-3) | 76.7 | 460.37792 | blended | – | – | – |
| $C_2H_5CN$, $v_{20}$=1−A | 11(1, 11) − 10(0, 10) | 108187.454(5e-3) | 565.3 | 11.097 | 27 | 67.0(1.8) | 6.6(3.2) | 190(96) |
| $C_2H_5CN$ | 41(11, 30) − 42(10, 33) | 108208.948(5e-2) | 504.5 | 8.8194 | 140 | 67.0(0.3) | 6.6(0.5) | 984(74) |
| $C_2H_5CN$ | 11(1, 11) − 10(0, 10) | 108210.415(5e-2) | 28.6 | 11.009 | 113 | 67.0(0.3) | 6.7(0.6) | 814(73) |
| $CH_3COCH_3$ | 14(2, 12) − 14(1, 13) AE | 108240.911(21e-3) | 63.4 | 39.19411 | 12 | 67.5(1.8) | 2.9(2.3) | 42(38) |
| $CH_3COCH_3$ | 14(2, 12) − 14(1, 13) EA | 108241.031(16e-3) | 63.4 | 78.40068 | blended | – | – | – |
| $CH_3COCH_3$ | 15(3, 12) − 15(2, 13) AA | 108326.033(16e-3) | 76.6 | 287.98169 | 25 | 67.0(0.5) | 2.2(0.5) | 18(12) |
| HCOCN | 5(1, 5) − 4(0, 4) | 108327.496(4e-3) | 9.8 | 17.42519 | blended | – | – | – |
| $CH_3COCH_3$ | 7(4, 3) − 7(1, 6) AA | 108331.398(21e-3) | 22.6 | 0.51266 | 20 | 67.0(1.8) | 7.4(3.3) | 157(59) |
| $CH_3COCH_3$ | 8(3, 5) − 7(4, 4) EA | 108358.421(11e-3) | 26.9 | 130.21505 | 86 | 67.0(0.1) | 3.1(1.1) | 100(27) |
| $CH_3COCH_3$ | 8(3, 5) − 7(4, 4) EE | 108387.595(8e-3) | 88.2 | 519.86714 | 28 | 67.2(1.3) | 6.3(2.4) | 368(75) |
| $CH_3COCH_3$ | 8(3, 5) − 7(4, 4) AA | 108424.565(11e-3) | 26.7 | 194.60833 | 30 | 67.0(1.0) | 4.2(3.1) | 133(66) |
| $CH_3COCH_3$ | 14(2, 12) − 14(1, 13) EE | 108434.511(16e-3) | 63.4 | 313.86255 | 36 | 67.0(1.7) | 7.8(2.7) | 301(117) |
| $C_2H_5OH$ | 13(3, 10) − 13(2, 11) | 108438.579(5e-2) | 88.2 | 18.79 | 119 | 67.0(0.5) | 7.8(1.0) | 984(122) |
| $C_2H_5OH$ | 8(2, 6) − 7(1, 6) | 108624.353(5e-2) | 91.9 | 4.7078 | 31 | 67.0(0.7) | 2.3(1.4) | 77(46) |
| $^{13}CN$ | 1(1, 1) − 0(1, 0), F = 1 − 1 | 108636.923(5e-2) | 5.2 | 1.932 | 38 | 67.0(1.0) | 5.3(1.9) | 217(75) |
| $^{13}CN$ | 1(2, 1) − 0(1, 1), F = 1 − 0 | 108638.212(5e-2) | 5.2 | 0.722 | blended | – | – | – |
| $^{13}CN$ | 1(2, 1) − 0(1, 1), F = 2 − 1 | 108643.590(5e-2) | 5.2 | 0.856 | 32 | 67.1(1.1) | 4.7(2.0) | 158(68) |
| $^{13}CN$ | 1(2, 1) − 0(1, 1), F = 0 − 1 | 108644.346(5e-2) | 5.2 | 0.642 | blended | – | – | – |
| $^{13}CN$ | 1(2, 1) − 0(1, 1), F = 1 − 1 | 108645.064(5e-2) | 5.2 | 0.551 | blended | – | – | – |
| $^{13}CN$ | 1(1, 1) − 0(1, 0), F = 2 − 1 | 108651.297(5e-2) | 5.2 | 3.276 | 49 | 67.1(0.7) | 4.6(1.3) | 240(67) |
| $^{13}CN$ | 1(2, 1) − 0(1, 1), F = 2 − 2 | 108657.646(5e-2) | 5.2 | 2.420 | 56 | 67.0(0.6) | 5.2(1.3) | 306(74) |
| $^{13}CN$ | 1(2, 1) − 0(1, 1), F = 1 − 2 | 108658.948(5e-2) | 5.2 | 0.669 | blended | – | – | – |
| $C_2H_5CN$, $v_{12}$=1−A | 12(2, 10) − 11(2, 9) | 108757.634(5e-2) | 807.1 | 169.86 | 44 | 67.2(1.1) | 3.3(1.1) | 154(112) |
| $^{13}CN$ | 1(2, 2) − 0(1, 1), F = 3 − 2 | 108780.201(5e-2) | 5.2 | 4.905 | 126 | 67.0(1.1) | 6.5(1.1) | 877(112) |
| $^{13}CN$ | 1(2, 2) − 0(1, 1), F = 2 − 1 | 108782.374(5e-2) | 5.2 | 2.586 | 105 | 67.1(1.1) | 1.8(1.1) | 21(12) |
| $^{13}CN$ | 1(2, 2) − 0(1, 1), F = 1 − 0 | 108786.982(5e-2) | 5.2 | 1.144 | 217 | 67.1(1.1) | 8.1(1.1) | 1883(112) |
| $CH_3OH$, vt=0-2 | 0(0) − 1(-1) E2, vt=0 | 108893.945(12e-3) | 13.1 | 3.9134 | 2092 | 67.0(0.) | 7.9(0.1) | 17556(74) |
| SiS | 6(0) − 5(0) | 108924.301(1e-3) | 18.3 | 5.62 | 20 | 68.0(4.3) | 6.5(4.6) | 160(101) |
| $CH_3C_6H$ | 70(4) − 69(4) | 108931.640(575e-3) | 307.2 | 313.98 | 34 | 67.4(2.6) | 4.4(4.1) | 164(160) |
| $C_2H_5CN$ | 12(2, 10) − 11(2, 9) | 108940.554(5e-2) | 38.2 | 172.93 | 611 | 67.0(0.2) | 8.3(0.5) | 5426(252) |
| $C_2H_5CN$ | 11(3, 9) − 12(0, 12) | 108940.696(4e-3) | 38.4 | 0.042598 | blended | – | – | – |
| $SO_2$ | 39(6, 34) − 38(7, 31) | 108955.915(2e-3) | 808.3 | 16.377 | 63 | 67.0(2.1) | 8.7(4.1) | 579(246) |
| $C_2H_5CN$, $v_{20}$=1−A | 12(2, 10) − 11(2, 9) | 109013.350(5e-2) | 574.9 | 169.87 | 61 | 67.0(1.3) | 4.8(2.2) | 310(145) |
| $HC_3N$, $v_4$=1 | 12 − 11 | 109023.305(2e-2) | 1279.6 | 161.07 | 106 | 68.2(0.7) | 4.7(1.3) | 526(148) |
| $CH_3COCH_3$ | 26(13, 13) − 26(12, 14) AE | 109089.772(96e-3) | 275.1 | 229.24048 | 46 | 67.2(1.2) | 4.2(3.3) | 161(146) |
| $CH_3COCH_3$ | 26(13, 13) − 26(12, 14) EA | 109090.636(94e-3) | 275.1 | 458.44205 | blended | – | – | – |
| $C_2H_5{}^{13}CN$ | 12(1, 11) − 11(1, 10) | 109101.845(1e-3) | 35.2 | 173.388 | 466 | 66.0(1.1) | 4.1(1.1) | 527(202) |
| $O^{13}CS$ | 9 − 8 | 109110.845(2e-3) | 26.2 | 4.605 | 229 | 67.0(1.1) | 6.1(1.1) | 1484(527) |
| $CH_3OH$, vt=0-2 | 14(5) − 15(4) E1, vt=0 | 109138.783(15e-3) | 379.7 | 13.593 | 733 | 67.0(1.1) | 10.1(1.1) | 7901(527) |
| $CH_3OH$, vt=0-2 | 16(-2) − 16(1) E2, vt=0 | 109153.184(14e-3) | 342.0 | 14.726 | 760 | 67.0(1.1) | 9.6(1.1) | 7762(527) |
| $HC_5N$ | 41 − 40 | 109160.973(7e-3) | 110.0 | 2306 | 18 | 67.0(1.1) | 7.2(1.1) | 94(52) |
| $HC_3N$ | 12 − 11 | 109173.634(1e-2) | 34.1 | 167.1 | 3403 | 67.0(1.1) | 8.3(1.1) | 30069(527) |
| $HC_3N$, $v_5$=1/$v_7$=3 | 12(-1, 0) − 11(1, 0) | 109183.021(2e-2) | 988.1 | 163.57 | 231 | 67.0(1.1) | 5.9(1.1) | 1457(527) |
| $HC_3N$, $v_5$=1/$v_7$=3 | 12(1, 0) − 11(-1, 0) | 109244.222(2e-2) | 988.1 | 163.55 | 211 | 67.0(0.4) | 6.2(0.7) | 1388(151) |
| SO | 3(2) − 2(1) | 109252.220(1e-1) | 21.1 | 3.5585 | 1532 | 67.0(0.) | 8.5(0.1) | 13851(187) |
| $HC_3N$, $v_6$=1 | 12(-1) − 11(1) | 109352.781(15e-3) | 751.8 | 165.47 | 311 | 67.0(0.5) | 7.3(1.2) | 2429(354) |
| aGg'−$(CH_2OH)_2$ | 10(6, 4) v=1 − 9(6, 3) v=0 | 109357.858(2e-3) | 45.1 | 246.16859 | 22 | 64.2(5.2) | 6.2(1.1) | 267(26) |
| aGg'−$(CH_2OH)_2$ | 10(6, 5) v=1 − 9(6, 4) v=0 | 109357.707(2e-3) | 45.1 | 191.44051 | blended | – | – | – |
| $HC_3N$, $v_6$=1 | 12(1) − 11(-1) | 109438.720(15e-3) | 751.8 | 165.46 | 271 | 67.0(1.1) | 8.9(1.1) | 2557(332) |
| $HC_3N$, $v_7$=1 | 12(-1) − 11(1) | 109442.013(2e-2) | 355.0 | 165.12 | 551 | 67.0(1.1) | 9.2(1.1) | 5369(332) |
| OCS | 9 − 8 | 109463.063(5e-3) | 26.3 | 4.6034 | 1697 | 67.0(1.1) | 9.2(1.1) | 16623(332) |
| HNCO | 5(1, 5) − 4(1, 4) | 109495.996(6e-3) | 59.0 | 11.847 | 560 | 67.0(1.1) | 9.9(1.1) | 5823(332) |
| $CH_3OCH_3$ | 8(2, 7) − 8(1, 8) EA | 109571.396(9e-3) | 38.3 | 23.947 | 101 | 66.8(1.7) | 4.1(3.3) | 441(385) |
| $CH_3OCH_3$ | 8(2, 7) − 8(1, 8) AE | 109571.403(9e-3) | 38.3 | 35.921 | blended | – | – | – |
| $CH_3OCH_3$ | 8(2, 7) − 8(1, 8) EE | 109574.088(7e-3) | 38.3 | 95.791 | 144 | 66.8(3.0) | 6.4(5.6) | 1300(860) |
| $CH_3OCH_3$ | 8(2, 7) − 8(1, 8) AA | 109576.778(11e-3) | 38.3 | 59.869 | 101 | 66.8(5.7) | 7.4(6.5) | 1140(699) |
| $HC_3N$, $v_7$=1 | 12(1) − 11(-1) | 109598.818(2e-2) | 355.0 | 165.12 | 573 | 67.0(0.3) | 6.6(0.6) | 4004(283) |
| $C_2H_5CN$ | 12(1, 11) − 11(1, 10) | 109650.263(5e-2) | 35.4 | 176.49 | 525 | 67.0(0.2) | 6.9(0.4) | 3843(237) |
| $HC_3N$, $v_6$=$v_7$=1 | 12(0, 0) − 11(0, 0) | 109736.687(15e-3) | 1070.5 | 165.77 | 110 | 67.0(0.5) | 5.1(0.5) | 600(303) |
| $HC_3N$, $v_6$=$v_7$=1 | 12(0, 1) − 11(0, 1) | 109740.155(15e-3) | 1071.7 | 165.77 | 106 | 67.0(0.5) | 4.8(0.5) | 543(303) |
| $HC_3N$, $v_6$=$v_7$=1 | 12(-2, 2) − 11(2, 2) | 109749.770(15e-3) | 1071.9 | 161.19 | 141 | 67.0(0.5) | 5.7(0.5) | 857(303) |
| $HC_3N$, $v_6$=$v_7$=1 | 12(2, 2) − 11(2, -2) | 109752.612(15e-3) | 1071.9 | 161.18 | blended | – | – | – |
| $NH_2CHO$ | 5(1, 4) − 4(1, 3) | 109753.549(25e-3) | 18.8 | 62.756 | 460 | 67.3(0.5) | 8.9(0.5) | 4351(303) |
| $SO_2$ | 17(5, 13) − 18(4, 14) | 109757.585(2e-3) | 202.1 | 6.6069 | 144 | 67.0(0.5) | 6.5(0.5) | 997(303) |
| $C^{18}O$ | 1 − 0 | 109782.173(6e-3) | 5.3 | 0.01221 | 4052 | 67.2(0.5) | 6.4(0.5) | 27535(303) |

**Table A2.** (Continued)

| Species | Transitions | Rest Freq. (MHz) | $E_u$ (K) | $\mu^2S$ ($D^2$) | $T_{mb}$ (mK) | $V_{LSR}$ (km $s^{-1}$) | $\Delta V$ (km $s^{-1}$) | $\int T_{mb}$ dv (mK km $s^{-1}$) |
|---|---|---|---|---|---|---|---|---|
| HNCO | 5(3, 2) − 4(3, 1) | 109833.487(7e-3) | 390.8 | 7.1906 | 240 | 67.0(0.5) | 6.1(0.5) | 1558(135) |
| $CH_3{}^{13}CH_2CN$ | 5(2, 4) − 4(1, 3) | 109843.903(1e-3) | 10.7 | 3.230 | 143 | 67.2(0.5) | 4.8(0.5) | 725(135) |
| $HC_3N$, $v_7$=2 | 12(0) − 11(0) | 109862.778(2e-3) | 676.0 | 165.5 | 261 | 67.0(0.5) | 6.3(0.5) | 1755(135) |
| $HC_3N$, $v_7$=2 | 12(-2) − 11(2) | 109865.961(2e-3) | 679.2 | 160.92 | 203 | 67.0(0.5) | 10.1(0.5) | 2189(135) |
| $HC_3N$, $v_7$=2 | 12(2) − 11(-2) | 109870.290(2e-3) | 679.2 | 160.91 | 181 | 67.0(0.5) | 5.7(0.5) | 1104(135) |
| HNCO | 5(2, 3) − 4(2, 2) | 109872.765(3e-2) | 186.1 | 10.012 | 398 | 67.0(0.5) | 9.3(0.5) | 3939(135) |
| HNCO | 5(2, 4) − 4(2, 3) | 109872.337(3e-2) | 186.1 | 10.013 | blended | – | – | – |
| HNCO | 5(0, 5) − 4(0, 4) | 109905.749(7e-3) | 15.8 | 12.482 | 1552 | 67.1(0.5) | 7.2(0.5) | 11832(135) |
| $C_2H_5CN$ | 22(1, 21) − 22(1, 22) | 109958.637(5e-2) | 111.4 | 1.7932 | 140 | 67.3(0.9) | 4.9(1.7) | 737(261) |
| $CH_3OCHO$ | 9(4, 6) − 8(4, 5) | 110035.269(1e-2) | 224.9 | 19.15 | 46 | 66.8(2.3) | 4.0(3.1) | 201(195) |
| $CH_3OCHO$ | 9(6, 4) − 8(6, 3) | 110050.332(1e-2) | 237.4 | 13.33 | 159 | 66.8(0.8) | 5.2(1.3) | 879(236) |
| $CH_3COCH_3$ | 9(3, 7) − 8(2, 6) AE | 110167.953(9e-2) | 29.9 | 104.0968 | 164 | 67.0(0.5) | 1.8(0.5) | 320(40) |
| $CH_3COCH_3$ | 9(2, 7) − 8(3, 6) EE | 110189.151(7e-3) | 29.9 | 832.21118 | 97 | 67.0(0.5) | 2.9(0.5) | 298(40) |
| $^{13}CO$ | 1 − 0 | 110201.35(0) | 5.3 | 0.01220 | 17968 | 66.5(0.5) | 7.5(0.5) | 144080(1400) |
| $CH_3COCH_3$ | 9(3, 7) − 8(2, 6) EE | 110208.703(7e-3) | 29.9 | 832.29803 | 186 | 67.5(1.2) | 2.1(1.8) | 418(334) |
| $CH_3COCH_3$ | 9(2, 7) − 8(3, 6) AA | 110229.230(11e-3) | 29.8 | 519.85325 | 79 | 67.4(2.8) | 3.8(3.5) | 398(319) |
| $CH_3COCH_3$ | 9(3, 7) − 8(2, 6) AA | 110249.386(11e-3) | 29.8 | 311.90432 | 58 | 67.5(2.1) | 0.9(0.7) | 42(23) |
| HNCO | 5(1, 4) − 4(1, 3) | 110298.089(5e-3) | 59.2 | 11.847 | 511 | 67.0(0.5) | 9.7(0.5) | 5291(241) |
| $CH_3{}^{13}CN$ | 6(4) − 5(4) | 110295.019(0.) | 132.8 | 102.537 | blended | – | – | – |
| $CH_3{}^{13}CN$ | 6(3) − 5(3) | 110309.800(1e-1) | 82.8 | 276.874 | 247 | 67.2(0.5) | 6.3(0.5) | 1643(241) |
| $CH_3{}^{13}CN$ | 6(2) − 5(2) | 110320.400(1e-1) | 47.1 | 164.054 | 227 | 67.1(0.5) | 5.0(0.5) | 1198(241) |
| $CH_3{}^{13}CN$ | 6(1) − 5(1) | 110326.770(1e-1) | 25.7 | 179.434 | 251 | 67.1(0.5) | 6.8(0.5) | 1812(241) |
| $CH_3{}^{13}CN$ | 6(0) − 5(0) | 110328.870(1e-1) | 18.5 | 184.563 | blended | – | – | – |
| $CH_3CN$ | 6(5, 0) − 5(5, 0) | 110330.345(0) | 197.1 | 56.399 | 668 | 67.3(0.5) | 9.9(0.5) | 7043(241) |
| $CH_3CN$ | 6(4, 0) − 5(4, 0) | 110349.471(0) | 132.8 | 102.54 | 937 | 67.3(0.5) | 9.2(0.5) | 9131(241) |
| $CH_3CN$ | 6(3, 0) − 5(-3, 0) | 110364.354(0) | 82.8 | 138.45 | 1317 | 67.3(0.5) | 10.4(0.5) | 14545(241) |
| $CH_3CN$ | 6(-3, 0) − 5(3, 0) | 110364.354(0) | 82.8 | 138.45 | blended | – | – | – |
| $CH_3CN$ | 6(2, 0) − 5(2, 0) | 1103749.89(0) | 47.1 | 164.06 | 1343 | 67.3(0.5) | 9.6(0.5) | 13788(241) |
| $CH_3CN$ | 6(1, 0) − 5(1, 0) | 110381.372(0) | 25.7 | 179.45 | 1310 | 67.3(0.5) | 7.9(0.5) | 11007(241) |
| $CH_3CN$ | 6(0, 0) − 5(0, 0) | 110383.500(0) | 18.5 | 184.58 | 1562 | 67.3(0.5) | 8.6(0.5) | 14259(241) |
| $CH_3OCHO$ | 9(8, 1) − 8(8, 0) E | 110447.180(1e-2) | 69.0 | 5.02983 | 32 | 67.0(3.7) | 6.4(5.2) | 216(208) |
| $C_2H_5OH$ | 21(3, 18) − 21(2, 19) | 110452.276(5e-2) | 208.7 | 35.016 | 42 | 67.3(5.3) | 8.4(7.7) | 401(341) |
| $CH_3OCHO$ | 9(8, 1) − 8(8, 0) A | 110455.372(1e-2) | 69.0 | 5.02998 | 81 | 67.0(2.1) | 6.3(5.3) | 460(457) |
| $CH_3OCHO$ | 9(8, 2) − 8(8, 1) E | 110458.014(1e-2) | 69.0 | 5.02965 | 48 | 67.0(2.0) | 3.0(2.8) | 178(153) |
| $CH_3OCHO$ | 9(7, 2) − 8(7, 1) E | 110525.741(1e-2) | 59.1 | 9.46492 | blended | – | – | – |
| $CH_3OCHO$ | 7(2, 6) − 6(1, 5) | 110526.190(1e-2) | 206.7 | 1.42 | 57 | 67.0(2.2) | 4.7(3.2) | 285(224) |
| $CH_3OCHO$ | 9(7, 2) − 8(7, 1) A | 110535.186(1e-2) | 59.1 | 9.561 | 238 | 67.0(0.6) | 7.7(1.4) | 1962(317) |
| $CH_3OCHO$ | 9(7, 3) − 8(7, 2) E | 110536.003(1e-2) | 59.1 | 9.46692 | blended | – | – | – |
| $C_2H_5OH$ | 7(2, 6) − 6(1, 6) | 110545.866(5e-2) | 84.9 | 1.3914 | 94 | 67.0(1.3) | 5.8(2.6) | 579(261) |
| $CH_3OCHO$ | 9(2, 6) − 8(1, 5) E | 110550.203(1e-2) | 19.0 | 1.39763 | 99 | 67.0(1.1) | 5.4(2.9) | 577(267) |
| $CH_3OCHO$ | 9(2, 6) − 8(1, 5) A | 110560.051(1e-2) | 19.0 | 1.39665 | 93 | 67.0(1.4) | 5.5(3.1) | 542(269) |
| $CH_3OCHO$ | 10(0,10) − 9(0, 9) | 110571.632(1e-2) | 217.9 | 26.10 | 49 | 67.0(2.7) | 5.5(4.1) | 291(248) |
| $CH_3CN$, $v_8$=1 | 6(-1, 3) − 5(1, 3) | 110609.594(6e-2) | 537.6 | 177.77 | 405 | 67.0(0.7) | 8.1(1.5) | 3502(589) |
| $CH_3CN$, $v_8$=1 | 6(5, 2) − 5(-5, 2) | 110637.052(1e-3) | 788.7 | 55.873 | 161 | 67.0(1.7) | 6.6(3.4) | 1139(540) |
| $CH_3OCHO$ | 9(6, 3) − 8(6, 2) E | 110652.813(1e-2) | 50.5 | 13.30853 | 165 | 67.0(2.8) | 5.6(5.3) | 1030(937) |
| $CH_3OCHO$ | 10(0,10) − 9(0, 9) E | 110655.310(1e-2) | 217.2 | 26.25577 | 148 | 67.0(2.7) | 5.2(4.0) | 922(629) |
| $CH_3OCHO$ | 9(6, 4) − 8(6, 3) E | 110662.315(1e-2) | 50.4 | 13.30855 | 389 | 67.0(0.8) | 11.8(1.9) | 4904(725) |
| $CH_3OCHO$ | 9(6, 3) − 8(6, 2) A | 110663.429(1e-2) | 50.4 | 13.31127 | blended | – | – | – |
| $CH_3OCHO$ | 9(6, 4) − 8(6, 3) A | 110663.273(1e-2) | 50.4 | 13.3113 | blended | – | – | – |
| $CH_3CN$, $v_8$=1 | 6(3, 1) − 5(3, 1) | 110680.294(7e-3) | 647.9 | 128.72357 | 265 | 67.0(1.8) | 9.2(4.1) | 2583(1050) |
| $CH_3CN$ $v_8$=1 | 6(3, 2) − 5(3, 2) | 110683.963(1e-3) | 655.7 | 55.87 | blended | – | – | – |
| $CH_3OCHO$ | 9(4, 6) − 8(4, 5) | 110684.123(1e-2) | 224.1 | 19.21 | 184 | 67.0(2.3) | 6.7(4.4) | 1309(928) |
| $CH_3CN$, $v_8$=1 | 6(2, 2) − 5(-2, 2) | 110695.592(6e-2) | 598.9 | 162.55 | 458 | 67.0(1.3) | 9.0(2.6) | 4376(1310) |
| $CH_3CN$, $v_8$=1 | 6(4, 3) − 5(-4, 3) | 110698.726(1e-3) | 604.8 | 101.58 | 369 | 67.0(1.4) | 6.9(2.7) | 2692(1260) |
| $CH_3CN$, $v_8$=1 | 6(1, 2) − 5(1, 2) | 110706.340(6e-2) | 564.2 | 177.77 | 154 | 67.0(1.1) | 9.6(1.1) | 1564(165) |
| $CH_3CN$, $v_8$=1 | 6(3, 3) − 5(3, 3) | 110709.3541(e-3) | 568.1 | 137.14 | 195 | 67.0(1.1) | 15.2(1.1) | 3160(165) |
| $CH_3CN$, $v_8$=1 | 6(0, 2) − 5(0, 2) | 110712.220(6e-2) | 543.8 | 182.85 | 406 | 67.0(1.1) | 13.8(1.1) | 5957(165) |
| $CH_3CN$, $v_8$=1 | 6(2, 3) − 5(2, 3) | 110716.278(6e-2) | 545.7 | 162.51 | 348 | 0. | 8.8(1.1) | 3250(165) |
| $CH_3OCHO$ | 9(1, 8) − 8(1, 7) | 110776.499(1e-2) | 215.7 | 23.14 | 91 | 67.0(1.1) | 4.0(1.1) | 163(39) |
| $CH_3OCHO$ | 10(1, 10) − 9(1, 9) E | 110788.664(1e-2) | 30.3 | 26.16584 | 302 | 67.3(1.1) | 7.5(1.1) | 2416(165) |
| $CH_3OCHO$ | 10(1, 10) − 9(1, 9) A | 110790.526(1e-2) | 30.3 | 26.17539 | 330 | 67.0(1.1) | 7.6(1.1) | 2665(165) |
| $CH_3CN$, $v_8$=1 | 6(1, 3) − 5(-1, 3) | 110823.126(6e-2) | 537.6 | 177.8 | 394 | 67.0(1.1) | 7.7 (1.1) | 3233(126) |
| $C_2H_3CN$ | 12(1, 12) − 11(1, 11) | 110839.968(1e-3) | 36.8 | 520.3 | 379 | 66.8(1.1) | 7.3(1.1) | 2959(126) |
| $CH_3OCHO$ | 9(5, 4) − 8(5, 3) E | 110873.955(1e-2) | 43.2 | 16.55557 | 132 | 67.0(1.1) | 4.9(1.1) | 686(126) |
| $CH_3OCHO$ | 9(3, 7) − 8(3, 6) E | 110879.766(1e-2) | 32.6 | 21.245 | 361 | 67.0(1.1) | 5.8(1.1) | 2244(126) |
| $CH_3OCHO$ | 9(5, 5) − 8(5, 4) A | 110880.447(1e-2) | 43.2 | 16.56015 | 287 | 67.0(1.1) | 6.5(1.1) | 1982(126) |
| $CH_3OCHO$ | 9(3, 7) − 8(3, 6) A | 110887.092(1e-2) | 32.6 | 21.25577 | 191 | 67.0(1.1) | 8.7(1.1) | 1768(126) |
| $CH_3OCHO$ | 9(5, 4) − 8(5, 3) A | 110890.256(1e-2) | 43.2 | 16.56106 | 156 | 67.0(1.1) | 7.2(1.1) | 1202(126) |
| $^{13}CH_2CHCN$ | 12(5, 7) − 11(5, 6) | 110912.201(1e-3) | 88.0 | 144.33238 | 30 | 67.0(1.1) | 3.9(1.1) | 125(45) |
| $^{13}CH_2CHCN$ | 12(4, 8) − 11(4, 7) | 110917.148(1e-3) | 68.8 | 155.24511 | 48 | 67.0(1.1) | 3.4(1.1) | 170(45) |
| $^{13}CH_2CHCN$ | 12(6, 6) − 11(6, 5) | 110922.659(1e-3) | 111.5 | 130.98788 | 46 | 67.1(1.1) | 4.4(1.1) | 215(45) |
| $^{13}CH_2CHCN$ | 12(3, 10) − 11(3, 9) | 110942.272(1e-3) | 53.8 | 163.74880 | 52 | 67.0(1.1) | 2.2(1.1) | 122(45) |
| $CH_3OCHO$ | 15(4, 12) − 15(3, 13) A | 110.962153(1e-2) | 81.8 | 3.66282 | 62 | 67.0(1.1) | 5.5(1.1) | 364(45) |
| $^{13}CH_2CHCN$ | 12(3, 9) − 11(3, 8) | 110972.080(1e-3) | 53.8 | 163.73780 | 67 | 66.8(1.1) | 4.2(1.1) | 299(45) |
| $CH_3COCH_3$ | 8(4, 4) − 7(5, 3) EE | 110.987131(16e-3) | 28.5 | 273.48458 | 56 | 67.2(1.1) | 2.2(1.1) | 133(45) |
| $CH_3OCHO$ | 10(0, 10) − 9(0, 9) E | 111169.903(1e-2) | 30.2 | 26.18776 | 276 | 67.0(1.1) | 5.8(1.1) | 1710(192) |
| $CH_3OCHO$ | 10(0, 10) − 9(0, 9) A | 111171.634(1e-2) | 30.2 | 26.19136 | 402 | 67.0(1.1) | 7.2(1.1) | 3072(192) |
| $CH_3OCHO$ | 9(4, 6) − 8(4, 5) A | 111195.962(1e-2) | 37.2 | 19.21722 | 201 | 67.0(1.1) | 9.1(1.1) | 1932(192) |
| $CH_3OCHO$ | 9(4, 6) − 8(4, 5) E | 111223.491(1e-2) | 37.2 | 18.18412 | 215 | 67.0(1.1) | 8.8(1.1) | 2017(192) |
| $CH_3COCH_3$ | 10(1, 9) − 9(2, 8) AE | 111243.339(11e-3) | 32.2 | 141.0573 | 104 | 67.2(1.1) | 7.3(1.1) | 802(192) |
| $CH_3COCH_3$ | 10(2, 9) − 9(1, 8) AE | 111243.388(11e-3) | 32.2 | 423.15082 | blended | – | – | – |
| $CH_3COCH_3$ | 10(1, 9) − 9(2, 8) EA | 111243.424(1e-2) | 32.2 | 282.09469 | blended | – | – | – |
| $CH_3COCH_3$ | 10(2, 9) − 9(1, 8) EA | 111243.472(1e-2) | 32.2 | 282.09445 | blended | – | – | – |
| $CH_3COCH_3$ | 10(1, 9) − 9(2, 8) EE | 111267.514(8e-2) | 32.1 | 1128.14194 | 112 | 67.2(1.1) | 6.6(1.1) | 784(192) |
| $CH_3COCH_3$ | 10(2, 9) − 9(1, 8) EE | 111267.565(8e-2) | 32.1 | 1128.14091 | blended | – | – | – |
| $C_2H_5OH$ | 17(3, 15) − 16(4, 12) | 111287.163(5e-2) | 140.0 | 4.9131 | blended | – | – | – |
| $CH_3OH$, vt=0-2 | $7(2)^+ - 8(1)^+$, vt=0 | 111289.453(13e-3) | 102.7 | 9.3425 | 1156 | 67.0(1.1) | 10.3(1.1) | 12738(192) |
| $CH_3COCH_3$ | 10(1, 9) − 9(2, 8) AA | 111291.573(12e-3) | 32.0 | 422.99289 | blended | – | – | – |
| $CH_3COCH_3$ | 10(2, 9) − 9(1, 8) AA | 111291.626(12e-3) | 32.0 | 704.90836 | blended | – | – | – |
| $C_2H_5CN$ | 12(3, 9) − 12(2, 10) | 111315.870(5e-2) | 43.6 | 9.9237 | 132 | 66.8(1.1) | 5.3(1.1) | 750(52) |
| $CH_3OCHO$ | 13(1, 12) − 13(1, 13) E | 111322.939(1e-2) | 54.6 | 0.76596 | 51 | 67.0(1.1) | 1.9(1.1) | 102(52) |
| $C_2H_5OH$ | 7(1, 7) − 7(0, 7) | 111344.327(5e-2) | 85.3 | 9.6676 | 80 | 67.0(1.1) | 8.7(1.1) | 747(52) |
| $CH_3OCHO$ | 9(4, 5) − 8(4, 4) E | 111408.412(1e-2) | 37.3 | 18.18767 | 208 | 67.0(0.4) | 7.6(0.8) | 1673(159) |
| $CH_3OCHO$ | 9(4, 5) − 8(4, 4) A | 111453.300(1e-2) | 37.2 | 19.21778 | 207 | 67.0(0.4) | 7.2(0.8) | 1595(159) |
| $CH_3COOH$, vt=0 | 10(0, 10) − 9(1, 9) E | 111507.280(1e-3) | 31.0 | 20.80201 | 15 | 67.0(1.1) | 1.2(1.1) | 41(19) |
| $CH_3COOH$, vt=0 | 10(0, 10) A1 − 9(1, 9) A2 | 111548.535(1e-3) | 30.5 | 20.40186 | 23 | 67.0(1.1) | 4.9(1.1) | 123(41) |
| $CH_3COOH$, vt=0 | 10(0, 10) A1 − 9(0, 9) A2 | 111548.536(1e-3) | 30.5 | 6.98023 | blended | – | – | – |
| $C_2H_5CN$ | 22(1, 21) − 22(0, 22) | 111574.577(5e-2) | 111.4 | 10.802 | 91 | 67.0(1.1) | 7.9(1.1) | 764(41) |
| aGg'−$(CH_2OH)_2$ | 11(1, 11) v=1 − 10(1, 10) v=0 | 111579.436(2e-3) | 31.2 | 413.2757 | 83 | 67.2(1.1) | 7.3(1.1) | 646(41) |
| $CH_3OH$, vt=0-2 | 17(-2) − 17(1) E2, vt=0 | 111626.514(15e-3) | 381.5 | 20.231 | 731 | 67.0(1.1) | 10.3(1.1) | 8053(144) |
| $CH_3OCHO$ | 9(1, 8) − 8(1, 7) E | 111674.131(1e-2) | 28.1 | 23.18984 | 285 | 67.0(1.1) | 8.6(1.1) | 2598(144) |
| $CH_3OCHO$ | 9(1, 8) − 8(1, 7) A | 111682.189(1e-2) | 28.1 | 23.19587 | 323 | 67.0(1.1) | 8.6(1.1) | 2955(144) |

**Table A2.** (Continued)

| Species | Transitions | Rest Freq. (MHz) | $E_u$ (K) | $\mu^2S$ ($D^2$) | $T_{mb}$ (mK) | $V_{LSR}$ (km $s^{-1}$) | ΔV (km $s^{-1}$) | $\int T_{mb}$ dv (mK km $s^{-1}$) |
|---|---|---|---|---|---|---|---|---|
| $CH_3OCHO$ | 9(4, 5) − 8(4, 5) E | 111713.138(14-2) | 37.3 | 1.02682 | 81 | 67.0(1.3) | 5.3(2.7) | 455(221) |
| $CH_3OCHO$ | 10(1, 10) − 9(0, 9) A | 111735.307(1e-2) | 30.3 | 3.84224 | 64 | 67.0(0.8) | 1.6(1.4) | 111(102) |
| $CH_3OCH_3$ | 19(3,16) − 19(2,17) AE | 111741.351(26e-3) | 187.5 | 123.39211 | blended | – | – | – |
| $CH_3OCH_3$ | 19(3,16) − 19(2,17) EE | 111742.794(25e-3) | 187.5 | 329.06069 | blended | – | – | – |
| $CH_3OCH_3$ | 19(3, 16) − 19(2, 17) AA | 111744.238(29e-3) | 187.5 | 205.6671 | 369 | 67.0(0.3) | 13.1(0.9) | 5132(320) |
| $CH_3OCH_3$ | 7(0, 7) − 6(1, 6) AA | 111782.562(8e-3) | 25.2 | 53.86755 | 542 | 67.0(0.2) | 8.7(0.5) | 5028(259) |
| $CH_3OCH_3$ | 7(0, 7) − 6(1, 6) EE | 111783.010(4e-3) | 25.3 | 86.2034 | blended | – | – | – |
| $CH_3OCH_3$ | 7(0, 7) − 6(1, 6) EA | 111783.647(7e-3) | 25.3 | 21.54865 | blended | – | – | – |
| $CH_3OCH_3$ | 7(0, 7) − 6(1, 6) AE | 111783.648(7e-3) | 25.3 | 32.32363 | blended | – | – | – |
| $CH_3OCH_3$ | 7(5, 2) − 8(4, 5) EE | 111812.674(31e-3) | 60.6 | 0.47164 | 219 | 67.0(0.5) | 8.3(0.5) | 1923(39) |
| $CH_3OCH_3$ | 18(3, 15) − 18(2, 16) EE | 111813.668(21e-3) | 115.4 | 386.29 | 172 | 67.0(0.5) | 6.3(0.5) | 1159(39) |
| $CH_3OCH_3$ | 18(3, 15) − 18(2, 16) AA | 111815.291(25e-3) | 168.9 | 144.84 | 164 | 67.0(0.5) | 4.2(0.5) | 729(39) |
| $C_2H_5CN$ | 17(2, 16) − 17(0, 17) | 111840.320(5e-2) | 69.9 | 1.2004 | 38 | 67.0(0.5) | 1.5(0.5) | 59(39) |
| $C_2H_5CN$ | 5(2, 4) − 4(1, 3) | 111910.806(5e-2) | 10.9 | 3.2027 | 86 | 67.0(0.5) | 1.7(1.2) | 159(87) |
| $C_2H_5CN$ | 18(2, 17) − 18(1, 18) | 111943.850(18e-2) | 77.6 | 9.5377 | 67 | 67.0(0.8) | 2.7(1.9) | 189(105) |
| $C_2H_5OH$ | 12(3, 9) − 12(2, 10) | 112129.544(5e-2) | 77.1 | 16.463 | 125 | 67.0(0.5) | 7.9(1.1) | 1056(135) |
| $CH_3OH$, vt=0-2 | 19(0)$^+$ − 18(2)$^+$, vt=0 | 112145.638(21e-3) | 440.1 | 0.00059 | 289 | 67.0(0.2) | 8.7(0.5) | 2667(140) |
| $CH_3CHO$ | 6(1, 6) − 5(1, 5) A, vt=0 | 112248.716(3e-3) | 21.1 | 73.76807 | 204 | 66.8(0.3) | 5.8(0.6) | 1273(122) |
| $CH_3CHO$ | 6(1, 6) − 5(1, 5) E, vt=0 | 112254.508(3e-3) | 21.2 | 73.79585 | 237 | 66.8(0.3) | 7.1(0.6) | 1788(139) |
| $CH_3OCHO$ | 9(3, 6) − 8(3, 5) | 112306.941(1e-2) | 220.5 | 21.20 | 76 | 67.0(0.6) | 5.2(1.2) | 422(83) |
| $C^{17}O$ | 1 − 0 | 112359.284(1e-3) | 5.4 | 0.01217 | 1078 | 67.0(0.1) | 7.1(0.1) | 8140(129) |
| $CH_3OCH_3$ | 15(2, 14) − 14(3, 11) AA | 112371.536(23e-3) | 114.1 | 17.316 | 279 | 67.2(0.2) | 11.4(0.6) | 3394(159) |
| t-HCOOH | 5(4, 2) − 4(4, 1) | 112432.292(3e-3) | 67.1 | 3.6372 | blended | – | – | – |
| t-HCOOH | 5(4, 1) − 4(4, 0) | 112432.319(3e-3) | 67.1 | 3.6372 | 75 | 67.0(0.7) | 7.1(1.2) | 565(108) |
| t-HCOOH | 5(3, 3) − 4(3, 2) | 112459.621(3e-3) | 44.8 | 6.4662 | 41 | 67.0(1.2) | 6.5(2.0) | 282(99) |
| t-HCOOH | 5(3, 2) − 4(3, 1) | 112467.007(3e-3) | 44.8 | 6.4654 | 24 | 67.0(1.1) | 1.9(1.9) | 50(48) |
| $CH_3OH$, vt=0-2 | 14(-3) − 15(2) E2, vt=0 | 112491.019(15e-3) | 306.4 | 0.28629 | 70 | 67.0(0.6) | 5.9(1.9) | 436(114) |
| $C_2H_5OH$ | 6(5, 2) − 7(4, 3) | 112523.049(5e-2) | 49.0 | 0.46766 | 99 | 67.0(0.5) | 5.4(0.8) | 571(93) |
| $C_2H_5CN$ | 13(1, 13) − 12(1, 12) | 112646.350(9e-2) | 39.0 | 191.45 | 671 | 67.0(0.1) | 8.4(0.2) | 5985(161) |
| $C_2H_5OH$ | 11(3, 9) − 10(4, 7) | 112746.252(5e-2) | 127.5 | 1.5782 | 65 | 67.0(0.5) | 1.2(0.8) | 81(59) |
| $C_2H_5OH$ | 2(2, 1) − 1(1, 0) | 112807.174(5e-2) | 7.5 | 3.2057 | 148 | 67.0(0.4) | 5.3(0.7) | 835(108) |
| $CH_3COCH_3$ | 31(23, 8) − 31(22, 9) EA | 112831.952(869e-3) | 421.0 | 406.1517 | 259 | 67.2(0.2) | 6.3(0.5) | 1725(119) |
| $CH_3COCH_3$ | 25(21, 5) − 25(20, 6) EE | 112839.702(145e-3) | 288.2 | 1174.28124 | 413 | 67.2(0.) | 8.5(0.4) | 3748(141) |
| t-HCOOH | 5(2, 3) − 4(2, 2) | 112891.443 (3e-3) | 28.9 | 8.4849 | 55 | 67.0(1.1) | 7.2(1.7) | 419(118) |
| $CH_3COCH_3$ | 23(10, 13) − 23(9, 14) AA | 112906.952(5e-3) | 209.3 | 889.30162 | 53 | 67.0(2.1) | 7.3(3.9) | 411(209) |
| $C_2H_5CN$ | 35(3, 32) − 35(2, 33) | 112985.628(5e-2) | 284.7 | 37.256 | 93 | 67.0(0.8) | 4.8(1.4) | 474(149) |
| $CH_3OCH_3$ | 20(3, 17) − 20(2, 18) EE | 113000.970(32e-3) | 206.1 | 348.88725 | blended | – | – | – |
| $CH_3OCH_3$ | 20(3, 17) − 20(2, 18) AA | 113002.265(34e-3) | 206.1 | 130.85038 | 176 | 67.0(0.5) | 9.8(0.5) | 1844(58) |
| $C_2H_3CN$ | 8(1, 8) − 7(0, 7) | 113030.746(1e-3) | 18.1 | 11.358 | 237 | 67.0(0.5) | 7.7(0.5) | 1947(58) |
| $CH_3OCH_3$ | 17(3, 14) − 17(2, 15) EA | 113057.427(19e-3) | 153.1 | 132.79 | 170 | 67.2(0.5) | 5.6(0.5) | 1010(58) |
| $CH_3OCH_3$ | 17(3, 14) − 17(2, 15) AE | 113057.425(18e-3) | 153.1 | 88.525 | blended | – | – | – |
| $CH_3OCH_3$ | 17(3, 14) − 17(2, 15) EE | 113059.249(17e-3) | 153.1 | 354.12 | 178 | 67.2(0.5) | 5.3(0.5) | 1013(58) |
| $CH_3OCH_3$ | 17(3, 14) − 17(2, 15) AA | 113061.072(22e-3) | 153.1 | 221.33 | 304 | 67.4(0.5) | 5.7(0.5) | 1842(58) |
| $^{13}CH_3CH_2CN$ | 13(2, 12) − 12(2, 11) | 113090.130(2e-3) | 42.5 | 184.75604 | 273 | 67.0(0.5) | 6.2(0.5) | 1788(58) |
| $C_2H_5OH$ | 10(2, 9) − 12(1, 10) | 113098.078(5e-2) | 51.0 | 8.3566 | 98 | 67.0(0.5) | 5.5(0.5) | 573(58) |
| CN | N= 1-0, J=1/2-1/2, F=1/2-3/2 | 113144.157(6e-3) | 5.4 | 1.2492 | 1046 | 66.7(0.5) | 7.6(0.5) | 8487(164) |
| CN | N= 1-0, J=1/2-1/2, F=3/2-1/2 | 113170.492(4e-3) | 5.4 | 1.2199 | 1432 | 66.7(0.5) | 7.4(0.5) | 11351(164) |
| CN | N= 1-0, J=1/2-1/2, F=3/2-3/2 | 113191.279(3e-3) | 5.4 | 1.5836 | 1231 | 66.7(0.5) | 7.7(0.5) | 10076(164) |
| $CH_3{}^{13}CH_2CN$ | 13(0, 13) − 12(0, 12) | 113255.654(2e-3) | 38.4 | 188.67329 | 75 | 67.0(0.5) | 3.2(0.1) | 257(77) |
| $C_2H_3CN$ | 20(2, 18) − 20(1, 19) | 113266.675(0) | 105.1 | 38.549 | 79 | 67.0(0.4) | 2.7(0.9) | 231(72) |
| $CH_3OCH_3$ | 10(6, 4) − 11(5, 6) EA | 113271.840(102e-3) | 100.7 | 3.71153 | 39 | 67.0(0.9) | 3.0(1.5) | 126(69) |
| $C_2H_3CN$ | 82(7, 76) − 81(8, 73) | 113383.287(30e-3) | 2151.2 | 11.78784 | 140 | 67.0(0.7) | 9.3(1.7) | 1395(189) |
| CCS | 9(8) − 8(7) | 113410.186(2e-2) | 33.6 | 65.427 | 146 | 67.0(0.9) | 7.1(1.7) | 2197(241) |
| $C_2H_5{}^{13}CN$ | 13(0, 13) − 12(0, 12) | 113432.857(1e-3) | 38.4 | 188.71059 | 115 | 66.0(0.7) | 6.8(1.3) | 832(166) |
| CN | N= 1-0, J=3/2-1/2, F=3/2-1/2 | 113488.120(3e-3) | 5.4 | 1.5838 | 1944 | 66.7(0.2) | 6.1(0.2) | 25355(641) |
| CN | N= 1-0, J=3/2-1/2, F=5/2-3/2 | 113490.970(2e-3) | 5.4 | 4.205 | 2139 | 66.7(0.) | 5.4(0.1) | 12277(568) |
| CN | N= 1-0, J=3/2-1/2, F=1/2-1/2 | 113499.644(3e-3) | 5.4 | 1.2491 | 356 | 66.7(0.2) | 9.2(0.4) | 3477(165) |
| CN | N= 1-0, J=3/2-1/2, F=3/2-3/2 | 113508.907(3e-3) | 5.4 | 1.2196 | 868 | 66.7(0.1) | 5.8(0.2) | 5402(146) |
| CN | N= 1-0, J=3/2-1/2, F=1/2-3/2 | 113520.432(4e-3) | 5.4 | 0.15263 | 90 | 66.7(0.4) | 2.0(0.6) | 187(68) |
| | | | | G010.62−00.38 | | | | |
| $NH_2CHO$ | 5(2, 4) − 4(2, 3) | 105972.665(37e-3) | 27.2 | 54.915 | 60 | -3.0(0.5) | 6.7(1.0) | 427(58) |
| $NH_2CHO$ | 5(3, 3) − 4(3, 2) | 106134.468(55e-3) | 42.1 | 41.845 | 31 | -3.0(0.9) | 9.3(3.0) | 305(147) |
| $NH_2CHO$ | 5(3, 2) − 4(3, 1) | 106141.442(55e-3) | 42.1 | 41.84 | 39 | -3.0(0.8) | 7.5(2.3) | 314(102) |
| CCS | 8(9) − 7(8) | 106347.726(2e-2) | 25.0 | 74.425 | 356 | -3.2(0.1) | 5.8(0.2) | 2215(56) |
| $HC_5N$ | 40 − 39 | 106498.910(7e-3) | 104.8 | 2249.7 | 71 | -3.0(0.4) | 8.1(0.9) | 619(63) |
| $CH_3SH$, v=0-2 | 20(-1, 20) − 20(2, 18) A, vt=1 | 106521.107(3e-3) | 553.8 | 1.9327 | 51 | -3.0(0.4) | 4.4(0.8) | 236(45) |
| $NH_2CHO$ | 5(2, 3) − 4(2, 2) | 106541.773(37e-2) | 27.2 | 54.915 | 78 | -3.0(0.3) | 4.7(0.7) | 398(50) |
| $C_2H_3CN$ | 11(1, 10) − 10(1, 9) | 106641.383(1e-3) | 32.9 | 476.24 | 53 | -3.5(0.4) | 8.0(1.6) | 449(66) |
| $C_2H_5OH$ | 13(1, 12) − 13(0, 13) | 106649.479(5e-2) | 79.4 | 10.463 | 36 | -3.0(0.6) | 4.8(2.3) | 187(61) |
| Hα | H (39) α | 106737.357(0) | – | – | 1087 | 2.3(0.1) | 45.0(2.5) | 12209(1590) |
| Heα | He (39) α | 106780.852(0) | – | – | 119 | 2.3(0.) | 22.6(1.4) | 2865(135) |
| $OC^{34}S$ | 9 − 8 | 106787.390(2e-3) | 25.6 | 4.601 | 50 | -2.8(0.3) | 2.8(0.6) | 149(35) |
| $CH_3OH$, vt=0-2 | 3(1)$^+$ − 4(0)$^+$, vt=0 | 107013.831(1e-2) | 28.3 | 12.036 | 1264 | -4.0(0.2) | 6.0(0.1) | 9350(166) |
| $SO_2$ | 27(3, 25) − 26(4, 22) | 107060.208(2e-3) | 369.4 | 8.2723 | 56 | 0.1(0.4) | 5.6(1.2) | 337(56) |
| $^{13}CH_3CN$ | 6(3) − 5(3) | 107178.424(0) | 82.4 | 276.826 | 53 | -1.1(0.5) | 5.8(0.5) | 331(20) |
| $^{13}CH_3CN$ | 6(2) − 5(2) | 107188.500(1e-1) | 46.6 | 164.068 | 25 | -1.0(0.5) | 6.4(0.5) | 171(20) |
| $^{13}CH_3CN$ | 6(1) − 5(1) | 107194.550(1e-1) | 25.2 | 179.427 | 33 | -1.0(0.5) | 3.1(0.5) | 108(20) |
| $^{13}CH_3CN$ | 6(0) − 5(0) | 107196.570(1e-1) | 18.0 | 184.590 | 52 | -1.0(0.5) | 6.7(0.5) | 368(20) |
| $^{13}C^{17}O$ | 1(2) − 0(3) | 107288.550(5e-2) | 5.1 | 0.016 | 48 | -0.5(0.5) | 3.3(0.5) | 169(16) |
| $^{13}C^{17}O$ | 1(3) − 0(3) | 107289.650(5e-2) | 5.1 | 0.024 | 51 | -0.4(0.5) | 4.0(0.5) | 220(16) |
| $C_2H_5CN$ | 12(7, 5) − 11(7, 4) | 107485.160(5e-2) | 88.0 | 117.36 | 89 | -4.0(0.2) | 1.4(0.4) | 129(30) |
| $C_2H_5CN$ | 12(6, 6) − 11(6, 5) | 107486.949(5e-2) | 73.6 | 133.42 | 44 | -4.0(0.4) | 2.8(1.0) | 130(40) |
| $C_2H_5CN$ | 12(8, 4) − 11(8, 3) | 107491.574(5e-2) | 104.6 | 98.829 | 55 | -4.0(0.2) | 1.2(0.8) | 70(31) |
| $C_2H_5CN$ | 12(5, 7) − 11(5, 6) | 107502.432(5e-2) | 61.3 | 146.99 | 49 | -4.0(0.3) | 2.1(0.6) | 108(32) |
| $C_2H_5CN$ | 12(9, 3) − 11(9, 2) | 107503.686(5e-2) | 123.5 | 77.819 | 77 | -4.0(0.1) | 1.1(0.4) | 93(25) |
| $C_2H_5CN$ | 12(11, 1) − 11(11, 0) | 107539.850(1e-3) | 167.8 | 28.408 | 25 | -4.0(0.5) | 7.8(0.5) | 209(21) |
| $C_2H_5CN$ | 12(4, 9) − 11(4, 8) | 107544.042(5e-2) | 51.3 | 158.12 | 53 | -4.0(0.5) | 7.8(0.5) | 439(21) |
| $C_2H_5CN$ | 12(4, 8) − 11(4, 7) | 107547.460(5e-2) | 51.3 | 158.11 | 49 | -4.0(0.5) | 1.3(0.5) | 66(21) |
| $C_2H_5CN$ | 12(3, 10) − 11(3, 9) | 107594.056(5e-2) | 43.6 | 166.77 | 94 | -4.0(0.2) | 1.4(3.5) | 62(35) |
| $SO_2$ | 12(4, 8) − 13(3, 11) | 107843.470(2e-3) | 111.0 | 4.5354 | 71 | 0.(0.1) | 1.9(0.3) | 147(20) |
| t-HCOOH | 5(1, 5) − 4(1, 4) | 108126.720(3e-3) | 18.8 | 9.6966 | 65 | -3.0(0.6) | 9.1(1.5) | 625(89) |
| $CH_3SH$, v=0-2 | 4(-1, 4) − 4(0, 4) A, vt=0 | 108379.758(1e-3) | 17.3 | 0.38561 | 47 | -3.0(0.1) | 7.6(1.2) | 384(59) |
| $^{13}CN$ | 1(1, 0) − 0(1, 1), F = 1 − 1 | 108412.862(5e-2) | 5.2 | 0.635 | 60 | -3.1(0.2) | 0.8(0.3) | 53(27) |
| $^{13}CN$ | 1(1, 0) − 0(1, 1), F = 1 − 2 | 108426.889(5e-2) | 5.2 | 1.267 | 84 | -3.1(0.1) | 6.3(0.5) | 559(49) |
| $^{13}CN$ | 1(1, 1) − 0(1, 0), F = 0 − 1 | 108631.121(5e-2) | 5.2 | 0.642 | 43 | -3.6(0.5) | 3.2(0.5) | 165(33) |
| $^{13}CN$ | 1(1, 1) − 0(1, 0), F = 1 − 1 | 108636.923(5e-2) | 5.2 | 1.932 | 108 | -3.3(0.5) | 4.6(0.5) | 529(33) |
| $^{13}CN$ | 1(2, 1) − 0(1, 1), F = 1 − 0 | 108638.212(5e-2) | 5.2 | 0.722 | 80 | -3.4(0.5) | 3.9(0.5) | 331(33) |
| $^{13}CN$ | 1(2, 1) − 0(1, 1), F = 2 − 1 | 108643.590(5e-2) | 5.2 | 0.856 | 64 | -3.5(0.5) | 3.4(0.5) | 232(33) |
| $^{13}CN$ | 1(2, 1) − 0(1, 1), F = 0 − 1 | 108644.346(5e-2) | 5.2 | 0.642 | 83 | -3.5(0.5) | 3.3(0.5) | 287(33) |

**Table A2.** (Continued)

| Species | Transitions | Rest Freq. (MHz) | $E_u$ (K) | $\mu^2S$ ($D^2$) | $T_{mb}$ (mK) | $V_{LSR}$ (km $s^{-1}$) | $\Delta V$ (km $s^{-1}$) | $\int T_{mb}$ dv (mK km $s^{-1}$) |
|---|---|---|---|---|---|---|---|---|
| $^{13}$CN | 1(2, 1) − 0(1, 1), F = 1 − 1 | 108645.064(5e-2) | 5.2 | 0.551 | blended | – | – | – |
| $^{13}$CN | 1(1, 1) − 0(1, 0), F = 2 − 1 | 108651.297(5e-2) | 5.2 | 3.276 | 200 | -3.5(0.5) | 5.5(0.5) | 1166(33) |
| $^{13}$CN | 1(2, 1) − 0(1, 1), F = 2 − 2 | 108657.646(5e-2) | 5.2 | 2.420 | 151 | -3.5(0.5) | 4.3(0.5) | 696(33) |
| $^{13}$CN | 1(2, 1) − 0(1, 1), F = 1 − 2 | 108658.948(5e-2) | 5.2 | 0.669 | 115 | -3.5(0.5) | 3.4(0.5) | 420(33) |
| $^{13}$CN | 1(2, 2) − 0(1, 1), F = 3 − 2 | 108780.201(5e-2) | 5.2 | 4.905 | 289 | -3.4(0.1) | 5.2(0.2) | 1601(671) |
| $^{13}$CN | 1(2, 2) − 0(1, 1), F = 2 − 1 | 108782.374(5e-2) | 5.2 | 2.586 | 199 | -3.4(0.1) | 5.9(0.4) | 1241(73) |
| $^{13}$CN | 1(2, 2) − 0(1, 1), F = 1 − 0 | 108786.982(5e-2) | 5.2 | 1.144 | 70 | -3.5(0.3) | 5.2(0.8) | 383(60) |
| $^{13}$CN | 1(2, 2) − 0(1, 1), F = 1 − 1 | 108793.753(5e-2) | 5.2 | 0.894 | 53 | -3.5(0.1) | 3.5(1.1) | 200(69) |
| $^{13}$CN | 1(2, 2) − 0(1, 1), F = 2 − 2 | 108796.400(5e-2) | 5.2 | 0.918 | 50 | -3.5(1.0) | 8.6(2.1) | 453(103) |
| $CH_3OH$, vt=0-2 | 0(0) − 1(-1) E2, vt=0 | 108893.945(12e-3) | 13.1 | 3.9134 | 1388 | -4.0(0.) | 7.6(0.1) | 11234(79) |
| SiS | 6(0) − 5(0) | 108924.301(1e-2) | 18.3 | 5.62 | 53 | -4.0(0.9) | 15.0(2.7) | 840(112) |
| $HC_3N$ | 12 − 11 | 109173.634(1e-2) | 34.1 | 167.1 | 5835 | -3.0(0.) | 7.5(0.1) | 46443(178) |
| SO | 3(2) − 2(1) | 109252.220(1e-1) | 21.1 | 3.5585 | 1740 | -2.5(0.) | 7.1(0.1) | 13056(84) |
| $HC_3N$, $v_7$=1 | 12(-1) − 11(1) | 109442.013(2e-2) | 355.0 | 165.12 | 45 | -3.0(0.7) | 6.7(1.7) | 321(81) |
| OCS | 9 − 8 | 109463.063(5e-3) | 26.3 | 4.6034 | 997 | -3.0(0.) | 7.0(0.1) | 7453(71) |
| H$\gamma$ | H (55) $\gamma$ | 109536.001(1e-3) | – | – | 99 | 2.3(2.8) | 20.3(5.2) | 2135(544) |
| $HC_3N$, $v_7$=1 | 12(1) − 11(-1) | 109598.818(2e-2) | 355.0 | 165.12 | 41 | -3.0(0.7) | 5.2(1.6) | 226(62) |
| $C_2H_5CN$ | 12(1, 11) − 11(1, 10) | 109650.263(5e-2) | 53.4 | 176.49 | 54 | -4.0(0.4) | 4.7(1.2) | 269(52) |
| $C^{18}O$ | 1 − 0 | 109782.173(6e-3) | 5.3 | 0.01221 | 10608 | -3.0(0.1) | 6.1(0.1) | 69430(329) |
| HNCO | 5(0, 5) − 4(0, 4) | 109905.749(7e-3) | 15.8 | 12.482 | 867 | -3.5(0.1) | 8.0(0.2) | 7357(120) |
| $C^{15}N$ | 1(2, 1) − 0(1, 0) | 110023.540(1e-1) | 5.3 | 1.386 | 46 | -3.6(0.7) | 2.5(1.4) | 122(64) |
| $C^{15}N$ | 1(2, 2) − 0(1, 1) | 110024.590(1e-1) | 5.3 | 3.504 | 76 | -3.8(1.2) | 5.5(1.5) | 443(181) |
| $^{13}$CO | 1 − 0 | 110201.35(0) | 5.3 | 0.01220 | 35122 | -3.0(0.1) | 7.2(0.1) | 26892(946) |
| HNCO | 5(1, 4) − 4(1, 3) | 110298.089(5e-3) | 59.2 | 11.847 | 2730 | -3.0(1.5) | 8.1(3.2) | 237(24) |
| $CH_3CN$ | 6(5, 0) − 5(5, 0) | 110330.345(0) | 197.1 | 56.399 | 68 | -4.0(0.5) | 8.7(0.5) | 632(30) |
| $CH_3CN$ | 6(4, 0) − 5(4, 0) | 110349.471(0) | 132.8 | 102.54 | 171 | -4.0(0.5) | 8.4(0.5) | 1533(144) |
| $CH_3CN$ | 6(3, 0) − 5(-3, 0) | 110364.354(0) | 82.8 | 138.45 | 692 | -4.0(0.5) | 8.7(0.5) | 6394(144) |
| $CH_3CN$ | 6(-3, 0) − 5(3, 0) | 110364.354(0) | 82.8 | 138.45 | blended | – | – | – |
| $CH_3CN$ | 6(2, 0) − 5(2, 0) | 110374.989(0) | 47.1 | 164.06 | 722 | -4.0(0.5) | 8.1(0.5) | 6227(144) |
| $CH_3CN$ | 6(1, 0) − 5(1, 0) | 110381.372(0) | 25.7 | 179.45 | 1318 | -4.0(0.5) | 6.3(0.5) | 8829(481) |
| $CH_3CN$ | 6(0, 0) − 5(0, 0) | 110383.500(0) | 18.5 | 184.58 | 1131 | -4.0(0.5) | 6.4(0.5) | 11054(481) |
| $CH_3OCHO$ | 10(0, 10) − 9(0, 9) E | 111169.903(1e-2) | 30.2 | 26.18776 | 15 | -4.0(0.5) | 3.6(0.5) | 57(32) |
| $CH_3OCHO$ | 10(0, 10) − 9(0, 9) A | 111171.634(1e-2) | 30.2 | 26.19136 | 46 | -4.0(0.5) | 5.5(0.5) | 240(32) |
| $CH_3OH$, vt=0-2 | $7(2)^+ - 8(1)^+$, vt=0 | 111289.453(13e-3) | 102.7 | 9.3425 | 154 | -4.0(0.5) | 4.4(0.5) | 724(48) |
| $CH_3OCH_3$ | 7(0, 7) − 6(1, 6) AA | 111782.600(1e-3) | 25.2 | 68.047 | 176 | -4.0(0.2) | 7.0(0.5) | 1301(88) |
| $HC_5N$ | 42 − 41 | 111823.024(0) | 115.4 | 2362.2 | 97 | -3.0(0.5) | 6.9(0.5) | 714(55) |
| H$\beta$ | H (48) $\beta$ | 111885.070(0) | – | – | 137 | 2.1(0.3) | 25.7(0.7) | 8498(207) |
| H$\epsilon$ | H (64) $\epsilon$ | 112124.899(0) | – | – | 56 | 2.4(2.0) | 44.6(7.2) | 2651(287) |
| $CH_3CHO$ | 6(1, 6) − 5(1, 5) A, vt=0 | 112248.716(3e-3) | 21.1 | 73.76807 | 263 | -3.2(0.5) | 12.8(2.0) | 3573(375) |
| $CH_3CHO$ | 6(1, 6) − 5(1, 5) E, vt=0 | 112254.508(3e-3) | 21.2 | 73.79585 | 321 | -3.2(0.4) | 8.3(1.0) | 2829(283) |
| $C^{17}O$ | 1 − 0 | 112359.284(1e-3) | 5.4 | 0.01217 | 3010 | -3.2(0.1) | 7.3(0.1) | 23339(181) |
| CN | N= 1-0, J=1/2-1/2, F=1/2-1/2 | 113123.370(6e-3) | 5.4 | 0.15271 | 900 | -3.0(0.3) | 6.9(0.7) | 6623(603) |
| CN | N= 1-0, J=1/2-1/2, F=1/2-3/2 | 113144.157(6e-3) | 5.4 | 1.2492 | 2893 | -3.0(0.1) | 6.7(0.3) | 20689(638) |
| CN | N= 1-0, J=1/2-1/2, F=3/2-1/2 | 113170.492(4e-3) | 5.4 | 1.2199 | 4398 | -3.0(0.1) | 7.0(0.2) | 32518(637) |
| CN | N= 1-0, J=1/2-1/2, F=3/2-3/2 | 113191.279(3e-3) | 5.4 | 1.5836 | 3621 | -3.0(0.1) | 7.1(0.2) | 27269(657) |
| CN | N= 1-0, J=3/2-1/2, F=3/2-1/2 | 113488.120(3e-3) | 5.4 | 1.5836 | 4036 | -3.0(0.5) | 4.0(0.5) | 16958(1110) |
| CN | N= 1-0, J=3/2-1/2, F=5/2-3/2 | 113490.970(2e-3) | 5.4 | 4.205 | 8611 | -3.0(0.5) | 4.2(0.5) | 38472(1110) |
| CN | N= 1-0, J=3/2-1/2, F=1/2-1/2 | 113499.644(3e-3) | 5.4 | 1.2491 | 1546 | -3.0(0.5) | 4.6(0.5) | 7584(1110) |
| CN | N= 1-0, J=3/2-1/2, F=3/2-3/2 | 113508.907(3e-3) | 5.4 | 1.2196 | 2357 | -3.0(0.5) | 7.8(0.5) | 19549(1110) |
| CN | N= 1-0, J=3/2-1/2, F=1/2-3/2 | 113520.432(4e-3) | 5.4 | 0.15263 | 203 | -3.0(0.5) | 3.1(0.5) | 678(132) |
| | | | | G011.49−01.48 | | | | |
| $CH_3OH$, vt=0-2 | $3(1)^+ - 4(0)^+$, vt=0 | 107013.831(1e-2) | 28.3 | 12.036 | 123 | 9.6 (0.4) | 6.9(1.3) | 902(114) |
| $^{13}$CN | 1(2, 2) − 0(1, 1), F = 3 − 2 | 108780.201(5e-2) | 5.2 | 4.905 | 87 | 10.4(0.4) | 3.7(1.1) | 339(71) |
| $^{13}$CN | 1(2, 2) − 0(1, 1), F = 2 − 1 | 108782.374(5e-2) | 5.2 | 2.586 | 85 | 10.4(0.3) | 1.9(0.6) | 169(46) |
| $^{13}$CN | 1(2, 2) − 0(1, 1), F = 1 − 0 | 108786.982(5e-2) | 5.2 | 1.144 | 32 | 10.3(0.8) | 3.3(1.5) | 115(54) |
| $CH_3OH$, vt=0-2 | 0(0) − 1(-1) E2, vt=0 | 108893.945(12e-3) | 13.1 | 3.9134 | 95 | 9.5 (0.5) | 3.7(0.5) | 369(26) |
| $HC_3N$ | 12 − 11 | 109173.634(1e-2) | 34.1 | 167.1 | 1848 | 10.5(0.) | 2.3(0.1) | 4511(54) |
| SO | 3(2) − 2(1) | 109252.220(1e-1) | 21.1 | 3.5585 | 259 | 10.6(0.1) | 2.2(0.3) | 596(65) |
| $C^{18}O$ | 1 − 0 | 109782.173(6e-3) | 5.3 | 0.01221 | 1420 | 10.5(0.5) | 1.4(0.5) | 2941(534) |
| $^{13}$CO | 1 − 0 | 110201.35(0) | 5.3 | 0.01220 | 11455 | 10.0(0.5) | 4.3(0.5) | 52654(1380) |
| $CH_3CN$ | 6(2, 0) − 5(2, 0) | 110374.989(0) | 47.1 | 164.06 | 32 | 10.0(2.1) | 4.2(0.2) | 141(112) |
| $CH_3CN$ | 6(1, 0) − 5(1, 0) | 110381.372(0) | 25.7 | 179.45 | 169 | 10.0(0.1) | 1.8(0.4) | 321(51) |
| $CH_3CN$ | 6(0, 0) − 5(0, 0) | 110383.500(0) | 18.5 | 184.58 | 156 | 10.0(0.2) | 2.2(0.4) | 365(55) |
| $CH_3OH$, vt=0-2 | $7(2)^+ - 8(1)^+$, vt=0 | 111289.453(13e-3) | 102.7 | 9.34234 | 99 | 9.1(0.2) | 1.1(0.8) | 118(57) |
| $C^{17}O$ | 1 − 0 | 112359.284(1e-3) | 5.4 | 0.01217 | 235 | 10.0(0.2) | 5.6(0.6) | 1402(128) |
| CN | N= 1-0, J=1/2-1/2, F=1/2-1/2 | 113123.370(6e-3) | 5.4 | 0.15271 | 295 | 10.2(0.5) | 2.5(0.5) | 779(109) |
| CN | N= 1-0, J=1/2-1/2, F=1/2-3/2 | 113144.157(6e-3) | 5.4 | 1.2492 | 1091 | 10.2(0.5) | 3.0(0.5) | 3465(109) |
| CN | N= 1-0, J=1/2-1/2, F=3/2-1/2 | 113170.492(4e-3) | 5.4 | 1.2199 | 1158 | 10.2(0.5) | 2.9(0.5) | 3564(109) |
| CN | N= 1-0, J=1/2-1/2, F=3/2-3/2 | 113191.279(3e-3) | 5.4 | 1.5836 | 1169 | 10.2(0.5) | 2.9(0.5) | 3616(109) |
| CN | N= 1-0, J=3/2-1/2, F=3/2-1/2 | 113488.120(3e-3) | 5.4 | 1.5836 | 1037 | 10.2(0.) | 3.2(0.1) | 3509(112) |
| CN | N= 1-0, J=3/2-1/2, F=5/2-3/2 | 113490.970(2e-3) | 5.4 | 4.205 | 2024 | 10.2(0.) | 3.3(0.1) | 7043(108) |
| CN | N= 1-0, J=3/2-1/2, F=1/2-1/2 | 113499.644(3e-3) | 5.4 | 1.2491 | 802 | 10.2(0.) | 3.0(0.1) | 2525(100) |
| CN | N= 1-0, J=3/2-1/2, F=3/2-3/2 | 113508.907(3e-3) | 5.4 | 1.2196 | 842 | 10.2(0.) | 3.0(0.1) | 2718(100) |
| CN | N= 1-0, J=3/2-1/2, F=1/2-3/2 | 113520.432(4e-3) | 5.4 | 0.15263 | 270 | 10.2(0.2) | 2.2(0.4) | 645(93) |
| | | | | G011.91−00.61 | | | | |
| $NH_2CHO$ | 5(2, 4) − 4(2, 3) | 105972.665(37e-3) | 27.2 | 54.915 | 27 | 36.0(0.8) | 10.0(1.5) | 291(46) |
| $NH_2CHO$ | 5(4, 1) − 4(4, 0) | 106107.870(88e-3) | 63.0 | 23.537 | 26 | 36.0(7.7) | 9.9(0.5) | 273(98) |
| $NH_2CHO$ | 5(3, 3) − 4(3, 2) | 106134.468(55e-3) | 42.1 | 41.845 | 11 | 36.0(0.5) | 7.1(0.5) | 171(98) |
| $NH_2CHO$ | 5(3, 2) − 4(3, 1) | 106141.442(55e-3) | 42.1 | 41.84 | 14 | 36.0(0.5) | 8.7(0.5) | 253(98) |
| CCS | 8(9) − 7(8) | 106347.726(2e-2) | 25.0 | 74.425 | 97 | 36.0(0.2) | 3.8(0.4) | 398(32) |
| $HC_5N$ | 40 − 39 | 106498.910(7e-3) | 104.8 | 2249.7 | 36 | 36.0(0.5) | 5.7(1.4) | 218(39) |
| $NH_2CHO$ | 5(2, 3) − 4(2, 2) | 106541.773(37e-3) | 27.2 | 54.915 | 23 | 36.0(0.7) | 5.9(1.7) | 143(36) |
| $C_2H_3CN$ | 11(1, 10) − 10(1, 9) | 106641.383(1e-3) | 32.9 | 476.24 | 34 | 35.7(0.7) | 9.4(2.3) | 337(59) |
| $CH_3OH$, vt=0-2 | $3(1)^+ - 4(0)^+$, vt=0 | 107013.831(1e-2) | 28.3 | 12.036 | 111 | 37.0(0.2) | 6.8(0.4) | 800(38) |
| $C_2H_5CN$ | 12(2, 11) − 11(2, 10) | 107043.527(5e-2) | 37.9 | 172.86 | 19 | 36.5(1.4) | 13.2(3.1) | 272(54) |
| $C_2H_5CN$ | 12(7, 5) − 11(7, 4) | 107485.160(5e-2) | 88.0 | 117.36 | 41 | 36.5(0.5) | 10.3(0.5) | 450(11) |
| $C_2H_5CN$ | 12(6, 6) − 11(6, 5) | 107486.949(5e-2) | 73.6 | 133.42 | 24 | 36.5(0.5) | 16.7(0.5) | 419(11) |
| $C_2H_5CN$ | 12(5, 7) − 11(5, 6) | 107502.432(5e-2) | 61.3 | 146.99 | 47 | 36.5(0.5) | 12.8(0.5) | 645(11) |
| $C_2H_5CN$ | 12(10, 2) − 11(10, 1) | 107519.861(5e-2) | 144.6 | 54.355 | 17 | 36.5(0.5) | 19.6(0.5) | 354(11) |
| $CH_3OCHO$ | 9( 2, 8) − 8( 2, 7) E | 107537.258(1e-2) | 28.8 | 22.60702 | 25 | 35.8(0.5) | 6.5(0.5) | 173(11) |
| $CH_3OCHO$ | 9( 2, 8) − 8( 2, 7) A | 107543.711(1e-2) | 28.8 | 22.61344 | blended | – | – | – |
| $C_2H_5CN$ | 12(4, 9) − 11(4, 8) | 107544.042(5e-2) | 51.3 | 158.12 | 31 | 36.5(0.5) | 11.5(0.5) | 379(11) |
| $C_2H_5CN$ | 12(4, 8) − 11(4, 7) | 107547.460(5e-2) | 51.3 | 158.11 | 29 | 36.5(0.5) | 11.4(0.5) | 349(11) |
| $C_2H_5CN$ | 12(3, 10) − 11(3, 9) | 107594.056(5e-2) | 43.6 | 166.77 | 40 | 36.5(0.5) | 10.9(0.5) | 463(11) |
| t-HCOOH | 5(1, 5) − 4(1, 4) | 108126.720(3e-3) | 18.8 | 9.6966 | 27 | 37.3(0.5) | 5.0(2.6) | 143(46) |
| $^{13}$CN | 1(1, 1) − 0(1, 0), F = 0 − 1 | 108631.121(5e-2) | 5.2 | 0.642 | 25 | 36.1(0.5) | 2.7(1.0) | 72(24) |

**Table A2.** (Continued)

| Species | Transitions | Rest Freq. (MHz) | $E_u$ (K) | $\mu^2 S$ ($D^2$) | $T_{mb}$ (mK) | $V_{LSR}$ (km $s^{-1}$) | $\Delta V$ (km $s^{-1}$) | $\int T_{mb}$ dv (mK km $s^{-1}$) |
|---|---|---|---|---|---|---|---|---|
| $^{13}$CN | 1(1, 1) − 0(1, 0), F = 1 − 1 | 108636.923(5e-2) | 5.2 | 1.932 | 63 | 36.0(0.2) | 2.8(0.6) | 191(32) |
| $^{13}$CN | 1(2, 1) − 0(1, 1), F = 1 − 0 | 108638.212(5e-2) | 5.2 | 0.722 | 23 | 36.0(0.6) | 2.4(1.0) | 58(26) |
| $^{13}$CN | 1(2, 1) − 0(1, 1), F = 2 − 1 | 108643.590(5e-2) | 5.2 | 0.856 | 75 | 36.2(0.1) | 0.8(0.3) | 54(13) |
| $^{13}$CN | 1(2, 1) − 0(1, 1), F = 0 − 1 | 108644.346(5e-2) | 5.2 | 0.642 | 59 | 36.2(0.1) | 0.5(0.3) | 34(12) |
| $^{13}$CN | 1(2, 1) − 0(1, 1), F = 1 − 1 | 108645.064(5e-2) | 5.2 | 0.551 | 27 | 36.0(0.4) | 2.7(1.0) | 80(26) |
| $^{13}$CN | 1(1, 1) − 0(1, 0), F = 2 − 1 | 108651.297(5e-2) | 5.2 | 3.276 | 92 | 36.0(0.1) | 2.9(0.4) | 287(28) |
| $^{13}$CN | 1(2, 1) − 0(1, 1), F = 2 − 2 | 108657.646(5e-2) | 5.2 | 2.420 | 82 | 36.0(0.2) | 2.3(0.4) | 196(31) |
| $^{13}$CN | 1(2, 1) − 0(1, 1), F = 1 − 2 | 108658.948(5e-2) | 5.2 | 0.669 | 32 | 36.1(0.5) | 4.1(1.1) | 138(34) |
| $^{13}$CN | 1(2, 2) − 0(1, 1), F = 3 − 2 | 108780.201(5e-2) | 5.2 | 4.905 | 142 | 36.1(0.1) | 2.9(0.2) | 444(26) |
| $^{13}$CN | 1(2, 2) − 0(1, 1), F = 2 − 1 | 108782.374(5e-2) | 5.2 | 2.586 | 78 | 36.1(0.1) | 2.2(0.5) | 182(28) |
| $^{13}$CN | 1(2, 2) − 0(1, 1), F = 1 − 0 | 108786.982(5e-2) | 5.2 | 1.144 | 43 | 36.1(0.3) | 3.0(0.6) | 139(25) |
| $^{13}$CN | 1(2, 2) − 0(1, 1), F = 1 − 1 | 108793.753(5e-2) | 5.2 | 0.894 | 36 | 36.0(0.4) | 3.5(0.8) | 136(28) |
| $^{13}$CN | 1(2, 2) − 0(1, 1), F = 2 − 2 | 108796.400(5e-2) | 5.2 | 0.918 | 43 | 36.0(0.2) | 1.2(0.4) | 54(17) |
| $CH_3OH$, vt=0-2 | 0(0) − 1(-1) E2, vt=0 | 108893.945(12e-3) | 13.1 | 3.9134 | 600 | 37.0(0.) | 8.2(0.1) | 5212(57) |
| $C_2H_5CN$ | 12(2, 10) − 11(2, 9) | 108940.554(5e-2) | 38.2 | 172.93 | blended | − | − | − |
| $C_2H_5CN$ | 11(3, 9) − 12(0, 12) | 108940.696(4e-3) | 38.4 | 0.042598 | 32 | 36.5(0.7) | 8.6(1.7) | 292(48) |
| $HC_3N$ | 12 − 11 | 109173.634(1e-2) | 34.1 | 167.1 | 1854 | 36.0(0.) | 5.2(0.1) | 10239(114) |
| SO | 3(2) − 2(1) | 109252.220(1e-1) | 21.1 | 3.5585 | 226 | 36.5(0.1) | 8.7(0.3) | 2097(50) |
| $HC_3N$, $v_7$=1 | 12(-1) − 11(1) | 109442.013(2e-2) | 355.0 | 165.12 | 33 | 36.0(0.5) | 9.9(0.5) | 346(37) |
| OCS | 9 − 8 | 109463.063(5e-3) | 26.3 | 4.6034 | 302 | 36.0(0.5) | 7.0(0.5) | 2241(37) |
| $HC_3N$, $v_7$=1 | 12(1) − 11(-1) | 109598.818(2e-2) | 355.0 | 165.12 | 27 | 36.0(0.9) | 9.5(2.0) | 274(53) |
| $C_2H_5CN$ | 12(1, 11) − 11(1, 10) | 109650.263(5e-2) | 53.4 | 176.49 | 25 | 36.5(1.1) | 9.8(2.1) | 266(57) |
| $C^{18}O$ | 1 − 0 | 109782.173(6e-3) | 5.3 | 0.01221 | 2909 | 36.5(0.1) | 3.0(0.1) | 9144(132) |
| HNCO | 5(0, 5) − 4(0, 4) | 109905.749(7e-3) | 15.8 | 12.482 | 735 | 36.0(0.) | 7.0(0.2) | 5464(91) |
| $C^{15}N$ | 1(2, 1) − 0(1, 0) | 110023.540(1e-1) | 5.3 | 1.386 | 32 | 35.0(0.7) | 6.1(1.2) | 210(43) |
| $C^{15}N$ | 1(2, 2) − 0(1, 1) | 110024.590(1e-1) | 5.3 | 3.504 | blended | − | − | − |
| $^{13}$CO | 1 − 0 | 110201.35(0) | 5.3 | 0.01220 | 6091 | 35.5(0.5) | 1.4(0.5) | 9086(390) |
| HNCO | 5(1, 4) − 4(1, 3) | 110298.089(5e-3) | 59.2 | 11.847 | 37 | 36.0(0.5) | 11.0(0.5) | 418(67) |
| $CH_3CN$ | 6(5, 0) − 5(5, 0) | 110330.345(0) | 197.1 | 56.399 | 47 | 36.0(0.5) | 17.0(0.5) | 845(67) |
| $CH_3CN$ | 6(4, 0) − 5(4, 0) | 110349.471(0) | 132.8 | 102.54 | 87 | 36.0(0.5) | 10.2(0.5) | 948(67) |
| $CH_3CN$ | 6(3, 0) − 5(-3, 0) | 110364.354(0) | 82.8 | 138.45 | 243 | 36.0(0.5) | 9.1(0.5) | 2354(67) |
| $CH_3CN$ | 6(-3, 0) − 5(3, 0) | 110364.354(0) | 82.8 | 138.45 | blended | − | − | − |
| $CH_3CN$ | 6(2, 0) − 5(2, 0) | 110374.989(0) | 47.1 | 164.06 | 279 | 36.0(0.5) | 8.4(0.5) | 2503(67) |
| $CH_3CN$ | 6(1, 0) − 5(1, 0) | 110381.372(0) | 25.7 | 179.45 | 466 | 36.0(0.5) | 5.2(0.5) | 2587(67) |
| $CH_3CN$ | 6(0, 0) − 5(0, 0) | 110383.500(0) | 18.5 | 184.58 | 608 | 36.0(0.5) | 7.3(0.5) | 4749(67) |
| $CH_3OH$, vt=0-2 | $7(2)^+ - 8(1)^+$, vt=0 | 111289.453(13e-3) | 102.7 | 9.3425 | 52 | 37.0(0.5) | 8.2(0.5) | 454(21) |
| $CH_3OCH_3$ | 7(0, 7) − 6(1, 6) AA | 111782.600(1e-3) | 25.2 | 68.047 | 48 | 36.1(0.8) | 9.9(1.8) | 501(100) |
| $CH_3CHO$ | 6(1, 6) − 5(1, 5) A, vt=0 | 112248.716(3e-3) | 21.1 | 73.76807 | 109 | 36.6(0.5) | 11.6(0.5) | 1355(23) |
| $CH_3CHO$ | 6(1, 6) − 5(1, 5) E, vt=0 | 112254.508(3e-3) | 21.2 | 73.79585 | 121 | 36.6(0.5) | 9.5(0.5) | 1225(23) |
| $C^{17}O$ | 1 − 0 | 112359.284(1e-3) | 5.4 | 0.01217 | 682 | 37.0(0.2) | 4564(103) | 3313(57) |
| CN | N= 1-0, J=1/2-1/2, F=1/2-1/2 | 113123.370(6e-3) | 5.4 | 0.15271 | 525 | 34.0(0.5) | 3.4(0.5) | 1917(91) |
| CN | N= 1-0, J=1/2-1/2, F=1/2-3/2 | 113144.157(6e-3) | 5.4 | 1.2492 | 718 | 34.0(0.5) | 3.3(0.5) | 2496(91) |
| CN | N= 1-0, J=1/2-1/2, F=3/2-1/2 | 113170.492(4e-3) | 5.4 | 1.2199 | 1019 | 34.0(0.5) | 3.1(0.5) | 3377(91) |
| CN | N= 1-0, J=1/2-1/2, F=3/2-3/2 | 113191.279(3e-3) | 5.4 | 1.5836 | 810 | 34.0(0.5) | 2.9(0.5) | 2527(91) |
| CN | N= 1-0, J=3/2-1/2, F=3/2-1/2 | 113488.120(3e-3) | 5.4 | 1.5836 | 989 | 34.0(0.5) | 4.5(0.5) | 4743(143) |
| CN | N= 1-0, J=3/2-1/2, F=5/2-3/2 | 113490.970(2e-3) | 5.4 | 4.205 | 1221 | 34.0(0.5) | 3.8(0.5) | 4970(143) |
| CN | N= 1-0, J=3/2-1/2, F=1/2-1/2 | 113499.644(3e-3) | 5.4 | 1.2491 | 474 | 34.0(0.5) | 3.7(0.5) | 1853(143) |
| CN | N= 1-0, J=3/2-1/2, F=3/2-3/2 | 113508.907(3e-3) | 5.4 | 1.2196 | 714 | 34.0(0.5) | 3.3(0.5) | 2530(143) |
| CN | N= 1-0, J=3/2-1/2, F=1/2-3/2 | 113520.432(4e-3) | 5.4 | 0.15263 | 219 | 34.0(0.5) | 3.4(0.5) | 797(143) |
| | | | | G012.80−00.20 | | | | |
| $NH_2CHO$ | 5(2, 4) − 4(2, 3) | 105972.665(37e-3) | 27.2 | 54.915 | 40 | 36.0(0.3) | 2.2(1.0) | 92(32) |
| CCS | 8(9) − 7(8) | 106347.726(2e-2) | 25.0 | 74.425 | 219 | 35.0(0.1) | 5.4(0.2) | 1272(40) |
| $HC_5N$ | 40 − 39 | 106498.910(7e-3) | 104.8 | 2249.7 | 83 | 36.0(0.5) | 7.3(0.5) | 647(21) |
| $CH_3SH$, v=0-2 | 2(-1, 2) − 2(0, 2) A, vt=0 | 106524.119(1e-2) | 8.8 | 1.3632 | 32 | 37.0(0.5) | 2.5(1.4) | 88(35) |
| $C_2H_3CN$ | 11(1, 10) − 10(1, 9) | 106641.383(1e-3) | 32.9 | 476.24 | 31 | 36.0(0.7) | 9.3(1.9) | 309(50) |
| H$\alpha$ | H (39) $\alpha$ | 106737.357(0) | − | − | 2287 | 37.2(0.5) | 33.5(0.5) | 81558(386) |
| He$\alpha$ | He (39) $\alpha$ | 106780.852(0) | − | − | 214 | 37.1(0.2) | 33.0(0.7) | 7541(116) |
| H$\varepsilon$ | H (65) $\varepsilon$ | 107206.108(0) | − | − | 132 | 37.6(0.5) | 39.6(1.3) | 5545(151) |
| $^{13}C^{17}O$ | 1(2) − 0(3) | 107288.550(5e-2) | 5.1 | 0.016 | 34 | 36.5(2.0) | 5.6(2.6) | 206(145) |
| $^{13}C^{17}O$ | 1(3) − 0(3) | 107289.650(5e-2) | 5.1 | 0.024 | 27 | 36.1(2.2) | 5.0(3.4) | 148(140) |
| $CH_3SH$, v=0-2 | 3(-1, 3) − 3(0, 3) A, vt=0 | 107316.441(1e-3) | 12.4 | 0.27881 | 49 | 37.0(0.3) | 6.2(1.0) | 323(43) |
| $CH_3C_3N$ | 26(2) − 25(2) | 107407.677(4e-3) | 99.5 | 116.3 | blended | − | − | − |
| $CH_3C_3N$ | 26(1) − 25(1) | 107410.776(4e-3) | 77.1 | 1171.5 | blended | − | − | − |
| $CH_3C_3N$ | 26(0) − 25(0) | 107411.809(4e-3) | 69.6 | 1173.3 | 42 | 35.0(0.6) | 9.1(1.3) | 414(53) |
| $CH_3SH$, v=0-2 | 4(-1, 4) − 4(0, 4) A, vt=0 | 108379.758(1e-3) | 17.3 | 0.38561 | 34 | 37.0(1.3) | 12.1(4.9) | 436(111) |
| $^{13}$CN | 1(1, 1) − 0(1, 0), F = 0 − 1 | 108631.121(5e-2) | 5.2 | 0.642 | 17 | 36.7(0.5) | 2.0(0.5) | 36(15) |
| $^{13}$CN | 1(1, 1) − 0(1, 0), F = 1 − 1 | 108636.923(5e-2) | 5.2 | 1.932 | 76 | 36.5(0.5) | 2.5(0.5) | 203(15) |
| $^{13}$CN | 1(2, 1) − 0(1, 1), F = 1 − 0 | 108638.212(5e-2) | 5.2 | 0.722 | 61 | 36.4(0.5) | 1.0(0.5) | 67(15) |
| $^{13}$CN | 1(2, 1) − 0(1, 1), F = 2 − 1 | 108643.590(5e-2) | 5.2 | 0.856 | 48 | 36.5(0.5) | 2.9(0.5) | 146(15) |
| $^{13}$CN | 1(2, 1) − 0(1, 1), F = 0 − 1 | 108644.346(5e-2) | 5.2 | 0.642 | blended | − | − | − |
| $^{13}$CN | 1(2, 1) − 0(1, 1), F = 1 − 1 | 108645.064(5e-2) | 5.2 | 0.551 | blended | − | − | − |
| $^{13}$CN | 1(1, 1) − 0(1, 0), F = 2 − 1 | 108651.297(5e-2) | 5.2 | 3.276 | 107 | 36.4(0.5) | 3.0(0.5) | 337(15) |
| $^{13}$CN | 1(2, 1) − 0(1, 1), F = 2 − 2 | 108657.646(5e-2) | 5.2 | 2.420 | 87 | 36.3(0.5) | 2.9(0.5) | 270(15) |
| $^{13}$CN | 1(2, 1) − 0(1, 1), F = 1 − 2 | 108658.948(5e-2) | 5.2 | 0.669 | 43 | 36.5(0.5) | 1.1(0.5) | 52(15) |
| $^{13}$CN | 1(2, 2) − 0(1, 1), F = 3 − 2 | 108780.201(5e-2) | 5.2 | 4.905 | 158 | 36.5(0.1) | 3.0(0.2) | 511(39) |
| $^{13}$CN | 1(2, 2) − 0(1, 1), F = 2 − 1 | 108782.374(5e-2) | 5.2 | 2.586 | 84 | 36.4(0.2) | 2.3(0.3) | 209(30) |
| $^{13}$CN | 1(2, 2) − 0(1, 1), F = 1 − 0 | 108786.982(5e-2) | 5.2 | 1.144 | 22 | 36.4(0.7) | 2.3(1.0) | 55(31) |
| $^{13}$CN | 1(2, 2) − 0(1, 1), F = 1 − 1 | 108793.753(5e-2) | 5.2 | 0.894 | 31 | 36.5(0.3) | 0.5(0.4) | 18(13) |
| $^{13}$CN | 1(2, 2) − 0(1, 1), F = 2 − 2 | 108796.400(5e-2) | 5.2 | 0.918 | 24 | 36.4(0.6) | 2.3(0.9) | 57(29) |
| $CH_3OH$, vt=0-2 | 0(0) − 1(-1) E2, vt=0 | 108893.945(12e-3) | 13.1 | 3.9134 | 696 | 36.0(0.1) | 6.4(0.2) | 4743(139) |
| $HC_5N$ | 41 − 40 | 109160.973(7e-3) | 110.0 | 2306 | 65 | 36.0(0.3) | 6.3(0.7) | 437(44) |
| $HC_3N$ | 12 − 11 | 109173.634(1e-2) | 34.1 | 167.1 | 4528 | 36.0(0.) | 5.6(0.1) | 26773(40) |
| SO | 3(2) − 2(1) | 109252.220(1e-1) | 21.1 | 3.5585 | 958 | 36.0(0.) | 6.0(0.1) | 6133(64) |
| OCS | 9 − 8 | 109463.063(5e-3) | 26.3 | 4.6034 | 515 | 36.0(0.) | 5.5(0.1) | 2996(60) |
| H$\gamma$ | H (55) $\gamma$ | 109536.001(0) | − | − | 271 | 37.8(0.6) | 26.2(1.1) | 7563(311) |
| $C^{18}O$ | 1 − 0 | 109782.173(6e-3) | 5.3 | 0.01221 | 8608 | 35.5(0.1) | 6.1(0.1) | 55461(369) |
| HNCO | 5(0, 5) − 4(0, 4) | 109905.749(7e-3) | 15.8 | 12.482 | 659 | 36.0(0.1) | 6.1(0.2) | 4248(118) |
| $^{13}$CO | 1 − 0 | 110201.35(0) | 5.3 | 0.01220 | 28721 | 35.4(0.1) | 6.7(0.1) | 20347(2210) |
| $CH_3CN$ | 6(4, 0) − 5(4, 0) | 110349.471(0) | 132.8 | 102.54 | 19 | 35.5(0.5) | 3.7(0.5) | 74(82) |
| $CH_3CN$ | 6(3, 0) − 5(-3, 0) | 110364.354(0) | 82.8 | 138.45 | 290 | 35.5(0.5) | 5.0(0.5) | 1535(85) |
| $CH_3CN$ | 6(-3, 0) − 5(3, 0) | 110364.354(0) | 82.8 | 138.45 | blended | − | − | − |
| $CH_3CN$ | 6(2, 0) − 5(2, 0) | 110374.989(0) | 47.1 | 146.06 | 339 | 35.5(0.5) | 5.0(0.5) | 1805(85) |
| $CH_3CN$ | 6(1, 0) − 5(1, 0) | 110381.372(0) | 25.7 | 179.45 | 655 | 35.5(0.5) | 5.5(0.5) | 3810(85) |
| $CH_3CN$ | 6(0, 0) − 5(0, 0) | 110383.500(0) | 18.5 | 184.58 | 662 | 35.5(0.5) | 4.6(0.5) | 3253(85) |
| H$\delta$ | H (60 ) $\delta$ | 110600.675(0) | − | − | 208 | 36.5(0.3) | 35.0(0.8) | 7740(201) |
| $CH_3C_3N$ | 27(2) − 26(2) | 111538.207(4e-3) | 104.9 | 1211.5 | 25 | 35.3(1.3) | 5.3(2.3) | 140(64) |

**Table A2.** (Continued)

| Species | Transitions | Rest Freq. (MHz) | $E_u$ (K) | $\mu^2S$ ($D^2$) | $T_{mb}$ (mK) | $V_{LSR}$ (km $s^{-1}$) | $\Delta V$ (km $s^{-1}$) | $\int T_{mb}$ dv (mK km $s^{-1}$) |
|---|---|---|---|---|---|---|---|---|
| $CH_3C_3N$ | 27(1) − 26(1) | 111541.424(4e-3) | 82.4 | 1216.7 | 21 | 35.3(1.9) | 8.2(4.1) | 185(82) |
| $CH_3C_3N$ | 27(0) − 26(0) | 111542.497(4e-3) | 74.9 | 1218.5 | 64 | 35.3(0.5) | 5.6(1.6) | 378(78) |
| t-HCOOH | 5(0, 5) − 4(0, 4) | 111746.784(3e-3) | 16.1 | 10.092 | 58 | 35.0(0.4) | 6.0(1.3) | 372(89) |
| $CH_3OCH_3$ | 19(3, 16) − 19(2, 17) AA | 111744.238(29e-3) | 187.5 | 259.8 | blended | – | – | – |
| $CH_3OCH_3$ | 7(0, 7) − 6(1, 6) AA | 111782.562(8e-3) | 25.2 | 68.047 | 68 | 36.0(0.5) | 9.3(2.3) | 674(113) |
| $CH_3OCH_3$ | 18(3, 15) − 18(2, 16) EE | 111813.668(21e-3) | 115.4 | 386.29 | blended | – | – | – |
| $HC_5N$ | 42 − 41 | 111823.024(0) | 115.4 | 2362.2 | 91 | 36.0(0.3) | 5.1(0.9) | 491(93) |
| H$\beta$ | H (48) $\beta$ | 111885.070(0) | – | – | 731 | 37.5(0.1) | 32.9(0.2) | 25616(150) |
| He$\beta$ | He (48) $\beta$ | 111930.663(0) | – | – | 81 | 38.2(0.9) | 27.7(2.4) | 2096(183) |
| H$\varepsilon$ | H (64) $\varepsilon$ | 112124.899(0) | – | – | 144 | 35.2(0.6) | 39.3(1.7) | 6033(203) |
| $CH_3CHO$ | 6(1, 6) − 5(1, 5) A, vt=0 | 112248.716(3e-3) | 21.1 | 73.76807 | 176 | 35.7(0.3) | 7.6(1.0) | 1412(126) |
| $CH_3CHO$ | 6(1, 6) − 5(1, 5) E, vt=0 | 112254.508(3e-3) | 21.2 | 73.79585 | 168 | 35.7(0.3) | 8.1(0.9) | 1454(122) |
| $C^{17}O$ | 1 − 0 | 112359.284(1e-3) | 5.4 | 0.01217 | 2556 | 35.0(0.1) | 7.0(0.1) | 19019(93) |
| CN | N= 1-0, J=1/2-1/2, F=1/2-1/2 | 113123.370(6e-3) | 5.4 | 0.15271 | 582 | 36.0(0.2) | 4.6(0.5) | 2852(262) |
| CN | N= 1-0, J=1/2-1/2, F=1/2-3/2 | 113144.157(6e-3) | 5.4 | 1.2492 | 1472 | 36.0(0.1) | 2.5(0.1) | 3869(172) |
| CN | N= 1-0, J=1/2-1/2, F=3/2-1/2 | 113170.492(4e-3) | 5.4 | 1.2199 | 2795 | 36.0(0.) | 3.7(0.1) | 10923(235) |
| CN | N= 1-0, J=1/2-1/2, F=3/2-3/2 | 113191.279(3e-3) | 5.4 | 1.5836 | 1904 | 36.0(0.) | 2.6(0.1) | 5338(178) |
| CCS | 9(8) − 8(7) | 113410.186(2e-2) | 33.6 | 65.427 | 119 | 35.0(0.3) | 6.2(0.7) | 783(99) |
| CN | N= 1-0, J=3/2-1/2, F=3/2-1/2 | 113488.120(3e-3) | 5.4 | 1.5838 | 2413 | 36.0(0.) | 2.8(0.1) | 7202(414) |
| CN | N= 1-0, J=3/2-1/2, F=5/2-3/2 | 113490.970(2e-3) | 5.4 | 4.205 | 5808 | 36.0(0.) | 2.7(0.1) | 16807(274) |
| CN | N= 1-0, J=3/2-1/2, F=1/2-1/2 | 113499.644(3e-3) | 5.4 | 1.2491 | 612 | 36.0(0.1) | 1.8(0.2) | 1158(172) |
| CN | N= 1-0, J=3/2-1/2, F=3/2-3/2 | 113508.907(3e-3) | 5.4 | 1.2196 | 1368 | 36.0(0.) | 2.7(0.2) | 3958(225) |
| | | | | G012.88+00.48 | | | | |
| $NH_2CHO$ | 5(2, 4) − 4(2, 3) | 105972.665(37e-3) | 27.2 | 54.915 | 48 | 32.0(0.3) | 5.0(1.1) | 256(37) |
| $NH_2CHO$ | 5(4, 1) − 4(4, 0) | 106107.870(88e-3) | 63.0 | 23.537 | 24 | 32.2(0.6) | 4.8(1.2) | 120(28) |
| $NH_2CHO$ | 5(3, 3) − 4(3, 2) | 106134.468(55e-3) | 42.1 | 41.845 | 30 | 32.2(0.5) | 5.0(1.0) | 160(28) |
| $NH_2CHO$ | 5(3, 2) − 4(3, 1) | 106141.442(55e-3) | 42.1 | 41.84 | 32 | 32.0(0.4) | 5.1(0.8) | 174(28) |
| CCS | 8(9) − 7(8) | 106347.726(2e-2) | 25.0 | 74.425 | 202 | 33.0(0.) | 2.6(0.1) | 560(22) |
| $HC_5N$ | 40 − 39 | 106498.910(7e-3) | 104.8 | 2249.7 | 39 | 33.0(0.4) | 4.2(0.8) | 173(30) |
| $NH_2CHO$ | 5(2, 3) − 4(2, 2) | 106541.773(37e-3) | 27.2 | 54.915 | 34 | 32.0(0.5) | 6.9(0.9) | 249(36) |
| $C_2H_3CN$ | 11(1, 10) − 10(1, 9) | 106641.383(1e-3) | 32.9 | 476.24 | 35 | 33.0(0.4) | 5.2(1.4) | 194(38) |
| $C_2H_5OH$ | 9(2, 8) − 9(1, 9) | 106723.558(5e-2) | 42.7 | 7.9044 | 31 | 33.0(0.4) | 2.3(0.8) | 78(24) |
| $^{34}SO$ | 3(2) − 2(1) | 106743.244(7e-2) | 20.9 | 3.557 | 60 | 32.7(0.5) | 3.5(0.9) | 220(56) |
| $C_2H_5OH$ | 6(1, 5) − 5(1, 4) | 106767.234(5e-2) | 80.7 | 9.6466 | 36 | 33.0(0.2) | 1.0(0.4) | 37(14) |
| $CH_3OCH_3$ | 9(1, 8) − 8(2, 7) EE | 106777.344(9e-3) | 43.4 | 58.573 | 49 | 32.6(0.4) | 10.6(0.8) | 558(43) |
| $OC^{34}S$ | 9 − 8 | 106787.390(2e-3) | 25.6 | 4.601 | 103 | 33.2(0.1) | 4.6(0.3) | 501(31) |
| $CH_3OH$, vt=0-2 | $3(1)^+ - 4(0)^+$, vt=0 | 107013.831(1e-2) | 28.3 | 12.036 | 533 | 33.0(0.) | 4.8(0.1) | 2747(47) |
| $C_2H_5CN$ | 12(2, 11) − 11(2, 10) | 107043.527(5e-2) | 37.9 | 172.86 | 67 | 33.5(0.) | 5.3(0.5) | 380(35) |
| $CH_3OH$, vt=0-2 | 15(-2) − 15(1) E2, vt=0 | 107159.906(14e-3) | 304.7 | 10.421 | 129 | 33.0(0.1) | 3.9(0.3) | 537(32) |
| $^{13}CH_3CN$ | 6(3) − 5(3) | 107178.424(0) | 82.4 | 276.826 | 31 | 33.8(0.4) | 2.9(1.0) | 96(29) |
| $^{13}CH_3CN$ | 6(2) − 5(2) | 107188.500(1e-1) | 46.6 | 164.068 | 33 | 33.7(0.3) | 2.6(0.6) | 93(23) |
| $^{13}CH_3CN$ | 6(1) − 5(1) | 107194.550(1e-1) | 25.2 | 179.427 | 43 | 33.5(0.7) | 9.8(1.2) | 446(61) |
| $^{13}CH_3CN$ | 6(0) − 5(0) | 107196.570(1e-1) | 18.0 | 184.590 | 36 | 33.5(0.3) | 1.6(0.7) | 62(30) |
| $^{13}C^{17}O$ | 1(2) − 0(3) | 107288.550(5e-2) | 5.1 | 0.016 | 52 | 33.5(0.3) | 1.9(0.7) | 105(53) |
| $^{13}C^{17}O$ | 1(3) − 0(3) | 107289.650(5e-2) | 5.1 | 0.024 | 39 | 33.5(0.8) | 3.7(1.7) | 156(64) |
| $C_2H_5CN$ | 12(7, 5) − 11(7, 4) | 107485.160(5e-2) | 88.0 | 117.36 | 33 | 33.5(0.3) | 2.4(0.7) | 86(34) |
| $C_2H_5CN$ | 12(6, 6) − 11(6, 5) | 107486.949(5e-2) | 73.6 | 133.42 | 84 | 33.5(0.3) | 7.3(0.7) | 656(53) |
| $C_2H_5CN$ | 12(5, 7) − 11(5, 6) | 107502.432(5e-2) | 61.3 | 146.99 | 33 | 33.5(0.5) | 6.4(1.0) | 225(36) |
| $C_2H_5CN$ | 12(10, 2) − 11(10, 1) | 107519.861(5e-2) | 144.6 | 54.355 | 94 | 33.5(0.2) | 7.1(0.5) | 712(41) |
| $CH_3OCHO$ | 9( 2, 8) − 8( 2, 7) E | 107537.258(1e-2) | 28.8 | 22.60702 | 84 | 33.2(0.2) | 4.5(0.5) | 405(36) |
| $CH_3OCHO$ | 9( 2, 8) − 8( 2, 7) A | 107543.711(1e-2) | 28.8 | 22.61344 | 118 | 33.2(0.1) | 4.5(0.3) | 567(33) |
| $C_2H_5CN$ | 12(4, 9) − 11(4, 8) | 107544.042(5e-2) | 51.3 | 158.12 | blended | – | – | – |
| $C_2H_5CN$ | 12(4, 8) − 11(4, 7) | 107547.460(5e-2) | 51.3 | 158.11 | 53 | 33.5(0.3) | 4.7(0.6) | 263(32) |
| $C_2H_5CN$ | 12(3, 10) − 11(3, 9) | 107594.056(5e-2) | 43.6 | 166.77 | 66 | 33.5(0.3) | 6.0(0.7) | 419(39) |
| $C_2H_5CN$ | 12(3, 9) − 11(3, 8) | 107734.723(5e-2) | 43.6 | 166.76 | 63 | 33.5(0.3) | 4.9(0.7) | 327(37) |
| $SO_2$ | 12(4, 8) − 13(3, 11) | 107843.470(2e-3) | 111.0 | 4.5354 | 59 | 33.0(0.3) | 6.2(0.7) | 392(36) |
| t-HCOOH | 5(1, 5) − 4(1, 4) | 108126.720(3e-3) | 18.8 | 9.6966 | 32 | 32.0(0.6) | 7.5(1.7) | 259(43) |
| $^{13}CN$ | 1(1, 1) − 0(1, 0), F = 1 − 1 | 108636.923(5e-2) | 5.2 | 1.932 | 89 | 33.2(0.5) | 4.7(0.5) | 440(18) |
| $^{13}CN$ | 1(2, 1) − 0(1, 1), F = 1 − 0 | 108638.212(5e-2) | 5.2 | 0.722 | blended | – | – | – |
| $^{13}CN$ | 1(2, 1) − 0(1, 1), F = 2 − 1 | 108643.590(5e-2) | 5.2 | 0.856 | 48 | 33.2(0.5) | 1.6(0.5) | 83(18) |
| $^{13}CN$ | 1(2, 1) − 0(1, 1), F = 0 − 1 | 108644.346(5e-2) | 5.2 | 0.642 | 59 | 33.0(0.5) | 3.4(0.5) | 212(18) |
| $^{13}CN$ | 1(2, 1) − 0(1, 1), F = 1 − 1 | 108645.064(5e-2) | 5.2 | 0.551 | blended | – | – | – |
| $^{13}CN$ | 1(1, 1) − 0(1, 0), F = 2 − 1 | 108651.297(5e-2) | 5.2 | 3.276 | 130 | 33.1(0.5) | 3.3(0.5) | 451(18) |
| $^{13}CN$ | 1(2, 1) − 0(1, 1), F = 2 − 2 | 108657.646(5e-2) | 5.2 | 2.420 | 85 | 33.2 (0.5) | 4.6(0.5) | 417(18) |
| $^{13}CN$ | 1(2, 1) − 0(1, 1), F = 1 − 2 | 108658.948(5e-2) | 5.2 | 0.669 | 27 | 33.1(0.5) | 1.1(0.5) | 32(18) |
| $^{13}CN$ | 1(2, 2) − 0(1, 1), F = 3 − 2 | 108780.201(5e-2) | 5.2 | 4.905 | 172 | 33.0 (0.1) | 3.2(0.2) | 593(39) |
| $^{13}CN$ | 1(2, 2) − 0(1, 1), F = 2 − 1 | 108782.374(5e-2) | 5.2 | 2.586 | 88 | 33.1(0.2) | 3.3(0.4) | 306(39) |
| $^{13}CN$ | 1(2, 2) − 0(1, 1), F = 1 − 0 | 108786.982(5e-2) | 5.2 | 1.144 | 34 | 33.0(0.5) | 2.6(0.8) | 96(33) |
| $^{13}CN$ | 1(2, 2) − 0(1, 1), F = 1 − 1 | 108793.753(5e-2) | 5.2 | 0.894 | 42 | 33.0(0.4) | 2.1(0.9) | 95(34) |
| $^{13}CN$ | 1(2, 2) − 0(1, 1), F = 2 − 2 | 108796.400(5e-2) | 5.2 | 0.918 | 58 | 33.1(0.2) | 1.1(0.4) | 67(23) |
| $CH_3OH$, vt=0-2 | 0(0) − 1(-1) E2, vt=0 | 108893.945(12e-3) | 13.1 | 3.9134 | 718 | 33.0(0.) | 4.0(0.1) | 3043(48) |
| $C_2H_5CN$ | 12(2, 10) − 11(2, 9) | 108940.554(5e-2) | 38.2 | 172.93 | blended | – | – | – |
| $C_2H_5CN$ | 11(3, 9) − 12(0, 12) | 108940.696(4e-3) | 38.4 | 0.042598 | 65 | 33.5(0.3) | 4.2(0.6) | 288(44) |
| $O^{13}CS$ | 9 − 8 | 109110.845(2e-3) | 26.2 | 4.605 | 56 | 33.2(0.3) | 3.4(0.7) | 199(35) |
| $CH_3OH$, vt=0-2 | 14(5) − 15(4) E1, vt=0 | 109138.783(15e-3) | 379.7 | 13.593 | 143 | 33.0(0.2) | 4.8(0.3) | 732(50) |
| $CH_3OH$, vt=0-2 | 16(-2) − 16(1) E2, vt=0 | 109153.184(14e-3) | 342.0 | 14.726 | 132 | 33.0(0.2) | 4.4(0.4) | 612(48) |
| $HC_5N$ | 41 − 40 | 109160.973(7e-3) | 110.0 | 2306 | 35 | 33.0(0.4) | 2.2(1.0) | 80(33) |
| $HC_3N$ | 12 − 11 | 109173.634(1e-2) | 34.1 | 167.1 | 3162 | 33.0(0.) | 3.8(0.1) | 12918(46) |
| SO | 3(2) − 2(1) | 109252.220(1e-1) | 21.1 | 3.5585 | 818 | 33.0(0.) | 4.3(0.1) | 3769(52) |
| $HC_3N$, $v_7$=1 | 12(-1) − 11(1) | 109442.013(2e-2) | 355.0 | 165.12 | 72 | 34.1(0.4) | 4.4(0.8) | 337(57) |
| OCS | 9 − 8 | 109463.063(5e-3) | 26.3 | 4.6034 | 618 | 33.0(0.) | 4.3(0.1) | 2857(61) |
| HNCO | 5(1, 5) − 4(1, 4) | 109495.996(6e-3) | 59.0 | 11.847 | 56 | 33.0(0.6) | 4.8(1.2) | 289(62) |
| $CH_3OCH_3$ | 8(2, 7) − 8(1, 8) EA | 109571.396(9e-3) | 38.3 | 23.947 | 41 | 32.5(0.6) | 2.8(1.2) | 120(49) |
| $CH_3OCH_3$ | 8(2, 7) − 8(1, 8) AE | 109571.403(9e-3) | 38.3 | 35.921 | blended | – | – | – |
| $CH_3OCH_3$ | 8(2, 7) − 8(1, 8) EE | 109574.088(7e-3) | 38.3 | 95.791 | 91 | 32.5(0.2) | 1.9(0.5) | 180(42) |
| $CH_3OCH_3$ | 8(2, 7) − 8(1, 8) AA | 109576.778(11e-3) | 38.3 | 59.869 | 44 | 32.5(0.5) | 2.1(0.9) | 98(43) |
| $HC_3N$, $v_7$=1 | 12(1) − 11(-1) | 109598.818(2e-2) | 355.0 | 165.12 | 66 | 34.1(0.5) | 5.0(0.8) | 356(60) |
| $C_2H_5CN$ | 12(1, 11) − 11(1, 10) | 109650.263(5e-2) | 35.4 | 176.49 | 45 | 33.5(0.6) | 4.1(1.0) | 200(58) |
| $C^{18}O$ | 1 − 0 | 109782.173(6e-3) | 5.3 | 0.01221 | 7489 | 33.5(0.1) | 3.3(0.1) | 26201(141) |
| HNCO | 5(2, 3) − 4(2, 2) | 109872.765(3e-2) | 186.1 | 10.012 | 52 | 33.0(0.6) | 3.3(1.2) | 183(64) |
| HNCO | 5(0, 5) − 4(0, 4) | 109905.749(7e-3) | 15.8 | 12.482 | 452 | 33.0(0.1) | 3.9(0.2) | 1882(72) |
| $C^{15}N$ | 1(2, 1) − 0(1, 0) | 110023.540(1e-1) | 5.3 | 1.386 | 46 | 30.2(0.5) | 4.8(1.2) | 238(49) |
| $C^{15}N$ | 1(2, 2) − 0(1, 1) | 110024.590(1e-1) | 5.3 | 3.504 | blended | – | – | – |
| $^{13}CO$ | 1 − 0 | 110201.35(0) | 5.3 | 0.01220 | 10525 | 34.0(0.1) | 5.1(0.1) | 57489(413) |
| HNCO | 5(1, 4) − 4(1, 3) | 110298.089(5e-3) | 59.2 | 11.847 | 67 | 33.0(0.5) | 4.3(0.5) | 310(77) |
| $CH_3CN$ | 6(5, 0) − 5(5, 0) | 110330.345(0) | 197.1 | 56.399 | 81 | 33.0(0.5) | 6.3(0.5) | 539(77) |
| $CH_3CN$ | 6(4, 0) − 5(4, 0) | 110349.471(0) | 132.8 | 102.54 | 177 | 33.0(0.5) | 5.6(0.5) | 1045(77) |
| $CH_3CN$ | 6(3, 0) − 5(-3, 0) | 110364.354(0) | 82.8 | 138.45 | 415 | 33.0(0.5) | 5.3(0.5) | 2357(77) |

**Table A2.** (Continued)

| Species | Transitions | Rest Freq. (MHz) | $E_u$ (K) | $\mu^2S$ ($D^2$) | $T_{mb}$ (mK) | $V_{LSR}$ (km $s^{-1}$) | $\Delta V$ (km $s^{-1}$) | $\int T_{mb}$ dv (mK km $s^{-1}$) |
|---|---|---|---|---|---|---|---|---|
| $CH_3CN$ | 6(-3, 0) − 5(3, 0) | 110364.354(0) | 82.8 | 138.45 | blended | – | – | – |
| $CH_3CN$ | 6(2, 0) − 5(2, 0) | 110374.989(0) | 47.1 | 164.06 | 454 | 33.0(0.5) | 5.2(0.5) | 2495(77) |
| $CH_3CN$ | 6(1, 0) − 5(1, 0) | 110381.372(0) | 25.7 | 179.45 | 648 | 33.0(0.5) | 5.4(0.5) | 3696(77) |
| $CH_3CN$ | 6(0, 0) − 5(0, 0) | 110383.500(0) | 18.5 | 184.58 | 728 | 33.0(0.5) | 3.9(0.5) | 3012(77) |
| $CH_3OCHO$ | 9(7, 3) − 8(7, 2) E | 110536.003(1e-2) | 59.1 | 9.46692 | 53 | 33.2(0.6) | 3.8(1.0) | 214(54) |
| $CH_3OCHO$ | 9(6, 3) − 8(6, 2) E | 110652.813(1e-2) | 50.5 | 13.30853 | 37 | 33.1(0.8) | 2.0(1.9) | 78(50) |
| $CH_3OCHO$ | 9(6, 3) − 8(6, 2) A | 110663.429(1e-2) | 50.4 | 13.31127 | 82 | 33.2(0.4) | 5.1(0.7) | 444(66) |
| $CH_3OCHO$ | 9(6, 4) − 8(6, 3) A | 110663.273(1e-2) | 50.4 | 13.3113 | blended | – | – | – |
| $CH_3OCHO$ | 10(1,10) − 9(1, 9) E | 110788.664(1e-2) | 30.3 | 26.16584 | 109 | 33.2(0.3) | 3.5(0.9) | 402(80) |
| $CH_3OCHO$ | 10(1,10) − 9(1, 9) A | 110790.526(1e-2) | 30.3 | 26.17539 | 99 | 33.2(0.3) | 2.4(0.7) | 250(66) |
| $CH_3OCHO$ | 9(5, 4) − 8(5, 3) E | 110873.955(1e-2) | 43.2 | 16.55557 | 31 | 33.2(0.4) | 1.7(1.2) | 56(40) |
| $CH_3OCHO$ | 9(3, 7) − 8(3, 6) E | 110879.766(1e-2) | 32.6 | 21.245 | 102 | 33.1(0.3) | 4.5(0.6) | 494(68) |
| $CH_3OCHO$ | 9(5, 5) − 8(5, 4) A | 110880.447(1e-2) | 43.2 | 16.56015 | blended | – | – | – |
| $CH_3OCHO$ | 9(5, 5) − 8(5, 4) E | 110882.331(1e-2) | 43.2 | 16.55225 | 61 | 33.1(0.6) | 1.4(0.7) | 87(38) |
| $CH_3OCHO$ | 9(3, 7) − 8(3, 6) A | 110887.092(1e-2) | 32.6 | 21.25577 | 61 | 33.1(0.1) | 2.7(1.1) | 176(57) |
| $CH_3OCHO$ | 9(5, 4) − 8(5, 3) A | 110890.256(1e-2) | 43.2 | 16.56106 | 71 | 33.0(0.5) | 0.7(0.4) | 55(21) |
| $CH_3OCHO$ | 10(0, 10) − 9(0, 9) E | 111169.903(1e-2) | 30.2 | 26.18776 | 114 | 33.0(0.5) | 3.5(0.5) | 427(18) |
| $CH_3OCHO$ | 10(0, 10) − 9(0, 9) A | 111171.634(1e-2) | 30.2 | 26.19136 | 93 | 33.0(0.5) | 3.6(0.5) | 361(18) |
| $CH_3OCHO$ | 9(4, 6) − 8(4, 5) A | 111195.962(1e-2) | 37.2 | 19.21722 | 71 | 33.0(0.5) | 3.4(0.5) | 257(18) |
| $CH_3OCHO$ | 9(4, 6) − 8(4, 5) E | 111223.491(1e-2) | 37.2 | 18.18412 | 67 | 33.0(0.5) | 3.9(0.5) | 275(18) |
| $CH_3OH$, vt=0-2 | $7(2)^+$ − $8(1)^+$, vt=0 | 111289.453(13e-3) | 102.7 | 9.3425 | 286 | 33.0(0.1) | 5.3(0.3) | 1617(69) |
| $CH_3OCHO$ | 9(4, 5) − 8(4, 4) E | 111408.412(1e-2) | 37.3 | 18.18767 | 81 | 33.2(0.2) | 2.7(0.5) | 237(43) |
| $CH_3OCHO$ | 9(4, 5) − 8(4, 4) A | 111453.300(1e-2) | 37.2 | 19.21778 | 61 | 33.2(0.5) | 5.0(0.8) | 319(57) |
| $CH_3OH$, vt=0-2 | 17(-2) − 17(1) E2, vt=0 | 111626.514(15e-3) | 381.5 | 20.231 | 156 | 33.0(0.2) | 4.7(0.4) | 776(54) |
| $CH_3OCHO$ | 9(1, 8) − 8(1, 7) E | 111674.131(1e-2) | 28.1 | 23.18984 | 122 | 33.2(0.2) | 2.4(0.4) | 313(38) |
| $CH_3OCHO$ | 9(1, 8) − 8(1, 7) A | 111682.189(1e-2) | 28.1 | 23.19587 | 118 | 33.0(0.2) | 2.3(0.4) | 291(38) |
| $CH_3OCH_3$ | 19(3, 16) − 19(2, 17) AA | 111744.238(29e-3) | 187.5 | 259.8 | 101 | 33.0(0.4) | 9.4(0.7) | 1012(74) |
| t-HCOOH | 5(0, 5) − 4(0, 4) | 111746.784(3e-3) | 16.1 | 10.092 | 30 | 32.0(0.5) | 1.3(0.6) | 39(24) |
| $CH_3OCH_3$ | 7(0, 7) − 6(1, 6) AA | 111782.562(8e-3) | 25.2 | 68.047 | 233 | 33.0(0.1) | 4.7(0.2) | 1172(55) |
| $CH_3OCH_3$ | 18(3, 15) − 18(2, 16) EE | 111813.668(21e-3) | 115.4 | 386.29 | 918 | 33.0(0.4) | 9.1(0.8) | 890(72) |
| $CH_3CHO$ | 6(1, 6) − 5(1, 5) A, vt=0 | 112248.716(3e-3) | 21.1 | 73.76807 | 106 | 33.0(0.2) | 2.9(0.4) | 330(41) |
| $CH_3CHO$ | 6(1, 6) − 5(1, 5) E, vt=0 | 112254.508(3e-3) | 21.2 | 73.79585 | 108 | 33.0(0.2) | 3.4(0.4) | 394(42) |
| $C^{17}O$ | 1 − 0 | 112359.284(1e-3) | 5.4 | 0.01217 | 2117 | 33.5(0.1) | 4.9(0.1) | 11101(71) |
| $C_2H_5CN$ | 13(1, 13) − 12(1, 12) | 112646.350(9e-2) | 39.0 | 191.45 | 82 | 33.5(0.4) | 3.8(1.1) | 334(63) |
| $CH_3OCH_3$ | 20(3, 17) − 20(2, 18) EE | 113000.970(32e-3) | 206.1 | 55.102 | 102 | 32.7(0.3) | 5.6(0.7) | 609(64) |
| $CH_3OCH_3$ | 17(3, 14) − 17(2, 15) EA | 113057.427(19e-3) | 153.1 | 132.79 | 9.5 | 32.6(0.4) | 4.5(2.0) | 455(140) |
| $CH_3OCH_3$ | 17(3, 14) − 17(2, 15) AE | 113057.425(18e-3) | 153.1 | 88.525 | blended | – | – | – |
| $CH_3OCH_3$ | 17(3, 14) − 17(2, 15) EE | 113059.249(17e-3) | 153.1 | 354.12 | 113 | 32.6(0.3) | 2.4(0.7) | 295(102) |
| $CH_3OCH_3$ | 17(3, 14) − 17(2, 15) AA | 113061.072(22e-3) | 153.1 | 221.33 | 77 | 32.7(0.3) | 1.9(0.5) | 153(38) |
| CN | N= 1-0, J=1/2-1/2, F=1/2-1/2 | 113123.370(6e-3) | 5.4 | 0.15271 | 646 | 34.5(0.5) | 3.7(0.5) | 2518(93) |
| CN | N= 1-0, J=1/2-1/2, F=1/2-3/2 | 113144.157(6e-3) | 5.4 | 1.2492 | 770 | 34.6(0.5) | 2.3(0.5) | 1898(93) |
| CN | N= 1-0, J=1/2-1/2, F=3/2-1/2 | 113170.492(4e-3) | 5.4 | 1.2199 | 981 | 34.6(0.5) | 2.2(0.5) | 2290(93) |
| CN | N= 1-0, J=1/2-1/2, F=3/2-3/2 | 113191.279(3e-3) | 5.4 | 1.5836 | 869 | 34.5(0.5) | 2.2(0.5) | 2032(93) |
| CN | N= 1-0, J=3/2-1/2, F=3/2-1/2 | 113488.120(3e-3) | 5.4 | 1.5836 | 642 | 34.5(0.5) | 4.8(0.5) | 3285(138) |
| CN | N= 1-0, J=3/2-1/2, F=5/2-3/2 | 113490.970(2e-3) | 5.4 | 4.205 | 1779 | 34.5(0.5) | 2.0(0.5) | 3870(138) |
| CN | N= 1-0, J=3/2-1/2, F=1/2-1/2 | 113499.644(3e-3) | 5.4 | 1.2491 | 411 | 34.6(0.5) | 2.3(0.5) | 1010(138) |
| CN | N= 1-0, J=3/2-1/2, F=3/2-3/2 | 113508.907(3e-3) | 5.4 | 1.2196 | 781 | 34.6(0.5) | 2.4(0.5) | 1978(138) |
| CN | N= 1-0, J=3/2-1/2, F=1/2-3/2 | 113520.432(4e-3) | 5.4 | 0.15263 | 153 | 34.6(0.5) | 1.8(0.5) | 294(138) |
| | | | | G012.90−00.24 | | | | |
| $CH_3OH$, vt=0-2 | 0(0) − 1(-1) E2, vt=0 | 108893.945(12e-3) | 13.1 | 3.9134 | 237 | 37.0(0.1) | 3.3(0.3) | 830(59) |
| $HC_3N$ | 12 − 11 | 109173.634(1e-2) | 34.1 | 167.1 | 576 | 36.4(0.) | 2.5(0.1) | 1533(62) |
| SO | 3(2) − 2(1) | 109252.220(1e-1) | 21.1 | 3.5585 | 140 | 36.5(0.2) | 1.5(0.5) | 222(58) |
| OCS | 9 − 8 | 109463.063(5e-3) | 26.3 | 4.6034 | 70 | 37.4(0.6) | 2.1(1.7) | 154(87) |
| $C^{18}O$ | 1 − 0 | 109782.173(6e-3) | 5.3 | 0.01221 | 6057 | 36.5(0.5) | 3.1(0.5) | 19937(495) |
| HNCO | 5(0, 5) − 4(0, 4) | 109905.749(7e-3) | 15.8 | 12.482 | 490 | 34.5(0.1) | 2.8(0.1) | 1436(73) |
| $^{13}CO$ | 1 − 0 | 110201.35(0) | 5.3 | 0.01220 | 16530 | 36.0(0.2) | 4.3(0.4) | 57789(2600) |
| $CH_3CN$ | 6(3, 0) − 5(-3, 0) | 110364.354(0) | 82.8 | 138.45 | 64 | 36.2(0.5) | 2.9(0.5) | 196(27) |
| $CH_3CN$ | 6(-3, 0) − 5(3, 0) | 110364.354(0) | 82.8 | 138.45 | blended | – | – | – |
| $CH_3CN$ | 6(2, 0) − 5(2, 0) | 110374.989(0) | 47.1 | 164.06 | 81 | 36.2(0.5) | 0.6(0.4) | 47(27) |
| $CH_3CN$ | 6(1, 0) − 5(1, 0) | 110381.372(0) | 25.7 | 179.45 | 131 | 36.2(0.5) | 2.7(0.5) | 371(27) |
| $CH_3CN$ | 6(0, 0) − 5(0, 0) | 110383.500(0) | 18.5 | 184.58 | 104 | 36.2(0.5) | 4.7(0.5) | 519(27) |
| $C^{17}O$ | 1(2) − 0(3) | 112358.777(2e-2) | 5.4 | 0.01623 | 1746 | 36.2(0.5) | 3.0(0.5) | 5547(265) |
| $C^{17}O$ | 1(4) − 0(3) | 112358.982(15e-3) | 5.4 | 0.03245 | 1351 | 36.1(0.5) | 2.2(0.5) | 3151(265) |
| $C^{17}O$ | 1 − 0 | 112359.284(1e-3) | 5.4 | 0.01217 | 380 | 36.1(0.5) | 1.6(0.5) | 632(265) |
| CN | N= 1-0, J=1/2-1/2, F=1/2-1/2 | 113123.370(6e-3) | 5.4 | 0.15271 | 410 | 37.1(0.5) | 3.0(0.5) | 1312(56) |
| CN | N= 1-0, J=1/2-1/2, F=1/2-3/2 | 113144.157(6e-3) | 5.4 | 1.2492 | 425 | 37.1(0.5) | 2.4(0.5) | 1099(56) |
| CN | N= 1-0, J=1/2-1/2, F=3/2-1/2 | 113170.492(4e-3) | 5.4 | 1.2199 | 505 | 37.1(0.5) | 2.4(0.5) | 1282(56) |
| CN | N= 1-0, J=1/2-1/2, F=3/2-3/2 | 113191.279(3e-3) | 5.4 | 1.5836 | 442 | 37.1(0.5) | 2.8(0.5) | 1322(56) |
| CN | N= 1-0, J=3/2-1/2, F=3/2-1/2 | 113488.120(3e-3) | 5.4 | 1.5836 | 331 | 37.3(0.2) | 4.2(0.6) | 1484(149) |
| CN | N= 1-0, J=3/2-1/2, F=5/2-3/2 | 113490.970(2e-3) | 5.4 | 4.205 | 609 | 37.4(0.) | 2.8(0.3) | 1839(121) |
| CN | N= 1-0, J=3/2-1/2, F=1/2-1/2 | 113499.644(3e-3) | 5.4 | 1.2491 | 220 | 37.3(0.3) | 4.5(1.1) | 1060(169) |
| CN | N= 1-0, J=3/2-1/2, F=3/2-3/2 | 113508.907(3e-3) | 5.4 | 1.2196 | 487 | 37.3(0.1) | 2.8(0.3) | 1426(128) |
| CN | N= 1-0, J=3/2-1/2, F=1/2-3/2 | 113520.432(4e-3) | 5.4 | 0.15263 | 257 | 37.3(0.2) | 3.3(0.5) | 901(116) |
| | | | | G012.90−00.26 | | | | |
| $NH_2CHO$ | 5(2, 4) − 4(2, 3) | 105972.665(37e-3) | 27.2 | 54.915 | 46 | 38.5(0.4) | 4.9(1.0) | 242(40) |
| CCS | 8(9) − 7(8) | 106347.726(2e-2) | 25.0 | 74.425 | 102 | 37.1(0.2) | 4.1(0.5) | 446(43) |
| $NH_2CHO$ | 5(2, 3) − 4(2, 2) | 106541.773(37e-3) | 27.2 | 54.915 | 33 | 38.4(0.7) | 7.5(1.2) | 259(46) |
| $^{34}SO$ | 3(2) − 2(1) | 106743.244(7e-2) | 20.9 | 3.557 | 48 | 37.3(0.3) | 3.2(1.0) | 167(37) |
| $CH_3OCH_3$ | 9(1, 8) − 8(2, 7) EE | 106777.344(9e-3) | 43.4 | 58.573 | 30 | 37.0(0.8) | 10.0(1.5) | 310(49) |
| $OC^{34}S$ | 9 − 8 | 106787.390(2e-3) | 25.6 | 4.601 | 60 | 38.8(0.3) | 3.3(0.6) | 212(33) |
| $CH_3OH$, vt=0-2 | $3(1)^+$ − $4(0)^+$, vt=0 | 107013.831(1e-2) | 28.3 | 12.036 | 1712 | 38.5(0.) | 2.5(0.1) | 4602(70) |
| $CH_3OH$, vt=0-2 | 15(-2) − 15(1) E2, vt=0 | 107159.906(14e-3) | 304.7 | 10.421 | 81 | 38.5(0.2) | 3.3(0.4) | 285(32) |
| $C_2H_5CN$ | 12(7, 5) − 11(7, 4) | 107485.160(5e-2) | 88.0 | 117.36 | 27 | 38.1(0.4) | 1.8(0.7) | 53(26) |
| $C_2H_5CN$ | 12(6, 6) − 11(6, 5) | 107486.949(5e-2) | 73.6 | 133.42 | 31 | 38.0(1.1) | 12.1(2.5) | 409(74) |
| $C_2H_5CN$ | 12(5, 7) − 11(5, 6) | 107502.432(5e-2) | 61.3 | 146.99 | 16 | 38.0(1.8) | 8.2(2.9) | 139(54) |
| $C_2H_5CN$ | 12(10, 2) − 11(10, 1) | 107519.861(5e-2) | 144.6 | 54.355 | 35 | 38.1(0.9) | 9.3(2.5) | 341(66) |
| $CH_3OCHO$ | 9( 2, 8) − 8( 2, 7) E | 107537.258(1e-2) | 28.8 | 22.60702 | 60 | 38.1(0.3) | 3.6(0.6) | 228(35) |
| $CH_3OCHO$ | 9( 2, 8) − 8( 2, 7) A | 107543.711(1e-2) | 28.8 | 22.61344 | 83 | 38.1(0.2) | 3.0(0.6) | 268(38) |
| $C_2H_5CN$ | 12(4, 9) − 11(4, 8) | 107544.042(5e-2) | 51.3 | 158.12 | blended | – | – | – |
| $C_2H_5CN$ | 12(4, 8) − 11(4, 7) | 107547.460(5e-2) | 51.3 | 158.11 | 39 | 38.1(0.5) | 5.7(1.5) | 240(47) |
| $C_2H_5CN$ | 12(3, 10) − 11(3, 9) | 107594.056(5e-2) | 43.6 | 166.77 | 49 | 38.1(0.4) | 6.6(1.4) | 340(53) |
| $SO_2$ | 12(4, 8) − 13(3, 11) | 107843.470(2e-3) | 111.0 | 4.5354 | 68 | 37.8(0.3) | 4.5(0.7) | 326(42) |
| $^{13}CN$ | 1(1, 1) − 0(1, 0), F = 0 − 1 | 108631.121(5e-2) | 5.2 | 0.642 | 54 | 37.7(0.2) | 1.0(0.6) | 58(26) |
| $^{13}CN$ | 1(1, 1) − 0(1, 0), F = 1 − 1 | 108636.923(5e-2) | 5.2 | 1.932 | 16 | 37.6(2.9) | 4.1(3.2) | 69(71) |
| $^{13}CN$ | 1(2, 1) − 0(1, 1), F = 1 − 0 | 108638.212(5e-2) | 5.2 | 0.722 | 60 | 37.6(0.7) | 4.5(1.3) | 287(87) |
| $^{13}CN$ | 1(2, 1) − 0(1, 1), F = 2 − 1 | 108643.590(5e-2) | 5.2 | 0.856 | 18 | 37.5(1.3) | 2.0(1.7) | 90(39) |
| $^{13}CN$ | 1(2, 1) − 0(1, 1), F = 0 − 1 | 108644.346(5e-2) | 5.2 | 0.642 | 52 | 37.5(1.0) | 3.8(1.5) | 211(102) |
| $^{13}CN$ | 1(2, 1) − 0(1, 1), F = 1 − 1 | 108645.064(5e-2) | 5.2 | 0.551 | blended | – | – | – |

**Table A2.** (Continued)

| Species | Transitions | Rest Freq. (MHz) | $E_u$ (K) | $\mu^2S$ ($D^2$) | $T_{mb}$ (mK) | $V_{LSR}$ (km $s^{-1}$) | $\Delta V$ (km $s^{-1}$) | $\int T_{mb}$ dv (mK km $s^{-1}$) |
|---|---|---|---|---|---|---|---|---|
| $^{13}CN$ | 1(1, 1) − 0(1, 0), F = 2 − 1 | 108651.297(5e-2) | 5.2 | 3.276 | 116 | 37.5(0.1) | 3.3(0.3) | 404(35) |
| $^{13}CN$ | 1(2, 1) − 0(1, 1), F = 2 − 2 | 108657.646(5e-2) | 5.2 | 2.420 | 95 | 37.6(0.2) | 3.1(0.4) | 311(33) |
| $^{13}CN$ | 1(2, 1) − 0(1, 1), F = 1 − 2 | 108658.948(5e-2) | 5.2 | 0.669 | 36 | 37.5(0.3) | 1.2(1.1) | 46(28) |
| $^{13}CN$ | 1(2, 2) − 0(1, 1), F = 3 − 2 | 108780.201(5e-2) | 5.2 | 4.905 | 147 | 37.5(0.1) | 3.6(0.3) | 557(46) |
| $^{13}CN$ | 1(2, 2) − 0(1, 1), F = 2 − 1 | 108782.374(5e-2) | 5.2 | 2.586 | 76 | 37.4(0.3) | 3.1(0.7) | 253(45) |
| $^{13}CN$ | 1(2, 2) − 0(1, 1), F = 1 − 0 | 108786.982(5e-2) | 5.2 | 1.144 | 28 | 37.4(0.7) | 3.3(1.9) | 98(45) |
| $^{13}CN$ | 1(2, 2) − 0(1, 1), F = 1 − 1 | 108793.753(5e-2) | 5.2 | 0.894 | 53 | 37.5(0.3) | 0.7(0.4) | 40(23) |
| $^{13}CN$ | 1(2, 2) − 0(1, 1), F = 2 − 2 | 108796.400(5e-2) | 5.2 | 0.918 | 38 | 37.5(0.4) | 0.8(0.5) | 34(22) |
| $CH_3OH$, vt=0-2 | 0(0) − 1(-1) E2, vt=0 | 108893.945(12e-3) | 13.1 | 3.9134 | 840 | 38.3(0.) | 6.8(0.1) | 6050(85) |
| $C_2H_5CN$ | 12(2, 10) − 11(2, 9) | 108940.554(5e-2) | 38.2 | 172.93 | 49 | 38.1(0.5) | 2.9(1.0) | 154(42) |
| $CH_3OH$, vt=0-2 | 14(5) − 15(4) E1, vt=0 | 109138.783(15e-3) | 379.7 | 13.593 | 114 | 38.1(0.2) | 2.9(0.3) | 348(38) |
| $CH_3OH$, vt=0-2 | 16(-2) − 16(1) E2, vt=0 | 109153.184(14e-3) | 342.0 | 14.726 | 57 | 38.3(0.4) | 3.9(0.7) | 238(36) |
| $HC_3N$ | 12 − 11 | 109173.634(1e-2) | 34.1 | 167.1 | 2872 | 37.0(0.) | 4.2(0.1) | 12789(86) |
| SO | 3(2) − 2(1) | 109252.220(1e-1) | 21.1 | 3.5585 | 552 | 37.5(0.) | 5.8(0.2) | 3400(70) |
| $HC_3N$, $v_7$=1 | 12(-1) − 11(1) | 109442.013(2e-2) | 355.0 | 165.12 | 63 | 37.5(0.4) | 4.2(0.8) | 279(54) |
| OCS | 9 − 8 | 109463.063(5e-3) | 26.3 | 4.6034 | 525 | 38.1(0.) | 5.4(0.1) | 3009(67) |
| HNCO | 5(1, 5) − 4(1, 4) | 109495.996(6e-3) | 59.0 | 11.847 | 69 | 38.5(0.4) | 4.5(0.9) | 328(56) |
| $CH_3OCH_3$ | 8(2, 7) − 8(1, 8) EE | 109574.088(7e-3) | 38.3 | 95.791 | 56 | 37.8(0.4) | 2.1(0.7) | 126(39) |
| $CH_3OCH_3$ | 8(2, 7) − 8(1, 8) EA | 109571.396(9e-3) | 38.3 | 23.947 | 54 | 37.8(0.4) | 2.8(0.7) | 161(44) |
| $CH_3OCH_3$ | 8(2, 7) − 8(1, 8) AE | 109571.403(9e-3) | 38.3 | 35.921 | blended | – | – | – |
| $CH_3OCH_3$ | 8(2, 7) − 8(1, 8) AA | 109576.778(11e-3) | 38.3 | 59.869 | 27 | 37.8(0.8) | 2.1(1.1) | 71(40) |
| $HC_3N$, $v_7$=1 | 12(1) − 11(-1) | 109598.818(2e-2) | 355.0 | 165.12 | 55 | 1.5 | 3.7(0.9) | 215(52) |
| $C_2H_5CN$ | 12(1, 11) − 11(1, 10) | 109650.263(5e-2) | 35.4 | 176.49 | 31 | 38.0(0.5) | 1.8(0.9) | 60(31) |
| $C^{18}O$ | 1 − 0 | 109782.173(6e-3) | 5.3 | 0.01221 | 5262 | 36.0(0.1) | 4.8(0.1) | 27091(269) |
| HNCO | 5(2, 3) − 4(2, 2) | 109872.765(3e-2) | 186.1 | 10.013 | 51 | 38.5(0.9) | 3.6(1.5) | 195(79) |
| HNCO | 5(2, 4) − 4(2, 3) | 109872.337(3e-2) | 186.1 | 10.012 | blended | – | – | – |
| HNCO | 5(0, 5) − 4(0, 4) | 109905.749(7e-3) | 15.8 | 12.482 | 700 | 38.5(0.1) | 6.3(0.2) | 4725(115) |
| $^{13}CO$ | 1 − 0 | 110201.35(0) | 5.3 | 0.01220 | 10821 | 36.2(0.5) | 6.8(0.5) | 78474(1440) |
| HNCO | 5(1, 4) − 4(1, 3) | 110298.089(5e-3) | 59.2 | 11.847 | 83 | 38.5(0.4) | 4.8(1.6) | 428(97) |
| $CH_3CN$ | 6(5, 0) − 5(5, 0) | 110330.345(0) | 197.1 | 56.399 | 55 | 38.0(0.6) | 5.8(1.4) | 336(76) |
| $CH_3CN$ | 6(4, 0) − 5(4, 0) | 110349.471(0) | 132.8 | 102.54 | 163 | 38.0(0.2) | 4.4(0.5) | 755(69) |
| $CH_3CN$ | 6(3, 0) − 5(-3, 0) | 110364.354(0) | 82.8 | 138.45 | 410 | 38.0(0.1) | 5.5(0.2) | 2412(76) |
| $CH_3CN$ | 6(-3, 0) − 5(3, 0) | 110364.354(0) | 82.8 | 138.45 | blended | – | – | – |
| $CH_3CN$ | 6(2, 0) − 5(2, 0) | 110374.989(0) | 47.1 | 164.06 | 445 | 38.0(0.1) | 5.3(0.2) | 2492(73) |
| $CH_3CN$ | 6(1, 0) − 5(1, 0) | 110381.372(0) | 25.7 | 179.45 | 700 | 38.0(0.1) | 5.1(0.2) | 3765(151) |
| $CH_3CN$ | 6(0, 0) − 5(0, 0) | 110383.500(0) | 18.5 | 184.58 | 762 | 38.0(0.1) | 5.3(0.2) | 4303(151) |
| $CH_3OCHO$ | 9(6, 3) − 8(6, 2) E | 110652.813(1e-2) | 50.5 | 13.30853 | 20 | 38.0(1.1) | 2.2(1.4) | 48(47) |
| $CH_3OCHO$ | 9(6, 3) − 8(6, 2) A | 110663.429(1e-2) | 50.4 | 13.31127 | 55 | 38.0(0.5) | 4.0(0.8) | 233(52) |
| $CH_3OCHO$ | 9(6, 4) − 8(6, 3) A | 110663.273(1e-2) | 50.4 | 13.3113 | blended | – | – | – |
| $CH_3OCHO$ | 10(1,10) − 9(1, 9) E | 110788.664(1e-2) | 30.3 | 26.16584 | 38 | 38.0(0.7) | 2.9(1.3) | 121(50) |
| $CH_3OCHO$ | 10(1,10) − 9(1, 9) A | 110790.526(1e-2) | 30.3 | 26.17539 | 78 | 38.0(0.3) | 1.5(1.1) | 126(52) |
| $CH_3OCHO$ | 9(5, 4) − 8(5, 3) E | 110873.955(1e-2) | 43.2 | 16.55557 | 97 | 38.0(0.1) | 0.5 (0.1) | 56(24) |
| $CH_3OCHO$ | 9(3, 7) − 8(3, 6) E | 110879.766(1e-2) | 32.6 | 21.245 | 42 | 38.1(0.6) | 2.9(1.0) | 128(51) |
| $CH_3OCHO$ | 9(5, 5) − 8(5, 4) A | 110880.447(1e-2) | 43.2 | 16.56015 | 38 | 38.1(0.7) | 2.6(1.2) | 105(49) |
| $CH_3OCHO$ | 9(3, 7) − 8(3, 6) A | 110887.092(1e-2) | 32.6 | 21.25577 | 29 | 38.1(0.2) | 0.5(0.2) | 69(25) |
| $CH_3OCHO$ | 9(5, 4) − 8(5, 3) A | 110890.256(1e-2) | 43.2 | 16.56106 | 26 | 38.1(0.8) | 2.1(1.1) | 58(41) |
| $CH_3OCHO$ | 10(0, 10) − 9(0, 9) A | 111171.634(1e-2) | 30.2 | 26.19136 | 57 | 38.0(0.8) | 8.7(1.8) | 532(108) |
| $CH_3OCHO$ | 9(4, 6) − 8(4, 5) A | 111195.962(1e-2) | 37.2 | 19.21722 | 55 | 38.0(0.1) | 0.5(0.1) | 55(28) |
| $CH_3OH$, vt=0-2 | $7(2)^+$ − $8(1)^+$, vt=0 | 111289.453(13e-3) | 102.7 | 9.3425 | 271 | 38.5(0.1) | 4.0(0.3) | 1159(70) |
| $CH_3OCHO$ | 9(4, 5) − 8(4, 4) A | 111453.300(1e-2) | 37.2 | 19.21778 | 43 | 38.1(0.5) | 2.1(1.3) | 97(52) |
| $CH_3OH$, vt=0-2 | 17(-2) − 17(1) E2, vt=0 | 111626.514(15e-3) | 381.5 | 20.231 | 55 | 38.5(0.5) | 4.1(0.9) | 240(59) |
| $CH_3OCHO$ | 9(1, 8) − 8(1, 7) E | 111674.131(1e-2) | 28.1 | 23.18984 | 52 | 38.0(0.5) | 2.6(0.7) | 147(47) |
| $CH_3OCHO$ | 9(1, 8) − 8(1, 7) A | 111682.189(1e-2) | 28.1 | 23.19587 | 62 | 38.0(0.4) | 3.0(0.8) | 195(520 |
| $CH_3OCH_3$ | 19(3, 16) − 19(2, 17) AA | 111744.238(29e-3) | 187.5 | 259.8 | 35 | 37.0(1.2) | 7.9(1.8) | 295(11) |
| $CH_3OCH_3$ | 7(0, 7) − 6(1, 6) AA | 111782.562(8e-3) | 25.2 | 68.047 | 178 | 37.0(0.2) | 4.8(0.4) | 902(69) |
| $CH_3CHO$ | 6(1, 6) − 5(1, 5) A, vt=0 | 112248.716(3e-3) | 21.1 | 73.76807 | 129 | 37.4(0.3) | 6.3(0.9) | 863(88) |
| $CH_3CHO$ | 6(1, 6) − 5(1, 5) E, vt=0 | 112254.508(3e-3) | 21.2 | 73.79585 | 133 | 37.4(0.2) | 5.0(0.6) | 704(71) |
| $C^{17}O$ | 1 − 0 | 112359.284(1e-3) | 5.4 | 0.01217 | 1534 | 36.5(0.1) | 6.0(0.1) | 9781(93) |
| CN | N= 1-0, J=1/2-1/2, F=1/2-1/2 | 113123.370(6e-3) | 5.4 | 0.15271 | 539 | 37.5(0.5) | 4.2(0.5) | 2424(125) |
| CN | N= 1-0, J=1/2-1/2, F=1/2-3/2 | 113144.157(6e-3) | 5.4 | 1.2492 | 796 | 37.4(0.5) | 5.6(0.5) | 4740(125) |
| CN | N= 1-0, J=1/2-1/2, F=3/2-1/2 | 113170.492(4e-3) | 5.4 | 1.2199 | 1108 | 37.5(0.5) | 5.2(0.5) | 6080(125) |
| CN | N= 1-0, J=1/2-1/2, F=3/2-3/2 | 113191.279(3e-3) | 5.4 | 1.5836 | 743 | 37.5(0.5) | 6.1(0.5) | 4797(125) |
| CN | N= 1-0, J=3/2-1/2, F=3/2-1/2 | 113488.120(3e-3) | 5.4 | 1.5838 | 698 | 37.3(0.5) | 3.9(0.5) | 2874(146) |
| CN | N= 1-0, J=3/2-1/2, F=5/2-3/2 | 113490.970(2e-3) | 5.4 | 4.205 | 1209 | 37.3(0.5) | 1.7(0.5) | 2186(146) |
| CN | N= 1-0, J=3/2-1/2, F=1/2-1/2 | 113499.644(3e-3) | 5.4 | 1.2491 | 508 | 37.3(0.5) | 4.3(0.5) | 2344(146) |
| CN | N= 1-0, J=3/2-1/2, F=3/2-3/2 | 113508.907(3e-3) | 5.4 | 1.2196 | 800 | 37.5(0.5) | 4.9(0.5) | 4170(146) |
| CN | N= 1-0, J=3/2-1/2, F=1/2-3/2 | 113520.432(4e-3) | 5.4 | 0.15263 | 260 | 37.5(0.5) | 4.8(0.5) | 1321(146) |
| | | **G014.33−00.64** | | | | | | |
| $NH_2CHO$ | 5(2, 4) − 4(2, 3) | 105972.665(37e-3) | 27.2 | 54.915 | 51 | 21.2(0.5) | 2.7(0.8) | 149(45) |
| CCS | 8(9) − 7(8) | 106347.726(2e-2) | 25.0 | 74.425 | 142 | 22.0(0.2) | 2.9(0.4) | 433(50) |
| $HC_5N$ | 40 − 39 | 106498.910(7e-3) | 104.8 | 2249.7 | 49 | 22.3(0.5) | 1.9(1.1) | 100(41) |
| $CH_3OCH_3$ | 9(1, 8) − 8(2, 7) AA | 106775.602(14e-3) | 43.4 | 36.603 | 58 | 22.0(0.3) | 2.2(0.7) | 136(40) |
| $CH_3OCH_3$ | 9(1, 8) − 8(2, 7) EE | 106777.344(9e-3) | 43.4 | 58.573 | 79 | 22.0(0.2) | 1.7(0.8) | 146(47) |
| $OC^{34}S$ | 9 − 8 | 106787.390(2e-3) | 25.6 | 4.601 | 67 | 22.9(0.3) | 2.5(1.2) | 178(55) |
| $CH_3OH$, vt=0-2 | $3(1)^+$ − $4(0)^+$, vt=0 | 107013.831(1e-2) | 28.3 | 12.036 | 553 | 22.5(0.) | 3.2(0.1) | 1856(52) |
| $CH_3OH$, vt=0-2 | 15(-2) − 15(1) E2, vt=0 | 107159.906(14e-3) | 304.7 | 10.421 | 45 | 22.5(0.7) | 4.5(1.5) | 216(61) |
| $CH_3OCHO$ | 9( 2, 8) − 8( 2, 7) E | 107537.258(1e-2) | 28.8 | 22.60702 | 117 | 22.1(0.2) | 3.4(0.6) | 417(57) |
| $CH_3OCHO$ | 9( 2, 8) − 8( 2, 7) A | 107543.711(1e-2) | 28.8 | 22.61344 | 96 | 22.1(0.3) | 4.3(1.1) | 443(75) |
| t-HCOOH | 5(1, 5) − 4(1, 4) | 108126.720(3e-3) | 18.8 | 9.6966 | 55 | 21.5(0.9) | 9.6(4.0) | 565(144) |
| $^{13}CN$ | 1(1, 1) − 0(1, 0), F = 0 − 1 | 108631.121(5e-2) | 5.2 | 0.642 | 36 | 23.7(0.4) | 1.2(1.1) | 44(33) |
| $^{13}CN$ | 1(1, 1) − 0(1, 0), F = 1 − 1 | 108636.923(5e-2) | 5.2 | 1.932 | 188 | 23.5(0.1) | 0.5(0.3) | 108(27) |
| $^{13}CN$ | 1(2, 1) − 0(1, 1), F = 1 − 0 | 108638.212(5e-2) | 5.2 | 0.722 | 51 | 23.5(0.7) | 5.7(1.5) | 314(72) |
| $^{13}CN$ | 1(2, 1) − 0(1, 1), F = 2 − 1 | 108643.590(5e-2) | 5.2 | 0.856 | 60 | 23.5(0.5) | 3.7(1.1) | 237(66) |
| $^{13}CN$ | 1(2, 1) − 0(1, 1), F = 0 − 1 | 108644.346(5e-2) | 5.2 | 0.642 | 52 | 23.4(0.5) | 2.5(0.8) | 136(54) |
| $^{13}CN$ | 1(2, 1) − 0(1, 1), F = 1 − 1 | 108645.064(5e-2) | 5.2 | 0.551 | blended | – | – | – |
| $^{13}CN$ | 1(1, 1) − 0(1, 0), F = 2 − 1 | 108651.297(5e-2) | 5.2 | 3.276 | 168 | 23.6(0.1) | 2.8(0.3) | 504(48) |
| $^{13}CN$ | 1(2, 1) − 0(1, 1), F = 2 − 2 | 108657.646(5e-2) | 5.2 | 2.420 | 107 | 23.5(0.2) | 2.8(0.6) | 314(53) |
| $^{13}CN$ | 1(2, 1) − 0(1, 1), F = 1 − 2 | 108658.948(5e-2) | 5.2 | 0.669 | 82 | 23.4(0.3) | 0.6(0.3) | 50(23) |
| $^{13}CN$ | 1(2, 2) − 0(1, 1), F = 3 − 2 | 108780.201(5e-2) | 5.2 | 4.905 | 228 | 23.5(0.1) | 2.2(0.3) | 545(53) |
| $^{13}CN$ | 1(2, 2) − 0(1, 1), F = 2 − 1 | 108782.374(5e-2) | 5.2 | 2.586 | 92 | 23.5(0.3) | 2.6(0.6) | 254(56) |
| $^{13}CN$ | 1(2, 2) − 0(1, 1), F = 1 − 0 | 108786.982(5e-2) | 5.2 | 1.144 | 76 | 23.5(0.1) | 0.5(0.3) | 44(25) |
| $^{13}CN$ | 1(2, 2) − 0(1, 1), F = 1 − 1 | 108793.753(5e-2) | 5.2 | 0.894 | 64 | 23.4(0.4) | 2.1(0.8) | 141(50) |
| $^{13}CN$ | 1(2, 2) − 0(1, 1), F = 2 − 2 | 108796.400(5e-2) | 5.2 | 0.918 | 30 | 23.4(0.9) | 3.3(1.8) | 105(62) |
| $CH_3OH$, vt=0-2 | 0(0) − 1(-1) E2, vt=0 | 108893.945(12e-3) | 13.1 | 3.9134 | 999 | 22.5(0.1) | 4.2(0.1) | 4456(95) |
| $CH_3OH$, vt=0-2 | 16(-2) − 16(1) E2, vt=0 | 109153.184 (14e-3) | 342.0 | 14.726 | 73 | 22.5(0.5) | 5.3(0.9) | 411(71) |
| $HC_5N$ | 41 − 40 | 109160.973(7e-3) | 110.0 | 2306 | 58 | 22.0(0.5) | 3.5(0.9) | 217(56) |
| $HC_3N$ | 12 − 11 | 109173.634(1e-2) | 34.1 | 167.1 | 4927 | 22.0(0.) | 3.1(0.1) | 16177(166) |
| SO | 3(2) − 2(1) | 109252.220(1e-1) | 21.1 | 3.5585 | 1628 | 22.0(0.) | 3.4(0.1) | 5825(146) |

**Table A2.** (Continued)

| Species | Transitions | Rest Freq. (MHz) | $E_u$ (K) | $\mu^2S$ ($D^2$) | $T_{mb}$ (mK) | $V_{LSR}$ (km $s^{-1}$) | $\Delta V$ (km $s^{-1}$) | $\int T_{mb}\,dv$ (mK km $s^{-1}$) |
|---|---|---|---|---|---|---|---|---|
| OCS | 9 − 8 | 109463.063(5e-3) | 26.3 | 4.6034 | 727 | 22.0(0.) | 3.8(0.1) | 2940(71) |
| $C^{18}O$ | 1 − 0 | 109782.173(6e-3) | 5.3 | 0.01221 | 3616 | 22.5(0.1) | 2.6(0.1) | 9898(91) |
| HNCO | 5(0, 5) − 4(0, 4) | 109905.749(7e-3) | 15.8 | 12.482 | 760 | 22.3(0.1) | 3.9(0.1) | 3140(93) |
| $C^{15}N$ | 1(2, 1) − 0(1, 0) | 110023.540(1e-1) | 5.3 | 1.386 | 63 | 21.6(0.4) | 0.6(0.2) | 40(34) |
| $C^{15}N$ | 1(2, 2) − 0(1, 1) | 110024.590(1e-1) | 5.3 | 3.504 | 70 | 22.0(0.5) | 2.9(1.3) | 216(77) |
| $^{13}CO$ | 1 − 0 | 110201.35(0) | 5.3 | 0.01220 | 11615 | 22.5(0.5) | 2.9(0.5) | 35311(1170) |
| $CH_3CN$ | 6(4, 0) − 5(4, 0) | 110349.471(0) | 132.8 | 102.54 | 109 | 21.8(0.5) | 5.1(0.5) | 596(87) |
| $CH_3CN$ | 6(3, 0) − 5(-3, 0) | 110364.354(0) | 82.8 | 138.45 | 357 | 21.6(0.5) | 4.5(0.5) | 1721(87) |
| $CH_3CN$ | 6(-3, 0) − 5(3, 0) | 110364.354(0) | 82.8 | 138.45 | blended | − | − | − |
| $CH_3CN$ | 6(2, 0) − 5(2, 0) | 1103749.89(0) | 47.1 | 164.06 | 442 | 21.6(0.5) | 4.2(0.5) | 1957(87) |
| $CH_3CN$ | 6(1, 0) − 5(1, 0) | 110381.372(0) | 25.7 | 179.45 | 760 | 21.7(0.5) | 4.0(0.5) | 3205(87) |
| $CH_3CN$ | 6(0, 0) − 5(0, 0) | 110383.500(0) | 18.5 | 184.58 | 949 | 21.7(0.5) | 3.8(0.5) | 3871(87) |
| $CH_3OCHO$ | 9(8, 1) − 8(8, 0) E | 110447.180(1e-2) | 69.0 | 5.02983 | 81 | 22.0(0.) | 0.6(0.3) | 78(26) |
| $CH_3OCHO$ | 9(8, 1) − 8(8, 0) A | 110455.372(1e-2) | 69.0 | 5.02998 | 87 | 22.0(0.2) | 1.1(0.9) | 102(52) |
| $CH_3OCHO$ | 9(8, 2) − 8(8, 1) E | 110458.014(1e-2) | 69.0 | 5.02965 | 63 | 22.0(0.1) | 0.7(0.5) | 36(17) |
| $CH_3OCHO$ | 9(6, 3) − 8(6, 2) E | 110652.813(1e-2) | 50.5 | 13.30853 | 52 | 22.0(0.5) | 2.5(1.0) | 14947(47) |
| $CH_3OCHO$ | 10(0,10) − 9(0, 9) E | 110655.310(1e-2) | 217.2 | 26.25577 | 50 | 22.0(0.5) | 1.4(0.5) | 77(43) |
| $CH_3OCHO$ | 9(6, 3) − 8(6, 2) A | 110663.429(1e-2) | 50.4 | 13.31127 | 44 | 22.0(1.4) | 3.8(2.5) | 179(145) |
| $CH_3OCHO$ | 9(6, 4) − 8(6, 3) A | 110663.273(1e-2) | 50.4 | 13.3113 | 92 | 22.0(0.7) | 4.4(1.6) | 429(154) |
| $CH_3OCHO$ | 10(1,10) − 9(1, 9) E | 110788.664(1e-2) | 30.3 | 26.16584 | 83 | 22.2(0.5) | 1.6(0.5) | 140(24) |
| $CH_3OCHO$ | 10(1,10) − 9(1, 9) A | 110790.526(1e-2) | 30.3 | 26.17539 | 143 | 22.2(0.5) | 4.5(0.5) | 678(24) |
| $CH_3OCHO$ | 9(5, 4) − 8(5, 3) E | 110873.955(1e-2) | 43.2 | 16.55557 | 78 | 22.2(0.5) | 4.2(0.5) | 352(24) |
| $CH_3OCHO$ | 9(3, 7) − 8(3, 6) E | 110879.766(1e-2) | 32.6 | 21.245 | 103 | 22.2(0.5) | 4.7(0.5) | 511(24) |
| $CH_3OCHO$ | 9(5, 5) − 8(5, 4) A | 110880.447(1e-2) | 43.2 | 16.56015 | 89 | 22.0(0.5) | 2.3(0.5) | 214(24) |
| $CH_3OCHO$ | 9(3, 7) − 8(3, 6) A | 110887.092(1e-2) | 32.6 | 21.25577 | 80 | 22.0(0.5) | 3.3(0.5) | 278(24) |
| $CH_3OCHO$ | 9(5, 4) − 8(5, 3) A | 110890.256(1e-2) | 43.2 | 16.56106 | 53 | 22.0(0.5) | 8.2(0.5) | 460(24) |
| $CH_3OCHO$ | 10(0, 10) − 9(0, 9) E | 111169.903(1e-2) | 30.2 | 26.18776 | 104 | 22.0(0.4) | 3.9(0.9) | 432(93) |
| $CH_3OCHO$ | 10(0, 10) − 9(0, 9) A | 111171.634(1e-2) | 30.2 | 26.19136 | 121 | 22.0(0.2) | 1.8(0.7) | 226(70) |
| $CH_3OCHO$ | 9(4, 6) − 8(4, 5) A | 111195.962(1e-2) | 37.2 | 19.21722 | 86 | 22.0(0.3) | 1.7(0.6) | 152(56) |
| $CH_3OCHO$ | 9(4, 6) − 8(4, 5) E | 111223.491(1e-2) | 37.2 | 18.18412 | 111 | 22.0(0.2) | 1.1(0.4) | 129(45) |
| $CH_3OH$, vt=0-2 | $7(2)^+ - 8(1)^+$, vt=0 | 111289.453(13e-3) | 102.7 | 9.3425 | 174 | 22.5(0.3) | 4.5(0.8) | 842(106) |
| $CH_3OCHO$ | 9(4, 5) − 8(4, 4) E | 111408.412(1e-2) | 37.3 | 18.18767 | 99 | 22.0(0.3) | 1.4(0.7) | 149(57) |
| $CH_3OCHO$ | 9(4, 5) − 8(4, 4) A | 111453.300(1e-2) | 37.2 | 19.21778 | 70 | 22.0(0.5) | 2.1(0.9) | 160(62) |
| $CH_3OH$, vt=0-2 | 17(-2) − 17(1) E2, vt=0 | 111626.514(15e-3) | 381.5 | 20.231 | 66 | 22.5(0.6) | 4.2(2.6) | 299(116) |
| $CH_3OCHO$ | 9(1, 8) − 8(1, 7) E | 111674.131(1e-2) | 28.1 | 23.18984 | 93 | 22.2(0.4) | 2.4(1.2) | 236(81) |
| $CH_3OCHO$ | 9(1, 8) − 8(1, 7) A | 111682.189(1e-2) | 28.1 | 23.19587 | 85 | 22.2(0.5) | 4.3(1.1) | 387(89) |
| $CH_3OCH_3$ | 7(0, 7) − 6(1, 6) AA | 111782.562(8e-3) | 169.8 | 68.047 | 182 | 22.0(0.2) | 4.9(0.6) | 951(97) |
| $CH_3OCH_3$ | 7(5, 2) − 8(4, 5) AA | 111809.374(33e-3) | 60.6 | 5.12083 | 106 | 22.0(0.4) | 4.1(0.9) | 465(90) |
| $CH_3CHO$ | 6(1, 6) − 5(1, 5) A, vt=0 | 112248.716(3e-3) | 21.1 | 73.76807 | 207 | 21.8(0.2) | 4.7(0.6) | 1034(106) |
| $CH_3CHO$ | 6(1, 6) − 5(1, 5) E, vt=0 | 112254.508(3e-3) | 21.2 | 73.79585 | 253 | 21.8(0.2) | 4.2(0.5) | 1138(105) |
| $C^{17}O$ | 1 − 0 | 112359.284(1e-3) | 5.4 | 0.01217 | 734 | 23.0(0.1) | 3.4(0.2) | 2652(116) |
| CN | N= 1-0, J=1/2-1/2, F=1/2-1/2 | 113123.370(6e-3) | 5.4 | 0.15271 | 684 | 22.5(0.5) | 3.0(0.5) | 2198(136) |
| CN | N= 1-0, J=1/2-1/2, F=1/2-3/2 | 113144.157(6e-3) | 5.4 | 1.2492 | 1289 | 22.5(0.5) | 3.3(0.5) | 4475(136) |
| CN | N= 1-0, J=1/2-1/2, F=3/2-1/2 | 113170.492(4e-3) | 5.4 | 1.2199 | 1513 | 22.7(0.5) | 3.5(0.5) | 5644(136) |
| CN | N= 1-0, J=1/2-1/2, F=3/2-3/2 | 113191.279(3e-3) | 5.4 | 1.5836 | 1300 | 22.7(0.5) | 3.3(0.5) | 4638(136) |
| CN | N= 1-0, J=3/2-1/2, F=3/2-1/2 | 113488.120(3e-3) | 5.4 | 1.5838 | 1378 | 22.7(0.5) | 3.0(0.5) | 4342(191) |
| CN | N= 1-0, J=3/2-1/2, F=5/2-3/2 | 113490.970(2e-3) | 5.4 | 4.205 | 2181 | 22.7(0.5) | 2.1(0.5) | 4897(191) |
| CN | N= 1-0, J=3/2-1/2, F=1/2-1/2 | 113499.644(3e-3) | 5.4 | 1.2491 | 740 | 22.5(0.5) | 3.5(0.5) | 2727(191) |
| CN | N= 1-0, J=3/2-1/2, F=3/2-3/2 | 113508.907(3e-3) | 5.4 | 1.2196 | 1529 | 22.5(0.5) | 3.2(0.5) | 3883(191) |
| CN | N= 1-0, J=3/2-1/2, F=1/2-3/2 | 113520.432(4e-3) | 5.4 | 0.15263 | 457 | 22.5(0.5) | 2.7(0.5) | 1295(191) |
| | | | | G015.03−00.67 | | | | |
| CCS | 8(9) − 7(8) | 106347.726(2e-2) | 25.0 | 74.425 | 49 | 20.0(0.4) | 3.8(0.6) | 198(37) |
| $HC_5N$ | 40 − 39 | 106498.910(7e-3) | 104.8 | 2249.7 | 43 | 19.0(0.4) | 2.2(0.7) | 100(33) |
| H$\alpha$ | H (39) $\alpha$ | 106737.357(0) | − | − | 834 | 15.4(0.2) | 37.5(0.3) | 33252(244) |
| He$\alpha$ | He (39) $\alpha$ | 106780.852(0) | − | − | 86 | 15.4(0.7) | 36.2(1.5) | 3316(131) |
| $CH_3OH$, vt=0-2 | $3(1)^+ - 4(0)^+$, vt=0 | 107013.831(1e-2) | 28.3 | 12.036 | 255 | 20.0(0.1) | 4.8(0.2) | 1297(50) |
| $CH_3OH$, vt=0-2 | 15(-2) − 15(1) E2, vt=0 | 107159.906(14e-3) | 304.7 | 10.421 | 41 | 20.0(0.6) | 4.6(0.9) | 203(45) |
| H$\varepsilon$ | H (65) $\varepsilon$ | 107206.108(0.) | − | − | 48 | 14.4(1.3) | 35.0(2.4) | 1793(126) |
| $^{13}CN$ | 1(1, 1) − 0(1, 0), F = 0 − 1 | 108631.121(5e-2) | 5.2 | 0.642 | 36 | 18.4(0.5) | 2.7(1.1) | 104(37) |
| $^{13}CN$ | 1(1, 1) − 0(1, 0), F = 1 − 1 | 108636.923(5e-2) | 5.2 | 1.932 | 60 | 18.4(0.4) | 2.9(1.0) | 185(53) |
| $^{13}CN$ | 1(2, 1) − 0(1, 1), F = 1 − 0 | 108638.212(5e-2) | 5.2 | 0.722 | 26 | 18.5(0.7) | 1.4(0.9) | 40(37) |
| $^{13}CN$ | 1(2, 1) − 0(1, 1), F = 2 − 1 | 108643.590(5e-2) | 5.2 | 0.856 | 51 | 18.5(0.4) | 2.9(0.8) | 160(40) |
| $^{13}CN$ | 1(2, 1) − 0(1, 1), F = 0 − 1 | 108644.346(5e-2) | 5.2 | 0.642 | 39 | 18.5(0.3) | 1.1(0.7) | 45(29) |
| $^{13}CN$ | 1(2, 1) − 0(1, 1), F = 1 − 1 | 108645.064(5e-2) | 5.2 | 0.551 | 39 | 18.5(0.4) | 1.4(1.1) | 58(33) |
| $^{13}CN$ | 1(1, 1) − 0(1, 0), F = 2 − 1 | 108651.297(5e-2) | 5.2 | 3.276 | 69 | 18.4(0.2) | 2.3(0.5) | 172(33) |
| $^{13}CN$ | 1(2, 1) − 0(1, 1), F = 2 − 2 | 108657.646(5e-2) | 5.2 | 2.420 | 25 | 18.4(0.6) | 1.3(1.0) | 34(30) |
| $^{13}CN$ | 1(2, 1) − 0(1, 1), F = 1 − 2 | 108658.948(5e-2) | 5.2 | 0.669 | 80 | 18.5(0.2) | 1.2(0.4) | 101(36) |
| $^{13}CN$ | 1(2, 2) − 0(1, 1), F = 3 − 2 | 108780.201(5e-2) | 5.2 | 4.905 | 131 | 18.3(0.1) | 2.3(0.4) | 325(42) |
| $^{13}CN$ | 1(2, 2) − 0(1, 1), F = 2 − 1 | 108782.374(5e-2) | 5.2 | 2.586 | 100 | 18.4(0.1) | 1.3(0.3) | 141(28) |
| $^{13}CN$ | 1(2, 2) − 0(1, 1), F = 1 − 0 | 108786.982(5e-2) | 5.2 | 1.144 | 82 | 18.4(0.1) | 0.5(0.3) | 47(17) |
| $^{13}CN$ | 1(2, 2) − 0(1, 1), F = 1 − 1 | 108793.753(5e-2) | 5.2 | 0.894 | 27 | 18.4(0.7) | 3.3(1.6) | 96(42) |
| $^{13}CN$ | 1(2, 2) − 0(1, 1), F = 2 − 2 | 108796.400(5e-2) | 5.2 | 0.918 | 41 | 18.5(0.3) | 1.9(0.7) | 83(29) |
| $CH_3OH$, vt=0-2 | 0(0) − 1(-1) E2, vt=0 | 108893.945(12e-3) | 13.1 | 3.9134 | 141 | 20.0(0.2) | 5.5(0.5) | 823(59) |
| $HC_5N$ | 41 − 40 | 109160.973(7e-3) | 110.0 | 2306 | 53 | 19.2(0.4) | 3.5(1.3) | 194(54) |
| $HC_3N$ | 12 − 11 | 109173.634(1e-2) | 34.1 | 167.1 | 3514 | 19.0(0.) | 2.7(0.1) | 10118(32) |
| SO | 3(2) − 2(1) | 109252.220(1e-1) | 21.1 | 3.5585 | 254 | 19.5(0.1) | 4.1(0.3) | 1116(59) |
| OCS | 9 − 8 | 109463.063(5e-3) | 26.3 | 4.6034 | 77 | 20.0(0.3) | 3.8(0.7) | 315(55) |
| H$\gamma$ | H (55) $\gamma$ | 109536.001(0) | − | − | 95 | 14.3(0.8) | 31.7(1.4) | 3201(144) |
| $C^{18}O$ | 1 − 0 | 109782.173(6e-3) | 5.3 | 0.01221 | 1883 | 19.5(0.1) | 2.7(0.1) | 5380(101) |
| HNCO | 5(0, 5) − 4(0, 4) | 109905.749(7e-3) | 15.8 | 12.482 | 41 | 19.8(0.5) | 3.5(1.2) | 154(51) |
| $C^{15}N$ | 1(2, 1) − 0(1, 0) | 110023.540(1e-1) | 5.3 | 1.386 | 73 | 18.5(0.3) | 2.7(0.6) | 212(48) |
| $C^{15}N$ | 1(2, 2) − 0(1, 1) | 110024.590(1e-1) | 5.3 | 3.504 | blended | − | − | − |
| $^{13}CO$ | 1 − 0 | 110201.35(0) | 5.3 | 0.01220 | 12057 | 19.5(0.5) | 3.4(0.5) | 43274(1090) |
| $CH_3CN$ | 6(3, 0) − 5(-3, 0) | 110364.354(0) | 82.8 | 138.45 | 133 | 20.0(0.2) | 4.1(0.7) | 581(71) |
| $CH_3CN$ | 6(-3, 0) − 5(3, 0) | 110364.354(0) | 82.8 | 138.45 | blended | − | − | − |
| $CH_3CN$ | 6(2, 0) − 5(2, 0) | 110374.989(0) | 47.1 | 164.06 | 183 | 20.0(0.1) | 3.0(0.4) | 588(63) |
| $CH_3CN$ | 6(1, 0) − 5(1, 0) | 110381.372(0) | 25.7 | 179.45 | 297 | 20.0(0.1) | 3.2(0.2) | 1012(61) |
| $CH_3CN$ | 6(0, 0) − 5(0, 0) | 110383.500(0) | 18.5 | 184.58 | 360 | 20.0(0.1) | 2.5(0.2) | 955(52) |
| H$\delta$ | H (60) $\delta$ | 110600.675(0) | − | − | 42 | 18.0(2.0) | 29.9(2.7) | 1331(160) |
| $CH_3OH$, vt=0-2 | $7(2)^+ - 8(1)^+$, vt=0 | 111289.453(13e-3) | 102.7 | 9.3425 | 50 | 20.0(0.9) | 4.4(1.3) | 237(86) |
| H$\beta$ | H (48) $\beta$ | 111885.070(0) | − | − | 204 | 14.8(0.6) | 33.6(1.1) | 7300(240) |
| H$\varepsilon$ | H (64) $\varepsilon$ | 112124.899(0) | − | − | 42 | 17.0(2.4) | 28.1(4.7) | 1270(199) |
| $C^{17}O$ | 1 − 0 | 112359.284(1e-3) | 5.4 | 0.01217 | 317 | 20.0(0.1) | 5.0(0.3) | 1692(74) |
| CN | N= 1-0, J=1/2-1/2, F=1/2-1/2 | 113123.370(6e-3) | 5.4 | 0.15271 | 420 | 19.5(0.1) | 2.1(0.3) | 955(114) |
| CN | N= 1-0, J=1/2-1/2, F=1/2-3/2 | 113144.157(6e-3) | 5.4 | 1.2492 | 2002 | 19.5(0.) | 3.1(0.1) | 6584(134) |
| CN | N= 1-0, J=1/2-1/2, F=3/2-1/2 | 113170.492(4e-3) | 5.4 | 1.2199 | 2461 | 19.5(0.) | 2.9(0.1) | 7677(232) |
| CN | N= 1-0, J=1/2-1/2, F=3/2-3/2 | 113191.279(3e-3) | 5.4 | 1.5836 | 2417 | 19.5(0.) | 2.1(0.1) | 8141(171) |
| CN | N= 1-0, J=3/2-1/2, F=3/2-1/2 | 113488.120(3e-3) | 5.4 | 1.5838 | 2570 | 19.5(0.5) | 3.7(0.5) | 10072(536) |

**Table A2.** (Continued)

| Species | Transitions | Rest Freq. (MHz) | E$_u$ (K) | $\mu^2$S (D$^2$) | T$_{mb}$ (mK) | V$_{LSR}$ (km s$^{-1}$) | $\Delta$V (km s$^{-1}$) | $\int$ T$_{mb}$ dv (mK km s$^{-1}$) |
|---|---|---|---|---|---|---|---|---|
| CN | N= 1-0, J=3/2-1/2, F=5/2-3/2 | 113490.970(2e-3) | 5.4 | 4.205 | 6093 | 19.3(0.5) | 3.3(0.5) | 21386(536) |
| CN | N= 1-0, J=3/2-1/2, F=1/2-1/2 | 113499.644(3e-3) | 5.4 | 1.2491 | 1463 | 19.3(0.5) | 3.2(0.5) | 4946(536) |
| CN | N= 1-0, J=3/2-1/2, F=3/2-3/2 | 113508.907(3e-3) | 5.4 | 1.2196 | 1671 | 19.4(0.5) | 3.3(0.5) | 5861(536) |
| CN | N= 1-0, J=3/2-1/2, F=1/2-3/2 | 113520.432(4e-3) | 5.4 | 0.15263 | 258 | 19.4(0.5) | 2.6(0.5) | 723(536) |
| | | G016.58−00.05 | | | | | | |
| CCS | 8(9) − 7(8) | 106347.726(2e-2) | 25.0 | 74.425 | 94 | 59.0(0.2) | 3.0(0.4) | 301(32) |
| OC$^{34}$S | 9 − 8 | 106787.390(2e-3) | 25.6 | 4.601 | 40 | 59.8(0.4) | 4.1(0.9) | 175(34) |
| CH$_3$OH, vt=0-2 | 3(1)$^+$ − 4(0)$^+$, vt=0 | 107013.831(1e-2) | 28.3 | 12.036 | 258 | 59.5(0.1) | 5.1(0.2) | 1406(39) |
| CH$_3$OH, vt=0-2 | 15(-2) − 15(1) E2, vt=0 | 107159.906(14e-3) | 304.7 | 10.421 | 29 | 59.5(0.5) | 3.8(0.9) | 114(28) |
| $^{13}$C$^{17}$O | 1(2) − 0(3) | 107288.550(5e-2) | 5.1 | 0.016 | 60 | 58.6(0.3) | 2.0(0.5) | 129(31) |
| $^{13}$C$^{17}$O | 1(3) − 0(3) | 107289.650(5e-2) | 5.1 | 0.024 | 53 | 58.3(0.1) | 0.5(0.4) | 31(22) |
| C$_2$H$_5$CN | 12(7, 5) − 11(7, 4) | 107485.160(5e-2) | 88.0 | 117.36 | 24 | 59.8(0.5) | 2.1(0.9) | 53(25) |
| C$_2$H$_5$CN | 12(6, 6) − 11(6, 5) | 107486.949(5e-2) | 73.6 | 133.42 | 28 | 59.8(0.5) | 3.3(1.4) | 100(34) |
| C$_2$H$_5$CN | 12(8, 4) − 11(8, 3) | 107491.574(5e-2) | 104.6 | 98.829 | 28 | 59.7(0.4) | 1.4(0.7) | 41(20) |
| $^{13}$CN | 1(1, 1) − 0(1, 0), F = 0 − 1 | 108631.121(5e-2) | 5.2 | 0.642 | 35 | 59.4(0.5) | 2.9(0.9) | 108(31) |
| $^{13}$CN | 1(1, 1) − 0(1, 0), F = 1 − 1 | 108636.923(5e-2) | 5.2 | 1.932 | 48 | 59.3(0.2) | 0.5(0.4) | 28(14) |
| $^{13}$CN | 1(2, 1) − 0(1, 1), F = 1 − 0 | 108638.212(5e-2) | 5.2 | 0.722 | 39 | 59.5(0.3) | 1.3(0.5) | 55(20) |
| $^{13}$CN | 1(2, 1) − 0(1, 1), F = 2 − 1 | 108643.590(5e-2) | 5.2 | 0.856 | 24 | 59.3(0.7) | 2.7(1.8) | 68(37) |
| $^{13}$CN | 1(2, 1) − 0(1, 1), F = 0 − 1 | 108644.346(5e-2) | 5.2 | 0.642 | 27 | 59.5(0.6) | 0.8(0.6) | 23(20) |
| $^{13}$CN | 1(2, 1) − 0(1, 1), F = 1 − 1 | 108645.064(5e-2) | 5.2 | 0.551 | blended | − | − | − |
| $^{13}$CN | 1(1, 1) − 0(1, 0), F = 2 − 1 | 108651.297(5e-2) | 5.2 | 3.276 | 79 | 59.5(0.2) | 3.2(0.4) | 268(33) |
| $^{13}$CN | 1(2, 1) − 0(1, 1), F = 2 − 2 | 108657.646(5e-2) | 5.2 | 2.420 | 48 | 59.5(0.3) | 3.1(0.6) | 156(31) |
| $^{13}$CN | 1(2, 1) − 0(1, 1), F = 1 − 2 | 108658.948(5e-2) | 5.2 | 0.669 | 70 | 59.5(0.1) | 0.5(0.2) | 41(16) |
| $^{13}$CN | 1(2, 2) − 0(1, 1), F = 3 − 2 | 108780.201(5e-2) | 5.2 | 4.905 | 100 | 59.4(0.2) | 3.0(0.3) | 319(34) |
| $^{13}$CN | 1(2, 2) − 0(1, 1), F = 2 − 1 | 108782.374(5e-2) | 5.2 | 2.586 | 62 | 59.5(0.2) | 1.9(0.4) | 128(27) |
| $^{13}$CN | 1(2, 2) − 0(1, 1), F = 1 − 0 | 108786.982(5e-2) | 5.2 | 1.144 | 13 | 59.5(1.2) | 3.4(1.4) | 49(31) |
| $^{13}$CN | 1(2, 2) − 0(1, 1), F = 1 − 1 | 108793.753(5e-2) | 5.2 | 0.894 | 28 | 59.5(0.3) | 0.8(0.5) | 22(17) |
| $^{13}$CN | 1(2, 2) − 0(1, 1), F = 2 − 2 | 108796.400(5e-2) | 5.2 | 0.918 | 19 | 59.5(0.8) | 2.3(1.2) | 46(29) |
| CH$_3$OH, vt=0-2 | 0(0) − 1(-1) E2, vt=0 | 108893.945(12e-3) | 13.1 | 3.9134 | 700 | 59.5(0.) | 4.4(0.1) | 3238(44) |
| O$^{13}$CS | 9 − 8 | 109110.845(2e-3) | 26.2 | 4.605 | 22 | 61.3(1.0) | 3.7(1.6) | 85(42) |
| HC$_3$N | 12 − 11 | 109173.634(1e-2) | 34.1 | 167.1 | 2038 | 60.0(0.) | 3.3(0.1) | 7201(50) |
| SO | 3(2) − 2(1) | 109252.220(1e-1) | 21.1 | 3.5585 | 415 | 59.5(0.1) | 4.1(0.1) | 1792(48) |
| OCS | 9 − 8 | 109463.063(5e-3) | 26.3 | 4.6034 | 400 | 59.5(0.1) | 4.1(0.1) | 1745(48) |
| C$^{18}$O | 1 − 0 | 109782.173(6e-3) | 5.3 | 0.01221 | 5856 | 59.0(0.5) | 3.3(0.5) | 20302(425) |
| HNCO | 5(0, 5) − 4(0, 4) | 109905.749(7e-3) | 15.8 | 12.482 | 510 | 59.4(0.1) | 3.8(0.1) | 2073(58) |
| $^{13}$CO | 1 − 0 | 110201.35(0) | 5.3 | 0.01220 | 18595 | 59.5(0.5) | 3.8(0.5) | 74595(1480) |
| CH$_3$CN | 6(4, 0) − 5(4, 0) | 110349.471(0) | 132.8 | 102.54 | 32 | 59.5(0.5) | 4.0(0.5) | 136(56) |
| CH$_3$CN | 6(3, 0) − 5(-3, 0) | 110364.354(0) | 82.8 | 138.54 | 176 | 59.5(0.5) | 5.1(0.5) | 955(56) |
| CH$_3$CN | 6(-3, 0) − 5(3, 0) | 110364.354(0) | 82.8 | 138.54 | blended | − | − | − |
| CH$_3$CN | 6(2, 0) − 5(2, 0) | 110374.989(0) | 47.1 | 164.06 | 223 | 59.5(0.5) | 4.4(0.5) | 1051(56) |
| CH$_3$CN | 6(1, 0) − 5(1, 0) | 110381.372(0) | 25.7 | 179.45 | 438 | 59.5(0.5) | 3.8(0.5) | 1786(56) |
| CH$_3$CN | 6(0, 0) − 5(0, 0) | 110383.500(0) | 18.5 | 184.58 | 468 | 59.5(0.5) | 4.3(0.5) | 2124(56) |
| CH$_3$OCHO | 10(1,10) − 9(1, 9) E | 110788.664(1e-2) | 30.3 | 26.16584 | 28 | 59.7(0.6) | 2.3(2.1) | 68(94) |
| CH$_3$OCHO | 10(1,10) − 9(1, 9) A | 110790.526(1e-2) | 30.3 | 26.17539 | 32 | 59.7(1.9) | 7.3(2.2) | 251(115) |
| CH$_3$OCHO | 9(5, 4) − 8(5, 3) E | 110873.955(1e-2) | 43.2 | 16.55557 | 40 | 59.7(0.6) | 3.9(1.5) | 168(53) |
| CH$_3$OCHO | 9(5, 5) − 8(5, 4) E | 110882.331(1e-2) | 43.2 | 16.55225 | 43 | 59.5(0.5) | 3.3(1.2) | 151(49) |
| CH$_3$OCHO | 9(3, 7) − 8(3, 6) A | 110887.092(1e-2) | 32.6 | 21.25577 | 40 | 59.5(0.5) | 2.1(0.8) | 92(28) |
| CH$_3$OCHO | 10(0, 10) − 9(0, 9) A | 111171.634(1e-2) | 30.2 | 26.19136 | 48 | 59.5(1.4) | 7.2(5.2) | 729(258) |
| CH$_3$OH, vt=0-2 | 7(2)$^+$ − 8( 1)$^+$, vt=0 | 111289.453(13e-3) | 102.7 | 9.3425 | 109 | 59.5(0.3) | 6.8(0.8) | 791(76) |
| CH$_3$OCHO | 9(4, 5) − 8(4, 4) A | 111453.300(1e-2) | 37.2 | 19.21778 | 27 | 59.7(1.6) | 7.9(5.2) | 397(168) |
| CH$_3$OCH$_3$ | 7(0, 7) − 6(1, 6) AA | 111782.562(8e-3) | 25.2 | 68.047 | 83 | 59.5(0.7) | 9.8(2.8) | 1042(161) |
| CH$_3$CHO | 6(1, 6) − 5(1, 5) A, vt=0 | 112248.716(3e-3) | 21.1 | 73.76807 | 129 | 59.5(0.2) | 4.0(0.4) | 550(57) |
| CH$_3$CHO | 6(1, 6) − 5(1, 5) E, vt=0 | 112254.508(3e-3) | 21.2 | 73.79585 | 78 | 59.5(0.4) | 4.6(1.5) | 381(92) |
| C$^{17}$O | 1 − 0 | 112359.284(1e-3) | 5.4 | 0.01217 | 1305 | 59.5(0.1) | 5.0(0.1) | 6889(78) |
| CN | N= 1-0, J=1/2-1/2, F=1/2-1/2 | 113123.370(6e-3) | 5.4 | 0.15271 | 448 | 59.5(0.2) | 4.0(0.4) | 1882(168) |
| CN | N= 1-0, J=1/2-1/2, F=1/2-3/2 | 113144.157(6e-3) | 5.4 | 1.2492 | 1021 | 59.5(0.1) | 4.0(0.2) | 4368(160) |
| CN | N= 1-0, J=1/2-1/2, F=3/2-1/2 | 113170.492(4e-3) | 5.4 | 1.2199 | 1226 | 59.5(0.1) | 4.0(0.2) | 5212(163) |
| CN | N= 1-0, J=1/2-1/2, F=3/2-3/2 | 113191.279(3e-3) | 5.4 | 1.5836 | 1096 | 59.5(0.1) | 4.1(0.2) | 4792(174) |
| CN | N= 1-0, J=3/2-1/2, F=3/2-1/2 | 113488.120(3e-3) | 5.4 | 1.5838 | 1154 | 59.5(0.5) | 4.4(0.5) | 5400(199) |
| CN | N= 1-0, J=3/2-1/2, F=5/2-3/2 | 113490.970(2e-3) | 5.4 | 4.205 | 2441 | 59.5(0.5) | 2.7(0.5) | 6962(199) |
| CN | N= 1-0, J=3/2-1/2, F=1/2-1/2 | 113499.644(3e-3) | 5.4 | 1.2491 | 550 | 59.5(0.5) | 5.7(0.5) | 3311(199) |
| CN | N= 1-0, J=3/2-1/2, F=3/2-3/2 | 113508.907(3e-3) | 5.4 | 1.2196 | 1057 | 59.5(0.5) | 4.4(0.5) | 4981(199) |
| CN | N= 1-0, J=3/2-1/2, F=1/2-3/2 | 113520.432(4e-3) | 5.4 | 0.15263 | 267 | 59.5(0.5) | 4.9(0.5) | 1387(199) |
| | | G023.00−00.41 | | | | | | |
| NH$_2$CHO | 5(2, 4) − 4(2, 3) | 105972.665(37e-3) | 27.2 | 54.915 | 35 | 77.2(0.6) | 9.8(1.4) | 360(60) |
| NH$_2$CHO | 5(3, 3) − 4(3, 2) | 106134.468(55e-3) | 42.1 | 41.845 | 27 | 77.0(1.5) | 10.7(3.7) | 560(91) |
| NH$_2$CHO | 5(3, 2) − 4(3, 1) | 106141.442(55e-3) | 42.1 | 41.84 | 30 | 77.0(1.0) | 9.1(2.5) | 288(69) |
| CCS | 8(9) − 7(8) | 106347.726(2e-2) | 25.0 | 74.425 | 61 | 77.0(0.3) | 5.0(1.0) | 323(44) |
| HC$_5$N | 40 − 39 | 106498.910(7e-3) | 104.8 | 2249.7 | 34 | 77.5(0.8) | 4.4(2.6) | 157(84) |
| NH$_2$CHO | 5(2, 3) − 4(2, 2) | 106541.773(37e-3) | 27.2 | 54.915 | 43 | 77.0(0.5) | 7.3(1.3) | 334(48) |
| CH$_3$OH, vt=0-2 | 3(1)$^+$ − 4(0)$^+$, vt=0 | 107013.831(1e-2) | 28.3 | 12.036 | 886 | 76.5(0.) | 4.2(0.1) | 3942(49) |
| C$_2$H$_5$CN | 12(2, 11) − 11(2, 10) | 107043.527(5e-2) | 37.9 | 172.86 | 26 | 78.5(0.9) | 9.9(1.8) | 277(49) |
| CH$_3$OH, vt=0-2 | 15(-2) − 15(1) E2, vt=0 | 107159.906(14e-3) | 304.7 | 10.421 | 28 | 76.5(0.5) | 0.8(0.5) | 38(9) |
| C$_2$H$_5$CN | 12(7, 5) − 11(7, 4) | 107485.160(5e-2) | 88.0 | 117.36 | 32 | 78.5(0.8) | 6.8(1.7) | 232(47) |
| C$_2$H$_5$CN | 12(5, 7) − 11(5, 6) | 107502.432(5e-2) | 61.3 | 146.99 | 27 | 78.5(0.8) | 7.1(1.3) | 207(44) |
| C$_2$H$_5$CN | 12(4, 9) − 11(4, 8) | 107544.042(5e-2) | 51.3 | 158.12 | 24 | 78.5(0.9) | 2.7(2.1) | 71(60) |
| C$_2$H$_5$CN | 12(4, 8) − 11(4, 7) | 107547.460(5e-2) | 51.3 | 158.11 | 21 | 78.7(2.0) | 9.1(3.1) | 207(75) |
| C$_2$H$_5$CN | 12(3, 10) − 11(3, 9) | 107594.056(5e-2) | 43.6 | 166.77 | 15 | 78.7(1.9) | 6.2(2.4) | 97(53) |
| C$_2$H$_5$CN | 12(3, 9) − 11(3, 8) | 107734.723(5e-2) | 43.6 | 166.76 | 14 | 78.5(0.5) | 0.5(0.3) | 17(8) |
| $^{13}$CN | 1(1, 0) − 0(1, 1), F = 1 − 2 | 108426.889(5e-2) | 5.2 | 1.267 | 35 | 77.0(0.4) | 2.6(0.9) | 98(29) |
| $^{13}$CN | 1(1, 1) − 0(1, 0), F = 1 − 1 | 108636.923(5e-2) | 5.2 | 1.932 | 62 | 76.9(0.3) | 2.7(0.6) | 177(38) |
| $^{13}$CN | 1(2, 1) − 0(1, 1), F = 1 − 0 | 108638.212(5e-2) | 5.2 | 0.722 | 39 | 77.0(0.3) | 0.8(0.6) | 32(22) |
| $^{13}$CN | 1(2, 1) − 0(1, 1), F = 2 − 1 | 108643.590(5e-2) | 5.2 | 0.856 | 38 | 77.1(0.3) | 0.9(0.6) | 36(24) |
| $^{13}$CN | 1(2, 1) − 0(1, 1), F = 0 − 1 | 108644.346(5e-2) | 5.2 | 0.642 | 62 | 76.8(0.2) | 1.6(0.7) | 106(34) |
| $^{13}$CN | 1(2, 1) − 0(1, 1), F = 1 − 1 | 108645.064(5e-2) | 5.2 | 0.551 | blended | − | − | − |
| $^{13}$CN | 1(1, 1) − 0(1, 0), F = 2 − 1 | 108651.297(5e-2) | 5.2 | 3.276 | 87 | 77.0(0.2) | 2.7(0.4) | 249(37) |
| $^{13}$CN | 1(2, 1) − 0(1, 1), F = 2 − 2 | 108657.646(5e-2) | 5.2 | 2.420 | 68 | 77.0(0.3) | 3.2(0.7) | 231(43) |
| $^{13}$CN | 1(2, 1) − 0(1, 1), F = 1 − 2 | 108658.948(5e-2) | 5.2 | 0.669 | 41 | 77.1(0.3) | 0.7(0.2) | 32(27) |
| $^{13}$CN | 1(2, 2) − 0(1, 1), F = 3 − 2 | 108780.201(5e-2) | 5.2 | 4.905 | 112 | 77.0(0.2) | 3.9(0.5) | 466(49) |
| $^{13}$CN | 1(2, 2) − 0(1, 1), F = 2 − 1 | 108782.374(5e-2) | 5.2 | 2.586 | 70 | 77.0(0.3) | 3.1(0.8) | 229(47) |
| $^{13}$CN | 1(2, 2) − 0(1, 1), F = 1 − 1 | 108793.753(5e-2) | 5.2 | 0.894 | 38 | 77.1(0.3) | 1.7(0.6) | 68(26) |
| $^{13}$CN | 1(2, 2) − 0(1, 1), F = 2 − 2 | 108796.400(5e-2) | 5.2 | 0.918 | 18 | 66.9(1.4) | 4.8(3.1) | 90(49) |
| CH$_3$OH, vt=0-2 | 0(0) − 1(-1) E2, vt=0 | 108893.945(12e-3) | 13.1 | 3.9134 | 495 | 76.5(0.1) | 10.7(0.2) | 5638(78) |
| C$_2$H$_5$CN | 12(2, 10) − 11(2, 9) | 108940.554(5e-2) | 38.2 | 172.93 | 19 | 78.5(1.3) | 6.9(2.2) | 138(47) |

**Table A2.** (Continued)

| Species | Transitions | Rest Freq. (MHz) | $E_u$ (K) | $\mu^2S$ ($D^2$) | $T_{mb}$ (mK) | $V_{LSR}$ (km $s^{-1}$) | ΔV (km $s^{-1}$) | $\int T_{mb}$ dv (mK km $s^{-1}$) |
|---|---|---|---|---|---|---|---|---|
| $CH_3OH$, vt=0-2 | 14(5) − 15(4) E1, vt=0 | 109138.783(15e-3) | 379.7 | 13.593 | 35 | 76.5(0.7) | 7.8(1.3) | 288(49) |
| $CH_3OH$, vt=0-2 | 16(-2) − 16(1) E2, vt=0 | 109153.184(14e-3) | 342.0 | 14.726 | 29 | 76.5(0.8) | 7.3(1.2) | 227(45) |
| $HC_3N$ | 12 − 11 | 109173.634(1e-2) | 34.1 | 167.1 | 1793 | 77.0(0.) | 4.4(0.1) | 8349(104) |
| SO | 3(2) − 2(1) | 109252.220(1e-1) | 21.1 | 3.5585 | 148 | 76.8(0.2) | 11.7(0.6) | 1850(72) |
| $HC_3N$, $v_7$=1 | 12(-1) − 11(1) | 109442.013(2e-2) | 355.0 | 165.12 | 30 | 80.0(0.4) | 14.8(2.5) | 635(78) |
| OCS | 9 − 8 | 109463.063(5e-3) | 26.3 | 4.6034 | 225 | 78.0(0.1) | 11.8(0.3) | 2823(63) |
| HNCO | 5(1, 5) − 4(1, 4) | 109495.996(6e-3) | 59.0 | 11.847 | 44 | 77.5(0.5) | 9.1(1.7) | 423(59) |
| $^{13}CO$ | 1 − 0 | 110201.35(0) | 5.3 | 0.01220 | 15397 | 76.3(0.5) | 4.4(0.5) | 38829(1250) |
| $HC_3N$, $v_7$=1 | 12(1) − 11(-1) | 109598.818(2e-2) | 355.0 | 165.12 | 39 | 80.0(0.8) | 10.9(2.0) | 449(67) |
| $C_2H_5CN$ | 12(1, 11) − 11(1, 10) | 109650.263(5e-2) | 35.4 | 176.49 | 22 | 78.7(1.2) | 6.3(2.2) | 150(52) |
| $C^{18}O$ | 1 − 0 | 109782.173(6e-3) | 5.3 | 0.01221 | 3525 | 76.5(0.5) | 4.8(0.5) | 18164(359) |
| HNCO | 5(0, 5) − 4(0, 4) | 109905.749(7e-3) | 15.8 | 12.482 | 619 | 77.5(0.1) | 10.8(0.3) | 7123(132) |
| HNCO | 5(1, 4) − 4(1, 3) | 110298.089(5e-3) | 59.2 | 11.847 | 39 | 77.5(0.7) | 8.1(1.9) | 336(61) |
| $CH_3CN$ | 6(5, 0) − 5(5, 0) | 110330.345(0) | 197.1 | 56.399 | 36 | 77.5(1.1) | 11.4(1.1) | 434(113) |
| $CH_3CN$ | 6(4, 0) − 5(4, 0) | 110349.471(0) | 132.8 | 102.54 | 84 | 77.5(1.1) | 8.0(1.1) | 716(113) |
| $CH_3CN$ | 6(3, 0) − 5(-3, 0) | 110364.354(0) | 82.8 | 138.54 | 215 | 77.5(1.1) | 8.7(1.1) | 1983(113) |
| $CH_3CN$ | 6(-3, 0) − 5(3, 0) | 110364.354(0) | 82.8 | 138.54 | blended | − | − | − |
| $CH_3CN$ | 6(2, 0) − 5(2, 0) | 110374.989(0) | 47.1 | 164.06 | 203 | 77.5(1.1) | 10.3(1.1) | 2237(113) |
| $CH_3CN$ | 6(1, 0) − 5(1, 0) | 110381.372(0) | 25.7 | 179.45 | 433 | 77.5(1.1) | 6.9(1.1) | 3158(113) |
| $CH_3CN$ | 6(0, 0) − 5(0, 0) | 110383.500(0) | 18.5 | 184.58 | 423 | 77.5(1.1) | 5.8(1.1) | 2612(113) |
| $CH_3OCHO$ | 10(1,10) − 9(1, 9) E | 110788.664(1e-2) | 30.3 | 26.16584 | 18 | 78.0(0.5) | 1.1(0.6) | 37(37) |
| $CH_3OCHO$ | 10(1,10) − 9(1, 9) A | 110790.526(1e-2) | 30.3 | 26.17539 | 28 | 78.0(1.2) | 2.8(3.5) | 85(67) |
| $C_2H_3CN$ | 12(1, 12) − 11(1, 11) | 110839.968(1e-3) | 36.8 | 520.3 | 39 | 77.9(0.) | 8.6(3.4) | 359(104) |
| $CH_3OCHO$ | 9(3, 7) − 8(3, 6) A | 110887.092(1e-2) | 32.6 | 21.25577 | 31 | 78.0(1.3) | 8.8(2.8) | 290(73) |
| $CH_3OCHO$ | 10(0, 10) − 9(0, 9) E | 111169.903(1e-2) | 30.2 | 26.18776 | 35 | 78.0(1.4) | 7.9(2.1) | 296(93) |
| $CH_3OCHO$ | 10(0, 10) − 9(0, 9) A | 111171.634(1e-2) | 30.2 | 26.19136 | 27 | 78.0(0.1) | 9.4(3.2) | 272(107) |
| $CH_3OH$, vt=0-2 | $7(2)^+$ − $8( 1)^+$, vt=0 | 111289.453(13e-3) | 102.7 | 9.3425 | 113 | 76.5(0.2) | 7.9(0.5) | 947(52) |
| $CH_3OH$, vt=0-2 | 17(-2) − 17(1) E2, vt=0 | 111626.514(15e-3) | 381.5 | 20.231 | 40 | 76.5(0.8) | 8.6(1.8) | 362(63) |
| $CH_3OCHO$ | 9(1, 8) − 8(1, 7) E | 111674.131(1e-2) | 28.1 | 23.18984 | 33 | 78.0(0.7) | 4.7(1.4) | 163(44) |
| $CH_3OCHO$ | 9(1, 8) − 8(1, 7) A | 111682.189(1e-2) | 28.1 | 23.19587 | 33 | 78.0(0.7) | 5.4(1.3) | 186(45) |
| $CH_3OCH_3$ | 19(3, 16) − 19(2, 17) AA | 111744.238(29e-3) | 187.5 | 259.8 | 21 | 77.0(2.6) | 16.0(5.7) | 359(110) |
| $CH_3OCH_3$ | 7(0, 7) − 6(1, 6) AA | 111782.562(8e-3) | 25.2 | 68.047 | 51 | 77.0(0.7) | 8.5(1.6) | 458(79) |
| $CH_3OCH_3$ | 18(3, 15) − 18(2, 16) EE | 111813.668(21e-3) | 115.4 | 386.29 | 26 | 77.0(1.1) | 4.5(1.8) | 124(54) |
| $CH_3CHO$ | 6(1, 6) − 5(1, 5) A, vt=0 | 112248.716(3e-3) | 21.1 | 73.76807 | 43 | 77.0(1.0) | 4.8(2.3) | 219(88) |
| $CH_3CHO$ | 6(1, 6) − 5(1, 5) E, vt=0 | 112254.508(3e-3) | 21.2 | 73.79585 | 51 | 77.0(1.3) | 12.6(3.5) | 683(149) |
| $C^{17}O$ | 1 − 0 | 112359.284(1e-3) | 5.4 | 0.01217 | 861 | 76.0(0.1) | 7.8(0.1) | 7148(32) |
| $C_2H_5CN$ | 13(1, 13) − 12(1, 12) | 112646.350(9e-2) | 39.0 | 191.45 | 33 | 79.0(1.3) | 8.8(2.5) | 310(86) |
| $CH_3OCH_3$ | 17(3, 14) − 17(2, 15) AA | 113061.072(22e-3) | 153.1 | 221.33 | 25 | 77.0(1.7) | 8.9(3.4) | 234(82) |
| CN | N= 1-0, J=1/2-1/2, F=1/2-1/2 | 113123.370(6e-3) | 5.4 | 0.15271 | 485 | 77.3(0.5) | 5.2(0.5) | 2706(113) |
| CN | N= 1-0, J=1/2-1/2, F=1/2-3/2 | 113144.157(6e-3) | 5.4 | 1.2492 | 643 | 77.3(0.5) | 9.5(0.5) | 6539(113) |
| CN | N= 1-0, J=1/2-1/2, F=3/2-1/2 | 113170.492(4e-3) | 5.4 | 1.2199 | 741 | 77.3(0.5) | 10.4(0.5) | 8186(113) |
| CN | N= 1-0, J=1/2-1/2, F=3/2-3/2 | 113191.279(3e-3) | 5.4 | 1.5836 | 552 | 77.3(0.5) | 10.4(0.5) | 6133(113) |
| CN | N= 1-0, J=3/2-1/2, F=3/2-1/2 | 113488.120(3e-3) | 5.4 | 1.5838 | 583 | 77.3(0.5) | 4.5(0.5) | 2778(108) |
| CN | N= 1-0, J=3/2-1/2, F=5/2-3/2 | 113490.970(2e-3) | 5.4 | 4.205 | 822 | 77.3(0.5) | 6.3(0.5) | 5513(108) |
| CN | N= 1-0, J=3/2-1/2, F=1/2-1/2 | 113499.644(3e-3) | 5.4 | 1.2491 | 176 | 77.3(0.5) | 7.8(0.5) | 1468(108) |
| CN | N= 1-0, J=3/2-1/2, F=3/2-3/2 | 113508.907(3e-3) | 5.4 | 1.2196 | 421 | 77.3(0.5) | 10.4(0.5) | 4686(108) |
| CN | N= 1-0, J=3/2-1/2, F=1/2-3/2 | 113520.432(4e-3) | 5.4 | 0.15263 | 253 | 77.3(0.5) | 4.5(0.5) | 1214(108) |
| | | | | G023.44−00.18 | | | | |
| $NH_2CHO$ | 5(2, 4) − 4(2, 3) | 105972.665(37e-3) | 27.2 | 54.915 | 26 | 101.5(0.7) | 7.4(2.4) | 203(52) |
| CCS | 8(9) − 7(8) | 106347.726(2e-2) | 25.0 | 74.425 | 89 | 101.3(0.2) | 4.1(0.5) | 383(33) |
| $NH_2CHO$ | 5(2, 3) − 4(2, 2) | 106541.773(37e-3) | 27.2 | 54.915 | 26 | 101.5(0.6) | 4.9(1.9) | 137(37) |
| Hα | H (39) α | 106737.357(0) | − | − | 20 | 95.9(1.4) | 14.5(2.5) | 312(58) |
| $OC^{34}S$ | 9 − 8 | 106787.390(2e-3) | 25.6 | 4.601 | 23 | 102.4(0.7) | 5.0(0.5) | 123(26) |
| $CH_3OH$, vt=0-2 | $3(1)^+$ − $4(0)^+$, vt=0 | 107013.831(1e-2) | 28.3 | 12.036 | 154 | 102.5(0.2) | 6.7(0.4) | 1088(58) |
| $^{13}C^{17}O$ | 1(2) − 0(3) | 107288.550(5e-2) | 5.1 | 0.016 | 43 | 100.8(0.4) | 5.0(1.1) | 232(41) |
| $CH_3OCHO$ | 9( 2, 8) − 8( 2, 7) E | 107537.258(1e-2) | 28.8 | 22.60702 | 23 | 101.5(0.6) | 5.2(3.5) | 126(49) |
| $CH_3OCHO$ | 9( 2, 8) − 8( 2, 7) A | 107543.711(1e-2) | 28.8 | 22.61344 | 27 | 101.5(0.8) | 5.4(1.2) | 153(33) |
| t-HCOOH | 5(1, 5) − 4(1, 4) | 108126.720(3e-3) | 18.8 | 9.6966 | 45 | 101.0(0.3) | 3.3(0.7) | 156(27) |
| $^{13}CN$ | 1(1, 1) − 0(1, 0), F = 1 − 1 | 108636.923(5e-2) | 5.2 | 1.932 | 20 | 100.6(0.5) | 4.1(0.5) | 87(13) |
| $^{13}CN$ | 1(2, 1) − 0(1, 1), F = 1 − 0 | 108638.212(5e-2) | 5.2 | 0.722 | 21 | 100.6(0.5) | 4.0(0.5) | 92(13) |
| $^{13}CN$ | 1(2, 1) − 0(1, 1), F = 2 − 1 | 108643.590(5e-2) | 5.2 | 0.856 | 24 | 100.4(0.5) | 3.8(0.5) | 98(13) |
| $^{13}CN$ | 1(2, 1) − 0(1, 1), F = 0 − 1 | 108644.346(5e-2) | 5.2 | 0.642 | blended | − | − | − |
| $^{13}CN$ | 1(2, 1) − 0(1, 1), F = 1 − 1 | 108645.064(5e-2) | 5.2 | 0.551 | blended | − | − | − |
| $^{13}CN$ | 1(1, 1) − 0(1, 0), F = 2 − 1 | 108651.297(5e-2) | 5.2 | 3.276 | 73 | 100.5(0.5) | 4.7(0.5) | 359(13) |
| $^{13}CN$ | 1(2, 1) − 0(1, 1), F = 2 − 2 | 108657.646(5e-2) | 5.2 | 2.420 | 52 | 100.5(0.5) | 1.9(0.5) | 106(13) |
| $^{13}CN$ | 1(2, 1) − 0(1, 1), F = 1 − 2 | 108658.948(5e-2) | 5.2 | 0.669 | 21 | 100.5(0.5) | 3.2(0.5) | 74(13) |
| $^{13}CN$ | 1(2, 2) − 0(1, 1), F = 3 − 2 | 108780.201(5e-2) | 5.2 | 4.905 | 103 | 100.5(0.2) | 3.8(0.6) | 420(53) |
| $^{13}CN$ | 1(2, 2) − 0(1, 1), F = 2 − 1 | 108782.374(5e-2) | 5.2 | 2.586 | 63 | 100.5(0.4) | 3.5(0.8) | 235(49) |
| $CH_3OH$, vt=0-2 | 0(0) − 1(-1) E2, vt=0 | 108893.945(12e-3) | 13.1 | 3.9134 | 799 | 102.5(0.) | 7.2( 0.1) | 6138(66) |
| $HC_3N$ | 12 − 11 | 109173.634(1e-2) | 34.1 | 167.1 | 2284 | 101.5(0.) | 4.4(0.1) | 10794(86) |
| SO | 3(2) − 2(1) | 109252.220(1e-1) | 21.1 | 3.55885 | 298 | 101.5(0.1) | 5.7(0.3) | 1811(61) |
| OCS | 9 − 8 | 109463.063(5e-3) | 26.3 | 4.6034 | 389 | 101.0(0.1) | 5.6(0.2) | 2315(65) |
| $C^{18}O$ | 1 − 0 | 109782.173(6e-3) | 5.3 | 0.01221 | 5815 | 101.5(0.5) | 4.1(0.5) | 25134(486) |
| HNCO | 5(0, 5) − 4(0, 4) | 109905.749(7e-3) | 15.8 | 12.482 | 906 | 101.5(0.) | 5.5(0.1) | 5351(103) |
| $^{13}CO$ | 1 − 0 | 110201.35(0) | 5.3 | 0.01220 | 15913 | 101.5(0.5) | 4.8(0.1) | 81668(1930) |
| $CH_3CN$ | 6(5, 0) − 5(5, 0) | 110330.345(0) | 197.1 | 56.399 | 35 | 101.3(0.5) | 9.7(0.5) | 367(69) |
| $CH_3CN$ | 6(4, 0) − 5(4, 0) | 110349.471(0) | 132.8 | 102.54 | 45 | 101.3(0.5) | 6.8(0.5) | 328(69) |
| $CH_3CN$ | 6(3, 0) − 5(-3, 0) | 110364.354(0) | 82.8 | 138.54 | 198 | 101.3(0.5) | 7.5(0.5) | 1568(69) |
| $CH_3CN$ | 6(-3, 0) − 5(3, 0) | 110364.354(0) | 82.8 | 138.54 | blended | − | − | − |
| $CH_3CN$ | 6(2, 0) − 5(2, 0) | 110374.989(0) | 47.1 | 164.06 | 258 | 101.5(0.5) | 7.0(0.5) | 1917(69) |
| $CH_3CN$ | 6(1, 0) − 5(1, 0) | 110381.372(0) | 25.7 | 179.45 | 599 | 101.5(0.5) | 4.2(0.5) | 2685(69) |
| $CH_3CN$ | 6(0, 0) − 5(0, 0) | 110383.500(0) | 18.5 | 184.58 | 678 | 101.5(0.5) | 6.1(0.5) | 4387(69) |
| $CH_3OCHO$ | 9(6, 3) − 8(6, 2) A | 110663.429(1e-2) | 50.4 | 13.31127 | 23 | 101.5(1.0) | 4.6(1.6) | 113(41) |
| $CH_3OCHO$ | 9(6, 4) − 8(6, 3) A | 110663.273(1e-2) | 50.4 | 13.3113 | blended | − | − | − |
| $CH_3OCHO$ | 10(1,10) − 9(1, 9) E | 110788.664(1e-2) | 30.3 | 26.16584 | 33 | 101.5(1.1) | 7.9(2.3) | 281(76) |
| $CH_3OCHO$ | 10(1,10) − 9(1, 9) A | 110790.526(1e-2) | 30.3 | 26.17539 | 37 | 101.5(0.3) | 1.4(0.6) | 53(34) |
| $CH_3OCHO$ | 9(5, 4) − 8(5, 3) E | 110873.955(1e-2) | 43.2 | 16.55557 | 54 | 101.5(0.5) | 7.9(0.5) | 452(15) |
| $CH_3OCHO$ | 9(3, 7) − 8(3, 6) E | 110879.766(1e-2) | 32.6 | 21.145 | 33 | 101.3(0.5) | 7.7(0.5) | 268(15) |
| $CH_3OCHO$ | 9(5, 5) − 8(5, 4) A | 110880.447(1e-2) | 43.2 | 16.56015 | blended | − | − | − |
| $CH_3OCHO$ | 9(5, 5) − 8(5, 4) E | 110882.331(1e-2) | 43.2 | 16.55225 | 31 | 101.3(0.5) | 10.0(0.5) | 331(15) |
| $CH_3OCHO$ | 9(3, 7) − 8(3, 6) A | 110887.092(1e-2) | 32.6 | 21.25577 | 45 | 101.5(0.5) | 1.6(0.5) | 77(15) |
| $CH_3OCHO$ | 10(0, 10) − 9(0, 9) E | 111169.903(1e-2) | 30.2 | 26.18776 | 64 | 101.5(0.5) | 3.1(0.5) | 208(13) |
| $CH_3OCHO$ | 10(0, 10) − 9(0, 9) A | 111171.634(1e-2) | 30.2 | 26.19136 | 55 | 101.5(0.5) | 3.6(0.5) | 210(13) |
| $CH_3OH$, vt=0-2 | $7(2)^+$ − $8( 1)^+$, vt=0 | 111289.453(13e-3) | 102.7 | 9.3425 | 38 | 102.5(0.5) | 3.2(1.5) | 131(53) |
| $CH_3OCHO$ | 9(1, 8) − 8(1, 7) E | 111674.131(1e-2) | 28.1 | 23.18984 | 26 | 101.5(1.1) | 6.9(2.5) | 188(69) |
| $CH_3OCHO$ | 9(1, 8) − 8(1, 7) A | 111682.189(1e-2) | 28.1 | 23.19587 | 34 | 101.5(1.1) | 9.1(2.7) | 327(87) |
| $CH_3OCH_3$ | 7(0, 7) − 6(1, 6) AA | 111782.600(8e-3) | 25.2 | 68.047 | 92 | 101.2(0.4) | 9.2(1.1) | 908(82) |
| $CH_3CHO$ | 6(1, 6) − 5(1, 5) A, vt=0 | 112248.716(3e-3) | 21.1 | 73.76807 | 191 | 101.5(0.2) | 6.0(0.5) | 1221(77) |
| $CH_3CHO$ | 6(1, 6) − 5(1, 5) E, vt=0 | 112254.508(3e-3) | 21.2 | 73.79585 | 170 | 101.5(0.2) | 5.5(0.6) | 998(74) |

**Table A2.** (Continued)

| Species | Transitions | Rest Freq. (MHz) | $E_u$ (K) | $\mu^2S$ ($D^2$) | $T_{mb}$ (mK) | $V_{LSR}$ (km $s^{-1}$) | $\Delta V$ (km $s^{-1}$) | $\int T_{mb}$ dv (mK km $s^{-1}$) |
|---|---|---|---|---|---|---|---|---|
| $C^{17}O$ | 1 − 0 | 112359.284(1e-3) | 5.4 | 0.01217 | 1473 | 101.0(0.1) | 6.9(0.1) | 10800(83) |
| CN | N= 1-0, J=1/2-1/2, F=1/2-1/2 | 113123.370(6e-3) | 5.4 | 0.15271 | 473 | 103.1(0.1) | 5.0(0.5) | 2523(168) |
| CN | N= 1-0, J=1/2-1/2, F=1/2-3/2 | 113144.157(6e-3) | 5.4 | 1.2492 | 856 | 103.0(0.) | 5.4(0.3) | 4916(173) |
| CN | N= 1-0, J=1/2-1/2, F=3/2-1/2 | 113170.492(4e-3) | 5.4 | 1.2199 | 1066 | 103.0(0.1) | 5.3(0.2) | 5992(173) |
| CN | N= 1-0, J=1/2-1/2, F=3/2-3/2 | 113191.279(3e-3) | 5.4 | 1.5836 | 961 | 103.0(0.1) | 5.1(0.2) | 5228(164) |
| CN | N= 1-0, J=3/2-1/2, F=3/2-1/2 | 113488.120(3e-3) | 5.4 | 1.5838 | 866 | 103.0(0.2) | 7.1(0.6) | 6549(385) |
| CN | N= 1-0, J=3/2-1/2, F=5/2-3/2 | 113490.970(2e-3) | 5.4 | 4.205 | 1107 | 103.0(0.1) | 2.8(0.2) | 3251(214) |
| CN | N= 1-0, J=3/2-1/2, F=1/2-1/2 | 113499.644(3e-3) | 5.4 | 1.2491 | 107 | 103.3(0.5) | 10.7(0.5) | 2354(62) |
| CN | N= 1-0, J=3/2-1/2, F=3/2-3/2 | 113508.907(3e-3) | 5.4 | 1.2196 | 217 | 103.3(0.5) | 11.8(0.5) | 2716(62) |
| CN | N= 1-0, J=3/2-1/2, F=1/2-3/2 | 113520.432(4e-3) | 5.4 | 0.15263 | 260 | 103.3(0.5) | 6.5(0.5) | 1805(62) |
| | | G027.36−00.16 | | | | | | |
| $NH_2CHO$ | 5(2, 4) − 4(2, 3) | 105972.665(37e-3) | 27.2 | 54.915 | 46 | 92.5(0.4) | 7.8(0.9) | 386(39) |
| $NH_2CHO$ | 5(3, 3) − 4(3, 2) | 106134.468(55e-3) | 42.1 | 41.845 | 28 | 92.5(0.7) | 8.1(1.4) | 240(38) |
| $NH_2CHO$ | 5(3, 2) − 4(3, 1) | 106141.442(55e-3) | 42.1 | 41.84 | 25 | 92.5(0.5) | 4.4(1.2) | 120(28) |
| CCS | 8(9) − 7(8) | 106347.726(2e-2) | 25.0 | 74.425 | 81 | 92.0(0.2) | 5.0(0.4) | 432(31) |
| $C_2H_5CN$ | 15(3, 12) − 15(2, 13) | 106375.033(5e-2) | 61.7 | 13.244 | 44 | 93.0(0.2) | 1.7(0.5) | 80(18) |
| $HC_5N$ | 40 − 39 | 106498.910(7e-3) | 104.8 | 2249.7 | 28 | 92.3(0.7) | 5.9(2.5) | 176(46) |
| $NH_2CHO$ | 5(2, 3) − 4(2, 2) | 106541.773(37e-3) | 27.2 | 54.915 | 44 | 92.5(0.4) | 7.4(0.9) | 350(35) |
| $C_2H_5OH$ | 13(1, 12) − 13(0, 13) | 106649.479(5e-2) | 79.4 | 476.24 | 38 | 93.5(0.4) | 6.3(0.9) | 256(34) |
| $C_2H_5OH$ | 6(1, 5) − 5(1, 4) | 106676.542(5e-2) | 76.1 | 9.325 | 16 | 93.5(1.0) | 6.3(1.4) | 106(30) |
| $C_2H_5OH$ | 9(2, 8) − 9(1, 9) | 106723.558(5e-2) | 42.7 | 7.9044 | 25 | 93.5(0.5) | 6.6(1.4) | 178(33) |
| H$\alpha$ | H (39) $\alpha$ | 106737.357(0) | − | − | 21 | 105.5(1.5) | 17.3(3.7) | 379(65) |
| $CH_3COCH_3$ | 18(6, 12) − 18(5, 13) AE | 106739.794(2e-2) | 121.8 | 54.78025 | 24 | 92.7(0.6) | 6.8(1.9) | 177(42) |
| $C_2H_5OH$ | 6(1, 5) − 5(1, 4) | 106767.234(5e-2) | 80.7 | 9.6466 | 17 | 93.5(1.2) | 7.8(1.9) | 138(37) |
| $CH_3OCH_3$ | 9(1, 8) − 8(2, 7) AA | 106775.602(14e-3) | 43.4 | 58.573 | 68 | 93.5(0.4) | 14.5(0.8) | 1049(54) |
| $OC^{34}S$ | 9 − 8 | 106787.390(2e-3) | 25.6 | 4.601 | 85 | 93.6(0.3) | 6.4(0.7) | 577(53) |
| $C_2H_5CN$ | 4(2, 2) − 3(1, 3) | 106905.507(2e-1) | 8.8 | 2.6677 | 18 | 93.0(0.8) | 6.3(1.5) | 124(29) |
| $CH_3OH$, vt=0-2 | $3(1)^+ - 4(0)^+$, vt=0 | 107013.831(1e-2) | 28.3 | 12.036 | 459 | 93.0(0.) | 7.5(0.1) | 3669(49) |
| $C_2H_5CN$ | 12(2, 11) − 11(2, 10) | 107043.527(5e-2) | 37.9 | 172.86 | 59 | 93.0(0.4) | 9.1(1.2) | 572(57) |
| $CH_3OH$, vt=0-2 | 15(-2) − 15(1) E2, vt=0 | 107159.906(14e-3) | 304.7 | 10.421 | 67 | 93.0(0.3) | 7.0(0.8) | 498(50) |
| $^{13}CH_3CN$ | 6(4) − 5(4) | 107164.310(0) | 132.5 | 102.548 | 35 | 93.6(0.6) | 4.8(1.3) | 179(41) |
| $^{13}CH_3CN$ | 6(3) − 5(3) | 107178.424(0) | 82.4 | 276.826 | 44 | 93.3(0.5) | 6.6(1.1) | 311(46) |
| $^{13}CH_3CN$ | 6(2) − 5(2) | 107188.500(1e-1) | 46.6 | 164.068 | 39 | 93.4(0.7) | 8.4(1.6) | 352(56) |
| $^{13}CH_3CN$ | 6(1) − 5(1) | 107194.550(1e-1) | 25.2 | 179.427 | 69 | 93.5(0.4) | 11.3(1.0) | 831(65) |
| $^{13}C^{17}O$ | 1(2) − 0(3) | 107288.550(5e-2) | 5.1 | 0.016 | 23 | 90.0(0.7) | 5.5(.14) | 125(31) |
| $CH_3COCH_3$ | 17(5, 12) − 17(4, 13) EE | 107376.810(15e-3) | 105.9 | 740.89033 | 28 | 92.7(0.8) | 7.7(1.5) | 230(43) |
| $CH_3COCH_3$ | 17(6, 12) − 17(5, 13) EE | 107376.851(15e-3) | 105.9 | 740.88976 | blended | − | − | − |
| $C_2H_5CN$ | 12(7, 5) − 11(7, 4) | 107485.160(5e-2) | 88.0 | 117.36 | 55 | 93.2(0.5) | 8.6(0.5) | 507(19) |
| $C_2H_5CN$ | 12(6, 6) − 11(6, 5) | 107486.949(5e-2) | 73.6 | 133.42 | 38 | 93.2(0.5) | 7.4(0.5) | 300(19) |
| $C_2H_5CN$ | 12(8, 4) − 11(8, 3) | 107491.574(5e-2) | 104.6 | 98.829 | 51 | 93.2(0.5) | 10.1(0.5) | 541(19) |
| $C_2H_5CN$ | 12(5, 7) − 11(5, 6) | 107502.432(5e-2) | 61.3 | 146.99 | 64 | 93.2(0.5) | 15.1(0.5) | 1035(19) |
| $C_2H_5CN$ | 12(10, 2) − 11(10, 1) | 107519.861(5e-2) | 144.6 | 54.355 | 26 | 93.2(0.5) | 13.6(0.5) | 375(19) |
| $CH_3COCH_3$ | 17(5, 12) − 17(4, 13) AA | 107525.628(19e-3) | 105.8 | 463.51993 | 14 | 92.5(0.5) | 16.5(0.5) | 253(19) |
| $CH_3COCH_3$ | 17(6, 12) − 17(5, 13) AA | 107525.670(19e-3) | 105.8 | 278.07892 | blended | − | − | − |
| $CH_3OCHO$ | 9( 2, 8) − 8( 2, 7) E | 107537.258(1e-2) | 28.8 | 22.60702 | 82 | 92.5(0.5) | 9.5(0.5) | 829(19) |
| $CH_3OCHO$ | 9( 2, 8) − 8( 2, 7) A | 107543.711(1e-2) | 28.8 | 22.61344 | 105 | 92.5(0.5) | 8.5(0.5) | 952(19) |
| $C_2H_5CN$ | 12(4, 9) − 11(4, 8) | 107544.042(5e-2) | 51.3 | 158.12 | blended | − | − | − |
| $C_2H_5CN$ | 12(4, 8) − 11(4, 7) | 107547.460(5e-2) | 51.3 | 158.11 | 63 | 93.0(0.5) | 7.0(0.5) | 468(19) |
| $C_2H_5CN$ | 12(3, 10) − 11(3, 9) | 107594.056(5e-2) | 43.6 | 166.77 | 55 | 93.0(1.1) | 13.9(3.7) | 1444(155) |
| $CH_3OCHO$ | 23(6, 17) − 23(5, 18) E | 107604.366(1e-2) | 189.0 | 7.68978 | blended | − | − | − |
| $C_2H_5CN$ | 12(3, 9) − 11(3, 8) | 107734.723(5e-2) | 43.6 | 166.76 | 59 | 93.0(0.3) | 8.7(0.9) | 550(45) |
| $OC^{33}S$ | 9 − 8 | 108084.784(2e-3) | 25.9 | 4.605 | 24 | 93.7(0.5) | 10.2(0.5) | 256(12) |
| t-HCOOH | 5(1, 5) − 4(1, 4) | 108126.720(3e-3) | 18.8 | 9.6966 | 48 | 92.5(0.3) | 5.1(0.7) | 258(33) |
| $CH_3COCH_3$ | 8(3, 5) − 7(4, 4) EE | 108387.595(8e-3) | 88.2 | 519.86714 | 20 | 92.7(1.3) | 14.7(4.3) | 311(64) |
| $CH_3COCH_3$ | 14(2, 12) − 14(1, 13) EE | 108434.511(16e-3) | 63.4 | 313.86255 | 31 | 92.7(0.4) | 2.7(1.7) | 88(34) |
| $C_2H_5OH$ | 13(3, 10) − 13(2, 11) | 108438.579(5e-2) | 88.2 | 18.79 | 27 | 93.5(0.7) | 7.5(1.7) | 219(42) |
| $^{13}CN$ | 1(1, 1) − 0(1, 0), F = 0 − 1 | 108631.121(5e-2) | 5.2 | 0.642 | 37 | 91.6(0.5) | 2.8(0.5) | 108(22) |
| $^{13}CN$ | 1(1, 1) − 0(1, 0), F = 1 − 1 | 108636.923(5e-2) | 5.2 | 1.932 | 72 | 91.3(0.5) | 7.2(0.5) | 549(22) |
| $^{13}CN$ | 1(2, 1) − 0(1, 1), F = 1 − 0 | 108638.212(5e-2) | 5.2 | 0.722 | blended | − | − | − |
| $^{13}CN$ | 1(2, 1) − 0(1, 1), F = 2 − 1 | 108643.590(5e-2) | 5.2 | 0.856 | 48 | 91.2(0.5) | 9.5(0.5) | 641(22) |
| $^{13}CN$ | 1(2, 1) − 0(1, 1), F = 0 − 1 | 108644.346(5e-2) | 5.2 | 0.642 | blended | − | − | − |
| $^{13}CN$ | 1(2, 1) − 0(1, 1), F = 1 − 1 | 108645.064(5e-2) | 5.2 | 0.551 | blended | − | − | − |
| $^{13}CN$ | 1(1, 1) − 0(1, 0), F = 2 − 1 | 108651.297(5e-2) | 5.2 | 3.276 | 85 | 91.1(0.5) | 3.4(0.5) | 308(22) |
| $^{13}CN$ | 1(2, 1) − 0(1, 1), F = 2 − 2 | 108657.646(5e-2) | 5.2 | 2.420 | 81 | 91.3(0.5) | 6.6(0.5) | 570(22) |
| $^{13}CN$ | 1(2, 1) − 0(1, 1), F = 1 − 2 | 108658.948(5e-2) | 5.2 | 0.669 | blended | − | − | − |
| $^{13}CN$ | 1(2, 2) − 0(1, 1), F = 3 − 2 | 108780.201(5e-2) | 5.2 | 4.905 | 138 | 91.2(0.1) | 3.6(0.3) | 527(36) |
| $^{13}CN$ | 1(2, 2) − 0(1, 1), F = 2 − 1 | 108782.374(5e-2) | 5.2 | 2.586 | 64 | 91.3(0.2) | 3.2(0.5) | 217(31) |
| $^{13}CN$ | 1(2, 2) − 0(1, 1), F = 1 − 0 | 108786.982(5e-2) | 5.2 | 1.144 | 29 | 91.2(0.7) | 1.9(1.6) | 58(22) |
| $^{13}CN$ | 1(2, 2) − 0(1, 1), F = 1 − 1 | 108793.753(5e-2) | 5.2 | 0.894 | 29 | 91.3(0.7) | 5.2(1.6) | 160(41) |
| $^{13}CN$ | 1(2, 2) − 0(1, 1), F = 2 − 2 | 108796.400(5e-2) | 5.2 | 0.918 | 40 | 91.3(0.4) | 3.0(0.8) | 131(30) |
| $CH_3OH$, vt=0-2 | 0(0) − 1(-1) E2, vt=0 | 108893.945(12e-3) | 13.1 | 3.9134 | 1039 | 93.0(0.) | 6.9(0.1) | 7669(63) |
| $C_2H_5CN$ | 12(2, 10) − 11(2, 9) | 108940.554(5e-2) | 38.2 | 172.93 | 55 | 93.0(0.4) | 8.6(0.9) | 509(47) |
| $O^{13}CS$ | 9 − 8 | 109110.845(2e-3) | 26.2 | 4.605 | 65 | 92.8(0.5) | 6.8(0.5) | 464(166) |
| $CH_3OH$, vt=0-2 | 14(5) − 15(4) E1, vt=0 | 109138.783(15e-3) | 379.7 | 13.593 | 74 | 93.0(0.3) | 8.7(0.6) | 685(44) |
| $CH_3OH$, vt=0-2 | 16(-2) − 16(1) E2, vt=0 | 109153.184(14e-3) | 342.0 | 14.726 | 65 | 93.0(0.3) | 7.3(0.7) | 507(41) |
| $HC_5N$ | 41 − 40 | 109160.973(7e-3) | 110.0 | 2306 | 53 | 92.5(0.6) | 8.5(1.8) | 922(77) |
| $HC_3N$ | 12 − 11 | 109173.634(1e-2) | 34.1 | 167.1 | 2379 | 92.0(0.) | 5.6(0.1) | 14294(150) |
| SO | 3(2) − 2(1) | 109252.220(1e-1) | 21.1 | 3.5585 | 392 | 92.5(0.1) | 6.5(0.2) | 2704(63) |
| $HC_3N$, $v_7$=1 | 12(-1) − 11(1) | 109442.013(2e-2) | 355.0 | 165.12 | 25 | 93.0(1.2) | 12.8(2.8) | 337(75) |
| OCS | 9 − 8 | 109463.063(5e-3) | 26.3 | 4.6034 | 632 | 93.0(0.) | 6.6(0.1) | 4419(54) |
| $CH_3OH$, vt=0-2 | $27(1)^- - 28(4)^-$, vt=2 | 109499.417(658e-3) | 1557.3 | 11.847 | 50 | 93.0(0.5) | 9.2(1.2) | 494(63) |
| $CH_3OCH_3$ | 8(2, 7) − 8(1, 8) EE | 109574.088(7e-3) | 38.3 | 95.791 | 75 | 93.5(0.5) | 6.5(0.5) | 1074(14) |
| $CH_3OCH_3$ | 8(2, 7) − 8(1, 8) AA | 109576.778(11e-3) | 38.3 | 59.869 | 55 | 93.5(0.5) | 4.2(0.5) | 243(14) |
| $HC_3N$, $v_7$=1 | 12(1) − 11(-1) | 109598.818(2e-5) | 355.0 | 165.12 | 25 | 93.0(0.5) | 6.5(0.5) | 353(14) |
| $C_2H_5CN$ | 12(1, 11) − 11(1, 10) | 109650.263(5e-2) | 53.4 | 176.49 | 64 | 93.0(0.4) | 8.6(1.2) | 582(60) |
| $NH_2CHO$ | 5(1, 4) − 4(1, 3) | 109753.549(25e-3) | 18.8 | 62.756 | 80 | 92.2(0.5) | 9.8(0.5) | 842(252) |
| $C^{18}O$ | 1 − 0 | 109782.173(6e-3) | 5.3 | 0.01221 | 4185 | 91.5(0.) | 4.0(0.5) | 17672(252) |
| HNCO | 5(2, 3) − 4(2, 2) | 109872.765(3e-2) | 186.1 | 10.012 | 30 | 93.0(0.8) | 3.1(2.3) | 101(58) |
| HNCO | 5(2, 4) − 4(2, 3) | 109872.337(3e-2) | 186.1 | 10.013 | blended | − | − | − |
| HNCO | 5(0, 5) − 4(0, 4) | 109905.749(7e-3) | 15.8 | 12.482 | 824 | 93.0(0.) | 5.8(0.1) | 5129(84) |
| $^{13}CO$ | 1 − 0 | 110201.35(0) | 5.3 | 0.01220 | 17180 | 92.0(0.1) | 4.1(0.5) | 74665(1020) |
| HNCO | 5(1, 4) − 4(1, 3) | 110298.089(5e-3) | 59.2 | 11.847 | 29 | 93.0(1.4) | 5.5(1.4) | 170(70) |
| $CH_3{}^{13}CN$ | 6(3) − 5(3) | 110309.800(1e-1) | 82.8 | 276.874 | 43 | 91.5(0.3) | 1.0(0.8) | 47(33) |
| $CH_3{}^{13}CN$ | 6(2) − 5(2) | 110320.400(1e-1) | 47.1 | 164.054 | 49 | 91.3(0.4) | 0.5(0.4) | 28(17) |
| $CH_3{}^{13}CN$ | 6(1) − 5(1) | 110326.770(1e-1) | 25.7 | 179.434 | 48 | 91.3(2.9) | 6.9(4.6) | 352(305) |
| $CH_3{}^{13}CN$ | 6(0) − 5(0) | 110328.870(1e-1) | 18.5 | 184.563 | 71 | 91.4(1.5) | 5.7(2.0) | 433(300) |
| $CH_3CN$ | 6(5, 0) − 5(5, 0) | 110330.345(0) | 197.1 | 56.399 | 71 | 92.3(1.5) | 5.7(2.0) | 433(300) |

**Table A2.** (Continued)

| Species | Transitions | Rest Freq. (MHz) | $E_u$ (K) | $\mu^2S$ ($D^2$) | $T_{mb}$ (mK) | $V_{LSR}$ (km $s^{-1}$) | $\Delta V$ (km $s^{-1}$) | $\int T_{mb}$ dv (mK km $s^{-1}$) |
|---|---|---|---|---|---|---|---|---|
| $CH_3CN$ | 6(4, 0) − 5(4, 0) | 110349.471(0) | 132.8 | 102.54 | 122 | 92.3(0.5) | 6.7(0.5) | 876(107) |
| $CH_3CN$ | 6(3, 0) − 5(-3, 0) | 110364.354(0) | 82.8 | 138.45 | 388 | 92.3(0.5) | 7.1(0.5) | 2948(107) |
| $CH_3CN$ | 6(-3, 0) − 5(3, 0) | 110364.354(0) | 82.8 | 138.45 | blended | – | – | – |
| $CH_3CN$ | 6(2, 0) − 5(2, 0) | 110374.989(0) | 47.1 | 164.06 | 441 | 92.3(0.5) | 7.0(0.5) | 3306(107) |
| $CH_3CN$ | 6(1, 0) − 5(1, 0) | 110381.372(0) | 25.7 | 179.45 | 754 | 92.5(0.5) | 6.5(0.5) | 5186(107) |
| $CH_3CN$ | 6(0, 0) − 5(0, 0) | 110383.500(0) | 18.5 | 184.58 | 826 | 92.5(0.5) | 5.9(0.5) | 5161(107) |
| $CH_3OCHO$ | 9(8, 1) − 8(8, 0) E | 110447.180(1e-2) | 69.0 | 5.02983 | 27 | 92.5(0.5) | 6.2(0.5) | 178(12) |
| $CH_3OCHO$ | 9(8, 1) − 8(8, 0) A | 110455.372(1e-2) | 69.0 | 5.02998 | blended | – | – | – |
| $CH_3OCHO$ | 9(8, 2) − 8(8, 1) E | 110458.014(1e-2) | 69.0 | 5.02965 | 24 | 92.5(0.5) | 6.2(0.5) | 157(12) |
| $CH_3OCHO$ | 9(7, 2) − 8(7, 1) E | 110525.741(1e-2) | 59.1 | 9.46492 | 39 | 92.5(0.7) | 6.1(1.6) | 253(52) |
| $CH_3OCHO$ | 9(7, 2) − 8(7, 1) A | 110535.186(1e-2) | 59.1 | 9.561 | 73 | 92.5(0.4) | 7.9(0.7) | 615(54) |
| $CH_3OCHO$ | 9(6, 3) − 8(6, 2) E | 110652.813(1e-2) | 50.5 | 13.30853 | 45 | 92.5(0.5) | 10.5(0.5) | 508(22) |
| $CH_3OCHO$ | 9(6, 3) − 8(6, 2) A | 110663.429(1e-2) | 50.4 | 13.31127 | 98 | 92.5(0.5) | 8.5(0.5) | 893(22) |
| $CH_3OCHO$ | 10(1,10) − 9(1, 9) E | 110788.664(1e-2) | 30.3 | 26.16584 | 129 | 92.5(0.3) | 8.8(0.5) | 1209(71) |
| $CH_3OCHO$ | 10(1,10) − 9(1, 9) A | 110790.526(1e-2) | 30.3 | 26.17539 | blended | – | – | – |
| $CH_3OCHO$ | 9(3, 7) − 8(3, 6) A | 110887.092(1e-2) | 32.6 | 21.25577 | 81 | 92.5(0.6) | 9.0(1.7) | 774(128) |
| $CH_3OCHO$ | 9(5, 4) − 8(5, 3) A | 110890.256(1e-2) | 43.2 | 16.56106 | blended | – | – | – |
| $C_2H_3CN$ | 2(2, 0) − 3(1, 3) | 110977.948(52e-3) | 499.7 | 0.0781 | 28 | 93.0(1.2) | 10.9(3.1) | 325(76) |
| $CH_3OCHO$ | 9(3, 7) − 8(3, 6) | 111005.672(1e-2) | 219.5 | 20.82222 | 69 | 92.5(0.3) | 4.1(0.8) | 304(45) |
| $CH_3OCHO$ | 10(0, 10) − 9(0, 9) E | 111169.903(1e-2) | 30.2 | 26.18776 | blended | – | – | – |
| $CH_3OCHO$ | 10(0, 10) − 9(0, 9) A | 111171.634(1e-2) | 30.2 | 26.19136 | 67 | 92.5(0.5) | 6.0(0.5) | 425(19) |
| $CH_3OCHO$ | 9(4, 6) − 8(4, 5) A | 111195.962(1e-2) | 37.2 | 19.21722 | 76 | 92.5(0.5) | 9.2(0.5) | 753(19) |
| $CH_3OCHO$ | 9(4, 6) − 8(4, 5) E | 111223.491(1e-2) | 37.2 | 18.18412 | blended | – | – | – |
| $CH_3COCH_3$ | 10(1, 9) − 9(2, 8)AE | 111243.339(11e-3) | 32.2 | 141.0573 | 32 | 92.8(1.0) | 8.9(2.6) | 298(67) |
| $CH_3COCH_3$ | 10(1, 9) − 9(2, 8)EE | 111267.514(8e-3) | 32.1 | 1128.14194 | 51 | 92.8(0.5) | 8.2(1.5) | 446(64) |
| $CH_3OH$, vt=0-2 | $7(2)^+ - 8(1)^+$, vt=0 | 111289.453(13e-3) | 102.7 | 9.3425 | 147 | 93.0(0.2) | 9.8(0.5) | 1532(69) |
| $CH_3OH$, vt=0-2 | 17(-2) − 17(1) E2, vt=0 | 111626.514(15e-3) | 381.5 | 20.231 | 66 | 93.0(0.6) | 7.8(1.3) | 551(7.1) |
| $CH_3OCHO$ | 10(1, 10) − 9(0, 9) A | 111735.307(1e-2) | 30.3 | 3.84224 | 52 | 92.5(0.5) | 6.8(0.5) | 645(26) |
| t-HCOOH | 5(0, 5) − 4(0, 4) | 111746.784(3e-3) | 16.1 | 10.092 | 121 | 92.0(0.5) | 5.7(0.5) | 1453(26) |
| $CH_3OCH_3$ | 19(3, 16) − 19(2, 17) AA | 111744.238(29e-3) | 187.5 | 259.8 | 57 | 93.5(0.5) | 7.4(0.5) | 446(26) |
| $CH_3OCH_3$ | 7(0, 7) − 6(1, 6) AA | 111782.562(8e-3) | 25.2 | 68.047 | 208 | 93.5(0.5) | 7.7(0.5) | 1713(26) |
| $CH_3OCH_3$ | 18(3, 15) − 18(2, 16) EE | 111813.668(21e-3) | 115.4 | 386.29 | 94 | 93.5(0.5) | 6.8(0.5) | 1258(26) |
| $CH_3CHO$ | 6(1, 6) − 5(1, 5) A, vt=0 | 112248.716(3e-3) | 21.1 | 73.76807 | 195 | 92.5(0.1) | 5.2(0.3) | 1088(57) |
| $CH_3CHO$ | 6(1, 6) − 5(1, 5) E, vt=0 | 112254.508(3e-3) | 21.2 | 73.79585 | 214 | 92.5(0.1) | 5.5(0.3) | 1248(58) |
| $C^{17}O$ | 1 − 0 | 112359.284(1e-3) | 5.4 | 0.01217 | 926 | 91.5(0.1) | 5.4(0.1) | 5311(77) |
| $CH_3COCH_3$ | 11(1, 11) − 10(0, 10) AE | 112365.987(13e-3) | 33.6 | 178.40946 | 44 | 93.0(1.2) | 6.2(4.3) | 574(129) |
| $CH_3COCH_3$ | 11(0, 11) − 10(1, 10) EE | 112373.549(9e-3) | 33.5 | 1426.94226 | 101 | 93.0(0.5) | 5.6(1.3) | 1195(123) |
| $CH_3COCH_3$ | 11(1, 11) − 10(0, 10) AA | 112381.030(14e-3) | 33.4 | 535.17491 | 51 | 93.0(1.2) | 7.6(3.1) | 824(140) |
| $C_2H_5CN$ | 13(1, 13) − 12(1, 12) | 112646.350(9e-2) | 39.0 | 191.45 | 80 | 93.0(0.7) | 6.8(2.2) | 1073(134) |
| $CH_3COCH_3$ | 8(8, 1) − 8(5, 4) EE | 112833.588(53e-3) | 34.1 | 0.45747 | 146 | 93.0(0.2) | 5.0(0.5) | 782(60) |
| $C_2H_3CN$ | 12(0, 12) − 11(0, 11) | 112840.637(1e-3) | 35.3 | 523.56 | 47 | 93.0(1.0) | 8.9(1.9) | 445(78) |
| t-HCOOH | 5(2, 3) − 4(2, 2) | 112891.443 (3e-3) | 28.9 | 8.4849 | 41 | 92.0(1.1) | 8.0(2.1) | 347(88) |
| $CH_3OCH_3$ | 20(3, 17) − 20(2, 18) EA | 112999.674(33e-3) | 206.1 | 55.102 | 101 | 93.5(0.4) | 13.1(1.3) | 1407(106) |
| $CH_3OCH_3$ | 20(3, 17) − 20(2, 18) AE | 112999.675(33e-3) | 206.1 | 110.17 | blended | – | – | – |
| $CH_3OCH_3$ | 17(3, 14) − 17(2, 15) EE | 113059.249(17e-3) | 153.1 | 354.12 | blended | – | – | – |
| $CH_3OCH_3$ | 17(3, 14) − 17(2, 15) AA | 113061.072(22e-3) | 153.1 | 221.33 | 109 | 93.5(0.5) | 15.2(1.2) | 1753(121) |
| CN | N= 1-0, J=1/2-1/2, F=1/2-1/2 | 113123.370(6e-3) | 5.4 | 0.15271 | 605 | 91.5(0.5) | 3.9(0.5) | 3529(196) |
| CN | N= 1-0, J=1/2-1/2, F=1/2-3/2 | 113144.157(6e-3) | 5.4 | 1.2492 | 1605 | 91.3(0.5) | 4.9(0.5) | 8288(296) |
| CN | N= 1-0, J=1/2-1/2, F=3/2-1/2 | 113170.492(4e-3) | 5.4 | 1.2199 | 2046 | 91.3(0.5) | 4.7(0.5) | 10330(196) |
| CN | N= 1-0, J=1/2-1/2, F=3/2-3/2 | 113191.279(3e-3) | 5.4 | 1.5836 | 1758 | 91.5(0.5) | 5.0(0.5) | 9318(196) |
| CN | N= 1-0, J=3/2-1/2, F=3/2-1/2 | 113488.120(3e-3) | 5.4 | 1.5838 | 1902 | 91.5(0.5) | 5.1(0.5) | 10268(348) |
| CN | N= 1-0, J=3/2-1/2, F=5/2-3/2 | 113490.970(2e-3) | 5.4 | 4.205 | 4002 | 91.2(0.5) | 5.5(0.5) | 23340(348) |
| CN | N= 1-0, J=3/2-1/2, F=1/2-1/2 | 113499.644(3e-3) | 5.4 | 1.2491 | 902 | 91.2(0.5) | 4.3(0.5) | 4140(348) |
| CN | N= 1-0, J=3/2-1/2, F=3/2-3/2 | 113508.907(3e-3) | 5.4 | 1.2196 | 1498 | 91.5(0.5) | 4.4(0.5) | 6970(348) |
| CN | N= 1-0, J=3/2-1/2, F=1/2-3/2 | 113520.432(4e-3) | 5.4 | 0.15263 | 254 | 91.5(0.5) | 4.4(0.5) | 11787(348) |
| | | G028.86+00.06 | | | | | | |
| $NH_2CHO$ | 5(2, 4) − 4(2, 3) | 105972.665(37e-3) | 27.2 | 54.915 | 14 | 103.0(1.5) | 10.8(5.2) | 164(85) |
| $NH_2CHO$ | 5(3, 3) − 4(3, 2) | 106134.468(55e-3) | 42.1 | 41.845 | 18 | 103.0(0.8) | 5.3(1.3) | 103(27) |
| $NH_2CHO$ | 5(3, 2) − 4(3, 1) | 106141.442(55e-3) | 42.1 | 41.84 | 15 | 103.0(0.7) | 3.6(1.2) | 59(22) |
| CCS | 8(9) − 7(8) | 106347.726(2e-2) | 25.0 | 74.425 | 155 | 103.1(0.1) | 3.0(0.2) | 494(24) |
| $HC_5N$ | 40 − 39 | 106498.910(7e-3) | 104.8 | 2249.7 | 32 | 103.1(0.3) | 3.3(0.9) | 112(24) |
| $NH_2CHO$ | 5(2, 3) − 4(2, 2) | 106541.773(37e-3) | 27.2 | 54.915 | 19 | 103.0(1.1) | 11.7(2.8) | 237(46) |
| $CH_3OH$, vt=0-2 | $3(1)^+ - 4(0)^+$, vt=0 | 107013.831(1e-2) | 28.3 | 12.036 | 242 | 103.5(0.1) | 4.8(0.2) | 1247(33) |
| $^{13}C^{17}O$ | 1(2) − 0(3) | 107288.550(5e-2) | 5.1 | 0.016 | 20 | 102.0(0.9) | 5.0(1.5) | 109(32) |
| $C_2H_5CN$ | 12(7, 5) − 11(7, 4) | 107485.160(5e-2) | 88.0 | 117.36 | 23 | 103.5(0.3) | 0.8(0.5) | 18(15) |
| $C_2H_5CN$ | 12(6, 6) − 11(6, 5) | 107486.949(5e-2) | 73.6 | 133.42 | 21 | 103.5(1.0) | 9.1(3.9) | 201(57) |
| $C_2H_5CN$ | 12(8, 4) − 11(8, 3) | 107491.574(5e-2) | 104.6 | 98.829 | 14 | 103.5(1.1) | 4.2(2.0) | 64(30) |
| $C_2H_5CN$ | 12(5, 7) − 11(5, 6) | 107502.432(5e-2) | 61.3 | 146.99 | 19 | 103.5(0.9) | 6.9(1.7) | 141(34) |
| $C_2H_5CN$ | 12(3, 9) − 11(3, 8) | 107734.723(5e-2) | 43.6 | 54.335 | 17 | 103.5(0.8) | 5.5(1.6) | 101(28) |
| $SO_2$ | 12(4, 8) − 13(3, 11) | 107843.470(2e-3) | 111.0 | 4.5354 | 29 | 105.2(0.4) | 3.5(1.0) | 108(26) |
| t-HCOOH | 5(1, 5) − 4(1, 4) | 108126.720(3e-3) | 18.8 | 9.6966 | 21 | 103.0(0.7) | 4.2(1.2) | 95(27) |
| $^{13}CN$ | 1(1, 0) − 0(1, 1), F = 1 − 1 | 108412.862(5e-2) | 5.2 | 0.635 | 50 | 103.5(0.1) | 1.1(0.4) | 57(17) |
| $^{13}CN$ | 1(1, 0) − 0(1, 1), F = 1 − 2 | 108426.889(5e-2) | 5.2 | 1.267 | 34 | 103.0(0.4) | 3.3(0.8) | 119(26) |
| $^{13}CN$ | 1(1, 1) − 0(1, 0), F = 1 − 1 | 108636.923(5e-2) | 5.2 | 1.932 | 49 | 103.2(0.3) | 2.7(1.0) | 144(36) |
| $^{13}CN$ | 1(2, 1) − 0(1, 1), F = 1 − 0 | 108638.212(5e-2) | 5.2 | 0.722 | 17 | 103.1(1.2) | 2.6(2.3) | 47(34) |
| $^{13}CN$ | 1(2, 1) − 0(1, 1), F = 2 − 1 | 108643.590(5e-2) | 5.2 | 0.856 | 25 | 103.0(0.4) | 1.3(0.6) | 36(18) |
| $^{13}CN$ | 1(2, 1) − 0(1, 1), F = 0 − 1 | 108644.346(5e-2) | 5.2 | 0.642 | 32 | 102.9(0.4) | 2.5(0.9) | 87(28) |
| $^{13}CN$ | 1(2, 1) − 0(1, 1), F = 1 − 1 | 108645.064(5e-2) | 5.2 | 0.551 | blended | – | – | – |
| $^{13}CN$ | 1(1, 1) − 0(1, 0), F = 2 − 1 | 108651.297(5e-2) | 5.2 | 3.276 | 77 | 103.1(0.2) | 2.7(0.4) | 225(28) |
| $^{13}CN$ | 1(2, 1) − 0(1, 1), F = 2 − 2 | 108657.646(5e-2) | 5.2 | 2.420 | 60 | 103.0(0.3) | 3.3(0.6) | 212(34) |
| $^{13}CN$ | 1(2, 1) − 0(1, 1), F = 1 − 2 | 108658.948(5e-2) | 5.2 | 0.669 | 28 | 103.1(0.3) | 0.8(0.5) | 21(18) |
| $^{13}CN$ | 1(2, 2) − 0(1, 1), F = 3 − 2 | 108780.201(5e-2) | 5.2 | 4.905 | 123 | 103.0(0.1) | 3.0(0.3) | 390(33) |
| $^{13}CN$ | 1(2, 2) − 0(1, 1), F = 2 − 1 | 108782.374(5e-2) | 5.2 | 2.586 | 54 | 103.2(0.3) | 2.8(0.5) | 161(29) |
| $^{13}CN$ | 1(2, 2) − 0(1, 1), F = 1 − 0 | 108786.982(5e-2) | 5.2 | 1.144 | 31 | 103.0(0.6) | 2.5(1.7) | 81(37) |
| $^{13}CN$ | 1(2, 2) − 0(1, 1), F = 1 − 1 | 108793.753(5e-2) | 5.2 | 0.894 | 44 | 103.1(0.3) | 1.3(0.4) | 60(19) |
| $CH_3OH$, vt=0-2 | 0(0) − 1(-1) E2, vt=0 | 108893.945(12e-3) | 13.1 | 3.9134 | 555 | 103.5(0.) | 3.7(0.1) | 2181(40) |
| $C_2H_5CN$ | 12(2, 10) − 11(2, 9) | 108940.554(5e-2) | 38.2 | 172.93 | 96 | 103.5(2.0) | 3.8(2.9) | 38(36) |
| $HC_3N$ | 12 − 11 | 109173.634(1e-2) | 34.1 | 167.1 | 1883 | 103.5(0.) | 3.5(0.1) | 6924(47) |
| SO | 3(2) − 2(1) | 109252.220(1e-1) | 21.1 | 3.5585 | 355 | 103.5(0.1) | 4.9(0.2) | 1835(49) |
| $HC_3N$, $v_7$=1 | 12(-1) − 11(1) | 109442.013(2e-2) | 355.0 | 165.12 | 22 | 104.2(0.7) | 4.4(2.1) | 104(43) |
| OCS | 9 − 8 | 109463.063(5e-3) | 26.3 | 4.6034 | 314 | 103.0(0.) | 4.1(0.2) | 1366(46) |
| $HC_3N$, $v_7$=1 | 12(1) − 11(-1) | 109598.818(2e-2) | 355.0 | 165.12 | 25 | 104.1(1.3) | 7.9(2.3) | 209(54) |
| $C^{18}O$ | 1 − 0 | 109782.173(6e-3) | 5.3 | 0.01221 | 5150 | 103.5(0.1) | 2.9(0.1) | 15663(83) |
| HNCO | 5(0, 5) − 4(0, 4) | 109905.749(7e-3) | 15.8 | 12.482 | 328 | 103.5(0.1) | 3.8(0.2) | 1333(54) |
| $C^{15}N$ | 1(2, 1) − 0(1, 0) | 110023.540(1e-1) | 5.3 | 1.386 | 35 | 102.7*0.5) | 4.2(1.5) | 152(41) |
| $C^{15}N$ | 1(2, 2) − 0(1, 1) | 110024.590(1e-1) | 5.3 | 3.504 | blended | – | – | – |
| $^{13}CO$ | 1 − 0 | 110201.35(0) | 5.3 | 0.01220 | 11713 | 103.5(0.5) | 3.2(0.5) | 39470(940) |
| $CH_3CN$ | 6(5, 0) − 5(5, 0) | 110330.345(0) | 197.1 | 56.399 | 22 | 103.6(1.0) | 3.1(2.0) | 75(45) |
| $CH_3CN$ | 6(4, 0) − 5(4, 0) | 110349.471(0) | 132.8 | 102.54 | 45 | 103.5(0.5) | 4.2(1.1) | 201(49) |

**Table A2.** (Continued)

| Species | Transitions | Rest Freq. (MHz) | $E_u$ (K) | $\mu^2 S$ ($D^2$) | $T_{mb}$ (mK) | $V_{LSR}$ (km $s^{-1}$) | $\Delta V$ (km $s^{-1}$) | $\int T_{mb}$ dv (mK km $s^{-1}$) |
|---|---|---|---|---|---|---|---|---|
| $CH_3CN$ | 6(3, 0) − 5(-3, 0) | 110364.354(0) | 82.8 | 138.45 | 167 | 103.5(0.2) | 5.2(0.4) | 933(57) |
| $CH_3CN$ | 6(-3, 0) − 5(3, 0) | 110364.354(0) | 82.8 | 138.45 | blended | − | − | − |
| $CH_3CN$ | 6(2, 0) − 5(2, 0) | 110374.989(0) | 47.1 | 164.06 | 200 | 103.5(0.1) | 4.4(0.3) | 926(54) |
| $CH_3CN$ | 6(1, 0) − 5(1, 0) | 110381.372(0) | 25.7 | 179.45 | 368 | 103.5(0.1) | 4.7(0.2) | 1834(72) |
| $CH_3CN$ | 6(0, 0) − 5(0, 0) | 110383.500(0) | 18.5 | 184.58 | 414 | 103.5(0.1) | 3.8(0.2) | 1679(66) |
| $CH_3OH$ | $7(2)^+ - 8(1)^+$, vt=0 | 111289.453(13e-3) | 102.7 | 9.3425 | 30 | 103.5(1.1) | 4.4(2.1) | 140(66) |
| $CH_3OCH_3$ | 7(0, 7) − 6(1, 6) AA | 111782.562(8e-3) | 25.2 | 68.047 | 25 | 102.8(0.7) | 1.8(1.5) | 41(40) |
| $CH_3OCH_3$ | 7(0, 7) − 6(1, 6) EE | 111783.010(4e-2) | 25.3 | 108.87 | blended | − | − | − |
| $CH_3CHO$ | 6(1, 6) − 5(1, 5) A, vt=0 | 112248.716(3e-3) | 21.1 | 73.76807 | 60 | 103.2(0.5) | 2.4(0.9) | 154(56) |
| $CH_3CHO$ | 6(1, 6) − 5(1, 5) E, vt=0 | 112254.508(3e-3) | 21.2 | 73.79585 | 81 | 103.2(0.3) | 1.7(0.7) | 149(52) |
| $C^{17}O$ | 1 − 0 | 112359.284(1e-3) | 5.4 | 0.01217 | 949 | 103.2(0.1) | 6.3(0.1) | 6376(69) |
| CN | N= 1-0, J=1/2-1/2, F=1/2-1/2 | 113123.370(6e-3) | 5.4 | 0.15271 | 512 | 103.0(0.5) | 3.2(0.5) | 1760(120) |
| CN | N= 1-0, J=1/2-1/2, F=1/2-3/2 | 113144.157(6e-3) | 5.4 | 1.2492 | 1037 | 103.0(0.5) | 4.6(0.5) | 5033(120) |
| CN | N= 1-0, J=1/2-1/2, F=3/2-1/2 | 113170.492(4e-3) | 5.4 | 1.2199 | 1444 | 103.0(0.5) | 3.9(0.5) | 5920(120) |
| CN | N= 1-0, J=1/2-1/2, F=3/2-3/2 | 113191.279(3e-3) | 5.4 | 1.5836 | 1058 | 103.0(0.5) | 5.1(0.5) | 5696(120) |
| CN | N= 1-0, J=3/2-1/2, F=3/2-1/2 | 113488.120(3e-3) | 5.4 | 1.5838 | 1100 | 103.0(0.5) | 4.2(0.5) | 4940(114) |
| CN | N= 1-0, J=3/2-1/2, F=5/2-3/2 | 113490.970(2e-3) | 5.4 | 4.205 | 1051 | 103.0(0.5) | 3.0(0.5) | 3341(114) |
| CN | N= 1-0, J=3/2-1/2, F=1/2-1/2 | 113499.644(3e-3) | 5.4 | 1.2491 | 194 | 103.0(0.5) | 2.0(0.5) | 663(114) |
| CN | N= 1-0, J=3/2-1/2, F=3/2-3/2 | 113508.907(3e-3) | 5.4 | 1.2196 | 805 | 103.0(0.5) | 4.0(0.5) | 3465(114) |
| CN | N= 1-0, J=3/2-1/2, F=1/2-3/2 | 113520.432(4e-3) | 5.4 | 0.15263 | 220 | 103.0(0.5) | 5.8(0.5) | 1350(114) |
| | | | | G029.95−00.01 | | | | |
| $NH_2CHO$ | 5(2, 4) − 4(2, 3) | 105972.665(37e-3) | 27.2 | 54.915 | 73 | 98.1(0.3) | 6.3(0.8) | 486(53) |
| $NH_2CHO$ | 5(4, 1) − 4(4, 0) | 106107.870(88e-3) | 63.0 | 23.537 | 43 | 98.1(0.5) | 4.3(0.9) | 196(41) |
| $NH_2CHO$ | 5(3, 3) − 4(3, 2) | 106134.468(55e-3) | 42.1 | 41.845 | 42 | 98.0(0.6) | 7.7(1.7) | 345(60) |
| $NH_2CHO$ | 5(3, 2) − 4(3, 1) | 106141.442(55e-3) | 42.1 | 41.84 | 57 | 98.0(0.5) | 7.6(1.0) | 462(55) |
| CCS | 8(9) − 7(8) | 106347.726(2e-2) | 25.0 | 74.425 | 242 | 97.3(0.1) | 3.3(0.1) | 837(33) |
| $HC_5N$ | 40 − 39 | 106498.910(7e-3) | 104.8 | 2249.7 | 69 | 97.5(0.3) | 4.2(0.6) | 309(36) |
| $NH_2CHO$ | 5(2, 3) − 4(2, 2) | 106541.773(37e-3) | 27.2 | 54.915 | 63 | 98.0(0.4) | 4.3(0.9) | 289(46) |
| $C_2H_3CN$ | 11(1, 10) − 10(1, 9) | 106641.383(1e-3) | 32.9 | 475.24 | 61 | 98.8(0.5) | 8.1(1.3) | 524(66) |
| H$\alpha$ | H (39) $\alpha$ | 106737.357(0) | − | − | 505 | 95.9(0.2) | 29.8(0.4) | 16016(190) |
| $CH_3OCH_3$ | 9(1, 8) − 8(2, 7) AA | 106775.602(14e-1) | 43.4 | 58.573 | 78 | 95.0(0.6) | 8.4(1.3) | 1401(98) |
| $OC^{34}S$ | 9 − 8 | 106787.390(2e-3) | 25.6 | 4.601 | 74 | 97.9(0.4) | 11.4(1.9) | 901(108) |
| $CH_3OH$, vt=0-2 | $3(1)^+ - 4(0)^+$, vt=0 | 107013.831(1e-2) | 28.3 | 12.036 | 686 | 98.0(0.) | 6.3(0.1) | 45738(76) |
| $C_2H_5CN$ | 12(2, 11) − 11(2, 10) | 107043.527(5e-2) | 37.9 | 172.86 | 91 | 97.5(0.3) | 7.0(0.7) | 685(57) |
| $CH_3OH$, vt=0-2 | 15(-2) − 15(1) E2, vt=0 | 107159.906(14e-3) | 304.7 | 10.421 | 120 | 98.2(0.3) | 5.2(0.7) | 660(73) |
| $C_2H_5CN$ | 12(7, 5) − 11(7, 4) | 107485.160(5e-2) | 88.0 | 117.36 | 108 | 97.4(0.4) | 4.3(1.1) | 489(111) |
| $C_2H_5CN$ | 12(6, 6) − 11(6, 5) | 107486.949(5e-2) | 73.6 | 133.42 | 107 | 97.4(0.4) | 3.8(1.1) | 436(104) |
| $C_2H_5CN$ | 12(8, 4) − 11(8, 3) | 107491.574(5e-2) | 104.6 | 98.829 | 58 | 97.4(0.5) | 3.7(1.2) | 228(60) |
| $C_2H_5CN$ | 12(5, 7) − 11(5, 6) | 107502.432(5e-2) | 61.3 | 146.99 | 107 | 97.4(0.3) | 7.2(0.8) | 821(79) |
| $C_2H_5CN$ | 12(10, 2) − 11(10, 1) | 107519.861(5e-2) | 144.6 | 54.355 | 48 | 97.5(0.5) | 2.7(1.3) | 139(51) |
| $C_2H_5CN$ | 12(4, 9) − 11(4, 8) | 107544.042(5e-2) | 51.3 | 158.12 | 124 | 97.5(0.2) | 4.6(0.7) | 603(71) |
| $C_2H_5CN$ | 12(4, 8) − 11(4, 7) | 107547.460(5e-2) | 51.3 | 158.11 | 89 | 97.5(0.3) | 4.9(0.8) | 466(66) |
| $C_2H_5CN$ | 12(3, 10) − 11(3, 9) | 107594.056(5e-2) | 43.6 | 166.77 | 83 | 97.5(0.4) | 4.2(0.9) | 376(64) |
| $C_2H_5CN$ | 12(3, 9) − 11(3, 8) | 107734.723(5e-2) | 43.6 | 166.76 | 72 | 97.3(0.5) | 5.4(1.0) | 412(71) |
| t-HCOOH | 5(1, 5) − 4(1, 4) | 108126.720(3e-3) | 18.8 | 9.6966 | 75 | 97.3(0.1) | 0.7(0.5) | 43(24) |
| $^{13}CN$ | 1(1, 1) − 0(1, 0), F = 0 − 1 | 108631.121(5e-2) | 5.2 | 0.642 | 40 | 96.8(0.3) | 0.8(0.5) | 33(21) |
| $^{13}CN$ | 1(1, 1) − 0(1, 0), F = 1 − 1 | 108636.923(5e-2) | 5.2 | 1.932 | 83 | 96.5(0.2) | 1.5(0.5) | 131(37) |
| $^{13}CN$ | 1(2, 1) − 0(1, 1), F = 1 − 0 | 108638.212(5e-2) | 5.2 | 0.722 | 43 | 96.5(0.4) | 1.5(0.7) | 67(31) |
| $^{13}CN$ | 1(2, 1) − 0(1, 1), F = 2 − 1 | 108643.590(5e-2) | 5.2 | 0.856 | 35 | 96.3(0.6) | 3.4(1.5) | 125(44) |
| $^{13}CN$ | 1(2, 1) − 0(1, 1), F = 0 − 1 | 108644.346(5e-2) | 5.2 | 0.642 | blended | − | − | − |
| $^{13}CN$ | 1(2, 1) − 0(1, 1), F = 1 − 1 | 108645.064(5e-2) | 5.2 | 0.551 | blended | − | − | − |
| $^{13}CN$ | 1(1, 1) − 0(1, 0), F = 2 − 1 | 108651.297(5e-2) | 5.2 | 3.276 | 124 | 96.6(0.2) | 3.1(0.3) | 412(40) |
| $^{13}CN$ | 1(2, 1) − 0(1, 1), F = 2 − 2 | 108657.646(5e-2) | 5.2 | 2.420 | 90 | 96.7(0.3) | 2.1(0.7) | 201(55) |
| $^{13}CN$ | 1(2, 1) − 0(1, 1), F = 1 − 2 | 108658.948(5e-2) | 5.2 | 0.669 | 84 | 96.5(0.1) | 0.9(0.5) | 79(45) |
| $^{13}CN$ | 1(2, 2) − 0(1, 1), F = 3 − 2 | 108780.201(5e-2) | 5.2 | 4.905 | 169 | 96.5(0.1) | 3.7(0.3) | 667(44) |
| $^{13}CN$ | 1(2, 2) − 0(1, 1), F = 2 − 1 | 108782.374(5e-2) | 5.2 | 2.586 | 97 | 96.5(0.2) | 3.0(0.4) | 306(38) |
| $^{13}CN$ | 1(2, 2) − 0(1, 1), F = 1 − 0 | 108786.982(5e-2) | 5.2 | 1.144 | 55 | 96.6(0.2) | 1.5(0.5) | 89(26) |
| $^{13}CN$ | 1(2, 2) − 0(1, 1), F = 1 − 1 | 108793.753(5e-2) | 5.2 | 0.894 | 37 | 96.5(0.5) | 3.2(1.0) | 124(38) |
| $^{13}CN$ | 1(2, 2) − 0(1, 1), F = 2 − 2 | 108796.400(5e-2) | 5.2 | 0.918 | 37 | 96.5(0.6) | 4.1(1.4) | 162(47) |
| $CH_3OH$, vt=0-2 | 0(0) − 1(-1) E2, vt=0 | 108893.945(12e-3) | 13.1 | 3.9134 | 705 | 97.8(0.) | 4.8(0.1) | 3572(54) |
| $CH_3OH$, vt=0-2 | 14(5) − 15(4) E1, vt=0 | 109138.783(15e-3) | 379.7 | 13.593 | 111 | 97.9(0.5) | 15.7(0.5) | 1860(40) |
| $CH_3OH$, vt=0-2 | 16(-2) − 16(1) E2, vt=0 | 109153.184 (14e-3) | 342.0 | 14.726 | 125 | 98.0(0.5) | 12.7(0.5) | 1692(40) |
| $HC_5N$ | 41 − 40 | 109160.973(7e-3) | 110.0 | 2306 | 59 | 97.0(0.5) | 10.9(0.5) | 683(40) |
| $HC_3N$ | 12 − 11 | 109173.634(1e-3) | 34.1 | 167.1 | 3055 | 96.8(0.) | 4.1(0.1) | 13452(127) |
| SO | 3(2) − 2(1) | 109252.220(1e-1) | 21.1 | 3.5585 | 747 | 97.1(0.1) | 6.6(0.4) | 5222(193) |
| $HC_3N$, $v_7$=1 | 12(-1) − 11(1) | 109442.013(2e-2) | 355.0 | 165.12 | 145 | 97.8(0.5) | 17.0(1.4) | 2617(167) |
| OCS | 9 − 8 | 109463.063(5e-3) | 26.3 | 4.6034 | 689 | 97.4(0.1) | 6.7(0.3) | 4913(147) |
| HNCO | 5(1, 5) − 4(1, 4) | 109495.996(6e-3) | 59.0 | 11.847 | 116 | 97.2(0.4) | 11.1(1.3) | 1373(118) |
| H$\gamma$ | H (55) $\gamma$ | 109536.001(0) | − | − | 81 | 99.1(1.3) | 30.6(4.8) | 2647(871) |
| $HC_3N$, $v_7$=1 | 12(1) − 11(-1) | 109598.818(2e-2) | 355.0 | 165.12 | 118 | 97.7(0.5) | 13.9(1.5) | 1746(173) |
| $C_2H_5CN$ | 12(1, 11) − 11(1, 10) | 109650.263(5e-2) | 35.4 | 176.49 | 103 | 97.5(0.3) | 6.7(0.8) | 736(69) |
| $NH_2CHO$ | 5(1, 4) − 4(1, 3) | 109753.549(25e-3) | 18.8 | 62.756 | 94 | 98.1(0.4) | 7.2(1.3) | 722(90) |
| $C^{18}O$ | 1 − 0 | 109782.173(6e-3) | 5.3 | 0.01221 | 5826 | 97.5(0.1) | 3.6(0.1) | 21703(88) |
| HNCO | 5(2, 3) − 4(2, 2) | 109872.765(3e-2) | 186.1 | 10.012 | 81 | 97.2(0.6) | 9.4(1.6) | 806(121) |
| HNCO | 5(2, 4) − 4(2, 3) | 109872.337(3e-2) | 186.1 | 10.013 | blended | − | − | − |
| HNCO | 5(0, 5) − 4(0, 4) | 109905.749(7e-3) | 15.8 | 12.482 | 457 | 97.0(0.1) | 5.0(0.3) | 2525(96) |
| $^{13}CO$ | 1 − 0 | 110201.35(0) | 5.3 | 0.01220 | 21872 | 97.2(0.5) | 4.5(0.5) | 103900(1810) |
| HNCO | 5(1, 4) − 4(1, 3) | 110298.089(5e-3) | 59.2 | 11.847 | 85 | 97.1(0.5) | 8.4(0.5) | 762(86) |
| $CH_3{}^{13}CN$ | 6(3) − 5(3) | 110309.800(1e-1) | 82.8 | 276.874 | 57 | 97.3(0.5) | 1.8(0.5) | 110(86) |
| $CH_3{}^{13}CN$ | 6(2) − 5(2) | 110320.400(1e-1) | 47.1 | 164.054 | 69 | 97.5(0.5) | 5.3(0.5) | 86(39) |
| $CH_3{}^{13}CN$ | 6(1) − 5(1) | 110326.770(1e-1) | 25.7 | 179.434 | 47 | 97.5(0.5) | 2.1(0.5) | 104(86) |
| $CH_3{}^{13}CN$ | 6(0) − 5(0) | 110328.870(1e-1) | 18.5 | 184.563 | 113 | 97.4(0.5) | 9.6(0.5) | 1152(86) |
| $CH_3CN$ | 6(4, 0) − 5(4, 0) | 110349.471(0) | 132.8 | 102.54 | 211 | 96.8(0.5) | 6.8(0.5) | 1522(86) |
| $CH_3CN$ | 6(3, 0) − 5(-3, 0) | 110364.354(0) | 82.8 | 138.45 | 497 | 96.7(0.5) | 6.8(0.5) | 3593(86) |
| $CH_3CN$ | 6(-3, 0) − 5(3, 0) | 110364.354(0) | 82.8 | 138.45 | blended | − | − | − |
| $CH_3CN$ | 6(2, 0) − 5(2, 0) | 110374.989(0) | 47.1 | 164.06 | 523 | 96.7(0.5) | 6.3(0.5) | 3536(86) |
| $CH_3CN$ | 6(1, 0) − 5(1, 0) | 110381.372(0) | 25.7 | 179.45 | 860 | 96.6(0.5) | 4.8(0.5) | 4432(86) |
| $CH_3CN$ | 6(0, 0) − 5(0, 0) | 110383.500(0) | 18.5 | 184.58 | 910 | 96.8(0.5) | 4.8(0.5) | 4670(86) |
| $CH_3OCHO$ | 9(7, 2) − 8(7, 1) E | 110525.741(1e-2) | 59.1 | 9.46492 | 44 | 96.6(1.0) | 5.6(2.3) | 261(80) |
| $CH_3OCHO$ | 9(7, 2) − 8(7, 1) A | 110535.186(1e-2) | 59.1 | 9.561 | 52 | 96.8(1.0) | 10.3(2.8) | 565(109) |
| $CH_3OCHO$ | 9(6, 3) − 8(6, 2) A | 110663.429(1e-2) | 50.4 | 13.31127 | 73 | 96.8(0.4) | 5.0(1.0) | 394(69) |
| $CH_3OCHO$ | 10(1,10) − 9(1, 9) E | 110788.664(1e-2) | 30.3 | 26.16584 | 68 | 96.8(0.9) | 2.4(1.1) | 169(66) |
| $CH_3OCHO$ | 10(1,10) − 9(1, 9) A | 110790.526(1e-2) | 30.3 | 26.17539 | blended | − | − | − |
| $CH_3OCHO$ | 9(5, 4) − 8(5, 3) E | 110873.955(1e-2) | 43.2 | 16.55557 | 76 | 96.7(0.5) | 11.7(0.5) | 946(25) |
| $CH_3OCHO$ | 9(5, 5) − 8(5, 4) A | 110880.447(1e-2) | 43.2 | 16.56015 | 87 | 96.7(0.5) | 8.9(0.5) | 829(25) |
| $CH_3OCHO$ | 9(5, 5) − 8(5, 4) E | 110882.331(1e-2) | 43.2 | 16.55225 | 56 | 96.7(0.4) | 11.3(0.5 | 675(25) |
| $CH_3OCHO$ | 9(3, 7) − 8(3, 6) A | 110887.092(1e-2) | 32.6 | 21.25577 | 70 | 96.6(0.3) | 5.0(0.5) | 372(25) |
| $CH_3OCHO$ | 9(5, 4) − 8(5, 3) A | 110890.256(1e-2) | 43.2 | 16.56106 | 72 | 96.7(0.5) | 4.1(0.5) | 316(25) |

**Table A2.** (Continued)

| Species | Transitions | Rest Freq. (MHz) | $E_u$ (K) | $\mu^2S$ ($D^2$) | $T_{mb}$ (mK) | $V_{LSR}$ (km $s^{-1}$) | ΔV (km $s^{-1}$) | $\int T_{mb}\,dv$ (mK km $s^{-1}$) |
|---|---|---|---|---|---|---|---|---|
| $CH_3OCHO$ | 10(0, 10) − 9(0, 9) E | 111169.903(1e-2) | 30.2 | 26.18776 | 76 | 96.6(0.5) | 2.7(0.9) | 217(92) |
| $CH_3OCHO$ | 10(0, 10) − 9(0, 9) A | 111171.634(1e-2) | 30.2 | 26.19136 | 64 | 96.6(0.7) | 4.8(2.5) | 325(126) |
| $CH_3OCHO$ | 9(4, 6) − 8(4, 5) A | 111195.962(1e-2) | 37.2 | 19.21722 | blended | – | – | – |
| $CH_3OCHO$ | 9(4, 6) − 8(4, 5) E | 111223.491(1e-2) | 37.2 | 18.18412 | 77 | 96.8(0.3) | 2.2(0.6) | 180(47) |
| $CH_3OH$, vt=0-2 | 7(2)$^+$ − 8(1)$^+$, vt=0 | 111289.453(13e-3) | 102.7 | 9.3425 | 263 | 97.8(0.2) | 7.8(0.4) | 2180(81) |
| $CH_3OH$, vt=0-2 | 15(2) − 14(5) E1, vt=1 | 111456.032(32e-3) | 677.6 | 0.079164 | 35 | 97.8(1.5) | 2.6(2.4) | 90(75) |
| $CH_3OH$, vt=0-2 | 17(-2) − 17(1) E2, vt=0 | 111626.514(15e-3) | 381.5 | 20.231 | 125 | 98.0(0.5) | 6.8(0.5) | 901(21) |
| $CH_3OCHO$ | 9(1, 8) − 8(1, 7) E | 111674.131(1e-2) | 28.1 | 23.18984 | 86 | 96.9(0.5) | 3.7(0.5) | 339(21) |
| $CH_3OCHO$ | 9(1, 8) − 8(1, 7) A | 111682.189(1e-2) | 28.1 | 23.19587 | 72 | 96.8(0.5) | 4.2(0.5) | 323(21) |
| $CH_3OCH_3$ | 19(3, 16) − 19(2, 17) AA | 111744.238(29e-3) | 187.5 | 259.8 | 108 | 95.1(0.5) | 10.7(0.5) | 1228(24) |
| $CH_3OCH_3$ | 7(0, 7) − 6(1, 6) AA | 111782.562(8e-3) | 25.2 | 68.047 | 180 | 95.1(0.5) | 6.5(0.5) | 1240(24) |
| $CH_3OCH_3$ | 18(3, 15) − 18(2, 16) AA | 111815.291(25e-3) | 168.9 | 386.29 | 104 | 95.0(0.5) | 10.1(0.5) | 1112(240 |
| $HC_5N$ | 42 − 41 | 111823.024(0) | 115.4 | 2362.2 | 53 | 97.0(0.5) | 10.8(0.5) | 604(24) |
| Hβ | H (48) β | 111885.070(0) | – | – | 143 | 96.5(0.8) | 23.9(1.6) | 3638(223) |
| $CH_3CHO$ | 6(1, 6) − 5(1, 5) A, vt=0 | 112248.716(3e-3) | 21.1 | 73.76807 | 104 | 96.4(0.3) | 2.5(0.6) | 276(65) |
| $CH_3CHO$ | 6(1, 6) − 5(1, 5) E, vt=0 | 112254.508(3e-3) | 21.2 | 73.79585 | 100 | 96.4(0.3) | 2.1(0.7) | 224(64) |
| $C^{17}O$ | 1 − 0 | 112359.284(1e-3) | 5.4 | 0.01217 | 1249 | 97.5(0.1) | 6.1(0.1) | 8114(94) |
| $CH_3OCH_3$ | 15(2, 14) − 14(3, 11) AA | 112371.536(23e-3) | 114.1 | 17.316 | 88 | 95.2(0.6) | 9.6(1.8) | 895(126) |
| $C_2H_5CN$ | 13(1, 13) − 12(1, 12) | 112646.350(9e-2) | 39.0 | 191.45 | 127 | 97.3(0.4) | 7.3(1.2) | 985(122) |
| $C_2H_3CN$ | 12(0, 12) − 11(0, 11) | 112840.637(1e-3) | 35.3 | 523.56 | 144 | 97.6(0.4) | 8.9(1.1) | 1376(148) |
| $CH_3OCH_3$ | 20(3, 17) − 20(2, 18) EA | 112999.674(33e-3) | 206.1 | 55.102 | 102 | 95.0(0.6) | 9.2(1.7) | 1006(132) |
| $CH_3OCH_3$ | 20(3, 17) − 20(2, 18) AE | 112999.675(33e-3) | 206.1 | 110.17 | blended | – | – | – |
| $CH_3OCH_3$ | 17(3, 14) − 17(2, 15) AA | 113061.072(22e-3) | 153.1 | 221.33 | 80 | 95.0(0.8) | 8.4(2.2) | 1430(150) |
| CN | N= 1-0, J=1/2-1/2, F=1/2-1/2 | 113123.370(6e-3) | 5.4 | 0.15271 | 527 | 97.4(0.5) | 4.3(0.5) | 2418(207) |
| CN | N= 1-0, J=1/2-1/2, F=1/2-3/2 | 113144.157(6e-3) | 5.4 | 1.2492 | 1885 | 97.4(0.5) | 3.9(0.5) | 7773(207) |
| CN | N= 1-0, J=1/2-1/2, F=3/2-1/2 | 113170.492(4e-3) | 5.4 | 1.2199 | 2540 | 97.4(0.5) | 3.8(0.5) | 10184(207) |
| CN | N= 1-0, J=1/2-1/2, F=3/2-3/2 | 113191.279(3e-3) | 5.4 | 1.5836 | 2126 | 97.4(0.5) | 4.2(0.5) | 9401(207) |
| CN | N= 1-0, J=3/2-1/2, F=3/2-1/2 | 113488.120(3e-3) | 5.4 | 1.5838 | 1866 | 97.4(0.5) | 3.5(0.5) | 6965(366) |
| CN | N= 1-0, J=3/2-1/2, F=5/2-3/2 | 113490.970(2e-3) | 5.4 | 4.205 | 5156 | 97.4(0.5) | 3.8(0.5) | 20965(366) |
| CN | N= 1-0, J=3/2-1/2, F=1/2-1/2 | 113499.644(3e-3) | 5.4 | 1.2491 | 890 | 97.4(0.5) | 4.0(0.5) | 3801(366) |
| CN | N= 1-0, J=3/2-1/2, F=3/2-3/2 | 113508.907(3e-3) | 5.4 | 1.2196 | 1660 | 97.4(0.5) | 3.7(0.5) | 6600(366) |
| CN | N= 1-0, J=3/2-1/2, F=1/2-3/2 | 113520.432(4e-3) | 5.4 | 0.15263 | 159 | 97.4(0.5) | 3.8(0.5) | 647(366) |
| | | | | G031.28+00.06 | | | | |
| $NH_2CHO$ | 5(2, 4) − 4(2, 3) | 105972.665(37e-3) | 27.2 | 54.915 | 28 | 109.0(1.0) | 7.1(2.8) | 209(68) |
| CCS | 8(9) − 7(8) | 106347.726(2e-2) | 25.0 | 74.425 | 143 | 108.7(0.1) | 3.6(0.3) | 547(35) |
| $C_2H_3CN$ | 11(1, 10) − 10(1, 9) | 106641.383(1e-3) | 32.9 | 476.24 | 52 | 109.1(0.2) | 1.8(0.5) | 98(24) |
| Hα | H (39) α | 106737.357(0) | – | – | 48 | 115.5(0.8) | 20.2(1.9) | 1029(85) |
| $CH_3OCH_3$ | 9(1, 8) − 8(2, 7) AA | 106775.602(14e-3) | 43.4 | 58.573 | 21 | 109.0(1.3) | 9.4(2.4) | 211(55) |
| $OC^{34}S$ | 9 − 8 | 106787.390(2e-3) | 25.6 | 4.601 | 50 | 109.1(0.3) | 2.8(0.6) | 149(31) |
| $CH_3OH$, vt=0-2 | 3(1)$^+$ − 4(0)$^+$, vt=0 | 107013.831(1e-2) | 28.3 | 12.036 | 677 | 109.2(0.) | 6.2(0.1) | 4453(55) |
| $CH_3OH$, vt=0-2 | 15(-2) − 15(1) E2, vt=0 | 107159.906(14e-3) | 304.7 | 0.017814 | 25 | 109.0(0.8) | 2.7( 1.5) | 73(37) |
| $^{13}C^{17}O$ | 1(2) − 0(3) | 107288.550(5e-2) | 5.1 | 0.016 | 33 | 107.2(0.6) | 4.0(1.2) | 141(38) |
| $CH_3OCHO$ | 9(2, 8) − 8(2, 7) E | 107537.258(1e-2) | 28.8 | 22.60702 | 40 | 109.1(0.7) | 8.6(1.3) | 362(53) |
| $CH_3OCHO$ | 9(2, 8) − 8(2, 7) A | 107543.711(1e-2) | 28.8 | 22.61344 | 55 | 109.1(0.5) | 7.4(1.5) | 440(60) |
| t-HCOOH | 5(1, 5) − 4(1, 4) | 108126.720(3e-3) | 18.8 | 9.6966 | 30 | 109.0(0.1) | 4.9(1.3) | 158(39) |
| $^{13}CN$ | 1(1, 1) − 0(1, 0), F = 0 − 1 | 108631.121(5e-2) | 5.2 | 0.642 | 30 | 109.0(0.4) | 2.3(1.1) | 73(29) |
| $^{13}CN$ | 1(1, 1) − 0(1, 0), F = 1 − 1 | 108636.923(5e-2) | 5.2 | 1.932 | 75 | 109.1(0.2) | 0.6(0.3) | 44(16) |
| $^{13}CN$ | 1(2, 1) − 0(1, 1), F = 1 − 0 | 108638.212(5e-2) | 5.2 | 0.722 | 70 | 109.0(0.3) | 4.4(0.7) | 325(46) |
| $^{13}CN$ | 1(2, 1) − 0(1, 1), F = 2 − 1 | 108643.590(5e-2) | 5.2 | 0.856 | 52 | 108.8(0.4) | 5.9(1.0) | 323(45) |
| $^{13}CN$ | 1(2, 1) − 0(1, 1), F = 0 − 1 | 108644.346(5e-2) | 5.2 | 0.642 | blended | – | – | – |
| $^{13}CN$ | 1(2, 1) − 0(1, 1), F = 1 − 1 | 108645.064(5e-2) | 5.2 | 0.551 | blended | – | – | – |
| $^{13}CN$ | 1(1, 1) − 0(1, 0), F = 2 − 1 | 108651.297(5e-2) | 5.2 | 3.276 | 104 | 109.0(0.2) | 3.7(0.3) | 411(35) |
| $^{13}CN$ | 1(2, 1) − 0(1, 1), F = 2 − 2 | 108657.646(5e-2) | 5.2 | 2.420 | 66 | 109.0(0.3) | 2.2(0.5) | 156(61) |
| $^{13}CN$ | 1(2, 1) − 0(1, 1), F = 1 − 2 | 108658.948(5e-2) | 5.2 | 0.669 | 58 | 109.0(0.6) | 5.0(1.1) | 308(74) |
| $^{13}CN$ | 1(2, 2) − 0(1, 1), F = 3 − 2 | 108780.201(5e-2) | 5.2 | 4.905 | 131 | 109.0(0.5) | 3.5(0.5) | 487(16) |
| $^{13}CN$ | 1(2, 2) − 0(1, 1), F = 2 − 1 | 108782.374(5e-2) | 5.2 | 2.586 | 78 | 109.0(0.5) | 2.5(0.5) | 211(16) |
| $^{13}CN$ | 1(2, 2) − 0(1, 1), F = 1 − 0 | 108786.982(5e-2) | 5.2 | 1.144 | 28 | 109.2(0.5) | 2.6(0.5) | 79(16) |
| $^{13}CN$ | 1(2, 2) − 0(1, 1), F = 1 − 1 | 108793.753(5e-2) | 5.2 | 0.894 | 15 | 109.1(0.5) | 1.7(0.5) | 28(16) |
| $^{13}CN$ | 1(2, 2) − 0(1, 1), F = 2 − 2 | 108796.400(5e-2) | 5.2 | 0.918 | 54 | 109.1(0.5) | 1.2(0.5) | 68(16) |
| $CH_3OH$, vt=0-2 | 0(0) − 1(-1) E2, vt=0 | 108893.945(12e-3) | 13.1 | 3.9134 | 1048 | 109.0(0.) | 4.6(0.1) | 5153(53) |
| $CH_3OH$, vt=0-2 | 14(5) − 15(4) E1, vt=0 | 109138.783(15e-3) | 379.7 | 13.593 | 31 | 109.2(1.2) | 13.5(2.2) | 447(71) |
| $CH_3OH$, vt=0-2 | 16(-2) − 16(1) E2, vt=0 | 109153.184(14e-3) | 342.0 | 14.726 | 44 | 109.0(0.7) | 10.0(1.5) | 472(62) |
| $HC_3N$ | 12 − 11 | 109173.634(1e-2) | 34.1 | 167.1 | 2977 | 109.0(0.) | 3.8(0.1) | 12059(69) |
| SO | 3(2) − 2(1) | 109252.220(1e-1) | 21.1 | 3.5585 | 557 | 109.0(0.) | 4.3(0.1) | 2577(56) |
| OCS | 9 − 8 | 109463.063(5e-3) | 26.3 | 4.6034 | 521 | 108.9(0.1) | 4.7(0.1) | 2627(60) |
| $CH_3OCH_3$ | 8(2, 7) − 8(1, 8) EE | 109574.088(7e-3) | 38.3 | 95.791 | 30 | 109.1(1.1) | 3.6(1.1) | 115(20) |
| $CH_3OCH_3$ | 8(2, 7) − 8(1, 8) AA | 109576.778(11e-3) | 38.3 | 59.869 | 81 | 109.1(1.0) | 6.4(1.1) | 142(20) |
| $NH_2CHO$ | 5(1, 4) − 4(1, 3) | 109753.549(25e-3) | 18.8 | 62.756 | 41 | 109.0(0.6) | 7.0(2.1) | 302(61) |
| $C^{18}O$ | 1 − 0 | 109782.173(6e-3) | 5.3 | 0.01221 | 4524 | 109.0(1.1) | 3.9(1.1) | 18568(717) |
| HNCO | 5(0, 5) − 4(0, 4) | 109905.749(7e-3) | 15.8 | 12.482 | 730 | 109.3(0.) | 4.2(0.1) | 3262(59) |
| $C^{15}N$ | 1(2, 1) − 0(1, 0) | 110023.540(1e-1) | 5.3 | 1.386 | 46 | 109.2(0.5) | 2.4(1.0) | 118(48) |
| $C^{15}N$ | 1(2, 2) − 0(1, 1) | 110024.590(1e-1) | 5.3 | 3.504 | blended | – | – | – |
| $^{13}CO$ | 1 − 0 | 110201.35(0) | 5.3 | 0.01220 | 8097 | 109.0(0.5) | 3.2(0.5) | 44913(837) |
| $CH_3CN$ | 6(4, 0) − 5(4, 0) | 110349.471(0) | 132.8 | 102.54 | 41 | 109.1(0.5) | 4.0(0.5) | 174(58) |
| $CH_3CN$ | 6(3, 0) − 5(-3, 0) | 110364.354(0) | 82.8 | 138.45 | 246 | 109.1(0.5) | 5.1(0.5) | 1331(58) |
| $CH_3CN$ | 6(-3, 0) − 5(3, 0) | 110364.354(0) | 82.8 | 138.45 | blended | – | – | – |
| $CH_3CN$ | 6(2, 0) − 5(2, 0) | 110374.989(0) | 47.1 | 164.06 | 321 | 109.0(0.5) | 4.3(0.5) | 1464(58) |
| $CH_3CN$ | 6(1, 0) − 5(1, 0) | 110381.372(0) | 25.7 | 179.45 | 630 | 109.0(0.4) | 4.6(0.5) | 3072(58) |
| $CH_3CN$ | 6(0, 0) − 5(0, 0) | 110383.500(0) | 18.5 | 184.58 | 755 | 109.1(0.5) | 5.40(0.5) | 3241(58) |
| $CH_3OCHO$ | 9(6, 3) − 8(6, 2) E | 110652.813(1e-2) | 50.5 | 13.30853 | 90 | 109.0(0.5) | 3.0(0.5) | 289(23) |
| $CH_3OCHO$ | 9(6, 3) − 8(6, 2) A | 110663.429(1e-2) | 50.4 | 13.31127 | 42 | 109.0(0.5) | 3.0(0.5) | 136(23) |
| $CH_3OCHO$ | 10(1,10) − 9(1, 9) E | 110788.664(1e-2) | 30.3 | 26.16584 | 37 | 109.0(0.5) | 3.1(1.8) | 124(59) |
| $CH_3OCHO$ | 10(1,10) − 9(1, 9) A | 110790.526(1e-2) | 30.3 | 26.17539 | 61 | 109.1(0.8) | 2.6(1.0) | 170(55) |
| $CH_3OCHO$ | 9(5, 4) − 8(5, 3) E | 110873.955(1e-2) | 43.2 | 16.5557 | 53 | 109.0(0.4) | 1.7(0.5) | 94(18) |
| $CH_3OCHO$ | 9(5, 5) − 8(5, 4) A | 110880.447(1e-2) | 43.2 | 16.56015 | 63 | 109.0(0.5) | 6.1(0.5) | 410(18) |
| $CH_3OCHO$ | 9(5, 5) − 8(5, 4) E | 110882.331(1e-2) | 43.2 | 16.55225 | 50 | 109.0(0.3) | 0.7(0.5) | 39(18) |
| $CH_3OCHO$ | 9(3, 7) − 8(3, 6) A | 110887.092(1e-2) | 32.6 | 21.25577 | 68 | 109.0(0.5) | 1.4(0.5) | 104(18) |
| $CH_3OH$, vt=0-2 | 7(2)$^+$ − 8(1)$^+$, vt=0 | 111289.453(13e-3) | 102.7 | 9.3425 | 86 | 109.0(0.5) | 6.0(0.9) | 548(84) |
| $CH_3OCHO$ | 9(1, 8) − 8(1, 7) E | 111674.131(1e-2) | 28.1 | 23.18984 | 39 | 109.2(0.8) | 3.0(1.5) | 124(61) |
| $CH_3OCHO$ | 9(1, 8) − 8(1, 7) A | 111682.189(1e-2) | 28.1 | 23.19587 | 94 | 109.0(0.3) | 1.1(0.1) | 108(69) |
| $CH_3OCH_3$ | 7(0, 7) − 6(1, 6) AA | 111782.562(8e-3) | 25.2 | 68.047 | 108 | 109.0(0.4) | 4.9(0.8) | 567(91) |
| $CH_3CHO$ | 6(1, 6) − 5(1, 5) A, vt=0 | 112248.716(3e-3) | 21.1 | 73.76807 | 123 | 108.8(0.3) | 3.7(0.7) | 478(87) |
| $CH_3CHO$ | 6(1, 6) − 5(1, 5) E, vt=0 | 112254.508(3e-3) | 21.2 | 73.79585 | 162 | 108.7(0.2) | 2.9(0.5) | 495(79) |
| $C^{17}O$ | 1 − 0 | 112359.284(1e-3) | 5.4 | 0.01217 | 1274 | 109.1(0.1) | 5.4(0.1) | 7338(83) |
| CN | N= 1-0, J=1/2-1/2, F=1/2-1/2 | 113123.370(6e-3) | 5.4 | 0.15271 | 457 | 109.0(0.1) | 4.7(0.2) | 2301(83) |
| CN | N= 1-0, J=1/2-1/2, F=1/2-3/2 | 113144.157(6e-3) | 5.4 | 1.2492 | 368 | 109.1(0.1) | 8.8(0.3) | 3427(107) |
| CN | N= 1-0, J=1/2-1/2, F=3/2-1/2 | 113170.492(4e-3) | 5.4 | 1.2199 | 545 | 109.1(0.1) | 7.9(0.2) | 4578(95) |
| CN | N= 1-0, J=1/2-1/2, F=3/2-3/2 | 113191.279(3e-3) | 5.4 | 1.5836 | 384 | 109.0(0.1) | 9.0(0.3) | 3659(102) |

**Table A2.** (Continued)

| Species | Transitions | Rest Freq. (MHz) | $E_u$ (K) | $\mu^2S$ ($D^2$) | $T_{mb}$ (mK) | $V_{LSR}$ (km $s^{-1}$) | ΔV (km $s^{-1}$) | $\int T_{mb}$ dv (mK km $s^{-1}$) |
|---|---|---|---|---|---|---|---|---|
| CN | N= 1-0, J=3/2-1/2, F=3/2-1/2 | 113488.120(3e-3) | 5.4 | 1.5838 | 515 | 109.1(1.1) | 2.8(1.1) | 1536(175) |
| CN | N= 1-0, J=3/2-1/2, F=5/2-3/2 | 113490.970(2e-3) | 5.4 | 4.205 | 939 | 109.0(1.1) | 3.9(1.1) | 3903(175) |
| CN | N= 1-0, J=3/2-1/2, F=1/2-1/2 | 113499.644(3e-3) | 5.4 | 1.2491 | 869 | 109.2(1.1) | 2.7(1.1) | 2510(175) |
| CN | N= 1-0, J=3/2-1/2, F=3/2-3/2 | 113508.907(3e-3) | 5.4 | 1.2196 | 285 | 109.2(1.1) | 6.3(1.1) | 1907(175) |
| CN | N= 1-0, J=3/2-1/2, F=1/2-3/2 | 113520.432(4e-3) | 5.4 | 0.15263 | 120 | 109.0(1.1) | 3.7(1.1) | 473(175) |
| | | | | G031.58+00.07 | | | | |
| CCS | 8(9) − 7(8) | 106347.726(2e-2) | 25.0 | 74.425 | 132 | 96.0(0.1) | 2.8(0.2) | 391(25) |
| $HC_5N$ | 40 − 39 | 106498.910(7e-3) | 104.8 | 2249.7 | 38 | 96.3(0.3) | 3.1(0.9) | 126(28) |
| $CH_3OH$, vt=0-2 | $3(1)^+ − 4(0)^+$, vt=0 | 107013.831(1e-2) | 28.3 | 12.036 | 241 | 96.5(0.1) | 4.2(0.2) | 1068(36) |
| $CH_3OH$, vt=0-2 | 15(-2) − 15(1) E2, vt=0 | 107159.906(14e-3) | 304.7 | 0.017814 | 20 | 96.6(0.6) | 2.6(1.0) | 57(22) |
| $CH_3OCHO$ | 9( 2, 8) − 8( 2, 7) E | 107537.258(1e-2) | 28.8 | 22.60702 | 26 | 96.5(0.5) | 2.4(1.3) | 67(30) |
| $CH_3OCHO$ | 9( 2, 8) − 8( 2, 7) A | 107543.711(1e-2) | 28.8 | 22.61344 | 15 | 96.5(0.9) | 1.8(1.6) | 30(24) |
| $^{13}CN$ | 1(1, 1) − 0(1, 0), F = 0 − 1 | 108631.121(5e-2) | 5.2 | 0.642 | 29 | 96.7(1.0) | 5.5(2.9) | 168(57) |
| $^{13}CN$ | 1(1, 1) − 0(1, 0), F = 1 − 1 | 108636.923(5e-2) | 5.2 | 1.932 | 39 | 96.5(0.6) | 8.4(1.6) | 349(57) |
| $^{13}CN$ | 1(2, 1) − 0(1, 1), F = 1 − 0 | 108638.212(5e-2) | 5.2 | 0.722 | blended | – | – | – |
| $^{13}CN$ | 1(2, 1) − 0(1, 1), F = 2 − 1 | 108643.590(5e-2) | 5.2 | 0.856 | 21 | 96.6(1.7) | 4.5(3.0) | 99(65) |
| $^{13}CN$ | 1(2, 1) − 0(1, 1), F = 0 − 1 | 108644.346(5e-2) | 5.2 | 0.642 | 47 | 96.5(0.5) | 3.3(1.3) | 163(68) |
| $^{13}CN$ | 1(2, 1) − 0(1, 1), F = 1 − 1 | 108645.064(5e-2) | 5.2 | 0.551 | blended | – | – | – |
| $^{13}CN$ | 1(1, 1) − 0(1, 0), F = 2 − 1 | 108651.297(5e-2) | 5.2 | 3.276 | 72 | 96.5(0.3) | 4.5(0.8) | 342(45) |
| $^{13}CN$ | 1(2, 1) − 0(1, 1), F = 2 − 2 | 108657.646(5e-2) | 5.2 | 2.420 | 44 | 96.8(0.6) | 8.6(2.0) | 398(66) |
| $^{13}CN$ | 1(2, 1) − 0(1, 1), F = 1 − 2 | 108658.948(5e-2) | 5.2 | 0.669 | blended | – | – | – |
| $^{13}CN$ | 1(2, 2) − 0(1, 1), F = 3 − 2 | 108780.201(5e-2) | 5.2 | 4.905 | 100 | 96.5(0.3) | 4.7(0.9) | 494(72) |
| $^{13}CN$ | 1(2, 2) − 0(1, 1), F = 2 − 1 | 108782.374(5e-2) | 5.2 | 2.586 | 66 | 96.5(0.4) | 3.0(1.0) | 214(61) |
| $^{13}CN$ | 1(2, 2) − 0(1, 1), F = 1 − 0 | 108786.982(5e-2) | 5.2 | 1.144 | 32 | 96.6(1.3) | 9.0(5.5) | 309(115) |
| $^{13}CN$ | 1(2, 2) − 0(1, 1), F = 1 − 1 | 108793.753(5e-2) | 5.2 | 0.894 | 16 | 96.5(0.4) | 2.1(0.8) | 35(20) |
| $^{13}CN$ | 1(2, 2) − 0(1, 1), F = 2 − 2 | 108796.400(5e-2) | 5.2 | 0.918 | 12 | 96.5(0.7) | 2.8(1.1) | 35(19) |
| $CH_3OH$, vt=0-2 | 0(0) − 1(-1) E2, vt=0 | 108893.945(12e-3) | 13.1 | 3.9134 | 633 | 96.4(0.1) | 4.8(0.1) | 3222(71) |
| $HC_3N$ | 12 − 11 | 109173.634(1e-2) | 34.1 | 167.1 | 2391 | 96.0(0.) | 3.3(0.1) | 8521(66) |
| SO | 3(2) − 2(1) | 109252.220(1e-1) | 21.1 | 3.5585 | 410 | 96.1(0.1) | 4.4(0.2) | 1937(72) |
| OCS | 9 − 8 | 109463.063(5e-3) | 26.3 | 4.6034 | 445 | 96.0(0.1) | 4.3(0.2) | 2036(79) |
| $C^{18}O$ | 1 − 0 | 109782.173(6e-3) | 5.3 | 0.01221 | 4646 | 96.0(0.5) | 3.4(0.5) | 16950(326) |
| HNCO | 5(0, 5) − 4(0, 4) | 109905.749(7e-3) | 15.8 | 12.482 | 572 | 96.0(0.) | 3.9(0.1) | 2373(49) |
| $^{13}CO$ | 1 − 0 | 110201.35(0) | 5.3 | 0.01220 | 14751 | 96.2(0.1) | 4.3(0.1) | 67567(648) |
| $CH_3CN$ | 6(4, 0) − 5(4, 0) | 110349.471(0) | 132.8 | 102.54 | 48 | 96.2(0.4) | 1.0(0.8) | 39(24) |
| $CH_3CN$ | 6(3, 0) − 5(-3, 0) | 110364.354(0) | 82.8 | 138.45 | 180 | 96.2(0.2) | 3.8(0.3) | 732(57) |
| $CH_3CN$ | 6(-3, 0) − 5(3, 0) | 110364.354(0) | 82.8 | 138.45 | blended | – | – | – |
| $CH_3CN$ | 6(2, 0) − 5(2, 0) | 110374.989(0) | 47.1 | 164.06 | 266 | 96.2(0.1) | 3.1(0.2) | 868(53) |
| $CH_3CN$ | 6(1, 0) − 5(1, 0) | 110381.372(0) | 25.7 | 179.45 | 504 | 96.2(0.1) | 3.6(0.1) | 1948(62) |
| $CH_3CN$ | 6(0, 0) − 5(0, 0) | 110383.500(0) | 18.5 | 184.58 | 619 | 96.1(0.) | 3.4(0.1) | 2210(61) |
| $CH_3OCH_3$ | 7(0, 7) − 6(1, 6) AA | 111782.562(8e-3) | 25.2 | 68.047 | 78 | 96.2(0.4) | 3.7(0.9) | 303(64) |
| $CH_3CHO$ | 6(1, 6) − 5(1, 5) A, vt=0 | 112248.716(3e-3) | 21.1 | 73.76807 | 125 | 96.0(0.3) | 3.0(0.6) | 398(67) |
| $CH_3CHO$ | 6(1, 6) − 5(1, 5) E, vt=0 | 112254.508(3e-3) | 21.2 | 73.79583 | 120 | 96.0(0.3) | 2.9(0.5) | 366(64) |
| $C^{17}O$ | 1 − 0 | 112359.284(1e-3) | 5.4 | 0.01217 | 1058 | 96.5(0.1) | 5.2(0.1) | 5813(63) |
| $C_2H_3CN$ | 12(0, 12) − 11(0, 11) | 112840.637(1e-3) | 35.3 | 523.56 | 134 | 95.8(0.2) | 3.0(0.4) | 426(47) |
| CN | N= 1-0, J=1/2-1/2, F=1/2-1/2 | 113123.370(6e-3) | 5.4 | 0.15271 | 786 | 96.0(0.5) | 5.1(0.5) | 4234(101) |
| CN | N= 1-0, J=1/2-1/2, F=1/2-3/2 | 113144.157(6e-3) | 5.4 | 1.2492 | 105 | 96.0(0.5) | 5.6(0.5) | 629(101) |
| CN | N= 1-0, J=1/2-1/2, F=3/2-1/2 | 113170.492(4e-3) | 5.4 | 1.2199 | 1002 | 96.1(0.5) | 4.6(0.5) | 4941(101) |
| CN | N= 1-0, J=1/2-1/2, F=3/2-3/2 | 113191.279(3e-3) | 5.4 | 1.5836 | 837 | 96.0(0.5) | 5.7(0.5) | 5119(101) |
| CCS | 9(8) − 8(7) | 113410.186(2e-2) | 33.6 | 65.427 | 73 | 96.0(0.5) | 4.5(0.5) | 354(120) |
| CN | N= 1-0, J=3/2-1/2, F=3/2-1/2 | 113488.120(3e-3) | 5.4 | 1.5838 | 744 | 96.0(0.5) | 4.9(0.5) | 3878(120) |
| CN | N= 1-0, J=3/2-1/2, F=5/2-3/2 | 113490.970(2e-3) | 5.4 | 4.205 | 1536 | 96.1(0.4) | 6.2(0.5) | 10093(120) |
| CN | N= 1-0, J=3/2-1/2, F=1/2-1/2 | 113499.644(3e-3) | 5.4 | 1.2491 | 452 | 96.0(0.7) | 4.8(0.5) | 2328(120) |
| CN | N= 1-0, J=3/2-1/2, F=3/2-3/2 | 113508.907(3e-3) | 5.4 | 1.2196 | 754 | 96.2(0.5) | 4.8(0.5) | 3876(120) |
| CN | N= 1-0, J=3/2-1/2, F=1/2-3/2 | 113520.432(4e-3) | 5.4 | 0.15263 | 159 | 96.0(0.5) | 3.8(0.5) | 648(120) |
| | | | | G032.04+00.05 | | | | |
| $NH_2CHO$ | 5(2, 4) − 4(2, 3) | 105972.665(37e-3) | 27.2 | 54.915 | 22 | 96.0(0.7) | 8.5(1.7) | 299(34) |
| $NH_2CHO$ | 5(3, 3) − 4(3, 2) | 106134.468(55e-3) | 42.1 | 41.845 | 21 | 96.1(0.4) | 2.6(1.7) | 58(24) |
| $NH_2CHO$ | 5(3, 2) − 4(3, 1) | 106141.442(55e-3) | 42.1 | 41.84 | 14 | 96.0(1.1) | 10.0(2.2) | 147(31) |
| CCS | 8(9) − 7(8) | 106347.726(2e-2) | 25.0 | 74.425 | 55 | 96.0(0.2) | 4.6(0.5) | 273(24) |
| $HC_5N$ | 40 − 39 | 106498.910(7e-3) | 104.8 | 2249.7 | 28 | 96.1(0.4) | 3.4(1.3) | 99(26) |
| $NH_2CHO$ | 5(2, 3) − 4(2, 2) | 106541.773(37e-3) | 27.2 | 54.915 | 21 | 96.0(0.9) | 11.0(1.9) | 245(37) |
| $^{34}SO$ | 3(2) − 2(1) | 106743.244(7e-2) | 20.9 | 3.557 | 27 | 95.6(0.5) | 4.9(1.5) | 139(32) |
| $CH_3OCH_3$ | 9(1, 8) − 8(2, 7) EE | 106777.344(9e-3) | 43.4 | 58.573 | 23 | 96.2(0.2) | 4.5(1.7) | 110(30) |
| $OC^{34}S$ | 9 − 8 | 106787.390(2e-3) | 25.6 | 4.601 | 28 | 95.9(0.5) | 4.8(0.9) | 142(27) |
| $CH_3OH$, vt=0-2 | $3(1)^+ − 4(0)^+$, vt=0 | 107013.831(1e-2) | 28.3 | 12.036 | 286 | 96.0(0.1) | 7.1(0.1) | 2148(37) |
| $C_2H_5CN$ | 12(2, 11) − 11(2, 10) | 107043.527(5e-2) | 37.9 | 172.86 | 25 | 95.8(0.6) | 6.0(1.3) | 161(31) |
| $CH_3OH$, vt=0-2 | 15(-2) − 15(1) E2, vt=0 | 107159.906(14e-3) | 304.7 | 10.421 | 26 | 96.1(0.4) | 2.9(1.2) | 80(25) |
| $^{13}CH_3CN$ | 6(2) − 5(2) | 107188.500(1e-1) | 46.6 | 164.068 | 15 | 95.4(0.5) | 1.2(0.5) | 19(8) |
| $^{13}CH_3CN$ | 6(1) − 5(1) | 107194.550(1e-1) | 25.2 | 179.427 | 22 | 95.6(0.5) | 3.4(0.5) | 78(8) |
| $^{13}CH_3CN$ | 6(0) − 5(0) | 107196.570(1e-1) | 18.0 | 184.590 | 14 | 95.6(0.5) | 5.2(0.5) | 80(8) |
| $C_2H_5CN$ | 12(5, 7) − 11(5, 6) | 107502.432(5e-2) | 61.3 | 146.99 | 14 | 95.8(0.4) | 7.0(1.4) | 103(25) |
| $CH_3OCHO$ | 9( 2, 8) − 8( 2, 7) E | 107537.258(1e-2) | 28.8 | 22.60702 | 21 | 96.0(0.3) | 4.3(1.4) | 94(27) |
| $CH_3OCHO$ | 9( 2, 8) − 8( 2, 7) A | 107543.711(1e-2) | 28.8 | 22.61344 | 41 | 96.1(0.3) | 3.4(0.6) | 148(25) |
| $C_2H_5CN$ | 12(4, 9) − 11(4, 8) | 107544.042(5e-2) | 51.3 | 158.12 | blended | – | – | – |
| $C_2H_5CN$ | 12(4, 8) − 11(4, 7) | 107547.460(5e-2) | 51.3 | 158.11 | 16 | 95.8(1.0) | 7.0(2.3) | 122(21) |
| $C_2H_5CN$ | 12(3, 10) − 11(3, 9) | 107594.056(5e-2) | 43.6 | 166.77 | 12 | 95.9(0.8) | 9.2(3.2) | 117(40) |
| $C_2H_5CN$ | 12(3, 9) − 11(3, 8) | 107734.723(5e-2) | 43.6 | 166.76 | 13 | 96.0(1.5) | 6.0(2.2) | 81(29) |
| t-HCOOH | 5(1, 5) − 4(1, 4) | 108126.720(3e-3) | 18.8 | 9.6966 | 31 | 95.8(0.5) | 7.7(1.5) | 251(37) |
| $^{13}CN$ | 1(1, 0) − 0(1, 1), F = 1 − 2 | 108426.889(5e-2) | 5.2 | 1.267 | 36 | 95.6(0.4) | 5.7(1.3) | 219(33) |
| $^{13}CN$ | 1(1, 1) − 0(1, 0), F = 1 − 1 | 108636.923(5e-2) | 5.2 | 1.932 | 61 | 95.4(0.1) | 2.6(0.4) | 166(21) |
| $^{13}CN$ | 1(2, 1) − 0(1, 1), F = 1 − 0 | 108638.212(5e-2) | 5.2 | 0.722 | 37 | 95.5(0.1) | 1.1(0.5) | 44(17) |
| $^{13}CN$ | 1(2, 1) − 0(1, 1), F = 2 − 1 | 108643.590(5e-2) | 5.2 | 0.856 | 46 | 95.5(0.1) | 0.5(0.2) | 27(11) |
| $^{13}CN$ | 1(2, 1) − 0(1, 1), F = 0 − 1 | 108644.346(5e-2) | 5.2 | 0.642 | 27 | 95.5(0.6) | 6.5(1.2) | 185(34) |
| $^{13}CN$ | 1(2, 1) − 0(1, 1), F = 1 − 1 | 108645.064(5e-2) | 5.2 | 0.551 | blended | – | – | – |
| $^{13}CN$ | 1(1, 1) − 0(1, 0), F = 2 − 1 | 108651.297(5e-2) | 5.2 | 3.276 | 75 | 95.5(0.2) | 4.8(0.4) | 384(29) |
| $^{13}CN$ | 1(2, 1) − 0(1, 1), F = 2 − 2 | 108657.646(5e-2) | 5.2 | 2.420 | 68 | 95.4(0.2) | 3.0(1.0) | 214(48) |
| $^{13}CN$ | 1(2, 1) − 0(1, 1), F = 1 − 2 | 108658.948(5e-2) | 5.2 | 0.669 | 21 | 95.5(0.7) | 2.8(1.1) | 62(31) |
| $^{13}CN$ | 1(2, 2) − 0(1, 1), F = 3 − 2 | 108780.201(5e-2) | 5.2 | 4.905 | 114 | 95.5(0.5) | 3.5(0.5) | 419(12) |
| $^{13}CN$ | 1(2, 2) − 0(1, 1), F = 2 − 1 | 108782.374(5e-2) | 5.2 | 2.586 | 56 | 95.5(0.5) | 3.9(0.5) | 233(12) |
| $^{13}CN$ | 1(2, 2) − 0(1, 1), F = 1 − 0 | 108786.982(5e-2) | 5.2 | 1.144 | 25 | 95.5(0.5) | 3.5(0.5) | 94(12) |
| $^{13}CN$ | 1(2, 2) − 0(1, 1), F = 1 − 1 | 108793.753(5e-2) | 5.2 | 0.894 | 39 | 95.4(0.5) | 1.4(0.5) | 59(12) |
| $^{13}CN$ | 1(2, 2) − 0(1, 1), F = 2 − 2 | 108796.400(5e-2) | 5.2 | 0.918 | 39 | 95.5(0.5) | 2.4(0.5) | 100(12) |
| $CH_3OH$, vt=0-2 | 0(0) − 1(-1) E2, vt=0 | 108893.945(12e-3) | 13.1 | 3.9134 | 952 | 96.1(0.) | 5.9(0.1) | 5940(47) |
| $C_2H_5CN$ | 12(2, 10) − 11(2, 9) | 108940.554(5e-2) | 38.2 | 172.93 | 22 | 96.0(0.8) | 5.8(1.5) | 135(34) |

**Table A2.** (Continued)

| Species | Transitions | Rest Freq. (MHz) | $E_u$ (K) | $\mu^2$S ($D^2$) | $T_{mb}$ (mK) | $V_{LSR}$ (km $s^{-1}$) | $\Delta$V (km $s^{-1}$) | $\int T_{mb}$ dv (mK km $s^{-1}$) |
|---|---|---|---|---|---|---|---|---|
| $HC_3N$ | 12 − 11 | 109173.634(1e-2) | 34.1 | 167.1 | 1854 | 96.0(0.) | 4.9(0.1) | 9689(68) |
| SO | 3(2) − 2(1) | 109252.220(1e-1) | 21.1 | 3.5585 | 409 | 96.2(0.1) | 6.8(0.2) | 2967(55) |
| OCS | 9 − 8 | 109463.063(5e-3) | 26.3 | 4.6034 | 417 | 96.0(0.) | 6.2(0.1) | 2749(46) |
| HNCO | 5(1, 5) − 4(1, 4) | 109495.996(6e-3) | 59.0 | 11.847 | 33 | 96.3(0.9) | 11.0(3.0) | 384(70) |
| $NH_2CHO$ | 5(1, 4) − 4(1, 3) | 109753.549(25e-3) | 18.8 | 62.756 | 24 | 96.0(1.2) | 8.7(6.7) | 421(42) |
| $C^{18}O$ | 1 − 0 | 109782.173(6e-3) | 5.3 | 0.01221 | 3366 | 96.0(0.1) | 4.7(0.1) | 16668(44) |
| HNCO | 5(0, 5) − 4(0, 4) | 109905.749(7e-3) | 15.8 | 12.482 | 1054 | 96.2(0.) | 4.4(0.1) | 4984(57) |
| $^{13}CO$ | 1 − 0 | 110201.35(0) | 5.3 | 0.01220 | 13435 | 95.5(0.5) | 5.4(0.5) | 76644(1160) |
| HNCO | 5(1, 4) − 4(1, 3) | 110298.089(5e-3) | 59.2 | 11.847 | 26 | 96.2(0.1) | 9.4(2.1) | 255(5.4) |
| $CH_3CN$ | 6(5, 0) − 5(5, 0) | 110330.345(0) | 197.1 | 56.399 | 25 | 96.1(0.5) | 9.3(0.5) | 248(61) |
| $CH_3CN$ | 6(4, 0) − 5(4, 0) | 110349.471(0) | 132.8 | 102.54 | 63 | 96.1(0.5) | 6.4(0.5) | 435(61) |
| $CH_3CN$ | 6(3, 0) − 5(-3, 0) | 110364.354(0) | 82.8 | 138.45 | 261 | 96.1(0.5) | 6.5(0.5) | 1805(61) |
| $CH_3CN$ | 6(-3, 0) − 5(3, 0) | 110364.354(0) | 82.8 | 138.45 | blended | – | – | – |
| $CH_3CN$ | 6(2, 0) − 5(2, 0) | 110374.989(0) | 47.1 | 164.06 | 280 | 96.1(0.5) | 6.1(0.5) | 1817(61) |
| $CH_3CN$ | 6(1, 0) − 5(1, 0) | 110381.372(0) | 25.7 | 179.45 | 530 | 96.1(0.5) | 5.9(0.5) | 3309(61) |
| $CH_3CN$ | 6(0, 0) − 5(0, 0) | 110383.500(0) | 18.5 | 184.58 | 570 | 96.1(0.5) | 5.1(0.5) | 3077(61) |
| $CH_3OCHO$ | 10(1,10) − 9(1, 9) E | 110788.664(1e-2) | 30.3 | 26.16584 | 33 | 96.0(0.5) | 4.7(1.1) | 166(38) |
| $CH_3OCHO$ | 10(1,10) − 9(1, 9) A | 110790.526(1e-2) | 30.3 | 26.17539 | 19 | 96.0(0.1) | 4.3(1.3) | 90(6) |
| $CH_3OCHO$ | 9(3, 7) − 8(3, 6) E | 110879.766(1e-2) | 32.6 | 21.245 | 38 | 96.1(0.6) | 4.8(1.1) | 192(41) |
| $CH_3OCHO$ | 10(0, 10) − 9(0, 9) E | 111169.903(1e-2) | 30.2 | 26.18776 | 45 | 96.0(0.3) | 2.2(0.7) | 108(29) |
| $CH_3OCHO$ | 10(0, 10) − 9(0, 9) A | 111171.634(1e-2) | 30.2 | 26.19136 | 28 | 96.0(0.7) | 3.3(1.0) | 98(34) |
| $CH_3OCHO$ | 9(4, 6) − 8(4, 5) A | 111195.962(1e-2) | 37.2 | 19.21722 | 37 | 96.1(0.1) | 7.1(1.1) | 62(22) |
| $CH_3OH$, vt=0-2 | $7(2)^+ - 8(1)^+$, vt=0 | 111289.453(13e-3) | 102.7 | 9.34234 | 75 | 96.0(0.3) | 6.7(0.6) | 537(44) |
| $CH_3OCHO$ | 9(4, 5) − 8(4, 4) A | 111453.300(1e-2) | 37.2 | 67.679 | 25 | 96.1(0.4) | 2.0(1.2) | 57(29) |
| $CH_3OH$, vt=0-2 | 17(-2) − 17(1) E2, vt=0 | 111626.514(15e-3) | 381.5 | 5.05816 | 22 | 95.7(1.0) | 6.4(1.4) | 150(38) |
| $CH_3OCHO$ | 9(1, 8) − 8(1, 7) E | 111674.131(1e-2) | 28.1 | 23.18984 | 52 | 95.9(0.2) | 2.3(0.6) | 125(27) |
| $CH_3OCHO$ | 9(1, 8) − 8(1, 7) A | 111682.189(1e-2) | 28.1 | 23.19587 | 28 | 95.9(0.7) | 5.8(1.2) | 173(38) |
| t-HCOOH | 5(0, 5) − 4(0, 4) | 111746.784(3e-3) | 16.1 | 10.092 | 50 | 96.0(0.3) | 3.2(0.7) | 170(30) |
| $CH_3OCH_3$ | 7(0, 7) − 6(1, 6) AA | 111782.562(8e-3) | 25.2 | 68.047 | 97 | 96.2(0.2) | 5.6(0.5) | 576(40) |
| $CH_3OCH_3$ | 18(3, 15) − 18(2, 16) EE | 111813.668(21e-3) | 115.4 | 386.29 | 21 | 96.2(1.0) | 6.8(2.0) | 149(41) |
| $CH_3CHO$ | 6(1, 6) − 5(1, 5) A, vt=0 | 112248.716(3e-3) | 21.1 | 73.76807 | 146 | 95.2(0.2) | 4.1(0.4) | 641(56) |
| $CH_3CHO$ | 6(1, 6) − 5(1, 5) E, vt=0 | 112254.508(3e-3) | 21.2 | 73.79585 | 127 | 95.2(0.2) | 5.1(0.6) | 699(65) |
| t-HCOOH | 5(2, 4) − 4(2, 3) | 112287.145 (3e-3) | 28.9 | 8.4851 | 27 | 96.0(1.2) | 6.6(2.6) | 187(66) |
| $C^{17}O$ | 1 − 0 | 112359.284(1e-3) | 5.4 | 0.01217 | 759 | 96.0(0.1) | 5.9(0.1) | 4772(70) |
| CN | N= 1-0, J=1/2-1/2, F=1/2-1/2 | 113123.370(6e-3) | 5.4 | 0.15271 | 488 | 95.0(0.5) | 3.6(0.5) | 1868(112) |
| CN | N= 1-0, J=1/2-1/2, F=1/2-3/2 | 113144.157(6e-3) | 5.4 | 1.2492 | 946 | 95.0(0.4) | 3.9(0.5) | 3963(112) |
| CN | N= 1-0, J=1/2-1/2, F=3/2-1/2 | 113170.492(4e-3) | 5.4 | 1.2199 | 1406 | 95.1(0.5) | 3.5( 0.5) | 5182(112) |
| CN | N= 1-0, J=1/2-1/2, F=3/2-3/2 | 113191.279(3e-3) | 5.4 | 1.5836 | 1084 | 95.0(0.7) | 3.7(0.5) | 4212(112) |
| CN | N= 1-0, J=3/2-1/2, F=3/2-1/2 | 113488.120(3e-3) | 5.4 | 1.5838 | 1095 | 95.1(0.5) | 4.5(0.5) | 5233(177) |
| CN | N= 1-0, J=3/2-1/2, F=5/2-3/2 | 113490.970(2e-3) | 5.4 | 4.205 | 2191 | 95.0(0.8) | 3.9(0.5) | 9104(177) |
| CN | N= 1-0, J=3/2-1/2, F=1/2-1/2 | 113499.644(3e-3) | 5.4 | 1.2491 | 572 | 95.0(0.5) | 3.4(0.5) | 2054(177) |
| CN | N= 1-0, J=3/2-1/2, F=3/2-3/2 | 113508.907(3e-3) | 5.4 | 1.2196 | 914 | 95.1(0.5) | 4.2(0.5) | 4054(177) |
| CN | N= 1-0, J=3/2-1/2, F=1/2-3/2 | 113520.432(4e-3) | 5.4 | 0.15263 | 232 | 95.0(0.6) | 3.7(0.5) | 902(177) |
| | | G034.39+00.22 | | | | | | |
| $NH_2CHO$ | 5(2, 4) − 4(2, 3) | 105972.665(37e-3) | 27.2 | 54.915 | 11 | 58.0(0.8) | 6.0(2.3) | 71(23) |
| CCS | 8(9) − 7(8) | 106347.726(2e-2) | 25.0 | 74.425 | 93 | 57.0(0.1) | 2.4(0.2) | 243(14) |
| $HC_5N$ | 40 − 39 | 106498.910(7e-3) | 104.8 | 2249.7 | 19 | 57.2(0.3) | 2.8(1.0) | 55(14) |
| $NH_2CHO$ | 5(2, 3) − 4(2, 2) | 106541.773(37e-3) | 27.2 | 54.915 | 90 | 58.1(1.1) | 7.2(2.2) | 69(20) |
| $CH_3OCHO$ | 9( 2, 8) − 8( 2, 7) E | 107537.258(1e-2) | 28.8 | 22.60702 | 21 | 57.0(0.4) | 2.8(2.0) | 63(18) |
| $CH_3OCHO$ | 9( 2, 8) − 8( 2, 7) A | 107543.711(1e-2) | 28.8 | 22.61344 | 17 | 57.1(0.9) | 9.0(2.8) | 161(34) |
| t-HCOOH | 5(1, 5) − 4(1, 4) | 108126.720(3e-3) | 18.8 | 9.6966 | 19 | 58.4(0.4) | 4.1(0.8) | 82(16) |
| $^{13}CN$ | 1(1, 0) − 0(1, 1), F = 1 − 2 | 108426.889(5e-2) | 5.2 | 1.267 | 34 | 57.6(0.2) | 1.9(0.6) | 70(15) |
| $^{13}CN$ | 1(1, 1) − 0(1, 0), F = 0 − 1 | 108631.121(5e-2) | 5.2 | 0.642 | 28 | 57.3(0.2) | 1.2(0.5) | 35(11) |
| $^{13}CN$ | 1(1, 1) − 0(1, 0), F = 1 − 1 | 108636.923(5e-2) | 5.2 | 1.932 | 55 | 57.5(0.1) | 1.6(0.3) | 91(12) |
| $^{13}CN$ | 1(2, 1) − 0(1, 1), F = 1 − 0 | 108638.212(5e-2) | 5.2 | 0.722 | 16 | 57.5(0.4) | 2.0(0.6) | 34(12) |
| $^{13}CN$ | 1(2, 1) − 0(1, 1), F = 2 − 1 | 108643.590(5e-2) | 5.2 | 0.856 | 21 | 57.4(0.4) | 2.5(0.8) | 55(16) |
| $^{13}CN$ | 1(2, 1) − 0(1, 1), F = 0 − 1 | 108644.346(5e-2) | 5.2 | 0.642 | 28 | 57.5(0.2) | 1.6(0.4) | 49(12) |
| $^{13}CN$ | 1(2, 1) − 0(1, 1), F = 1 − 1 | 108645.064(5e-2) | 5.2 | 0.551 | blended | – | – | – |
| $^{13}CN$ | 1(1, 1) − 0(1, 0), F = 2 − 1 | 108651.297(5e-2) | 5.2 | 3.276 | 75 | 57.7(0.1) | 2.6(0.2) | 208(15) |
| $^{13}CN$ | 1(2, 1) − 0(1, 1), F = 2 − 2 | 108657.646(5e-2) | 5.2 | 2.420 | 55 | 57.6(0.1) | 1.3(0.3) | 76(21) |
| $^{13}CN$ | 1(2, 1) − 0(1, 1), F = 1 − 2 | 108658.948(5e-2) | 5.2 | 0.669 | 19 | 57.6(0.8) | 5.8(1.8) | 118(33) |
| $^{13}CN$ | 1(2, 2) − 0(1, 1), F = 3 − 2 | 108780.201(5e-2) | 5.2 | 4.905 | 109 | 57.5(0.1) | 1.9(0.2) | 215(20) |
| $^{13}CN$ | 1(2, 2) − 0(1, 1), F = 2 − 1 | 108782.374(5e-2) | 5.2 | 2.586 | 60 | 57.6(0.2) | 1.9(0.4) | 124(21) |
| $^{13}CN$ | 1(2, 2) − 0(1, 1), F = 1 − 0 | 108786.982(5e-2) | 5.2 | 1.144 | 35 | 57.5(0.2) | 0.8(0.6) | 30(15) |
| $^{13}CN$ | 1(2, 2) − 0(1, 1), F = 1 − 1 | 108793.753(5e-2) | 5.2 | 0.894 | 17 | 57.6(0.4) | 0.5(0.3) | 100(12) |
| $^{13}CN$ | 1(2, 2) − 0(1, 1), F = 2 − 2 | 108796.400(5e-2) | 5.2 | 0.918 | 95 | 57.5(0.7) | 1.1(0.9) | 11(10) |
| $CH_3OH$, vt=0-2 | 0(0) − 1(-1) E2, vt=0 | 108893.945(12e-3) | 13.1 | 3.9134 | 403 | 56.5(0.) | 4.3(0.1) | 1850(32) |
| SiS | 6 − 5 | 108924.277(82e-3) | 18.3 | 5.62 | 21 | 56.4(0.2) | 3.5(0.5) | 17(11) |
| $HC_3N$ | 12 − 11 | 109173.634(1e-2) | 34.1 | 16.71 | 1373 | 56.5(0.) | 2.8(0.1) | 4152(30) |
| SO | 3(2) − 2(1) | 109252.220(1e-1) | 21.1 | 3.5585 | 210 | 56.0(0.1) | 3.8(0.1) | 845(26) |
| OCS | 9 − 8 | 109463.063(5e-3) | 26.3 | 4.6034 | 178 | 56.5(0.1) | 3.5(0.2) | 671(23) |
| $C^{18}O$ | 1 − 0 | 109782.173(6e-3) | 5.3 | 0.01221 | 2792 | 57.5(0.5) | 4.1(0.5) | 12195(180) |
| HNCO | 5(0, 5) − 4(0, 4) | 109905.749(7e-3) | 15.8 | 12.482 | 532 | 56.7(0.1) | 3.5(0.1) | 1960(39) |
| $^{13}CO$ | 1 − 0 | 110201.35(0) | 5.3 | 0.01220 | 10322 | 57.0(0.1) | 4.9(0.1) | 53360(328) |
| $CH_3CN$ | 6(4, 0) − 5(4, 0) | 110349.471(0) | 132.8 | 102.54 | 22 | 56.5(0.6) | 4.9(1.3) | 113(28) |
| $CH_3CN$ | 6(3, 0) − 5(-3, 0) | 110364.354(0) | 82.8 | 138.45 | 86 | 56.5(0.2) | 5.3(0.4) | 488(32) |
| $CH_3CN$ | 6(-3, 0) − 5(3, 0) | 110364.354(0) | 82.8 | 138.45 | blended | – | – | – |
| $CH_3CN$ | 6(2, 0) − 5(2, 0) | 110374.989(0) | 47.1 | 164.06 | 104 | 56.5(0.1) | 4.8(0.3) | 530(29) |
| $CH_3CN$ | 6(1, 0) − 5(1, 0) | 110381.372(0) | 25.7 | 179.45 | 235 | 56.5(0.1) | 3.8(0.2) | 947(31) |
| $CH_3CN$ | 6(0, 0) − 5(0, 0) | 110383.500(0) | 18.5 | 184.58 | 271 | 56.5(0.) | 3.9(0.1) | 1114(31) |
| $CH_3OCHO$ | 10(1,10) − 9(1, 9) E | 110788.664(1e-2) | 30.3 | 26.16584 | 25 | 56.8(0.2) | 1.0(0.5) | 14(8) |
| $CH_3OCHO$ | 10(1,10) − 9(1, 9) A | 110790.526(1e-2) | 30.3 | 16.17539 | 24 | 56.8(0.3) | 1.1(1.1) | 19(17) |
| $CH_3OCHO$ | 9(3, 7) − 8(3, 6) E | 110879.766(1e-2) | 32.6 | 21.245 | 20 | 56.8(0.9) | 4.5(1.7) | 97(35) |
| $CH_3OCH_3$ | 7(0, 7) − 6(1, 6) AA | 111782.562(8e-3) | 25.2 | 68.047 | 33 | 57.0(0.5) | 3.1(1.0) | 109(33) |
| $CH_3CHO$ | 6(1, 6) − 5(1, 5) A, vt=0 | 112248.716(3e-3) | 21.1 | 73.76807 | 86 | 57.2(0.2) | 2.6(0.5) | 238(44) |
| $CH_3CHO$ | 6(1, 6) − 5(1, 5) E, vt=0 | 112254.508(3e-3) | 21.2 | 73.79585 | 94 | 57.2(0.2) | 2.4(0.5) | 241(42) |
| $C^{17}O$ | 1 − 0 | 112359.284(1e-3) | 5.4 | 0.01217 | 680 | 57.0(0.1) | 5.3(0.1) | 3861(31) |
| CN | N= 1-0, J=1/2-1/2, F=1/2-1/2 | 113123.370(6e-3) | 5.4 | 0.15271 | 484 | 57.0(0.5) | 2.7(0.5) | 1371(75) |
| CN | N= 1-0, J=1/2-1/2, F=1/2-3/2 | 113144.157(6e-3) | 5.4 | 1.2492 | 725 | 57.0(0.5) | 3.3(0.5) | 2518(75) |
| CN | N= 1-0, J=1/2-1/2, F=3/2-1/2 | 113170.492(4e-3) | 5.4 | 1.2199 | 945 | 57.0(0.4) | 3.3(0.5) | 3341(75) |
| CN | N= 1-0, J=1/2-1/2, F=3/2-3/2 | 113191.279(3e-3) | 5.4 | 1.5836 | 702 | 57.1(0.5) | 3.7(0.5) | 2743(75) |
| CN | N= 1-0, J=3/2-1/2, F=3/2-1/2 | 113488.120(3e-3) | 5.4 | 1.5838 | 756 | 57.0(0.6) | 4.0(0.5) | 3187(111) |
| CN | N= 1-0, J=3/2-1/2, F=5/2-3/2 | 113490.970(2e-3) | 5.4 | 4.205 | 1091 | 57.1(0.5) | 3.5(0.5) | 4077(111) |
| CN | N= 1-0, J=3/2-1/2, F=1/2-1/2 | 113499.644(3e-3) | 5.4 | 1.2491 | 436 | 57.0(0.8) | 3.3(0.5) | 1538(111) |
| CN | N= 1-0, J=3/2-1/2, F=3/2-3/2 | 113508.907(3e-3) | 5.4 | 1.2196 | 725 | 57.1(0.5) | 2.8(0.5) | 2194(111) |
| CN | N= 1-0, J=3/2-1/2, F=1/2-3/2 | 113520.432(4e-3) | 5.4 | 0.15263 | 254 | 57.0(0.9) | 2.8(0.5) | 761(111) |
| | | G035.02+00.34 | | | | | | |

**Table A2.** (Continued)

| Species | Transitions | Rest Freq. | $E_u$ | $\mu^2$S | $T_{mb}$ | $V_{LSR}$ | $\Delta$V | $\int T_{mb}$ dv |
|---|---|---|---|---|---|---|---|---|
| | | (MHz) | (K) | (D$^2$) | (mK) | (km s$^{-1}$) | (km s$^{-1}$) | (mK km s$^{-1}$) |
| CCS | 8(9) − 7(8) | 106347.726(2e-2) | 25.0 | 74.425 | 121 | 53.0(0.1) | 3.4(0.2) | 439(24) |
| HC$_5$N | 40 − 39 | 106498.910(7e-3) | 104.8 | 2249.7 | 22 | 53.2(0.4) | 4.4(0.8) | 102(18) |
| $^{34}$SO | 3(2) − 2(1) | 106743.244(7e-2) | 20.9 | 3.557 | 26 | 51.6(0.3) | 3.9(1.0) | 106(23) |
| CH$_3$OH, vt=0-2 | 3(1)$^+$ − 4(0)$^+$, vt=0 | 107013.831(1e-2) | 28.3 | 12.036 | 403 | 52.3(0.) | 3.8(0.1) | 1610(22) |
| t-HCOOH | 5(1, 5) − 4(1, 4) | 108126.720(3e-3) | 18.8 | 9.6966 | 19 | 53.0(0.1) | 0.9(0.2) | 41(11) |
| $^{13}$CN | 1(1, 0) − 0(1, 1), F = 1 − 2 | 108426.889(5e-2) | 5.2 | 1.267 | 22 | 53.1(0.3) | 2.3(0.5) | 53(12) |
| $^{13}$CN | 1(1, 1) − 0(1, 0), F = 0 − 1 | 108631.121(5e-2) | 5.2 | 0.642 | 19 | 52.9(0.5) | 0.5(0.3) | 11(6) |
| $^{13}$CN | 1(1, 1) − 0(1, 0), F = 1 − 1 | 108636.923(5e-2) | 5.2 | 1.932 | 39 | 53.0(0.5) | 1.6(0.5) | 65(7) |
| $^{13}$CN | 1(2, 1) − 0(1, 1), F = 1 − 0 | 108638.212(5e-2) | 5.2 | 0.722 | 21 | 53.0(0.5) | 1.2(0.5) | 27(7) |
| $^{13}$CN | 1(2, 1) − 0(1, 1), F = 2 − 1 | 108643.590(5e-2) | 5.2 | 0.856 | 22 | 52.8(0.5) | 2.6(0.5) | 59(7) |
| $^{13}$CN | 1(2, 1) − 0(1, 1), F = 0 − 1 | 108644.346(5e-2) | 5.2 | 0.642 | 19 | 52.9(0.5) | 1.6(0.5) | 31(7) |
| $^{13}$CN | 1(2, 1) − 0(1, 1), F = 1 − 1 | 108645.064(5e-2) | 5.2 | 0.551 | blended | – | – | – |
| $^{13}$CN | 1(1, 1) − 0(1, 0), F = 2 − 1 | 108651.297(5e-2) | 5.2 | 3.276 | 49 | 53.0(0.5) | 3.4(0.5) | 180(7) |
| $^{13}$CN | 1(2, 1) − 0(1, 1), F = 2 − 2 | 108657.646(5e-2) | 5.2 | 2.420 | 27 | 53.0(0.5) | 2.9(0.5) | 83(7) |
| $^{13}$CN | 1(2, 1) − 0(1, 1), F = 1 − 2 | 108658.948(5e-2) | 5.2 | 0.669 | 16 | 53.0(0.5) | 3.4(0.5) | 58(7) |
| $^{13}$CN | 1(2, 2) − 0(1, 1), F = 3 − 2 | 108780.201(5e-2) | 5.2 | 4.905 | 69 | 53.1(0.1) | 3.5(0.3) | 258(19) |
| $^{13}$CN | 1(2, 2) − 0(1, 1), F = 2 − 1 | 108782.374(5e-2) | 5.2 | 2.586 | 40 | 53.0(0.2) | 2.9(0.6) | 124(19) |
| $^{13}$CN | 1(2, 2) − 0(1, 1), F = 1 − 0 | 108786.982(5e-2) | 5.2 | 1.144 | 19 | 53.0(0.4) | 2.3(0.7) | 47(15) |
| $^{13}$CN | 1(2, 2) − 0(1, 1), F = 1 − 1 | 108793.753(5e-2) | 5.2 | 0.894 | 17 | 52.9(0.5) | 2.8(1.2) | 52(18) |
| $^{13}$CN | 1(2, 2) − 0(1, 1), F = 2 − 2 | 108796.400(5e-2) | 5.2 | 0.918 | 10 | 53.0(0.6) | 2.3(1.6) | 25(15) |
| CH$_3$OH, vt=0-2 | 0(0) − 1(-1) E2, vt=0 | 108893.945(12e-3) | 13.1 | 3.9134 | 361 | 52.1(0.) | 3.3(0.1) | 1263(21) |
| HC$_3$N | 12 − 11 | 109173.634(1e-2) | 34.1 | 167.1 | 1751 | 53.0(0.) | 4.4(0.1) | 8156(23) |
| SO | 3(2) − 2(1) | 109252.220(1e-1) | 21.1 | 3.5585 | 610 | 52.5(0.) | 4.1(0.1) | 2673(32) |
| OCS | 9 − 8 | 109463.063(5e-3) | 26.3 | 4.6034 | 158 | 52.3(0.1) | 5.2(0.4) | 878(44) |
| C$^{18}$O | 1 − 0 | 109782.173(6e-3) | 5.3 | 0.01221 | 4103 | 52.0(0.1) | 2.7(0.1) | 11673(35) |
| HNCO | 5(0, 5) − 4(0, 4) | 109905.749(7e-3) | 15.8 | 12.482 | 263 | 53.1(0.1) | 3.0(0.1) | 833(20) |
| $^{13}$CO | 1 − 0 | 110201.35(0) | 5.3 | 0.01220 | 10413 | 52.0(0.5) | 4.6(0.5) | 51081(952) |
| CH$_3$CN | 6(4, 0) − 5(4, 0) | 110349.471(0) | 132.8 | 102.54 | 13 | 52.1(0.5) | 2.1(0.5) | 76(13) |
| CH$_3$CN | 6(3, 0) − 5(-3, 0) | 110364.354(0) | 82.8 | 138.45 | 66 | 52.2(0.4) | 5.3(0.7) | 373(48) |
| CH$_3$CN | 6(-3, 0) − 5(3, 0) | 110364.354(0) | 82.8 | 138.45 | blended | – | – | – |
| CH$_3$CN | 6(2, 0) − 5(2, 0) | 110374.989(0) | 47.1 | 164.06 | 93 | 52.2(0.2) | 4.6(0.5) | 453(45) |
| CH$_3$CN | 6(1, 0) − 5(1, 0) | 110381.372(0) | 25.7 | 179.45 | 195 | 52.2(0.2) | 4.3(0.3) | 898(73) |
| CH$_3$CN | 6(0, 0) − 5(0, 0) | 110383.500(0) | 18.5 | 184.58 | 244 | 52.1(0.1) | 5.1(0.3) | 1320(78) |
| CH$_3$OH, vt=0-2 | 7(2)$^+$ − 8(1)$^+$, vt=0 | 111289.453(13e-3) | 102.7 | 9.3425 | 13 | 52.1(2.3) | 6.3(4.2) | 87(61) |
| CH$_3$CHO | 6(1, 6) − 5(1, 5) A, vt=0 | 112248.716(3e-3) | 21.1 | 73.76807 | 48 | 52.0(1.1) | 2.6(1.1) | 133(18) |
| CH$_3$CHO | 6(1, 6) − 5(1, 5) E, vt=0 | 112254.508(3e-3) | 21.2 | 73.79585 | 52 | 52.0(1.1) | 1.5(1.1) | 86(18) |
| t-HCOOH | 5(2, 4) − 4(2, 3) | 112287.145 (3e-3) | 28.9 | 8.4851 | 25 | 52.8(1.1) | 9.4(1.1) | 253(18) |
| C$^{17}$O | 1 − 0 | 112359.284(1e-3) | 5.4 | 0.01217 | 855 | 52.2(0.1) | 4.7(0.1) | 4267(32) |
| CN | N= 1-0, J=1/2-1/2, F=1/2-1/2 | 113123.370(6e-3) | 5.4 | 0.15271 | 302 | 53.1(0.5) | 3.4(0.5) | 1082(105) |
| CN | N= 1-0, J=1/2-1/2, F=1/2-3/2 | 113144.157(6e-3) | 5.4 | 1.2492 | 829 | 53.1(0.5) | 4.4(0.5) | 3868(105) |
| CN | N= 1-0, J=1/2-1/2, F=3/2-1/2 | 113170.492(4e-3) | 5.4 | 1.2199 | 982 | 53.0(0.3) | 4.3(0.5) | 4459(105) |
| CN | N= 1-0, J=1/2-1/2, F=3/2-3/2 | 113191.279(3e-3) | 5.4 | 1.5836 | 878 | 53.0(0.5) | 4.7(0.5) | 4429(105) |
| CCS | 9(8) − 8(7) | 113410.186(2e-2) | 33.6 | 65.427 | 46 | 53.0(0.5) | 7.2(0.5) | 351(117) |
| CN | N= 1-0, J=3/2-1/2, F=3/2-1/2 | 113488.120(3e-3) | 5.4 | 1.5838 | 791 | 53.0(0.6) | 5.4(0.5) | 4511(117) |
| CN | N= 1-0, J=3/2-1/2, F=5/2-3/2 | 113490.970(2e-3) | 5.4 | 4.205 | 2133 | 53.0(0.5) | 2.7(0.5) | 6028(117) |
| CN | N= 1-0, J=3/2-1/2, F=1/2-1/2 | 113499.644(3e-3) | 5.4 | 1.2491 | 534 | 53.1(0.4) | 4.9(0.5) | 2802(117) |
| CN | N= 1-0, J=3/2-1/2, F=3/2-3/2 | 113508.907(3e-3) | 5.4 | 1.2196 | 728 | 53.0(0.5) | 4.4(0.5) | 3444(117) |
| CN | N= 1-0, J=3/2-1/2, F=1/2-3/2 | 113520.432(4e-3) | 5.4 | 0.15263 | 202 | 53.0(0.5) | 3.8(0.5) | 809(117) |
| | | | | G035.19−00.74 | | | | |
| NH$_2$CHO | 5(2, 4) − 4(2, 3) | 105972.665(37e-3) | 27.2 | 54.915 | 26 | 33.0(0.7) | 5.9(1.3) | 163(34) |
| CCS | 8(9) − 7(8) | 106347.726(2e-3) | 25.0 | 74.425 | 188 | 33.8(0.1) | 3.6(0.2) | 716(27) |
| HC$_5$N | 40 − 39 | 106498.910(7e-3) | 104.8 | 2249.7 | 65 | 34.3(0.2) | 3.4(0.4) | 236(25) |
| NH$_2$CHO | 5(2, 3) − 4(2, 2) | 106541.773(37e-3) | 27.2 | 54.915 | 21 | 33.2(0.9) | 7.0(1.5) | 159(36) |
| $^{34}$SO | 3(2) − 2(1) | 106743.244(7e-2) | 20.9 | 3.557 | 28 | 32.3(0.9) | 10.2(3.1) | 309(65) |
| CH$_3$OCH$_3$ | 9(1, 8) − 8(2, 7) EE | 106777.344(9e-3) | 43.4 | 58.573 | 20 | 32.5(1.4) | 11.4(2.0) | 246(99) |
| OC$^{34}$S | 9 − 8 | 106787.390(2e-3) | 25.6 | 4.601 | 27 | 32.5(0.7) | 5.1(1.5) | 148(40) |
| CH$_3$OH, vt=0-2 | 3(1)$^+$ − 4(0)$^+$, vt=0 | 107013.831(1e-2) | 28.3 | 12.036 | 1154 | 31.8(0.) | 4.4(0.1) | 5394(69) |
| CH$_3$OH, vt=0-2 | 15(-2) − 15(1) E2, vt=0 | 107159.906(14e-3) | 304.7 | 10.421 | 72 | 31.7(0.2) | 6.3(0.7) | 487(40) |
| CH$_3$OCHO | 9( 2, 8) − 8( 2, 7) E | 107537.258(1e-2) | 28.8 | 22.60702 | 31 | 33.1(0.6) | 5.5(0.9) | 184(33) |
| CH$_3$OCHO | 9( 2, 8) − 8( 2, 7) A | 107543.711(1e-2) | 28.8 | 22.61344 | 48 | 33.1(0.4) | 6.0(0.9) | 307(39) |
| SO$_2$ | 12(4, 8) − 13(3, 11) | 107843.470(2e-3) | 111.0 | 4.5354 | 22 | 31.7(1.1) | 8.9(2.2) | 207(46) |
| t-HCOOH | 5(1, 5) − 4(1, 4) | 108126.720(3e-3) | 18.8 | 9.6966 | 58 | 33.8(0.2) | 2.1(0.5) | 133(25) |
| $^{13}$CN | 1(1, 0) − 0(1, 1), F = 1 − 2 | 108426.889(5e-2) | 5.2 | 1.267 | 53 | 33.9(0.3) | 3.8(1.0) | 216(39) |
| $^{13}$CN | 1(1, 1) − 0(1, 0), F = 1 − 1 | 108636.923(5e-2) | 5.2 | 1.932 | 64 | 33.7(0.3) | 4.8(0.5) | 324(34) |
| $^{13}$CN | 1(2, 1) − 0(1, 1), F = 1 − 0 | 108638.212(5e-2) | 5.2 | 0.722 | blended | – | – | – |
| $^{13}$CN | 1(2, 1) − 0(1, 1), F = 2 − 1 | 108643.590(5e-2) | 5.2 | 0.856 | 51 | 33.8(0.3) | 4.3(0.8) | 232(35) |
| $^{13}$CN | 1(2, 1) − 0(1, 1), F = 0 − 1 | 108644.346(5e-2) | 5.2 | 0.642 | blended | – | – | – |
| $^{13}$CN | 1(2, 1) − 0(1, 1), F = 1 − 1 | 108645.064(5e-2) | 5.2 | 0.551 | blended | – | – | – |
| $^{13}$CN | 1(1, 1) − 0(1, 0), F = 2 − 1 | 108651.297(5e-2) | 5.2 | 3.276 | 102 | 33.9(0.1) | 3.6(0.3) | 387(31) |
| $^{13}$CN | 1(2, 1) − 0(1, 1), F = 2 − 2 | 108657.646(5e-2) | 5.2 | 2.420 | 74 | 33.7(0.2) | 4.6(0.5) | 360(36) |
| $^{13}$CN | 1(2, 1) − 0(1, 1), F = 1 − 2 | 108658.948(5e-2) | 5.2 | 0.669 | blended | – | – | – |
| $^{13}$CN | 1(2, 2) − 0(1, 1), F = 3 − 2 | 108780.201(5e-2) | 5.2 | 4.905 | 161 | 44.0(0.1) | 3.8(0.3) | 657(35) |
| $^{13}$CN | 1(2, 2) − 0(1, 1), F = 2 − 1 | 108782.374(5e-2) | 5.2 | 2.586 | 98 | 33.9(0.1) | 3.2(0.4) | 332(31) |
| $^{13}$CN | 1(2, 2) − 0(1, 1), F = 1 − 0 | 108786.982(5e-2) | 5.2 | 1.144 | 44 | 33.9(0.3) | 3.3(0.6) | 154(28) |
| $^{13}$CN | 1(2, 2) − 0(1, 1), F = 1 − 1 | 108793.753(5e-2) | 5.2 | 0.894 | 35 | 33.9(0.4) | 2.9(0.7) | 109(26) |
| $^{13}$CN | 1(2, 2) − 0(1, 1), F = 2 − 2 | 108796.400(5e-2) | 5.2 | 0.918 | 21 | 33.8(0.6) | 2.9(1.0) | 64(25) |
| CH$_3$OH, vt=0-2 | 0(0) − 1(-1) E2, vt=0 | 108893.945(12e-3) | 13.1 | 3.9134 | 678 | 31.7(0.) | 6.2(0.1) | 4509(42) |
| CH$_3$OH, vt=0-2 | 14(5) − 15(4) E1, vt=0 | 109138.783(15e-3) | 379.7 | 13.593 | 95 | 31.7(0.5) | 5.5(0.5) | 554(226) |
| CH$_3$OH, vt=0-2 | 16(-2) − 16(1) E2, vt=0 | 109153.184 (14e-3) | 342.0 | 14.726 | 86 | 31.8(0.5) | 6.0(0.5) | 549(226) |
| HC$_5$N | 41 − 40 | 109160.973(7e-3) | 110.0 | 2306 | 39 | 34.3(0.5) | 4.7(0.5) | 197(26) |
| HC$_3$N | 12 − 11 | 109173.634(1e-2) | 34.1 | 167.1 | 3544 | 34.0(0.5) | 4.2(0.5) | 15815(226) |
| SO | 3(2) − 2(1) | 109252.220(1e-1) | 21.1 | 3.5585 | 601 | 34.0(0.) | 5.8(0.1) | 3698(54) |
| OCS | 9 − 8 | 109463.063(5e-3) | 26.3 | 4.6034 | 351 | 33.7(0.1) | 6.4(0.2) | 2388(60) |
| C$^{18}$O | 1 − 0 | 109782.173(6e-3) | 5.3 | 0.01221 | 3604 | 34.0(0.1) | 3.5(0.1) | 13603(65) |
| HNCO | 5(2, 3) − 4(2, 2) | 109872.765(3e-2) | 186.1 | 10.013 | 45 | 33.5(0.3) | 1.6(0.9) | 75(36) |
| HNCO | 5(2, 4) − 4(2, 3) | 109872.337(3e-2) | 186.1 | 10.012 | blended | – | – | – |
| HNCO | 5(0, 5) − 4(0, 4) | 109905.749(7e-3) | 15.8 | 12.482 | 641 | 33.6(0.) | 4.2(0.1) | 2838(59) |
| C$^{15}$N | 1(2, 1) − 0(1, 0) | 110023.540(1e-1) | 5.3 | 1.386 | 22 | 34.3(0.3) | 0.5(0.1) | 12(10) |
| C$^{15}$N | 1(2, 2) − 0(1, 1) | 110024.590(1e-1) | 5.3 | 3.504 | 34 | 34.0(0.6) | 1.8(1.2) | 66(60) |
| $^{13}$CO | 1 − 0 | 110201.35(0) | 5.3 | 0.01220 | 14113 | 34.0(0.1) | 5.4(0.1) | 81157(1200) |
| HNCO | 5(1, 4) − 4(1, 3) | 110298.089(5e-3) | 59.2 | 11.847 | 28 | 33.5(0.5) | 3.4(0.5) | 101(71) |
| CH$_3$CN | 6(5, 0) − 5(5, 0) | 110330.345(0) | 197.1 | 56.399 | 22 | 33.2(0.8) | 2.6(0.5) | 62(41) |
| CH$_3$CN | 6(4, 0) − 5(4, 0) | 110349.471(0) | 132.8 | 102.482 | 58 | 33.2(0.5) | 5.8(0.5) | 355(71) |
| CH$_3$CN | 6(3, 0) − 5(-3, 0) | 110364.354(0) | 82.8 | 138.45 | 314 | 33.2(0.4) | 6.0(0.5) | 1996(71) |
| CH$_3$CN | 6(-3, 0) − 5(3, 0) | 110364.354(0) | 82.8 | 138.45 | blended | – | – | – |

**Table A2.** (Continued)

| Species | Transitions | Rest Freq. | $E_u$ | $\mu^2S$ | $T_{mb}$ | $V_{LSR}$ | $\Delta V$ | $\int T_{mb}\,dv$ |
|---|---|---|---|---|---|---|---|---|
| | | (MHz) | (K) | ($D^2$) | (mK) | (km $s^{-1}$) | (km $s^{-1}$) | (mK km $s^{-1}$) |
| $CH_3CN$ | 6(2, 0) − 5(2, 0) | 110374.989(0) | 47.1 | 164.06 | 342 | 33.2(0.5) | 5.5(0.5) | 2016(71) |
| $CH_3CN$ | 6(1, 0) − 5(1, 0) | 110381.372(0) | 25.7 | 179.45 | 561 | 33.2(0.6) | 4.3(0.5) | 2560(71) |
| $CH_3CN$ | 6(0, 0) − 5(0, 0) | 110383.500(0) | 18.5 | 184.58 | 742 | 33.2(0.5) | 6.2(0.5) | 4886(71) |
| $CH_3OCHO$ | 9(6, 3) − 8(6, 2) E | 110652.813(1e-2) | 50.5 | 13.30853 | 25 | 33.0(0.5) | 1.3(1.0) | 27(25) |
| $CH_3OCHO$ | 9(6, 4) − 8(6, 3) A | 110663.273(1e-2) | 50.4 | 13.31127 | 55 | 33.0(0.5) | 5.6(0.8) | 332(50) |
| $CH_3OCHO$ | 10(1,10) − 9(1, 9) E | 110788.664(1e-2) | 30.3 | 26.16584 | 21 | 33.0(1.2) | 2.6(1.9) | 57(55) |
| $CH_3OCHO$ | 10(1,10) − 9(1, 9) A | 110790.526(1e-2) | 30.3 | 26.17539 | 55 | 33.0(1.3) | 9.0(1.9) | 526(145) |
| $CH_3OCHO$ | 9(5, 4) − 8(5, 3) E | 110873.955(1e-2) | 43.2 | 16.55557 | 48 | 33.1(0.3) | 2.3(1.0) | 116(37) |
| $CH_3OCHO$ | 9(3, 7) − 8(3, 6) E | 110879.766(1e-2) | 32.6 | 21.245 | 43 | 33.1(0.4) | 1.6(0.8) | 71(44) |
| $CH_3OCHO$ | 9(5, 5) − 8(5, 4) A | 110880.447(1e-2) | 43.2 | 16.56015 | 57 | 33.0(0.7) | 6.9(1.3) | 423(78) |
| $CH_3OCHO$ | 9(3, 7) − 8(3, 6) A | 110887.092(1e-2) | 32.6 | 21.25577 | 44 | 33.0(0.5) | 5.3(1.3) | 247(50) |
| $CH_3OCHO$ | 9(5, 4) − 8(5, 3) A | 110890.256(1e-2) | 43.2 | 16.56106 | 13 | 33.0(1.5) | 4.1(2.1) | 59(41) |
| $CH_3OCHO$ | 10(0, 10) − 9(0, 9) E | 111169.903(1e-2) | 30.2 | 26.18776 | 53 | 33.2(0.5) | 2.8(0.5) | 159(13) |
| $CH_3OCHO$ | 10(0, 10) − 9(0, 9) A | 111171.634(1e-2) | 30.2 | 26.19136 | 68 | 33.1(0.5) | 5.9(0.5) | 422(13) |
| $CH_3OCHO$ | 9(4, 6) − 8(4, 5) A | 111195.962(1e-2) | 37.2 | 19.21722 | 64 | 33.2(0.5) | 5.3(0.5) | 359(13) |
| $CH_3OCHO$ | 9(4, 6) − 8(4, 5) E | 111223.491(1e-2) | 37.2 | 18.18412 | 51 | 33.1(0.5) | 3.7(0.5) | 203(33) |
| $CH_3OH$, vt=0-2 | 7(2)$^+$ − 8(1)$^+$, vt=0 | 111289.453(13e-3) | 102.7 | 9.3425 | 248 | 31.8(0.3) | 5.6(0.2) | 1484(51) |
| $CH_3OCHO$ | 9(4, 5) − 8(4, 4) A | 111453.300(1e-2) | 37.2 | 19.21778 | 45 | 33.0(0.) | 5.2(0.8) | 249(44) |
| $CH_3OH$, vt=0-2 | 17(-2) − 17(1) E2, vt=0 | 111626.514(15e-3) | 381.5 | 20.231 | 79 | 31.7(0.5) | 6.3(0.5) | 526(13) |
| $CH_3OCHO$ | 9(1, 8) − 8(1, 7) E | 111674.131(1e-2) | 28.1 | 23.18984 | 35 | 33.0(0.5) | 6.5(0.5) | 462(13) |
| $CH_3OCHO$ | 9(1, 8) − 8(1, 7) A | 111682.189(1e-2) | 28.1 | 23.19587 | 42 | 33.0(0.5) | 3.8(0.5) | 171(13) |
| $CH_3OCHO$ | 10(1, 10) − 9(0, 9) A | 111735.307(1e-2) | 30.3 | 3.84224 | 20 | 33.1(2.5) | 14.1(7.0) | 295(103) |
| $CH_3OCH_3$ | 19(3, 16) − 19(2, 17) AA | 111744.238(29e-3) | 187.5 | 259.8 | 40 | 31.6(1.0) | 11.0(1.6) | 467(71) |
| $CH_3OCH_3$ | 7(0, 7) − 6(1, 6) AA | 111782.562(8e-3) | 25.2 | 68.047 | 60 | 31.6(0.3) | 7.6(0.8) | 736(64) |
| $CH_3CHO$ | 6(1, 6) − 5(1, 5) A, vt=0 | 112248.716(3e-3) | 21.1 | 73.76807 | 215 | 33.3(0.1) | 3.7(0.2) | 858(48) |
| $CH_3CHO$ | 6(1, 6) − 5(1, 5) E, vt=0 | 112254.508(3e-3) | 21.2 | 73.79585 | 220 | 33.2(0.1) | 3.8(0.3) | 901(50) |
| $C^{17}O$ | 1 − 0 | 112359.284(1e-3) | 5.4 | 0.01217 | 787 | 33.8(0.1) | 5.5(0.1) | 4570(59) |
| CN | N= 1-0, J=1/2-1/2, F=1/2-1/2 | 113123.370(6e-3) | 5.4 | 0.15271 | 697 | 33.5(0.5) | 4.9(0.5) | 2873(153) |
| CN | N= 1-0, J=1/2-1/2, F=1/2-3/2 | 113144.157(6e-3) | 5.4 | 1.2492 | 1013 | 33.5(0.4) | 7.3(0.5) | 7877(153) |
| CN | N= 1-0, J=1/2-1/2, F=3/2-1/2 | 113170.492(4e-3) | 5.4 | 1.2199 | 1271 | 33.5(0.5) | 6.9(0.5) | 9314(153) |
| CN | N= 1-0, J=1/2-1/2, F=3/2-3/2 | 113191.279(3e-3) | 5.4 | 1.5836 | 1006 | 33.5(0.3) | 8.3(0.5) | 8910(153) |
| CCS | 9(8) − 8(7) | 113410.186(2e-2) | 33.6 | 65.427 | 82 | 33.5(0.5) | 3.1(0.5) | 271(189) |
| CN | N= 1-0, J=3/2-1/2, F=3/2-1/2 | 113488.120(3e-3) | 5.4 | 1.5838 | 1428 | 33.3(0.5) | 12.7(0.5) | 19325(189) |
| CN | N= 1-0, J=3/2-1/2, F=5/2-3/2 | 113490.970(2e-3) | 5.4 | 4.205 | 1707 | 33.5(0.5) | 1.8(0.5) | 3341(189) |
| CN | N= 1-0, J=3/2-1/2, F=1/2-1/2 | 113499.644(3e-3) | 5.4 | 1.2491 | 652 | 33.5(0.7) | 7.3(0.5) | 5081(189) |
| CN | N= 1-0, J=3/2-1/2, F=3/2-3/2 | 113508.907(3e-3) | 5.4 | 1.2196 | 928 | 33.4(0.5) | 6.7(0.5) | 6654(189) |
| CN | N= 1-0, J=3/2-1/2, F=1/2-3/2 | 113520.432(4e-3) | 5.4 | 0.15263 | 249 | 33.5(0.8) | 6.3(0.5) | 1668(189) |
| | | | | G035.20−01.73 | | | | |
| CCS | 8(9) − 7(8) | 106347.726(2e-2) | 25.0 | 74.425 | 73 | 43.5(0.2) | 5.5(0.5) | 427(34) |
| Hα | H (39) α | 106737.357(0) | − | − | 140 | 47.1(0.3) | 25.2(0.6) | 3753(82) |
| $CH_3OH$, vt=0-2 | 3(1)$^+$ − 4(0)$^+$, vt=0 | 107013.831(1e-2) | 28.3 | 12.036 | 68 | 43.0(0.4) | 3.3(0.8) | 237(52) |
| t-HCOOH | 5(1, 5) − 4(1, 4) | 108126.720(3e-3) | 18.8 | 9.6966 | 17 | 43.3(0.6) | 2.1(1.7) | 30(21) |
| $^{13}CN$ | 1(1, 1) − 0(1, 0), F = 1 − 1 | 108636.923(5e-2) | 5.2 | 1.932 | 24 | 43.5(0.7) | 6.6(1.6) | 172(34) |
| $^{13}CN$ | 1(2, 1) − 0(1, 1), F = 1 − 0 | 108638.212(5e-2) | 5.2 | 0.722 | blended | − | − | − |
| $^{13}CN$ | 1(2, 1) − 0(1, 1), F = 2 − 1 | 108643.590(5e-2) | 5.2 | 0.856 | 17 | 43.4(0.9) | 6.5(1.7) | 120(32) |
| $^{13}CN$ | 1(2, 1) − 0(1, 1), F = 0 − 1 | 108644.346(5e-2) | 5.2 | 0.642 | blended | − | − | − |
| $^{13}CN$ | 1(2, 1) − 0(1, 1), F = 1 − 1 | 108645.064(5e-2) | 5.2 | 0.551 | blended | − | − | − |
| $^{13}CN$ | 1(1, 1) − 0(1, 0), F = 2 − 1 | 108651.297(5e-2) | 5.2 | 3.276 | 46 | 43.5(0.3) | 4.0(0.6) | 199(26) |
| $^{13}CN$ | 1(2, 1) − 0(1, 1), F = 2 − 2 | 108657.646(5e-2) | 5.2 | 2.420 | 36 | 43.1(0.4) | 5.6(0.9) | 216(31) |
| $^{13}CN$ | 1(2, 1) − 0(1, 1), F = 1 − 2 | 108658.948(5e-2) | 5.2 | 0.669 | blended | − | − | − |
| $^{13}CN$ | 1(2, 2) − 0(1, 1), F = 3 − 2 | 108780.201(5e-2) | 5.2 | 4.905 | 70 | 43.5(0.1) | 4.2(0.5) | 311(28) |
| $^{13}CN$ | 1(2, 2) − 0(1, 1), F = 2 − 1 | 108782.374(5e-2) | 5.2 | 2.586 | 32 | 43.5(0.3) | 2.9(0.7) | 100(22) |
| $^{13}CN$ | 1(2, 2) − 0(1, 1), F = 1 − 0 | 108786.982(5e-2) | 5.2 | 1.144 | 17 | 43.3(1.0) | 5.0(1.6) | 91(29) |
| $^{13}CN$ | 1(2, 2) − 0(1, 1), F = 1 − 1 | 108793.753(5e-2) | 5.2 | 0.894 | 27 | 43.5(0.3) | 1.1(0.3) | 32(14) |
| $^{13}CN$ | 1(2, 2) − 0(1, 1), F = 2 − 2 | 108796.400(5e-2) | 5.2 | 0.918 | 80 | 43.5(1.5) | 2.5(1.80) | 21(20) |
| $CH_3OH$, vt=0-2 | 0(0) − 1(-1) E2, vt=0 | 108893.945(12e-3) | 13.1 | 3.9134 | 144 | 43.1(0.1) | 4.0(0.2) | 619(28) |
| $HC_3N$ | 12 − 11 | 109173.634(1e-2) | 34.1 | 167.1 | 830 | 43.4(0.) | 4.7(0.1) | 4187(27) |
| SO | 3(2) − 2(1) | 109252.220(1e-1) | 21.1 | 3.5585 | 422 | 43.3(0.1) | 5.6(0.1) | 2540(50) |
| OCS | 9 − 8 | 109463.063(5e-3) | 26.3 | 4.6034 | 135 | 43.5(0.1) | 4.2(0.2) | 599(25) |
| Hγ | H (55) γ | 109536.001(0) | − | − | 23 | 45.1(1.3) | 20.1(3.2) | 486(66) |
| $C^{18}O$ | 1 − 0 | 109782.173(6e-3) | 5.3 | 0.01221 | 1918 | 44.0(0.1) | 3.9(0.2) | 8060(431) |
| HNCO | 5(0, 5) − 4(0, 4) | 109905.749(7e-3) | 15.8 | 12.482 | 114 | 43.5(0.1) | 5.2(0.3) | 626(30) |
| $C^{15}N$ | 1(2, 1) − 0(1, 0) | 110023.540(1e-1) | 5.3 | 1.386 | 37 | 42.7(0.5) | 5.0(1.2) | 194(42) |
| $C^{15}N$ | 1(2, 2) − 0(1, 1) | 110024.590(1e-1) | 5.3 | 3.504 | 42 | 42.6(0.2) | 0.7(0.6) | 31(18) |
| $^{13}CO$ | 1 − 0 | 110201.35(0) | 5.3 | 0.01220 | 9104 | 44.0(0.2) | 2.8(0.4) | 26753(4410) |
| HNCO | 5(1, 4) − 4(1, 3) | 110298.089(5e-3) | 59.2 | 11.847 | 28 | 43.4(0.4) | 2.4(1.3) | 70(29) |
| $CH_3CN$ | 6(4, 0) − 5(4, 0) | 110349.471(0) | 132.8 | 102.54 | 34 | 43.3(0.4) | 3.5(1.0) | 125(29) |
| $CH_3CN$ | 6(3, 0) − 5(-3, 0) | 110364.354(0) | 82.8 | 138.45 | 76 | 43.3(0.2) | 4.7(0.6) | 379(37) |
| $CH_3CN$ | 6(-3, 0) − 5(3, 0) | 110364.354(0) | 82.8 | 138.45 | blended | − | − | − |
| $CH_3CN$ | 6(2, 0) − 5(2, 0) | 110374.989(0) | 47.1 | 164.06 | 83 | 43.1(0.2) | 5.4(0.5) | 483(37) |
| $CH_3CN$ | 6(1, 0) − 5(1, 0) | 110381.372(0) | 25.7 | 179.45 | 148 | 43.1(0.2) | 5.2(0.5) | 811(60) |
| $CH_3CN$ | 6(0, 0) − 5(0, 0) | 110383.500(0) | 18.5 | 184.58 | 180 | 43.3(0.1) | 3.8(0.3) | 722(55) |
| $CH_3OH$, vt=0-2 | 7(2)$^+$ − 8(1)$^+$, vt=0 | 111289.453(13e-3) | 102.7 | 9.3425 | 41 | 43.0(0.6) | 1.6(1.2) | 71(40) |
| Hβ | H (48) β | 111885.070(0) | − | − | 31 | 47.9(1.2) | 16.8(2.8) | 563(81) |
| $CH_3CHO$ | 6(1, 6) − 5(1, 5) A, vt=0 | 112248.716(3e-3) | 21.1 | 73.76807 | 48 | 43.6(0.3) | 2.7(0.7) | 136(31) |
| $CH_3CHO$ | 6(1, 6) − 5(1, 5) E, vt=0 | 112254.508(3e-3) | 21.2 | 73.79585 | 53 | 43.5(0.3) | 2.8(0.7) | 160(33) |
| $C^{17}O$ | 1 − 0 | 112359.284(1e-3) | 5.4 | 0.01217 | 495 | 43.8(0.1) | 4.7(0.2) | 2487(99) |
| CN | N= 1-0, J=1/2-1/2, F=1/2-1/2 | 113123.370(6e-3) | 5.4 | 0.15271 | 1203 | 42.7(0.5) | 3.2(0.5) | 4089(132) |
| CN | N= 1-0, J=1/2-1/2, F=1/2-3/2 | 113144.157(6e-3) | 5.4 | 1.2492 | 980 | 42.7(0.5) | 5.2(0.5) | 5431(132) |
| CN | N= 1-0, J=1/2-1/2, F=3/2-1/2 | 113170.492(4e-3) | 5.4 | 1.2199 | 743 | 42.7(0.6) | 1.9(0.5) | 1482(132) |
| CN | N= 1-0, J=1/2-1/2, F=3/2-3/2 | 113191.279(3e-3) | 5.4 | 1.5836 | 997 | 42.7(0.5) | 5.4(0.5) | 5751(132) |
| CN | N= 1-0, J=3/2-1/2, F=3/2-1/2 | 113488.120(3e-3) | 5.4 | 1.5838 | 930 | 42.7(0.5) | 5.7(0.5) | 5648(206) |
| CN | N= 1-0, J=3/2-1/2, F=5/2-3/2 | 113490.970(2e-3) | 5.4 | 4.205 | 1982 | 42.7(0.4) | 2.8(0.5) | 5864(206) |
| CN | N= 1-0, J=3/2-1/2, F=1/2-1/2 | 113499.644(3e-3) | 5.4 | 1.2491 | 758 | 42.7(0.5) | 2.7(0.5) | 2183(206) |
| CN | N= 1-0, J=3/2-1/2, F=3/2-3/2 | 113508.907(3e-3) | 5.4 | 1.2196 | 912 | 42.7(0.7) | 3.0(0.5) | 2870(206) |
| CN | N= 1-0, J=3/2-1/2, F=1/2-3/2 | 113520.432(4e-3) | 5.4 | 0.15263 | 192 | 42.7(0.5) | 4.0(0.5) | 802(206) |
| | | | | G037.43+01.51 | | | | |
| CCS | 8(9) − 7(8) | 106347.726(2e-2) | 25.0 | 74.425 | 85 | 43.3(0.1) | 3.0(0.4) | 276(26) |
| $HC_5N$ | 40 − 39 | 106498.910(7e-3) | 104.8 | 2249.7 | 27 | 44.0(0.5) | 5.5(1.4) | 157(31) |
| $^{34}SO$ | 3(2) − 2(1) | 106743.244(7e-2) | 20.9 | 3.557 | 40 | 43.7(0.2) | 3.2(0.6) | 135(20) |
| $CH_3OH$, vt=0-2 | 3(1)$^+$ − 4(0)$^+$, vt=0 | 107013.831(1e-2) | 28.3 | 12.036 | 209 | 43.0(0.) | 5.0(0.1) | 1105(22) |
| $CH_3OH$, vt=0-2 | 15(-2) − 15(1) E2, vt=0 | 107159.906(14e-3) | 304.7 | 0.017814 | 42 | 43.1(0.3) | 4.6(0.5) | 205(23) |
| $CH_3OCHO$ | 9( 2, 8) − 8( 2, 7) E | 107537.258(1e-2) | 28.8 | 22.60702 | 20 | 44.3(0.6) | 7.1(1.2) | 149(24) |
| $CH_3OCHO$ | 9( 2, 8) − 8( 2, 7) A | 107543.711(1e-2) | 28.8 | 22.61344 | 26 | 44.2(0.3) | 2.9(0.7) | 79(16) |
| $SO_2$ | 12(4, 8) − 13(3, 11) | 107843.470(2e-3) | 111.0 | 4.5354 | 19 | 43.5(0.7) | 5.4(1.6) | 111(28) |
| t-HCOOH | 5(1, 5) − 4(1, 4) | 108126.720(3e-3) | 18.8 | 9.6966 | 35 | 44.1(0.3) | 3.1(0.6) | 117(20) |

**Table A2.** (Continued)

| Species | Transitions | Rest Freq. (MHz) | $E_u$ (K) | $\mu^2S$ ($D^2$) | $T_{mb}$ (mK) | $V_{LSR}$ (km $s^{-1}$) | $\Delta V$ (km $s^{-1}$) | $\int T_{mb}\,dv$ (mK km $s^{-1}$) |
|---|---|---|---|---|---|---|---|---|
| $^{13}CN$ | 1(1, 0) − 0(1, 1), F = 1 − 2 | 108426.889(5e-2) | 5.2 | 1.267 | 26 | 43.6(0.3) | 2.6(0.7) | 73(17) |
| $^{13}CN$ | 1(1, 1) − 0(1, 0), F = 0 − 1 | 108631.121(5e-2) | 5.2 | 0.642 | 38 | 43.9(0.1) | 0.5(0.1) | 22(9) |
| $^{13}CN$ | 1(1, 1) − 0(1, 0), F = 1 − 1 | 108636.923(5e-2) | 5.2 | 1.932 | 17 | 43.7(0.4) | 0.8(0.6) | 15(12) |
| $^{13}CN$ | 1(2, 1) − 0(1, 1), F = 1 − 0 | 108638.212(5e-2) | 5.2 | 0.722 | 18 | 43.6(0.9) | 4.0(1.4) | 77(33) |
| $^{13}CN$ | 1(2, 1) − 0(1, 1), F = 2 − 1 | 108643.590(5e-2) | 5.2 | 0.856 | 22 | 43.6(0.5) | 2.8(0.8) | 66(20) |
| $^{13}CN$ | 1(2, 1) − 0(1, 1), F = 0 − 1 | 108644.346(5e-2) | 5.2 | 0.642 | 25 | 43.9(0.4) | 2.3(1.1) | 62(23) |
| $^{13}CN$ | 1(2, 1) − 0(1, 1), F = 1 − 1 | 108645.064(5e-2) | 5.2 | 0.551 | blended | − | − | − |
| $^{13}CN$ | 1(1, 1) − 0(1, 0), F = 2 − 1 | 108651.297(5e-2) | 5.2 | 3.276 | 48 | 43.6(0.2) | 3.1(0.5) | 156(20) |
| $^{13}CN$ | 1(2, 1) − 0(1, 1), F = 2 − 2 | 108657.646(5e-2) | 5.2 | 2.420 | 38 | 43.7(0.3) | 2.6(1.0) | 108(30) |
| $^{13}CN$ | 1(2, 1) − 0(1, 1), F = 1 − 2 | 108658.948(5e-2) | 5.2 | 0.669 | 11 | 43.6(1.2) | 3.8(2.5) | 46(29) |
| $^{13}CN$ | 1(2, 2) − 0(1, 1), F = 3 − 2 | 108780.201(5e-2) | 5.2 | 4.905 | 75 | 43.5(0.1) | 3.0(0.3) | 243(18) |
| $^{13}CN$ | 1(2, 2) − 0(1, 1), F = 2 − 1 | 108782.374(5e-2) | 5.2 | 2.586 | 25 | 43.6(0.4) | 4.8(0.9) | 129(23) |
| $^{13}CN$ | 1(2, 2) − 0(1, 1), F = 1 − 0 | 108786.982(5e-2) | 5.2 | 1.144 | 18 | 43.6(0.4) | 2.3(1.1) | 45(17) |
| $^{13}CN$ | 1(2, 2) − 0(1, 1), F = 1 − 1 | 108793.753(5e-2) | 5.2 | 0.894 | 12 | 43.6(0.7) | 2.0(1.1) | 26(15) |
| $^{13}CN$ | 1(2, 2) − 0(1, 1), F = 2 − 2 | 108796.400(5e-2) | 5.2 | 0.918 | 12 | 43.6(0.8) | 4.4(2.7) | 56(25) |
| $CH_3OH$, vt=0-2 | 0(0) − 1(-1) E2, vt=0 | 108893.945(12e-3) | 13.1 | 3.9134 | 606 | 43.2(0.) | 3.6(0.1) | 2345(23) |
| $CH_3OH$, vt=0-2 | 14(5) − 15(4) E1, vt=0 | 109138.783(15e-3) | 379.7 | 13.593 | 49 | 43.1(1.1) | 7.6(1.1) | 399(200) |
| $CH_3OH$, vt=0-2 | 16(-2) − 16(1) E2, vt=0 | 109153.184(14e-3) | 342.0 | 14.726 | 59 | 43.1(1.1) | 5.9(1.1) | 368(200) |
| $HC_5N$ | 41 − 40 | 109160.973(7e-3) | 110.0 | 2306 | 27 | 44.3(0.1) | 5.2(1.1) | 150(200) |
| $HC_3N$ | 12 − 11 | 109173.634(1e-3) | 34.1 | 167.1 | 1622 | 44.3(0.2) | 2.9(1.1) | 5058(200) |
| SO | 3(2) − 2(1) | 109252.220(1e-1) | 21.1 | 3.5585 | 770 | 44.0(0.) | 3.3(0.1) | 2700(32) |
| OCS | 9 − 8 | 109463.063(5e-3) | 26.3 | 4.6034 | 238 | 44.2(0.1) | 3.9(0.2) | 982(36) |
| HNCO | 5(1, 5) − 4(1, 4) | 109495.996(6e-3) | 59.0 | 11.847 | 39 | 43.5(0.6) | 9.2(1.9) | 385(60) |
| $C^{18}O$ | 1 − 0 | 109782.173(6e-3) | 5.3 | 0.01221 | 3751 | 44.0(0.1) | 2.6(0.1) | 10269(12) |
| HNCO | 5(0, 5) − 4(0, 4) | 109905.749(7e-3) | 15.8 | 12.482 | 437 | 43.4(0.) | 2.8(0.1) | 1322(37) |
| $C^{15}N$ | 1(2, 1) − 0(1, 0) | 110023.540(1e-1) | 5.3 | 1.386 | 38 | 43.5(0.3) | 2.1(0.7) | 85(24) |
| $C^{15}N$ | 1(2, 2) − 0(1, 1) | 110024.590(1e-1) | 5.3 | 3.504 | 66 | 43.5(0.1) | 1.1(0.3) | 80(20) |
| $^{13}CO$ | 1 − 0 | 110201.35(0) | 5.3 | 0.01220 | 22204 | 44.0(0.5) | 3.2(0.5) | 75998(2220) |
| HNCO | 5(1, 4) − 4(1, 3) | 110298.089(5e-3) | 59.2 | 11.847 | 35 | 43.5(0.5) | 6.8(1.5) | 253(42) |
| $CH_3CN$ | 6(5, 0) − 5(5, 0) | 110330.345(0) | 197.1 | 56.399 | 80 | 44.0(0.5) | 6.7(0.5) | 58(27) |
| $CH_3CN$ | 6(4, 0) − 5(4, 0) | 110349.471(0) | 132.8 | 102.54 | 30 | 44.1(0.5) | 6.9(0.5) | 225(27) |
| $CH_3CN$ | 6(3, 0) − 5(-3, 0) | 110364.354(0) | 82.8 | 138.45 | 105 | 44.0(0.4) | 4.8(0.5) | 539(27) |
| $CH_3CN$ | 6(-3, 0) − 5(3, 0) | 110364.354(0) | 82.8 | 138.45 | blended | − | − | − |
| $CH_3CN$ | 6(2, 0) − 5(2, 0) | 110374.989(0) | 47.1 | 164.06 | 129 | 44.0(0.5) | 4.2(0.5) | 580(27) |
| $CH_3CN$ | 6(1, 0) − 5(1, 0) | 110381.372(0) | 25.7 | 179.45 | 257 | 44.2(0.3) | 3.6(0.5) | 979(27) |
| $CH_3CN$ | 6(0, 0) − 5(0, 0) | 110383.500(0) | 18.5 | 184.58 | 293 | 44.1(0.7) | 3.5(0.5) | 1078(27) |
| $CH_3OCHO$ | 9(5, 4) − 8(5, 3) E | 110873.955(1e-2) | 43.2 | 16.55557 | 26 | 44.5(0.3) | 2.8(1.1) | 30(25) |
| $CH_3OCHO$ | 9(5, 5) − 8(5, 4) A | 110880.447(1e-2) | 43.2 | 16.56015 | 29 | 44.5(1.1) | 4.6(2.0) | 144(55) |
| $CH_3OCHO$ | 9(5, 5) − 8(5, 4) E | 110882.331(1e-2) | 43.2 | 16.55225 | 23 | 44.4(1.5) | 7.6(2.9) | 185(61) |
| $CH_3OCHO$ | 9(3, 7) − 8(3, 6) A | 110887.092(1e-2) | 32.6 | 21.25577 | 22 | 44.4(0.9) | 3.5(1.8) | 81(45) |
| $CH_3OCHO$ | 10(0, 10) − 9(0, 9) E | 111169.903(1e-2) | 30.2 | 26.18776 | 20 | 44.4(1.1) | 6.0(1.1) | 126(11) |
| $CH_3OCHO$ | 10(0, 10) − 9(0, 9) A | 111171.634(1e-2) | 30.2 | 26.19136 | 97 | 44.5(1.1) | 8.0(1.8) | 82(11) |
| $CH_3OCHO$ | 9(4, 6) − 8(4, 5) A | 111195.962(1e-2) | 37.2 | 19.21722 | 11 | 44.6(1.1) | 5.9(1.1) | 69(11) |
| $CH_3OCHO$ | 9(4, 6) − 8(4, 5) E | 111223.491(1e-2) | 37.2 | 18.18412 | 17 | 44.5(1.1) | 3.1(1.3) | 57(25) |
| $CH_3OH$, vt=0-2 | $7(2)^{+}$ − $8(1)^{+}$, vt=0 | 111.289.453(13e-3) | 102.7 | 9.3425 | 128 | 43.2(0.8) | 6.4(0.4) | 873(39) |
| $CH_3OCHO$ | 9(4, 5) − 8(4, 4) A | 111453.300(1e-2) | 37.2 | 19.21778 | 86 | 44.5(1.4) | 3.9(2.8) | 36(24) |
| $CH_3OH$, vt=0-2 | 17(-2) − 17(1) E2, vt=0 | 111626.514(15e-3) | 381.5 | 20.231 | 56 | 43.3(0.3) | 6.0(0.8) | 362(38) |
| $CH_3OCHO$ | 9(1, 8) − 8(1, 7) E | 111674.131(1e-2) | 28.1 | 23.18984 | 29 | 44.5(0.6) | 5.6(1.1) | 173(34) |
| $CH_3OCHO$ | 9(1, 8) − 8(1, 7) A | 111682.189(1e-2) | 28.1 | 23.19587 | 18 | 44.4(1.4) | 7.3(2.6) | 140(43) |
| t-HCOOH | 5(0, 5) − 4(0, 4) | 111746.784(3e-3) | 16.1 | 259.8 | 42 | 44.0(0.3) | 4.5(1.3) | 204(41) |
| $CH_3OCH_3$ | 7(0, 7) − 6(1, 6) AA | 111782.562(8e-3) | 25.2 | 68.047 | 44 | 44.2(0.4) | 6.5(1.1) | 307(41) |
| $CH_3OCH_3$ | 18(3, 15) − 18(2, 16) EE | 111813.668(21e-3) | 115.4 | 386.29 | 24 | 44.1(0.4) | 2.0(0.9) | 51(21) |
| $CH_3CHO$ | 6(1, 6) − 5(1, 5) A, vt=0 | 112248.716(3e-3) | 21.1 | 73.76807 | 75 | 44.0(0.2) | 2.7(0.3) | 213(26) |
| $CH_3CHO$ | 6(1, 6) − 5(1, 5) E, vt=0 | 112254.508(3e-3) | 21.2 | 73.79585 | 67 | 44.0(0.2) | 3.1(0.5) | 220(30) |
| t-HCOOH | 5(2, 4) − 4(2, 3) | 112287.145 (3e-3) | 28.9 | 8.4851 | 32 | 44.2(1.1) | 3.4(1.1) | 116(26) |
| $C^{17}O$ | 1 − 0 | 112359.284(1e-3) | 5.4 | 0.01217 | 735 | 44.0(0.1) | 5.0(0.1) | 3904(56) |
| t-HCOOH | 5(2, 3) − 4(2, 2) | 112891.443 (3e-3) | 28.9 | 8.4849 | 31 | 44.1(0.6) | 7.2(1.8) | 236(47) |
| CN | N= 1-0, J=1/2-1/2, F=1/2-1/2 | 113123.370(6e-3) | 5.4 | 0.15271 | 304 | 44.1(0.5) | 2.7(0.5) | 884(142) |
| CN | N= 1-0, J=1/2-1/2, F=1/2-3/2 | 113144.157(6e-3) | 5.4 | 1.2492 | 1375 | 44.0(0.6) | 3.2(0.5) | 466(142) |
| CN | N= 1-0, J=1/2-1/2, F=3/2-1/2 | 113170.492(4e-3) | 5.4 | 1.2199 | 1496 | 44.1(0.5) | 3.3(0.5) | 5260(142) |
| CN | N= 1-0, J=1/2-1/2, F=3/2-3/2 | 113191.279(3e-3) | 5.4 | 1.5836 | 1528 | 44.1(0.4) | 3.4(0.5) | 5493(142) |
| CN | N= 1-0, J=3/2-1/2, F=3/2-1/2 | 113488.120(3e-3) | 5.4 | 1.5838 | 1319 | 44.0(0.5) | 3.3(0.5) | 4640(178) |
| CN | N= 1-0, J=3/2-1/2, F=5/2-3/2 | 113490.970(2e-3) | 5.4 | 4.205 | 3045 | 44.1(0.5) | 3.6(0.5) | 11596(178) |
| CN | N= 1-0, J=3/2-1/2, F=1/2-1/2 | 113499.644(3e-3) | 5.4 | 1.2491 | 974 | 44.1(0.4) | 3.0(0.5) | 3126(178) |
| CN | N= 1-0, J=3/2-1/2, F=3/2-3/2 | 113508.907(3e-3) | 5.4 | 1.2196 | 1161 | 44.1(0.5) | 3.0(0.5) | 3767(178) |
| CN | N= 1-0, J=3/2-1/2, F=1/2-3/2 | 113520.432(4e-3) | 5.4 | 0.15263 | 176 | 44.2(0.8) | 3.0(0.5) | 566(178) |
| | | G043.16+00.01 | | | | | | |
| $SO_2$, $v_2$=1 | 10(1, 9) − 10(0, 10) | 105956.755(0) | 799.9 | 17.803 | 43 | 10.0(0.7) | 8.4(1.4) | 379(59) |
| CCS | 8(9) − 7(8) | 106347.726(2e-2) | 25.0 | 74.425 | 66 | 8.1(0.6) | 17.2(1.9) | 1210(97) |
| H$\alpha$ | H (39) $\alpha$ | 106737.357(0) | − | − | 1316 | 8.2(0.1) | 36.2(0.2) | 50729(338) |
| $^{34}SO$ | 3(2) − 2(1) | 106743.244(7e-2) | 20.9 | 3.557 | 452 | 9.1(0.2) | 3.1(0.6) | 6288(0.5) |
| He$\alpha$ | He (39) $\alpha$ | 106780.852(0) | − | − | 118 | 8.1(0.9) | 28.4(2.1) | 3569(239) |
| $CH_3OH$, vt=0-2 | $3(1)^{+}$ − $4(0)^{+}$, vt=0 | 107013.831(1e-2) | 28.3 | 12.036 | 159 | 11.8(0.5) | 3.7(0.5) | 623(75) |
| $SO_2$ | 27(3, 25) − 26(4, 22) | 107060.208(2e-3) | 369.4 | 8.2723 | 511 | 11.0(0.5) | 12.3(0.5) | 6716(75) |
| $CH_3OH$, vt=0-2 | 15(-2) − 15(1) E2, vt=0 | 107159.906(14e-3) | 304.7 | 10.421 | 25 | 11.9(1.1) | 7.4(2.3) | 194(50) |
| H$\varepsilon$ | H (65) $\varepsilon$ | 107206.108(0) | − | − | 43 | 8.1(0.9) | 20.4(2.1) | 933(85) |
| $C_2H_5CN$ | 12(7, 5) − 11(7, 4) | 107485.160(5e-2) | 88.0 | 117.36 | 34 | 12.0(0.3) | 1.8(0.9) | 65(24) |
| $C_2H_5CN$ | 12(6, 6) − 11(6, 5) | 107486.949(5e-2) | 73.6 | 133.42 | 30 | 12.0(0.3) | 1.3(0.7) | 42(19) |
| $C_2H_5CN$ | 12(8, 4) − 11(8, 3) | 107491.574(5e-2) | 104.6 | 98.829 | 11 | 12.0(0.5) | 8.2(0.5) | 188(88) |
| $C_2H_5CN$ | 12(5, 7) − 11(5, 6) | 107502.432(5e-2) | 61.3 | 146.99 | 20 | 12.0(0.9) | 5.6(1.5) | 117(35) |
| $C_2H_5CN$ | 12(4, 9) − 11(4, 8) | 107544.042(5e-2) | 51.3 | 158.12 | 22 | 12.1(0.9) | 5.8(2.8) | 134(51) |
| $C_2H_5CN$ | 12(4, 8) − 11(4, 7) | 107547.460(5e-2) | 51.3 | 158.11 | 26 | 12.0(0.9) | 8.2(2.0) | 231(51) |
| $C_2H_5CN$ | 12(3, 10) − 11(3, 9) | 107594.056(5e-2) | 43.6 | 166.77 | 19 | 12.0(1.2) | 9.6(3.6) | 199(56) |
| $SO_2$ | 12(4, 8) − 13(3, 11) | 107843.470(2e-3) | 111.0 | 4.5354 | 793 | 11.0(0.) | 13.7(0.1) | 11546(67) |
| $^{33}SO$ | 3(2, 2) − 2(1, 1) | 107925.997(93e-3) | 21.0 | 1.187 | 41 | 9.5(0.6) | 15.6(1.4) | 675(52) |
| $^{33}SO$ | 3(2, 1) − 2(1, 1) | 107957.322(88e-3) | 21.0 | 1.187 | 55 | 9.5(0.5) | 15.9(1.0) | 925(52) |
| $^{33}SO$ | 3(2, 2) − 2(1, 2) | 107977.361(94e-3) | 21.0 | 1.518 | 11 | 9.3(2.3) | 16.3(4.6) | 196(52) |
| $^{33}SO$ | 3(2, 3) − 2(1, 3) | 108019.667(186e-3) | 21.0 | 1.280 | 49 | 9.5(5.2) | 9.0(3.9) | 47(33) |
| t-HCOOH | 5(1, 5) − 4(1, 4) | 108126.720(3e-3) | 18.8 | 9.6966 | 60 | 7.9(0.5) | 7.8(1.2) | 991(62) |
| $SO_2$ | 39(6, 34) − 38(7, 31) | 108955.915(2e-3) | 808.3 | 16.377 | 61 | 11.0(0.4) | 7.0(1.2) | 895(62) |
| $CH_3OH$, vt=0-2 | 14(5) − 15(4) E1, vt=0 | 109138.783(15e-3) | 379.7 | 13.593 | 26 | 12.0(1.1) | 9.5(1.1) | 260(23) |
| $CH_3OH$, vt=0-2 | 16(-2) − 16(1) E2, vt=0 | 109153.184 (14e-3) | 342.0 | 14.726 | 18 | 12.0(1.1) | 5.7(1.1) | 210(23) |
| $HC_3N$ | 12 − 11 | 109173.634(1e-2) | 34.1 | 167.1 | 1346 | 10.1(1.1) | 7.4(1.1) | 10538(323) |
| SO | 3(2) − 2(1) | 109252.220(1e-1) | 21.1 | 3.5585 | 4488 | 7.9(0.) | 7.8(0.1) | 69561(156) |
| $HC_3N$, v7=1 | 12(-1) − 11(1) | 109442.013(2e-2) | 355.0 | 165.12 | 442 | 10.0(1.1) | 7.4(1.1) | 6934(119) |
| OCS | 9 − 8 | 109463.063(5e-3) | 26.3 | 4.6034 | 44 | 9.5(1.1) | 7.4(1.1) | 348(119) |
| HNCO | 5(1, 5) − 4(1, 4) | 109495.996(6e-3) | 59.0 | 23.947 | 126 | 10.0(1.1) | 10.7(1.1) | 1443(119) |
| H$\gamma$ | H (55) $\gamma$ | 109536.001(0) | − | − | 113 | 8.6(0.6) | 25.4(1.3) | 3042(149) |

**Table A2.** (Continued)

| Species | Transitions | Rest Freq. (MHz) | $E_u$ (K) | $\mu^2S$ ($D^2$) | $T_{mb}$ (mK) | $V_{LSR}$ (km $s^{-1}$) | $\Delta V$ (km $s^{-1}$) | $\int T_{mb}$ dv (mK km $s^{-1}$) |
|---|---|---|---|---|---|---|---|---|
| $HC_3N$, v7=1 | 12(1) − 11(-1) | 109598.818(2e-2) | 355.0 | 165.12 | 67 | 10.0(0.5) | 13.2(1.1) | 938(72) |
| $SO_2$ | 17(5, 13) − 18(4, 14) | 109757.585(2e-3) | 202.1 | 6.6069 | 592 | 11.0(0.2) | 14.2(0.5) | 8936(274) |
| $C^{18}O$ | 1 − 0 | 109782.173(6e-3) | 5.3 | 0.01221 | 2425 | 9.6(0.1) | 6.6(0.2) | 17000(651) |
| HNCO | 5(2, 3) − 4(2, 2) | 109872.765(3e-2) | 186.1 | 10.013 | 55 | 10.0(0.4) | 8.8(0.9) | 519(50) |
| HNCO | 5(2, 4) − 4(2, 3) | 109872.337(3e-2) | 186.1 | 10.012 | blended | – | – | – |
| HNCO | 5(0, 5) − 4(0, 4) | 109905.749(7e-3) | 15.8 | 12.482 | 410 | 10.0(0.1) | 13.7(0.2) | 5967(62) |
| $^{13}CO$ | 1 − 0 | 110201.35(0) | 5.3 | 0.01220 | 21121 | 9.7(0.1) | 9.5(0.2) | 215520(5020) |
| HNCO | 5(1, 4) − 4(1, 3) | 110298.089(5e-3) | 59.2 | 11.847 | 136 | 10.1(0.5) | 13.9(0.5) | 2016(72) |
| $CH_3CN$ | 6(4, 0) − 5(4, 0) | 110349.471(0) | 132.8 | 102.54 | 28 | 9.8(0.5) | 10.8(0.5) | 327(72) |
| $CH_3CN$ | 6(3, 0) − 5(-3, 0) | 110364.354(0) | 82.8 | 138.45 | 52 | 9.8(0.5) | 10.6(0.5) | 591(72) |
| $CH_3CN$ | 6(-3, 0) − 5(3, 0) | 110364.354(0) | 82.8 | 138.45 | blended | – | – | – |
| $CH_3CN$ | 6(2, 0) − 5(2, 0) | 110374.989(0) | 47.1 | 164.06 | 220 | 9.9(0.5) | 14.1(0.5) | 3307(72) |
| $CH_3CN$ | 6(1, 0) − 5(1, 0) | 110381.372(0) | 25.7 | 179.45 | 187 | 9.8(0.5) | 16.4(0.5) | 3259(72) |
| $CH_3CN$ | 6(0, 0) − 5(0, 0) | 110383.500(0) | 18.5 | 184.58 | 553 | 10.0(0.5) | 16.2(0.5) | 9545(72) |
| $CH_3OCHO$ | 10(1,10) − 9(1, 9) A | 110790.526(1e-2) | 30.3 | 26.294 | 30 | 10.0(1.0) | 14.1(1.8) | 451(61) |
| $CH_3OCHO$ | 10(0, 10) − 9(0, 9) E | 111169.903(1e-2) | 30.2 | 26.18773 | 38 | 10.1(1.5) | 18.9(4.5) | 895(130) |
| $CH_3OH$, vt=0-2 | $7(2)^+ - 8(1)^+$, vt=0 | 111289.453(13e-3) | 102.7 | 9.3425 | 143 | 12.0(0.4) | 16.5(0.9) | 2524(114) |
| $CH_3OH$, vt=0-2 | 15(2) − 14(5) E1, vt=1 | 111456.032(32e-3) | 677.6 | 0.079164 | 33 | 12.0(1.4) | 14.9(3.6) | 529(131) |
| t-HCOOH | 5(0, 5) − 4(0, 4) | 111746.784(3e-2) | 16.1 | 10.092 | 80 | 7.9(1.1) | 14.1(1.1) | 1195(59) |
| $SO_2$ | 31(3, 29) − 30(4, 26) | 111755.021(2e-3) | 476.9 | 6.4499 | 238 | 11.0(1.1) | 13.2(1.1) | 3350(59) |
| $CH_3OCH_3$ | 7(0, 7) − 6(1, 6) AA | 111782.562(8e-3) | 25.2 | 68.047 | 39 | 10.0(1.1) | 12.8(1.1) | 526(59) |
| H$\beta$ | H (48) $\beta$ | 111885.070(0) | – | – | 299 | 8.8(0.5) | 28.1(1.0) | 8958(294) |
| $CH_3CHO$ | 6(1, 6) − 5(1, 5) A, vt=0 | 112248.716(3e-3) | 21.1 | 73.76807 | 74 | 9.9(3.5) | 16.8(8.0) | 1317(881) |
| $CH_3CHO$ | 6(1, 6) − 5(1, 5) E, vt=0 | 112254.508(3e-3) | 21.2 | 73.79585 | 75 | 10.0(3.6) | 15.7(5.3) | 1256(833) |
| t-HCOOH | 5(2, 4) − 4(2, 3) | 112287.145 (3e-3) | 28.9 | 8.4851 | 37 | 8.0(1.2) | 11.8(2.9) | 466(91) |
| $C^{17}O$ | 1 − 0 | 112359.284(1e-3) | 5.4 | 0.01217 | 942 | 9.5(0.2) | 15.9(0.4) | 15918(370) |
| $C_2H_5CN$ | 13(1, 13) − 12(1, 12) | 112646.350(9e-2) | 39.0 | 191.45 | 17 | 12.1(3.7) | 15.7(11.2) | 285(147) |
| CN | N= 1-0, J=1/2-1/2, F=1/2-1/2 | 113123.370(6e-3) | 5.4 | 0.15271 | 244 | 6.3(1.2) | 3.6(2.9) | 932(511) |
| CN | N= 1-0, J=1/2-1/2, F=1/2-3/2 | 113144.157(6e-3) | 5.4 | 1.2492 | 871 | 6.1(0.5) | 6.6(1.0) | 11245(894) |
| CN | N= 1-0, J=1/2-1/2, F=3/2-1/2 | 113170.492(4e-3) | 5.4 | 1.2199 | 846 | 6.3(0.4) | 5.0(0.8) | 4511(683) |
| CN | N= 1-0, J=1/2-1/2, F=3/2-3/2 | 113191.279(3e-3) | 5.4 | 1.5836 | 1115 | 6.1(0.4) | 6.6(0.9) | 15565(944) |
| CN | N= 1-0, J=3/2-1/2, F=5/2-3/2 | 113490.970(2e-3) | 5.4 | 4.205 | 2977 | 6.1(0.2) | 11.8(0.3) | 37432(1250) |
| CN | N= 1-0, J=3/2-1/2, F=1/2-1/2 | 113499.644(3e-3) | 5.4 | 1.2491 | 622 | 6.1(0.1) | 9.6(1.9) | 6386(1200) |
| CN | N= 1-0, J=3/2-1/2, F=3/2-3/2 | 113508.907(3e-3) | 5.4 | 1.2196 | 756 | 6.1(0.1) | 12.8(1.9) | 10312(1090) |
| CN | N= 1-0, J=3/2-1/2, F=1/2-3/2 | 113520.432(4e-3) | 5.4 | 0.15263 | 98 | 6.2(0.6) | 15.6(10.5) | 1632(1680) |
| | | G043.79−00.12 | | | | | | |
| $NH_2CHO$ | 5(2, 4) − 4(2, 3) | 105972.665(37e-3) | 27.2 | 54.915 | 16 | 43.0(1.0) | 8.7(2.2) | 145(32) |
| $NH_2CHO$ | 5(3, 3) − 4(3, 2) | 106134.468(55e-3) | 42.1 | 41.845 | 19 | 43.0(0.4) | 2.5(1.1) | 50(18) |
| $NH_2CHO$ | 5(3, 2) − 4(3, 1) | 106141.442(55e-3) | 42.1 | 41.84 | 66 | 43.1(2.4) | 7.7(5.3) | 54(32) |
| CCS | 8(9) − 7(8) | 106347.726(2e-2) | 25.0 | 74.425 | 62 | 43.5(0.1) | 5.5(0.4) | 362(21) |
| $NH_2CHO$ | 5(2, 3) − 4(2, 2) | 106541.773(37e-3) | 27.2 | 54.915 | 17 | 43.0(0.5) | 2.8(1.3) | 53(18) |
| H$\alpha$ | H (39) $\alpha$ | 106737.357(0) | – | – | 21 | 65.9(1.7) | 43.7(4.1) | 996(82) |
| $^{34}SO$ | 3(2) − 2(1) | 106743.244(7e-2) | 20.9 | 3.557 | 43 | 43.0(0.3) | 6.2(0.8) | 282(32) |
| $OC^{34}S$ | 9 − 8 | 106787.390(2e-3) | 25.6 | 4.601 | 14 | 42.3(1.1) | 6.9(2.1) | 104(31) |
| $CH_3OH$, vt=0-2 | $3(1)^+ - 4(0)^+$, vt=0 | 107013.831(1e-2) | 28.3 | 12.036 | 203 | 43.3(0.1) | 6.1(0.2) | 1319(34) |
| $^{13}C^{17}O$ | 1(2) − 0(3) | 107288.550(5e-2) | 5.1 | 0.016 | 20 | 43.2(0.7) | 7.2(1.5) | 153(28) |
| $SO_2$ | 27(3, 25) − 26(4, 22) | 107060.208(2e-3) | 369.4 | 8.2723 | 29 | 43.5(0.6) | 6.4(1.2) | 196(35) |
| $CH_3OH$, vt=0-2 | 15(-2) − 15(1) E2, vt=0 | 107159.906(14e-3) | 304.7 | 10.421 | 20 | 43.5(0.2) | 1.9(0.5) | 80(21) |
| $CH_3OCHO$ | 9( 2, 8) − 8( 2, 7) E | 107537.258(1e-2) | 28.8 | 22.60702 | 13 | 43.2(1.5) | 12.9(3.5) | 177(37) |
| $CH_3OCHO$ | 9( 2, 8) − 8( 2, 7) A | 107543.711(1e-2) | 28.8 | 22.61344 | 21 | 43.3(0.5) | 4.5(0.9) | 103(20) |
| $C_2H_5CN$ | 12(3, 9) − 11(3, 8) | 107734.723(5e-2) | 43.6 | 166.76 | 14 | 40.1(0.8) | 5.4(1.4) | 800(21) |
| $SO_2$ | 12(4, 8) − 13(3, 11) | 107843.470(2e-3) | 111.0 | 4.5354 | 72 | 43.5(0.2) | 7.9(0.5) | 601(29) |
| t-HCOOH | 5(1, 5) − 4(1, 4) | 108126.720(3e-3) | 18.8 | 9.6966 | 26 | 43.6(0.5) | 5.4(1.0) | 149(26) |
| $^{13}CN$ | 1(1, 0) − 0(1, 1), F = 1 − 2 | 108426.889(5e-2) | 5.2 | 1.267 | 76 | 44.0(2.2) | 4.1(3.8) | 33(29) |
| $^{13}CN$ | 1(1, 1) − 0(1, 0), F = 1 − 1 | 108636.923(5e-2) | 5.2 | 1.932 | 22 | 43.4(0.5) | 4.8(1.0) | 112(22) |
| $^{13}CN$ | 1(2, 1) − 0(1, 1), F = 1 − 0 | 108638.212(5e-2) | 5.2 | 0.722 | blended | – | – | – |
| $^{13}CN$ | 1(2, 1) − 0(1, 1), F = 2 − 1 | 108643.590(5e-2) | 5.2 | 0.856 | 13 | 44.3(0.7) | 2.3(1.9) | 32(23) |
| $^{13}CN$ | 1(2, 1) − 0(1, 1), F = 0 − 1 | 108644.346(5e-2) | 5.2 | 0.642 | 10 | 44.4(2.1) | 4.4(3.5) | 43(25) |
| $^{13}CN$ | 1(2, 1) − 0(1, 1), F = 1 − 1 | 108645.064(5e-2) | 5.2 | 0.551 | blended | – | – | – |
| $^{13}CN$ | 1(1, 1) − 0(1, 0), F = 2 − 1 | 108651.297(5e-2) | 5.2 | 3.276 | 36 | 44.0(0.3) | 4.4(0.6) | 170(21) |
| $^{13}CN$ | 1(2, 1) − 0(1, 1), F = 2 − 2 | 108657.646(5e-2) | 5.2 | 2.420 | 18 | 43.8(0.6) | 6.1(1.3) | 117(25) |
| $^{13}CN$ | 1(2, 1) − 0(1, 1), F = 1 − 2 | 108658.948(5e-2) | 5.2 | 0.669 | blended | – | – | – |
| $^{13}CN$ | 1(2, 2) − 0(1, 1), F = 3 − 2 | 108780.201(5e-2) | 5.2 | 4.905 | 51 | 44.0(0.8) | 4.7(1.2) | 254(77) |
| $^{13}CN$ | 1(2, 2) − 0(1, 1), F = 2 − 1 | 108782.374(5e-2) | 5.2 | 2.586 | 26 | 44.1(1.3) | 3.9(2.1) | 111(76) |
| $^{13}CN$ | 1(2, 2) − 0(1, 1), F = 1 − 0 | 108786.982(5e-2) | 5.2 | 1.144 | 14 | 44.1(1.0) | 1.5(2.8) | 22(19) |
| $^{13}CN$ | 1(2, 2) − 0(1, 1), F = 1 − 1 | 108793.753(5e-2) | 5.2 | 0.894 | 59 | 44.0(2.1) | 3.1(2.5) | 21(19) |
| $^{13}CN$ | 1(2, 2) − 0(1, 1), F = 2 − 2 | 108796.400(5e-2) | 5.2 | 0.918 | 10 | 44.0(0.9) | 1.8(1.5) | 17(15) |
| $CH_3OH$, vt=0-2 | 0(0) − 1(-1) E2, vt=0 | 108893.945(12e-3) | 13.1 | 3.9134 | 583 | 43.5(0.) | 6.6(0.1) | 4098(38) |
| $CH_3OH$, vt=0-2 | 14(5) − 15(4) E1, vt=0 | 109138.783(15e-3) | 379.7 | 13.593 | 42 | 43.5(1.1) | 2.9(1.1) | 127(75) |
| $CH_3OH$, vt=0-2 | 16(-2) − 16(1) E2, vt=0 | 109153.184 (14e-3) | 342.0 | 14.726 | 42 | 43.5(1.1) | 1.8(1.1) | 78(75) |
| $HC_3N$ | 12 − 11 | 109173.634(1e-2) | 34.1 | 167.1 | 1287 | 44.0(0.1) | 5.3(1.1) | 7325(75) |
| SO | 3(2) − 2(1) | 109252.220(1e-1) | 21.1 | 3.5585 | 721 | 44.1(0.) | 6.5(0.1) | 4967(50) |
| $HC_3N$, $v_7$=1 | 12(-1) − 11(1) | 109442.013(2e-2) | 355.0 | 165.12 | 15 | 44.0(1.4) | 5.2(3.0) | 84(44) |
| OCS | 9 − 8 | 109463.063(5e-3) | 26.3 | 4.6034 | 283 | 43.5(0.1) | 6.1(0.2) | 1827(47) |
| HNCO | 5(1, 5) − 4(1, 4) | 109495.996(6e-3) | 59.0 | 11.847 | 283 | 44.0(0.9) | 4.0(1.7) | 88(36) |
| $HC_3N$, $v_7$=1 | 12(1) − 11(-1) | 109598.818(2e-2) | 355.0 | 165.12 | 81 | 44.0(2.9) | 5.1(3.4) | 44(42) |
| $SO_2$ | 17(5, 13) − 18(4, 14) | 109757.585(2e-3) | 202.1 | 6.6069 | 47 | 43.4(1.1) | 7.9(1.1) | 396(366) |
| $C^{18}O$ | 1 − 0 | 109782.173(6e-3) | 5.3 | 0.01221 | 2700 | 44.0(1.1) | 5.6(1.1) | 16055(366) |
| HNCO | 5(2, 3) − 4(2, 2) | 109872.765(3e-2) | 186.1 | 10.013 | 25 | 43.0(0.6) | 4.4(0.9) | 119(30) |
| HNCO | 5(2, 4) − 4(2, 3) | 109872.337(3e-2) | 186.1 | 10.012 | blended | – | – | – |
| HNCO | 5(0, 5) − 4(0, 4) | 109905.749(7e-3) | 15.8 | 12.482 | 356 | 43.0(0.1) | 6.9(0.1) | 2609(3) |
| $C^{15}N$ | 1(2, 1) − 0(1, 0) | 110023.540(1e-1) | 5.3 | 1.386 | blended | – | – | – |
| $C^{15}N$ | 1(2, 2) − 0(1, 1) | 110024.590(1e-1) | 5.3 | 3.504 | 28 | 44.2(0.6) | 8.1(1.3) | 241(35) |
| $^{13}CO$ | 1 − 0 | 110201.35(0) | 5.3 | 0.01220 | 15367 | 44.0(0.5) | 6.5(0.5) | 106870(1170) |
| HNCO | 5(1, 4) − 4(1, 3) | 110298.089(5e-3) | 59.2 | 11.847 | 46 | 43.0(0.2) | 2.2(0.5) | 105(21) |
| $CH_3CN$ | 6(4, 0) − 5(4, 0) | 110349.471(0) | 132.8 | 102.54 | 36 | 42.8(0.6) | 6.1(1.0) | 234(36) |
| $CH_3CN$ | 6(3, 0) − 5(-3, 0) | 110364.354(0) | 82.8 | 138.45 | 152 | 42.8(0.1) | 6.2(0.3) | 1003(37) |
| $CH_3CN$ | 6(-3, 0) − 5(3, 0) | 110364.354(0) | 82.8 | 138.45 | blended | – | – | – |
| $CH_3CN$ | 6(2, 0) − 5(2, 0) | 110374.989(0) | 47.1 | 164.06 | 152 | 42.8(0.1) | 6.7(0.3) | 1080(39) |
| $CH_3CN$ | 6(1, 0) − 5(1, 0) | 110381.372(0) | 25.7 | 179.45 | 251 | 42.8(0.4) | 6.4(0.5) | 1715(252) |
| $CH_3CN$ | 6(0, 0) − 5(0, 0) | 110383.500(0) | 18.5 | 184.58 | 284 | 42.7(0.3) | 6.4(0.4) | 1931(241) |
| $C_2H_5CN$ | 2(2, 0) − 1(0, 1) | 110654.431(2e-3) | 5.7 | 0.00237 | 13 | 40.0(1.1) | 2.0(0.9) | 51(20) |
| $CH_3OCHO$ | 10(0, 10) − 9(0, 9) E | 111169.903(1e-2) | 30.2 | 26.18776 | 27 | 43.2(0.5) | 3.7(1.2) | 106(31) |
| $CH_3OCHO$ | 10(0, 10) − 9(0, 9) A | 111171.634(1e-2) | 30.2 | 26.19136 | 31 | 43.2(0.3) | 1.1(0.9) | 38(18) |
| $CH_3OH$, vt=0-2 | $7(2)^+ - 8(1)^+$, vt=0 | 111289.453(13e-3) | 102.7 | 9.3425 | 112 | 43.4(0.1) | 4.2(0.3) | 497(29) |
| $CH_3OH$, vt=0-2 | 17(-2) − 17(1) E2, vt=0 | 111626.514(15e-3) | 381.5 | 20.231 | 54 | 43.5(0.2) | 2.5(0.4) | 144(22) |
| $CH_3OCHO$ | 9(1, 8) − 8(1, 7) E | 111674.131(1e-2) | 28.1 | 23.18984 | 19 | 43.3(0.9) | 5.7(1.4) | 113(32) |
| $CH_3OCHO$ | 9(1, 8) − 8(1, 7) A | 111682.189(1e-2) | 28.1 | 23.19587 | 16 | 43.3(1.0) | 5.7(1.7) | 95(31) |

**Table A2.** (Continued)

| Species | Transitions | Rest Freq. (MHz) | $E_u$ (K) | $\mu^2S$ ($D^2$) | $T_{mb}$ (mK) | $V_{LSR}$ (km $s^{-1}$) | $\Delta V$ (km $s^{-1}$) | $\int T_{mb}$ dv (mK km $s^{-1}$) |
|---|---|---|---|---|---|---|---|---|
| t-HCOOH | 5(0, 5) − 4(0, 4) | 111746.784(3e-3) | 16.1 | 10.092 | 39 | 43.5(0.5) | 8.3(1.3) | 343(44) |
| $CH_3OCH_3$ | 7(0, 7) − 6(1, 6) AA | 111782.562(8e-3) | 25.2 | 68.047 | 54 | 44.2(0.3) | 6.4(0.7) | 373(37) |
| $CH_3CHO$ | 6(1, 6) − 5(1, 5) A, vt=0 | 112248.716(3e-3) | 21.1 | 73.76807 | 62 | 43.5(0.3) | 6.1(0.6) | 404(36) |
| $CH_3CHO$ | 6(1, 6) − 5(1, 5) E, vt=0 | 112254.508(3e-3) | 21.2 | 73.79585 | 80 | 43.5(0.2) | 4.7(0.4) | 400(32) |
| t-HCOOH | 5(2, 4) − 4(2, 3) | 112287.145 (3e-3) | 28.9 | 8.4851 | 26 | 43.5(0.7) | 5.5(2.4) | 152(52) |
| $C^{17}O$ | 1 − 0 | 112359.284(1e-3) | 5.4 | 0.01217 | 751 | 44.2(0.1) | 7.1(0.1) | 5648(68) |
| CN | N= 1-0, J=1/2-1/2, F=1/2-1/2 | 113123.370(6e-3) | 5.4 | 0.15271 | 209 | 44.0(0.3) | 10.4(0.7) | 2316(128) |
| CN | N= 1-0, J=1/2-1/2, F=1/2-3/2 | 113144.157(6e-3) | 5.4 | 1.2492 | 822 | 44.0(0.) | 6.7(0.1) | 5838(97) |
| CN | N= 1-0, J=1/2-1/2, F=3/2-1/2 | 113170.492(4e-3) | 5.4 | 1.2199 | 986 | 44.1(0.) | 6.5(0.1) | 6831(95) |
| CN | N= 1-0, J=1/2-1/2, F=3/2-3/2 | 113191.279(3e-3) | 5.4 | 1.5836 | 916 | 44.0(0.) | 6.9(0.1) | 6683(98) |
| CCS | 9(8) − 8(7) | 113410.186(2e-2) | 33.6 | 65.427 | 58 | 43.5(1.1) | 10.8(1.1) | 673(39) |
| CN | N= 1-0, J=3/2-1/2, F=3/2-1/2 | 113488.120(3e-3) | 5.4 | 1.5838 | 652 | 44.0(1.1) | 5.6(1.1) | 3874(264) |
| CN | N= 1-0, J=3/2-1/2, F=5/2-3/2 | 113490.970(2e-3) | 5.4 | 4.205 | 1623 | 44.2(1.0) | 8.3(1.1) | 14269(264) |
| CN | N= 1-0, J=3/2-1/2, F=1/2-1/2 | 113499.644(3e-3) | 5.4 | 1.2491 | 488 | 44.0(1.1) | 7.7(1.1) | 3990(264) |
| CN | N= 1-0, J=3/2-1/2, F=3/2-3/2 | 113508.907(3e-3) | 5.4 | 1.2196 | 731 | 44.1(1.1) | 6.7(1.1) | 5188(264) |
| CN | N= 1-0, J=3/2-1/2, F=1/2-3/2 | 113520.432(4e-3) | 5.4 | 0.15263 | 129 | 44.0(1.0) | 9.3(1.1) | 1272(264) |
| | | G049.48−00.36 | | | | | | |
| $SO_2$, $v_2$=1 | 10(1, 9) − 10(0, 10) | 105956.755(0) | 17.803 | 205.6671 | 63 | 60.0(0.5) | 5.8(1.1) | 393(70) |
| $NH_2CHO$ | 5(2, 4) − 4(2, 3) | 105972.665(37e-3) | 27.2 | 54.915 | 181 | 59.1(0.2) | 7.8(0.5) | 1501(81) |
| $CH_3SH$, v=0-2 | 2(-1, 1) − 2(0, 1) A, vt=0 | 105998.367(1e-3) | 6.3 | 0.82 | 26 | 59.4(0.5) | 0.9(0.8) | 26(24) |
| $NH_2CHO$ | 5(4, 1) − 4(4, 0) | 106107.870(88e-3) | 63.0 | 23.537 | 127 | 59.0(0.2) | 6.4(0.4) | 868(57) |
| $NH_2CHO$ | 5(4, 2) − 4(4, 1) | 106107.845(88e-3) | 63.0 | 23.537 | blended | – | – | – |
| $NH_2CHO$ | 5(3, 3) − 4(3, 2) | 106134.468(55e-3) | 42.1 | 41.845 | 146 | 59.0(0.2) | 7.2(0.4) | 1126(62) |
| $NH_2CHO$ | 5(3, 2) − 4(3, 1) | 106141.442(55e-3) | 42.1 | 41.84 | 153 | 59.0(0.2) | 7.2(0.4) | 1169(63) |
| $CH_3COCH_3$ | 19(8, 12) − 19(7, 13) AE | 106156.273(24e-3) | 138.6 | 379.31359 | 37 | 59.3(0.7) | 5.1(1.5) | 201(53) |
| $CH_3COCH_3$ | 19(8, 12) − 19(7, 13) EA | 106156.370(26e-3) | 138.6 | 252.8703 | blended | – | – | – |
| $CH_3COCH_3$ | 19(7, 12) − 19(6, 13) EE | 106273.673(22e-3) | 138.6 | 1012.2419 | 58 | 59.3(0.5) | 6.9(1.0) | 423(56) |
| $CH_3COCH_3$ | 19(8, 12) − 19(7, 13) EE | 106274.499(22e-3) | 138.6 | 1012.22624 | blended | – | – | – |
| CCS | 8(9) − 7(8) | 106347.726(2e-2) | 25.0 | 74.425 | 58 | 61.5(0.4) | 4.7(0.8) | 293(47) |
| $CH_3COCH_3$ | 19(7, 12) − 19(6, 13) AA | 106390.849(26e-3) | 138.5 | 633.24693 | 31 | 59.3(0.7) | 4.8(1.7) | 160(50) |
| $CH_3COCH_3$ | 19(8, 12) − 19(7, 13) AA | 106391.693(26e-3) | 138.5 | 379.9848 | 92 | 59.2(2.7) | 5.6(3.1) | 55(45) |
| $HC_5N$ | 40 − 39 | 106498.910(7e-3) | 104.8 | 2249.7 | 19 | 64.6(3.5) | 12.7(9.4) | 260(132) |
| $NH_2CHO$ | 5(2, 3) − 4(2, 2) | 106541.773(37e-3) | 27.2 | 54.915 | 169 | 59.1(0.2) | 8.1(0.5) | 1461(83) |
| $C_2H_3CN$ | 11(1, 10) − 10(1, 9) | 106641.383(1e-3) | 32.9 | 476.24 | 40 | 61.0(0.4) | 5.1(0.8) | 220(35) |
| $C_2H_5OH$ | 13(1, 12) − 13(0, 13) | 106649.479(5e-2) | 79.4 | 10.463 | 84 | 60.3(0.2) | 7.2(0.5) | 642(43) |
| $C_2H_5OH$ | 6(1, 5) − 5(1, 4) | 106676.542(5e-2) | 76.1 | 9.325 | 76 | 60.0(0.3) | 5.6(0.8) | 894(55) |
| $C_2H_5OH$ | 69(3, 67) − 69(2, 67) | 106714.984(5e-2) | 2016.8 | 73.939 | 97 | 60.0(0.7) | 8.1(2.0) | 838(186) |
| Hα | H (39) α | 106737.357(0) | – | – | 1286 | 55.4(0.5) | 29.4(0.5) | 40170(210) |
| $C_2H_5OH$ | 47(5, 43) − 47(4, 43) | 106758.301(5e-2) | 1030.6 | 50.577 | 82 | 60.0(0.5) | 13.2(0.5) | 1141(61) |
| Heα | He (39) α | 106780.852(0) | – | – | 164 | 56.7(0.5) | 25.5(0.8) | 4537(51) |
| $CH_3COCH_3$ | 18(6, 12) − 18(5, 13) EE | 106873.162(18e-3) | 121.8 | 877.18596 | 50 | 59.3(0.7) | 9.4(1.5) | 503(69) |
| $CH_3COCH_3$ | 18(7, 12) − 18(6, 13) EE | 106873.359(18e-3) | 121.8 | 877.18275 | blended | – | – | – |
| $CH_3OH$, vt=0-2 | $3(1)^+ - 4(0)^+$, vt=0 | 107013.831(1e-2) | 28.3 | 12.036 | 1294 | 59.8(0.1) | 8.2(0.1) | 11319(145) |
| $C_2H_5CN$ | 12(2, 11) − 11(2, 10) | 107043.527(5e-2) | 37.9 | 172.86 | 155 | 60.0(0.5) | 12.1(0.5) | 2002(51) |
| $SO_2$ | 27(3, 25) − 26(4, 22) | 107060.208(2e-3) | 369.4 | 8.2723 | 295 | 60.0(0.5) | 10.1(0.5) | 3178(51) |
| $CH_3OH$, vt=0-2 | 15(-2) − 15(1) E2, vt=0 | 107159.906(14e-3) | 304.7 | 10.421 | 227 | 59.8(0.5) | 7.2(0.5) | 1730(23) |
| $^{13}CH_3CN$ | 6(3) − 5(3) | 107178.424(0) | 82.4 | 276.826 | 45 | 59.2(0.8) | 3.6(1.4) | 172(71) |
| $^{13}CH_3CN$ | 6(2) − 5(2) | 107188.500(1e-1) | 46.6 | 164.068 | 30 | 59.4(1.1) | 4.8(1.7) | 152(75) |
| $^{13}CH_3CN$ | 6(1) − 5(1) | 107194.550(1e-1) | 25.2 | 179.427 | 65 | 59.1(0.5) | 5.8(0.5) | 400(22) |
| $^{13}CH_3CN$ | 6(0) − 5(0) | 107196.570(1e-1) | 18.0 | 184.590 | 37 | 59.5(2.0) | 4.2(3.1) | 223(165) |
| Hε | H (65) ε | 107206.108(0) | – | – | 56 | 54.2(1.2) | 23.7(0.5) | 703(94) |
| $CH_3COCH_3$ | 11(9, 3) − 10(10, 0) AE | 107225.457(56e-3) | 57.6 | 1.5476 | 36 | 59.2(0.5) | 2.6(0.5) | 98(15) |
| $^{13}C^{17}O$ | 1(2) − 0(3) | 107288.550(5e-2) | 5.1 | 0.016 | 33 | 59.8(0.7) | 3.6(1.5) | 126(79) |
| $CH_3SH$, v=0-2 | 3(-1, 3) − 3(0, 3) A, vt=0 | 107316.441(1e-3) | 12.4 | 1.9002 | 46 | 59.3(0.5) | 13.4(0.5) | 647(20) |
| $CH_3COCH_3$ | 17(5, 12) − 17(4, 13) EE | 107376.810(15e-3) | 105.9 | 740.89033 | 73 | 59.2(0.7) | 8.6(2.5) | 668(138) |
| $CH_3COCH_3$ | 17(6, 12) − 17(5, 13) EE | 107376.851(15e-3) | 105.9 | 740.88976 | blended | – | – | – |
| $C_2H_5CN$ | 12(7, 5) − 11(7, 4) | 107485.160(5e-2) | 88.0 | 117.36 | 161 | 60.0(0.5) | 9.5(0.5) | 1637(36) |
| $C_2H_5CN$ | 12(6, 6) − 11(6, 5) | 107486.949(5e-2) | 73.6 | 133.42 | 69 | 60.0(0.5) | 5.2(0.5) | 386(36) |
| $C_2H_5CN$ | 12(5, 7) − 11(5, 6) | 107502.432(5e-2) | 61.3 | 146.99 | 169 | 60.0(0.4) | 8.1(0.5) | 1459(36) |
| $CH_3COCH_3$ | 5(3, 2) − 4(2, 3) EE | 107515.906(11e-3) | 12.3 | 65.21048 | 14 | 59.2(0.5) | 0.6(0.5) | 89(36) |
| $C_2H_5CN$ | 12(10, 2) − 11(10, 1) | 107519.861(5e-2) | 144.6 | 54.355 | 40 | 60.1(0.3) | 7.4(0.5) | 317(36) |
| $CH_3COCH_3$ | 17(5, 12) − 17(4, 13) AA | 107525.628(19e-3) | 105.8 | 463.51993 | 26 | 59.2(0.5) | 3.9(0.5) | 110(36) |
| $CH_3COCH_3$ | 17(6, 12) − 17(5, 13) AA | 107525.670(19e-3) | 105.8 | 278.07892 | blended | – | – | – |
| $CH_3OCHO$ | 9( 2, 8) − 8( 2, 7) E | 107537.258(1e-2) | 28.8 | 22.60702 | 163 | 60.0(0.5) | 7.2(0.5) | 1244(36) |
| $CH_3OCHO$ | 9( 2, 8) − 8( 2, 7) A | 107543.711(1e-2) | 28.8 | 22.61344 | 240 | 60.0(0.5) | 7.3(0.5) | 1862(36) |
| $C_2H_5CN$ | 12(4, 9) − 11(4, 8) | 107544.042(5e-2) | 51.3 | 158.12 | blended | – | – | – |
| $C_2H_5CN$ | 12(4, 8) − 11(4, 7) | 107547.460(5e-2) | 51.3 | 158.11 | 97 | 60.1(0.5) | 6.9(0.5) | 709(36) |
| $CH_3OCHO$ | 23(6, 17) − 23(5, 18) A | 107590.389(1e-2) | 189.0 | 7.68646 | 58 | 60.0(0.4) | 7.0(0.5) | 434(24) |
| $C_2H_5CN$ | 12(3, 10) − 11(3, 9) | 107594.056(5e-2) | 43.6 | 166.77 | 132 | 60.1(0.5) | 10.5(0.5) | 1466(24) |
| $CH_3OCHO$ | 23(6, 17) − 23(5, 18) E | 107604.366(1e-2) | 189.0 | 7.68978 | 52 | 60.0(0.4) | 14.2(0.5) | 785(24) |
| $CH_3COCH_3$ | 15(8, 7) − 14(11, 3) EA | 107634.402(112e-3) | 95.7 | 0.76503 | 33 | 59.2(0.9) | 3.5(2.2) | 122(94) |
| $C_2H_5CN$ | 12(3, 9) − 11(3, 8) | 107734.723(5e-2) | 43.6 | 166.76 | 100 | 60.2(0.3) | 7.3(0.7) | 775(63) |
| $CH_3COCH_3$ | 27(15, 13) − 27(14, 14) EE | 107772.098(95e-3) | 298.7 | 1976.08819 | 18 | 59.2(0.8) | 1.5(1.2) | 28(26) |
| $CH_3COCH_3$ | 16(4, 12) − 16(3, 13) EE | 107797.721(13e-3) | 90.8 | 602.22608 | 32 | 59.3(0.7) | 4.8(1.4) | 164(49) |
| $CH_3COCH_3$ | 16(5, 12) − 16(4, 13) EE | 107797.728(13e-3) | 90.8 | 602.226 | blended | – | – | – |
| $SO_2$ | 12(4, 8) − 13(3, 11) | 107843.470(2e-3) | 111.0 | 4.5354 | 392 | 60.0(0.1) | 8.4(0.1) | 3520(47) |
| $CH_3OCHO$ | 15(5, 10) − 15(4, 11) E | 108045.959(1e-2) | 87.9 | 4.11041 | 31 | 60.1(0.5) | 3.0(1.2) | 100(34) |
| $CH_3OCHO$ | 15(5, 10) − 15(4, 11) A | 108050.939(1e-2) | 87.9 | 4.11748 | 37 | 60.0(0.3) | 1.2(0.5) | 46(20) |
| t-HCOOH | 5(1, 5) − 4(1, 4) | 108126.720(3e-6) | 18.8 | 9.6966 | 170 | 60.3(0.5) | 8.1(0.5) | 1468(21) |
| $CH_3COCH_3$ | 15(3, 12) − 15(2,13) EE | 108147.056(13e-3) | 76.7 | 460.37793 | 49 | 59.3(0.5) | 5.5(0.5) | 290(21) |
| $CH_3COCH_3$ | 15(4, 12) − 15(3,13) EE | 108147.057(13e-3) | 76.7 | 460.37792 | blended | – | – | – |
| $CH_3COCH_3$ | 14(2, 12) − 14(1, 13) AE | 108240.911(21e-3) | 63.4 | 39.19411 | 21 | 59.2(1.7) | 4.7(4.1) | 103(58) |
| $CH_3COCH_3$ | 14(2, 12) − 14(1, 13) EA | 108241.031(16e-3) | 63.4 | 78.40068 | blended | – | – | – |
| $CH_3COCH_3$ | 7(4, 3) − 7(1, 6) AA | 108331.398(21e-3) | 22.6 | 0.51266 | 17 | 59.2(0.5) | 4.3(0.5) | 79(17) |
| $CH_3COCH_3$ | 8(3, 5) − 7(4, 4) AE | 108342.518(12e-3) | 26.9 | 65.10119 | 26 | 59.2(0.5) | 1.3(0.5) | 36(17) |
| $CH_3COCH_3$ | 8(3, 5) − 7(4, 4) EA | 108358.421(11e-3) | 26.9 | 130.21505 | 26 | 59.3(0.5) | 5.1(0.5) | 416(17) |
| $CH_3COCH_3$ | 8(3, 5) − 7(4, 4) EE | 108387.595(8e-3) | 88.2 | 519.86714 | 57 | 59.3(0.5) | 2.4(0.5) | 757(17) |
| $^{13}CN$ | 1(1, 0) − 0(1, 1), F = 1 − 0 | 108406.091(5e-2) | 5.2 | 0.191 | 27 | 61.1(1.1) | 5.8(1.1) | 461(29) |
| $^{13}CN$ | 1(1, 0) − 0(1, 1), F = 1 − 1 | 108412.862(5e-2) | 5.2 | 0.635 | 33 | 61.0(1.1) | 6.2(1.1) | 216(29) |
| $CH_3COCH_3$ | 8(3, 5) − 7(4, 4) AA | 108424.565(11e-3) | 26.7 | 194.60833 | 37 | 59.3(1.1) | 8.1(1.1) | 323(29) |
| $^{13}CN$ | 1(1, 0) − 0(1, 1), F = 1 − 2 | 108426.889(5e-2) | 5.2 | 1.267 | 10 | 60.8(1.1) | 2.8(1.1) | 243(29) |
| $CH_3COCH_3$ | 14(2, 12) − 14(1, 13) EE | 108434.511(16e-3) | 63.4 | 313.86255 | 44 | 59.2(1.1) | 9.6(1.1) | 452(29) |
| $C_2H_5OH$ | 13(3, 10) − 13(2, 11) | 108438.579(5e-2) | 88.2 | 18.79 | 44 | 60.2(1.1) | 6.4(1.1) | 774(29) |
| $CH_3COCH_3$ | 13(1, 12) − 13(0, 13) AE | 108461.338(27e-3) | 51.0 | 60.36275 | 102 | 59.3(1.1) | 6.3(1.1) | 686(29) |
| $CH_3COCH_3$ | 13(2, 12) − 13(1, 13) EA | 108461.496(19e-3) | 51.0 | 40.24091 | blended | – | – | – |
| $C_2H_5OH$ | 16(2, 15) − 15(3, 12) | 108524.526(5e-2) | 118.2 | 2.9899 | 19 | 60.1(3.7) | 7.2(8.1) | 146(144) |
| $^{13}CN$ | 1(1, 1) − 0(1, 0), F = 1 − 1 | 108636.923(5e-2) | 5.2 | 1.932 | 31 | 61.0(0.9) | 3.1(1.5) | 103(49) |
| $^{13}CN$ | 1(2, 1) − 0(1, 1), F = 1 − 0 | 108638.212(5e-2) | 5.2 | 0.722 | 32 | 61.0(0.7) | 2.1(1.4) | 73(45) |
| $^{13}CN$ | 1(2, 1) − 0(1, 1), F = 2 − 1 | 108643.590(5e-2) | 5.2 | 0.856 | 27 | 60.8(1.0) | 6.5(1.5) | 185(52) |
| $^{13}CN$ | 1(2, 1) − 0(1, 1), F = 0 − 1 | 108644.346(5e-2) | 5.2 | 0.642 | blended | – | – | – |

**Table A2.** (Continued)

| Species | Transitions | Rest Freq. (MHz) | $E_u$ (K) | $\mu^2 S$ ($D^2$) | $T_{mb}$ (mK) | $V_{LSR}$ (km $s^{-1}$) | $\Delta V$ (km $s^{-1}$) | $\int T_{mb}\,dv$ (mK km $s^{-1}$) |
|---|---|---|---|---|---|---|---|---|
| $^{13}CN$ | 1(2, 1) − 0(1, 1), F = 1 − 1 | 108645.064(5e-2) | 5.2 | 0.551 | blended | – | – | – |
| $^{13}CN$ | 1(1, 1) − 0(1, 0), F = 2 − 1 | 108651.297(5e-2) | 5.2 | 3.276 | 74 | 61.0(0.3) | 4.8(0.6) | 380(46) |
| $^{13}CN$ | 1(2, 1) − 0(1, 1), F = 2 − 2 | 108657.646(5e-2) | 5.2 | 2.420 | 56 | 61.2(0.5) | 5.7(0.9) | 341(51) |
| $^{13}CN$ | 1(2, 1) − 0(1, 1), F = 1 − 2 | 108658.948(5e-2) | 5.2 | 0.669 | blended | – | – | – |
| $^{13}CN$ | 1(2, 2) − 0(1, 1), F = 3 − 2 | 108780.201(5e-2) | 5.2 | 4.905 | 97 | 61.1(0.5) | 4.5(0.5) | 465(19) |
| $^{13}CN$ | 1(2, 2) − 0(1, 1), F = 2 − 1 | 108782.374(5e-2) | 5.2 | 2.586 | 76 | 61.1(0.5) | 6.8(0.5) | 550(19) |
| $^{13}CN$ | 1(2, 2) − 0(1, 1), F = 1 − 0 | 108786.982(5e-2) | 5.2 | 1.144 | 22 | 61.0(0.5) | 2.1(0.5) | 49(19) |
| $^{13}CN$ | 1(2, 2) − 0(1, 1), F = 1 − 1 | 108793.753(5e-2) | 5.2 | 0.894 | 44 | 61.0(0.5) | 5.2(0.5) | 244(19) |
| $^{13}CN$ | 1(2, 2) − 0(1, 1), F = 2 − 2 | 108796.400(5e-2) | 5.2 | 0.918 | 31 | 61.0(0.5) | 2.6(0.5) | 87(19) |
| $CH_3OH$, vt=0-2 | 0(0) − 1(-1) E2, vt=0 | 108893.945(12e-3) | 13.1 | 3.9134 | 666 | 59.7(0.1) | 9.3(0.2) | 6574(128) |
| $C_2H_5CN$ | 12(2, 10) − 11(2, 9) | 108940.554(5e-2) | 38.2 | 172.93 | blended | – | – | – |
| $C_2H_5CN$ | 11(3, 9) − 12(0, 12) | 108940.696(4e-3) | 38.4 | 0.042598 | 145 | 60.0(0.5) | 8.6(0.5) | 1323(31) |
| $SO_2$ | 39(6, 34) − 38(7, 31) | 108955.915(2e-3) | 808.3 | 16.377 | 82 | 60.0(0.5) | 8.7(0.5) | 755(31) |
| $CH_3OH$, vt=0-2 | 14(5) − 15(4) E1, vt=0 | 109138.783(15e-3) | 379.7 | 13.593 | 276 | 59.8(0.5) | 11.4(0.5) | 3347(273) |
| $CH_3OH$, vt=0-2 | 16(-2) − 16(1) E2, vt=0 | 109153.184 (14e-3) | 342.0 | 14.926 | 282 | 59.8(0.5) | 13.3(0.5) | 4003(273) |
| $HC_3N$ | 12 − 11 | 109173.634(1e-2) | 34.1 | 167.1 | 3724 | 60.5(0.5) | 6.2(0.5) | 24591(273) |
| SO | 3(2) − 2(1) | 109252.220(1e-1) | 21.1 | 3.5585 | 1469 | 61.0(0.) | 9.5(0.1) | 14783(83) |
| $HC_3N$, $v_7$=1 | 12(-1) − 11(1) | 109442.013(2e-2) | 355.0 | 165.12 | 121 | 60.6(0.3) | 11.1(0.8) | 1430(82) |
| OCS | 9 − 8 | 109463.063(5e-3) | 26.3 | 4.6034 | 667 | 60.0(0.1) | 8.3(0.1) | 5896(67) |
| HNCO | 5(1, 5) − 4(1, 4) | 109495.996(6e-3) | 59.0 | 11.847 | 345 | 60.0(0.1) | 9.2(0.2) | 3394(71) |
| $CH_3OCH_3$ | 8(2, 7) − 8(1, 8) AA | 109576.778(11e-3) | 38.3 | 59.869 | 55 | 59.0(1.1) | 9.9(2.0) | 577(116) |
| $HC_3N$, $v_7$=1 | 12(1) − 11(-1) | 109598.818(2e-2) | 355.0 | 165.12 | 137 | 60.6(0.9) | 6.5(1.2) | 113(58) |
| $C_2H_5CN$ | 12(1, 11) − 11(1, 10) | 109650.263(5e-2) | 35.4 | 176.49 | 132 | 60.2(0.3) | 11.2(1.4) | 1566(126) |
| $CH_3SH$, v=0-2 | 5(-1, 5) − 5(0, 5) A, vt=0 | 109719.946 (1e-3) | 23.5 | 2.9509 | 61 | 59.3(2.0) | 3.5(4.4) | 229(243) |
| $NH_2CHO$ | 5(1, 4) − 4(1, 3) | 109753.549(25e-3) | 18.8 | 62.756 | 196 | 59.2(1.9) | 8.9(3.8) | 1859(868) |
| $SO_2$ | 17(5, 13) − 18(4, 14) | 109757.585(2e-3) | 202.1 | 6.6069 | 295 | 60.0(1.2) | 8.7(2.9) | 27538(949) |
| $C^{18}O$ | 1 − 0 | 109782.173(6e-3) | 5.3 | 0.01221 | 3345 | 61.0(0.1) | 7.1(0.1) | 25396(248) |
| HNCO | 5(3, 2) − 4(3, 1) | 109833.487(7e-3) | 390.8 | 7.1906 | 144 | 60.1(0.5) | 6.9(0.5) | 1060(66) |
| HNCO | 5(2, 3) − 4(2, 2) | 109872.765(3e-2) | 186.1 | 10.012 | 322 | 60.0(0.5) | 9.9(0.5) | 2289(66) |
| HNCO | 5(2, 4) − 4(2, 3) | 109872.337(3e-2) | 186.1 | 10.013 | blended | – | – | – |
| $C_2H_5CN$ | 10(5, 5) − 11(4, 8) | 109880.580(3e-3) | 51.4 | 1.4514 | 10 | 60.2(0.5) | 2.3(0.5) | 26(66) |
| HNCO | 5(0, 5) − 4(0, 4) | 109905.749(7e-3) | 15.8 | 12.482 | 519 | 60.0(1.1) | 10.9(1.1) | 6041(126) |
| $C_2H_5CN$ | 22(1, 21) − 22(1, 22) | 109958.637(5e-2) | 111.4 | 1.7932 | 90 | 60.0(0.1) | 9.5(0.6) | 912(57) |
| $CH_3COCH_3$ | 6(5, 2) − 5(4, 1) EE | 109994.365(17e-3) | 18.2 | 375.7236 | 47 | 59.3(0.1) | 3.5(1.0) | 176(43) |
| $C^{15}N$ | 1(2, 1) − 0(1, 1) | 110004.091(3e-2) | 5.3 | 0.717 | 52 | 61.8(1.4) | 8.7(3.5) | 482(158) |
| $C^{15}N$ | 1(2, 1) − 0(1, 0) | 110023.540(1e-1) | 5.3 | 1.386 | 49 | 61.7(1.0) | 1.4(1.7) | 74(8.4) |
| $C^{15}N$ | 1(2, 2) − 0(1, 1) | 110024.590(1e-1) | 5.3 | 3.504 | 53 | 61.7(0.8) | 2.1(0.9) | 156(119) |
| $CH_3OCHO$ | 9(4, 6) − 8(4, 5) A | 110035.269(1e-2) | 224.9 | 19.15168 | 12 | 59.9(3.9) | 3.2(4.8) | 41(74) |
| $CH_3OCHO$ | 9(6, 4) − 8(6, 3) E | 110050.332(1e-2) | 237.4 | 13.33458 | 43 | 60.0(0.7) | 0.9(1.1) | 40(47) |
| $^{13}CO$ | 1 − 0 | 110201.35(0) | 5.3 | 0.01220 | 23549 | 60.5(0.1) | 4.7(0.5) | 117380(1630) |
| HNCO | 5(1, 4) − 4(1, 3) | 110298.089(5e-3) | 59.2 | 11.847 | 280 | 60.0(0.5) | 7.9(0.5) | 2359(1630) |
| $CH_3{}^{13}CN$ | 6(3) − 5(3) | 110309.800(1e-1) | 82.8 | 276.874 | blended | – | – | – |
| $CH_3{}^{13}CN$ | 6(2) − 5(2) | 110320.400(1e-1) | 47.1 | 164.054 | 379 | 60.1(0.5) | 9.3(0.5) | 5003(153) |
| $CH_3{}^{13}CN$ | 6(1) − 5(1) | 110326.770(1e-1) | 25.7 | 179.434 | 76 | 60.1(0.5) | 6.2(0.5) | 1642(153) |
| $CH_3{}^{13}CN$ | 6(0) − 5(0) | 110328.870(1e-1) | 18.5 | 184.563 | 70 | 60.0(0.5) | 8.9(0.5) | 1399(153) |
| $CH_3CN$ | 6(5, 0) − 5(5, 0) | 110330.345(0) | 197.1 | 56.399 | blended | – | – | – |
| $CH_3CN$ | 6(4, 0) − 5(4, 0) | 110349.471(0) | 132.8 | 102.54 | 278 | 60.2(0.5) | 6.7(0.5) | 3979(153) |
| $CH_3CN$ | 6(3, 0) − 5(-3, 0) | 110364.354(0) | 82.8 | 138.45 | 491 | 60.3(0.3) | 8.9(0.5) | 4655(153) |
| $CH_3CN$ | 6(-3, 0) − 5(3, 0) | 110364.354(0) | 82.8 | 138.45 | blended | – | – | – |
| $CH_3CN$ | 6(2, 0) − 5(2, 0) | 110374.989(0) | 47.1 | 164.06 | 915 | 60.3(0.5) | 9.1(0.5) | 8820(153) |
| $CH_3CN$ | 6(1, 0) − 5(1, 0) | 110381.372(0) | 25.7 | 179.45 | 878 | 60.3(0.4) | 8.3(0.5) | 7764(153) |
| $CH_3CN$ | 6(0, 0) − 5(0, 0) | 110383.500(0) | 18.5 | 184.58 | 1312 | 60.1(0.5) | 6.9(0.5) | 17853(153) |
| $CH_3COCH_3$ | 6(5, 2) − 5(4, 1) AA | 110401.333(11e-3) | 18.2 | 279.46535 | 43 | 59.1(0.7) | 5.7(1.6) | 261(65) |
| $CH_3COCH_3$ | 8(4, 5) − 7(3, 4) EE | 110409.372(7e-3) | 26.8 | 530.75828 | 54 | 59.3(0.6) | 8.0(1.8) | 461(82) |
| $CH_3OCHO$ | 9(8, 1) − 8(8, 0) E | 110447.180(1e-2) | 69.0 | 5.02983 | 42 | 60.2(0.6) | 3.9(1.4) | 173(51) |
| $CH_3OCHO$ | 9(8, 1) − 8(8, 0) A | 110455.372(1e-2) | 69.0 | 5.02998 | 63 | 60.2(0.8) | 7.5(1.7) | 501(132) |
| $CH_3OCHO$ | 9(8, 2) − 8(8, 1) E | 110458.014(1e-2) | 69.0 | 5.02965 | 65 | 60.0(0.9) | 10.1(2.1) | 696(141) |
| $CH_3COCH_3$ | 8(4, 5) − 7(3, 4) AA | 110490.618(11e-3) | 26.7 | 331.30071 | 50 | 59.1(0.5) | 4.0(1.2) | 212(52) |
| $CH_3OCHO$ | 9(7, 2) − 8(7, 1) E | 110525.741(1e-2) | 59.1 | 9.46492 | blended | – | – | – |
| $CH_3OCHO$ | 7(2, 6) − 6(1, 5) A | 110526.190(1e-2) | 206.7 | 1.41631 | 98 | 60.2(1.4) | 12.3(4.0) | 1292(305) |
| $CH_3OCHO$ | 9(7, 2) − 8(7, 1) A | 110535.186(1e-2) | 59.1 | 9.46711 | 202 | 60.0(0.6) | 9.9(1.4) | 2127(245) |
| $CH_3OCHO$ | 9(7, 3) − 8(7, 2) E | 110536.003(1e-2) | 59.1 | 9.46692 | blended | – | – | – |
| $C_2H_5OH$ | 7(2, 6) − 6(1, 6) | 110545.866(5e-2) | 84.9 | 1.3914 | 60 | 60.0(1.9) | 8.9(4.9) | 569(255) |
| $CH_3OCHO$ | 9(2, 6) − 8(1, 5) E | 110550.203(1e-2) | 19.0 | 1.39763 | 29 | 60.1(4.2) | 10.7(10.4) | 317(265) |
| $CH_3OCHO$ | 9(2, 6) − 8(1, 5) A | 110560.051(1e-2) | 19.0 | 1.39665 | 23 | 60.0(4.3) | 8.2(6.7) | 167(183) |
| $CH_3OCHO$ | 10(0,10) − 9(0, 9) | 110571.632(1e-2) | 217.9 | 26.10484 | 55 | 60.0(1.6) | 6.2(3.2) | 366(182) |
| $CH_3OCHO$ | 10(0,10) − 9(0, 9) E | 110655.310(1e-2) | 217.2 | 26.25577 | 90 | 60.0(2.3) | 7.1(2.7) | 686(211) |
| $CH_3OCHO$ | 9(6, 4) − 8(6, 3) E | 110662.315(1e-2) | 50.4 | 13.30855 | 216 | 60.0(1.1) | 8.2(1.0) | 1881(213) |
| $CH_3OCHO$ | 9(6, 4) − 8(6, 3) A | 110663.273(1e-2) | 50.4 | 13.3113 | blended | – | – | – |
| $CH_3OCHO$ | 9(6, 3) − 8(6, 2) A | 110663.429(1e-2) | 50.4 | 13.31127 | blended | – | – | – |
| $CH_3CN$, $v_8$=1 | 6(3, 1) − 5(3, 1) | 110680.294(7e-3) | 647.9 | 128.72357 | 40 | 59.9(1.1) | 4.9(1.1) | 210(70) |
| $CH_3CN$, $v_8$=1 | 6(5, 2) − 5(5, 2) | 110683.952(1e-2) | 655.6 | 52.44313 | 57 | 59.9(1.0) | 7.7(1.1) | 467(70) |
| $CH_3CN$, $v_8$=1 | 6(2, 1) − 5(2, 1) | 110695.473(7e-3) | 598.9 | 305.1398 | 134 | 59.9(1.1) | 9.3(1.1) | 1333(70) |
| $CH_3CN$, $v_8$=1 | 6(4, 2) − 5(4, 2) | 110698.717(8e-3) | 604.7 | 190.69518 | 80 | 59.7(1.1) | 6.6(1.1) | 563(70) |
| $CH_3CN$, $v_8$=1 | 6(1, 1) − 5(1, 1) | 110706.243(7e-3) | 564.2 | 166.85665 | 124 | 59.9(1.1) | 6.3(1.1) | 1665(70) |
| $CH_3CN$, $v_8$=1 | 6(0, 1) − 5(0, 1) | 110712.176(7e-3) | 543.8 | 171.63268 | 132 | 59.8(1.0) | 8.1(1.1) | 1132(70) |
| $CH_3CN$, $v_8$=1 | 6(2, 2) − 5(2, 2) | 110716.257(6e-3) | 545.7 | 152.57534 | 123 | 59.9(1.1) | 10.8(1.1) | 1412(70) |
| $CH_3OCHO$ | 9(1, 8) − 8(1, 7) | 110776.499(1e-2) | 215.7 | 23.1436 | 61 | 60.0(1.1) | 7.3(1.1) | 469(111) |
| $CH_3OCHO$ | 10(1,10) − 9(1, 9) E | 110788.664(1e-2) | 30.3 | 26.16584 | 219 | 60.2(1.0) | 7.8(1.1) | 1821(111) |
| $CH_3OCHO$ | 10(1,10) − 9(1, 9) A | 110790.526(1e-2) | 30.3 | 16.17539 | 196 | 60.1(1.1) | 7.6(1.1) | 580(111) |
| $CH_3CN$, $v_8$=1 | 6(1, 2) − 5(-1, 2) | 110823.116(6e-3) | 537.6 | 166.88912 | 115 | 60.0(0.6) | 8.2(1.3) | 1004(137) |
| $C_2H_3CN$ | 12(1, 12) − 11(1, 11) | 110839.968(1e-3) | 36.8 | 520.3 | 42 | 61.1(1.3) | 6.0(2.5) | 268(112) |
| $CH_3OCHO$ | 9(5, 4) − 8(5, 3) E | 110873.955(1e-2) | 43.2 | 16.55557 | 100 | 60.0(0.6) | 4.3(1.0) | 461(99) |
| $CH_3OCHO$ | 9(5, 5) − 8(5, 4) E | 110882.331(1e-2) | 43.2 | 16.55225 | 222 | 60.1(0.3) | 8.6(0.7) | 2035(139) |
| $CH_3OCHO$ | 9(3, 7) − 8(3, 6) A | 110887.092(1e-2) | 32.6 | 21.25577 | 124 | 60.0(0.5) | 6.9(1.4) | 906(144) |
| $CH_3OCHO$ | 9(5, 4) − 8(5, 3) A | 110890.256(1e-2) | 43.2 | 16.56106 | 74 | 60.1(0.7) | 4.1(1.2) | 323(105) |
| $CH_3OCHO$ | 9(4, 6) − 8(4, 4) E | 110918.768(1e-2) | 37.2 | 1.02704 | 28 | 60.0(2.0) | 7.5(4.8) | 445(235) |
| $CH_3COOH$, vt=0 | 9(1, 8) A1 − 8(2, 7) A2 | 110954.111(1e-3) | 29.3 | 15.70004 | 42 | 59.0(3.8) | 9.5(5.2) | 429(195) |
| $CH_3COOH$, vt=0 | 9(2, 8) A1 − 8(2, 7) A2 | 110954.171(1e-3) | 29.3 | 5.68984 | blended | – | – | – |
| $CH_3COOH$, vt=0 | 9(1, 8) A1 − 8(1, 7) A2 | 110954.555(1e-3) | 29.3 | 5.6898 | blended | – | – | – |
| $CH_3COOH$, vt=0 | 9(2, 8) A1 − 8(1, 7) A2 | 110954.615(1e-3) | 29.3 | 15.6999 | blended | – | – | – |
| $CH_3OCHO$ | 15(4, 12) − 15(3, 13) A | 110962.153(1e-2) | 81.8 | 3.66282 | 13 | 60.0(1.3) | 3.7(1.7) | 50(31) |
| $CH_3COCH_3$ | 8(4, 4) − 7(5, 3) EE | 110987.131(16e-3) | 28.5 | 273.48458 | 26 | 59.3(2.0) | 6.8(4.3) | 192(107) |
| $CH_3OCHO$ | 9(3, 7) − 8(3, 6) E | 111005.672(1e-2) | 219.5 | 20.82222 | 75 | 60.0(0.8) | 6.1(2.0) | 973(139) |
| $CH_3COCH_3$ | 6(4, 3) − 5( 3, 3) EA | 111067.701(9e-3) | 17.0 | 0.36744 | 43 | 59.3(1.0) | 4.4(2.2) | 199(83) |
| $CH_3OCHO$ | 10(0, 10) − 9(0, 9) E | 111169.903(1e-2) | 30.2 | 26.18776 | 247 | 60.0(0.2) | 8.4(0.4) | 2216(103) |
| $CH_3OCHO$ | 10(0, 10) − 9(0, 9) A | 111171.634(1e-2) | 30.2 | 26.19136 | blended | – | – | – |
| $CH_3OCHO$ | 9(4, 6) − 8(4, 5) A | 111195.962(1e-2) | 37.2 | 19.21722 | 123 | 60.0(0.4) | 6.3(0.8) | 830(90) |
| $CH_3OCHO$ | 9(4, 6) − 8(4, 5) E | 111223.491(1e-2) | 37.2 | 18.18412 | blended | – | – | – |
| $CH_3COCH_3$ | 10(1, 9) − 9(2, 8) AE | 111243.339(11e-3) | 32.2 | 141.0573 | 154 | 59.2(0.1) | 6.5(0.6) | 1063(91) |
| $CH_3COCH_3$ | 10(2, 9) − 9(1, 8) AE | 111243.388(11e-3) | 32.2 | 423.15082 | blended | – | – | – |

**Table A2.** (Continued)

| Species | Transitions | Rest Freq. | $E_u$ | $\mu^2S$ | $T_{mb}$ | $V_{LSR}$ | $\Delta V$ | $\int T_{mb}\,dv$ |
|---|---|---|---|---|---|---|---|---|
| | | (MHz) | (K) | ($D^2$) | (mK) | (km $s^{-1}$) | (km $s^{-1}$) | (mK km $s^{-1}$) |
| $CH_3COCH_3$ | 10(1, 9) − 9(2, 8) EA | 111243.424(1e-2) | 32.2 | 282.09469 | blended | – | – | – |
| $CH_3COCH_3$ | 10(2, 9) − 9(1, 8) EA | 111243.472(1e-2) | 32.2 | 282.09445 | blended | – | – | – |
| $CH_3COCH_3$ | 10(1, 9) − 9(2, 8) EE | 111267.514(8e-3) | 32.1 | 1128.14194 | 103 | 59.3(0.5)) | 8.4(1.2) | 919(110) |
| $CH_3COCH_3$ | 10(2, 9) − 9(1, 8) EE | 111267.565(8e-3) | 32.1 | 1128.14091 | blended | – | – | – |
| $CH_3OH$, vt=0-2 | $7(2)^+ - 8(1)^+$, vt=0 | 111289.453(13e-3) | 102.7 | 9.3425 | 151 | 60.0(0.3) | 8.7(0.8) | 1391(109) |
| $CH_3COCH_3$ | 10(1, 9) − 9(2, 8) AA | 111291.573(12e-3) | 32.0 | 422.99289 | 574 | 59.3(0.1) | 9.7(0.2) | 5914(108) |
| $C_2H_5OH$ | 7(1, 7) − 7(0, 7) | 111344.327(5e-2) | 85.3 | 9.6676 | 54 | 60.1(1.0) | 4.2(2.1) | 242(114) |
| $CH_3OCHO$ | 9(4, 5) − 8(4, 4) E | 111408.412(1e-2) | 37.3 | 18.18767 | 98 | 60.0(0.6) | 4.5(1.1) | 470(114) |
| $CH_3OCHO$ | 9(4, 5) − 8(4, 4) A | 111453.300(1e-2) | 37.2 | 19.21778 | 124 | 60.0(0.5) | 4.5(1.1) | 593(125) |
| $CH_3COOH$, vt=0 | 10(0, 10) − 9(1, 9) E | 111507.280(1e-3) | 31.0 | 20.80201 | 29 | 59.0(0.8) | 4.1(2.2) | 127(58) |
| $CH_3COOH$, vt=0 | 10(0, 10) A1 − 9(1, 9) A2 | 111548.535(1e-3) | 30.5 | 20.40186 | 58 | 59.0(0.7) | 8.6(1.5) | 532(82) |
| $CH_3COOH$, vt=0 | 10(0, 10) A1 − 9(0, 9) A2 | 111548.536(1e-3) | 30.5 | 6.98023 | blended | – | – | – |
| $CH_3OCHO$ | 9(1, 8) − 8(1, 7) E | 111674.131(1e-2) | 28.1 | 23.18984 | 188 | 60.1(0.2) | 7.2(0.4) | 1445(75) |
| $CH_3OCHO$ | 9(1, 8) − 8(1, 7) A | 111682.189(1e-2) | 28.1 | 23.19587 | 179 | 60.0(0.1) | 6.9(0.4) | 1314(74) |
| $CH_3OCHO$ | 10(1, 10) − 9(0, 9) E | 111734.002(1e-2) | 30.3 | 3.84434 | blended | – | – | – |
| $CH_3OCHO$ | 10(1, 10) − 9(0, 9) A | 111735.307(1e-2) | 30.3 | 3.84224 | 105 | 60.1(1.1) | 10.1(1.1) | 1131(95) |
| $CH_3OCH_3$ | 9(3,16) − 19(2,17) EE | 111742.794(25e-3) | 187.5 | 329.06069 | 127 | 59.0(1.1) | 11.5(1.1) | 1552(95) |
| $CH_3OCH_3$ | 19(3, 16) − 19(2, 17) AA | 111744.238(29e-3) | 187.5 | 205.6671 | 188 | 59.1(1.1) | 12.5(1.1) | 2501(95) |
| $SO_2$ | 31(3, 29) − 30(4, 26) | 111755.021(2e-3) | 476.9 | 6.4499 | 153 | 60.0(1.1) | 9.9(1.1) | 1618(95) |
| $CH_3OCH_3$ | 7(0, 7) − 6(1, 6) AA | 111782.562(8e-3) | 25.2 | 53.86755 | 254 | 59.1(1.1) | 8.1(1.1) | 2187(95) |
| $CH_3OCH_3$ | 7(0, 7) − 6(1, 6) EE | 111783.010(4e-2) | 25.3 | 86.2034 | blended | – | – | – |
| $CH_3OCH_3$ | 7(0, 7) − 6(1, 6) EA | 111783.647(7e-3) | 25.3 | 21.54865 | blended | – | – | – |
| $CH_3OCH_3$ | 7(0, 7) − 6(1, 6) AE | 111783.648(7e-3) | 25.3 | 32.32363 | blended | – | – | – |
| $CH_3COCH_3$ | 24(11, 13) − 24(10, 14) EE | 111797.250(55e-3) | 230.4 | 1557.78153 | 34 | 59.3(0.6) | 4.1(1.3) | 150(41) |
| $CH_3OCH_3$ | 7(5, 3) − 8(4, 5) EE | 111804.813(26e-3) | 60.6 | 7.72103 | 22 | 59.0(0.7) | 4.0(1.0) | 96(34) |
| $CH_3OCH_3$ | 7(5, 2) − 8(4, 5) EE | 111812.674(31e-3) | 60.6 | 0.47164 | 119 | 59.2(0.3) | 10.9(0.6) | 1380(88) |
| $HC_5N$ | 42 − 41 | 111823.024(0) | 115.4 | 2362.2 | 41 | 61.1(1.2) | 9.5(2.8) | 846(106) |
| H$\beta$ | H (48) $\beta$ | 111885.070(0) | – | – | 342 | 56.2(0.4) | 27.4(1.0) | 9969(313) |
| $CH_3OCHO$ | 9(3, 6) − 8(3, 5) E | 112011.966(1e-2) | 219.9 | 21.00957 | 32 | 60.0(0.6) | 1.2(0.8) | 42(32) |
| $C_2H_5OH$ | 12(3, 9) − 12(2, 10) | 112129.544(5e-2) | 77.1 | 16.463 | 139 | 59.8(0.5) | 6.3(0.5) | 1809(27) |
| $CH_3OH$, vt=0-2 | $19(0)^+ - 18(2)^+$, vt=0 | 112145.638(21e-3) | 440.1 | 0.00059 | 120 | 60.0(0.5) | 9.0(0.5) | 1154(27) |
| $CH_3CHO$ | 6(1, 6) − 5(1, 5) A, vt=0 | 112248.716(3e-3) | 21.1 | 73.76807 | 70 | 59.1(0.9) | 5.3(1.4) | 396(113) |
| $CH_3CHO$ | 6(1, 6) − 5(1, 5) E, vt=0 | 112254.508(3e-3) | 21.2 | 73.79585 | 86 | 59.1(0.8) | 6.7(1.4) | 617(132) |
| t-HCOOH | 5(2, 4) − 4(2, 3) | 112287.145 (3e-3) | 28.9 | 8.4851 | 107 | 60.0(0.5) | 5.1(1.0) | 583(115) |
| $CH_3OCHO$ | 25( 5,20)-25( 4,21) A | 112310.915(1e-2) | 214.4 | 7.80962 | 43 | 59.8(1.1) | 3.4(2.3) | 155(94) |
| $C^{17}O$ | 1 − 0 | 112359.284(1e-3) | 5.4 | 0.01217 | 924 | 61.5(0.5) | 8.1(0.5) | 7974(91) |
| $CH_3COCH_3$ | 11(1, 11) − 10(0, 10) AE | 112365.987(13e-3) | 33.6 | 178.40946 | 71 | 59.3(0.5) | 3.4 (0.5) | 258(91) |
| $CH_3COCH_3$ | 11(0, 11) − 10(1, 10) EE | 112373.549(9e-3) | 33.5 | 1426.94226 | 175 | 59.3(0.5) | 7.8(0.5) | 1448(91) |
| $CH_3COCH_3$ | 11(0, 11) − 10(1, 10) AA | 112381.030(14e-3) | 33.4 | 891.85807 | 62 | 59.3(0.5) | 7.7(0.5) | 505(91) |
| t-HCOOH | 5(4, 2) − 4(4, 1) | 112432.292(3e-3) | 67.1 | 3.6372 | blended | – | – | – |
| t-HCOOH | 5(4, 1) − 4(4, 0) | 112432.319(3e-3) | 67.1 | 3.6372 | 85 | 60.1(0.7) | 6.8(1.1) | 523(113) |
| t-HCOOH | 5(3, 3) − 4(3, 2) | 112459.621(3e-3) | 44.8 | 6.4662 | 73 | 60.0(0.7) | 4.7(1.1) | 362(98) |
| t-HCOOH | 5(3, 2) − 4(3, 1) | 112467.007(3e-3) | 44.8 | 6.4654 | 58 | 60.0(0.8) | 4.2(1.4) | 257(94) |
| $C_2H_5CN$ | 13(1, 13) − 12(1, 12) | 112646.350(9e-2) | 39.0 | 191.45 | 129 | 60.1(0.3) | 7.0(0.7) | 955(90) |
| $NH_2CHO$ | 8(3, 6) − 9(2, 7) | 112654.015(112e-3) | 63.5 | 0.84513 | 60 | 59.1(0.5) | 3.1(1.1) | 199(61) |
| $CH_3OCHO$ | 14(5, 9) −14(4, 10) E | 112672.759(1e-2) | 78.9 | 3.64313 | 50 | 60.1(0.9) | 7.7(1.8) | 409(93) |
| $CH_3OCHO$ | 14(5, 9) −14(4, 10) A | 112676.856(1e-2) | 78.9 | 3.67559 | 42 | 60.0(0.7) | 2.8(1.2) | 124(55) |
| $C_2H_5OH$ | 45(5, 41) − 45(4, 41) | 112819.638(5e-2) | 954.0 | 43.302 | 99 | 59.8(0.6) | 2.9(1.0) | 306(108) |
| $C_2H_5OH$ | 18(2, 17) − 18(1, 17) | 112894.167(5e-2) | 207.2 | 13.554 | 141 | 60.0(0.7) | 9.5(1.5) | 1419(200) |
| $CH_3OCH_3$ | 20(3, 17) − 20(2, 18) AA | 113002.265(34e-3) | 206.1 | 130.85038 | 86 | 59.0(0.7) | 6.1(1.4) | 554(120) |
| $CH_3OCH_3$ | 17(3, 14) − 17(2, 15) EA | 113057.427(19e-3) | 153.1 | 132.79 | 25 | 59.0(1.9) | 1.5(0.4) | 89(41) |
| $CH_3OCH_3$ | 17(3, 14) − 17(2, 15) AE | 113057.425(18e-3) | 153.1 | 88.525 | blended | – | – | – |
| $CH_3OCH_3$ | 17(3, 14) − 17(2, 15) EE | 113059.249(17e-3) | 153.1 | 354.12 | 67 | 59.1(1.0) | 3.2(2.3) | 226(136) |
| $CH_3OCH_3$ | 17(3, 14) − 17(2, 15) AA | 113061.072(22e-3) | 153.1 | 221.33 | 69 | 59.0(0.5) | 0.8(0.1) | 69(56) |
| $C_2H_5OH$ | 10(2, 9) − 12(1, 10) | 113098.078(5e-2) | 51.0 | 8.3566 | 57 | 60.0(1.7) | 4.2(2.9) | 258(150) |
| CN | N= 1-0, J=1/2-1/2, F=1/2-1/2 | 113123.370(6e-3) | 5.4 | 0.15271 | 404 | 60.0(0.5) | 6.4(0.5) | 2745(320) |
| CN | N= 1-0, J=1/2-1/2, F=1/2-3/2 | 113144.157(6e-3) | 5.4 | 1.2492 | 2222 | 59.8(0.4) | 6.0(0.5) | 14252(320) |
| CN | N= 1-0, J=1/2-1/2, F=3/2-1/2 | 113170.492(4e-3) | 5.4 | 1.2199 | 2804 | 59.8(0.3) | 6.1(0.5) | 18201(320) |
| CN | N= 1-0, J=1/2-1/2, F=3/2-3/2 | 113191.279(3e-3) | 5.4 | 1.5836 | 2843 | 59.8(0.5) | 5.9(0.5) | 17944(320) |
| $C_2H_5OH$ | 6(1, 6) − 6(0, 6) | 113325.517(5e-2) | 79.6 | 8.8225 | 22 | 60.0(2.2) | 3.1(1.8) | 74(43) |
| CCS | 9(8) − 8(7) | 113410.186(2e-2) | 33.6 | 65.427 | 64 | 61.5(0.5) | 7.6(1.4) | 519(97) |
| CN | N= 1-0, J=3/2-1/2, F=3/2-1/2 | 113488.120(3e-3) | 5.4 | 1.5838 | 742 | 60.1(1.1) | 6.0(1.1) | 4732(1140) |
| CN | N= 1-0, J=3/2-1/2, F=5/2-3/2 | 113490.970(2e-3) | 5.4 | 4.205 | 6332 | 60.0(1.1) | 6.6(1.1) | 44322 (1140) |
| CN | N= 1-0, J=3/2-1/2, F=1/2-1/2 | 113499.644(3e-3) | 5.4 | 1.2491 | 1485 | 60.0(1.0) | 5.9(1.1) | 9304(1140) |
| CN | N= 1-0, J=3/2-1/2, F=3/2-3/2 | 113508.907(3e-3) | 5.4 | 1.2196 | 1932 | 60.1(1.1) | 6.1(1.1) | 12525(1140) |
| CN | N= 1-0, J=3/2-1/2, F=1/2-3/2 | 113520.432(4e-3) | 5.4 | 0.15263 | 212 | 60.0(1.1) | 7.8(1.1) | 1768(1140) |
| | | | G049.48−00.38 | | | | | |
| $SO_2$, $v_2$=1 | 10(1, 9) − 10(0, 10) | 105956.755(0) | 799.9 | 17.803 | 64 | 58.2(0.3) | 6.9(0.9) | 470(52) |
| $NH_2CHO$ | 5(2, 4) − 4(2, 3) | 105972.665(37e-3) | 27.2 | 54.915 | 340 | 57.0(0.1) | 9.3(0.2) | 3385(51) |
| $CH_3OCHO$ | 3(3, 1) − 2(2, 0) A | 105977.940(1e-2) | 9.5 | 1.13661 | 86 | 56.2(0.3) | 6.3(0.7) | 577(51) |
| $CH_3OCHO$ | 3(3, 1) − 2(2, 1) E | 106018.879(1e-2) | 9.5 | 0.96781 | 56 | 56.2(0.5) | 4.9(0.5) | 295(29) |
| $CH_3OCHO$ | 3(3, 0) − 2(2, 0) E | 106031.705(1e-2) | 9.5 | 0.96583 | 66 | 56.1(0.5) | 5.7(0.5) | 405(29) |
| $NH_2CHO$ | 5(4, 1) − 4(4, 0) | 106107.870(88e-3) | 63.0 | 23.537 | 249 | 57.1(0.5) | 9.3(0.5) | 2458)29) |
| $NH_2CHO$ | 5(4, 2) − 4(4, 1) | 106107.845(88e-3) | 63.0 | 23.537 | blended | – | – | – |
| $CH_3OCHO$ | 3(3, 0) − 2(2, 1) A | 106125.344(1e-2) | 9.5 | 1.13527 | 97 | 56.1(0.5) | 5.8(0.5) | 595(29) |
| $NH_2CHO$ | 5(3, 3) − 4(3, 2) | 106134.468(55e-3) | 42.1 | 41.845 | 240 | 57.0(0.5) | 9.3(0.5) | 2363(29) |
| $NH_2CHO$ | 5(3, 2) − 4(3, 1) | 106141.442(55e-3) | 42.1 | 41.84 | 261 | 57.0( 0.5) | 8.9(0.5) | 2471(29) |
| $CH_3COCH_3$ | 19(7, 12) − 19(6, 13) EE | 106273.673(22e-3) | 138.6 | 1012.2419 | 59 | 57.1(0.4) | 4.2(1.0) | 264(50) |
| $CH_3COCH_3$ | 19(8, 12) − 19(7, 13) EE | 106274.499(22e-3) | 138.6 | 1012.22624 | blended | – | – | – |
| CCS | 8(9) − 7(8) | 106347.726(2e-2) | 25.0 | 74.425 | 175 | 56.5(0.5) | 6.0(0.5) | 1126(18) |
| $CH_3COCH_3$ | 19(7, 12) − 19(6, 13) AA | 106390.849(26e-3) | 138.5 | 633.24693 | 30 | 57.0(0.5) | 5.1(0.5) | 161(18) |
| $CH_3COCH_3$ | 19(8, 12) − 19(7, 13) AA | 106391.693(26e-3) | 138.5 | 379.9848 | blended | – | – | – |
| $HC_5N$ | 40 − 39 | 106498.910(7e-3) | 104.8 | 2249.7 | 12 | 57.5(2.4) | 4.6(2.5) | 170(82) |
| $NH_2CHO$ | 5(2, 3) − 4(2, 2) | 106541.773(37e-3) | 27.2 | 54.915 | 296 | 57.1(0.2) | 7.7(0.5) | 2434(133) |
| $CH_3OCHO$ | 14(4, 11) − 14(3, 12) E | 106632.804(1e-2) | 72.9 | 3.49007 | 106 | 56.2(0.4) | 4.4(0.9) | 495(95) |
| $C_2H_3CN$ | 11(1, 10) − 10(1, 9) | 106641.383(1e-3) | 32.9 | 476.24 | 74 | 58.5(0.8) | 7.2(1.5) | 566(112) |
| $CH_3OCHO$ | 9(2, 8) − 8(2, 7) A | 106648.754(1e-2) | 216.4 | 22.53919 | 265 | 56.0(0.2) | 6.7(0.4) | 1903(110) |
| $CH_3OCHO$ | 14(4, 11) − 14(3, 12) A | 106668.134(1e-2) | 72.9 | 3.48762 | 102 | 56.0(0.5) | 5.9(1.0) | 644(101) |
| $C_2H_5OH$ | 6(1, 5) − 5(1, 4) | 106676.542(5e-2) | 76.1 | 9.325 | 79 | 57.2(0.9) | 9.3(1.7) | 790(128) |
| $C_2H_5OH$ | 9(2, 8) − 9(1, 9) | 106723.558(5e-2) | 42.7 | 7.9044 | 143 | 57.1(1.1) | 8.6(1.1) | 1312(213) |
| H$\alpha$ | H (39) $\alpha$ | 106737.357(0) | – | – | 509 | 59.4(0.5) | 26.9(0.5) | 14554(107) |
| $^{34}SO$ | 3(2) − 2(1) | 106743.244(7e-2) | 20.9 | 3.557 | 249 | 56.8(0.5) | 5.5(1.6) | 1454(434) |
| $C_2H_5OH$ | 6(1, 5) − 5(1, 4) | 106767.234(5e-2) | 80.7 | 9.6466 | 99 | 57.1(1.1) | 8.8(1.1) | 928(213) |
| $CH_3OCH_3$ | 9(1, 8) − 8(2, 7) AA | 106775.602(14e-3) | 43.4 | 36.603 | blended | – | – | – |
| $CH_3OCH_3$ | 9(1, 8) − 8(2, 7) EE | 106777.344(9e-3) | 43.4 | 58.573 | 382 | 55.4(0.2) | 13.8(0.5) | 5610(154) |
| $CH_3OCH_3$ | 9(1, 8) − 8(2, 7) EA | 106779.091(11e-3) | 43.4 | 21.963 | blended | – | – | – |
| $CH_3OCH_3$ | 9(1, 8) − 8(2, 7) AE | 106779.083(11e-3) | 43.4 | 14.645 | blended | – | – | – |
| $OC^{34}S$ | 9 − 8 | 106787.390(2e-3) | 25.6 | 4.601 | 323 | 56.6(0.9) | 7.8(2.4) | 2677(637) |
| $CH_3COCH_3$ | 18(6, 12) − 18(5, 13) EE | 106873.162(18e-3) | 121.8 | 877.18596 | 32 | 57.0(1.1) | 3.3(2.1) | 113(71) |
| $CH_3COCH_3$ | 18(7, 12) − 18(6, 13) EE | 106873.359(18e-3) | 121.8 | 877.18275 | blended | – | – | – |
| aGg'−$(CH_2OH)_2$ | 12(1, 12) v=0 − 11(1, 11) v=1 | 106907.385(2e-3) | 36.3 | 467.50155 | 12 | 56.0(2.9) | 3.8(2.7) | 59(33) |

**Table A2.** (Continued)

| Species | Transitions | Rest Freq. (MHz) | $E_u$ (K) | $\mu^2$S ($D^2$) | $T_{mb}$ (mK) | $V_{LSR}$ (km $s^{-1}$) | $\Delta$V (km $s^{-1}$) | $\int T_{mb}$ dv (mK km $s^{-1}$) |
|---|---|---|---|---|---|---|---|---|
| $HOCO^+$ | 5(0, 5) − 4(0, 4) | 106913.545(3e-3) | 15.4 | 36.454 | 32 | 55.3(1.2) | 3.5(1.9) | 119(71) |
| $C_2H_5OH$ | 19(2, 18) − 19(1, 18) | 106931.232(5e-2) | 222.5 | 25.014 | 50 | 57.0(0.8) | 4.0(1.3) | 215(80) |
| $CH_3COCH_3$ | 18(6, 12) − 18(5, 13) AA | 107006.295(22e-3) | 121.8 | 329.26249 | 22 | 57.1(0.5) | 3.9(0.5) | 92(30) |
| $CH_3COCH_3$ | 18(7, 12) − 18(6, 13) AA | 107006.496(22e-3) | 121.8 | 548.83353 | blended | – | – | – |
| $CH_3OH$, vt=0-2 | $3(1)^+ - 4(0)^+$, vt=0 | 107013.831(1e-2) | 28.3 | 12.036 | 3834 | 55.5(0.5) | 8.7(0.5) | 35527(300) |
| $CH_3OCHO$ | 9(2, 8) − 8(2, 7) | 107022.159(1e-2) | 215.7 | 22.64935 | 196 | 55.0(0.5) | 7.1(0.5) | 1472(300) |
| aGg'−$(CH_2OH)_2$ | 10(2, 9) v=1 − 9(2, 8) v=0 | 107040.005(2e-3) | 29.0 | 305.75751 | blended | – | – | – |
| $C_2H_5CN$ | 12(2, 11) − 11(2, 10) | 107043.527(5e-2) | 37.9 | 172.86 | 245 | 57.0(0.5) | 10.3(0.5) | 2675(300) |
| $SO_2$ | 27(3, 25) − 26(4, 22) | 107060.208(2e-3) | 369.4 | 8.2723 | 232 | 58.0(0.5) | 8.2(0.5) | 2024(300) |
| aGg'−$(CH_2OH)_2$ | 10(3, 7) v=1 − 9(3, 7) v=1 | 107073.219(1e-3) | 32.0 | 3.03815 | 44 | 55.1(0.5) | 3.6(0.5) | 169(30) |
| $CH_3OH$, vt=0-2 | 15(-2) − 15(1) E2, vt=0 | 107159906(14e-3) | 304.7 | 10.421 | 756 | 56.5(0.1) | 8.2(0.2) | 6566(124) |
| $^{13}CH_3CN$ | 6(3) − 5(3) | 107178.424(0) | 82.4 | 276.826 | 79 | 57.0(0.5) | 5.0(0.5) | 421(83) |
| $^{13}CH_3CN$ | 6(2) − 5(2) | 107188.500(1e-1) | 46.6 | 164.068 | 59 | 57.7(0.5) | 5.8(0.5) | 368(83) |
| $^{13}CH_3CN$ | 6(1) − 5(1) | 107194.550(1e-1) | 25.2 | 179.427 | 111 | 57.2(0.5) | 7.7(0.5) | 897(83) |
| $^{13}CH_3CN$ | 6(0) − 5(0) | 107196.570(1e-1) | 18.0 | 184.590 | blended | – | – | – |
| $HOCO^+$ | 5(1, 4) − 4(1, 3) | 107315.356(2e-3) | 52.8 | 34.996 | 36 | 55.2(0.6) | 1.8(1.8) | 68(52) |
| $CH_3COCH_3$ | 11(9, 3) − 10(10, 1) EE | 107371.058(62e-3) | 57.5 | 12.17983 | 51 | 57.0(0.6) | 3.3(1.1) | 179(62) |
| $C_2H_5OH$ | 23(2, 22) − 22(3, 19) | 107381.496(5e-2) | 232.9 | 1.1762 | 16 | 58.1(1.4) | 2.4(1.6) | 42(40) |
| $C_2H_5CN$ | 12(7, 5) − 11(7, 4) | 107485.160(5e-2) | 88.0 | 117.36 | 358 | 58.1(0.5) | 11.8(0.5) | 4504(83) |
| $C_2H_5CN$ | 12(6, 6) − 11(6, 5) | 107486.949(5e-2) | 73.6 | 133.42 | blended | – | – | – |
| $C_2H_5CN$ | 12(8, 4) − 11(8, 3) | 107491.574(5e-2) | 73.6 | 98.829 | 150 | 58.0(0.5) | 8.7(0.5) | 1393(83) |
| $C_2H_5CN$ | 12(5, 7) − 11(5, 6) | 107502.432(5e-2) | 104.6 | 146.99 | 364 | 58.0(0.5) | 9.8(0.5) | 3787(83) |
| $C_2H_5CN$ | 12(10, 2) − 11(10, 1) | 107519.861(5e-2) | 61.3 | 54.355 | 97 | 58.1(0.5) | 9.0(0.5) | 934(83) |
| $CH_3OCHO$ | 9( 2, 8) − 8( 2, 7) E | 107537.258(1e-2) | 28.8 | 22.60702 | 632 | 56.1(0.5) | 7.5(0.5) | 5078(83) |
| $CH_3OCHO$ | 9( 2, 8) − 8( 2, 7) A | 107543.711(1e-2) | 28.8 | 22.61344 | 763 | 56.2(0.5) | 8.0(0.5) | 6477(83) |
| $C_2H_5CN$ | 12(4, 9) − 11(4, 8) | 107544.042(5e-2) | 51.3 | 158.12 | blended | – | – | – |
| $C_2H_5CN$ | 12(4, 8) − 11(4, 7) | 107547.460(5e-2) | 51.3 | 158.11 | 184 | 58.0(0.5) | 8.5(0.5) | 1668(83) |
| $C_2H_5CN$ | 12(3, 10) − 11(3, 9) | 107594.056(5e-2) | 43.6 | 166.77 | 252 | 58.2(0.5) | 8.7(0.5) | 2319(83) |
| $CH_3OCHO$ | 23(6, 17) − 23(5, 18) E | 107604.366(1e-2) | 189.0 | 7.68978 | 97 | 56.0(0.5) | 10.1(0.5) | 1042(83) |
| $CH_3COCH_3$ | 16(4, 12) − 16(3, 13) AE | 107633.312(16e-3) | 90.9 | 75.21131 | 39 | 56.2(1.5) | 6.4(2.7) | 266(110) |
| $C_2H_5CN$ | 12(3, 9) − 11(3, 8) | 107734.723(5e-3) | 43.6 | 166.76 | 206 | 57.0(0.3) | 9.3(0.7) | 2051(140) |
| $CH_3COCH_3$ | 16(4, 12) − 16(3, 13) EE | 107797.721(13e-3) | 90.8 | 602.22608 | 37 | 57.1(0.7) | 2.8(0.7) | 39(29) |
| $SO_2$ | 12(4, 8) − 13(3, 11) | 107843.470(2e-3) | 111.0 | 4.5354 | 407 | 58.2(0.1) | 8.7(0.3) | 3780(123) |
| $CH_3OCHO$ | 15(5, 10) − 15(4, 11) E | 108045.959(1e-2) | 87.9 | 4.11041 | 69 | 56.1(0.7) | 3.5(1.3) | 259(94) |
| $CH_3OCHO$ | 15(5, 10) − 15(4, 11) A | 108050.939(1e-2) | 87.9 | 4.11748 | 74 | 56.0(0.7) | 4.0(1.2) | 312(100) |
| $CH_3OH$, vt=0-2 | 18(-1) − 19(-2) E2, vt=1 | 108058.877(31e-3) | 809.1 | 10.162 | 72 | 55.6(0.6) | 2.9(1.1) | 222(86) |
| $OC^{33}S$ | 9 − 8 | 108084.784(2e-3) | 25.9 | 4.605 | 69 | 57.1(0.6) | 7.2(1.4) | 526(89) |
| t-HCOOH | 5(1, 5) − 4(1, 4) | 108126.720(3e-3) | 18.8 | 9.6966 | 208 | 57.0(0.3) | 7.1(0.6) | 1568(120) |
| $CH_3COCH_3$ | 15(3, 12) − 15(2,13) EE | 108147.056(13e-3) | 76.7 | 460.37793 | 24 | 57.0(1.7) | 3.3(2.5) | 86(78) |
| $CH_3COCH_3$ | 15(4, 12) − 15(3,13) EE | 108147.057(13e-3) | 76.7 | 460.37792 | blended | – | – | – |
| $C_2H_5CN$ | 11(1, 11) − 10(0, 10) | 108210.415(5e-3) | 28.6 | 11.009 | 26 | 58.2(0.7) | 2.4(1.5) | 65(34) |
| $CH_3COCH_3$ | 14(2, 12) − 14(1, 13) AE | 108240.911(21e-3) | 63.4 | 39.19411 | 26 | 56.8(0.7) | 2.8(1.6) | 77(37) |
| $CH_3COCH_3$ | 14(2, 12) − 14(1, 13) EA | 108241.031(16e-3) | 63.4 | 78.40068 | blended | – | – | – |
| $CH_3COCH_3$ | 7(4, 3) − 7(1, 6) AA | 108331.398(21e-3) | 22.6 | 0.51266 | 42 | 57.1(0.4) | 5.9(1.1) | 261(42) |
| $CH_3COCH_3$ | 8(3, 5) − 7(4, 4) EA | 108358.421(11e-3) | 26.9 | 130.21505 | 29 | 57.0(1.0) | 10.6(2.6) | 326(64) |
| $CH_3COCH_3$ | 8(3, 5) − 7(4, 4) EE | 108387.595(8e-3) | 88.2 | 519.86714 | 67 | 57.0(0.7) | 15.5(1.6) | 1311(94) |
| $CH_3COCH_3$ | 8(3, 5) − 7(4, 4) AA | 108424.565(11e-3) | 26.7 | 194.60833 | 45 | 56.9(0.5) | 11.8(0.5) | 574(21) |
| $CH_3COCH_3$ | 14(2, 12) − 14(1, 13) EE | 108434.511(16e-3) | 63.4 | 313.86255 | 24 | 56.8(0.5) | 7.1(0.5) | 179(21) |
| $C_2H_5OH$ | 13(3, 10) − 13(2, 11) | 108438.579(5e-2) | 88.2 | 18.79 | 175 | 56.9(0.5) | 10.5(0.5) | 1967(21) |
| $CH_3COCH_3$ | 13(1, 12) − 13(0, 13) AE | 108461.338(27e-3) | 51.0 | 60.36275 | 29 | 57.1(0.5) | 1.8(0.5) | 56(21) |
| $CH_3COCH_3$ | 13(2, 12) − 13(1, 13) EA | 108461.496(19e-3) | 51.0 | 40.24091 | blended | – | – | – |
| $C_2H_5OH$ | 16(2, 15) − 15(3, 12) | 108524.526(5e-2) | 118.2 | 2.9899 | 18 | 57.0(0.9) | 7.2(1.5) | 37(30) |
| $CH_3OCHO$ | 22(4, 18) − 22(4, 19) E | 108539.641(1e-2) | 165.3 | 2.33438 | 44 | 56.0(0.4) | 1.1(0.3) | 65(52) |
| $CH_3OCHO$ | 22(4, 18) − 22(4, 19) A | 108616.604(1e-2) | 165.3 | 2.33534 | 43 | 56.1(0.7) | 6.6(2.1) | 303(66) |
| $C_2H_5OH$ | 8(2, 6) − 7(1, 6) | 108624.353(5e-2) | 91.9 | 4.7078 | 118 | 57.0(0.3) | 9.8(0.7) | 1227(70) |
| $CH_3COCH_3$ | 14(2, 12) − 14(1, 13) AA | 108627.774(18e-3) | 63.3 | 117.8051 | 35 | 57.0(0.8) | 4.8(2.2) | 180(63) |
| $^{13}CN$ | 1(1, 1) − 0(1, 0), F = 1 − 1 | 108636.923(5e-2) | 5.2 | 1.932 | 88 | 55.3(0.3) | 7.9(0.7) | 732(60) |
| $^{13}CN$ | 1(2, 1) − 0(1, 1), F = 1 − 0 | 108638.212(5e-2) | 5.2 | 0.722 | blended | – | – | – |
| $^{13}CN$ | 1(2, 1) − 0(1, 1), F = 2 − 1 | 108643.590(5e-2) | 5.2 | 0.856 | 101 | 55.1(0.3) | 8.5(0.7) | 912(63) |
| $^{13}CN$ | 1(2, 1) − 0(1, 1), F = 0 − 1 | 108644.346(5e-2) | 5.2 | 0.642 | blended | – | – | – |
| $^{13}CN$ | 1(2, 1) − 0(1, 1), F = 1 − 1 | 108645.064(5e-2) | 5.2 | 0.551 | blended | – | – | – |
| $^{13}CN$ | 1(1, 1) − 0(1, 0), F = 2 − 1 | 108651.297(5e-2) | 5.2 | 3.276 | 110 | 55.9(0.2) | 6.7(0.5) | 780(52) |
| $^{13}CN$ | 1(2, 1) − 0(1, 1), F = 2 − 2 | 108657.646(5e-2) | 5.2 | 2.420 | 105 | 55.1(0.3) | 9.1(0.7) | 1018(65) |
| $^{13}CN$ | 1(2, 1) − 0(1, 1), F = 1 − 2 | 108658.948(5e-2) | 5.2 | 0.669 | blended | – | – | – |
| $CH_3COCH_3$ | 13(1, 12) − 13(0, 13) EE | 108668.617(20e-3) | 50.9 | 161.12614 | 22 | 57.1(1.0) | 5.3(2.0) | 123(47) |
| $^{13}CN$ | 1(2, 2) − 0(1, 1), F = 3 − 2 | 108780.201(5e-2) | 5.2 | 4.905 | 21 | 54.6(0.7) | 2.2(1.4) | 47(25) |
| $^{13}CN$ | 1(2, 2) − 0(1, 1), F = 2 − 1 | 108782.374(5e-2) | 5.2 | 2.586 | 181 | 54.5(0.1) | 9.7(0.3) | 1878(50) |
| $^{13}CN$ | 1(2, 2) − 0(1, 1), F = 1 − 0 | 108786.982(5e-2) | 5.2 | 1.144 | 44 | 54.8(0.2) | 1.3(0.6) | 59(21) |
| $^{13}CN$ | 1(2, 2) − 0(1, 1), F = 1 − 1 | 108793.753(5e-2) | 5.2 | 0.894 | 92 | 54.8(0.3) | 6.3(0.7) | 620(72) |
| $^{13}CN$ | 1(2, 2) − 0(1, 1), F = 2 − 2 | 108796.400(5e-2) | 5.2 | 0.918 | 48 | 54.6(0.8) | 8.9(1.4) | 450(74) |
| $CH_3OCHO$ | 14(3, 12) − 14(2, 13) E | 108834.930(1e-2) | 67.8 | 2.6613 | 110 | 56.0(0.3) | 7.3(0.6) | 853(50) |
| $CH_3OCHO$ | 14(3, 12) − 14(2, 13) A | 108883.567(1e-2) | 67.8 | 2.6588 | 95 | 55.9(0.3) | 6.7(0.5) | 681(48) |
| $CH_3OH$, vt=0-2 | 0(0) − 1(-1) E2, vt=0 | 108893.945(12e-3) | 13.1 | 3.9134 | 3659 | 56.5(0.1) | 8.3(0.1) | 3659 |
| SiS | 6(0) − 5(0) | 108924.301(1e-3) | 18.3 | 5.62 | 25 | 58.0(2.9) | 8.6(4.7) | 229(137) |
| $C_2H_5CN$ | 12(2, 10) − 11(2, 9) | 108940.554(5e-2) | 38.2 | 172.93 | 271 | 57.8(0.3) | 9.6(0.6) | 2773(158) |
| $C_2H_5CN$ | 11(3, 9) − 12(0, 12) | 108940.696(4e-3) | 38.4 | 0.042598 | blended | – | – | – |
| $O^{13}CS$ | 9 − 8 | 109110.845(2e-3) | 26.2 | 4.605 | 148 | 56.2(0.5) | 6.3(0.5) | 995(430) |
| $CH_3OH$, vt=0-2 | 14(5) − 15(4) E1, vt=0 | 109138.783(15e-3) | 379.7 | 13.593 | 886 | 56.6(1.1) | 9.7(1.1) | 9120(863) |
| $CH_3OH$, vt=0-2 | 16(-2) − 16(1) E2, vt=0 | 109153.184 (14e-3) | 342.0 | 14.726 | 865 | 56.5(1.1) | 8.1(1.1) | 8366(863) |
| $HC_5N$ | 41 − 40 | 109160.973(7e-3) | 110.0 | 2306 | 276 | 57.5(1.1) | 7.2(1.1) | 2117(863) |
| $HC_3N$ | 12 − 11 | 109173.634(1e-2) | 34.1 | 167.1 | 5955 | 56.2(1.1) | 8.4(1.1) | 53000(863) |
| SO | 3(2) − 2(1) | 109252.220(1e-4) | 21.1 | 3.5585 | 4353 | 58.0(1.1) | 8.7(1.1) | 40288(718) |
| $CH_3OCHO$ | 10(1, 9) − 9(2, 8) E | 109292.214(1e-2) | 34.0 | 2.15335 | 62 | 56.0(1.1) | 8.2(1.1) | 541(18) |
| aGg'−$(CH_2OH)_2$ | 10(6, 4) v=1 − 9(6, 3) v=0 | 109357.858(2e-3) | 45.1 | 246.16859 | 64 | 56.2(0.8) | 6.9(1.5) | 471(105) |
| aGg'−$(CH_2OH)_2$ | 10(6, 5) v=1 − 9(6, 4) v=0 | 109357.707(2e-3) | 45.1 | 191.44051 | blended | – | – | – |
| $CH_3OCHO$ | 21(5, 17) − 20(6, 14) E | 109369.294(1e-2) | 154.1 | 1.05667 | 41 | 56.0(0.4) | 4.7(1.1) | 46(43) |
| $CH_3OCHO$ | 9(8, 1) − 8(8, 0) | 109390.436(1e-2) | 257.0 | 5.03021 | 22 | 56.1(1.9) | 4.1(3.2) | 95(77) |
| $C_2H_5OH$ | 19(4, 15) − 18(5, 14) | 109394.865(5e-2) | 180.5 | 5.6423 | 18 | 57.1(2.2) | 3.7(3.1) | 74(72) |
| $HC_3N$, $v_7$=1 | 12(-1) − 11(1) | 109442.013(2e-2) | 355.0 | 165.12 | 305 | 59.6(1.1)) | 13.7(1.1) | 4457(463) |
| OCS | 9 − 8 | 109463.063(5e-3) | 26.3 | 4.6034 | 2656 | 56.5(1.1) | 8.8(1.1) | 24918(463) |
| HNCO | 5(1, 5) − 4(1, 4) | 109495.996(6e-3) | 59.0 | 11.847 | 477 | 57.0(1.1) | 9.4(1.1) | 4770(463) |
| $CH_3OCH_3$ | 8(2, 7) − 8(1, 8) EA | 109571.396(9e-3) | 38.3 | 23.947 | 300 | 56.0(1.1) | 6.3(1.1) | 2019(113) |
| $CH_3OCH_3$ | 8(2, 7) − 8(1, 8) AE | 109571.403(9e-3) | 38.3 | 35.921 | blended | – | – | – |
| $CH_3OCH_3$ | 8(2, 7) − 8(1, 8) EE | 109574.088(7e-3) | 38.3 | 95.791 | 391 | 56.0(1.1) | 5.7(1.1) | 2381(113) |
| $CH_3OCH_3$ | 8(2, 7) − 8(1, 8) AA | 109576.778(11e-3) | 38.3 | 59.869 | 257 | 56.1(1.1) | 5.3(1.1) | 1447(113) |
| $HC_3N$, $v_7$=1 | 12(1) − 11(-1) | 109598.818(2e-2) | 355.0 | 165.12 | 304 | 59.7(1.1) | 10.4(1.1) | 3368(113) |
| $C_2H_5CN$ | 12(1, 11) − 11(1, 10) | 109650.263(5e-2) | 35.4 | 176.49 | 235 | 58.0(0.3) | 8.7(0.6) | 2179(128) |
| $CH_3OCHO$ | 9(6, 3) − 8(6, 2) | 109662.944(1e-2) | 238.1 | 13.32847 | 74 | 56.0(0.6) | 4.8(1.2) | 383(94) |
| aGg'−$(CH_2OH)_2$ | 5(3, 3) v=1 − 4(2, 3) v=0 | 109683.440(2e-3) | 12.1 | 6.02253 | 20 | 56.1(4.3) | 8.2(6.6) | 143(126) |
| $NH_2CHO$ | 5(1, 4) − 4(1, 3) | 109753.549(25e-3) | 18.8 | 62.756 | 403 | 57.0(1.1) | 10.8(1.1) | 4631(881) |
| $SO_2$ | 17(5, 13) − 18(4, 14) | 109757.585(2e-3) | 202.1 | 6.6069 | 243 | 58.0(1.1) | 7.4(1.1) | 1906(881) |

**Table A2.** (Continued)

| Species | Transitions | Rest Freq. | $E_u$ | $\mu^2S$ | $T_{mb}$ | $V_{LSR}$ | $\Delta V$ | $\int T_{mb}$ dv |
|---|---|---|---|---|---|---|---|---|
| | | (MHz) | (K) | ($D^2$) | (mK) | (km $s^{-1}$) | (km $s^{-1}$) | (mK km $s^{-1}$) |
| $CH_3OCHO$ | 9(3, 7) − 8(3, 6) | 109763.737(1e-2) | 220.2 | 21.17892 | 116 | 56.1(1.1) | 5.5(1.1) | 685(440) |
| $CH_3OCHO$ | 9(5, 5) − 8(5, 4) | 109770.995(1e-2) | 230.8 | 16.50962 | 202 | 56.0(1.1) | 2.9(1.1) | 617(332) |
| $CH_3OCHO$ | 9(5, 4) − 8(5, 3) | 109778.835(1e-2) | 230.8 | 16.51108 | blended | − | − | − |
| $C^{18}O$ | 1 − 0 | 109782.173(6e-3) | 5.3 | 0.01221 | 5832 | 57.0(1.1) | 6.9(1.1) | 43108(881) |
| HNCO | 5(3, 2) − 4(3, 1) | 109833.487(7e-3) | 390.8 | 7.1906 | 81 | 57.0(1.0) | 2.7(2.5) | 232(213) |
| HNCO | 5(2, 3) − 4(2, 2) | 109872.765(3e-2) | 186.1 | 10.012 | 323 | 57.1(0.5) | 7.8(1.0) | 2730(362) |
| HNCO | 5(2, 4) − 4(2, 3) | 109872.337(3e-2) | 186.1 | 10.013 | blended | − | − | − |
| HNCO | 5(0, 5) − 4(0, 4) | 109905.749(7e-3) | 15.8 | 12.482 | 1408 | 57.0(0.1) | 8.7(0.3) | 13042(403) |
| $CH_3OCHO$ | 9(4, 6) − 8(4, 5) A | 110035.269(1e-2) | 224.9 | 19.15168 | 137 | 56.0(0.4) | 4.8(0.8) | 697(118) |
| $CH_3OCHO$ | 9(6, 4) − 8(6, 3), E | 110050.332(1e-2) | 237.4 | 13.33458 | 103 | 56.1(0.6) | 4.8(1.2) | 523(121) |
| $^{13}CO$ | 1 − 0 | 110201.35(0) | 5.3 | 0.01220 | 33635 | 57.3(0.1) | 8.0(0.1) | 286900(174) |
| $CH_3OCHO$ | 10(0, 10) − 9(1, 9) E | 110224.567(1e-2) | 30.2 | 3.83574 | 217 | 56.0(0.3) | 5.7(0.7) | 1326(159) |
| $CH_3OCHO$ | 10(0, 10) − 9(1, 9) A | 110226.855(1e-2) | 30.2 | 3.83269 | 209 | 56.1(0.2) | 5.9(0.8) | 1307(175) |
| $CH_3OCHO$ | 10(1, 10) − 9(1, 9) E | 110238.713(1e-2) | 217.2 | 26.23975 | 215 | 56.0(0.2) | 6.0(0.5) | 1367(97) |
| $CH_3OCHO$ | 9(4, 5) − 8(4, 4) A | 110250.337(1e-2) | 224.9 | 19.15261 | 194 | 56.0(0.3) | 7.4(0.5) | 1531(105) |
| $CH_3OCHO$ | 9(5, 5) − 8(5, 4) E | 110262.642(1e-2) | 230.0 | 16.57884 | 129 | 56.1(0.3) | 5.4(0.7) | 745(90) |
| HNCO | 5(1, 4) − 4(1, 3) | 110298.089(5e-3) | 59.2 | 11.847 | 495 | 57.0(0.1) | 10.9(0.3) | 5760(135) |
| $CH_3{}^{13}CN$ | 6(4) − 5(4) | 110295.019(0.) | 132.8 | 102.537 | blended | − | − | − |
| $CH_3{}^{13}CN$ | 6(3) − 5(3) | 110309.800(1e-1) | 82.8 | 276.874 | 97 | 55.7(0.5) | 5.5(0.5) | 568(412) |
| $CH_3{}^{13}CN$ | 6(2) − 5(2) | 110320.400(1e-1) | 47.1 | 164.054 | 82 | 55.6(0.5) | 5.3(0.5) | 466(412) |
| $CH_3{}^{13}CN$ | 6(1) − 5(1) | 110326.770(1e-1) | 25.7 | 179.434 | 457 | 55.6(0.5) | 7.4(0.5) | 6644(412) |
| $CH_3{}^{13}CN$ | 6(0) − 5(0) | 110328.870(1e-1) | 18.5 | 184.563 | blended | − | − | − |
| $CH_3CN$ | 6(5, 0) − 5(5, 0) | 110330.345(0) | 197.1 | 56.399 | blended | − | − | − |
| $CH_3CN$ | 6(4, 0) − 5(4, 0) | 110349.471(0) | 132.8 | 102.54 | 900 | 56.0(0.5) | 9.7(0.5) | 9334(412) |
| $CH_3CN$ | 6(3, 0) − 5(-3, 0) | 110364.354(0) | 82.8 | 138.45 | 2069 | 56.1(0.5) | 9.7(0.5) | 21388(412) |
| $CH_3CN$ | 6(-3, 0) − 5(3, 0) | 110364.354(0) | 82.8 | 138.45 | blended | − | − | − |
| $CH_3CN$ | 6(2, 0) − 5(2, 0) | 110374.989(0) | 47.1 | 164.06 | 1970 | 56.1(0.5) | 9.6(0.5) | 20220(412) |
| $CH_3CN$ | 6(1, 0) − 5(1, 0) | 110381.372(0) | 25.7 | 179.45 | 2143 | 56.0(0.5) | 10.0(0.5) | 22879(412) |
| $CH_3CN$ | 6(0, 0) − 5(0, 0) | 110383.500(0) | 18.5 | 184.58 | 2317 | 56.0(0.4) | 9.5(0.5) | 23314(412) |
| $CH_3OCHO$ | 9(8, 1) − 8(8, 0) E | 110447.180(1e-2) | 69.0 | 5.02983 | 162 | 56.0(0.3) | 5.6(0.6) | 957(100) |
| $C_2H_5OH$ | 21(3, 18) − 21(2, 19) | 110452.276(5e-2) | 208.7 | 35.016 | 125 | 57.0(0.2) | 5.3(2.4) | 1502(294) |
| $CH_3OCHO$ | 9(8, 1) − 8(8, 0) A | 110455.372(1e-2) | 69.0 | 5.02998 | 301 | 56.0(0.2) | 5.3(0.8) | 1690(318) |
| $CH_3OCHO$ | 9(8, 2) − 8(8, 1) E | 110458.014(1e-2) | 69.0 | 5.02965 | 180 | 56.1(0.4) | 5.3(0.9) | 1023(168) |
| $CH_3OCHO$ | 9(7, 2) − 8(7, 1) E | 110525.741(1e-2) | 59.1 | 9.46492 | 307 | 56.0(0.5) | 6.5(0.5) | 2135(64) |
| $CH_3OCHO$ | 7(2, 6) − 6(1, 5) | 110526.190(1e-2) | 206.7 | 1.41631 | blended | − | − | − |
| $CH_3OCHO$ | 9(7, 2) − 8(7, 1) A | 110535.186(1e-2) | 59.1 | 9.561 | 632 | 56.0(0.5) | 7.7(0.5) | 5185(64) |
| $CH_3OCHO$ | 9(7, 3) − 8(7, 2) E | 110536.003(1e-2) | 59.1 | 9.46692 | blended | − | − | − |
| $C_2H_5OH$ | 7(2, 6) − 6(1, 6) | 110545.866(5e-2) | 84.9 | 1.3914 | 65 | 56.1(0.5) | 3.7(0.5) | 256(64) |
| $CH_3OCHO$ | 9(2, 6) − 8(1, 5) E | 110550.203(1e-2) | 19.0 | 1.39763 | 72 | 56.0(0.4) | 3.3(0.5) | 255(64) |
| $CH_3OCHO$ | 9(2, 6) − 8(1, 5) A | 110560.051(1e-2) | 19.0 | 1.39665 | 76 | 56.0(0.5) | 2.6(0.5) | 212(64) |
| $CH_3OCHO$ | 10(0,10) − 9(0, 9) A | 110571.632(1e-2) | 217.9 | 26.10484 | 206 | 56.0(0.3) | 5.5(0.5) | 1199(64) |
| $CH_3CN$, $v_8$=1 | 6(-1, 3) − 5(1, 3) | 110609.594(6e-2) | 537.6 | 177.77 | 173 | 58.0(0.8) | 8.2(1.6) | 1521(282) |
| $CH_3OCHO$ | 9(6, 3) − 8(6, 2) E | 110652.813(1e-2) | 50.5 | 13.30853 | 382 | 56.0(0.4) | 10.8(1.0) | 4413(337) |
| $CH_3OCHO$ | 9(6, 4) − 8(6, 3) E | 110662.315(1e-2) | 50.4 | 13.308555 | 796 | 56.0(0.2) | 9.1(0.4) | 7730(308) |
| $CH_3OCHO$ | 9(6, 3) − 8(6, 2) A | 110663.429(1e-2) | 50.4 | 13.31127 | blended | − | − | − |
| $CH_3OCHO$ | 9(6, 4) − 8(6, 3) A | 110663.273(1e-2) | 50.4 | 13.3113 | blended | − | − | − |
| $CH_3CN$, $v_8$=1 | 6(3, 1) − 5(3, 1) | 110680.294(7e-3) | 647.9 | 128.72357 | 101 | 58.1(3.3) | 10.2(5.7) | 2271(631) |
| $CH_3CN$ $v_8$=1 | 6(3, 2) − 5(3, 2) | 110683.963(1e-3) | 655.7 | 55.87 | blended | − | − | − |
| $CH_3OCHO$ | 9(4, 6) − 8(4, 5) E | 110684.123(1e-2) | 224.1 | 19.21258 | 188 | 56.0(0.5) | 5.3(1.8) | 1057(428) |
| $CH_3CN$, $v_8$=1 | 6(2, 1) − 5(2, 1) | 110695.473(7e-3) | 598.9 | 305.1398 | 214 | 58.0(0.5) | 14.9(0.5) | 3404(89) |
| $CH_3CN$, $v_8$=1 | 6(4, 2) − 5(4, 2) | 110698.717(8e-3) | 604.7 | 190.69518 | 175 | 58.0(0.3) | 14.6(0.5) | 2713(89) |
| $CH_3CN$, $v_8$=1 | 6(1, 1) − 5(1, 1) | 110706.243(7e-3) | 564.2 | 166.85665 | 255 | 58.0(0.5) | 9.3(0.5) | 2512(89) |
| $CH_3CN$, $v_8$=1 | 6(3, 3) − 5(3, 3) | 110709.3541(e-3) | 568.1 | 137.14 | 153 | 57.8(0.5) | 6.0(0.5) | 985(89) |
| $CH_3CN$, $v_8$=1 | 6(0, 1) − 5(0, 1) | 110712.176(7e-3) | 543.8 | 171.63268 | 192 | 58.0(0.4) | 8.8(0.5) | 1800(89) |
| $CH_3CN$, $v_8$=1 | 6(2, 2) − 5(2, 2) | 110716.257(6e-3) | 545.7 | 152.57534 | 176 | 58.1(0.5) | 9.6(0.5) | 1794(89) |
| $CH_3OCHO$ | 9(1, 8) − 8(1, 7) A | 110776.499(1e-2) | 215.7 | 23.1436 | 190 | 56.1(0.5) | 6.3(0.5) | 1277(89) |
| $CH_3OCHO$ | 10(1, 10) − 9(1, 9) E | 110788.664(1e-2) | 30.3 | 26.16584 | 954 | 56.0(0.4) | 10.5(0.5) | 10682(89) |
| $CH_3OCHO$ | 10(1, 10) − 9(1, 9) A | 110790.526(1e-2) | 30.3 | 26.17539 | blended | − | − | − |
| $CH_3CN$, $v_8$=1 | 6(1, 2) − 5(-1, 2) | 110823.116(6e-3) | 537.6 | 166.88912 | 147 | 58.0(0.2) | 8.6(0.6) | 1350(100) |
| $C_2H_3CN$ | 12(1, 12) − 11(1, 11) | 110839.968(1e-3) | 36.8 | 520.3 | 87 | 58.5(0.5) | 7.5(1.0) | 695(90) |
| $CH_3OCHO$ | 9(5, 4) − 8(5, 3) E | 110873.955(1e-2) | 43.2 | 16.55557 | 464 | 56.0(0.1) | 6.3(0.2) | 3127(90) |
| $CH_3OCHO$ | 9(3, 7) − 8(3, 6) E | 110879.766(1e-2) | 32.6 | 21.245 | 89 | 55.7(0.1) | 11.4(0.2) | 10768(120) |
| $CH_3OCHO$ | 9(5, 5) − 8(5, 4) A | 110880.447(1e-2) | 43.2 | 16.56015 | blended | − | − | − |
| $CH_3OCHO$ | 9(5, 5) − 8(5, 4) E | 110882.331(1e-2) | 43.2 | 16.55225 | blended | − | − | − |
| $CH_3OCHO$ | 9(3, 7) − 8(3, 6) A | 110887.092(1e-2) | 32.6 | 21.25577 | 601 | 56.1(0.1) | 8.0(0.3) | 5147(173) |
| $CH_3OCHO$ | 9(5, 4) − 8(5, 3) A | 110890.256(1e-2) | 43.2 | 16.56106 | 467 | 56.0(0.1) | 5.7(0.3) | 1830(149) |
| $CH_3OCHO$ | 9(4, 6) − 8(4, 5) E | 110918.768(1e-2) | 37.2 | 1.02704 | 119 | 56.0(0.4) | 5.4(1.0) | 679(104) |
| $C_2H_5OH$ | 15(8, 8) − 16(7, 9) | 110931.121(5e-2) | 181.8 | 2.4208 | 78 | 57.0(0.7) | 5.8(1.4) | 482(106) |
| $CH_3COOH$, vt=0 | 9(1, 8) A1 − 8(2, 7) A2 | 110954.111(1e-3) | 29.3 | 15.70004 | 52 | 58.0(1.2) | 8.6(2.9) | 470(133) |
| $CH_3COOH$, vt=0 | 9(2, 8) A1 − 8(2, 7) A2 | 110954.171(1e-3) | 29.3 | 5.68984 | blended | − | − | − |
| $CH_3COOH$, vt=0 | 9(1, 8) A1 − 8(1, 7) A2 | 110954.555(1e-3) | 29.3 | 5.6898 | blended | − | − | − |
| $CH_3COOH$, vt=0 | 9(2, 8) A1 − 8(1, 7) A2 | 110954.615(1e-3) | 29.3 | 15.6999 | blended | − | − | − |
| $CH_3OCHO$ | 15(4, 12) − 15(3, 13) A | 110962.153(1e-2) | 81.8 | 3.66282 | 142 | 56.0(0.4) | 5.6(0.8) | 853(108) |
| $CH_3COCH_3$ | 8(4, 4) − 7(5, 3) EE | 110987.131(16e-3) | 28.5 | 273.48458 | 48 | 57.0(1.1) | 6.3(2.0) | 326(105) |
| $CH_3OCHO$ | 9(3, 7) − 8(3, 6) E | 111005.672(1e-2) | 219.5 | 21.245 | 208 | 56.0(0.2) | 8.2(0.4) | 1809(80) |
| $CH_3COCH_3$ | 6(4, 3) − 5( 3, 3) EA | 111067.701(9e-3) | 17.0 | 0.36744 | 54 | 57.1(0.6) | 5.5(1.5) | 313(67) |
| $CH_3OCHO$ | 9(1, 8) − 8(1, 7) | 111094.124(1e-2) | 215.0 | 23.2438 | 208 | 56.2(0.2) | 6.9(0.4) | 1522(72) |
| $CH_3OCHO$ | 10(0, 10) − 9(0, 9) E | 111169.903(1e-2) | 30.2 | 26.18776 | blended | − | − | − |
| $CH_3OCHO$ | 10(0, 10) − 9(0, 9) A | 111171.634(1e-2) | 30.2 | 26.19136 | 1014 | 56.1(0.5) | 10.6(0.5) | 11432(167) |
| $CH_3OCHO$ | 9(4, 6) − 8(4, 5) A | 111195.962(1e-2) | 37.2 | 19.21722 | 586 | 56.0(0.4) | 8.3(0.5) | 5177(167) |
| $CH_3OCHO$ | 9(4, 6) − 8(4, 5) E | 111223.491(1e-2) | 37.2 | 18.18412 | 584 | 56.0(0.5) | 7.7(0.5) | 4796(167) |
| $CH_3COCH_3$ | 10(1, 9) − 9(2, 8) AE | 111243.339(11e-3) | 32.2 | 141.0573 | 144 | 57.0(0.5) | 10.5(0.5) | 1613(167) |
| $CH_3COCH_3$ | 10(2, 9) − 9(1, 8) AE | 111243.388(11e-3) | 32.2 | 423.15082 | blended | − | − | − |
| $CH_3COCH_3$ | 10(1, 9) − 9(2, 8) EA | 111243.424(1e-2) | 32.2 | 282.09469 | blended | − | − | − |
| $CH_3COCH_3$ | 10(2, 9) − 9(1, 8) EA | 111243.472(1e-2) | 32.2 | 282.09445 | blended | − | − | − |
| $CH_3COCH_3$ | 10(1, 9) − 9(2, 8) EE | 111267.514(8e-3) | 32.1 | 1128.14194 | 189 | 57.0(0.5) | 8.4(0.5) | 1699(167) |
| $CH_3COCH_3$ | 10(2, 9) − 9(1, 8) EE | 111267.565(8e-3) | 32.1 | 1128.14091 | blended | − | − | − |
| $C_2H_5OH$ | 17(3, 15) − 16(4, 12) | 111287163(5e-2) | 140.0 | 4.9131 | blended | − | − | − |
| $CH_3OH$, vt=0-2 | $7(2)^+ - 8(1)^+$, vt=0 | 111289.453(13e-3) | 102.7 | 9.3425 | 1767 | 56.5(0.5) | 10.3(0.5) | 19307(167) |
| $CH_3COCH_3$ | 10(1, 9) − 9(2, 8) AA | 111291.573(12e-3) | 32.0 | 422.99289 | blended | − | − | − |
| $CH_3COCH_3$ | 10(2, 9) − 9(1, 8) AA | 111291.626(12e-3) | 32.0 | 704.90836 | blended | − | − | − |
| $CH_3OCHO$ | 13(1, 12) − 13(1, 13) E | 111322.939(1e-2) | 54.6 | 0.76596 | 57 | 56.0(1.8) | 4.4(3.4) | 262(205) |
| $C_2H_5OH$ | 7(1, 7) − 7(0, 7) | 111344.327(5e-2) | 85.3 | 9.6676 | 142 | 57.2(1.1) | 9.9(2.6) | 1492(330) |
| $CH_3OCHO$ | 13(1, 12) − 13(1, 13) A | 111383.495(1e-2) | 54.6 | 0.76649 | 57 | 56.1(2.3) | 9.5(9.0) | 1158(478) |
| $CH_3OCHO$ | 9(4, 5) − 8(4, 4) E | 111408.412(1e-2) | 37.3 | 18.18767 | 551 | 56.0(0.5) | 7.9(0.5) | 4609(65) |
| $CH_3OCHO$ | 13(1, 12) − 13(0, 13) E | 111431.973(1e-2) | 54.6 | 1.37515 | 82 | 56.0(0.4) | 5.9(0.5) | 520(65) |
| $CH_3OCHO$ | 9(4, 5) − 8(4, 4) A | 111453.300(1e-2) | 37.2 | 19.21778 | 66 | 56.0(0.5) | 4.9(0.5) | 343(65) |
| $CH_3OCHO$ | 13(1, 12) − 13(0, 13) A | 111492.386(1e-2) | 54.6 | 1.37358 | 599 | 56.2(0.5) | 7.5(0.5) | 4802(65) |
| $CH_3COOH$, vt=0 | 10(0, 10) − 9(1, 9) E | 111507.280(1e-3) | 31.0 | 20.80201 | 52 | 58.2(0.7) | 7.8(1.7) | 429(74) |
| $CH_3COOH$, vt=0 | 10(0, 10) A1 − 9(1, 9) A2 | 111548.535(1e-3) | 30.5 | 20.40186 | 34 | 58.1(1.0) | 8.8(1.8) | 320(69) |
| $CH_3COOH$, vt=0 | 10(0, 10) A1 − 9(0, 9) A2 | 111548.536(1e-3) | 30.5 | 6.98023 | blended | − | − | − |
| $CH_3OH$, vt=0-2 | 17(-2) − 17(1) E2, vt=0 | 111626.514(15e-3) | 381.5 | 20.231 | 941 | 56.5(0.1) | 9.8(0.2) | 9793(208) |
| $CH_3OCHO$ | 9(1, 8) − 8(1, 7) E | 111674.131(1e-2) | 28.1 | 23.18984 | 743 | 56.0(0.1) | 8.1(0.3) | 6380(199) |

**Table A2.** (Continued)

| Species | Transitions | Rest Freq. (MHz) | $E_u$ (K) | $\mu^2 S$ ($D^2$) | $T_{mb}$ (mK) | $V_{LSR}$ (km $s^{-1}$) | $\Delta V$ (km $s^{-1}$) | $\int T_{mb}$ dv (mK km $s^{-1}$) |
|---|---|---|---|---|---|---|---|---|
| $CH_3OCHO$ | 9(1, 8) − 8(1, 7) A | 111682.189(1e-2) | 28.1 | 23.19587 | 722 | 56.0(0.1) | 8.3(0.3) | 6359(192) |
| $CH_3OCHO$ | 9(4, 5) − 8(4, 5) E | 111713.138(14-2) | 37.3 | 1.02682 | 91 | 56.1(1.1) | 8.7(1.1) | 844(241) |
| $CH_3OCHO$ | 10(1, 10) − 9(0, 9) A | 111735.307(1e-2) | 30.3 | 3.84224 | 327 | 56.0(1.1) | 9.9(1.1) | 3445(241) |
| $CH_3OCH_3$ | 19(3,16) − 19(2,17) AE | 111741.351(26e-3) | 187.5 | 123.39211 | blended | – | – | – |
| $CH_3OCH_3$ | 19(3,16) − 19(2,17) EE | 111742.794(25e-3) | 187.5 | 329.06069 | blended | – | – | – |
| $CH_3OCH_3$ | 19(3, 16) − 19(2, 17) AA | 111744.238(29e-3) | 187.5 | 205.6671 | 632 | 56.0(1.1) | 15.7(1.1) | 10586(241) |
| $CH_3OCH_3$ | 7(0, 7) − 6(1, 6) AA | 111782.562(8e-3) | 25.2 | 53.86755 | 1141 | 56.2(1.1) | 8.3(1.1) | 10078(241) |
| $CH_3OCH_3$ | 7(0, 7) − 6(1, 6) EE | 111783.010(4e-2) | 25.3 | 86.2034 | blended | – | – | – |
| $CH_3OCH_3$ | 7(0, 7) − 6(1, 6) EA | 111783.647(7e-3) | 25.3 | 21.54865 | blended | – | – | – |
| $CH_3OCH_3$ | 7(0, 7) − 6(1, 6) AE | 111783.648(7e-3) | 25.3 | 32.32363 | blended | – | – | – |
| $CH_3OCH_3$ | 7(5, 3) − 8(4, 4) EE | 111794.034(34e-3) | 60.6 | 0.47169 | blended | – | – | – |
| $CH_3OCH_3$ | 7(5, 3) − 8(4, 4) AE | 111797.334(29e-3) | 60.6 | 1.02408 | blended | – | – | – |
| $CH_3OCH_3$ | 7(5, 3) − 8(4, 4) EA | 111797.837(26e-3) | 60.6 | 2.01433 | 55 | 56.0(1.0) | 7.9(2.1) | 463(144) |
| $CH_3OCH_3$ | 7(5, 2) − 8(4, 5) EE | 111801.894(25e-3) | 60.6 | 7.72144 | 72 | 56.1(1.1) | 10.2(4.1) | 1554(232) |
| $CH_3OCH_3$ | 7(5, 2) − 8(4, 5) AA | 111809.374(33e-3) | 60.6 | 5.12083 | 547 | 56.0(0.1) | 11.6(0.3) | 6756(182) |
| $HC_5N$ | 42 − 41 | 111823.024(0) | 115.4 | 2362.2 | 55 | 57.5(1.7) | 6.3(4.5) | 1435(210) |
| aGg'−$(CH_2OH)_2$ | 11(0, 11) v=1 − 10(0, 10) v=0 | 111841.702(2e-3) | 31.2 | 334.78228 | 67 | 56.0(0.8) | 8.2(2.6) | 1159(148) |
| H$\beta$ | H (48) $\beta$ | 111885.070(0) | – | – | 162 | 60.1(0.5) | 25.1(1.0) | 4343(166) |
| $CH_3OCHO$ | 9(3, 6) − 8(3, 5) | 112011.966(1e-2) | 219.9 | 21.00957 | 218 | 56.2(0.2) | 6.2(0.5) | 1446(100) |
| $C_2H_5OH$ | 9(6, 3) − 10(5, 6) | 112047.555(5e-2) | 83.0 | 1.0874 | 44 | 57.2(1.4) | 7.2(3.3) | 335(146) |
| $C_2H_5OH$ | 9(6, 4) − 10(5, 5) | 112046.635(5e-2) | 83.0 | 1.0874 | blended | – | – | – |
| $CH_3OH$, vt=0-2 | $19(0)^+ - 18(2)^+$, vt=0 | 112145.638(21e-3) | 440.1 | 0.00059 | 220 | 56.5(1.1) | 14.8(1.1) | 3459(100) |
| $CH_3CHO$ | 6(1, 6) − 5(1, 5) A, vt=0 | 112248.716(3e-3) | 21.1 | 73.76807 | 452 | 58.0(1.1) | 9.0(1.1) | 4348(143) |
| $CH_3CHO$ | 6(1, 6) − 5(1, 5) E, vt=0 | 112254.508(3e-3) | 21.2 | 73.79585 | 524 | 58.0(1.0) | 9.4(1.1) | 5218(143) |
| $C_2H_5OH$ | 9(1, 8) − 8(0, 8) | 112269.238(5e-2) | 96.5 | 3.943 | 67 | 58.2(1.0) | 9.2(1.1) | 1297(143) |
| t-HCOOH | 5(2, 4) − 4(2, 3) | 112287.145(3e-3) | 28.9 | 8.4851 | 168 | 58.1(1.0) | 7.1(1.1) | 1272(143) |
| $CH_3OCHO$ | 9(3, 6) − 8(3, 5) | 112306.941(1e-2) | 220.5 | 21.20275 | 196 | 56.0(0.4) | 5.1(1.0) | 1055(172) |
| $C^{17}O$ | 1 − 0 | 112359.284(1e-3) | 5.4 | 0.01217 | 1704 | 56.5(0.1) | 8.0(0.1) | 14432(221) |
| $CH_3COCH_3$ | 11(1, 11) − 10(0, 10) AE | 112365.987(13e-3) | 33.6 | 178.40946 | 80 | 57.0(0.9) | 4.7(1.3) | 398(146) |
| $CH_3COCH_3$ | 11(1, 11) − 10(0, 10) EA | 112366.032(11e-3) | 33.6 | 356.79399 | blended | – | – | – |
| $CH_3COCH_3$ | 11(0, 11) − 10(1, 10) EE | 112373.549(9e-3) | 33.5 | 1426.94226 | 408 | 57.2(0.2) | 9.7(0.6) | 4196(234) |
| $CH_3COCH_3$ | 6(5, 1) − 5( 4, 1) EE | 112375.101(8e-3) | 18.4 | 70.65642 | blended | – | – | – |
| $CH_3COCH_3$ | 11(0, 11) − 10(1, 10) AA | 112381.030(14e-3) | 33.4 | 891.85807 | 79 | 57.1(1.0) | 3.7(1.9) | 309(138) |
| t-HCOOH | 5(4, 2) − 4(4, 1) | 112432.292(3e-3) | 67.1 | 3.6372 | blended | – | – | – |
| t-HCOOH | 5(4, 1) − 4(4, 0) | 112432.319(3e-3) | 67.1 | 3.6372 | 80 | 57.0(0.6) | 3.6(1.7) | 303(129) |
| t-HCOOH | 5(3, 3) − 4(3, 2) | 112459.621(3e-3) | 44.8 | 6.4662 | 89 | 56.8(0.9) | 5.8(1.5) | 553(158) |
| t-HCOOH | 5(3, 2) − 4(3, 1) | 112467.007(3e-3) | 44.8 | 6.4654 | 104 | 56.9(0.6) | 3.6(1.3) | 397(131) |
| $CH_3OH$, vt=0-2 | 14(-3) − 15(2) E2, vt=0 | 112491.019(15e-3) | 306.4 | 0.28629 | 77 | 56.7(0.8) | 3.9(1.3) | 322(124) |
| $C_2H_5CN$ | 13(1, 13) − 12(1, 12) | 112646.350(9e-2) | 39.0 | 191.45 | 255 | 58.0(0.3) | 8.5(0.9) | 2314(193) |
| $CH_3OCHO$ | 14(5, 9) −14(4, 10) E | 112672.759(1e-2) | 78.9 | 3.64313 | 115 | 56.0(0.6) | 5.0(1.2) | 607(143) |
| $CH_3OCHO$ | 14(5, 9) −14(4, 10) A | 112676.856(1e-2) | 78.9 | 3.67559 | 102 | 56.3(0.6) | 4.8(1.2) | 521(133) |
| $C_2H_5OH$ | 11(3, 9) − 10(4, 7) | 112746.252(5e-2) | 127.5 | 1.5782 | 91 | 56.8(0.7) | 3.8(1.2) | 368(129) |
| $C_2H_5OH$ | 2(2, 1) − 1(1, 0) | 112807.174(5e-2) | 7.5 | 3.2057 | 67 | 56.8(1.0) | 4.8(1.8) | 344(139) |
| $CH_3COCH_3$ | 23(10, 13) − 23(9, 14) EE | 112831.025(45e-3) | 209.3 | 1421.81619 | 28 | 57.2(2.6) | 4.4(3.4) | 134(130) |
| $CH_3COCH_3$ | 23(11, 13) − 23(10, 14) EE | 112838.230(45e-3) | 209.3 | 1421.96282 | blended | – | – | – |
| $C_2H_3CN$ | 12(0, 12) − 11(0, 11) | 112840.637(1e-2) | 35.3 | 523.56 | 97 | 58.5(0.9) | 7.6(1.6) | 782(178) |
| $CH_3OCHO$ | 14(3, 11) − 13(4, 10) E | 112852.231(1e-2) | 70.0 | 1.08582 | 22 | 56.0(2.5) | 1.5(0.5) | 82(36) |
| $CH_3OCHO$ | 14(3, 11) − 13(4, 10) A | 112869.893(1e-2) | 70.0 | 1.08568 | 38 | 56.1(1.6) | 3.0(2.2) | 120(104) |
| t-HCOOH | 5(2, 3) − 4(2, 2) | 112891.443 (3e-3) | 28.9 | 8.4849 | 182 | 57.2(0.5) | 7.8(1.2) | 1513(199) |
| $CH_3OCH_3$ | 20(3, 17) − 20(2, 18) EA | 112999.674(33e-3) | 206.1 | 87.23585 | 466 | 55.6(0.2) | 9.2(0.4) | 4545(199) |
| $CH_3OCH_3$ | 20(3, 17) − 20(2, 18) AE | 112999.675(33e-3) | 206.1 | 43.6109 | blended | – | – | – |
| $CH_3OCH_3$ | 17(3, 14) − 17(2, 15) AA | 113061.072(22e-3) | 153.1 | 221.33 | 542 | 55.6(0.3) | 11.6(0.5) | 6691(267) |
| $C_2H_5OH$ | 10(2, 9) − 12(1, 10) | 113098.078(5e-2) | 51.0 | 8.3566 | 162 | 57.0(0.6) | 6.0(1.2) | 1041(194) |
| CN | N= 1-0, J=1/2-1/2, F=1/2-1/2 | 113123.370(6e-3) | 5.4 | 0.15271 | 606 | 55.1(1.1) | 6.6(1.1) | 4236(781) |
| CN | N= 1-0, J=1/2-1/2, F=1/2-3/2 | 113144.157(6e-3) | 5.4 | 1.2492 | 2180 | 55.0(1.1) | 8.0(1.1) | 18669(781) |
| CN | N= 1-0, J=1/2-1/2, F=3/2-1/2 | 113170.492(4e-3) | 5.4 | 1.2199 | 3065 | 55.0(1.0) | 7.9(1.1) | 25683(781) |
| CN | N= 1-0, J=1/2-1/2, F=3/2-3/2 | 113191.279(3e-3) | 5.4 | 1.5836 | 2726 | 55.0(0.9) | 8.1(1.1) | 23382(781) |
| $CH_3OCH_3$ | 10(6, 4) − 11(5, 6) EE | 113275.765(97e-3) | 100.7 | 14.77486 | 70 | 55.5(1.0) | 5.5(1.9) | 405(126) |
| $CH_3OCH_3$ | 10(6, 4) − 11(5, 7) AA | 113280.325(1e-1) | 100.7 | 5.57556 | 54 | 55.5(1.1) | 4.6(2.0) | 265(112) |
| $CH_3OCHO$ | 22(6, 16) − 22(5, 17) A | 113299.505(1e-2) | 175.0 | 6.95078 | 84 | 56.0(0.6) | 4.0(1.1) | 357(102) |
| $C_2H_5OH$ | 6(1, 6) − 5(2, 4) | 113314.491(5e-2) | 79.6 | 0.5853 | 91 | 57.2(0.7) | 3.4(1.3) | 331(127) |
| $C_2H_5OH$ | 6(1, 6) − 6(0, 6) | 113325.517(5e-2) | 79.6 | 8.8225 | 54 | 57.1(1.3) | 4.6(2.6) | 262(145) |
| CCS | 9(8) − 8(7) | 113410.186(2e-2) | 33.6 | 65.427 | 195 | 56.5(1.1) | 9.9(1.1) | 2053(802) |
| CN | N= 1-0, J=3/2-1/2, F=3/2-1/2 | 113488.120(3e-3) | 5.4 | 1.5838 | 5177 | 55.0(0.9) | 9.5(1.1) | 52219(802) |
| CN | N= 1-0, J=3/2-1/2, F=5/2-3/2 | 113490.970(2e-3) | 5.4 | 4.205 | blended | – | – | – |
| CN | N= 1-0, J=3/2-1/2, F=1/2-1/2 | 113499.644(3e-3) | 5.4 | 1.2491 | 1468 | 55.1(1.1) | 8.0(1.1) | 12426(802) |
| CN | N= 1-0, J=3/2-1/2, F=3/2-3/2 | 113508.907(3e-3) | 5.4 | 1.2196 | 1989 | 55.0(1.0) | 8.2(1.1) | 17317(802) |
| CN | N= 1-0, J=3/2-1/2, F=1/2-3/2 | 113520.432(4e-3) | 5.4 | 0.15263 | 316 | 55.1(1.0) | 6.0(1.1) | 2027(802) |
| | | G059.78+00.06 | | | | | | |
| CCS | 8(9) − 7(8) | 106347.726(2e-2) | 25.0 | 74.425 | 148 | 22.5(0.1) | 1.9(0.1) | 293(18) |
| $HC_5N$ | 40 − 39 | 106498.910(7e-3) | 104.8 | 2249.7 | 30 | 22.6(0.3) | 2.0(0.5) | 63(1.5) |
| $CH_3OH$, vt=0-2 | $3(1)^+ - 4(0)^+$, vt=0 | 107013.831(1e-2) | 28.3 | 12.036 | 100 | 21.0(0.2) | 5.4(0.4) | 569(35) |
| $CH_3OH$, vt=0-2 | 15(-2) − 15(1) E2, vt=0 | 107159.906(14e-3) | 304.7 | 10.421 | 14 | 21.1(0.7) | 3.2(1.5) | 49(20) |
| t-HCOOH | 5(1, 5) − 4(1, 4) | 108126.720(3e-3) | 18.8 | 9.6966 | 38 | 22.0(0.3) | 3.7(0.8) | 152(26) |
| $^{13}CN$ | 1(1, 0) − 0(1, 1), F = 1 − 1 | 108412.862(5e-2) | 5.2 | 0.635 | 19 | 22.6(0.6) | 2.7(0.9) | 54(20) |
| $^{13}CN$ | 1(1, 0) − 0(1, 1), F = 1 − 2 | 108426.889(5e-2) | 5.2 | 1.267 | 25 | 22.2(0.4) | 2.0(0.7) | 54(18) |
| $^{13}CN$ | 1(1, 1) − 0(1, 0), F = 0 − 1 | 108631.121(5e-2) | 5.2 | 0.642 | 28 | 22.6(0.3) | 1.7(0.5) | 50(15) |
| $^{13}CN$ | 1(1, 1) − 0(1, 0), F = 1 − 1 | 108636.923(5e-2) | 5.2 | 1.932 | 80 | 22.5(0.5) | 1.8(0.5) | 153(13) |
| $^{13}CN$ | 1(2, 1) − 0(1, 1), F = 1 − 0 | 108638.212(5e-2) | 5.2 | 0.722 | 34 | 22.6(0.3) | 3.1(0.8) | 112(25) |
| $^{13}CN$ | 1(2, 1) − 0(1, 1), F = 2 − 1 | 108643.590(5e-2) | 5.2 | 0.856 | 17 | 22.6(1.4) | 3.6(2.4) | 65(56) |
| $^{13}CN$ | 1(2, 1) − 0(1, 1), F = 0 − 1 | 108644.346(5e-2) | 5.2 | 0.642 | 22 | 22.4(0.5) | 1.8(1.5) | 48(40) |
| $^{13}CN$ | 1(2, 1) − 0(1, 1), F = 1 − 1 | 108645.064(5e-2) | 5.2 | 0.551 | 29 | 22.5(0.3) | 0.9(0.5) | 27(17) |
| $^{13}CN$ | 1(1, 1) − 0(1, 0), F = 2 − 1 | 108651.297(5e-2) | 5.2 | 3.276 | 109 | 22.6(0.1) | 1.9(0.2) | 217(18) |
| $^{13}CN$ | 1(2, 1) − 0(1, 1), F = 2 − 2 | 108657.646(5e-2) | 5.2 | 2.420 | 93 | 22.6(0.1) | 1.4(0.2) | 137(16) |
| $^{13}CN$ | 1(2, 1) − 0(1, 1), F = 1 − 2 | 108658.948(5e-2) | 5.2 | 0.669 | 28 | 22.6(0.4) | 2.8(0.8) | 84(22) |
| $^{13}CN$ | 1(2, 2) − 0(1, 1), F = 3 − 2 | 108780.201(5e-2) | 5.2 | 4.905 | 161 | 22.4(0.1) | 1.9(0.1) | 326(20) |
| $^{13}CN$ | 1(2, 2) − 0(1, 1), F = 2 − 1 | 108782.374(5e-2) | 5.2 | 2.586 | 127 | 22.6(0.1) | 1.3(0.2) | 181(17) |
| $^{13}CN$ | 1(2, 2) − 0(1, 1), F = 1 − 0 | 108786.982(5e-2) | 5.2 | 1.144 | 66 | 22.6(0.1) | 0.8(0.2) | 54(12) |
| $^{13}CN$ | 1(2, 2) − 0(1, 1), F = 1 − 1 | 108793.753(5e-2) | 5.2 | 0.894 | 43 | 22.5(0.2) | 1.8(0.4) | 83(17) |
| $^{13}CN$ | 1(2, 2) − 0(1, 1), F = 2 − 2 | 108796.400(5e-2) | 5.2 | 0.918 | 49 | 22.5(0.2) | 1.4(0.4) | 76(18) |
| $CH_3OH$, vt=0-2 | 0(0) − 1(-1) E2, vt=0 | 108893.945(12e-3) | 13.1 | 3.9134 | 582 | 21.0(0.1) | 2.9(0.1) | 1768(27) |
| $HC_5N$ | 41 − 40 | 109160.973(7e-3) | 110.0 | 2306 | 29 | 22.5(0.5) | 3.1(0.9) | 97(31) |
| $HC_3N$ | 12 − 11 | 109173.634(1e-2) | 34.1 | 167.1 | 2385 | 22.5(0.) | 2.0(0.1) | 5131(29) |
| SO | 3(2) − 2(1) | 109252.220(1e-1) | 21.1 | 3.5585 | 1099 | 23.0(0.) | 2.0(0.1) | 2379(21) |
| OCS | 9 − 8 | 109463.063(5e-3) | 26.3 | 4.6034 | 184 | 23.0(0.1) | 3.1(0.2) | 598(27) |
| $C^{15}N$ | 1(1, 1) − 0(1, 1) | 109689.610(1e-1) | 5.3 | 1.386 | 24 | 23.9(0.8) | 6.7(1.5) | 174(38) |
| $C^{18}O$ | 1 − 0 | 109782.173(6e-3) | 5.3 | 0.01221 | 2005 | 22.8(0.1) | 2.4(0.1) | 5177(26) |
| HNCO | 5(0, 5) − 4(0, 4) | 109905.749(7e-3) | 15.8 | 12.482 | 235 | 23.2(0.1) | 3.2(0.1) | 789(28) |
| $C^{15}N$ | 1(2, 1) − 0(1, 0) | 110023.540(1e-1) | 5.3 | 1.386 | 44 | 22.2(0.2) | 1.1(0.5) | 53(20) |

**Table A2.** (Continued)

| Species | Transitions | Rest Freq. | $E_u$ | $\mu^2S$ | $T_{mb}$ | $V_{LSR}$ | $\Delta V$ | $\int T_{mb}\,dv$ |
|---|---|---|---|---|---|---|---|---|
| | | (MHz) | (K) | ($D^2$) | (mK) | (km $s^{-1}$) | (km $s^{-1}$) | (mK km $s^{-1}$) |
| $C^{15}N$ | 1(2, 2) − 0(1, 1) | 110024.590(1e-1) | 5.3 | 3.504 | 40 | 22.3(0.3) | 2.3(1.4) | 97(38) |
| $^{13}CO$ | 1 − 0 | 110201.35(0) | 5.3 | 0.01220 | 15471 | 22.8(0.1) | 3.1(0.1) | 51180(221) |
| $CH_3CN$ | 6(3, 0) − 5(-3, 0) | 110364.354(0) | 82.8 | 138.45 | 57 | 22.2(0.5) | 3.5(0.5) | 212(21) |
| $CH_3CN$ | 6(-3, 0) − 5(3, 0) | 110364.354(0) | 82.8 | 138.45 | blended | − | − | − |
| $CH_3CN$ | 6(2, 0) − 5(2, 0) | 110374.989(0) | 47.1 | 164.06 | 100 | 22.3(0.5) | 2.8(0.5) | 292(21) |
| $CH_3CN$ | 6(1, 0) − 5(1, 0) | 110381.372(0) | 25.7 | 179.45 | 229 | 22.3(0.4) | 2.3(0.5) | 565(21) |
| $CH_3CN$ | 6(0, 0) − 5(0, 0) | 110383.500(0) | 18.5 | 184.58 | 279 | 22.3(0.3) | 2.5(0.5) | 737(21) |
| $CH_3OH$, vt=0-2 | $7(2)^+ - 8(1)^+$, vt=0 | 111289.453(13e-3) | 102.7 | 9.3425 | 27 | 21.2(0.8) | 2.0(1.6) | 59(40) |
| t-HCOOH | 5(0, 5) − 4(0, 4) | 111746.784(3e-3) | 16.1 | 10.092 | 32 | 22.0(0.6) | 1.7(0.8) | 58(36) |
| $CH_3CHO$ | 6(1, 6) − 5(1, 5) A, vt=0 | 112248.716(3e-3) | 21.1 | 73.76807 | 74 | 22.1(0.5) | 1.6(0.5) | 124(15) |
| $CH_3CHO$ | 6(1, 6) − 5(1, 5) E, vt=0 | 112254.508(3e-3) | 21.2 | 73.79585 | 40 | 22.1(0.4) | 3.2(0.5) | 137(15) |
| $C^{17}O$ | 1 − 0 | 112359.284(1e-3) | 5.4 | 0.01217 | 399 | 23.0(0.1) | 2.7(0.1) | 1141(43) |
| t-HCOOH | 5(2, 3) − 4(2, 2) | 112891.443 (3e-3) | 28.9 | 8.4849 | 35 | 22.1(0.4) | 1.4(0.7) | 51(26) |
| CN | N= 1-0, J=1/2-1/2, F=1/2-1/2 | 113123.370(6e-3) | 5.4 | 0.15271 | 573 | 22.5(0.5) | 1.8(0.5) | 1112(173) |
| CN | N= 1-0, J=1/2-1/2, F=1/2-3/2 | 113144.157(6e-3) | 5.4 | 1.2492 | 2003 | 22.5(0.) | 2.2(0.5) | 4745(173) |
| CN | N= 1-0, J=1/2-1/2, F=3/2-1/2 | 113170.492(4e-3) | 5.4 | 1.2199 | 2221 | 22.6(0.5) | 2.4(0.5) | 5776(173) |
| CN | N= 1-0, J=1/2-1/2, F=3/2-3/2 | 113191.279(3e-3) | 5.4 | 1.5836 | 2160 | 22.5(0.4) | 2.4(0.5) | 5461(173) |
| CCS | 9(8) − 8(7) | 113.410.186(2e-2) | 33.6 | 65.427 | 57 | 22.5(0.5) | 1.8(0.5) | 110(35) |
| CN | N= 1-0, J=3/2-1/2, F=3/2-1/2 | 113488.120(3e-3) | 5.4 | 1.5838 | 2138 | 22.5(0.) | 2.5(0.5) | 5682(235) |
| CN | N= 1-0, J=3/2-1/2, F=5/2-3/2 | 113490.970(2e-3) | 5.4 | 4.205 | 4207 | 22.5(0.4) | 2.8(0.5) | 12365(235) |
| CN | N= 1-0, J=3/2-1/2, F=1/2-1/2 | 113499.644(3e-3) | 5.4 | 1.2491 | 1360 | 22.5(0.6) | 2.3(0.5) | 3295(235) |
| CN | N= 1-0, J=3/2-1/2, F=3/2-3/2 | 113508.907(3e-3) | 5.4 | 1.2196 | 1785 | 22.6(0.5) | 2.4(0.5) | 4606(235) |
| CN | N= 1-0, J=3/2-1/2, F=1/2-3/2 | 113520.432(4e-3) | 5.4 | 0.15263 | 349 | 22.5(0.5) | 2.2(0.5) | 830(235) |
| G069.54−00.97 | | | | | | | | |
| CCS | 8(9) − 7(8) | 106347.726(2e-2) | 25.0 | 74.425 | 96 | 11.5(0.1) | 3.6(0.2) | 372(20) |
| $HC_5N$ | 40 − 39 | 106498.910(7e-3) | 104.8 | 2249.7 | 23 | 11.8(0.5) | 5.0(1.2) | 123(25) |
| Hα | H (39) α | 106737.357(0) | − | − | 58 | 3.8(0.6) | 32.5(1.7) | 2003(82) |
| $CH_3OH$, vt=0-2 | $3(1)^+ - 4(0)^+$, vt=0 | 107013.831(1e-2) | 28.3 | 12.036 | 257 | 11.5(0.5) | 3.7(0.5) | 1019(26) |
| $CH_3OH$, vt=0-2 | 15(-2) − 15(1) E2, vt=0 | 107159.906(14e-3) | 304.7 | 10.421 | 24 | 11.5(3.6) | 4.4(4.8) | 113(112) |
| $CH_3OCHO$ | 9( 2, 8) − 8( 2, 7) E | 107537.258(1e-2) | 28.8 | 22.60702 | 19 | 13.5(0.4) | 2.5(1.2) | 51(19) |
| $CH_3OCHO$ | 9( 2, 8) − 8( 2, 7) A | 107543.711(1e-2) | 28.8 | 22.61344 | 28 | 13.6(0.3) | 2.1(0.7) | 64(17) |
| $SO_2$ | 12(4, 8) − 13(3, 11) | 107843.470(2e-3) | 111.0 | 4.5354 | 22 | 9.8(0.6) | 3.5(2.6) | 81(36) |
| t-HCOOH | 5(1, 5) − 4(1, 4) | 108126.720(3e-3) | 18.8 | 9.6966 | 26 | 11.0(0.4) | 6.0(0.7) | 165(19) |
| $^{13}CN$ | 1(1, 0) − 0(1, 1), F = 1 − 1 | 108412.862(5e-2) | 5.2 | 0.635 | 30 | 11.6(0.3) | 3.6(0.9) | 116(23) |
| $^{13}CN$ | 1(1, 0) − 0(1, 1), F = 1 − 2 | 108426.889(5e-2) | 5.2 | 1.267 | 35 | 11.6(0.2) | 1.8(0.7) | 66(36) |
| $^{13}CN$ | 1(1, 1) − 0(1, 0), F = 1 − 1 | 108636.923(5e-2) | 5.2 | 1.932 | 42 | 11.4(0.5) | 3.5(0.5) | 156(10) |
| $^{13}CN$ | 1(2, 1) − 0(1, 1), F = 1 − 0 | 108638.212(5e-2) | 5.2 | 0.722 | 29 | 11.7(0.5) | 4.3(0.5) | 133(10) |
| $^{13}CN$ | 1(2, 1) − 0(1, 1), F = 2 − 1 | 108643.590(5e-2) | 5.2 | 0.856 | 26 | 11.5(0.5) | 4.3(0.5) | 118(10) |
| $^{13}CN$ | 1(2, 1) − 0(1, 1), F = 0 − 1 | 108644.346(5e-2) | 5.2 | 0.642 | 24 | 11.8(0.5) | 6.9(0.5) | 176(10) |
| $^{13}CN$ | 1(2, 1) − 0(1, 1), F = 1 − 1 | 108645.064(5e-2) | 5.2 | 0.551 | blended | − | − | − |
| $^{13}CN$ | 1(1, 1) − 0(1, 0), F = 2 − 1 | 108651.297(5e-2) | 5.2 | 3.276 | 92 | 11.5(0.5) | 4.2(0.5) | 408(10) |
| $^{13}CN$ | 1(2, 1) − 0(1, 1), F = 2 − 2 | 108657.646(5e-2) | 5.2 | 2.420 | 64 | 11.5(0.5) | 3.5(0.5) | 245(10) |
| $^{13}CN$ | 1(2, 1) − 0(1, 1), F = 1 − 2 | 108658.948(5e-2) | 5.2 | 0.669 | 20 | 11.6(0.5) | 5.3(0.5) | 111(10) |
| $^{13}CN$ | 1(2, 2) − 0(1, 1), F = 3 − 2 | 108780.201(5e-2) | 5.2 | 4.905 | 134 | 11.5(0.1) | 3.3(0.2) | 465(20) |
| $^{13}CN$ | 1(2, 2) − 0(1, 1), F = 2 − 1 | 108782.374(5e-2) | 5.2 | 2.586 | 76 | 11.6(0.1) | 4.0(0.4) | 323(23) |
| $^{13}CN$ | 1(2, 2) − 0(1, 1), F = 1 − 0 | 108786.982(5e-2) | 5.2 | 1.144 | 16 | 11.5(0.8) | 6.4(1.7) | 107(27) |
| $^{13}CN$ | 1(2, 2) − 0(1, 1), F = 1 − 1 | 108793.753(5e-2) | 5.2 | 0.894 | 18 | 11.6(0.6) | 4.5(1.3) | 84(22) |
| $^{13}CN$ | 1(2, 2) − 0(1, 1), F = 2 − 2 | 108796.400(5e-2) | 5.2 | 0.918 | 31 | 11.5(0.3) | 2.8(0.5) | 92(17) |
| $CH_3OH$, vt=0-2 | 0(0) − 1(-1) E2, vt=0 | 108893.945(12e-3) | 13.1 | 3.9134 | 439 | 11.6(0.1) | 4.9(0.1) | 2324(51) |
| $HC_3N$ | 12 − 11 | 109173.634(1e-2) | 34.1 | 167.1 | 2098 | 11.5(0.) | 3.7(0.1) | 8263(275) |
| SO | 3(2) − 2(1) | 109252.220(1e-1) | 21.1 | 3.5585 | 595 | 11.0(0.) | 5.0(0.2) | 3179(81) |
| OCS | 9 − 8 | 109463.063(5e-3) | 26.3 | 4.6034 | 220 | 11.3(0.1) | 6.0(0.4) | 1399(69) |
| $C^{18}O$ | 1 − 0 | 109782.173(6e-3) | 5.3 | 0.01221 | 3182 | 11.2(0.1) | 3.9(0.1) | 13178(51) |
| HNCO | 5(0, 5) − 4(0, 4) | 109905.749(7e-3) | 15.8 | 12.482 | 398 | 11.1(0.1) | 4.4(0.1) | 1850(46) |
| $C^{15}N$ | 1(2, 1) − 0(1, 0) | 110023.540(1e-1) | 5.3 | 1.386 | 42 | 10.9(0.8) | 3.4(1.9) | 152(86) |
| $C^{15}N$ | 1(2, 2) − 0(1, 1) | 110024.590(1e-1) | 5.3 | 3.504 | 27 | 10.7(1.1) | 3.1(1.9) | 91(73) |
| $^{13}CO$ | 1 − 0 | 110201.35(0) | 5.3 | 0.01220 | 15790 | 11.5(0.1) | 4.7(0.1) | 79650(133) |
| $CH_3CN$ | 6(4, 0) − 5(4, 0) | 110349.471(0) | 132.8 | 102.54 | 21 | 11.7(0.7) | 5.0(1.3) | 115(29) |
| $CH_3CN$ | 6(3, 0) − 5(-3, 0) | 110364.354(0) | 82.8 | 138.45 | 122 | 11.7(0.1) | 6.2(0.3) | 805(35) |
| $CH_3CN$ | 6(-3, 0) − 5(3, 0) | 110364.354(0) | 82.8 | 138.45 | blended | − | − | − |
| $CH_3CN$ | 6(2, 0) − 5(2, 0) | 110374.989(0) | 47.1 | 164.06 | 161 | 11.8(0.1) | 4.9(0.1) | 837(31) |
| $CH_3CN$ | 6(1, 0) − 5(1, 0) | 110381.372(0) | 25.7 | 179.45 | 266 | 11.7(0.1) | 3.9(0.2) | 1117(41) |
| $CH_3CN$ | 6(0, 0) − 5(0, 0) | 110383.500(0) | 18.5 | 184.58 | 322 | 11.6(0.1) | 4.8(0.2) | 1660(45) |
| t-HCOOH | 26(6, 20) − 27(5, 23) | 110640.753(9e-3) | 493.7 | 0.18082 | 13 | 11.1(1.1) | 2.9(2.3) | 39(26) |
| $CH_3OCHO$ | 10(0, 10) − 9(0, 9) E | 111169.903(1e-2) | 30.2 | 26.18776 | 24 | 13.5(0.2) | 1.1(1.2) | 39(19) |
| $CH_3OCHO$ | 10(0, 10) − 9(0, 9) A | 111171.634(1e-2) | 30.2 | 16.19136 | blended | − | − | − |
| $CH_3OH$, vt=0-2 | 17(-2) − 17(1) E2, vt=0 | 111626.514(15e-3) | 381.5 | 20.231 | 24 | 11.5(0.7) | 6.8(1.4) | 174(39) |
| $CH_3OCHO$ | 9(1, 8) − 8(1, 7) E | 111674.131(1e-2) | 28.1 | 23.18984 | 12 | 13.6(2.0) | 4.9(3.3) | 48(32) |
| t-HCOOH | 5(0, 5) − 4(0, 4) | 111746.784(3e-3) | 16.1 | 10.092 | 42 | 10.8(0.3) | 4.0(0.8) | 178(31) |
| $CH_3OCH_3$ | 7(0, 7) − 6(1, 6) AA | 111782.562(8e-3) | 25.2 | 68.047 | 31 | 11.0(0.5) | 5.7(1.1) | 192(36) |
| $HC_5N$ | 42 − 41 | 111823.024(0) | 115.4 | 2362.2 | 36 | 11.8(0.5) | 3.1(1.0) | 121(32) |
| $CH_3CHO$ | 6(1, 6) − 5(1, 5) A, vt=0 | 112248.716(3e-3) | 21.1 | 73.76807 | 64 | 11.5(0.2) | 3.7(0.5) | 250(30) |
| $CH_3CHO$ | 6(1, 6) − 5(1, 5) E, vt=0 | 112254.508(3e-3) | 21.2 | 73.79585 | 79 | 11.5(0.2) | 3.2(0.4) | 269(27) |
| t-HCOOH | 5(2, 4) − 4(2, 3) | 112287.145(3e-3) | 28.9 | 8.4851 | 33 | 11.2(0.3) | 1.9(0.5) | 69(20) |
| $C^{17}O$ | 1 − 0 | 112359.284(1e-3) | 5.4 | 0.01217 | 764 | 11.0(0.1) | 5.5(0.1) | 4513(52) |
| t-HCOOH | 5(2, 3) − 4(2, 2) | 112891.443(3e-3) | 28.9 | 8.4849 | 37 | 11.1(0.3) | 2.1(1.6) | 85(25) |
| CN | N= 1-0, J=1/2-1/2, F=1/2-1/2 | 113123.370(6e-3) | 5.4 | 0.15271 | 52 | 11.5(0.5) | 3.8(0.5) | 2090(183) |
| CN | N= 1-0, J=1/2-1/2, F=1/2-3/2 | 113144.157(6e-3) | 5.4 | 1.2492 | 1585 | 11.5(0.5) | 4.3(0.5) | 7328(183) |
| CN | N= 1-0, J=1/2-1/2, F=3/2-1/2 | 113170.492(4e-3) | 5.4 | 1.2199 | 1955 | 11.5(0.4) | 4.3(0.5) | 8928(183) |
| CN | N= 1-0, J=1/2-1/2, F=3/2-3/2 | 113191.279(3e-3) | 5.4 | 1.5836 | 1684 | 11.5(0.5) | 4.5(0.5) | 8097(183) |
| CN | N= 1-0, J=3/2-1/2, F=3/2-1/2 | 113488.120(3e-3) | 5.4 | 1.5838 | 1778 | 11.5(0.6) | 3.8(0.5) | 7143(314) |
| CN | N= 1-0, J=3/2-1/2, F=5/2-3/2 | 113490.970(2e-3) | 5.4 | 4.205 | 3262 | 11.5(0.5) | 4.4(0.5) | 15171(314) |
| CN | N= 1-0, J=3/2-1/2, F=1/2-1/2 | 113499.644(3e-3) | 5.4 | 1.2491 | 962 | 11.5(0.4) | 4.9(0.5) | 5043(314) |
| CN | N= 1-0, J=3/2-1/2, F=3/2-3/2 | 113508.907(3e-3) | 5.4 | 1.2196 | 1387 | 11.5(0.3) | 4.5(0.5) | 6654(314) |
| CN | N= 1-0, J=3/2-1/2, F=1/2-3/2 | 113520.432(4e-3) | 5.4 | 0.15263 | 302 | 11.5(0.5) | 4.3(0.5) | 1370(314) |
| G075.76+00.33 | | | | | | | | |
| CCS | 8(9) − 7(8) | 106347.726(2e-2) | 25.0 | 74.425 | 112 | -1.5(0.1) | 3.0(0.2) | 361(18) |
| $HC_5N$ | 40 − 39 | 106498.910(7e-3) | 104.8 | 2249.7 | 30 | -2.2(0.2) | 4.0(0.6) | 129(16) |
| $C_2H_5OH$ | 13(1, 12) − 13(0, 13) | 106649.479(5e-2) | 79.4 | 2362.2 | 24 | -4.3(0.5) | 3.3(0.5) | 84(9) |
| $C_2H_5OH$ | 6(1, 5) − 5(1, 4) | 106676.542(5e-2) | 76.1 | 9.325 | 20 | -4.3(0.5) | 7.3(0.5) | 157(88) |
| Hα | H (39) α | 106737.357(0) | − | − | 83 | -15.1(0.5) | 30.8(1.6) | 2730(105) |
| $CH_3OH$, vt=0-2 | $3(1)^+ - 4(0)^+$, vt=0 | 107013.831(1e-2) | 28.3 | 12.036 | 103 | -2.5(0.1) | 6.0(0.3) | 654(29) |
| t-HCOOH | 5(1, 5) − 4(1, 4) | 108126.720(3e-3) | 18.8 | 9.6966 | 29 | -2.0(0.3) | 2.2(0.3) | 67(16) |
| $^{13}CN$ | 1(1, 0) − 0(1, 1), F = 1 − 0 | 108406.091(5e-2) | 5.2 | 0.191 | 12 | -1.7(0.9) | 3.3(2.1) | 410(34) |
| $^{13}CN$ | 1(1, 0) − 0(1, 1), F = 1 − 1 | 108412.862(5e-2) | 5.2 | 0.635 | 22 | -1.2(0.2) | 1.2(0.7) | 28(14) |

**Table A2.** (Continued)

| Species | Transitions | Rest Freq. (MHz) | E$_u$ (K) | $\mu^2$S (D$^2$) | T$_{mb}$ (mK) | V$_{LSR}$ (km s$^{-1}$) | $\Delta$V (km s$^{-1}$) | $\int$ T$_{mb}$ dv (mK km s$^{-1}$) |
|---|---|---|---|---|---|---|---|---|
| $^{13}$CN | 1(1, 0) − 0(1, 1), F = 1 − 2 | 108426.889(5e-2) | 5.2 | 1.267 | 40 | -1.8(0.2) | 3.6(0.6) | 153(21) |
| $^{13}$CN | 1(1, 1) − 0(1, 0), F = 0 − 1 | 108631.121(5e-2) | 5.2 | 0.642 | 12 | -1.4(0.4) | 1.6(0.8) | 20(10) |
| $^{13}$CN | 1(1, 1) − 0(1, 0), F = 1 − 1 | 108636.923(5e-2) | 5.2 | 1.932 | 52 | -1.8(0.2) | 3.0(0.4) | 169(19) |
| $^{13}$CN | 1(2, 1) − 0(1, 1), F = 1 − 0 | 108638.212(5e-2) | 5.2 | 0.722 | 24 | -1.8(0.3) | 1.5(0.7) | 39(16) |
| $^{13}$CN | 1(2, 1) − 0(1, 1), F = 2 − 1 | 108643.590(5e-2) | 5.2 | 0.856 | 25 | -1.6(0.6) | 2.6(1.2) | 69(36) |
| $^{13}$CN | 1(2, 1) − 0(1, 1), F = 0 − 1 | 108644.346(5e-2) | 5.2 | 0.642 | 24 | -1.9(0.7) | 3.1(1.4) | 77(36) |
| $^{13}$CN | 1(2, 1) − 0(1, 1), F = 1 − 1 | 108645.064(5e-2) | 5.2 | 0.551 | blended | – | – | – |
| $^{13}$CN | 1(1, 1) − 0(1, 0), F = 2 − 1 | 108651.297(5e-2) | 5.2 | 3.276 | 65 | -1.8(0.1) | 2.9(0.2) | 199(15) |
| $^{13}$CN | 1(2, 1) − 0(1, 1), F = 2 − 2 | 108657.646(5e-2) | 5.2 | 2.420 | 38 | -1.8(0.1) | 2.2(0.5) | 88(31) |
| $^{13}$CN | 1(2, 1) − 0(1, 1), F = 1 − 2 | 108658.948(5e-2) | 5.2 | 0.669 | 21 | -1.7(0.9) | 5.6(1.5) | 127(38) |
| $^{13}$CN | 1(2, 2) − 0(1, 1), F = 3 − 2 | 108780.201(5e-2) | 5.2 | 4.905 | 90 | -1.9(0.1) | 3.1(0.3) | 300(19) |
| $^{13}$CN | 1(2, 2) − 0(1, 1), F = 2 − 1 | 108782.374(5e-2) | 5.2 | 2.586 | 40 | -1.8(0.2) | 3.8(0.6) | 164(20) |
| $^{13}$CN | 1(2, 2) − 0(1, 1), F = 1 − 0 | 108786.982(5e-2) | 5.2 | 1.144 | 28 | -1.8(0.3) | 3.3(0.6) | 96(16) |
| $^{13}$CN | 1(2, 2) − 0(1, 1), F = 1 − 1 | 108793.753(5e-2) | 5.2 | 0.894 | 19 | -1.7(0.5) | 4.4(1.4) | 89(21) |
| $^{13}$CN | 1(2, 2) − 0(1, 1), F = 2 − 2 | 108796.400(5e-2) | 5.2 | 0.918 | 17 | -1.8(0.4) | 2.2(0.7) | 40(13) |
| HC$_3$N | 12 − 11 | 109173.634(1e-2) | 34.1 | 167.1 | 2235 | -2.0(0.) | 3.7(0.1) | 8688(32) |
| SO | 3(2) − 2(1) | 109252.220(1e-1) | 21.1 | 3.5585 | 518 | -1.5(0.) | 4.4(0.1) | 2444(44) |
| OCS | 9 − 8 | 109463.063(5e-3) | 26.3 | 4.6034 | 133 | -1.7(0.1) | 5.0(0.3) | 713(31) |
| C$^{18}$O | 1 − 0 | 109782.173(6e-3) | 5.3 | 0.01221 | 1561 | -1.7(0.1) | 3.8(0.1) | 6380(33) |
| HNCO | 5(0, 5) − 4(0, 4) | 109905.749(7e-3) | 15.8 | 12.482 | 201 | -2.0(0.2) | 6.8(0.6) | 1455(94) |
| C$^{15}$N | 1(2, 1) − 0(1, 0) | 110023.540(1e-1) | 5.3 | 1.386 | 28 | -1.6(1.0) | 7.3(1.7) | 214(63) |
| C$^{15}$N | 1(2, 2) − 0(1, 1) | 110024.590(1e-1) | 5.3 | 3.504 | 36 | -1.7(0.5) | 4.4(1.1) | 170(37) |
| $^{13}$CO | 1 − 0 | 110201.35(0) | 5.3 | 0.01220 | 9801 | -2.0(0.1) | 5.3(0.1) | 54771(208) |
| CH$_3$CN | 6(4, 0) − 5(4, 0) | 110349.471(0) | 132.8 | 102.54 | 21 | -2.0(0.3) | 2.4(0.5) | 54(390 |
| CH$_3$CN | 6(3, 0) − 5(-3, 0) | 110364.354(0) | 82.8 | 138.45 | 103 | -2.0(0.5) | 4.8(0.5) | 526(39) |
| CH$_3$CN | 6(-3, 0) − 5(3, 0) | 110364.354(0) | 82.8 | 138.45 | blended | – | – | – |
| CH$_3$CN | 6(2, 0) − 5(2, 0) | 110374.989(0) | 47.1 | 164.06 | 142 | -2.0(0.4) | 3.8(0.5) | 578(39) |
| CH$_3$CN | 6(1, 0) − 5(1, 0) | 110381.372(0) | 25.7 | 179.45 | 299 | -2.0(0.5) | 4.1(0.5) | 1300(39) |
| CH$_3$CN | 6(0, 0) − 5(0, 0) | 110383.500(0) | 18.5 | 184.58 | 351 | -2.0(0.5) | 3.9(0.5) | 1473(39) |
| HC$_5$N | 42 − 41 | 111823.024(0) | 115.4 | 2362.2 | 25 | -2.2(1.1) | 7.6(2.4) | 200(58) |
| CH$_3$CHO | 6(1, 6) − 5(1, 5) A, vt=0 | 112248.716(3e-3) | 21.1 | 73.76807 | 86 | -1.7(0.4) | 8.8(1.1) | 802(75) |
| CH$_3$CHO | 6(1, 6) − 5(1, 5) E, vt=0 | 112254.508(3e-3) | 21.2 | 73.79585 | 100 | -1.7(0.) | 5.6(1.0) | 598(86) |
| C$^{17}$O | 1 − 0 | 112359.284(1e-3) | 5.4 | 0.01217 | 369 | -1.7(0.1) | 6.7(0.4) | 2640(129) |
| CN | N= 1-0, J=1/2-1/2, F=1/2-1/2 | 113123.370(6e-3) | 5.4 | 0.15271 | 337 | -1.7(0.5) | 4.2(0.5) | 1520(149) |
| CN | N= 1-0, J=1/2-1/2, F=1/2-3/2 | 113144.157(6e-3) | 5.4 | 1.2492 | 1319 | -1.7(0.1) | 5.1(0.5) | 7089(149) |
| CN | N= 1-0, J=1/2-1/2, F=3/2-1/2 | 113170.492(4e-3) | 5.4 | 1.2199 | 1469 | -1.7(0.5) | 4.9(0.5) | 7670(149) |
| CN | N= 1-0, J=1/2-1/2, F=3/2-3/2 | 113191.279(3e-3) | 5.4 | 1.5836 | 1382 | -1.7(0.1) | 5.4(0.5) | 7977(149) |
| CCS | 9(8) − 8(7) | 113410186(2e-2) | 33.6 | 65.427 | 18 | -1.5(0.5) | 6.1(0.5) | 1088(207) |
| CN | N= 1-0, J=3/2-1/2, F=3/2-1/2 | 113488.120(3e-3) | 5.4 | 1.5838 | 110 | -1.7(0.4) | 5.1(0.5) | 5989(207) |
| CN | N= 1-0, J=3/2-1/2, F=5/2-3/2 | 113490.970(2e-3) | 5.4 | 4.205 | 2444 | -1.7(0.5) | 7.3(0.5) | 18996(207) |
| CN | N= 1-0, J=3/2-1/2, F=1/2-1/2 | 113499.644(3e-3) | 5.4 | 1.2491 | 885 | -1.7(0.4) | 5.2(0.5) | 4909(207) |
| CN | N= 1-0, J=3/2-1/2, F=3/2-3/2 | 113508.907(3e-3) | 5.4 | 1.2196 | 1103 | -1.7(0.3) | 5.5(0.5) | 6495(207) |
| CN | N= 1-0, J=3/2-1/2, F=1/2-3/2 | 113520.432(4e-3) | 5.4 | 0.15263 | 187 | -1.7(0.5) | 4.9(0.5) | 969(207) |
| | | G078.12+03.63 | | | | | | |
| NH$_2$CHO | 5(2, 4) − 4(2, 3) | 105972.665(37e-3) | 27.2 | 54.915 | 28 | -1.0(0.7) | 15.5(2.3) | 373(48) |
| NH$_2$CHO | 5(4, 1) − 4(4, 0) | 106107.870(88e-3) | 63.0 | 23.537 | 13 | -1.0(1.8) | 5.5(4.1) | 221(51) |
| NH$_2$CHO | 5(4, 2) − 4(4, 1) | 106107.845(88e-3) | 63.0 | 23.537 | blended | – | – | – |
| NH$_2$CHO | 5(3, 3) − 4(3, 2) | 106134.468(55e-3) | 42.1 | 41.845 | 22 | -1.0(1.1) | 9.7(2.1) | 222(62) |
| NH$_2$CHO | 5(3, 2) − 4(3, 1) | 106141.442(55e-3) | 42.1 | 41.84 | 14 | -1.0(2.3) | 10.6(9.1) | 298(93) |
| CCS | 8(9) − 7(8) | 106347.726(2e-2) | 25.0 | 74.425 | 87 | -4.0(0.1) | 3.1(0.4) | 290(27) |
| NH$_2$CHO | 5(2, 3) − 4(2, 2) | 106541.773(37e-3) | 27.2 | 54.915 | 22 | -1.0(1.0) | 12.3(2.0) | 295(47) |
| CH$_3$OH, vt=0-2 | $3(1)^+ - 4(0)^+$, vt=0 | 107013.831(1e-2) | 28.3 | 12.036 | 197 | -4.1(0.1) | 8.2(0.2) | 1724(37) |
| CH$_3$OH, vt=0-2 | 15(-2) − 15(1) E2, vt=0 | 107159.906(14e-3) | 304.7 | 10.421 | 31 | -4.0(0.7) | 8.7(1.7) | 283(48) |
| $^{13}$CN | 1(1, 0) − 0(1, 1), F = 1 − 0 | 108406.091(5e-2) | 5.2 | 0.191 | 17 | -4.1(1.2) | 2.7(1.7) | 48(28) |
| $^{13}$CN | 1(1, 0) − 0(1, 1), F = 1 − 1 | 108412.862(5e-2) | 5.2 | 0.635 | 29 | -4.2(0.5) | 3.3(0.8) | 101(29) |
| $^{13}$CN | 1(1, 0) − 0(1, 1), F = 1 − 2 | 108426.889(5e-2) | 5.2 | 1.267 | 47 | -4.2(0.3) | 2.4(0.9) | 121(32) |
| $^{13}$CN | 1(1, 1) − 0(1, 0), F = 0 − 1 | 108631.121(5e-2) | 5.2 | 0.642 | 50 | -4.3(0.2) | 0.6(0.3) | 33(13) |
| $^{13}$CN | 1(1, 1) − 0(1, 0), F = 1 − 1 | 108636.923(5e-2) | 5.2 | 1.932 | 78 | -4.2(0.1) | 1.4(0.3) | 114(25) |
| $^{13}$CN | 1(2, 1) − 0(1, 1), F = 1 − 0 | 108638.212(5e-2) | 5.2 | 0.722 | 26 | -4.1(0.9) | 7.1(1.5) | 197(43) |
| $^{13}$CN | 1(2, 1) − 0(1, 1), F = 2 − 1 | 108643.590(5e-2) | 5.2 | 0.856 | 38 | -4.3(0.2) | 0.8(0.3) | 33(19) |
| $^{13}$CN | 1(2, 1) − 0(1, 1), F = 0 − 1 | 108644.346(5e-2) | 5.2 | 0.642 | 29 | -4.5(0.8) | 4.9(1.4) | 149(42) |
| $^{13}$CN | 1(2, 1) − 0(1, 1), F = 1 − 1 | 108645.064(5e-2) | 5.2 | 0.551 | blended | – | – | – |
| $^{13}$CN | 1(1, 1) − 0(1, 0), F = 2 − 1 | 108651.297(5e-2) | 5.2 | 3.276 | 134 | -4.1(0.1) | 1.5(0.2) | 219(19) |
| $^{13}$CN | 1(2, 1) − 0(1, 1), F = 2 − 2 | 108657.646(5e-2) | 5.2 | 2.420 | 85 | -4.2(0.1) | 2.0(0.3) | 180(23) |
| $^{13}$CN | 1(2, 1) − 0(1, 1), F = 1 − 2 | 108658.948(5e-2) | 5.2 | 0.669 | 34 | -4.1(0.3) | 1.5(0.6) | 55(19) |
| $^{13}$CN | 1(2, 2) − 0(1, 1), F = 3 − 2 | 108780.201(5e-2) | 5.2 | 4.905 | 163 | -4.1(0.1) | 2.2(0.2) | 387(32) |
| $^{13}$CN | 1(2, 2) − 0(1, 1), F = 2 − 1 | 108782.374(5e-2) | 5.2 | 2.586 | 77 | -4.1(0.2) | 2.1(0.4) | 170(29) |
| $^{13}$CN | 1(2, 2) − 0(1, 1), F = 1 − 0 | 108786.982(5e-2) | 5.2 | 1.144 | 47 | -4.2(0.2) | 1.1(2.7) | 54(22) |
| $^{13}$CN | 1(2, 2) − 0(1, 1), F = 1 − 1 | 108793.753(5e-2) | 5.2 | 0.894 | 38 | -4.1(0.5) | 3.4(1.1) | 135(39) |
| $^{13}$CN | 1(2, 2) − 0(1, 1), F = 2 − 2 | 108796.400(5e-2) | 5.2 | 0.918 | 23 | -4.2(0.7) | 2.1(1.3) | 52(30) |
| CH$_3$OH, vt=0-2 | 0(0) − 1(-1) E2, vt=0 | 108893.945(12e-3) | 13.1 | 3.9134 | 134 | -4.0(0.1) | 7.8(0.4) | 1109(43) |
| HC$_3$N | 12 − 11 | 109173.634(1e-2) | 34.1 | 167.1 | 2450 | -4.1(0.) | 3.0(0.1) | 7729(90) |
| SO | 3(2) − 2(1) | 109252.220(1e-1) | 21.1 | 3.5585 | 162 | -3.8(0.2) | 6.9(0.4) | 1193(57) |
| HC$_3$N, v$_7$=1 | 12(-1) − 11(1) | 109442.013(2e-2) | 355.0 | 165.12 | 35 | -3.0(0.5) | 4.1(1.2) | 151(36) |
| OCS | 9 − 8 | 109463.063(5e-3) | 26.3 | 4.6034 | 123 | -3.9(0.2) | 6.9(0.4) | 896(43) |
| HC$_3$N, v$_7$=1 | 12(1) − 11(-1) | 109598.818(2e-2) | 355.0 | 165.12 | 15 | -3.0(1.2) | 3.7(2.2) | 61(34) |
| HNCO | 5(1, 5) − 4(1, 4) | 109495.996(6e-3) | 59.0 | 11.847 | 43 | -4.0(0.4) | 8.4(0.9) | 387(34) |
| NH$_2$CHO | 5(1, 4) − 4(1, 3) | 109753.549(25e-3) | 18.8 | 62.756 | 30 | -4.2(1.1) | 7.2(1.1) | 229(200) |
| C$^{18}$O | 1 − 0 | 109782.173(6e-3) | 5.3 | 0.01221 | 1239 | -4.0(1.1) | 3.4(1.1) | 4480(200) |
| HNCO | 5(0, 5) − 4(0, 4) | 109905.749(7e-3) | 15.8 | 12.482 | 188 | -4.1(0.1) | 4.3(0.6) | 866(77) |
| C$^{15}$N | 1(2, 1) − 0(1, 0) | 110023.540(1e-1) | 5.3 | 1.386 | 25 | -4.0(1.4) | 4.5(1.9) | 117(62) |
| C$^{15}$N | 1(2, 2) − 0(1, 1) | 110024.590(1e-1) | 5.3 | 3.504 | 44 | -3.8(0.5) | 2.5(0.8) | 117(60) |
| $^{13}$CO | 1 − 0 | 110201.35(0) | 5.3 | 0.01220 | 10768 | -4.0(0.1) | 2.5(0.1) | 28275(407) |
| CH$_3$CN | 6(4, 0) − 5(4, 0) | 110349.471(0) | 132.8 | 102.54 | 59 | -4.1(0.5) | 5.3(0.5) | 334(42) |
| CH$_3$CN | 6(3, 0) − 5(-3, 0) | 110364.354(0) | 82.8 | 138.45 | 141 | -4.1(0.3) | 7.8(0.5) | 1178(42) |
| CH$_3$CN | 6(-3, 0) − 5(3, 0) | 110364.354(0) | 82.8 | 138.45 | blended | – | – | – |
| CH$_3$CN | 6(2, 0) − 5(2, 0) | 110374.989(0) | 47.1 | 164.06 | 140 | -4.0(0.5) | 7.3(0.5) | 1095(42) |
| CH$_3$CN | 6(1, 0) − 5(1, 0) | 110381.372(0) | 25.7 | 179.45 | 225 | -4.1(0.5) | 5.4(0.5) | 1293(42) |
| CH$_3$CN | 6(0, 0) − 5(0, 0) | 110383.500(0) | 18.5 | 184.58 | 256 | -4.0(0.4) | 5.6(0.5) | 1527(42) |
| CH$_3$OH, vt=0-2 | $7(2)^+ - 8(1)^+$, vt=0 | 111289.453(13e-3) | 102.7 | 9.3425 | 89 | -4.0(0.4) | 7.8(0.7) | 745(67) |
| C$^{17}$O | 1 − 0 | 112359.284(1e-3) | 5.4 | 0.01217 | 263 | -4.2(0.1) | 5.2(0.3) | 1468(58) |
| CN | N= 1-0, J=1/2-1/2, F=1/2-1/2 | 113123.370(6e-3) | 5.4 | 0.15271 | 801 | -3.5(0.5) | 2.1(0.5) | 1764(214) |
| CN | N= 1-0, J=1/2-1/2, F=1/2-3/2 | 113144.157(6e-3) | 5.4 | 1.2492 | 2400 | -3.5(0.) | 2.7(0.5) | 6808(214) |
| CN | N= 1-0, J=1/2-1/2, F=3/2-1/2 | 113170.492(4e-3) | 5.4 | 1.2199 | 2805 | -3.5(0.4) | 2.7(0.5) | 7964(214) |
| CN | N= 1-0, J=1/2-1/2, F=3/2-3/2 | 113191.279(3e-3) | 5.4 | 1.5836 | 2638 | -3.4(0.5) | 2.7(0.5) | 7620(214) |

**Table A2.** (Continued)

| Species | Transitions | Rest Freq. (MHz) | $E_u$ (K) | $\mu^2S$ ($D^2$) | $T_{mb}$ (mK) | $V_{LSR}$ (km $s^{-1}$) | $\Delta V$ (km $s^{-1}$) | $\int T_{mb}$ dv (mK km $s^{-1}$) |
|---|---|---|---|---|---|---|---|---|
| CN | N= 1-0, J=3/2-1/2, F=3/2-1/2 | 113488.120(3e-3) | 5.4 | 1.5838 | 2792 | -3.5(0.5) | 2.6(0.5) | 7867(537) |
| CN | N= 1-0, J=3/2-1/2, F=5/2-3/2 | 113490.970(2e-3) | 5.4 | 4.205 | 6181 | -3.5(0.8) | 2.9(0.5) | 18859(537) |
| CN | N= 1-0, J=3/2-1/2, F=1/2-1/2 | 113499.644(3e-3) | 5.4 | 1.2491 | 1855 | -3.4(0.5) | 2.6(0.5) | 5195(537) |
| CN | N= 1-0, J=3/2-1/2, F=3/2-3/2 | 113508.907(3e-3) | 5.4 | 1.2196 | 2260 | -3.5(0.6) | 2.5(0.5) | 6087(537) |
| CN | N= 1-0, J=3/2-1/2, F=1/2-3/2 | 113520.432(4e-3) | 5.4 | 0.15263 | 637 | -3.5(0.5) | 1.9(0.5) | 1305(537) |
| | | | | G081.75+00.59 | | | | |
| CCS | 8(9) − 7(8) | 106347.726(2e-2) | 25.0 | 74.425 | 211 | -4.1(0.3) | 2.1(0.1) | 476(14) |
| $HC_5N$ | 40 − 39 | 106498.910(7e-3) | 104.8 | 2249.7 | 75 | -4.0(0.1) | 2.2(0.2) | 172(13) |
| $CH_3OH$, vt=0-2 | $3(1)^+ - 4(0)^+$, vt=0 | 107013.831(1e-2) | 28.3 | 12.036 | 89 | -5.5(0.2) | 1.4(0.4) | 130(27) |
| t-HCOOH | 5(1, 5) − 4(1, 4) | 108126.720(3e-3) | 18.8 | 9.6966 | 38 | -4.0(0.2) | 2.4(0.5) | 100(17) |
| $^{13}CN$ | 1(1, 0) − 0(1, 1), F = 1 − 1 | 108412.862(5e-2) | 5.2 | 0.635 | 26 | -4.0(0.3) | 2.2(0.8) | 59(18) |
| $^{13}CN$ | 1(1, 0) − 0(1, 1), F = 1 − 2 | 108426.889(5e-2) | 5.2 | 1.267 | 67 | -4.1(0.1) | 1.8(0.2) | 132(15) |
| $^{13}CN$ | 1(1, 1) − 0(1, 0), F = 0 − 1 | 108631.121(5e-2) | 5.2 | 0.642 | 32 | -3.8(0.2) | 2.4(0.4) | 81(15) |
| $^{13}CN$ | 1(1, 1) − 0(1, 0), F = 1 − 1 | 108636.923(5e-2) | 5.2 | 1.932 | 102 | -3.9(0.1) | 2.1(0.2) | 228(17) |
| $^{13}CN$ | 1(2, 1) − 0(1, 1), F = 1 − 0 | 108638.212(5e-2) | 5.2 | 0.722 | 44 | -4.1(0.2) | 1.6(0.4) | 74(14) |
| $^{13}CN$ | 1(2, 1) − 0(1, 1), F = 2 − 1 | 108643.590(5e-2) | 5.2 | 0.856 | 30 | -4.0(0.4) | 2.1(0.9) | 69(55) |
| $^{13}CN$ | 1(2, 1) − 0(1, 1), F = 0 − 1 | 108644.346(5e-2) | 5.2 | 0.642 | 40 | -3.9(0.7) | 3.9(1.1) | 166(56) |
| $^{13}CN$ | 1(2, 1) − 0(1, 1), F = 1 − 1 | 108645.064(5e-2) | 5.2 | 0.551 | blended | − | − | − |
| $^{13}CN$ | 1(1, 1) − 0(1, 0), F = 2 − 1 | 108651.297(5e-2) | 5.2 | 3.276 | 159 | -4.0(0.1) | 1.9(0.1) | 327(16) |
| $^{13}CN$ | 1(2, 1) − 0(1, 1), F = 2 − 2 | 108657.646(5e-2) | 5.2 | 2.420 | 113 | -3.9(0.1) | 1.7(0.1) | 206(15) |
| $^{13}CN$ | 1(2, 1) − 0(1, 1), F = 1 − 2 | 108658.948(5e-2) | 5.2 | 0.669 | 20 | -4.0(0.4) | 3.0(0.9) | 63(18) |
| $^{13}CN$ | 1(2, 2) − 0(1, 1), F = 3 − 2 | 108780.201(5e-2) | 5.2 | 4.905 | 201 | -4.1(0.1) | 2.2(0.1) | 474(24) |
| $^{13}CN$ | 1(2, 2) − 0(1, 1), F = 2 − 1 | 108782.374(5e-2) | 5.2 | 2.586 | 107 | -3.9(0.1) | 2.1(0.3) | 238(24) |
| $^{13}CN$ | 1(2, 2) − 0(1, 1), F = 1 − 0 | 108786.982(5e-2) | 5.2 | 1.144 | 55 | -4.0(0.2) | 2.4(0.6) | 140(27) |
| $^{13}CN$ | 1(2, 2) − 0(1, 1), F = 1 − 1 | 108793.753(5e-2) | 5.2 | 0.894 | 47 | -3.9(0.3) | 2.9(0.7) | 146(28) |
| $^{13}CN$ | 1(2, 2) − 0(1, 1), F = 2 − 2 | 108796.400(5e-2) | 5.2 | 0.918 | 31 | -4.1(0.4) | 2.6(1.2) | 86(28) |
| $CH_3OH$, vt=0-2 | 0(0) − 1(-1) E2, vt=0 | 108893.945(12e-3) | 13.1 | 3.9134 | 40 | -5.6(0.) | 3.0(0.1) | 1284(32) |
| $HC_5N$ | 41 − 40 | 109160.973(7e-3) | 110.0 | 2306 | 64 | -4.0(0.5) | 3.0(1.2) | 207(19) |
| $HC_3N$ | 12 − 11 | 109173.634(1e-2) | 34.1 | 167.1 | 3578 | -4.1(0.) | 2.3(0.1) | 8942(57) |
| SO | 3(2) − 2(1) | 109252.220(1e-1) | 21.1 | 3.5585 | 7956 | -4.1(0.1) | 2.4(0.1) | 2060(57) |
| OCS | 9 − 8 | 109463.063(5e-3) | 26.3 | 4.6034 | 184 | -3.9(0.) | 2.3(0.1) | 454(21) |
| $C^{18}O$ | 1 − 0 | 109782.173(6e-3) | 5.3 | 0.01221 | 5214 | -4.0(0.1) | 2.3(0.1) | 12589(455) |
| HNCO | 5(0, 5) − 4(0, 4) | 109905.749(7e-3) | 15.8 | 12.482 | 90 | -3.7(0.) | 2.1(0.4) | 201(25) |
| $C^{15}N$ | 1(2, 1) − 0(1, 0) | 110023.540(1e-1) | 5.3 | 1.386 | 41 | -4.3(0.2) | 1.6(0.5) | 68(20) |
| $C^{15}N$ | 1(2, 2) − 0(1, 1) | 110024.590(1e-1) | 5.3 | 3.504 | 100 | -4.1(0.1) | 1.9(0.3) | 204(23) |
| $^{13}CO$ | 1 − 0 | 110201.35(0) | 5.3 | 0.01220 | 25526 | -4.1(0.1) | 2.6(0.1) | 70887(413) |
| $CH_3CN$ | 6(3, 0) − 5(-3, 0) | 110364.354(0) | 82.8 | 138.45 | 67 | -4.0(0.4) | 3.4(0.5) | 244(42) |
| $CH_3CN$ | 6(-3, 0) − 5(3, 0) | 110364.354(0) | 82.8 | 138.45 | blended | − | − | − |
| $CH_3CN$ | 6(2, 0) − 5(2, 0) | 110374.989(0) | 47.1 | 164.06 | 138 | -4.0(0.5) | 2.0(0.5) | 299(42) |
| $CH_3CN$ | 6(1, 0) − 5(1, 0) | 110381.372(0) | 25.7 | 179.45 | 351 | -4.1(0.5) | 2.3(0.5) | 844(42) |
| $CH_3CN$ | 6(0, 0) − 5(0, 0) | 110383.500(0) | 18.5 | 184.58 | 446 | -4.0(0.5) | 2.3(0.5) | 1098(42) |
| $CH_3OH$, vt=0-2 | $7(2)^+ - 8(1)^+$, vt=0 | 111289.453(13e-3) | 102.7 | 9.3425 | 27 | -5.5(0.5) | 4.9(0.9) | 138(28) |
| t-HCOOH | 5(0, 5) − 4(0, 4) | 111746.784(3e-3) | 16.1 | 10.092 | 55 | -4.0(0.2) | 1.9(0.5) | 110(25) |
| $CH_3CHO$ | 6(1, 6) − 5(1, 5) A, vt=0 | 112248.716(3e-3) | 21.1 | 73.76807 | 89 | -4.2(0.2) | 2.5(0.3) | 235(28) |
| $CH_3CHO$ | 6(1, 6) − 5(1, 5) E, vt=0 | 112254.508(3e-3) | 21.2 | 73.79585 | 109 | -4.1(0.1) | 2.9(0.3) | 338(31) |
| $C^{17}O$ | 1 − 0 | 112359.284(1e-3) | 5.4 | 0.01217 | 1056 | -4.0(0.1) | 2.5(0.2) | 2848(192) |
| CN | N= 1-0, J=1/2-1/2, F=1/2-1/2 | 113123.370(6e-3) | 5.4 | 0.15271 | 984 | -4.1(0.5) | 2.2(0.5) | 2285(171) |
| CN | N= 1-0, J=1/2-1/2, F=1/2-3/2 | 113144.157(6e-3) | 5.4 | 1.2492 | 2284 | -4.0(0.5) | 2.3(0.5) | 5698(171) |
| CN | N= 1-0, J=1/2-1/2, F=3/2-1/2 | 113170.492(4e-3) | 5.4 | 1.2199 | 2601 | -4.0(0.4) | 2.3(0.5) | 6316(171) |
| CN | N= 1-0, J=1/2-1/2, F=3/2-3/2 | 113191.279(3e-3) | 5.4 | 1.5836 | 2304 | -4.0(0.5) | 2.3(0.5) | 5743(171) |
| CCS | 9(8) − 8(7) | 113410.186(2e-2) | 33.6 | 65.427 | 86 | -4.0(0.5) | 1.7(0.5) | 157(21) |
| CN | N= 1-0, J=3/2-1/2, F=3/2-1/2 | 113488.120(3e-3) | 5.4 | 1.5838 | 2368 | -4.0(0.5) | 2.4(0.5) | 6014(198) |
| CN | N= 1-0, J=3/2-1/2, F=5/2-3/2 | 113490.970(2e-3) | 5.4 | 4.205 | 3457 | -4.0(0.) | 2.5(0.5) | 9208(198) |
| CN | N= 1-0, J=3/2-1/2, F=1/2-1/2 | 113499.644(3e-3) | 5.4 | 1.2491 | 1608 | -4.1(0.5) | 2.4(0.5) | 4077(198) |
| CN | N= 1-0, J=3/2-1/2, F=3/2-3/2 | 113508.907(3e-3) | 5.4 | 1.2196 | 2165 | -4.0(0.4) | 2.3(0.5) | 5236(198) |
| CN | N= 1-0, J=3/2-1/2, F=1/2-3/2 | 113520.432(4e-3) | 5.4 | 0.15263 | 642 | -4.0(0.7) | 2.1(0.5) | 1468(198) |
| | | | | G081.87+00.78 | | | | |
| $NH_2CHO$ | 5(2, 4) − 4(2, 3) | 105972.665(37e-3) | 27.2 | 54.915 | 35 | 9.5(0.5)) | 6.2(1.2) | 234(34) |
| $NH_2CHO$ | 5(4, 1) − 4(4, 0) | 106107.870(88e-3) | 63.0 | 23.537 | 19 | 9.5(1.1) | 9.9(2.4) | 201(43) |
| $NH_2CHO$ | 5(4, 2) − 4(4, 1) | 106107.845(88e-3) | 63.0 | 23.537 | blended | − | − | − |
| $NH_2CHO$ | 5(3, 3) − 4(3, 2) | 106134.468(55e-3) | 42.1 | 41.845 | 25 | 9.4(0.7) | 7.2(1.5) | 190(36) |
| $NH_2CHO$ | 5(3, 2) − 4(3, 1) | 106141.442(55e-3) | 42.1 | 41.84 | 24 | 9.4(1.1) | 7.6(3.1) | 366(59) |
| CCS | 8(9) − 7(8) | 106347.726(2e-2) | 25.0 | 74.425 | 126 | 9.3(0.1) | 3.0(0.2) | 399(20) |
| $NH_2CHO$ | 5(2, 3) − 4(2, 2) | 106541.773(37e-3) | 27.2 | 54.915 | 36 | 9.5(0.3) | 4.4(0.8) | 170(26) |
| $C_2H_5OH$ | 9(2, 8) − 9(1, 9) | 106723.558(5e-2) | 42.7 | 7.9044 | 24 | 9.0(0.4) | 3.5(0.9) | 88 (21) |
| $^{34}SO$ | 3(2) − 2(1) | 106743.244(7e-2) | 20.9 | 3.557 | 131 | 9.7(0.1) | 5.2(0.3) | 88(21) |
| $C_2H_5OH$ | 6(1, 5) − 5(1, 4) | 106767.234(5e-2) | 80.7 | 9.6466 | 14 | 8.9(1.0) | 3.0(2.0) | 44(22) |
| $CH_3OCH_3$ | 9(1, 8) − 8(2, 7) AA | 106775.602(14e-3) | 43.4 | 36.603 | 17 | 9.1(1.0)) | 5.0(2.3) | 89(38) |
| $CH_3OCH_3$ | 9(1, 8) − 8(2, 7) EE | 106777.344(9e-3) | 43.4 | 58.573 | 40 | 9.0(0.4) | 5.7(1.3) | 243(43) |
| $CH_3OCH_3$ | 9(1, 8) − 8(2, 7) EA | 106779.091(11e-3) | 43.4 | 21.963 | 26 | 9.0(0.3) | 1.3(0.6) | 35(17) |
| $CH_3OCH_3$ | 9(1, 8) − 8(2, 7) EE | 106779.083(11e-3) | 43.4 | 14.645 | blended | − | − | − |
| $OC^{34}S$ | 9 − 8 | 106787.390(2e-3) | 25.6 | 4.601 | 47 | 8.4(0.4) | 3.9(1.0) | 196(44) |
| $HOCO^+$ | 5(0, 5) − 4(0, 4) | 106913.545(3e-3) | 15.4 | 36.454 | 39 | 9.0(0.3) | 3.3(0.6) | 140(22) |
| $CH_3OH$, vt=0-2 | $3(1)^+ - 4(0)^+$, vt=0 | 107013.831(1e-2) | 28.3 | 12.036 | 933 | 8.7(0.) | 6.2(0.1) | 6141(34) |
| $SO_2$ | 27(3, 25) − 26(4, 22) | 107060.208(2e-3) | 369.4 | 8.2723 | 78 | 9.0(0.2) | 6.6(0.6) | 545(36) |
| $CH_3OH$, vt=0-2 | 15(-2) − 15(1) E2, vt=0 | 107159.906(14e-3) | 304.7 | 10.421 | 124 | 8.8(0.1) | 5.5(0.3) | 719(36) |
| $HOCO^+$ | 5(1, 4) − 4(1, 3) | 107315.356(21e-3) | 52.8 | 34.996 | 13 | 8.9(1.1) | 5.8(2.0) | 83(28) |
| $C_2H_5CN$ | 12(7, 5) − 11(7, 4) | 107485.160(5e-2) | 88.0 | 117.36 | 26 | 8.8(0.7) | 4.4(1.6) | 120(38) |
| $C_2H_5CN$ | 12(6, 6) − 11(6, 5) | 107486.949(5e-2) | 73.6 | 133.42 | 34 | 8.8(0.3) | 2.2(0.7) | 79(31) |
| $C_2H_5CN$ | 12(5, 7) − 11(5, 6) | 107502.432(5e-2) | 61.3 | 146.99 | 37 | 8.8(0.3) | 4.1(0.9) | 161(28) |
| $CH_3OCHO$ | 9( 2, 8) − 8( 2, 7) E | 107537.258(1e-2) | 28.8 | 22.60702 | 69 | 9.0(0.2) | 4.3 ( 0.5) | 316(28) |
| $CH_3OCHO$ | 9( 2, 8) − 8( 2, 7) A | 107543.711(1e-2) | 28.8 | 22.61344 | 76 | 9.0(0.2) | 6.1(0.5) | 496(33) |
| $C_2H_5CN$ | 12(3, 10) − 11(3, 9) | 107594.056(5e-2) | 43.6 | 166.77 | 26 | 8.8(0.4) | 1.8(0.9) | 50(20) |
| $C_2H_5CN$ | 12(3, 9) − 11(3, 8) | 107734.723(5e-2) | 43.6 | 166.76 | 22 | 8.7(0.6) | 1.8(0.7) | 41(22) |
| $SO_2$ | 12(4, 8) − 13(3, 11) | 107843.470(2e-3) | 111.0 | 4.5354 | 191 | 9.1(0.2) | 6.1(0.4) | 1243(71) |
| t-HCOOH | 5(1, 5) − 4(1, 4) | 108126.720(3e-3) | 18.8 | 9.6966 | 69 | 9.6(0.2) | 5.1(0.6) | 370(33) |
| $C_2H_5OH$ | 13(3, 10) − 13(2, 11) | 108438.579(5e-2) | 88.2 | 18.79 | 29 | 8.9(0.4) | 3.0(0.8) | 92(22) |
| $^{13}CN$ | 1(1, 1) − 0(1, 0), F = 0 − 1 | 108631.121(5e-2) | 5.2 | 0.642 | 14 | 9.6(0.7) | 2.4(1.6) | 38(22) |
| $^{13}CN$ | 1(1, 1) − 0(1, 0), F = 1 − 1 | 108636.923(5e-2) | 5.2 | 1.932 | 36 | 9.2(0.4) | 3.6(0.9) | 138(28) |
| $^{13}CN$ | 1(2, 1) − 0(1, 1), F = 1 − 0 | 108638.212(5e-2) | 5.2 | 0.722 | 15 | 9.1(0.5) | 0.9(0.7) | 15(10) |
| $^{13}CN$ | 1(2, 1) − 0(1, 1), F = 2 − 1 | 108643.590(5e-2) | 5.2 | 0.856 | 27 | 9.8(0.5) | 4.9(1.0) | 143(29) |
| $^{13}CN$ | 1(2, 1) − 0(1, 1), F = 0 − 1 | 108644.346(5e-2) | 5.2 | 0.642 | blended | − | − | − |
| $^{13}CN$ | 1(2, 1) − 0(1, 1), F = 1 − 1 | 108645.064(5e-2) | 5.2 | 0.551 | blended | − | − | − |
| $^{13}CN$ | 1(1, 1) − 0(1, 0), F = 2 − 1 | 108651.297(5e-2) | 5.2 | 3.276 | 50 | 9.2(0.3) | 3.9(0.5) | 209(27) |

**Table A2.** (Continued)

| Species | Transitions | Rest Freq. | $E_u$ | $\mu^2S$ | $T_{mb}$ | $V_{LSR}$ | $\Delta V$ | $\int T_{mb}\,dv$ |
|---|---|---|---|---|---|---|---|---|
| | | (MHz) | (K) | ($D^2$) | (mK) | (km $s^{-1}$) | (km $s^{-1}$) | (mK km $s^{-1}$) |
| $^{13}CN$ | 1(2, 1) − 0(1, 1), F = 2 − 2 | 108657.646(5e-2) | 5.2 | 2.420 | 39 | 9.1(0.3) | 2.9(0.5) | 123(22) |
| $^{13}CN$ | 1(2, 2) − 0(1, 1), F = 3 − 2 | 108780.201(5e-2) | 5.2 | 4.905 | 96 | 9.1(0.1) | 4.0(0.3) | 406(26) |
| $^{13}CN$ | 1(2, 2) − 0(1, 1), F = 2 − 1 | 108782.374(5e-2) | 5.2 | 2.586 | 70 | 9.3(0.1) | 2.6(0.3) | 195(21) |
| $^{13}CN$ | 1(2, 2) − 0(1, 1), F = 1 − 0 | 108786.982(5e-2) | 5.2 | 1.144 | 20 | 9.2(0.7) | 4.9(1.3) | 107(27) |
| $^{13}CN$ | 1(2, 2) − 0(1, 1), F = 1 − 1 | 108793.753(5e-2) | 5.2 | 0.894 | 28 | 9.1(0.3) | 2.3(0.7) | 70(19) |
| $^{13}CN$ | 1(2, 2) − 0(1, 1), F = 2 − 2 | 108796.400(5e-2) | 5.2 | 0.918 | 29 | 9.1(0.2) | 1.2(0.5) | 38(14) |
| $CH_3OH$, vt=0-2 | 0(0) − 1(-1) E2, vt=0 | 108893.945(12e-3) | 13.1 | 3.9134 | 949 | 8.9(0.) | 4.8(0.1) | 4871(28) |
| $CH_3OH$, vt=0-2 | 14(5) − 15(4) E1, vt=0 | 109138.783(15e-3) | 379.7 | 13.593 | 155 | 8.8(0.1) | 6.1(0.2) | 996(16) |
| $CH_3OH$, vt=0-2 | 16(-2) − 16(1) E2, vt=0 | 109153.184(14e-3) | 342.0 | 14.726 | 151 | 8.8(0.1) | 6.0(0.2) | 972(30) |
| $HC_3N$ | 12 − 11 | 109173.634(1e-2) | 34.1 | 167.1 | 3208 | 9.5(0.) | 4.5(0.1) | 15237(29) |
| SO | 3(2) − 2(1) | 109252.220(1e-1) | 21.1 | 3.5585 | 2373 | 9.7(0.) | 5.5(0.1) | 14002(38) |
| $HC_3N$, $v_7$=1 | 12(-1) − 11(1) | 109442.013(2e-2) | 355.0 | 165.12 | 58 | 9.0(0.4) | 9.6(0.9) | 595(51) |
| OCS | 9 − 8 | 109463.063(5e-3) | 26.3 | 4.6034 | 600 | 9.5(0.) | 5.7(0.1) | 3618(40) |
| HNCO | 5(1, 5) − 4(1, 4) | 109495.996(6e-3) | 59.0 | 11.847 | 132 | 9.6(0.2) | 7.8(0.4) | 1101(49) |
| $C^{15}N$ | 1(2, 1) − 0(1, 0) | 110023.540(1e-1) | 5.3 | 1.386 | 34 | 10.0(0.1) | 0.5(0.4) | 93(18) |
| $C^{15}N$ | 1(2, 2) − 0(1, 1) | 110024.590(1e-1) | 5.3 | 3.504 | 50 | 10.4(0.4) | 5.7(1.1) | 305(48) |
| $^{13}CO$ | 1 − 0 | 110201.35(0) | 5.3 | 0.01220 | 25745 | 9.5(0.1) | 4.6(0.1) | 125640(1060) |
| $CH_3OCH_3$ | 8(2, 7) − 8(1, 8) EA | 109571.396(9e-3) | 38.3 | 23.947 | 46 | 9.0(0.6) | 4.3(1.0) | 212(69) |
| $CH_3OCH_3$ | 8(2, 7) − 8(1, 8) AE | 109571.403(9e-3) | 38.3 | 35.921 | blended | – | – | – |
| $CH_3OCH_3$ | 8(2, 7) − 8(1, 8) EE | 109574.088(7e-3) | 38.3 | 95.791 | 38 | 8.9(0.6) | 6.8(3.5) | 279(113) |
| $CH_3OCH_3$ | 8(2, 7) − 8(1, 8) AA | 109576.778(11e-3) | 38.3 | 59.869 | 41 | 9.0(0.6) | 3.6(1.6) | 161(63) |
| $HC_3N$, $v_7$=1 | 12(1) − 11(-1) | 109598.818(2e-2) | 355.0 | 165.12 | 45 | 9.5(0.5) | 9.0(1.4) | 435(52) |
| $NH_2CHO$ | 5(1, 4) − 4(1, 3) | 109753.549(25e-3) | 18.8 | 62.765 | 31 | 9.5(0.5) | 6.4(0.5) | 213(67) |
| $SO_2$ | 17(5, 13) − 18(4, 14) | 109757.585(2e-3) | 202.1 | 6.6069 | 174 | 9.0(0.5) | 5.4(0.5) | 1004(267) |
| $C^{18}O$ | 1 − 0 | 109782.173(6e-3) | 5.3 | 0.01221 | 4665 | 9.5(0.1) | 3.7(0.1) | 18226(0.3) |
| HNCO | 5(3, 2) − 4(3, 1) | 109833.487(7e-3) | 390.8 | 7.1906 | 24 | 9.0(0.9) | 6.8(1.7) | 176(44) |
| HNCO | 5(2, 3) − 4(2, 2) | 109872.765(3e-2) | 186.1 | 10.012 | 61 | 9.1(0.4) | 6.9(0.8) | 448(47) |
| HNCO | 5(2, 4) − 4(2, 3) | 109872.337(3e-2) | 186.1 | 10.013 | blended | – | – | – |
| HNCO | 5(0, 5) − 4(0, 4) | 109905.749(7e-3) | 15.8 | 12.482 | 599 | 9.0(0.) | 5.4(0.1) | 3409(52) |
| HNCO | 5(1, 4) − 4(1, 3) | 110298.089(5e-3) | 59.2 | 11.847 | 97 | 8.9(0.3) | 7.2(0.7) | 739(65) |
| $CH_3CN$ | 6(5, 0) − 5(5, 0) | 110330.345(0) | 197.1 | 56.399 | 41 | 9.5(0.5) | 8.1(0.5) | 351(112) |
| $CH_3CN$ | 6(4, 0) − 5(4, 0) | 110349.471(0) | 132.8 | 102.54 | 142 | 9.6(0.4) | 7.5(0.5) | 1129(112) |
| $CH_3CN$ | 6(3, 0) − 5(-3, 0) | 110364.354(0) | 82.8 | 138.45 | 532 | 9.6(0.5) | 6.4(0.5) | 3638(112) |
| $CH_3CN$ | 6(-3, 0) − 5(3, 0) | 110364.354(0) | 82.8 | 138.45 | blended | – | – | – |
| $CH_3CN$ | 6(2, 0) − 5(2, 0) | 110374.989(0) | 47.1 | 164.06 | 535 | 9.6(0.5) | 5.9(0.5) | 3383(112) |
| $CH_3CN$ | 6(1, 0) − 5(1, 0) | 110381.372(0) | 25.7 | 179.45 | 879 | 9.5(0.4) | 5.0(0.5) | 4632(112) |
| $CH_3CN$ | 6(0, 0) − 5(0, 0) | 110383.500(0) | 18.5 | 184.58 | 941 | 9.6(0.5) | 5.4(0.5) | 5385(112) |
| $CH_3OCHO$ | 9(7, 2) − 8(7, 1) E | 110525.741(1e-2) | 59.1 | 9.46492 | 33 | 9.0(1.1) | 3.9(1.1) | 137(37) |
| $CH_3OCHO$ | 9(7, 2) − 8(7, 1) A | 110535.186(1e-2) | 59.1 | 9.561 | 45 | 9.1(1.1) | 10.3(1.1) | 495(37) |
| $CH_3OCHO$ | 9(7, 3) − 8(7, 2) E | 110536.003(1e-2) | 59.1 | 9.46692 | blended | – | – | – |
| $CH_3OCHO$ | 9(2, 6) − 8(1, 5) E | 110550.203(1e-2) | 19.0 | 1.39763 | 23 | 9.0(1.1) | 6.2(1.1) | 151(37) |
| $CH_3OCHO$ | 9(2, 6) − 8(1, 5) A | 110560.051(1e-2) | 19.0 | 1.39665 | 15 | 9.0(1.1) | 5.7(1.1) | 185(37) |
| $CH_3OCHO$ | 9(6, 3) − 8(6, 2) E | 110652.813(1e-2) | 50.5 | 13.30853 | 31 | 9.1(1.1) | 10.5(2.3) | 340(67) |
| $CH_3OCHO$ | 9(6, 3) − 8(6, 2) A | 110663.429(1e-2) | 50.4 | 13.31127 | 75 | 9.2(0.4) | 10.2(1.1) | 815(70) |
| $CH_3OCHO$ | 9(6, 4) − 8(6, 3) A | 110663.273(1e-2) | 50.4 | 13.3113 | blended | – | – | – |
| $CH_3OCHO$ | 10(1,10) − 9(1, 9) E | 110788.664(1e-2) | 30.3 | 26.16584 | 74 | 9.1(0.2) | 3.0(0.6) | 233(43) |
| $CH_3OCHO$ | 10(1,10) − 9(1, 9) A | 110790.526(1e-2) | 30.3 | 26.17539 | 75 | 9.1(0.3) | 4.9(0.7) | 388(50) |
| $CH_3OCHO$ | 9(5, 4) − 8(5, 3) E | 110873.955(1e-2) | 43.2 | 16.55557 | 47 | 9.0(0.3) | 3.6(0.7) | 179(34) |
| $CH_3OCHO$ | 9(3, 7) − 8(3, 6) E | 110879.766(1e-2) | 32.6 | 21.245 | 98 | 9.0(0.2) | 4.9(0.5) | 506(49) |
| $CH_3OCHO$ | 9(5, 5) − 8(5, 4) A | 110880.447(1e-2) | 43.2 | 16.56015 | 55 | 9.0(0.4) | 3.9(1.1) | 228(51) |
| $CH_3OCHO$ | 9(3, 7) − 8(3, 6) A | 110887.092(1e-2) | 32.6 | 21.25577 | 71 | 9.0(0.3) | 4.7(0.6) | 354(41) |
| $CH_3OCHO$ | 9(5, 4) − 8(5, 3) A | 110890.256(1e-2) | 43.2 | 16.56106 | 50 | 9.0(0.4) | 3.8(0.9) | 205(38) |
| $C_2H_5CN$ | 15(6, 10) − 16(5, 11) | 111186.955(2e-1) | 91.6 | 2.6027 | 81 | 9.0(0.3) | 3.1(0.7) | 268(98) |
| $C_2H_5CN$ | 15(6, 9) − 16(5, 12) | 111188.164(4e-3) | 91.6 | 2.6027 | 97 | 9.0(0.3) | 6.9(1.4) | 715(127) |
| $CH_3OCHO$ | 9(4, 6) − 8(4, 5) A | 111195.962(1e-2) | 37.2 | 19.21722 | 73 | 9.0(0.5) | 5.6(0.5) | 433(17) |
| $CH_3OH$, vt=0-2 | $7(2)^+ − 8(1)^+$, vt=0 | 111289.453(13e-3) | 102.7 | 9.3425 | 439 | 8.8(0.1) | 8.2(0.3) | 3816(116) |
| $CH_3OCHO$ | 9(4, 5) − 8(4, 4) E | 111408.412(1e-2) | 37.3 | 18.18767 | 56 | 9.0(0.5) | 4.0(0.5) | 241(17) |
| $CH_3OCHO$ | 9(4, 5) − 8(4, 4) A | 111453.300(1e-2) | 37.2 | 19.21778 | 44 | 9.1(0.5) | 4.7(0.5) | 218(17) |
| $CH_3OH$, vt=0-2 | 17(-2) − 17(1) E2, vt=0 | 111626.514(15e-3) | 381.5 | 20.231 | 171 | 8.8(0.5) | 7.6(0.5) | 1390(19) |
| $CH_3OCHO$ | 9(1, 8) − 8(1, 7) E | 111674.131(1e-2) | 28.1 | 23.18984 | 76 | 9.1(0.4) | 5.7(0.5) | 466(19) |
| $CH_3OCHO$ | 9(1, 8) − 8(1, 7) A | 111682.189(1e-2) | 28.1 | 23.19587 | 79 | 9.0(0.5) | 4.7(0.5) | 401(19) |
| $CH_3OCH_3$ | 19(3,16) − 19(2,17) AE | 111741.351(26e-3) | 187.5 | 123.39211 | 52 | 9.0(0.5) | 4.4(0.5) | 245(23) |
| $CH_3OCH_3$ | 9(3,16) − 19(2,17) EE | 111742.794(25e-3) | 187.5 | 329.06069 | 72 | 9.1(0.4) | 5.4(0.5) | 414(23) |
| $CH_3OCH_3$ | 19(3, 16) − 19(2, 17) AA | 111744.238(29e-3) | 187.5 | 205.6671 | 60 | 9.0(0.5) | 3.7(0.5) | 240(23) |
| $SO_2$ | 31(3, 29) − 30(4, 26) | 111755.021(2e-3) | 476.9 | 6.4499 | 105 | 8.8(0.5) | 6.4(0.5) | 72-(23) |
| t-HCOOH | 5(0, 5) − 4(0, 4) | 111746.784(3e-3) | 16.1 | 10.029 | 49 | 9.5(0.5) | 10.7(0.5) | 1129(23) |
| $CH_3OCH_3$ | 7(0, 7) − 6(1, 6) AA | 111782.562(8e-3) | 25.2 | 53.86755 | 170 | 9.0(0.5) | 7.1(0.5) | 1281(23) |
| $CH_3OCH_3$ | 7(5, 3) − 8(4, 5) AA | 111804.354(33e-3) | 60.6 | 3.07241 | 35 | 9.1(0.3) | 3.0(0.5) | 113(14) |
| $CH_3OCH_3$ | 7(5, 3) − 8(4, 5) EE | 111804.813(26e-3) | 60.6 | 7.72103 | blended | – | – | – |
| $CH_3OCH_3$ | 7(5, 2) − 8(4, 5) AA | 111809.374(33e-3) | 60.6 | 5.12083 | 54 | 9.1(0.5) | 6.5(0.5) | 372(14) |
| $CH_3OCH_3$ | 7(5, 2) − 8(4, 5) EE | 111812.674(31e-3) | 60.6 | 0.47164 | 15 | 9.0(0.5) | 7.8(0.5) | 121(14) |
| $C_2H_5OH$ | 12(3, 9) − 12(2, 10) | 112129.544(5e-2) | 77.1 | 16.463 | 30 | 8.9(1.7) | 10.3(4.8) | 326(118) |
| $CH_3OH$, vt=0-2 | $19(0)^+ − 18(2)^+$, vt=0 | 112145.638(21e-3) | 440.1 | 0.00059 | 39 | 8.9(0.9) | 5.0(2.1) | 208(76) |
| $CH_3CHO$ | 6(1, 6) − 5(1, 5) A, vt=0 | 112248.716(3e-3) | 21.1 | 73.76807 | 192 | 9.7(0.2) | 3.7(0.5) | 767(95) |
| $CH_3CHO$ | 6(1, 6) − 5(1, 5) E, vt=0 | 112254.508(3e-3) | 21.2 | 73.79585 | 189 | 9.7(0.3) | 4.3(0.6) | 860(108) |
| t-HCOOH | 5(2, 4) − 4(2, 3) | 112287.145 (3e-3) | 28.9 | 8.4851 | 52 | 9.5(0.7) | 9.0(1.5) | 495(78) |
| $C^{17}O$ | 1 − 0 | 112359.284(1e-3) | 5.4 | 0.01217 | 996 | 9.7(0.1) | 5.1(0.2) | 5437(165) |
| t-HCOOH | 5(2, 3) − 4(2, 2) | 112891.443 (3e-3) | 28.9 | 8.4849 | 51 | 9.5(0.8) | 1.4(1.3) | 79(70) |
| $CH_3OCH_3$ | 20(3, 17) − 20(2, 18) EE | 113000.970(32e-3) | 206.1 | 348.88725 | 35 | 9.1(0.4) | 3.0(0.5) | 114(21) |
| $CH_3OCH_3$ | 17(3, 14) − 17(2, 15) EA | 113057.427(19e-3) | 153.1 | 70.07874 | 41 | 9.1(0.5) | 1.0(0.5) | 43(21) |
| $CH_3OCH_3$ | 17(3, 14) − 17(2, 15) AE | 113057.433(18e-3) | 153.1 | 105.12023 | blended | – | – | – |
| $CH_3OCH_3$ | 17(3, 14) − 17(2, 15) EE | 113059.249(17e-3) | 153.1 | 280.33166 | 54 | 9.1(0.5) | 4.2(0.5) | 245(21) |
| $CH_3OCH_3$ | 17(3, 14) − 17(2, 15) AA | 113061.072(22e-3) | 153.1 | 221.33 | 37 | 9.0(0.8) | 2.7(0.5) | 108(21) |
| $C_2H_5OH$ | 10(2, 9) − 12(1, 10) | 113098.078(5e-2) | 51.0 | 8.3566 | 187 | 8.9(0.5) | 7.3(0.5) | 1457(21) |
| CN | N= 1-0, J=1/2-1/2, F=1/2-1/2 | 113123.370(6e-3) | 5.4 | 0.15271 | 379 | 9.4(0.5) | 4.6(0.5) | 1857(210) |
| CN | N= 1-0, J=1/2-1/2, F=1/2-3/2 | 113144.157(6e-3) | 5.4 | 1.2492 | 1741 | 9.4(0.5) | 4.7(0.5) | 8684(210) |
| CN | N= 1-0, J=1/2-1/2, F=3/2-1/2 | 113170.492(4e-3) | 5.4 | 1.2199 | 1955 | 9.4(0.5) | 4.5(0.5) | 9263(210) |
| CN | N= 1-0, J=1/2-1/2, F=3/2-3/2 | 113191.279(3e-3) | 5.4 | 1.5836 | 1935 | 9.4(0.5) | 4.8(0.5) | 9901(210) |
| CCS | 9(8) − 8(7) | 113410.186(2e-2) | 33.6 | 65.427 | 54 | 9.5(0.4) | 6.3(0.5) | 363(254) |
| CN | N= 1-0, J=3/2-1/2, F=3/2-1/2 | 113488.120(3e-3) | 5.4 | 1.5838 | 1968 | 9.4(0.6) | 4.3(0.5) | 8979(254) |
| CN | N= 1-0, J=3/2-1/2, F=5/2-3/2 | 113490.970(2e-3) | 5.4 | 4.205 | 3279 | 9.4(0.5) | 5.6(0.5) | 19712(254) |
| CN | N= 1-0, J=3/2-1/2, F=1/2-1/2 | 113499.644(3e-3) | 5.4 | 1.2491 | 1190 | 9.4(0.4) | 4.9(0.5) | 6214(254) |
| CN | N= 1-0, J=3/2-1/2, F=3/2-3/2 | 113508.907(3e-3) | 5.4 | 1.2196 | 1587 | 9.4(0.5) | 4.7(0.5) | 7995(254) |
| CN | N= 1-0, J=3/2-1/2, F=1/2-3/2 | 113520.432(4e-3) | 5.4 | 0.15263 | 286 | 9.4(0.5) | 4.4(0.5) | 1350(254) |
| | | G092.67+03.07 | | | | | | |
| CCS | 8(9) − 7(8) | 106347.726(2e-2) | 25.0 | 74.425 | 113 | -6.0(0.1) | 2.1(0.2) | 254(20) |
| $^{34}SO$ | 3(2) − 2(1) | 106743.244(7e-2) | 20.9 | 3.557 | 38 | -6.5(0.2) | 2.8(0.6) | 114(20) |
| $CH_3OH$, vt=0-2 | $3(1)^+ − 4(0)^+$, vt=0 | 107013.831(1e-2) | 28.3 | 12.036 | 201 | -6.5(0.1) | 5.3(0.1) | 1132(25) |
| $CH_3OH$, vt=0-2 | 15(-2) − 15(1) E2, vt=0 | 107159.906(14e-3) | 304.7 | 10.421 | 21 | -6.5(0.5) | 4.1(1.0) | 89(22) |
| t-HCOOH | 5(1, 5) − 4(1, 4) | 108126.720(3e-3) | 18.8 | 9.6966 | 35 | -5.7(0.3) | 3.5(0.8) | 130(23) |

**Table A2.** (Continued)

| Species | Transitions | Rest Freq. (MHz) | $E_u$ (K) | $\mu^2S$ ($D^2$) | $T_{mb}$ (mK) | $V_{LSR}$ (km $s^{-1}$) | $\Delta V$ (km $s^{-1}$) | $\int T_{mb}$ dv (mK km $s^{-1}$) |
|---|---|---|---|---|---|---|---|---|
| $^{13}$CN | 1(1, 1) − 0(1, 0), F = 0 − 1 | 108631.121(5e-2) | 5.2 | 0.642 | 30 | -5.8(0.5) | 1.5(0.5) | 47(8) |
| $^{13}$CN | 1(1, 1) − 0(1, 0), F = 1 − 1 | 108636.923(5e-2) | 5.2 | 1.932 | 45 | -5.8(0.5) | 2.5(0.5) | 121(8) |
| $^{13}$CN | 1(2, 1) − 0(1, 1), F = 1 − 0 | 108638.212(5e-2) | 5.2 | 0.722 | 20 | -5.7(0.5) | 2.7(0.5) | 59(8) |
| $^{13}$CN | 1(2, 1) − 0(1, 1), F = 2 − 1 | 108643.590(5e-2) | 5.2 | 0.856 | 11 | -5.8(0.5) | 3.0(0.5) | 37(8) |
| $^{13}$CN | 1(2, 1) − 0(1, 1), F = 0 − 1 | 108644.346(5e-2) | 5.2 | 0.642 | 27 | -5.8(0.5) | 5.4(0.5) | 155(8) |
| $^{13}$CN | 1(2, 1) − 0(1, 1), F = 1 − 1 | 108645.064(5e-2) | 5.2 | 0.551 | blended | – | – | – |
| $^{13}$CN | 1(1, 1) − 0(1, 0), F = 2 − 1 | 108651.297(5e-2) | 5.2 | 3.276 | 67 | -5.6(0.5) | 2.1(0.5) | 154(8) |
| $^{13}$CN | 1(2, 1) − 0(1, 1), F = 2 − 2 | 108657.646(5e-2) | 5.2 | 2.420 | 52 | -5.8(0.5) | 3.0(0.5) | 166(8) |
| $^{13}$CN | 1(2, 1) − 0(1, 1), F = 1 − 2 | 108658.948(5e-2) | 5.2 | 0.669 | 20 | -5.6(0.5) | 2.3(0.5) | 47(8) |
| $^{13}$CN | 1(2, 2) − 0(1, 1), F = 3 − 2 | 108780.201(5e-2) | 5.2 | 4.905 | 102 | -5.7(0.2) | 2.2(0.5) | 241(39) |
| $^{13}$CN | 1(2, 2) − 0(1, 1), F = 2 − 1 | 108782.374(5e-2) | 5.2 | 2.586 | 51 | -5.6(0.4) | 3.0(1.3) | 160(48) |
| $^{13}$CN | 1(2, 2) − 0(1, 1), F = 1 − 0 | 108786.982(5e-2) | 5.2 | 1.144 | 14 | -5.7(0.7) | 6.4(3.3) | 96(10) |
| $^{13}$CN | 1(2, 2) − 0(1, 1), F = 1 − 1 | 108793.753(5e-2) | 5.2 | 0.894 | 29 | -5.6(0.7) | 2.5(1.1) | 78(36) |
| $^{13}$CN | 1(2, 2) − 0(1, 1), F = 2 − 2 | 108796.400(5e-2) | 5.2 | 0.918 | 86 | -5.8(2.9) | 4.3(0.8) | 55(39) |
| $CH_3OH$, vt=0-2 | 0(0) − 1(-1) E2, vt=0 | 108893.945(12e-3) | 13.1 | 3.9134 | 443 | -6.3(0.) | 4.0(0.1) | 1876(33) |
| $HC_3N$ | 12 − 11 | 109173.634(1e-2) | 34.1 | 167.1 | 3091 | -6.1(0.) | 2.4(0.1) | 7883(38) |
| SO | 3(2) − 2(1) | 109252.220(1e-1) | 21.1 | 3.5585 | 751 | -6.0(0.) | 3.5(0.1) | 2800(74) |
| OCS | 9 − 8 | 109463.063(5e-3) | 26.3 | 4.6034 | 203 | -5.8(0.1) | 3.7(0.2) | 801(34) |
| $C^{18}O$ | 1 − 0 | 109782.173(6e-3) | 5.3 | 0.01221 | 1833 | -6.0(0.1) | 2.4(0.1) | 4748(29) |
| HNCO | 5(0, 5) − 4(0, 4) | 109905.749(7e-3) | 15.8 | 12.482 | 230 | -6.0(0.1) | 3.4(0.2) | 825(34) |
| $C^{15}N$ | 1(2, 1) − 0(1, 0) | 110023.540(1e-1) | 5.3 | 1.386 | 21 | -5.9(1.1) | 5.8(1.7) | 129(43) |
| $C^{15}N$ | 1(2, 2) − 0(1, 1) | 110024.590(1e-1) | 5.3 | 3.504 | 57 | -6.1(0.1) | 1.1(0.4) | 66(24) |
| $^{13}$CO | 1 − 0 | 110201.35(0) | 5.3 | 0.01220 | 18817 | -6.0(0.1) | 2.5(0.1) | 49959(137) |
| $CH_3CN$ | 6(4, 0) − 5(4, 0) | 110349.471(0) | 132.8 | 102.54 | 28 | -6.0(0.5) | 4.1(0.5) | 123(51) |
| $CH_3CN$ | 6(3, 0) − 5(-3, 0) | 110364.354(0) | 82.8 | 138.45 | 147 | -6.0(0.7) | 4.7(0.5) | 729(51) |
| $CH_3CN$ | 6(-3, 0) − 5(3, 0) | 110364.354(0) | 82.8 | 138.45 | blended | – | – | – |
| $CH_3CN$ | 6(2, 0) − 5(2, 0) | 110374.989(0) | 47.1 | 164.06 | 183 | -6.0(0.5) | 4.2(0.5) | 818(51) |
| $CH_3CN$ | 6(1, 0) − 5(1, 0) | 110381.372(0) | 25.7 | 179.45 | 404 | -6.0(0.4) | 3.5(0.5) | 1490(51) |
| $CH_3CN$ | 6(0, 0) − 5(0, 0) | 110383.500(0) | 18.5 | 184.58 | 476 | -6.0(0.5) | 3.5(0.5) | 1779(51) |
| $CH_3OH$, vt=0-2 | $7(2)^+ - 8(1)^+$, vt=0 | 111289.453(13e-3) | 102.7 | 9.3425 | 59 | -6.5(0.5) | 3.9(0.9) | 246(60) |
| t-HCOOH | 5(0, 5) − 4(0, 4) | 111746.784(3e-3) | 16.1 | 10.092 | 23 | -6.1(0.8) | 3.0(1.2) | 73(32) |
| $CH_3OCH_3$ | 7(0, 7) − 6(1, 6) AA | 111782.562(8e-3) | 25.2 | 68.047 | 43 | -6.0(0.4) | 3.6(0.7) | 166(36) |
| $CH_3CHO$ | 6(1, 6) − 5(1, 5) A, vt=0 | 112248.716(3e-3) | 21.1 | 73.76807 | 106 | -6.2(0.1) | 2.7(0.4) | 306(36) |
| $CH_3CHO$ | 6(1, 6) − 5(1, 5) E, vt=0 | 112254.508(3e-3) | 21.2 | 73.79585 | 128 | -6.0(0.1) | 3.8(0.4) | 514(45) |
| $C^{17}O$ | 1 − 0 | 112359.284(1e-3) | 5.4 | 0.01217 | 400 | -6.2(0.1) | 2.1(0.3) | 470(70) |
| CN | N= 1-0, J=1/2-1/2, F=1/2-1/2 | 113123.370(6e-3) | 5.4 | 0.15271 | 425 | -5.8(0.5) | 2.9(0.5) | 1290(140) |
| CN | N= 1-0, J=1/2-1/2, F=1/2-3/2 | 113144.157(6e-3) | 5.4 | 1.2492 | 1677 | -5.8(0.6) | 2.8(0.5) | 4997(140) |
| CN | N= 1-0, J=1/2-1/2, F=3/2-1/2 | 113170.492(4e-3) | 5.4 | 1.2199 | 1776 | -5.8(0.5) | 2.8(0.5) | 5224(140) |
| CN | N= 1-0, J=1/2-1/2, F=3/2-3/2 | 113191.279(3e-3) | 5.4 | 1.5836 | 1815 | -5.8(0.5) | 2.8(0.5) | 5425(140) |
| CCS | 9(8) − 8(7) | 113410.186(2e-2) | 33.6 | 65.427 | 51 | -6.1(0.5) | 7.7(0.5) | 417(191) |
| CN | N= 1-0, J=3/2-1/2, F=3/2-1/2 | 113488.120(3e-3) | 5.4 | 1.5838 | 1627 | -5.8(0.5) | 3.0(0.5) | 5.2(191) |
| CN | N= 1-0, J=3/2-1/2, F=5/2-3/2 | 113490.970(2e-3) | 5.4 | 4.205 | 3466 | -5.8(0.) | 2.8(0.5) | 10513(191) |
| CN | N= 1-0, J=3/2-1/2, F=1/2-1/2 | 113499.644(3e-3) | 5.4 | 1.2491 | 1223 | -5.7(0.5) | 2.9(0.5) | 3713(191) |
| CN | N= 1-0, J=3/2-1/2, F=3/2-3/2 | 113508.907(3e-3) | 5.4 | 1.2196 | 1470 | -5.8(0.3) | 2.8(0.5) | 4339(191) |
| CN | N= 1-0, J=3/2-1/2, F=1/2-3/2 | 113520.432(4e-3) | 5.4 | 0.15263 | 255 | -5.8(0.5) | 3.9(0.5) | 1049(191) |
| | | G109.87+02.11 | | | | | | |
| CCS | 8(9) − 7(8) | 106347.726(2e-2) | 25.0 | 74.425 | 60 | -11.0(0.3) | 2.5(0.5) | 162((33) |
| $HC_5N$ | 40 − 39 | 106498.910(7e-3) | 104.8 | 2249.7 | 41 | -10.5(0.3) | 4.2(0.8) | 181(25) |
| $^{34}$SO | 3(2) − 2(1) | 106743.244(7e-2) | 20.9 | 3.557 | 73 | -10.8(0.2) | 4.7(0.4) | 364(26) |
| $CH_3C^{15}N$ | 6(5) − 5(5) | 107010.770(6e-2) | 196.9 | 56.494 | 5554 | -10.5(0.1) | 1.0(0.1) | 60(23) |
| $CH_3OH$, vt=0-2 | $3(1)^+ - 4(0)^+$, vt=0 | 107013.831(1e-2) | 28.3 | 12.036 | 142 | -11.1(1.1) | 4.1(1.1) | 627(73) |
| $SO_2$ | 27(3, 25) − 26(4, 22) | 107060.208(2e-3) | 369.4 | 8.2723 | 53 | -9.2(0.3) | 9.2(0.9) | 520(39) |
| $CH_3OH$, vt=0-2 | 15(-2) − 15(1) E2, vt=0 | 107159.906(14e-3) | 304.7 | 10.421 | 48 | -11.0(0.2) | 3.5(0.4) | 176(19) |
| $SO_2$ | 12(4, 8) − 13(3, 11) | 107843.470(2e-3) | 111.0 | 4.5354 | 129 | -9.0(0.1) | 9.1(0.3) | 1250(31) |
| t-HCOOH | 5(1, 5) − 4(1, 4) | 108126.720(3e-3) | 18.8 | 9.6966 | 38 | -10.8(0.3) | 5.1(0.9) | 210(26) |
| $^{13}$CN | 1(1, 0) − 0(1, 1), F = 1 − 0 | 108406.091(5e-2) | 5.2 | 0.191 | 22 | -11.0(0.4) | 4.3(2.2) | 100(31) |
| $^{13}$CN | 1(1, 0) − 0(1, 1), F = 1 − 1 | 108412.862(5e-2) | 5.2 | 0.635 | 18 | -11.0(0.8) | 5.5(2.7) | 103(31) |
| $^{13}$CN | 1(1, 0) − 0(1, 1), F = 1 − 2 | 108426.889(5e-2) | 5.2 | 1.267 | 29 | -10.7(0.5) | 7.7(1.6) | 241(33) |
| $^{13}$CN | 1(1, 1) − 0(1, 0), F = 0 − 1 | 108631.121(5e-2) | 5.2 | 0.642 | 18 | -10.5(0.5) | 3.3(0.9) | 63(17) |
| $^{13}$CN | 1(1, 1) − 0(1, 0), F = 1 − 1 | 108636.923(5e-2) | 5.2 | 1.932 | 54 | -10.8(0.2) | 1.5(0.3) | 86(17) |
| $^{13}$CN | 1(2, 1) − 0(1, 1), F = 1 − 0 | 108638.212(5e-2) | 5.2 | 0.722 | 43 | -10.5(0.2) | 2.1(0.5) | 96(20) |
| $^{13}$CN | 1(2, 1) − 0(1, 1), F = 2 − 1 | 108643.590(5e-2) | 5.2 | 0.856 | 30 | -10.5(0.2) | 1.2(0.5) | 38(18) |
| $^{13}$CN | 1(2, 1) − 0(1, 1), F = 0 − 1 | 108644.346(5e-2) | 5.2 | 0.642 | 30 | -10.8(0.3) | 2.1(1.2) | 67(30) |
| $^{13}$CN | 1(2, 1) − 0(1, 1), F = 1 − 1 | 108645.064(5e-2) | 5.2 | 0.551 | 24 | -10.5(0.4) | 1.8(0.7) | 47(20) |
| $^{13}$CN | 1(1, 1) − 0(1, 0), F = 2 − 1 | 108651.297(5e-2) | 5.2 | 3.276 | 79 | -11.0(0.1) | 3.9(0.3) | 331(20) |
| $^{13}$CN | 1(2, 1) − 0(1, 1), F = 2 − 2 | 108657.646(5e-2) | 5.2 | 2.420 | 37 | -11.0(0.2) | 1.1(0.4) | 44(18) |
| $^{13}$CN | 1(2, 1) − 0(1, 1), F = 1 − 2 | 108658.948(5e-2) | 5.2 | 0.669 | 38 | -10.8(0.4) | 5.5(0.7) | 221(31) |
| $^{13}$CN | 1(2, 2) − 0(1, 1), F = 3 − 2 | 108780.201(5e-2) | 5.2 | 4.905 | 105 | -11.1(0.1) | 3.6(0.3) | 407(26) |
| $^{13}$CN | 1(2, 2) − 0(1, 1), F = 2 − 1 | 108782.374(5e-2) | 5.2 | 2.586 | 59 | -11.0(0.2) | 2.6(0.4) | 165(22) |
| $^{13}$CN | 1(2, 2) − 0(1, 1), F = 1 − 0 | 108786.982(5e-2) | 5.2 | 1.144 | 24 | -11.0(0.4) | 2.7(0.8) | 67(21) |
| $^{13}$CN | 1(2, 2) − 0(1, 1), F = 1 − 1 | 108793.753(5e-2) | 5.2 | 0.894 | 25 | -10.9(0.3) | 0.8(0.6) | 21(11) |
| $^{13}$CN | 1(2, 2) − 0(1, 1), F = 2 − 2 | 108796.400(5e-2) | 5.2 | 0.918 | 18 | -11.0(0.5) | 3.0(0.7) | 59(20) |
| $CH_3OH$, vt=0-2 | 0(0) − 1(-1) E2, vt=0 | 108893.945(12e-3) | 13.1 | 3.9134 | 174 | -11.0(0.1) | 4.3(0.3) | 790(40) |
| $CH_3OH$, vt=0-2 | 14(5) − 15(4) E1, vt=0 | 109138.783(15e-3) | 379.7 | 13.593 | 69 | -11.2(1.1) | 2.9(1.1) | 214(76) |
| $CH_3OH$, vt=0-2 | 16(-2) − 16(1) E2, vt=0 | 109153.184 (14e-3) | 342.0 | 14.726 | 55 | -11.0(1.0) | 2.9(1.1) | 166(76) |
| $HC_5N$ | 41 − 40 | 109160.973(7e-3) | 110.0 | 2306 | 19 | -10.5(0.1) | 5.8(1.1) | 120(76) |
| $HC_3N$ | 12 − 11 | 109173.634(1e-2) | 34.1 | 167.1 | 2335 | -11.0(0.3) | 4.0(1.1) | 9937(76) |
| SO | 3(2) − 2(1) | 109252.220(1e-1) | 21.1 | 3.5585 | 1293 | -11.0(0.) | 4.8(0.1) | 6661(102) |
| $HC_3N$, $v_7$=1 | 12(-1) − 11(1) | 109442.013(2e-2) | 355.0 | 165.12 | 31 | -11.0(0.5) | 8.9(0.5) | 294(12) |
| OCS | 9 − 8 | 109463.063(5e-3) | 26.3 | 4.6034 | 111 | -11.2(0.5) | 4.4(0.5) | 516(12) |
| HNCO | 5(1, 5) − 4(1, 4) | 109495.996(6e-3) | 59.0 | 11.847 | 34 | -10.0(0.5) | 5.1(0.5) | 185(12) |
| $HC_3N$, $v_7$=1 | 12(1) − 11(-1) | 109598.818(2e-2) | 355.0 | 165.12 | 47 | -11.0(0.2) | 4.5(0.6) | 225(23) |
| $SO_2$ | 17(5, 13) − 18(4, 14) | 109757.585(2e-3) | 202.1 | 6.6069 | 106 | -9.0(0.2) | 7.7(0.5) | 861(45) |
| $C^{18}O$ | 1 − 0 | 109782.173(6e-3) | 5.3 | 0.01221 | 4636 | -11.8(0.1) | 3.4(0.1) | 16543(27) |
| HNCO | 5(2, 3) − 4(2, 2) | 109872.765(3e-2) | 186.1 | 10.012 | 37 | -10.0(0.4) | 3.9(0.9) | 154(35) |
| HNCO | 5(2, 4) − 4(2, 3) | 109872.337(3e-2) | 186.1 | 10.013 | blended | – | – | – |
| HNCO | 5(0, 5) − 4(0, 4) | 109905.749(7e-3) | 15.8 | 12.482 | 183 | -10.2(0.2) | 2.9(0.5) | 567(79) |
| $C^{15}N$ | 1(2, 1) − 0(1, 0) | 110023.540(1e-1) | 5.3 | 1.386 | 40 | -10.9(0.3) | 2.1(0.8) | 92(33) |
| $C^{15}N$ | 1(2, 2) − 0(1, 1) | 110024.590(1e-1) | 5.3 | 3.504 | 71 | -10.5(0.2) | 3.5(0.5) | 264(32) |
| $^{13}$CO | 1 − 0 | 110201.35(0) | 5.3 | 0.01220 | 20251 | -11.0(0.1) | 4.5(0.1) | 97104(539) |
| HNCO | 5(1, 4) − 4(1, 3) | 110298.089(5e-3) | 59.2 | 11.847 | 63 | -10.0(0.5) | 7.2(0.5) | 484(23) |
| $CH_3CN$ | 6(5, 0) − 5(5, 0) | 110330.345(0) | 197.1 | 56.399 | blended | – | – | – |
| $CH_3CN$ | 6(4, 0) − 5(4, 0) | 110349.471(0) | 132.8 | 102.54 | 46 | -11.2(0.7) | 6.6(0.5) | 1163(49) |
| $CH_3CN$ | 6(3, 0) − 5(-3, 0) | 110364.354(0) | 82.8 | 138.45 | 139 | -11.1(0.5) | 5.5(0.5) | 812(49) |
| $CH_3CN$ | 6(-3, 0) − 5(3, 0) | 110364.354(0) | 82.8 | 138.45 | blended | – | – | – |

**Table A2.** (Continued)

| Species | Transitions | Rest Freq. (MHz) | $E_u$ (K) | $\mu^2S$ ($D^2$) | $T_{mb}$ (mK) | $V_{LSR}$ (km $s^{-1}$) | $\Delta V$ (km $s^{-1}$) | $\int T_{mb}$ dv (mK km $s^{-1}$) |
|---|---|---|---|---|---|---|---|---|
| $CH_3CN$ | 6(2, 0) − 5(2, 0) | 110374.989(0) | 47.1 | 164.06 | 152 | -11.2(0.5) | 5.2(0.5) | 842(49) |
| $CH_3CN$ | 6(1, 0) − 5(1, 0) | 110381.372(0) | 25.7 | 179.45 | 379 | -11.2(0.4) | 3.9(0.5) | 1588(49) |
| $CH_3CN$ | 6(0, 0) − 5(0, 0) | 110383.500(0) | 18.5 | 184.58 | 311 | -11.2(0.5) | 4.0(0.5) | 1321(49) |
| $CH_3OH$, vt=0-2 | $7(2)^+ - 8(1)^+$, vt=0 | 111289.453(13e-3) | 102.7 | 9.3425 | 162 | -10.9(0.1) | 4.6(0.3) | 800(35) |
| $CH_3OH$, vt=0-2 | 17(-2) − 17(1) E2, vt=0 | 111626.514(15e-3) | 381.5 | 20.231 | 81 | -11.0(0.1) | 2.5(0.6) | 216(35) |
| t-HCOOH | 5(0, 5) − 4(0, 4) | 111746.784(3e-3) | 16.1 | 10.092 | 42 | -10.9(0.3) | 1.8(0.7) | 81(26) |
| $SO_2$ | 31(3, 29) − 30(4, 26) | 111755.021(2e-3) | 476.9 | 6.4499 | 34 | -9.2(0.4) | 2.9(1.6) | 105(39) |
| $HC_5N$ | 42 − 41 | 111823.024(0) | 115.4 | 2362.2 | 18 | -10.5(0.8) | 3.1(0.9) | 61(27) |
| $CH_3CHO$ | 6(1, 6) − 5(1, 5) A, vt=0 | 112248.716(3e-3) | 21.1 | 73.76808 | 44 | -11.3(0.5) | 4.2(0.5) | 198(17) |
| $CH_3CHO$ | 6(1, 6) − 5(1, 5) E, vt=0 | 112254.508(3e-3) | 21.2 | 73.79585 | 33 | -11.3(0.5) | 5.0(0.5) | 176(17) |
| t-HCOOH | 5(2, 4) − 4(2, 3) | 112287.145 (3e-3) | 28.9 | 8.4851 | 39 | -10.9(0.2) | 1.9(0.5) | 81(21) |
| $C^{17}O$ | 1 − 0 | 112359.284(1e-3) | 5.4 | 0.01217 | 1016 | -11.2(0.1) | 5.4(0.1) | 5799(41) |
| CN | N= 1-0, J=1/2-1/2, F=1/2-1/2 | 113123.370(6e-3) | 5.4 | 0.15271 | 396 | -11.0(0.3) | 3.5(0.5) | 1459(159) |
| CN | N= 1-0, J=1/2-1/2, F=1/2-3/2 | 113144.157(6e-3) | 5.4 | 1.2492 | 1479 | -11.0(0.5) | 4.4(0.5) | 7001(159) |
| CN | N= 1-0, J=1/2-1/2, F=3/2-1/2 | 113170.492(4e-3) | 5.4 | 1.2199 | 1604 | -11.0(0.6) | 4.4(0.5) | 7526(159) |
| CN | N= 1-0, J=1/2-1/2, F=3/2-3/2 | 113191.279(3e-3) | 5.4 | 1.5836 | 1597 | -11.0(0.5) | 4.6(0.5) | 7809(159) |
| CN | N= 1-0, J=3/2-1/2, F=3/2-1/2 | 113488.120(3e-3) | 5.4 | 1.5838 | 1495 | -11.0(0.5) | 4.4(0.5) | 7976(312) |
| CN | N= 1-0, J=3/2-1/2, F=5/2-3/2 | 113490.970(2e-3) | 5.4 | 4.205 | 2224 | -11.0(0.5) | 5.7(0.5) | 13535(312) |
| CN | N= 1-0, J=3/2-1/2, F=1/2-1/2 | 113499.644(3e-3) | 5.4 | 1.2491 | 1139 | -11.0(0.9) | 4.5(0.5) | 5421(312) |
| CN | N= 1-0, J=3/2-1/2, F=3/2-3/2 | 113508.907(3e-3) | 5.4 | 1.2196 | 1282 | -11.0(0.5) | 4.6(0.5) | 6232(312) |
| CN | N= 1-0, J=3/2-1/2, F=1/2-3/2 | 113520.432(4e-3) | 5.4 | 0.15263 | 324 | -11.0(0.5) | 3.7(0.5) | 1269(312) |
| | | G111.54+00.77 | | | | | | |
| $NH_2CHO$ | 5(2, 4) − 4(2, 3) | 105972.665(37e-3) | 27.2 | 54.915 | 27 | -58.0(0.4) | 1.4(0.9) | 40(21) |
| $NH_2CHO$ | 5(4, 1) − 4(4, 0) | 106107.870(88e-3) | 63.0 | 23.537 | 24 | -58.0(0.3) | 5.7(0.6) | 142(15) |
| $NH_2CHO$ | 5(4, 2) − 4(4, 1) | 106107.845(88e-3) | 63.0 | 23.537 | blended | – | – | – |
| $NH_2CHO$ | 5(3, 3) − 4(3, 2) | 106134.468(55e-3) | 42.1 | 41.845 | 96 | -58.1(0.7) | 5.3(1.3) | 54(15) |
| $NH_2CHO$ | 5(3, 2) − 4(3, 1) | 106141.442(55e-3) | 42.1 | 41.84 | 22 | -58.0(0.3) | 4.8(0.8) | 113(17) |
| CCS | 8(9) − 7(8) | 106347.726(2e-2) | 25.0 | 74.425 | 57 | -57.1(0.1) | 3.8(0.3) | 234(14) |
| $NH_2CHO$ | 5(2, 3) − 4(2, 2) | 106541.773(37e-3) | 27.2 | 54.915 | 19 | 58.0(0.4) | 2.9(0.6) | 61(14) |
| $C_2H_5OH$ | 13(1, 12) − 13(0, 13) | 106649.479(5e-2) | 79.4 | 10.463 | 27 | -57.5(0.5) | 6.6(1.7) | 189(32) |
| $C_2H_5OH$ | 6(1, 5) − 5(1, 4) | 106676.542(5e-2) | 76.1 | 9.325 | 19 | -57.5(0.7) | 6.8(2.2) | 138(30) |
| $C_2H_5OH$ | 9(2, 8) − 9(1, 9) | 106723.558(5e-2) | 42.7 | 7.9044 | 23 | -57.5(0.2) | 2.6(0.5) | 54(13) |
| H$\alpha$ | H (39) $\alpha$ | 106737.357(0) | – | – | 224 | -63.7(0.2) | 26.6(0.7) | 4432(182) |
| $C_2H_5OH$ | 6(1, 5) − 5(1, 4) | 106767.234(5e-2) | 80.7 | 9.6466 | 24 | -57.5(0.3) | 3.6(1.0) | 93(21) |
| $CH_3OCH_3$ | 9(1, 8) − 8(2, 7) AA | 106775.602(14e-3) | 43.4 | 36.603 | 16 | -57.8(0.5) | 5.3(0.5) | 88(82) |
| $CH_3OCH_3$ | 9(1, 8) − 8(2, 7) EE | 106777.344(9e-3) | 43.4 | 58.573 | 26 | -57.8(0.5) | 5.1(0.5) | 141(82) |
| $CH_3OCH_3$ | 9(1, 8) − 8(2, 7) EA | 106779.091(11e-3) | 43.4 | 21.963 | 22 | -57.9(0.5) | 3.2(0.5) | 76(82) |
| $CH_3OCH_3$ | 9(1, 8) − 8(2, 7) EE | 106779.083(11e-3) | 43.4 | 14.645 | blended | – | – | – |
| $CH_3OH$, vt=0-2 | $3(1)^+ - 4(0)^+$, vt=0 | 107013.831(1e-2) | 28.3 | 12.036 | 3200 | -58.2(0.) | 5.1(0.1) | 17510(16) |
| $CH_3OH$, vt=0-2 | 15(-2) − 15(1) E2, vt=0 | 107159.906(14e-3) | 304.7 | 10.421 | 44 | -58.1(0.2) | 2.4(0.4) | 109(18) |
| $CH_3OCHO$ | 9( 2, 8) − 8( 2, 7) E | 107537.258(1e-2) | 28.8 | 22.60702 | 53 | -58.5(0.1) | 3.2(0.3) | 181(13) |
| $CH_3OCHO$ | 9( 2, 8) − 8( 2, 7) A | 107543.711(1e-2) | 28.8 | 22.61344 | 58 | -58.5(0.1) | 2.9(0.2) | 178(12) |
| $SO_2$ | 12(4, 8) − 13(3, 11) | 107843.470(2e-3) | 111.0 | 4.5354 | 16 | -52.0(0.7) | 5.2(1.4) | 87(22) |
| t-HCOOH | 5(1, 5) − 4(1, 4) | 108126.720(3e-3) | 18.8 | 9.6966 | 27 | -58.6(0.3) | 4.1(0.6) | 118(17) |
| $C_2H_5OH$ | 13(3, 10) − 13(2, 11) | 108438.579(5e-2) | 88.2 | 18.79 | 22 | -57.5(0.3) | 0.8(0.7) | 18(16) |
| $^{13}CN$ | 1(1, 1) − 0(1, 0), F = 1 − 1 | 108636.923(5e-2) | 5.2 | 1.932 | 21 | -57.2(0.5) | 3.4(1.0) | 77(37) |
| $^{13}CN$ | 1(2, 1) − 0(1, 1), F = 1 − 0 | 108638.212(5e-2) | 5.2 | 0.722 | 10 | -57.4(3.0) | 3.7(2.9) | 19(12) |
| $^{13}CN$ | 1(2, 1) − 0(1, 1), F = 2 − 1 | 108643.590(5e-2) | 5.2 | 0.856 | 14 | -57.7(0.6) | 3.7(1.0) | 54(16) |
| $^{13}CN$ | 1(2, 1) − 0(1, 1), F = 0 − 1 | 108644.346(5e-2) | 5.2 | 0.642 | blended | – | – | – |
| $^{13}CN$ | 1(2, 1) − 0(1, 1), F = 1 − 1 | 108645.064(5e-2) | 5.2 | 0.551 | blended | – | – | – |
| $^{13}CN$ | 1(1, 1) − 0(1, 0), F = 2 − 1 | 108651.297(5e-2) | 5.2 | 3.276 | 36 | -57.1(0.2) | 3.6(0.5) | 139(18) |
| $^{13}CN$ | 1(2, 1) − 0(1, 1), F = 2 − 2 | 108657.646(5e-2) | 5.2 | 2.420 | 25 | -57.1(0.3) | 3.3(0.7) | 87(17) |
| $^{13}CN$ | 1(2, 2) − 0(1, 1), F = 3 − 2 | 108780.201(5e-2) | 5.2 | 4.905 | 47 | -57.0(0.2) | 4.0(0.5) | 198(20) |
| $^{13}CN$ | 1(2, 2) − 0(1, 1), F = 2 − 1 | 108782.374(5e-2) | 5.2 | 2.586 | 28 | -57.2(0.3) | 3.3(0.6) | 97(17) |
| $^{13}CN$ | 1(2, 2) − 0(1, 1), F = 1 − 0 | 108786.982(5e-2) | 5.2 | 1.144 | 14 | -57.4(0.4) | 1.0(0.6) | 14(9) |
| $CH_3OH$, vt=0-2 | 0(0) − 1(-1) E2, vt=0 | 108893.945(12e-3) | 13.1 | 3.9134 | 644 | -58.0(0.) | 5.2(0.1) | 3585(18) |
| $CH_3OH$, vt=0-2 | 14(5) − 15(4) E1, vt=0 | 109138.783(15e-3) | 379.7 | 13.593 | 119 | -58.1(0.5) | 2.8(0.5) | 362(69) |
| $CH_3OH$, vt=0-2 | 16(-2) − 16(1) E2, vt=0 | 109153.184(14e-3) | 342.0 | 14.726 | 70 | -58.0(0.5) | 3.5(0.5) | 262(69) |
| $HC_3N$ | 12 − 11 | 109173.634(1e-2) | 34.1 | 167.1 | 1261 | -57.0(0.1) | 3.9(0.5) | 522(69) |
| SO | 3(2) − 2(1) | 109252.220(1e-1) | 21.1 | 3.5585 | 737 | -57.2(0.4) | 4.6(0.5) | 3644(69) |
| $HC_3N$, $v_7$=1 | 12(-1) − 11(1) | 109442.013(2e-2) | 355.0 | 165.12 | 21 | -52.0(1.3) | 7.9(5.1) | 408(69) |
| OCS | 9 − 8 | 109463.063(5e-3) | 26.3 | 4.6034 | 236 | -57.6(0.) | 4.5(0.1) | 1125(23) |
| HNCO | 5(1, 5) − 4(1, 4) | 109495.996(6e-3) | 59.0 | 11.847 | 24 | -59.0(0.4) | 3.5(0.5) | 89(17) |
| H$\gamma$ | H (55) $\gamma$ | 109536.001(0) | – | – | 16 | -62.8(1.4) | 23.0(2.5) | 381(45) |
| $CH_3OCH_3$ | 8(2, 7) − 8(1, 8) EA | 109571.396(9e-3) | 38.3 | 23.947 | 22 | -58.0(0.3) | 2.2(0.8) | 53(14) |
| $CH_3OCH_3$ | 8(2, 7) − 8(1, 8) AE | 109571.403(9e-3) | 38.3 | 35.921 | blended | – | – | – |
| $CH_3OCH_3$ | 8(2, 7) − 8(1, 8) EE | 109574.088(7e-3) | 38.3 | 95.791 | 32 | -58.0(0.2) | 2.7(0.4) | 92(13) |
| $CH_3OCH_3$ | 8(2, 7) − 8(1, 8) AA | 109576.778(11e-3) | 38.3 | 59.869 | 17 | -58.0(0.4) | 2.4(0.8) | 44(13) |
| $HC_3N$, $v_7$=1 | 12(1) − 11(-1) | 109598.818(2e-2) | 355.0 | 165.12 | 22 | -52.0(0.7) | 7.4(2.2) | 125(26) |
| $NH_2CHO$ | 5(1, 4) − 4(1, 3) | 109753.549(25e-3) | 18.8 | 62.756 | 38 | -58.2(0.5) | 5.6(0.5) | 23(16) |
| $SO_2$ | 17(5, 13) − 18(4, 14) | 109757.585(2e-3) | 202.1 | 6.6069 | 39 | -52.1(0.5) | 8.1(0.5) | 333(162) |
| $C^{18}O$ | 1 − 0 | 109782.173(6e-3) | 5.3 | 0.01221 | 2158 | -57.0(0.5) | 4.2(0.5) | 9721(162) |
| HNCO | 5(2, 3) − 4(2, 2) | 109872.765(3e-2) | 186.1 | 10.012 | 43 | -59.2(0.5) | 3.2(1.0) | 147(46) |
| HNCO | 5(2, 4) − 4(2, 3) | 109872.337(3e-2) | 186.1 | 10.013 | blended | – | – | – |
| HNCO | 5(0, 5) − 4(0, 4) | 109905.749(7e-3) | 15.8 | 12.482 | 153 | -59.0(0.2) | 4.3(0.4) | 702(58) |
| $C^{15}N$ | 1(2, 1) − 0(1, 0) | 110023.540(1e-1) | 5.3 | 1.386 | 20 | -56.8(0.4) | 2.6(0.8) | 57(16) |
| $C^{15}N$ | 1(2, 2) − 0(1, 1) | 110024.590(1e-1) | 5.3 | 3.504 | blended | – | – | – |
| $CH_3OCHO$ | 10(1,10) − 9(1, 9) A | 110153.652(1e-2) | 218.0 | 26.08377 | 32 | -58.6(0.3) | 3.6(0.7) | 125(20) |
| $^{13}CO$ | 1 − 0 | 110201.35(0) | 5.3 | 0.01220 | 14371 | -57.2(0.1) | 5.6(0.1) | 85828(394) |
| HNCO | 5(1, 4) − 4(1, 3) | 110298.089(5e-3) | 59.2 | 11.847 | 26 | -58.8(0.5) | 3.6(0.5) | 98(29) |
| $CH_3CN$ | 6(5, 0) − 5(5, 0) | 110330.345(0) | 197.1 | 56.399 | 14 | -58.0(0.5) | 4.7(0.5) | 7.0(29) |
| $CH_3CN$ | 6(4, 0) − 5(4, 0) | 110349.471(0) | 132.8 | 102.54 | 57 | -58.0(0.4) | 4.0(0.5) | 248(29) |
| $CH_3CN$ | 6(3, 0) − 5(-3, 0) | 110364.354(0) | 82.8 | 138.45 | 175 | -58.1(0.5) | 4.1(0.5) | 769(29) |
| $CH_3CN$ | 6(-3, 0) − 5(3, 0) | 110364.354(0) | 82.8 | 138.45 | blended | – | – | – |
| $CH_3CN$ | 6(2, 0) − 5(2, 0) | 110374.989(0) | 47.1 | 164.06 | 185 | -58.0(0.5) | 4.2(0.5) | 825(29) |
| $CH_3CN$ | 6(1, 0) − 5(1, 0) | 110381.372(0) | 25.7 | 179.45 | 287 | -58.0(0.7) | 4.2(0.5) | 1290(29) |
| $CH_3CN$ | 6(0, 0) − 5(0, 0) | 110383.500(0) | 18.5 | 184.58 | 307 | -58.0(0.5) | 4.6(0.5) | 1517(29) |
| $CH_3OCHO$ | 9(8, 1) − 8(8, 0) E | 110447.180(1e-2) | 69.0 | 5.02983 | 16 | -58.5(0.4) | 0.7(0.5) | 90(79) |
| $CH_3OCHO$ | 9(8, 1) − 8(8, 0) A | 110455.372(1e-2) | 69.0 | 5.02998 | 16 | -58.3(0.6) | 3.7(1.2) | 62(21) |
| $CH_3OCHO$ | 9(8, 2) − 8(8, 1) E | 110458.014(1e-2) | 69.0 | 5.02965 | 27 | -58.5(0.3) | 2.3(1.0) | 66(20) |
| $CH_3OCHO$ | 9(2, 6) − 8(1, 5) | 110462.101(1e-2) | 206.0 | 1.36450 | 22 | -58.5(0.1) | 0.6(0.5) | 13(9) |
| $CH_3OCHO$ | 9(7, 2) − 8(7, 1) E | 110525.741(1e-2) | 59.1 | 9.46492 | 37 | -58.5(0.3) | 3.0(1.7) | 117(38) |
| $CH_3OCHO$ | 9(7, 2) − 8(7, 1) A | 110535.186(1e-2) | 59.1 | 9.561 | blended | – | – | – |
| $CH_3OCHO$ | 9(7, 3) − 8(7, 2) E | 110536.003(1e-2) | 59.1 | 9.46492 | 57 | -58.4(0.2) | 4.5(0.8) | 276(33) |
| $CH_3OCHO$ | 9(2, 6) − 8(1, 5) E | 110550.203(1e-2) | 19.0 | 1.39763 | 17 | -58.5(0.9) | 4.2(2.1) | 76(29) |
| $CH_3OCHO$ | 9(2, 6) − 8(1, 5) A | 110560.051(1e-2) | 19.0 | 1.39665 | 82 | -58.5(1.8) | 3.4(2.8) | 30(24) |
| $CH_3OCHO$ | 10(0,10) − 9(0, 9) A | 110571.632(1e-2) | 217.9 | 26.10484 | 17 | -58.5(0.2) | 3.9(2.5) | 72(32) |
| $CH_3OCHO$ | 9(6, 3) − 8(6, 2) E | 110652.813(1e-2) | 50.5 | 13.30853 | 37 | -58.3(0.4) | 4.4(1.1) | 173(37) |
| $CH_3OCHO$ | 9(6, 4) − 8(6, 3) E | 110662.315(1e-2) | 50.4 | 13.30855 | 26 | -58.3(0.6) | 6.5(1.9) | 182(42) |

**Table A2.** (Continued)

| Species | Transitions | Rest Freq. (MHz) | $E_u$ (K) | $\mu^2S$ ($D^2$) | $T_{mb}$ (mK) | $V_{LSR}$ (km $s^{-1}$) | $\Delta V$ (km $s^{-1}$) | $\int T_{mb}$ dv (mK km $s^{-1}$) |
|---|---|---|---|---|---|---|---|---|
| $CH_3OCHO$ | 9(6, 3) − 8(6, 2) A | 110663.429(1e-2) | 50.4 | 13.31127 | 12 | -58.5(0.7) | 2.0(1.6) | 26(18) |
| $CH_3OCHO$ | 9(6, 4) − 8(6, 3) A | 110663.273(1e-2) | 50.4 | 13.3113 | blended | – | – | – |
| $CH_3OCHO$ | 9(4, 6) − 8(4, 5) E | 110684.123(1e-2) | 224.1 | 19.21258 | 61 | -58.5(0.2) | 6.8(0.8) | 443(36) |
| $CH_3OCHO$ | 9(1, 8) − 8(1, 7) A | 110776.499(1e-2) | 215.7 | 23.1436 | 24 | -58.5(0.5) | 3.2(0.5) | 118(96) |
| $CH_3OCHO$ | 10(1,10) − 9(1, 9) E | 110788.664(1e-2) | 30.3 | 26.16584 | 68 | -58.4(0.5) | 3.8(0.5) | 272(96) |
| $CH_3OCHO$ | 10(1,10) − 9(1, 9) A | 110790.526(1e-2) | 30.3 | 26.17539 | 68 | -58.5(0.4) | 3.9(0.5) | 283(96) |
| $CH_3OCHO$ | 9(5, 4) − 8(5, 3) E | 110873.955(1e-2) | 43.2 | 16.55557 | 39 | -58.5(0.9) | 2.8(0.5) | 116(16) |
| $CH_3OCHO$ | 9(3, 7) − 8(3, 6) E | 110879.766(1e-2) | 32.6 | 21.245 | 66 | -58.5(0.5) | 4.5(0.5) | 321(16) |
| $CH_3OCHO$ | 9(5, 5) − 8(5, 4) E | 110882.331(1e-2) | 43.2 | 16.55225 | 44 | -58.6(0.5) | 2.8(0.5) | 128(16) |
| $CH_3OCHO$ | 9(3, 7) − 8(3, 6) A | 110887.092(1e-2) | 32.6 | 21.25577 | 60 | -58.6(0.5) | 6.3(0.5) | 407(16) |
| $CH_3OCHO$ | 9(5, 4) − 8(5, 3) A | 110890.256(1e-2) | 43.2 | 16.56106 | 38 | -58.5(0.5) | 9.0(0.5) | 361(16) |
| $CH_3OCHO$ | 10(0, 10) − 9(0, 9) E | 111169.903(1e-2) | 30.2 | 26.18776 | 62 | -58.7(0.3) | 2.4(0.7) | 157(38) |
| $CH_3OCHO$ | 10(0, 10) − 9(0, 9) A | 111171.634(1e-2) | 30.2 | 26.19136 | 58 | -58.5(0.3) | 2.2(0.7) | 134(35) |
| $CH_3OCHO$ | 9(4, 6) − 8(4, 5) A | 111195.962(1e-2) | 37.2 | 19.21722 | 48 | -58.5(0.2) | 2.3(0.5) | 117(22) |
| $CH_3OCHO$ | 9(4, 6) − 8(4, 5) E | 111223.491(1e-2) | 37.2 | 18.18412 | 41 | -58.5(0.3) | 2.6(0.5) | 114(23) |
| $CH_3OH$, vt=0-2 | $7(2)^+ - 8(1)^+$, vt=0 | 111289.453(13e-3) | 102.7 | 9.3425 | 292 | -58.0(0.1) | 3.8(0.2) | 1177(45) |
| $CH_3OCHO$ | 9(4, 5) − 8(4, 4) E | 111408.412(1e-2) | 37.3 | 18.18767 | 32 | -58.4(0.3) | 2.1(0.5) | 71(19) |
| $CH_3OCHO$ | 9(4, 5) − 8(4, 4) A | 111453.300(1e-2) | 37.2 | 19.21778 | 42 | -58.5(0.3) | 2.5(0.5) | 112(21) |
| $CH_3OH$, vt=0-2 | 17(-2) − 17(1) E2, vt=0 | 111626.514(15e-3) | 381.5 | 20.231 | 45 | -58.2(0.5) | 2.3(0.5) | 112(74) |
| $CH_3OCHO$ | 9(1, 8) − 8(1, 7) E | 111674.131(1e-2) | 28.1 | 23.18984 | 48 | -58.5(0.5) | 3.1(0.5) | 158(74) |
| $CH_3OCHO$ | 9(1, 8) − 8(1, 7) A | 111682.189(1e-2) | 28.1 | 23.19587 | 56 | -58.5(0.7) | 3.6(0.5) | 214(8) |
| $CH_3OCHO$ | 9(4, 5) − 8(4, 5) E | 111713.138(14-2) | 37.3 | 1.02682 | 85 | -58.5(0.5) | 2.5(0.5) | 22(8) |
| $CH_3OCHO$ | 10(1, 10) − 9(0, 9) A | 111735.307(1e-2) | 30.3 | 3.84224 | 19 | -58.4(0.5) | 1.3(0.5) | 28(8) |
| $CH_3OCHO$ | 10(1, 10) − 9(0, 9) E | 111734.002(1e-2) | 30.3 | 3.84434 | blended | – | – | – |
| t-HCOOH | 5(0, 5) − 4(0, 4) | 111746.784(3e-3) | 16.1 | 10.092 | 12 | -58.5(0.5) | 3.1(0.5) | 40(8) |
| $CH_3OCH_3$ | 7(0, 7) − 6(1, 6) AA | 111782.562(8e-3) | 25.2 | 53.86755 | 27 | -58.0(0.5) | 3.8(0.5) | 109(8) |
| $CH_3OCH_3$ | 7(0, 7) − 6(1, 6) EE | 111783.010(4e-2) | 25.3 | 86.2034 | 18 | -58.1(0.5) | 8.3(0.5) | 155(8) |
| $CH_3OCH_3$ | 7(0, 7) − 6(1, 6) EA | 111783.647(7e-3) | 25.3 | 21.54865 | blended | – | – | – |
| $CH_3OCH_3$ | 7(5, 3) − 8(4, 4) EE | 111794.034(34e-3) | 60.6 | 0.47169 | 19 | -58.0(0.1) | 5.8(0.5) | 119(8) |
| $CH_3OCH_3$ | 7(5, 3) − 8(4, 4) AE | 111797.334(29e-3) | 60.6 | 1.02408 | blended | – | – | – |
| $CH_3OCH_3$ | 7(5, 3) − 8(4, 4) EA | 111797.837(26e-3) | 60.6 | 2.01433 | 44 | -58.0(0.5) | 4.7(0.5) | 220(8) |
| $CH_3OCH_3$ | 7(5, 2) − 8(4, 5) EA | 111801.851(34e-3) | 60.6 | 2.01464 | blended | – | – | – |
| $CH_3OCH_3$ | 7(5, 2) − 8(4, 5) EE | 111801.894(25e-3) | 60.6 | 7.72144 | 14 | -58.0(0.3) | 1.7(0.5) | 25(9) |
| $CH_3OCH_3$ | 7(5, 3) − 8(4, 5) AA | 111804.354(33e-3) | 60.6 | 3.07241 | 13 | -58.1(0.5) | 1.7(0.5) | 22(9) |
| $CH_3OCH_3$ | 7(5, 3) − 8(4, 5) EE | 111804.813(26e-3) | 60.6 | 7.72103 | blended | – | – | – |
| $CH_3OCH_3$ | 7(5, 2) − 8(4, 5) EE | 111812.674(31e-3) | 60.6 | 0.47164 | 21 | -58.0(0.5) | 3.9(0.5) | 89(9) |
| $CH_3OCH_3$ | 18(3, 15) − 18(2, 16) EE | 111813.668(21e-3) | 115.4 | 305.79762 | 34 | -58.0(0.5) | 4.8(0.5) | 177(9) |
| $CH_3OCH_3$ | 18(3, 15) − 18(2, 16) AA | 111815.291(25e-3) | 168.9 | 114.66248 | 16 | -58.0(0.7) | 5.4(0.5) | 91(9) |
| $CH_3OH$, vt=0-2 | 34(8) − 33(9) E1, vt=0 | 111846.089(145e-3) | 172.0 | 38.605 | 34 | -58.0(0.4) | 3.1(0.5) | 112(35) |
| Hβ | H (48) β | 111885.070(0) | – | – | 38 | -62.2(1.6) | 24.2(3.1) | 967(114) |
| $C_2H_5OH$ | 12(3, 9) − 12(2, 10) | 112129.544(5e-2) | 77.1 | 16.463 | 28 | -57.5(0.) | 5.8(1.2) | 177(30) |
| $CH_3OH$, vt=0-2 | $19(0)^+ - 18(2)^+$, vt=0 | 112145.638(21e-3) | 440.1 | 0.00059 | 64 | -58.0(0.1) | 2.2(0.4) | 147(19) |
| $CH_3CHO$ | 6(1, 6) − 5(1, 5) A, vt=0 | 112248.716(3e-3) | 21.1 | 73.76807 | 71 | -57.0(0.2) | 3.0(0.5) | 227(36) |
| $CH_3CHO$ | 6(1, 6) − 5(1, 5) E, vt=0 | 112254.508(3e-3) | 21.2 | 73.79585 | 70 | -57.0(0.2) | 2.4(0.5) | 181(34) |
| t-HCOOH | 5(2, 4) − 4(2, 3) | 112287.145 (3e-3) | 28.9 | 8.4851 | 29 | -58.5(0.5) | 1.8(0.5) | 18(36) |
| $C^{17}O$ | 1 − 0 | 112359.284(1e-3) | 5.4 | 0.01217 | 512 | -57.0(0.5) | 6.1(0.5) | 3342(36) |
| $CH_3OH$, vt=0-2 | $19(0)^+ - 18(2)^+$, vt=0 | 112145.638(21e-3) | 440.1 | 0.00059 | 22 | -58.0(0.5) | 3.9(0.8) | 90(21) |
| $CH_3OCHO$ | 14(5, 9) −14(4, 10) E | 112672.759(1e-2) | 78.9 | 3.64313 | 16 | -58.5(1.9) | 9.6(6.0) | 320(83) |
| $CH_3OCHO$ | 14(5, 9) −14(4, 10) A | 112676.856(1e-2) | 78.9 | 3.67559 | 12 | -58.5(1.3) | 7.5(2.4) | 97(44) |
| $C_2H_5OH$ | 11(3, 9) − 10(4, 7) | 112746.252(5e-2) | 127.5 | 1.5782 | 31 | -57.5(0.2) | 1.2(0.6) | 38(15) |
| $CH_3OCH_3$ | 20(3, 17) − 20(2, 18) EE | 113000.970(32e-3) | 206.1 | 348.88725 | 12 | -57.8(0.5) | 4.1(0.5) | 53(11) |
| $CH_3OCH_3$ | 20(3, 17) − 20(2, 18) AA | 113002.265(34e-3) | 206.1 | 130.85038 | 21 | -57.8(0.4) | 4.7(0.5) | 107(11) |
| $CH_3OCH_3$ | 17(3, 14) − 17(2, 15) EA | 113057.427(19e-3) | 153.1 | 132.79 | 16 | -58.0(0.5) | 2.8(0.5) | 50(11) |
| $CH_3OCH_3$ | 17(3, 14) − 17(2, 15) AE | 113057.425(18e-3) | 153.1 | 88.525 | blended | – | – | – |
| $CH_3OCH_3$ | 17(3, 14) − 17(2, 15) EE | 113059.249(17e-3) | 153.1 | 354.12 | 33 | -58.1(0.6) | 2.6(0.5) | 91(11) |
| $CH_3OCH_3$ | 17(3, 14) − 17(2, 15) AA | 113061.072(22e-3) | 153.1 | 221.33 | 17 | -58.1(0.8) | 2.1(0.5) | 39(11) |
| CN | N= 1-0, J=1/2-1/2, F=1/2-1/2 | 113123.370(6e-3) | 5.4 | 0.15271 | 180 | -57.5(0.2) | 6.0(0.8) | 1143(108) |
| CN | N= 1-0, J=1/2-1/2, F=1/2-3/2 | 113144.157(6e-3) | 5.4 | 1.2492 | 789 | -57.5(0.1) | 7.2(0.3) | 6078(143) |
| CN | N= 1-0, J=1/2-1/2, F=3/2-1/2 | 113170.492(4e-3) | 5.4 | 1.2199 | 887 | -57.5(0.) | 6.9(0.2) | 6490(135) |
| CN | N= 1-0, J=1/2-1/2, F=3/2-3/2 | 113191.279(3e-3) | 5.4 | 1.5836 | 893 | -57.5(0.1) | 7.5(0.2) | 7173(145) |
| CCS | 9(8) − 8(7) | 113410.186(2e-2) | 33.6 | 65.427 | 28 | -57.0(0.5) | 10.0(0.5) | 301(177) |
| CN | N= 1-0, J=3/2-1/2, F=3/2-1/2 | 113488.120(3e-3) | 5.4 | 1.5838 | 1425 | -57.4(0.5) | 5.8(0.5) | 8816(177) |
| CN | N= 1-0, J=3/2-1/2, F=5/2-3/2 | 113490.970(2e-3) | 5.4 | 4.205 | 2194 | -57.5(0.5) | 5.8(0.5) | 13510(177) |
| CN | N= 1-0, J=3/2-1/2, F=1/2-1/2 | 113499.644(3e-3) | 5.4 | 1.2491 | 572 | -57.5(0.6) | 7.0(0.5) | 4264(177) |
| CN | N= 1-0, J=3/2-1/2, F=3/2-3/2 | 113508.907(3e-3) | 5.4 | 1.2196 | 725 | -57.4(0.5) | 6.0(0.5) | 4658(177) |
| CN | N= 1-0, J=3/2-1/2, F=1/2-3/2 | 113520.432(4e-3) | 5.4 | 0.15263 | 93 | -57.5(0.5) | 5.0(0.5) | 497(177) |
| G121.29+00.65 | | | | | | | | |
| CCS | 8(9) − 7(8) | 106347.726(2e-2) | 25.0 | 74.425 | 147 | -17.5(0.) | 2.5(0.1) | 400(11) |
| $HC_5N$ | 40 − 39 | 106498.910(7e-3) | 104.8 | 2249.7 | 42 | -17.6(0.1) | 2.4(0.3) | 109(11) |
| $^{34}SO$ | 3(2) − 2(1) | 106743.244(7e-2) | 20.9 | 3.557 | 26 | -17.5(0.2) | 3.4(0.5) | 95(13) |
| $CH_3OH$, vt=0-2 | $3(1)^+ - 4(0)^+$, vt=0 | 107013.831(1e-2) | 28.3 | 12.036 | 201 | -17.5(0.) | 2.8(0.1) | 606(19) |
| $CH_3OH$, vt=0-2 | 15(-2) − 15(1) E2, vt=0 | 107159.906(14e-3) | 304.7 | 10.421 | 92 | -17.5(0.6) | 3.1(1.2) | 30(13) |
| $CH_3OCHO$ | 9( 2, 8) − 8( 2, 7) E | 107537.258(1e-2) | 28.8 | 22.60702 | 13 | -18.0(0.5) | 2.4(0.9) | 34(13) |
| $CH_3OCHO$ | 9( 2, 8) − 8( 2, 7) A | 107543.711(1e-2) | 28.8 | 22.61344 | 14 | -18.0(0.7) | 1.8(0.9) | 15(10) |
| t-HCOOH | 5(1, 5) − 4(1, 4) | 108126.720(3e-3) | 18.8 | 9.6966 | 33 | -17.5(0.2) | 2.3(0.4) | 81(14) |
| $^{13}CN$ | 1(1, 0) − 0(1, 1), F = 1 − 1 | 108412.862(5e-2) | 5.2 | 0.635 | 13 | -18.2(0.3) | 1.9(0.6) | 26(8) |
| $^{13}CN$ | 1(1, 0) − 0(1, 1), F = 1 − 2 | 108426.889(5e-2) | 5.2 | 1.267 | 25 | -17.5(0.2) | 3.0(0.6) | 79(12) |
| $^{13}CN$ | 1(1, 1) − 0(1, 0), F = 0 − 1 | 108631.121(5e-2) | 5.2 | 0.642 | 17 | -17.7(0.3) | 2.6(0.9) | 48(12) |
| $^{13}CN$ | 1(1, 1) − 0(1, 0), F = 1 − 1 | 108636.923(5e-2) | 5.2 | 1.932 | 32 | -17.4(0.5) | 2.5(0.5) | 84(6) |
| $^{13}CN$ | 1(2, 1) − 0(1, 1), F = 1 − 0 | 108638.212(5e-2) | 5.2 | 0.722 | 16 | -17.5(0.5) | 4.2(0.5) | 71(6) |
| $^{13}CN$ | 1(2, 1) − 0(1, 1), F = 2 − 1 | 108643.590(5e-2) | 5.2 | 0.856 | 13 | -17.7(0.5) | 1.2(0.5) | 17(6) |
| $^{13}CN$ | 1(2, 1) − 0(1, 1), F = 0 − 1 | 108644.346(5e-2) | 5.2 | 0.642 | 25 | -17.9(0.5) | 3.2(0.5) | 85(6) |
| $^{13}CN$ | 1(2, 1) − 0(1, 1), F = 1 − 1 | 108645.064(5e-2) | 5.2 | 0.551 | blended | – | – | – |
| $^{13}CN$ | 1(1, 1) − 0(1, 0), F = 2 − 1 | 108651.297(5e-2) | 5.2 | 3.276 | 67 | -17.5(0.5) | 2.3(0.5) | 167(6) |
| $^{13}CN$ | 1(2, 1) − 0(1, 1), F = 2 − 2 | 108657.646(5e-2) | 5.2 | 2.420 | 43 | -17.4(0.5) | 2.4(0.5) | 108(6) |
| $^{13}CN$ | 1(2, 1) − 0(1, 1), F = 1 − 2 | 108658.948(5e-2) | 5.2 | 0.669 | 11 | -17.3(0.5) | 1.8(0.5) | 21(6) |
| $^{13}CN$ | 1(2, 2) − 0(1, 1), F = 3 − 2 | 108780.201(5e-2) | 5.2 | 4.905 | 84 | -17.5(0.1) | 2.6(0.1) | 236(11) |
| $^{13}CN$ | 1(2, 2) − 0(1, 1), F = 2 − 1 | 108782.374(5e-2) | 5.2 | 2.586 | 45 | -17.7(0.1) | 2.6(0.2) | 125(11) |
| $^{13}CN$ | 1(2, 2) − 0(1, 1), F = 1 − 0 | 108786.982(5e-2) | 5.2 | 1.144 | 21 | -17.6(0.2) | 2.0(0.4) | 45(9) |
| $^{13}CN$ | 1(2, 2) − 0(1, 1), F = 1 − 1 | 108793.753(5e-2) | 5.2 | 0.894 | 23 | -17.5(0.2) | 1.2(0.5) | 30(9) |
| $^{13}CN$ | 1(2, 2) − 0(1, 1), F = 2 − 2 | 108796.400(5e-2) | 5.2 | 0.918 | 15 | -17.5(0.3) | 2.4(0.5) | 40(10) |
| $CH_3OH$, vt=0-2 | 0(0) − 1(-1) E2, vt=0 | 108893.945(12e-3) | 13.1 | 3.9134 | 476 | -17.5(0.) | 3.0(0.1) | 1502(14) |
| $HC_5N$ | 41 − 40 | 109160.973(7e-3) | 110.0 | 2306 | 36 | -17.5(0.2) | 2.3(0.4) | 87(12) |
| $HC_3N$ | 12 − 11 | 109173.634(1e-2) | 34.1 | 167.1 | 2257 | -17.5(0.) | 2.6(0.1) | 6247(13) |
| SO | 3(2) − 2(1) | 109252.220(1e-1) | 21.1 | 3.5585 | 687 | 17.3(0.) | 2.8(0.1) | 2012(26) |
| OCS | 9 − 8 | 109463.063(5e-3) | 26.3 | 4.6069 | 223 | -17.5(0.) | 2.6(0.1) | 620(12) |
| $C^{18}O$ | 1 − 0 | 109782.173(6e-3) | 5.3 | 0.01221 | 2233 | -17.5(0.1) | 2.6(0.1) | 6148(16) |
| HNCO | 5(0, 5) − 4(0, 4) | 109905.749(7e-3) | 15.8 | 12.482 | 507 | -18.0(0.) | 3.0(0.1) | 1647(28) |

**Table A2.** (Continued)

| Species | Transitions | Rest Freq. (MHz) | $E_u$ (K) | $\mu^2$S ($D^2$) | $T_{mb}$ (mK) | $V_{LSR}$ (km $s^{-1}$) | $\Delta$V (km $s^{-1}$) | $\int T_{mb}$ dv (mK km $s^{-1}$) |
|---|---|---|---|---|---|---|---|---|
| $C^{15}N$ | 1(2, 1) − 0(1, 1) | 110004.091(3e-2) | 5.3 | 0.717 | 18 | -17.4(0.4) | 2.5(1.3) | 47(17) |
| $C^{15}N$ | 1(2, 1) − 0(1, 0) | 110023.540(1e-1) | 5.3 | 1.386 | 18 | -17.2(0.5) | 3.4(1.0) | 67(18) |
| $C^{15}N$ | 1(2, 2) − 0(1, 1) | 110024.590(1e-1) | 5.3 | 3.504 | 31 | -17.8(0.2) | 2.3(0.5) | 76(16) |
| $CH_3OCHO$ | 10(1,10) − 9(1, 9) A | 110153.652(1e-2) | 218.0 | 26.08377 | 168 | -18.0(0.1) | 4.2(0.2) | 758(24) |
| $^{13}CO$ | 1 − 0 | 110201.35(0) | 5.3 | 0.01220 | 13904 | -17.5(0.1) | 2.9(0.1) | 42842(240) |
| $CH_3CN$ | 6(4, 0) − 5(4, 0) | 110349.471(0) | 132.8 | 102.54 | 17 | -17.5(0.4) | 0.6(0.5) | 11(2) |
| $CH_3CN$ | 6(3, 0) − 5(-3, 0) | 110364.354(0) | 82.8 | 138.45 | 80 | -17.5(0.5) | 2.8(0.5) | 240(32) |
| $CH_3CN$ | 6(-3, 0) − 5(3, 0) | 110364.354(0) | 82.8 | 138.45 | blended | – | – | – |
| $CH_3CN$ | 6(2, 0) − 5(2, 0) | 110374.989(0) | 47.1 | 164.06 | 125 | -17.4(0.5) | 2.8(0.5) | 366(32) |
| $CH_3CN$ | 6(1, 0) − 5(1, 0) | 110381.372(0) | 25.7 | 179.45 | 295 | -17.5(0.9) | 2.9(0.5) | 903(32) |
| $CH_3CN$ | 6(0, 0) − 5(0, 0) | 110383.500(0) | 18.5 | 184.58 | 346 | -17.5(0.5) | 3.0(0.5) | 1108(32) |
| $CH_3OCHO$ | 10(1,10) − 9(1, 9) E | 110788.664(1e-2) | 30.3 | 26.16584 | 19 | -18.1(0.3) | 1.8(0.6) | 38(12) |
| $CH_3OCHO$ | 10(1,10) − 9(1, 9) A | 110790.526(1e-2) | 30.3 | 26.17539 | 24 | -18.0(0.2) | 0.9(0.5) | 23(9) |
| $CH_3OCHO$ | 9(3, 7) − 8(3, 6) E | 110879.766(1e-2) | 32.6 | 21.245 | 77 | -18.0(1.4) | 2.4(1.7) | 19(18) |
| $CH_3OCHO$ | 10(0, 10) − 9(0, 9) E | 111169.903(1e-2) | 30.2 | 26.18776 | 19 | -18.0(0.4) | 2.2(1.3) | 44(17) |
| $CH_3OCHO$ | 10(0, 10) − 9(0, 9) A | 111171.634(1e-2) | 30.2 | 26.19136 | 12 | -17.9(0.8) | 1.2(1.1) | 13(10) |
| $CH_3OCHO$ | 9(4, 6) − 8(4, 5) E | 111223.491(1e-2) | 37.2 | 18.18412 | 16 | -17.9(0.4) | 2.5(0.9) | 44(15) |
| $CH_3OH$, vt=0-2 | 7(2)$^+$ − 8(1)$^+$, vt=0 | 111289.453(13e-3) | 102.7 | 9.3425 | 26 | -17.4(0.2) | 1.3(0.5) | 35(11) |
| $CH_3OCHO$ | 9(4, 5) − 8(4, 4) E | 111408.412(1e-2) | 37.3 | 18.18767 | 23 | -17.9(0.3) | 2.3(0.6) | 56(14) |
| $CH_3OCHO$ | 9(4, 5) − 8(4, 4) A | 111453.300(1e-2) | 37.2 | 19.21778 | 23 | -17.9(0.4) | 4.1(0.9) | 103(19) |
| $CH_3OH$, vt=0-2 | 17(-2) − 17(1) E2, vt=0 | 111626.514(15e-3) | 381.5 | 20.231 | 25 | -17.5(0.2) | 1.0(0.4) | 27(10) |
| $CH_3OCHO$ | 9(1, 8) − 8(1, 7) E | 111674.131(1e-2) | 28.1 | 23.18984 | 10 | -18.0(0.8) | 2.7(1.4) | 28(15) |
| $CH_3OCHO$ | 9(1, 8) − 8(1, 7) A | 111682.189(1e-2) | 28.1 | 23.19587 | 24 | -18.0(0.2) | 1.6(0.4) | 41(11) |
| t-HCOOH | 5(0, 5) − 4(0, 4) | 111746.784(3e-3) | 16.1 | 10.092 | 33 | -17.5(0.3) | 2.4(0.5) | 85(18) |
| $HC_5N$ | 42 − 41 | 111823.024(0) | 115.4 | 2362.2 | 34 | -17.3(0.2) | 1.7(0.4) | 64(12) |
| $CH_3CHO$ | 6(1, 6) − 5(1, 5) A, vt=0 | 112248.716(3e-3) | 21.1 | 73.76807 | 106 | -18.1(0.5) | 3.0(0.5) | 334(11) |
| $CH_3CHO$ | 6(1, 6) − 5(1, 5) E, vt=0 | 112254.508(3e-3) | 21.2 | 73.79585 | 114 | -18.1(0.6) | 2.7(0.5) | 324(11) |
| t-HCOOH | 5(2, 4) − 4(2, 3) | 112287.145(3e-3) | 28.9 | 8.4851 | 19 | -17.6(0.5) | 1.9(0.5) | 39(11) |
| $C^{17}O$ | 1 − 0 | 112359.284(1e-3) | 5.4 | 0.01217 | 414 | -17.8(0.1) | 2.5(0.1) | 1118(100) |
| CN | N= 1-0, J=1/2-1/2, F=1/2-1/2 | 113123.370(6e-3) | 5.4 | 0.15271 | 418 | -17.5(0.5) | 3.0(0.5) | 1346(110) |
| CN | N= 1-0, J=1/2-1/2, F=1/2-3/2 | 113144.157(6e-3) | 5.4 | 1.2492 | 1300 | -17.5(0.4) | 3.1(0.5) | 4220(110) |
| CN | N= 1-0, J=1/2-1/2, F=3/2-1/2 | 113170.492(4e-3) | 5.4 | 1.2199 | 1387 | -17.3(0.5) | 3.1(0.5) | 4581(110) |
| CN | N= 1-0, J=1/2-1/2, F=3/2-3/2 | 113191.279(3e-3) | 5.4 | 1.5836 | 1389 | -17.5(0.5) | 3.1(0.5) | 4649(110) |
| CCS | 9(8) − 8(7) | 113410.186(2e-2) | 33.6 | 65.427 | 46 | -17.5(0.5) | 4.6(0.5) | 226(166) |
| CN | N= 1-0, J=3/2-1/2, F=3/2-1/2 | 113488.120(3e-3) | 5.4 | 1.5838 | 1332 | -17.5(0.) | 3.1(0.5) | 4410(166) |
| CN | N= 1-0, J=3/2-1/2, F=5/2-3/2 | 113490.970(2e-3) | 5.4 | 4.205 | 3406 | -17.5(0.) | 2.1(0.5) | 7682(166) |
| CN | N= 1-0, J=3/2-1/2, F=1/2-1/2 | 113499.644(3e-3) | 5.4 | 1.2491 | 905 | -17.5(0.5) | 3.2(0.5) | 3071(166) |
| CN | N= 1-0, J=3/2-1/2, F=3/2-3/2 | 113508.907(3e-3) | 5.4 | 1.2196 | 1242 | -17.5(0.7) | 3.3(0.5) | 4310(166) |
| CN | N= 1-0, J=3/2-1/2, F=1/2-3/2 | 113520.432(4e-3) | 5.4 | 0.15263 | 298 | -17.5(0.5) | 3.2(0.5) | 1011(166) |
| | | G123.06−06.30 | | | | | | |
| CCS | 8(9) − 7(8) | 106347.726(2e-2) | 25.0 | 74.425 | 89 | -30.5(0.1) | 3.2(0.2) | 300(14) |
| $HC_5N$ | 40 − 39 | 106498.910(7e-3) | 104.8 | 2249.7 | 22 | -31.0(0.3) | 3.6(1.1) | 84(17) |
| $^{34}SO$ | 3(2) − 2(1) | 106743.244(7e-2) | 20.9 | 3.557 | 28 | -30.7(0.3) | 4.9(1.2) | 147(24) |
| $CH_3OH$, vt=0-2 | 3(1)$^+$ − 4(0)$^+$, vt=0 | 107013.831(1e-2) | 28.3 | 12.036 | 226 | -30.4(0.) | 4.8(0.1) | 1163(17) |
| $CH_3OH$, vt=0-2 | 15(-2) − 15(1) E2, vt=0 | 107159.906(14e-3) | 304.7 | 10.421 | 19 | -30.4(0.4) | 8.1(1.1) | 168(18) |
| $CH_3OCHO$ | 9( 2, 8) − 8( 2, 7) E | 107537.258(1e-2) | 28.8 | 22.60702 | 23 | -30.4(0.3) | 2.6(0.5) | 63(12) |
| $CH_3OCHO$ | 9( 2, 8) − 8( 2, 7) A | 107543.711(1e-2) | 28.8 | 22.61344 | 15 | -30.5(0.6) | 6.9(1.2) | 113(19) |
| t-HCOOH | 5(1, 5) − 4(1, 4) | 108126.720(3e-3) | 18.8 | 9.6966 | 23 | -30.0(0.4) | 3.1(0.7) | 75(17) |
| $^{13}CN$ | 1(1, 0) − 0(1, 1), F = 1 − 1 | 108412.862(5e-2) | 5.2 | 0.635 | 13 | -30.7(0.4) | 3.1(2.7) | 44(21) |
| $^{13}CN$ | 1(1, 0) − 0(1, 1), F = 1 − 2 | 108426.889(5e-2) | 5.2 | 1.267 | 22 | -31.0(0.3) | 3.5(0.8) | 83(13) |
| $^{13}CN$ | 1(1, 1) − 0(1, 0), F = 0 − 1 | 108631.121(5e-2) | 5.2 | 0.642 | 16 | -31.0(0.3) | 1.8(0.7) | 32(9) |
| $^{13}CN$ | 1(1, 1) − 0(1, 0), F = 1 − 1 | 108636.923(5e-2) | 5.2 | 1.932 | 39 | -31.0(0.1) | 2.3(0.3) | 95(11) |
| $^{13}CN$ | 1(2, 1) − 0(1, 1), F = 1 − 0 | 108638.212(5e-2) | 5.2 | 0.722 | 24 | -31.1(0.2) | 1.4(0.3) | 36(9) |
| $^{13}CN$ | 1(2, 1) − 0(1, 1), F = 2 − 1 | 108643.590(5e-2) | 5.2 | 0.856 | 23 | -31.0(0.2) | 3.3(0.6) | 80(12) |
| $^{13}CN$ | 1(2, 1) − 0(1, 1), F = 0 − 1 | 108644.346(5e-2) | 5.2 | 0.642 | 27 | -31.3(0.1) | 1.5(0.3) | 42(9) |
| $^{13}CN$ | 1(2, 1) − 0(1, 1), F = 1 − 1 | 108645.064(5e-2) | 5.2 | 0.551 | blended | – | – | – |
| $^{13}CN$ | 1(1, 1) − 0(1, 0), F = 2 − 1 | 108651.297(5e-2) | 5.2 | 3.276 | 61 | -31.1(0.1) | 2.6(0.2) | 167(10) |
| $^{13}CN$ | 1(2, 1) − 0(1, 1), F = 2 − 2 | 108657.646(5e-2) | 5.2 | 2.420 | 41 | -31.0(0.1) | 3.0(0.4) | 132(16) |
| $^{13}CN$ | 1(2, 1) − 0(1, 1), F = 1 − 2 | 108658.948(5e-2) | 5.2 | 0.669 | 7 | -31.4(1.4) | 4.7(2.1) | 35(16) |
| $^{13}CN$ | 1(2, 2) − 0(1, 1), F = 3 − 2 | 108780.201(5e-2) | 5.2 | 4.905 | 91 | -31.0(0.5) | 2.6(0.5) | 253(6) |
| $^{13}CN$ | 1(2, 2) − 0(1, 1), F = 2 − 1 | 108782.374(5e-2) | 5.2 | 2.586 | 43 | -31.1(0.5) | 2.9(0.5) | 133(6) |
| $^{13}CN$ | 1(2, 2) − 0(1, 1), F = 1 − 0 | 108786.982(5e-2) | 5.2 | 1.144 | 17 | -31.0(0.5) | 2.4(0.5) | 42(6) |
| $^{13}CN$ | 1(2, 2) − 0(1, 1), F = 1 − 1 | 108793.753(5e-2) | 5.2 | 0.894 | 15 | -31.1(0.5) | 1.0(0.5) | 16(6) |
| $^{13}CN$ | 1(2, 2) − 0(1, 1), F = 2 − 2 | 108796.400(5e-2) | 5.2 | 0.918 | 17 | -31.0(0.5) | 1.7(0.5) | 31(6) |
| $CH_3OH$, vt=0-2 | 0(0) − 1(-1) E2, vt=0 | 108893.945(12e-3) | 13.1 | 3.9134 | 649 | -30.4(0.) | 4.6(0.1) | 3167(21) |
| $HC_5N$ | 41 − 40 | 109160.973(7e-3) | 110.0 | 2306 | 32 | -31.0(0.3) | 1.8(0.7) | 62(19) |
| $HC_3N$ | 12 − 11 | 109173.634(1e-2) | 34.1 | 167.1 | 2169 | -30.7(0.) | 3.0(0.1) | 6832(25) |
| SO | 3(2) − 2(1) | 109252.220(1e-1) | 21.1 | 3.5585 | 680 | -30.5(0.) | 4.7(0.1) | 3373(32) |
| OCS | 9 − 8 | 109463.063(5e-3) | 26.3 | 4.6034 | 254 | -30.5(0.) | 4.3(0.1) | 1167(19) |
| HNCO | 5(1, 5) − 4(1, 4) | 109495.996(6e-3) | 59.0 | 11.847 | 13 | -31.0(0.7) | 4.7(1.1) | 66(17) |
| $C^{18}O$ | 1 − 0 | 109782.173(6e-3) | 5.3 | 0.01221 | 1451 | -30.1(0.1) | 3.4(0.1) | 5248(16) |
| HNCO | 5(2, 3) − 4(2, 2) | 109872.765(3e-2) | 186.1 | 10.012 | 10 | -31.0(1.9) | 3.1(3.0) | 19(20) |
| HNCO | 5(2, 4) − 4(2, 3) | 109872.337(3e-2) | 186.1 | 10.013 | blended | – | – | – |
| HNCO | 5(0, 5) − 4(0, 4) | 109905.749(7e-3) | 15.8 | 12.482 | 323 | -31.0(0.1) | 4.0(0.1) | 1377(38) |
| $C^{15}N$ | 1(2, 1) − 0(1, 1) | 110004.091(3e-2) | 5.3 | 0.717 | 11 | -29.8(0.9) | 6.3(2.7) | 73(24) |
| $C^{15}N$ | 1(2, 1) − 0(1, 0) | 110023.540(1e-1) | 5.3 | 1.386 | 22 | -30.2(0.8) | 3.4(1.4) | 80(35) |
| $C^{15}N$ | 1(2, 2) − 0(1, 1) | 110024.590(1e-1) | 5.3 | 3.504 | 38 | -30.1(0.2) | 1.7(0.4) | 60(30) |
| $CH_3OCHO$ | 10(1,10) − 9(1, 9) A | 110153.652(1e-2) | 218.0 | 26.08377 | 129 | -30.4(0.1) | 4.6(0.2) | 625(20) |
| $^{13}CO$ | 1 − 0 | 110201.35(0) | 5.3 | 0.01220 | 13491 | -30.0(0.1) | 3.7(0.1) | 53603(85) |
| HNCO | 5(1, 4) − 4(1, 3) | 110298.089(5e-3) | 59.2 | 11.847 | 15 | -31.1(1.1) | 6.4(1.1) | 102(57) |
| $CH_3CN$ | 6(4, 0) − 5(4, 0) | 110349.471(0) | 132.8 | 102.54 | 16 | -30.5(1.1) | 5.0(1.1) | 83(57) |
| $CH_3CN$ | 6(3, 0) − 5(-3, 0) | 110364.354(0) | 82.8 | 138.45 | 112 | -30.5(1.0) | 4.9(1.1) | 584(57) |
| $CH_3CN$ | 6(-3, 0) − 5(3, 0) | 110364.354(0) | 82.8 | 138.45 | blended | – | – | – |
| $CH_3CN$ | 6(2, 0) − 5(2, 0) | 110374.989(0) | 47.1 | 164.06 | 152 | -30.4(1.1) | 4.2(1.1) | 680(57) |
| $CH_3CN$ | 6(1, 0) − 5(1, 0) | 110381.372(0) | 25.7 | 179.45 | 297 | -30.5(1.1) | 3.6(1.1) | 1140(57) |
| $CH_3CN$ | 6(0, 0) − 5(0, 0) | 110383.500(0) | 18.5 | 184.58 | 346 | -30.5(0.9) | 4.3(1.1) | 1589(57) |
| $CH_3OCHO$ | 9(7, 3) − 8(7, 2) E | 110536.003(1e-2) | 59.1 | 9.46692 | 10 | -30.4(1.3) | 4.4(3.6) | 47(29) |
| $CH_3OCHO$ | 9(2, 6) − 8(1, 5) A | 110560.051(1e-2) | 19.0 | 1.39665 | 290 | -30.4(0.2) | 3.0(0.1) | 920(23) |
| $CH_3OCHO$ | 9(6, 3) − 8(6, 2) A | 110663.429(1e-2) | 50.4 | 13.31127 | 21 | -30.4(0.5) | 2.8(0.1) | 539(22) |
| $CH_3OCHO$ | 9(6, 4) − 8(6, 3) A | 110663.273(1e-2) | 50.4 | 13.3113 | blended | – | – | – |
| $CH_3OCHO$ | 10(1,10) − 9(1, 9) E | 110788.664(1e-2) | 30.3 | 26.16584 | 17 | -30.5(0.7) | 3.8(1.6) | 69(25) |
| $CH_3OCHO$ | 10(1,10) − 9(1, 9) A | 110790.526(1e-2) | 30.3 | 26.17539 | 23 | -30.4(0.4) | 2.1(0.8) | 51(19) |
| $CH_3OCHO$ | 9(5, 4) − 8(5, 3) E | 110873.955(1e-2) | 43.2 | 16.55557 | 10 | -30.4(2.5) | 3.0(2.0) | 24(11) |
| $CH_3OCHO$ | 9(3, 7) − 8(3, 6) E | 110879.766(1e-2) | 32.6 | 21.245 | 29 | -30.4(0.6) | 2.7(1.3) | 81(35) |
| $CH_3OCHO$ | 9(5, 5) − 8(5, 4) E | 110882.331(1e-2) | 43.2 | 16.55225 | 17 | -30.4(1.3) | 2.1(1.9) | 33(30) |
| $CH_3OCHO$ | 9(3, 7) − 8(3, 6) A | 110887.092(1e-2) | 32.6 | 21.25577 | 16 | -30.4(1.2) | 2.5(1.5) | 41(34) |
| $CH_3OCHO$ | 9(5, 4) − 8(5, 3) A | 110890.256(1e-2) | 43.2 | 16.56106 | 23 | -30.4(0.7) | 2.4(1.4) | 60(33) |

**Table A2.** (Continued)

| Species | Transitions | Rest Freq. (MHz) | $E_u$ (K) | $\mu^2S$ ($D^2$) | $T_{mb}$ (mK) | $V_{LSR}$ (km $s^{-1}$) | $\Delta V$ (km $s^{-1}$) | $\int T_{mb}$ dv (mK km $s^{-1}$) |
|---|---|---|---|---|---|---|---|---|
| $CH_3OCHO$ | 10(0, 10) − 9(0, 9) E | 111169.903(1e-2) | 30.2 | 26.18776 | 33 | -30.4(0.3) | 2.3(0.7) | 80(22) |
| $CH_3OCHO$ | 10(0, 10) − 9(0, 9) A | 111171.634(1e-2) | 30.2 | 26.19136 | 30 | -30.5(0.4) | 3.9(1.2) | 126(30) |
| $CH_3OCHO$ | 9(4, 6) − 8(4, 5) A | 111195.962(1e-2) | 37.2 | 19.21722 | 18 | -30.4(0.4) | 1.8(0.7) | 35(16) |
| $CH_3OCHO$ | 9(4, 6) − 8(4, 5) E | 111223.491(1e-2) | 37.2 | 18.18412 | 13 | -30.4(0.7) | 1.6(1.4) | 23(16) |
| $CH_3OH$, vt=0-2 | 7(2)$^+$ − 8(1)$^+$, vt=0 | 111289.453(13e-3) | 102.7 | 9.3425 | 50 | -30.5(0.3) | 6.6(0.6) | 349(33) |
| $CH_3OCHO$ | 9(4, 5) − 8(4, 4) E | 111408.412(1e-2) | 37.3 | 18.18767 | 14 | -30.4(0.7) | 4.4(1.6) | 64(20) |
| $CH_3OCHO$ | 9(4, 5) − 8(4, 4) A | 111453.300(1e-2) | 37.2 | 19.21778 | 72 | -30.4(1.9) | 7.3(3.4) | 56(25) |
| $CH_3OH$, vt=0-2 | 17(-2) − 17(1) E2, vt=0 | 111.626.514(15e-3) | 381.5 | 20.231 | 24 | -30.4(0.5) | 7.0(1.4) | 177(29) |
| $CH_3OCHO$ | 9(1, 8) − 8(1, 7) E | 111674.131(1e-2) | 28.1 | 23.18984 | 31 | -30.5(0.3) | 3.4(1.0) | 114(23) |
| $CH_3OCHO$ | 9(1, 8) − 8(1, 7) A | 111682.189(1e-2) | 28.1 | 23.19587 | 24 | -30.4(0.5) | 4.8(1.1) | 120(24) |
| $CH_3OCHO$ | 10(1, 10) − 9(0, 9) E | 111734.002(1e-2) | 30.3 | 3.84434 | 38 | -30.5(1.4) | 0.6(0.1) | 23(9) |
| $CH_3OCHO$ | 10(1, 10) − 9(0, 9) A | 111735.307(1e-2) | 30.3 | 3.84224 | 32 | -30.4(0.1) | 0.5(0.2) | 18(8) |
| t-HCOOH | 5(0, 5) − 4(0, 4) | 111746.784(3e-3) | 16.1 | 10.092 | 34 | -30.0(0.4) | 6.3(1.0) | 230(28) |
| $CH_3OCH_3$ | 7(0, 7) − 6(1, 6) AA | 111782.562(8e-3) | 25.2 | 68.047 | 50 | -30.5(0.2) | 4.2(0.5) | 226(24) |
| $HC_5N$ | 42 − 41 | 111823.024(0) | 115.4 | 2362.2 | 13 | -31.0(0.5) | 1.3(0.8) | 18(12) |
| $CH_3CHO$ | 6(1, 6) − 5(1, 5) A, vt=0 | 112248.716(3e-3) | 21.1 | 73.76807 | 144 | -30.5(0.5) | 4.3(0.5) | 662(21) |
| $CH_3CHO$ | 6(1, 6) − 5(1, 5) E, vt=0 | 112254.508(3e-3) | 21.2 | 73.79585 | 142 | -30.5(0.6) | 5.1(0.5) | 766(21) |
| t-HCOOH | 5(2, 4) − 4(2, 3) | 112287.145 (3e-3) | 28.9 | 8.4851 | 20 | -30.0(0.5) | 5.3(0.5) | 1759(21) |
| $C^{17}O$ | 1 − 0 | 112359.284(1e-3) | 5.4 | 0.01217 | 311 | -30.3(0.5) | 5.3(0.5) | 1759(21) |
| t-HCOOH | 5(4, 2) − 4(4, 1) | 112432.292(3e-3) | 67.1 | 3.6372 | blended | − | − | − |
| t-HCOOH | 5(4, 1) − 4(4, 0) | 112432.319(3e-3) | 67.1 | 3.6372 | 22 | -30.0(0.3) | 1.4(0.5) | 32(12) |
| t-HCOOH | 5(3, 3) − 4(3, 2) | 112459.621(3e-3) | 44.8 | 6.4662 | 19 | -30.0(0.3) | 1.3(0.6) | 27(12) |
| t-HCOOH | 5(3, 2) − 4(3, 1) | 112467.007(3e-3) | 44.8 | 6.4654 | 19 | -30.0(0.5) | 3.4(0.8) | 67(18) |
| CN | N= 1-0, J=1/2-1/2, F=1/2-1/2 | 113123.370(6e-3) | 5.4 | 0.15271 | 356 | -30.5(0.) | 2.8(0.1) | 1078(27) |
| CN | N= 1-0, J=1/2-1/2, F=1/2-3/2 | 113144.157(6e-3) | 5.4 | 1.2492 | 1351 | -30.5(0.) | 3.3(0.1) | 4796(37) |
| CN | N= 1-0, J=1/2-1/2, F=3/2-1/2 | 113170.492(4e-3) | 5.4 | 1.2199 | 1489 | -30.5(0.) | 3.3(0.1) | 5229(32) |
| CN | N= 1-0, J=1/2-1/2, F=3/2-3/2 | 113191.279(3e-3) | 5.4 | 1.5836 | 1443 | -30.5(0.1) | 3.4(0.1) | 5249(30) |
| CCS | 9(8) − 8(7) | 113410.186(2e-2) | 33.6 | 65.427 | 29 | -30.5(0.5) | 5.5(0.5) | 326(167) |
| CN | N= 1-0, J=3/2-1/2, F=3/2-1/2 | 113488.120(3e-3) | 5.4 | 1.5838 | 1433 | -30.4(0.5) | 3.6(0.5) | 5503(167) |
| CN | N= 1-0, J=3/2-1/2, F=5/2-3/2 | 113490.970(2e-3) | 5.4 | 4.205 | 2701 | -30.5(0.4) | 3.6(0.5) | 10428(167) |
| CN | N= 1-0, J=3/2-1/2, F=1/2-1/2 | 113499.644(3e-3) | 5.4 | 1.2491 | 1010 | -30.4(0.5) | 3.3(0.5) | 3590(167) |
| CN | N= 1-0, J=3/2-1/2, F=3/2-3/2 | 113508.907(3e-3) | 5.4 | 1.2196 | 1211 | -30.5(0.8) | 3.4(0.5) | 4440(167) |
| CN | N= 1-0, J=3/2-1/2, F=1/2-3/2 | 113520.432(4e-3) | 5.4 | 0.15263 | 280 | -30.5(0.5) | 2.8(0.5) | 840(167) |
| | | G133.94+01.06 | | | | | | |
| CCS | 8(9) − 7(8) | 106347.726(2e-2) | 25.0 | 74.425 | 80 | -47.0(0.2) | 4.1(0.4) | 348(32) |
| H$\alpha$ | H (39) $\alpha$ | 106737.357(0) | − | − | 622 | -45.0(0.5) | 28.6(0.5) | 18955(95) |
| $CH_3OCH_3$ | 9(1, 8) − 8(2, 7) AE | 106779.083(11e-3) | 43.4 | 17.39008 | 105 | -47.1(0.5) | 20.5(0.5) | 2289(83) |
| $OC^{34}S$ | 9 − 8 | 106787.390(2e-3) | 25.6 | 4.601 | 85 | -47.8(0.4) | 10.1(1.0) | 914(77) |
| $HOCO^+$ | 5(0, 5) − 4(0, 4) | 106913.545(3e-3) | 15.4 | 36.454 | 39 | -47.0(0.4) | 1.4(0.6) | 59(28) |
| $CH_3OH$, vt=0-2 | 3(1)$^+$ − 4(0)$^+$, vt=0 | 107013.831(1e-2) | 28.3 | 12.036 | 10420 | -46.5(0.) | 1.8(0.1) | 19724(808) |
| $CH_3OH$, vt=0-2 | 15(-2) − 15(1) E2, vt=0 | 107159.906(14e-3) | 304.7 | 10.421 | 99 | -46.5(0.3) | 7.1(0.5) | 746(50) |
| $HOCO^+$ | 5(1, 4) − 4(1, 3) | 107315.356(2e-3) | 52.8 | 34.996 | 21 | -47.0(0.5) | 1.5(1.3) | 34(24) |
| $C_2H_5CN$ | 12(7, 5) − 11(7, 4) | 107485.160(5e-2) | 88.0 | 117.36 | 60 | -47.0(0.5) | 4.3(0.5) | 28(15) |
| $C_2H_5CN$ | 12(6, 6) − 11(6, 5) | 107486.949(5e-2) | 73.6 | 133.42 | 58 | -47.0(0.4) | 7.9(0.5) | 493(15) |
| $C_2H_5CN$ | 12(5, 7) − 11(5, 6) | 107502.432(5e-2) | 61.3 | 146.99 | 18 | -47.0(0.5) | 3.8(0.5) | 75(15) |
| $C_2H_5CN$ | 12(10, 2) − 11(10, 1) | 107519.861(5e-2) | 144.6 | 54.355 | 58 | -47.0(0.4) | 7.0(0.5) | 432(15) |
| $CH_3OCHO$ | 9( 2, 8) − 8( 2, 7) E | 107537.258(1e-2) | 28.8 | 22.60702 | 98 | -47.1(0.5) | 6.6(0.5) | 692(15) |
| $CH_3OCHO$ | 9( 2, 8) − 8( 2, 7) A | 107543.711(1e-2) | 28.8 | 22.61344 | 121 | -47.1(0.5) | 5.6(0.5) | 716(15) |
| $C_2H_5CN$ | 12(4, 9) − 11(4, 8) | 107544.042(5e-2) | 51.3 | 158.12 | blended | − | − | − |
| $C_2H_5CN$ | 12(4, 8) − 11(4, 7) | 107547.460(5e-2) | 51.3 | 158.11 | 33 | -47.0(0.5) | 7.8(0.5) | 408(15) |
| $C_2H_5CN$ | 12(3, 10) − 11(3, 9) | 107594.056(5e-2) | 43.6 | 166.77 | 31 | -47.0(1.3) | 10.5(2.5) | 340(76) |
| $CH_3OCHO$ | 23(6, 17) − 23(5, 18) E | 107604.366(1e-2) | 189.0 | 7.68978 | 17 | -47.0(0.8) | 2.2(1.7) | 41(31) |
| $C_2H_5CN$ | 12(3, 9) − 11(3, 8) | 107734.723(5e-2) | 43.6 | 166.76 | 18 | -47.0(1.4) | 3.7(2.1) | 73(47) |
| $SO_2$ | 12(4, 8) − 13(3, 11) | 107843.470(2e-3) | 111.0 | 4.5354 | 111 | -48.0(0.2) | 4.6(0.4) | 548(38) |
| $CH_3OCHO$ | 15(5, 10) − 15(4, 11) E | 108045.959(1e-2) | 87.9 | 4.11041 | 17 | -48.0(0.4) | 1.1(0.8) | 20(18) |
| $CH_3OCHO$ | 15(5, 10) − 15(4, 11) A | 108050.939(1e-2) | 87.9 | 4.11748 | 19 | -47.0(1.3) | 8.9(2.4) | 182(50) |
| $OC^{33}S$ | 9 − 8 | 108084.784(2e-3) | 25.9 | | 23 | -46.9(2.8) | 5.6(3.7) | 222(55) |
| t-HCOOH | 5(1, 5) − 4(1, 4) | 108126.720(3e-3) | 18.8 | 9.6966 | 41 | -46.5(0.5) | 7.3(1.1) | 321(47) |
| $^{13}CN$ | 1(1, 0) − 0(1, 1), F = 1 − 2 | 108426.889(5e-2) | 5.2 | 1.267 | 33 | -47.3(0.6) | 1.8(1.1) | 63(35) |
| $^{13}CN$ | 1(1, 1) − 0(1, 0), F = 0 − 1 | 108631.121(5e-2) | 5.2 | 0.642 | 41 | -47.0(1.1) | 1.1(1.0) | 48(16) |
| $^{13}CN$ | 1(1, 1) − 0(1, 0), F = 1 − 1 | 108636.923(5e-2) | 5.2 | 1.932 | 33 | -47.6(1.1) | 8.7(1.1) | 302(16) |
| $^{13}CN$ | 1(2, 1) − 0(1, 1), F = 1 − 0 | 108638.212(5e-2) | 5.2 | 0.722 | blended | − | − | − |
| $^{13}CN$ | 1(2, 1) − 0(1, 1), F = 2 − 1 | 108643.590(5e-2) | 5.2 | 0.856 | 23 | -47.8(1.1) | 2.8(1.1) | 317(16) |
| $^{13}CN$ | 1(2, 1) − 0(1, 1), F = 0 − 1 | 108644.346(5e-2) | 5.2 | 0.642 | blended | − | − | − |
| $^{13}CN$ | 1(2, 1) − 0(1, 1), F = 1 − 1 | 108645.064(5e-2) | 5.2 | 0.551 | blended | − | − | − |
| $^{13}CN$ | 1(1, 1) − 0(1, 0), F = 2 − 1 | 108651.297(5e-2) | 5.2 | 3.276 | 36 | -47.2(1.1) | 4.1(1.1) | 160(16) |
| $^{13}CN$ | 1(2, 1) − 0(1, 1), F = 2 − 2 | 108657.646(5e-2) | 5.2 | 2.420 | 38 | -47.9(1.1) | 2.7(1.1) | 110(16) |
| $^{13}CN$ | 1(2, 1) − 0(1, 1), F = 1 − 2 | 108658.948(5e-2) | 5.2 | 0.669 | blended | − | − | − |
| $^{13}CN$ | 1(2, 2) − 0(1, 1), F = 3 − 2 | 108780.201(5e-2) | 5.2 | 4.905 | 52 | -47.2(1.6) | 3.4(2.9) | 190(180) |
| $^{13}CN$ | 1(2, 2) − 0(1, 1), F = 2 − 1 | 108782.374(5e-2) | 5.2 | 2.586 | 29 | -47.2(3.5) | 5.6(1.0) | 172(79) |
| $^{13}CN$ | 1(2, 2) − 0(1, 1), F = 1 − 0 | 108786.982(5e-2) | 5.2 | 1.144 | 14 | -47.1(1.1) | 7.9(2.1) | 264(77) |
| $^{13}CN$ | 1(2, 2) − 0(1, 1), F = 1 − 1 | 108793.753(5e-2) | 5.2 | 0.894 | 19 | -47.3(2.4) | 3.2(0.3) | 65(9) |
| $^{13}CN$ | 1(2, 2) − 0(1, 1), F = 2 − 2 | 108796.400(5e-2) | 5.2 | 0.918 | 27 | -47.1(2.2) | 4.5(0.4) | 128(14) |
| $CH_3OH$, vt=0-2 | 0(0) − 1(-1) E2, vt=0 | 108893.945(12e-3) | 13.1 | 3.9134 | 1108 | -46.5(0.) | 6.0(0.1) | 5857(43) |
| $SO_2$ | 39(6, 34) − 38(7, 31) | 108955.915(2e-3) | 808.3 | 16.377 | 44 | -48.0(0.5) | 6.3(1.2) | 297(49) |
| $CH_3OH$, vt=0-2 | 14(5) − 15(4) E1, vt=0 | 109138.783(15e-3) | 379.7 | 13.593 | 172 | -46.5(0.2) | 8.6(0.5) | 1574(72) |
| $CH_3OH$, vt=0-2 | 16(-2) − 16(1) E2, vt=0 | 109153.184 (14e-3) | 342.0 | 14.726 | 130 | -46.5(0.3) | 10.2(0.7) | 1412(78) |
| $HC_3N$ | 12 − 11 | 109173.634(1e-2) | 34.1 | 167.1 | 2716 | -47.5(0.) | 3.9(0.1) | 11190(49) |
| SO | 3(2) − 2(1) | 109252.220(1e-1) | 21.1 | 3.5585 | 2137 | -47.5(0.) | 5.6(0.1) | 12686(55) |
| $HC_3N$, $v_7$=1 | 12(-1) − 11(1) | 109442.013(2e-2) | 355.0 | 165.12 | 35 | -47.0(1.1) | 8.5(4.2) | 620(100) |
| OCS | 9 − 8 | 109463.063(5e-3) | 26.3 | 4.6034 | 772 | -47.5(0.) | 6.8(0.1) | 5581(50) |
| HNCO | 5(1, 5) − 4(1, 4) | 109495.996(6e-3) | 59.0 | 11.847 | 24 | -47.0(1.2) | 8.1(2.6) | 203(55) |
| H$\gamma$ | H (55) $\gamma$ | 109536.001(0) | − | − | 64 | -45.1(0.8) | 21.8(1.7) | 1478(111) |
| $CH_3OCH_3$ | 8(2, 7) − 8(1, 8) EA | 109571.396(9e-3) | 38.3 | 23.947 | 62 | -47.5(0.6) | 2.8(1.1) | 122(25) |
| $CH_3OCH_3$ | 8(2, 7) − 8(1, 8) AE | 109571.403(9e-3) | 38.3 | 35.921 | blended | − | − | − |
| $CH_3OCH_3$ | 8(2, 7) − 8(1, 8) EE | 109574.088(7e-3) | 38.3 | 95.791 | 50 | -47.6(0.5) | 6.2(1.1) | 331(25) |
| $CH_3OCH_3$ | 8(2, 7) − 8(1, 8) AA | 109576.778(11e-3) | 38.3 | 59.869 | 48 | -47.5(0.5) | 9.6(1.1) | 486(25) |
| $C_2H_5CN$ | 12(1, 11) − 11(1, 10) | 109650.263(5e-2) | 35.4 | 176.49 | 22 | -47.0(0.9) | 5.7(1.8) | 136(43) |
| $HC_3N$, $v_7$=1 | 12(1) − 11(-1) | 109598.818(2e-2) | 355.0 | 165.12 | 44 | -46.9(0.5) | 5.8(0.9) | 274(44) |
| $SO_2$ | 17(5, 13) − 18(4, 14) | 109757.585(2e-3) | 202.1 | 6.6069 | 60 | -48.0(0.4) | 7.9(1.0) | 506(59) |
| $C^{18}O$ | 1 − 0 | 109782.173(6e-3) | 5.3 | 0.01221 | 2920 | -47.5(0.1) | 4.5(0.1) | 13864(44) |
| HNCO | 5(0, 5) − 4(0, 4) | 109905.749(7e-3) | 15.8 | 12.482 | 265 | -47.0(0.1) | 5.0(0.3) | 1397(61) |
| $^{13}CO$ | 1 − 0 | 110201.35(0) | 5.3 | 0.01220 | 19449 | -47.5(0.1) | 4.9(0.1) | 100770(102) |
| HNCO | 5(1, 4) − 4(1, 3) | 110298.089(5e-3) | 59.2 | 11.847 | 23 | -47.0(1.6) | 4.0(2.9) | 98(73) |
| $CH_3CN$ | 6(5, 0) − 5(5, 0) | 110330.345(0) | 197.1 | 56.399 | 33 | -47.5(0.8) | 2.8(1.7) | 99(60) |
| $CH_3CN$ | 6(4, 0) − 5(4, 0) | 110349.471(0) | 132.8 | 102.54 | 108 | -47.5(0.4) | 5.1(0.8) | 582(84) |
| $CH_3CN$ | 6(3, 0) − 5(-3, 0) | 110364.354(0) | 82.8 | 138.45 | 371 | -47.5(0.1) | 6.6(0.3) | 2612(98) |
| $CH_3CN$ | 6(-3, 0) − 5(3, 0) | 110364.354(0) | 82.8 | 138.45 | blended | − | − | − |

**Table A2.** (Continued)

| Species | Transitions | Rest Freq. | $E_u$ | $\mu^2S$ | $T_{mb}$ | $V_{LSR}$ | $\Delta V$ | $\int T_{mb}$ dv |
|---|---|---|---|---|---|---|---|---|
| | | (MHz) | (K) | ($D^2$) | (mK) | (km $s^{-1}$) | (km $s^{-1}$) | (mK km $s^{-1}$) |
| $CH_3CN$ | 6(2, 0) − 5(2, 0) | 110374.989(0) | 47.1 | 164.06 | 365 | -47.5(0.1) | 6.3(0.3) | 2443(101) |
| $CH_3CN$ | 6(1, 0) − 5(1, 0) | 110381.372(0) | 25.7 | 179.45 | 502 | -47.4(0.1) | 4.1(0.2) | 2198(181) |
| $CH_3CN$ | 6(0, 0) − 5(0, 0) | 110383.500(0) | 18.5 | 184.58 | 702 | -47.4(0.1) | 6.6(0.3) | 4928(207) |
| $CH_3OCHO$ | 7(2, 6) − 6(1, 5) | 110526.190(1e-2) | 206.7 | 1.41631 | 52 | -47.1(0.5) | 3.8(0.5) | 209(18) |
| $CH_3OCHO$ | 9(7, 2) − 8(7, 1) A | 110535.186(1e-2) | 59.1 | 9.46711 | 96 | -47.1(0.5) | 7.1(0.5) | 728(18) |
| $CH_3OCHO$ | 9(2, 6) − 8(1, 5) E | 110550.203(1e-2) | 19.0 | 1.39763 | 125 | -47.0(0.5) | 2.1(0.5) | 274(18) |
| $CH_3OCHO$ | 9(2, 6) − 8(1, 5) A | 110560.051(1e-2) | 19.0 | 1.39665 | 21 | -47.0(0.4) | 1.7(0.5) | 39(18) |
| $CH_3OCHO$ | 9(6, 3) − 8(6, 2) E | 110652.813(1e-2) | 50.5 | 13.30853 | 148 | -47.0(0.2) | 8.9(0.5) | 1408(65) |
| $CH_3OCHO$ | 9(6, 3) − 8(6, 2) A | 110663.429(1e-2) | 50.4 | 13.31127 | 61 | -47.0(0.6) | 11.9(1.2) | 779(72) |
| $CH_3OCHO$ | 9(6, 4) − 8(6, 3) A | 110663.273(1e-2) | 50.4 | 13.3113 | blended | – | – | – |
| $CH_3OCHO$ | 10(1,10) − 9(1, 9) E | 110788.664(1e-2) | 30.3 | 26.16584 | 169 | -47.2(1.1) | 4.0(1.1) | 713(68) |
| $CH_3OCHO$ | 10(1,10) − 9(1, 9) A | 110790.526(1e-2) | 30.3 | 26.17539 | 234 | -47.0(1.1) | 4.4(1.1) | 1100(68) |
| $CH_3OCHO$ | 9(5, 4) − 8(5, 3) E | 110873.955(1e-2) | 43.2 | 16.55557 | 56 | -47.2(1.1) | 6.8(1.1) | 401(62) |
| $CH_3OCHO$ | 9(3, 7) − 8(3, 6) E | 110879.766(1e-2) | 32.6 | 21.245 | 152 | -47.2(1.1) | 4.3(1.1) | 689(62) |
| $CH_3OCHO$ | 9(5, 5) − 8(5, 4) A | 110880.447(1e-2) | 43.2 | 16.56015 | 133 | -47.0(1.1) | 6.2(1.1) | 877(62) |
| $CH_3OCHO$ | 9(3, 7) − 8(3, 6) A | 110887.092(1e-2) | 32.6 | 21.25577 | 92 | -47.1(1.0) | 3.8(1.1) | 373(62) |
| $CH_3OCHO$ | 9(5, 4) − 8(5, 3) A | 110890.256(1e-2) | 43.2 | 16.56106 | 99 | -47.0(1.0) | 10.5(1.1) | 1113(62) |
| $CH_3OCHO$ | 10(0, 10) − 9(0, 9) E | 111169.903(1e-2) | 30.2 | 26.18776 | 76 | -47.0(0.3) | 2.0(0.9) | 165(105) |
| $CH_3OCHO$ | 10(0, 10) − 9(0, 9) A | 111171.634(1e-2) | 30.2 | 26.19136 | 185 | -47.0(0.4) | 7.3(0.9) | 1445(160) |
| $CH_3OCHO$ | 9(4, 6) − 8(4, 5) A | 111195.962(1e-2) | 37.2 | 19.21722 | 90 | -47.0(0.4) | 2.8(0.9) | 269(59) |
| $CH_3OCHO$ | 9(4, 6) − 8(4, 5) E | 111223.491(1e-2) | 37.2 | 18.18412 | 72 | -47.1(0.5) | 6.3(0.9) | 483(70) |
| $CH_3OH$, vt=0-2 | 7(2)$^+$ − 8(1)$^+$, vt=0 | 111289.453(13e-3) | 102.7 | 9.3425 | 683 | -46.4(0.1) | 5.8(0.2) | 4247(80) |
| $CH_3OCHO$ | 9(4, 5) − 8(4, 4) E | 111408.412(1e-2) | 37.3 | 18.18767 | 74 | -47.0(0.5) | 1.9(0.8) | 151(68) |
| $CH_3OCHO$ | 9(4, 5) − 8(4, 4) A | 111453.300(1e-2) | 37.2 | 19.21778 | 69 | -47.0(0.7) | 2.8(1.4) | 208(88) |
| $CH_3OH$, vt=0-2 | 17(-2) − 17(1) E2, vt=0 | 111626.514(15e-3) | 381.5 | 20.231 | 88 | -46.5(0.5) | 3.8(0.5) | 358(22) |
| $CH_3OCHO$ | 9(1, 8) − 8(1, 7) E | 111674.131(1e-2) | 28.1 | 23.18984 | 99 | -47.0(0.5) | 5.1(0.5) | 539(22) |
| $CH_3OCHO$ | 9(1, 8) − 8(1, 7) A | 111682.189(1e-2) | 28.1 | 23.19587 | 119 | -47.0(0.3) | 3.6(0.5) | 456(22) |
| $CH_3OCHO$ | 10(1, 10) − 9(0, 9) E | 111734.002(1e-2) | 30.3 | 3.84434 | 48 | -47.0(0.8) | 4.1(1.1) | 212(48) |
| $CH_3OCHO$ | 10(1, 10) − 9(0, 9) A | 111735.307(1e-2) | 30.3 | 3.84224 | 34 | -47.1(0.5) | 1.5(1.1) | 56(48) |
| $CH_3OCH_3$ | 19(3,16) − 19(2,17) AE | 111741.351(26e-3) | 187.5 | 123.39211 | 30 | -47.5(1.1) | 2.8(1.1) | 88(48) |
| $CH_3OCH_3$ | 9(3,16) − 19(2,17) EE | 111742.794(25e-3) | 187.5 | 329.06069 | 99 | -47.5(1.0) | 6.8(1.1) | 718(48) |
| $CH_3OCH_3$ | 19(3, 16) − 19(2, 17) AA | 111744.238(29e-3) | 187.5 | 205.6671 | 26 | -47.5(1.0) | 8.3(1.1) | 230(48) |
| t-HCOOH | 5(0, 5) − 4(0, 4) | 111746.784(3e-3) | 16.1 | 10.092 | blended | – | – | – |
| $CH_3OCH_3$ | 7(0, 7) − 6(1, 6) AA | 111782.562(8e-3) | 25.2 | 53.86755 | 216 | -47.5(1.1) | 7.7(1.1) | 1779(48) |
| $CH_3OCH_3$ | 7(5, 3) − 8(4, 5) AA | 111804.354(33e-3) | 60.6 | 3.07241 | 74 | -47.5(0.8) | 3.7(1.7) | 291(149) |
| $CH_3OCH_3$ | 7(5, 3) − 8(4, 5) EE | 111804.813(26e-3) | 60.6 | 7.72103 | blended | – | – | – |
| $CH_3OCH_3$ | 7(5, 2) − 8(4, 5) AA | 111809.374(33e-3) | 60.6 | 5.12083 | 86 | -47.5(2.1) | 3.5(1.2) | 318(116) |
| $CH_3OCH_3$ | 7(5, 2) − 8(4, 5) EE | 111812.674(31e-3) | 60.6 | 0.47164 | 77 | -47.5(0.8) | 2.5(2.1) | 203(216) |
| H$\beta$ | H (48) $\beta$ | 111885.070(0) | – | – | 134 | -46.6(1.0) | 25.9(1.7) | 3709(257) |
| $CH_3CHO$ | 6(1, 6) − 5(1, 5) A, vt=0 | 112248.716(3e-3) | 21.1 | 73.76807 | 127 | -47.6(0.5) | 3.9(1.1) | 521(122) |
| $CH_3CHO$ | 6(1, 6) − 5(1, 5) E, vt=0 | 112254.508(3e-3) | 21.2 | 73.79585 | 131 | -47.6(0.4) | 4.2(1.2) | 582(133) |
| $C^{17}O$ | 1 − 0 | 112359.284(1e-3) | 5.4 | 0.01217 | 748 | -47.0(0.1) | 6.1(0.1) | 4844(97) |
| t-HCOOH | 5(2, 4) − 4(2, 3) | 112287.145(3e36) | 28.9 | 8.4851 | 54 | 1.5 | 2.8(1.4) | 163(61) |
| t-HCOOH | 5(3, 3) − 4(3, 2) | 112459.621(3e-3) | 44.8 | 6.4662 | 25 | -46.0(1.4) | 5.4(3.0) | 146(76) |
| $C_2H_5CN$ | 13(1, 13) − 12(1, 12) | 112646.350(9e-2) | 39.0 | 191.45 | 63 | -47.0(0.7) | 9.2(2.1) | 614(97) |
| $CH_3OCHO$ | 14(5, 9) −14(4, 10) E | 112672.759(1e-2) | 78.9 | 3.64313 | 39 | -47.0(3.2) | 8.9(7.4) | 374(327) |
| $CH_3OCHO$ | 14(5, 9) −14(4, 10) A | 112676.856(1e-2) | 78.9 | 3.67559 | 38 | -47.0(2.8) | 10.1(2.8) | 409(389) |
| $CH_3OCH_3$ | 20(3, 17) − 20(2, 18) EE | 113000.970(32e-3) | 206.1 | 348.88725 | 65 | -47.5(0.5) | 9.5(0.5) | 662(24) |
| $CH_3OCH_3$ | 17(3, 14) − 17(2, 15) EA | 113057.427(19e-3) | 153.1 | 132.79 | 207 | -47.5(0.4) | 4.9(0.5) | 1078(24) |
| $CH_3OCH_3$ | 17(3, 14) − 17(2, 15) AE | 113057.425(18e-3) | 153.1 | 88.525 | blended | – | – | – |
| $CH_3OCH_3$ | 17(3, 14) − 17(2, 15) EE | 113059.249(17e-3) | 153.1 | 354.12 | 111 | -47.4(0.6) | 2.1(0.5) | 243(24) |
| $CH_3OCH_3$ | 17(3, 14) − 17(2, 15) AA | 113061.072(22e-3) | 153.1 | 221.33 | 70 | -47.5(0.6) | 2.7(0.5) | 205(24) |
| CN | N= 1-0, J=1/2-1/2, F=1/2-1/2 | 113123.370(6e-3) | 5.4 | 0.15271 | 237 | -47.5(0.5) | 5.4(0.5) | 1371(132) |
| CN | N= 1-0, J=1/2-1/2, F=1/2-3/2 | 113144.157(6e-3) | 5.4 | 1.2492 | 1001 | -47.4(0.5) | 5.1(0.5) | 5466(132) |
| CN | N= 1-0, J=1/2-1/2, F=3/2-1/2 | 113170.492(4e-3) | 5.4 | 1.2199 | 1109 | -47.5(0.6) | 5.0(0.5) | 5894(132) |
| CN | N= 1-0, J=1/2-1/2, F=3/2-3/2 | 113191.279(3e-3) | 5.4 | 1.5836 | 1100 | -47.5(0.5) | 5.4(0.5) | 6341(132) |
| CCS | 9(8) − 8(7) | 113410.186(2e-2) | 33.6 | 65.427 | 53 | -47.1(0.3) | 3.6(0.5) | 200(162) |
| CN | N= 1-0, J=3/2-1/2, F=3/2-1/2 | 113488.120(3e-3) | 5.4 | 1.5838 | 1041 | -47.5(0.5) | 7.8(0.5) | 8606(162) |
| CN | N= 1-0, J=3/2-1/2, F=5/2-3/2 | 113490.970(2e-3) | 5.4 | 4.205 | 2212 | -47.3(0.5) | 4.1(0.5) | 9610(162) |
| CN | N= 1-0, J=3/2-1/2, F=1/2-1/2 | 113499.644(3e-3) | 5.4 | 1.2491 | 660 | -47.5(0.4) | 5.5(0.5) | 3879(162) |
| CN | N= 1-0, J=3/2-1/2, F=3/2-3/2 | 113508.907(3e-3) | 5.4 | 1.2196 | 849 | -47.5(0.4) | 5.5(0.5) | 4933(162) |
| CN | N= 1-0, J=3/2-1/2, F=1/2-3/2 | 113520.432(4e-3) | 5.4 | 0.15263 | 109 | -47.5(0.5) | 4.1(0.5) | 477(162) |
| | | G168.06+00.82 | | | | | | |
| $CH_3OH$, vt=0-2 | 0(0) − 1(-1) E2, vt=0 | 108893.945(12e-3) | 13.1 | 3.9134 | 163 | -25.5(0.1) | 1.7(0.2) | 291(30) |
| $HC_3N$ | 12 − 11 | 109173.634(1e-2) | 34.1 | 167.1 | 142 | -25.6(0.1) | 1.8(0.4) | 274(37) |
| SO | 3(2) − 2(1) | 109252.220(1e-1) | 21.1 | 3.5585 | 470 | -25.0(0.) | 2.5(0.1) | 1236(42) |
| $C^{18}O$ | 1 − 0 | 109782.173(6e-3) | 5.3 | 0.01221 | 1068 | -25.4(0.1) | 2.0(0.1) | 2233(38) |
| $^{13}CO$ | 1 − 0 | 110201.35(0) | 5.3 | 0.01220 | 944 | -25.5(0.1) | 2.4(0.1) | 24147(77) |
| $C^{17}O$ | 1 − 0 | 112359.284(1e-3) | 5.4 | 0.01217 | 142 | -25.3(0.5) | 7.8(3.2) | 1175(0.3) |
| CN | N= 1-0, J=1/2-1/2, F=1/2-3/2 | 113144.157(6e-3) | 5.4 | 1.2492 | 182 | -25.5(0.1) | 2.2(0.4) | 431(59) |
| CN | N= 1-0, J=1/2-1/2, F=3/2-1/2 | 113170.492(4e-3) | 5.4 | 1.2199 | 206 | -25.5(0.1) | 2.1(0.3) | 459(52) |
| CN | N= 1-0, J=1/2-1/2, F=3/2-3/2 | 113191.279(3e-3) | 5.4 | 1.5836 | 230 | -25.4(0.1) | 2.4(0.3) | 598(58) |
| CN | N= 1-0, J=3/2-1/2, F=3/2-1/2 | 113488.120(3e-3) | 5.4 | 1.5838 | 220 | -25.5(0.2) | 1.9(0.3) | 442(63) |
| CN | N= 1-0, J=3/2-1/2, F=5/2-3/2 | 113490.970(2e-3) | 5.4 | 4.205 | 465 | -25.5(0.1) | 2.2(0.2) | 1100(66) |
| CN | N= 1-0, J=3/2-1/2, F=1/2-1/2 | 113499.644(3e-3) | 5.4 | 1.2491 | 226 | -25.5(0.5) | 1.8(0.3) | 424(58) |
| CN | N= 1-0, J=3/2-1/2, F=3/2-3/2 | 113508.907(3e-3) | 5.4 | 1.2196 | 176 | -25.5(0.4) | 3.3(0.8) | 619(95) |
| CN | N= 1-0, J=3/2-1/2, F=1/2-3/2 | 113520.432(4e-3) | 5.4 | 0.15263 | 47 | -25.5(0.4) | 2.0(1.2) | 101(57) |
| | | G176.51+00.20 | | | | | | |
| CCS | 8(9) − 7(8) | 106347.726(2e-2) | 25.0 | 74.425 | 117 | -18.0(0.) | 2.0(0.1) | 248(10) |
| $^{13}CN$ | 1(1, 1) − 0(1, 0), F = 0 − 1 | 108631.121(5e-2) | 5.2 | 0.642 | 13 | -17.8(0.5) | 1.5(1.2) | 20(10) |
| $^{13}CN$ | 1(1, 1) − 0(1, 0), F = 1 − 1 | 108636.923(5e-2) | 5.2 | 1.932 | 34 | -17.8(0.1) | 1.0(0.2) | 37(5) |
| $^{13}CN$ | 1(2, 1) − 0(1, 1), F = 1 − 0 | 108638.212(5e-2) | 5.2 | 0.722 | 12 | -17.7(0.3) | 1.1(0.5) | 14(6) |
| $^{13}CN$ | 1(2, 1) − 0(1, 1), F = 2 − 1 | 108643.590(5e-2) | 5.2 | 0.856 | 12 | -17.3(0.6) | 3.9(1.1) | 48(13) |
| $^{13}CN$ | 1(2, 1) − 0(1, 1), F = 0 − 1 | 108644.346(5e-2) | 5.2 | 0.642 | blended | – | – | – |
| $^{13}CN$ | 1(2, 1) − 0(1, 1), F = 1 − 1 | 108645.064(5e-2) | 5.2 | 0.551 | blended | – | – | – |
| $^{13}CN$ | 1(1, 1) − 0(1, 0), F = 2 − 1 | 108651.297(5e-2) | 5.2 | 3.276 | 39 | -17.7(0.1) | 1.5(0.2) | 64(8) |
| $^{13}CN$ | 1(2, 1) − 0(1, 1), F = 2 − 2 | 108657.646(5e-2) | 5.2 | 2.420 | 32 | -17.8(0.1) | 1.6(0.4) | 54(9) |
| $^{13}CN$ | 1(2, 2) − 0(1, 1), F = 3 − 2 | 108780.201(5e-2) | 5.2 | 4.905 | 50 | -17.6(0.1) | 1.7(0.2) | 94(9) |
| $^{13}CN$ | 1(2, 2) − 0(1, 1), F = 2 − 1 | 108782.374(5e-2) | 5.2 | 2.586 | 25 | -17.8(0.2) | 2.5(0.4) | 67(10) |
| $^{13}CN$ | 1(2, 2) − 0(1, 1), F = 1 − 0 | 108786.982(5e-2) | 5.2 | 1.144 | 12 | -17.8(0.3) | 1.2(0.4) | 15(6) |
| $^{13}CN$ | 1(2, 2) − 0(1, 1), F = 1 − 1 | 108793.753(5e-2) | 5.2 | 0.894 | 12 | -17.6(0.3) | 1.3(0.6) | 17(7) |
| $^{13}CN$ | 1(2, 2) − 0(1, 1), F = 2 − 2 | 108796.400(5e-2) | 5.2 | 0.918 | 14 | -17.8(0.2) | 0.8(0.5) | 12(6) |
| $CH_3OH$, vt=0-2 | 0(0) − 1(-1) E2, vt=0 | 108893.945(12e-3) | 13.1 | 3.9134 | 249 | -18.2(0.1) | 2.1(0.1) | 545(11) |
| $HC_3N$ | 12 − 11 | 109173.634(1e-2) | 34.1 | 167.1 | 1139 | -17.3(0.) | 1.8(0.1) | 2197(12) |
| SO | 3(2) − 2(1) | 109252.220(1e-1) | 21.1 | 3.5585 | 406 | -18.0(0.) | 2.0(0.1) | 864(17) |
| OCS | 9 − 8 | 109463.063(5e-3) | 26.3 | 4.6034 | 54 | -18.5(0.1) | 3.1(0.3) | 175(15) |
| $C^{18}O$ | 1 − 0 | 109782.173(6e-3) | 5.3 | 0.01221 | 1686 | -17.2(0.1) | 2.1(0.1) | 3839(20) |

**Table A2.** (Continued)

| Species | Transitions | Rest Freq. (MHz) | $E_u$ (K) | $\mu^2S$ ($D^2$) | $T_{mb}$ (mK) | $V_{LSR}$ (km $s^{-1}$) | $\Delta V$ (km $s^{-1}$) | $\int T_{mb}$ dv (mK km $s^{-1}$) |
|---|---|---|---|---|---|---|---|---|
| HNCO | 5(0, 5) − 4(0, 4) | 109905.749(7e-3) | 15.8 | 12.482 | 145 | -18.0(0.) | 1.8(0.1) | 275(15) |
| $C^{15}N$ | 1(2, 1) − 0(1, 1) | 110004.091(3e-2) | 5.3 | 0.717 | 15 | -17.8(0.3) | 1.1(0.7) | 18(10) |
| $C^{15}N$ | 1(2, 1) − 0(1, 0) | 110023.540(1e-1) | 5.3 | 1.386 | 24 | -18.3(0.2) | 1.1(0.5) | 29(11) |
| $C^{15}N$ | 1(2, 2) − 0(1, 1) | 110024.590(1e-1) | 5.3 | 3.504 | 23 | -18.2(0.3) | 1.8(0.7) | 44(13) |
| $^{13}CO$ | 1 − 0 | 110201.35(0) | 5.3 | 0.01220 | 9564 | -17.8(0.1) | 2.8(0.1) | 28426(121) |
| $CH_3CN$ | 6(3, 0) − 5(-3, 0) | 110364.354(0) | 82.8 | 138.45 | 16 | -18.1(0.5) | 2.0(0.9) | 33(15) |
| $CH_3CN$ | 6(-3, 0) − 5(3, 0) | 110364.354(0) | 82.8 | 138.45 | blended | – | – | – |
| $CH_3CN$ | 6(2, 0) − 5(2, 0) | 110374.989(0) | 47.1 | 164.06 | 29 | -18.1(0.2) | 1.6(0.4) | 50(13) |
| $CH_3CN$ | 6(1, 0) − 5(1, 0) | 110381.372(0) | 25.7 | 179.45 | 94 | -18.1(0.1) | 1.4(0.2) | 143(13) |
| $CH_3CN$ | 6(0, 0) − 5(0, 0) | 110383.500(0) | 18.5 | 184.58 | 96 | -18.1(0.1) | 1.8(0.2) | 186(15) |
| $CH_3OH$, vt=0-2 | $7(2)^+ - 8(1)^+$, vt=0 | 111289.453(13e-3) | 102.7 | 9.3425 | 12 | -18.2(1.0) | 1.9(1.4) | 25(21) |
| $CH_3OCH_3$ | 7(0, 7) − 6(1, 6) AA | 111782.562(8e-3) | 25.2 | 53.86755 | 19 | -18.0(0.4) | 3.5(0.8) | 70(17) |
| $CH_3CHO$ | 6(1, 6) − 5(1, 5) A, vt=0 | 112248.716(3e-3) | 21.1 | 73.76807 | 57 | -18.3(0.2) | 3.8(0.7) | 232(30) |
| $CH_3CHO$ | 6(1, 6) − 5(1, 5) E, vt=0 | 112254.508(3e-3) | 21.2 | 73.79585 | 62 | -18.3(0.2) | 2.9(0.6) | 190(27) |
| $C^{17}O$ | 1 − 0 | 112359.284(1e-3) | 5.4 | 0.01217 | 316 | -18.0(0.1) | 2.1(0.1) | 705(31) |
| CN | N= 1-0, J=1/2-1/2, F=1/2-1/2 | 113123.370(6e-3) | 5.4 | 0.15271 | 222 | -18.0(0.5) | 1.5(0.5) | 362(61) |
| CN | N= 1-0, J=1/2-1/2, F=1/2-3/2 | 113144.157(6e-3) | 5.4 | 1.2492 | 950 | -18.0(0.5) | 2.1(0.5) | 2092(61) |
| CN | N= 1-0, J=1/2-1/2, F=3/2-1/2 | 113170.492(4e-3) | 5.4 | 1.2199 | 984 | -18.0(0.4) | 2.1(0.5) | 2175(61) |
| CN | N= 1-0, J=1/2-1/2, F=3/2-3/2 | 113191.279(3e-3) | 5.4 | 1.5836 | 1007 | -18.0(0.5) | 2.3(0.5) | 2422(61) |
| CCS | 9(8) − 8(7) | 113410.186(2e-2) | 33.6 | 65.427 | 43 | -18.0(0.3) | 1.0(0.5) | 44(99) |
| CN | N= 1-0, J=3/2-1/2, F=3/2-1/2 | 113488.120(3e-3) | 5.4 | 1.5838 | 990 | -18.0(0.5) | 2.2(0.5) | 2321(99) |
| CN | N= 1-0, J=3/2-1/2, F=5/2-3/2 | 113490.970(2e-3) | 5.4 | 4.205 | 1889 | -18.0(0.5) | 2.5(0.5) | 5077(99) |
| CN | N= 1-0, J=3/2-1/2, F=1/2-1/2 | 113499.644(3e-3) | 5.4 | 1.2491 | 730 | -18.0(0.4) | 2.1(0.5) | 1638(99) |
| CN | N= 1-0, J=3/2-1/2, F=3/2-3/2 | 113508.907(3e-3) | 5.4 | 1.2196 | 883 | -18.0(0.5) | 2.2(0.5) | 2053(99) |
| CN | N= 1-0, J=3/2-1/2, F=1/2-3/2 | 113520.432(4e-3) | 5.4 | 0.15263 | 149 | -18.0(0.7) | 1.9(0.5) | 304(99) |
| | | G183.72−03.66 | | | | | | |
| CCS | 8(9) − 7(8) | 106347.726(2e-2) | 25.0 | 74.425 | 119 | 2.2(0.) | 2.1(0.1) | 272(98) |
| $HOCO^+$ | 5(0, 5) − 4(0, 4) | 106913.545(3e-3) | 15.4 | 36.454 | 40 | 2.2(0.2) | 2.7(0.5) | 113(16) |
| $CH_3OH$, vt=0-2 | $3(1)^+ - 4(0)^+$, vt=0 | 107013.831(1e-2) | 28.3 | 12.036 | 13 | 2.5(0.4) | 5.5(0.8) | 78(13) |
| $HOCO^+$ | 5(1, 4) − 4(1, 3) | 107315.356(2e-3) | 52.8 | 34.996 | 15 | 2.2(0.2) | 1.7(0.5) | 87(46) |
| $^{13}CN$ | 1(1, 0) − 0(1, 1), F = 1 − 0 | 108406.091(5e-2) | 5.2 | 0.191 | 99 | 2.6(0.3) | 1.0(0.5) | 10(6) |
| $^{13}CN$ | 1(1, 0) − 0(1, 1), F = 1 − 1 | 108412.862(5e-2) | 5.2 | 0.635 | 13 | 2.1(0.3) | 2.0(0.7) | 28(9) |
| $^{13}CN$ | 1(1, 0) − 0(1, 1), F = 1 − 2 | 108426.889(5e-2) | 5.2 | 1.267 | 30 | 2.4(0.1) | 1.3(0.3) | 40(7) |
| $^{13}CN$ | 1(1, 1) − 0(1, 0), F = 1 − 1 | 108636.923(5e-2) | 5.2 | 1.932 | 30 | 2.1(0.1) | 1.7(0.3) | 56(9) |
| $^{13}CN$ | 1(2, 1) − 0(1, 1), F = 1 − 0 | 108638.212(5e-2) | 5.2 | 0.722 | 10 | 2.2(0.5) | 1.8(0.8) | 19(9) |
| $^{13}CN$ | 1(2, 1) − 0(1, 1), F = 2 − 1 | 108643.590(5e-2) | 5.2 | 0.856 | 19 | 2.2(0.2) | 0.7(0.5) | 14(7) |
| $^{13}CN$ | 1(2, 1) − 0(1, 1), F = 0 − 1 | 108644.346(5e-2) | 5.2 | 0.642 | 94 | 2.1(0.6) | 2.9(1.2) | 29(11) |
| $^{13}CN$ | 1(2, 1) − 0(1, 1), F = 1 − 1 | 108645.064(5e-2) | 5.2 | 0.551 | blended | – | – | – |
| $^{13}CN$ | 1(1, 1) − 0(1, 0), F = 2 − 1 | 108651.297(5e-2) | 5.2 | 3.276 | 51 | 2.3(0.1) | 1.6(0.2) | 85(9) |
| $^{13}CN$ | 1(2, 1) − 0(1, 1), F = 2 − 2 | 108657.646(5e-2) | 5.2 | 2.420 | 40 | 2.4(0.2) | 1.6(0.2) | 67(9) |
| $^{13}CN$ | 1(2, 1) − 0(1, 1), F = 1 − 2 | 108658.948(5e-2) | 5.2 | 0.669 | 13 | 2.1(0.4) | 2.5(0.9) | 34(11) |
| $^{13}CN$ | 1(2, 2) − 0(1, 1), F = 3 − 2 | 108780.201(5e-2) | 5.2 | 4.905 | 77 | 2.3(0.5) | 1.6(0.5) | 132(5) |
| $^{13}CN$ | 1(2, 2) − 0(1, 1), F = 2 − 1 | 108782.374(5e-2) | 5.2 | 2.586 | 42 | 2.2(0.5) | 1.4(0.5) | 63(5) |
| $^{13}CN$ | 1(2, 2) − 0(1, 1), F = 1 − 0 | 108786.982(5e-2) | 5.2 | 1.144 | 83 | 2.1(0.5) | 2.7(0.5) | 24(5) |
| $^{13}CN$ | 1(2, 2) − 0(1, 1), F = 1 − 1 | 108793.753(5e-2) | 5.2 | 0.894 | 31 | 2.4(0.5) | 0.5(0.1) | 18(5) |
| $^{13}CN$ | 1(2, 2) − 0(1, 1), F = 2 − 2 | 108796.400(5e-2) | 5.2 | 0.918 | 11 | 2.3(0.5) | 1.6(0.5) | 19(5) |
| $CH_3OH$, vt=0-2 | 0(0) − 1(-1) E2, vt=0 | 108893.945(12e-3) | 13.1 | 3.9134 | 206 | 2.6(0.) | 2.8(0.1) | 625(15) |
| $HC_3N$ | 12 − 11 | 109173.634(1e-2) | 34.1 | 167.1 | 1571 | 2.0(0.) | 1.6(0.1) | 2631(24) |
| SO | 3(2) − 2(1) | 109252.220(1e-1) | 21.1 | 3.5585 | 198 | 2.2(0.) | 4.0(0.1) | 847(19) |
| OCS | 9 − 8 | 109463.063(5e-3) | 26.3 | 4.6034 | 74 | 2.0(0.1) | 3.2(0.4) | 252(26) |
| $C^{18}O$ | 1 − 0 | 109782.173(6e-3) | 5.3 | 0.01221 | 686 | 1.8(0.1) | 1.6(0.1) | 1167(20) |
| HNCO | 5(0, 5) − 4(0, 4) | 109905.749(7e-3) | 15.8 | | 12.482 142 | 2.3(0.) | 1.9(0.1) | 294(15) |
| $C^{15}N$ | 1(2, 1) − 0(1, 1) | 110004.091(3e-2) | 5.3 | 0.717 | 5 | 2.1(0.5) | 0.5(0.3) | 30(5) |
| $C^{15}N$ | 1(2, 1) − 0(1, 0) | 110023.540(1e-1) | 5.3 | 1.386 | 17 | 1.9(0.5) | 1.5(0.5) | 26(5) |
| $C^{15}N$ | 1(2, 2) − 0(1, 1) | 110024.590(1e-1) | 5.3 | 3.504 | 30 | 2.3(0.5) | 1.5(0.5) | 49(5) |
| $^{13}CO$ | 1 − 0 | 110201.35(0) | 5.3 | 0.01220 | 4310 | 1.9(0.1) | 2.5(0.1) | 11395(110) |
| $CH_3CN$ | 6(3, 0) − 5(-3, 0) | 110364.354(0) | 82.8 | 138.45 | 33 | 2.0(0.2) | 3.5(0.5) | 122(15) |
| $CH_3CN$ | 6(-3, 0) − 5(3, 0) | 110364.354(0) | 82.8 | 138.45 | blended | – | – | – |
| $CH_3CN$ | 6(2, 0) − 5(2, 0) | 110374.989(0) | 47.1 | 164.06 | 44 | 2.0(0.1) | 2.5(0.5) | 119(15) |
| $CH_3CN$ | 6(1, 0) − 5(1, 0) | 110381.372(0) | 25.7 | 179.45 | 120 | 2.1(0.) | 2.0(0.1) | 257(12) |
| $CH_3CN$ | 6(0, 0) − 5(0, 0) | 110383.500(0) | 18.5 | 184.58 | 132 | 2.0(0.) | 2.1(0.1) | 302(12) |
| $CH_3OH$, vt=0-2 | $7(2)^+ - 8(1)^+$, vt=0 | 111289.453(13e-3) | 102.7 | 9.3425 | 13 | 2.5(1.0) | 10.2(2.7) | 137(29) |
| $CH_3OCH_3$ | 7(0, 7) − 6(1, 6) AA | 111782.562(8e-3) | 25.2 | 53.86755 | 18 | 2.5(0.4) | 2.9(0.9) | 56(15) |
| $CH_3CHO$ | 6(1, 6) − 5(1, 5) A, vt=0 | 112248.716(3e-3) | 21.1 | 73.76807 | 34 | 2.7(0.5) | 1.4(0.9) | 49(31) |
| $CH_3CHO$ | 6(1, 6) − 5(1, 5) E, vt=0 | 112254.508(3e-3) | 21.2 | 73.79585 | 30 | 2.6(0.6) | 1.5(0.7) | 48(30) |
| $C^{17}O$ | 1 − 0 | 112359.284(1e-3) | 5.4 | 0.01217 | 845 | 2.1(0.2) | 3.7(0.5) | 337(42) |
| CN | N= 1-0, J=1/2-1/2, F=1/2-1/2 | 113123.370(6e-3) | 5.4 | 0.15271 | 281 | 2.0(0.5) | 2.0(0.5) | 590(83) |
| CN | N= 1-0, J=1/2-1/2, F=1/2-3/2 | 113144.157(6e-3) | 5.4 | 1.2492 | 1135 | 2.0(0.) | 2.0(0.5) | 2457(83) |
| CN | N= 1-0, J=1/2-1/2, F=3/2-1/2 | 113170.492(4e-3) | 5.4 | 1.2199 | 1207 | 2.1(0.5) | 2.1(0.5) | 2657(83) |
| CN | N= 1-0, J=1/2-1/2, F=3/2-3/2 | 113191.279(3e-3) | 5.4 | 1.5836 | 1228 | 2.1(0.5) | 2.1(0.5) | 2724(83) |
| CCS | 9(8) − 8(7) | 113.410.186(2e-2) | 33.6 | 65.427 | 29 | 2.2(0.4) | 4.8(0.5) | 148(110) |
| CN | N= 1-0, J=3/2-1/2, F=3/2-1/2 | 113488.120(3e-3) | 5.4 | 1.5838 | 1151 | 2.0(0.5) | 2.0(0.5) | 2510(110) |
| CN | N= 1-0, J=3/2-1/2, F=5/2-3/2 | 113490.970(2e-3) | 5.4 | 4.205 | 2098 | 2.0(0.) | 2.4(0.5) | 5381(110) |
| CN | N= 1-0, J=3/2-1/2, F=1/2-1/2 | 113499.644(3e-3) | 5.4 | 1.2491 | 876 | 2.0(0.5) | 2.1(0.5) | 1942(110) |
| CN | N= 1-0, J=3/2-1/2, F=3/2-3/2 | 113508.907(3e-3) | 5.4 | 1.2196 | 1038 | 2.0(0.4) | 2.0(0.5) | 2174(110) |
| CN | N= 1-0, J=3/2-1/2, F=1/2-3/2 | 113520.432(4e-3) | 5.4 | 0.15263 | 242 | 2.0(0.5) | 1.8(0.5) | 459(110) |
| | | G188.94+00.88 | | | | | | |
| CCS | 8(9) − 7(8) | 106347.726(2e-2) | 25.0 | 74.425 | 84 | 3.4(0.1) | 2.5(0.2) | 221(15) |
| $^{34}SO$ | 3(2) − 2(1) | 106743.244(7e-2) | 20.9 | 3.557 | 45 | 3.0(0.2) | 3.2(0.9) | 154(27) |
| $CH_3OH$, vt=0-2 | $3(1)^+ - 4(0)^+$, vt=0 | 107013.831(1e-2) | 28.3 | 12.036 | 89 | 2.9(0.2) | 4.0(0.6) | 376(40) |
| t-HCOOH | 5(1, 5) − 4(1, 4) | 108126.720(3e-3) | 18.8 | 9.6966 | 20 | 3.0(0.4) | 3.1(1.0) | 66(19) |
| $^{13}CN$ | 1(1, 1) − 0(1, 0), F = 0 − 1 | 108631.121(5e-2) | 5.2 | 0.642 | 28 | 3.1(0.2) | 0.8(0.3) | 24(9) |
| $^{13}CN$ | 1(1, 1) − 0(1, 0), F = 1 − 1 | 108636.923(5e-2) | 5.2 | 1.932 | 29 | 3.2(0.3) | 2.5(0.6) | 76(15) |
| $^{13}CN$ | 1(2, 1) − 0(1, 1), F = 1 − 0 | 108638.212(5e-2) | 5.2 | 0.722 | 17 | 3.3(0.6) | 2.8(1.1) | 104(21) |
| $^{13}CN$ | 1(2, 1) − 0(1, 1), F = 2 − 1 | 108643.590(5e-2) | 5.2 | 0.856 | 51 | 3.0(0.1) | 2.2(0.5) | 122(15) |
| $^{13}CN$ | 1(2, 1) − 0(1, 1), F = 0 − 1 | 108644.346(5e-2) | 5.2 | 0.642 | 36 | 3.0(0.2) | 2.1(0.5) | 81(16) |
| $^{13}CN$ | 1(2, 1) − 0(1, 1), F = 1 − 1 | 108645.064(5e-2) | 5.2 | 0.551 | blended | – | – | – |
| $^{13}CN$ | 1(1, 1) − 0(1, 0), F = 2 − 1 | 108651.297(5e-2) | 5.2 | 3.276 | 51 | 3.1(0.5) | 2.2(0.5) | 121(6) |
| $^{13}CN$ | 1(2, 1) − 0(1, 1), F = 2 − 2 | 108657.646(5e-2) | 5.2 | 2.420 | 35 | 3.0(0.5) | 2.3(0.5) | 85(6) |
| $^{13}CN$ | 1(2, 1) − 0(1, 1), F = 1 − 2 | 108658.948(5e-2) | 5.2 | 0.669 | blended | – | – | – |
| $^{13}CN$ | 1(2, 2) − 0(1, 1), F = 3 − 2 | 108780.201(5e-2) | 5.2 | 4.905 | 51 | 3.1(0.1) | 2.1(0.3) | 114(16) |
| $^{13}CN$ | 1(2, 2) − 0(1, 1), F = 2 − 1 | 108782.374(5e-2) | 5.2 | 2.586 | 41 | 3.1(0.2) | 1.7(0.4) | 72(14) |

**Table A2.** (Continued)

| Species | Transitions | Rest Freq. (MHz) | $E_u$ (K) | $\mu^2S$ ($D^2$) | $T_{mb}$ (mK) | $V_{LSR}$ (km $s^{-1}$) | $\Delta V$ (km $s^{-1}$) | $\int T_{mb}$ dv (mK km $s^{-1}$) |
|---|---|---|---|---|---|---|---|---|
| $^{13}CN$ | 1(2, 2) − 0(1, 1), F = 1 − 0 | 108786.982(5e-2) | 5.2 | 1.144 | 17 | 3.3(0.5) | 2.1(1.3) | 38(18) |
| $CH_3OH$, vt=0-2 | 0(0) − 1(-1) E2, vt=0 | 108893.945(12e-3) | 13.1 | 3.9134 | 548 | 3.1(0.) | 2.9(0.1) | 1713(20) |
| $HC_3N$ | 12 − 11 | 109173.634(1e-2) | 34.1 | 167.1 | 1348 | 3.3(0.) | 2.5(0.1) | 3565(19) |
| SO | 3(2) − 2(1) | 109252.220(1e-1) | 21.1 | 3.5585 | 959 | 3.4(0.) | 2.6(0.1) | 2686(25) |
| OCS | 9 − 8 | 109463.063(5e-3) | 26.3 | 4.6034 | 193 | 3.3(0.1) | 2.6(0.1) | 538(21) |
| $C^{18}O$ | 1 − 0 | 109782.173(6e-3) | 5.3 | 0.01221 | 1265 | 3.0(0.1) | 3.0(0.1) | 3994(17) |
| HNCO | 5(0, 5) − 4(0, 4) | 109905.749(7e-3) | 15.8 | 12.482 | 211 | 3.2(0.1) | 2.7(0.1) | 607(24) |
| $C^{15}N$ | 1(2, 1) − 0(1, 0) | 110023.540(1e-1) | 5.3 | 1.386 | blended | – | – | – |
| $C^{15}N$ | 1(2, 2) − 0(1, 1) | 110024.590(1e-1) | 5.3 | 3.504 | 34 | 3.6(0.6) | 2.7(1.0) | 135(31) |
| $^{13}CO$ | 1 − 0 | 110201.35(0) | 5.3 | 0.01220 | 12122 | 3.0(0.1) | 3.6(0.1) | 46171(138) |
| $CH_3CN$ | 6(3, 0) − 5(-3, 0) | 110364.354(0) | 82.8 | 138.45 | 36 | 3.2(0.4) | 3.0(0.5) | 114(18) |
| $CH_3CN$ | 6(-3, 0) − 5(3, 0) | 110364.354(0) | 82.8 | 138.45 | blended | – | – | – |
| $CH_3CN$ | 6(2, 0) − 5(2, 0) | 110374.989(0) | 47.1 | 164.06 | 64 | 3.2(0.5) | 2.7(0.5) | 186(18) |
| $CH_3CN$ | 6(1, 0) − 5(1, 0) | 110381.372(0) | 25.7 | 179.45 | 125 | 3.2(0.4) | 2.9(0.5) | 386(18) |
| $CH_3CN$ | 6(0, 0) − 5(0, 0) | 110383.500(0) | 18.5 | 184.58 | 162 | 3.2(0.5) | 3.0(0.5) | 513(18) |
| t-HCOOH | 5(0, 5) − 4(0, 4) | 111746.784(3e-3) | 16.1 | 10.092 | 43 | 3.0(0.2) | 2.3(0.5) | 105(22) |
| $CH_3CHO$ | 6(1, 6) − 5(1, 5) A, vt=0 | 112248.716(3e-3) | 21.1 | 73.76807 | 63 | 3.2(0.3) | 1.9(0.6) | 128(35) |
| $CH_3CHO$ | 6(1, 6) − 5(1, 5) E, vt=0 | 112254.508(3e-3) | 21.2 | 73.79585 | 79 | 3.2(0.3) | 2.6(0.6) | 214(42) |
| $C^{17}O$ | 1 − 0 | 112359.284(1e-3) | 5.4 | 0.01217 | 243 | 3.0(0.2) | 3.2(0.3) | 819(89) |
| CN | N= 1-0, J=1/2-1/2, F=1/2-1/2 | 113123.370(6e-3) | 5.4 | 0.15271 | 229 | 3.2(0.5) | 2.7(0.5) | 663(122) |
| CN | N= 1-0, J=1/2-1/2, F=1/2-3/2 | 113144.157(6e-3) | 5.4 | 1.2492 | 1322 | 3.2(0.3) | 3.1(0.5) | 4335(122) |
| CN | N= 1-0, J=1/2-1/2, F=3/2-1/2 | 113170.492(4e-3) | 5.4 | 1.2199 | 1438 | 3.2(0.) | 2.9(0.5) | 4422(122) |
| CN | N= 1-0, J=1/2-1/2, F=3/2-3/2 | 113191.279(3e-3) | 5.4 | 1.5836 | 1423 | 3.2(0.5) | 3.0(0.5) | 4925(122) |
| CCS | 9(8) − 8(7) | 113410.186(2e-2) | 33.6 | 65.427 | 40 | 3.4(0.4) | 3.8(0.7) | 164(28) |
| CN | N= 1-0, J=3/2-1/2, F=3/2-1/2 | 113488.120(3e-3) | 5.4 | 1.5838 | 1402 | 3.2(0.) | 3.1(0.1) | 4618(27) |
| CN | N= 1-0, J=3/2-1/2, F=5/2-3/2 | 113490.970(2e-3) | 5.4 | 4.205 | 3251 | 3.2(0.) | 3.3(0.1) | 11329(22) |
| CN | N= 1-0, J=3/2-1/2, F=1/2-1/2 | 113499.644(3e-3) | 5.4 | 1.2491 | 980 | 3.2(0.) | 3.0(0.1) | 3140(25) |
| CN | N= 1-0, J=3/2-1/2, F=3/2-3/2 | 113508.907(3e-3) | 5.4 | 1.2196 | 1127 | 3.2(0.) | 3.0(0.1) | 3565(26) |
| CN | N= 1-0, J=3/2-1/2, F=1/2-3/2 | 113520.432(4e-3) | 5.4 | 0.15263 | 144 | 3.2(0.1) | 3.1(0.2) | 482(26) |
| | | G192.60−00.04 | | | | | | |
| $NH_2CHO$ | 5(2, 4) − 4(2, 3) | 105972.665(37e-3) | 27.2 | 54.915 | 46 | 5.5(0.3) | 4.8(0.6) | 236(26) |
| $NH_2CHO$ | 5(4, 1) − 4(4, 0) | 106107.870(88e-3) | 63.0 | 23.537 | 40 | 5.4(0.5) | 5.8(0.5) | 246(79) |
| $NH_2CHO$ | 5(4, 2) − 4(4, 1) | 106107.845(88e-3) | 63.0 | 23.537 | blended | – | – | – |
| $CH_3OCHO$ | 3(3, 0) − 2(2, 1) A | 106125.344(1e-2) | 9.5 | 1.13527 | 19 | 7.0(0.5) | 5.4(0.5) | 110(79) |
| $NH_2CHO$ | 5(3, 3) − 4(3, 2) | 106134.468(55e-3) | 42.1 | 41.845 | 32 | 5.5(0.5) | 4.1(0.5) | 139(79) |
| $NH_2CHO$ | 5(3, 2) − 4(3, 1) | 106141.442(55e-3) | 42.1 | 41.84 | 39 | 5.5(0.4) | 4.2(0.5) | 174(79) |
| CCS | 8(9) − 7(8) | 106347.726(2e-2) | 25.0 | 74.425 | 93 | 7.5(0.1) | 1.5(0.2) | 151(19) |
| $NH_2CHO$ | 5(2, 3) − 4(2, 2) | 106541.773(37e-3) | 27.2 | 54.915 | 21 | 5.4(0.6) | 5.3(1.1) | 120(25) |
| $^{34}SO$ | 3(2) − 2(1) | 106743.244(7e-2) | 20.9 | 3.557 | 67 | 7.0(0.1) | 2.8(0.4) | 199(19) |
| $CH_3OH$, vt=0-2 | $3(1)^+ - 4(0)^+$, vt=0 | 107013.831(1e-2) | 28.3 | 12.036 | 9838 | 5.5(0.5) | 1.5(0.5) | 16136(942) |
| $CH_3OH$, vt=0-2 | 15(-2) − 15(1) E2, vt=0 | 107159.906(14e-3) | 304.7 | 10.421 | 47 | 5.5(0.2) | 4.2(0.4) | 214(18) |
| $CH_3OCHO$ | 9(2, 8) − 8(2, 7) E | 107537.258(1e-2) | 28.8 | 22.60702 | 25 | 7.0(0.3) | 2.6(0.9) | 70(18) |
| $CH_3OCHO$ | 9(2, 8) − 8(2, 7) A | 107543.711(1e-2) | 28.8 | 22.61344 | 29 | 7.1(0.3) | 2.6(0.6) | 80(17) |
| $SO_2$ | 12(4, 8) − 13(3, 11) | 107843.470(2e-3) | 111.0 | 4.5354 | 15 | 6.5(0.7) | 6.4(1.3) | 100(22) |
| t-HCOOH | 5(1, 5) − 4(1, 4) | 108126.720(3e-3) | 18.8 | 9.6966 | 45 | 5.5(0.3) | 4.5(0.6) | 215(28) |
| $^{13}CN$ | 1(1, 0) − 0(1, 1), F = 1 − 2 | 108426.889(5e-2) | 5.2 | 1.267 | 17 | 6.0(0.4) | 2.5(0.9) | 45(14) |
| $^{13}CN$ | 1(1, 1) − 0(1, 0), F = 0 − 1 | 108631.121(5e-2) | 5.2 | 0.642 | 14 | 6.2(0.5) | 1.5(0.5) | 23(6) |
| $^{13}CN$ | 1(1, 1) − 0(1, 0), F = 1 − 1 | 108636.923(5e-2) | 5.2 | 1.932 | 31 | 6.6(0.5) | 3.0(0.5) | 97(6) |
| $^{13}CN$ | 1(2, 1) − 0(1, 1), F = 1 − 0 | 108638.212(5e-2) | 5.2 | 0.722 | blended | – | – | – |
| $C_2H_5OH$ | 13(3, 10) − 13(2, 11) | 108438.579(5e-2) | 88.2 | 18.79 | 25 | 5.7(0.4) | 4.3(1.0) | 116(21) |
| $^{13}CN$ | 1(2, 1) − 0(1, 1), F = 2 − 1 | 108643.590(5e-2) | 5.2 | 0.856 | 21 | 6.8(0.5) | 1.6(0.5) | 35(6) |
| $^{13}CN$ | 1(2, 1) − 0(1, 1), F = 0 − 1 | 108644.346(5e-2) | 5.2 | 0.642 | blended | – | – | – |
| $^{13}CN$ | 1(2, 1) − 0(1, 1), F = 1 − 1 | 108645.064(5e-2) | 5.2 | 0.551 | blended | – | – | – |
| $^{13}CN$ | 1(1, 1) − 0(1, 0), F = 2 − 1 | 108651.297(5e-2) | 5.2 | 3.276 | 55 | 6.7(0.5) | 1.8(0.5) | 104(6) |
| $^{13}CN$ | 1(2, 1) − 0(1, 1), F = 2 − 2 | 108657.646(5e-2) | 5.2 | 2.420 | 47 | 7.0(0.5) | 1.8(0.5) | 89(6) |
| $^{13}CN$ | 1(2, 1) − 0(1, 1), F = 1 − 2 | 108658.948(5e-2) | 5.2 | 0.669 | blended | – | – | – |
| $^{13}CN$ | 1(2, 2) − 0(1, 1), F = 3 − 2 | 108780.201(5e-2) | 5.2 | 4.905 | 95 | 7.3(0.1) | 2.0(0.2) | 203(18) |
| $^{13}CN$ | 1(2, 2) − 0(1, 1), F = 2 − 1 | 108782.374(5e-2) | 5.2 | 2.586 | 47 | 7.5(0.2) | 2.3(0.4) | 113(18) |
| $^{13}CN$ | 1(2, 2) − 0(1, 1), F = 1 − 0 | 108786.982(5e-2) | 5.2 | 1.144 | 20 | 7.1(0.4) | 1.6(0.9) | 34(16) |
| $CH_3OH$, vt=0-2 | 0(0) − 1(-1) E2, vt=0 | 108893.945(12e-3) | 13.1 | 3.9134 | 632 | 5.5(0.) | 3.5(0.1) | 2341(26) |
| $CH_3OH$, vt=0-2 | 14(5) − 15(4) E1, vt=0 | 109138.783(15e-3) | 379.7 | 13.593 | 44 | 5.4(0.5) | 4.8(0.5) | 222(114) |
| $CH_3OH$, vt=0-2 | 16(-2) − 16(1) E2, vt=0 | 109153.184(14e-3) | 342.0 | 14.726 | 46 | 5.5(0.5) | 4.2(0.5) | 206(114) |
| $HC_3N$ | 12 − 11 | 109173.634(1e-2) | 34.1 | 167.1 | 1784 | 7.2(0.5) | 2.3(0.5) | 4357(114) |
| SO | 3(2) − 2(1) | 109252.220(1e-1) | 21.1 | 3.5585 | 1497 | 7.3(0.) | 2.5(0.1) | 4011(24) |
| OCS | 9 − 8 | 109463.063(5e-3) | 26.3 | 4.6034 | 249 | 7.5(0.1) | 2.7(0.2) | 710(47) |
| HNCO | 5(1, 5) − 4(1, 4) | 109495.996(6e-3) | 59.0 | 11.847 | 31 | 5.2(0.6) | 1.8(1.0) | 59(34) |
| $SO_2$ | 17(5, 13) − 18(4, 14) | 109757.585(2e-3) | 202.1 | 6.6069 | 25 | 6.4(0.6) | 1.2(1.0) | 33(29) |
| $C^{18}O$ | 1 − 0 | 109782.173(6e-3) | 5.3 | 0.01221 | 2080 | 7.8(0.1) | 3.0(0.1) | 6699(57) |
| HNCO | 5(2, 3) − 4(2, 2) | 109872.765(3e-2) | 186.1 | 10.012 | 26 | 5.2(0.5) | 1.2(0.9) | 32(250 |
| HNCO | 5(2, 4) − 4(2, 3) | 109872.337(3e-2) | 186.1 | 10.013 | blended | – | – | – |
| HNCO | 5(0, 5) − 4(0, 4) | 109905.749(7e-3) | 15.8 | 12.482 | 257 | 5.2(0.1) | 3.2(0.1) | 880(33) |
| $^{13}CO$ | 1 − 0 | 110201.35(0) | 5.3 | 0.01220 | 22496 | 7.5(0.1) | 3.2(0.1) | 77667(75) |
| $CH_3CN$ | 6(5, 0) − 5(5, 0) | 110330.345(0) | 197.1 | 56.399 | blended | – | – | – |
| $CH_3CN$ | 6(4, 0) − 5(4, 0) | 110349.471(0) | 132.8 | 102.54 | 38 | 6.4(0.4) | 3.8(0.5) | 152(24) |
| $CH_3CN$ | 6(3, 0) − 5(-3, 0) | 110364.354(0) | 82.8 | 138.45 | 114 | 6.4(0.5) | 4.6(0.5) | 554(24) |
| $CH_3CN$ | 6(-3, 0) − 5(3, 0) | 110364.354(0) | 82.8 | 138.45 | blended | – | – | – |
| $CH_3CN$ | 6(2, 0) − 5(2, 0) | 110374.989(0) | 47.1 | 164.06 | 121 | 6.4(0.5) | 4.0(0.5) | 513(24) |
| $CH_3CN$ | 6(1, 0) − 5(1, 0) | 110381.372(0) | 25.7 | 179.45 | 221 | 6.3(0.5) | 3.2(0.5) | 762(24) |
| $CH_3CN$ | 6(0, 0) − 5(0, 0) | 110383.500(0) | 18.5 | 184.58 | 250 | 6.4(0.4) | 4.1(0.5) | 1085(24) |
| $C_2H_5OH$ | 21(3, 18) − 21(2, 19) | 110452.276(5e-2) | 208.7 | 35.016 | 14 | 5.5(1.0) | 2.0(1.9) | 30(23) |
| $CH_3OCHO$ | 9(8, 1) − 8(8, 0) A | 110455.372(1e-2) | 69.0 | 5.02998 | 14 | 7.0(1.0) | 2.8(1.8) | 43(26) |
| $CH_3OCHO$ | 9(7, 3) − 8(7, 2) E | 110536.003(1e-2) | 59.1 | 9.46692 | 19 | 7.0(0.7) | 3.1(1.6) | 64(30) |
| $CH_3OCHO$ | 9(6, 4) − 8(6, 3) E | 110662.315(1e-2) | 50.4 | 13.30855 | 25 | 7.0(0.5) | 1.8(0.5) | 47(7) |
| $CH_3OCHO$ | 9(6, 3) − 8(6, 2) A | 110663.429(1e-2) | 50.4 | 13.31127 | 25 | 7.1(0.5) | 3.1(0.5) | 82(7) |
| $CH_3OCHO$ | 9(6, 4) − 8(6, 3) A | 110663.273(1e-2) | 50.4 | 13.3113 | blended | – | – | – |
| $CH_3OCHO$ | 10(1,10) − 9(1, 9) E | 110788.664(1e-2) | 30.3 | 26.16584 | 29 | 7.0(0.4) | 2.3(0.9) | 72(22) |
| $CH_3OCHO$ | 10(1,10) − 9(1, 9) A | 110790.526(1e-2) | 30.3 | 26.17539 | 21 | 7.0(0.6) | 1.4(1.4) | 31(22) |
| $CH_3OCHO$ | 9(3, 7) − 8(3, 6) E | 110879.766(1e-2) | 32.6 | 21.245 | 25 | 7.0(0.2) | 0.5(0.3) | 15(13) |
| $CH_3OCHO$ | 9(5, 5) − 8(5, 4) A | 110880.447(1e-2) | 43.2 | 16.56015 | 29 | 7.1(0.5) | 3.8(1.0) | 119(31) |
| $CH_3OCHO$ | 9(5, 5) − 8(5, 4) E | 110882.331(1e-2) | 43.2 | 16.55225 | 28 | 7.0(0.3) | 1.4(0.7) | 41(19) |
| $CH_3OCHO$ | 9(3, 7) − 8(3, 6) A | 110887.092(1e-2) | 32.6 | 21.25577 | 20 | 7.1(1.0) | 6.3(2.2) | 134(42) |
| $CH_3OCHO$ | 9(5, 4) − 8(5, 3) A | 110890.256(1e-2) | 43.2 | 16.56106 | 21 | 7.0(0.8) | 3.3(1.6) | 75(31) |
| $CH_3OCHO$ | 10(0, 10) − 9(0, 9) E | 111169.903(1e-2) | 30.2 | 26.18776 | 34 | 7.0(0.4) | 2.7(0.5) | 99(14) |
| $CH_3OCHO$ | 10(0, 10) − 9(0, 9) A | 111171.634(1e-2) | 30.2 | 26.19136 | 33 | 7.0(0.5) | 6.8(0.5) | 237(14) |
| $CH_3OCHO$ | 9(4, 6) − 8(4, 5) E | 111223.491(1e-2) | 37.2 | 18.18412 | 20 | 7.0(1.0) | 5.4(3.3) | 113(47) |
| $CH_3OH$, vt=0-2 | $7(2)^+ - 8(1)^+$, vt=0 | 111289.453(13e-3) | 102.7 | 9.3425 | 185 | 5.5(0.) | 4.9(0.2) | 969(31) |
| $CH_3OH$, vt=0-2 | 17(-2) − 17(1) E2, vt=0 | 111626.514(15e-3) | 381.5 | 20.231 | 406 | 5.5(0.) | 1.2(0.5) | 499(64) |
| $CH_3OCHO$ | 9(1, 8) − 8(1, 7) E | 111674.131(1e-2) | 28.1 | 23.18984 | 33 | 7.0(0.6) | 9.3(0.5) | 325(64) |

**Table A2.** (Continued)

| Species | Transitions | Rest Freq. (MHz) | $E_u$ (K) | $\mu^2S$ ($D^2$) | $T_{mb}$ (mK) | $V_{LSR}$ (km $s^{-1}$) | $\Delta V$ (km $s^{-1}$) | $\int T_{mb}$ dv (mK km $s^{-1}$) |
|---|---|---|---|---|---|---|---|---|
| $CH_3OCHO$ | 9(1, 8) − 8(1, 7) A | 111682.189(1e-2) | 28.1 | 23.19587 | 29 | 7.0(0.5) | 9.8(0.5) | 301(64) |
| t-HCOOH | 5(0, 5) − 4(0, 4) | 111746.784(3e-3) | 16.1 | 10.092 | 50 | 5.5(0.3) | 4.2(0.8) | 222(40) |
| $CH_3CHO$ | 6(1, 6) − 5(1, 5) A, vt=0 | 112248.716(3e-3) | 21.1 | 73.76807 | 92 | 6.4(0.2) | 3.2(0.6) | 318(45) |
| $CH_3CHO$ | 6(1, 6) − 5(1, 5) E, vt=0 | 112254.508(3e-3) | 21.2 | 73.79585 | 94 | 6.4(0.2) | 2.2(0.4) | 225(34) |
| t-HCOOH | 5(2, 4) − 4(2, 3) | 112287.145 (3e-3) | 28.9 | 8.4851 | 22 | 5.5(0.7) | 2.4(1.5) | 55(33) |
| $C^{17}O$ | 1 − 0 | 112359.284(1e-3) | 5.4 | 0.01217 | 403 | 7.8(0.1) | 4.6(0.1) | 1987(46) |
| t-HCOOH | 5(3, 2) − 4(3, 1) | 112467.007(3e-3) | 44.8 | 6.4654 | 35 | 5.5(0.5) | 4.1(0.5) | 154(11) |
| t-HCOOH | 5(2, 3) − 4(2, 2) | 112891.443 (3e-3) | 28.9 | 8.4849 | 25 | -5.5(0.7) | 2.0(1.2) | 53(35) |
| CN | N= 1-0, J=1/2-1/2, F=1/2-1/2 | 113123.370(6e-3) | 5.4 | 0.15271 | 319 | 7.5(0.5) | 2.5(0.5) | 860(157) |
| CN | N= 1-0, J=1/2-1/2, F=1/2-3/2 | 113144.157(6e-3) | 5.4 | 1.2492 | 1820 | 7.5(0.4) | 2.9(0.5) | 5555(157) |
| CN | N= 1-0, J=1/2-1/2, F=3/2-1/2 | 113170.492(4e-3) | 5.4 | 1.2199 | 1879 | 7.5(0.5) | 2.9(0.5) | 5725(157) |
| CN | N= 1-0, J=1/2-1/2, F=3/2-3/2 | 113191.279(3e-3) | 5.4 | 1.5836 | 2109 | 7.5(0.) | 3.0(0.5) | 6814(157) |
| CCS | 9(8) − 8(7) | 113410.186(2e-2) | 33.6 | 65.427 | 56 | 7.5(0.5) | 7.2(0.5) | 429(234) |
| CN | N= 1-0, J=3/2-1/2, F=3/2-1/2 | 113488.120(3e-3) | 5.4 | 1.5838 | 1923 | 7.5(0.5) | 3.0(0.5) | 6168(234) |
| CN | N= 1-0, J=3/2-1/2, F=5/2-3/2 | 113490.970(2e-3) | 5.4 | 4.205 | 4457 | 7.5(0.) | 3.2(0.5) | 15062 (234) |
| CN | N= 1-0, J=3/2-1/2, F=1/2-1/2 | 113499.644(3e-3) | 5.4 | 1.2491 | 1289 | 7.5(0.5) | 3.1(0.5) | 4220(234) |
| CN | N= 1-0, J=3/2-1/2, F=3/2-3/2 | 113508.907(3e-3) | 5.4 | 1.2196 | 1582 | 7.5(0.3) | 3.0(0.5) | 5101(234) |
| CN | N= 1-0, J=3/2-1/2, F=1/2-3/2 | 113520.432(4e-3) | 5.4 | 0.15263 | 223 | 7.5(0.5) | 3.3(0.5) | 786(234) |
| | | G209.00−19.38 | | | | | | |
| CCS | 8(9) − 7(8) | 106347.726(2e-2) | 25.0 | 74.425 | 41 | 8.7(0.1) | 1.9(0.2) | 81(9) |
| Hα | H (39) α | 106737.357(0) | − | − | 1003 | -1.4(0.) | 25.1(0.1) | 26798(76) |
| Heα | He (39) α | 106780.852(0) | − | − | 115 | -2.2(0.9) | 17.4(2.3) | 2126(257) |
| $CH_3OH$, vt=0-2 | $3(1)^+ - 4(0)^+$, vt=0 | 107013.831(1e-2) | 28.3 | 12.036 | 346 | 8.0(0.) | 3.1(0.1) | 1135(19) |
| $CH_3OH$, vt=0-2 | 15(-2) − 15(1) E2, vt=0 | 107159.906(14e-3) | 304.7 | 10.421 | 19 | 8.0(0.4) | 3.7(1.0) | 76(15) |
| Hε | H (65) ε | 107206.108(0) | − | − | 50 | -1.0 | 21.5(0.8) | 1141(42) |
| $C_2H_5CN$ | 12(7, 5) − 11(7, 4) | 107485.160(5e-2) | 88.0 | 117.36 | blended | − | − | − |
| $C_2H_5CN$ | 12(6, 6) − 11(6, 5) | 107486.949(5e-2) | 73.6 | 133.42 | 14 | 7.0(0.9) | 10.0(1.7) | 141(34) |
| $C_2H_5CN$ | 12(8, 4) − 11(8, 3) | 107491.574(5e-2) | 104.6 | 98.829 | 15 | 7.1(1.1) | 11.8(1.1) | 184(9) |
| $C_2H_5CN$ | 12(5, 7) − 11(5, 6) | 107502.432(5e-2) | 61.3 | 146.99 | 13 | 7.1(1.0) | 13.5(1.1) | 180(9) |
| $CH_3OCHO$ | 9( 2, 8) − 8( 2, 7) E | 107537.258(1e-2) | 28.8 | 22.60702 | 24 | 8.0(1.1) | 3.9(1.1) | 100(9) |
| $CH_3OCHO$ | 9( 2, 8) − 8( 2, 7) A | 107543.711(1e-2) | 28.8 | 22.61344 | 21 | 8.0(1.1) | 5.7(1.1) | 124(9) |
| $C_2H_5CN$ | 12(4, 9) − 11(4, 8) | 107544.042(5e-2) | 51.3 | 158.12 | blended | − | − | − |
| $C_2H_5CN$ | 12(4, 8) − 11(4, 7) | 107547.460(5e-2) | 51.3 | 158.11 | 13 | 7.0(0.9) | 12.0(1.1) | 164(9) |
| $C_2H_5CN$ | 12(3, 10) − 11(3, 9) | 107594.056(5e-2) | 43.6 | 166.77 | 12 | 7.1(1.1) | 6.3(1.1) | 80(9) |
| $C_2H_5CN$ | 12(3, 9) − 11(3, 8) | 107734.723(5e-2) | 43.6 | 166.76 | 11 | 7.1(0.8) | 3.2(1.6) | 38(17) |
| $SO_2$ | 12(4, 8) − 13(3, 11) | 107843.470(2e-3) | 111.0 | 4.5354 | 27 | 7.0(0.6) | 8.1(1.1) | 234(33) |
| $^{13}CN$ | 1(1, 1) − 0(1, 0), F = 0 − 1 | 108631.121(5e-2) | 5.2 | 0.642 | 9 | 7.1(0.4) | 1.1(0.4) | 11(10) |
| $^{13}CN$ | 1(1, 1) − 0(1, 0), F = 1 − 1 | 108636.923(5e-2) | 5.2 | 1.932 | 19 | 7.3(0.6) | 6.5(1.5) | 133(26) |
| $^{13}CN$ | 1(2, 1) − 0(1, 1), F = 1 − 0 | 108638.212(5e-2) | 5.2 | 0.722 | 13 | 7.4(1.0) | 4.1(2.9) | 55(33) |
| $^{13}CN$ | 1(2, 1) − 0(1, 1), F = 2 − 1 | 108643.590(5e-2) | 5.2 | 0.856 | 13 | 7.6(1.0) | 4.2(2.6) | 58(32) |
| $^{13}CN$ | 1(2, 1) − 0(1, 1), F = 0 − 1 | 108644.346(5e-2) | 5.2 | 0.642 | blended | − | − | − |
| $^{13}CN$ | 1(2, 1) − 0(1, 1), F = 1 − 1 | 108645.064(5e-2) | 5.2 | 0.551 | blended | − | − | − |
| $^{13}CN$ | 1(1, 1) − 0(1, 0), F = 2 − 1 | 108651.297(5e-2) | 5.2 | 3.276 | 22 | 8.1(0.5) | 6.1(3.1) | 142(42) |
| $^{13}CN$ | 1(2, 1) − 0(1, 1), F = 2 − 2 | 108657.646(5e-2) | 5.2 | 2.420 | 26 | 7.8(0.4) | 4.6(1.2) | 127(24) |
| $^{13}CN$ | 1(2, 1) − 0(1, 1), F = 1 − 2 | 108658.948(5e-2) | 5.2 | 0.669 | blended | − | − | − |
| $^{13}CN$ | 1(2, 2) − 0(1, 1), F = 3 − 2 | 108780.201(5e-2) | 5.2 | 4.905 | 14 | 8.3(0.4) | 2.9(0.9) | 45(11) |
| $^{13}CN$ | 1(2, 2) − 0(1, 1), F = 2 − 1 | 108782.374(5e-2) | 5.2 | 2.586 | 16 | 8.1(0.5) | 3.2(1.3) | 54(15) |
| $^{13}CN$ | 1(2, 2) − 0(1, 1), F = 1 − 0 | 108786.982(5e-2) | 5.2 | 1.144 | 37 | 8.5(0.1) | 3.0(0.4) | 118(13) |
| $^{13}CN$ | 1(2, 2) − 0(1, 1), F = 1 − 1 | 108793.753(5e-2) | 5.2 | 0.894 | 21 | 7.6(0.2) | 2.5(0.6) | 55(12) |
| $^{13}CN$ | 1(2, 2) − 0(1, 1), F = 2 − 2 | 108796.400(5e-2) | 5.2 | 0.918 | 13 | 8.0(0.3) | 1.7(0.8) | 23(9) |
| $CH_3OH$, vt=0-2 | 0(0) − 1(-1) E2, vt=0 | 108893.945(12e-3) | 13.1 | 3.9134 | 160 | 7.8(0.1) | 3.3(0.2) | 563(21) |
| $C_2H_5CN$ | 12(2, 10) − 11(2, 9) | 108940.554(5e-2) | 38.2 | 172.93 | blended | − | − | − |
| $C_2H_5CN$ | 11(3, 9) − 12(0, 12) | 108940.696(4e-3) | 38.4 | 0.042598 | 13 | 7.0(0.7) | 10.7(2.4) | 148(23) |
| $HC_3N$ | 12 − 11 | 109173.634(1e-2) | 34.1 | 167.1 | 1102 | 8.5(0.) | 2.2(0.1) | 2599(35) |
| SO | 3(2) − 2(1) | 109252.220(1e-1) | 21.1 | 3.5585 | 267 | 8.6(0.1) | 3.3(0.3) | 3783(56) |
| OCS | 9 − 8 | 109463.063(5e-2) | 26.3 | 4.6034 | 141 | 8.5(0.) | 3.5(0.2) | 523(17) |
| Hγ | H (55) γ | 109536.000(0) | − | − | 135 | -1.0 | 24.4(0.4) | 3505(52) |
| $C^{18}O$ | 1 − 0 | 109782.173(6e-3) | 5.3 | 0.01221 | 955 | 8.2(0.3) | 2.8(0.1) | 2832(16) |
| HNCO | 5(0, 5) − 4(0, 4) | 109905.749(7e-3) | 15.8 | 12.482 | 74 | 8.5(0.2) | 6.1(0.6) | 484(34) |
| $C^{15}N$ | 1(2, 1) − 0(1, 1) | 110004.091(3e-2) | 5.3 | 0.717 | 16 | 7.2(1.6) | 4.3(3.8) | 242(54) |
| $C^{15}N$ | 1(2, 1) − 0(1, 0) | 110023.540(1e-1) | 5.3 | 1.386 | 8 | 7.8(1.0) | 1.1(0.1) | 9(3) |
| $C^{15}N$ | 1(2, 2) − 0(1, 1) | 110024.590(1e-1) | 5.3 | 3.504 | blended | − | − | − |
| $^{13}CO$ | 1 − 0 | 110201.35(0) | 5.3 | 0.01220 | 11340 | 8.2(0.1) | 2.9(0.1) | 34664(91) |
| HNCO | 5(1, 4) − 4(1, 3) | 110298.089(5e-3) | 59.2 | 11.847 | 16 | 8.5(0.9) | 3.8(1.9) | 65(30) |
| $CH_3CN$ | 6(4, 0) − 5(4, 0) | 110349.471(0) | 132.8 | 102.54 | 35 | 8.5(1.1) | 5.6(1.1) | 207(47) |
| $CH_3CN$ | 6(3, 0) − 5(-3, 0) | 110364.354(0) | 82.8 | 138.45 | 133 | 8.5(1.0) | 4.7(1.1) | 665(47) |
| $CH_3CN$ | 6(-3, 0) − 5(3, 0) | 110364.354(0) | 82.8 | 138.45 | blended | − | − | − |
| $CH_3CN$ | 6(2, 0) − 5(2, 0) | 110374.989(0) | 47.1 | 164.06 | 143 | 8.5(1.1) | 4.0(1.1) | 612(47) |
| $CH_3CN$ | 6(1, 0) − 5(1, 0) | 110381.372(0) | 25.7 | 179.45 | 220 | 8.5(1.0) | 3.6(1.1) | 850(47) |
| $CH_3CN$ | 6(0, 0) − 5(0, 0) | 110383.500(0) | 18.5 | 184.58 | 256 | 8.4(1.1) | 3.5(1.1) | 946(47) |
| $CH_3OCHO$ | 9(7, 2) − 8(7, 1) E | 110525.741(1e-2) | 59.1 | 9.46492 | 20 | 8.0(0.7) | 1.9(2.1) | 41(32) |
| $CH_3OCHO$ | 9(7, 2) − 8(7, 1) A | 110535.186(1e-2) | 59.1 | 9.46711 | 16 | 8.1(1.4) | 5.3(2.7) | 90(45) |
| Hδ | H (60 ) δ | 110600.675(0) | − | − | 76 | -1.1 | 22.9(0.7) | 1850(52) |
| Hζ | H (68) ζ | 110636.1051(0) | − | − | 29 | -1.5 | 19.4(1.5) | 593(48) |
| $CH_3OCHO$ | 9(6, 3) − 8(6, 2) E | 110652.813(1e-2) | 50.5 | 13.30853 | 14 | 8.0(0.4) | 1.6(1.1) | 23(14) |
| $CH_3OCHO$ | 9(6, 4) − 8(6, 3) A | 110663.273(1e-2) | 50.4 | 13.3113 | 12 | 8.0(0.7) | 2.3(1.6) | 31(17) |
| $CH_3OCHO$ | 10(1,10) − 9(1, 9) E | 110788.664(1e-2) | 30.3 | 26.16584 | 33 | 8.0(0.5) | 1.5(0.5) | 54(8) |
| $CH_3OCHO$ | 10(1,10) − 9(1, 9) A | 110790.526(1e-2) | 30.3 | 26.17539 | 34 | 7.9(0.5) | 2.4(0.5) | 88(8) |
| $CH_3OCHO$ | 9(5, 4) − 8(5, 3) E | 110873.955(1e-2) | 43.2 | 16.55557 | 10 | 8.1(1.0) | 2.3(1.4) | 25(18) |
| $CH_3OCHO$ | 9(5, 5) − 8(5, 4) A | 110880.447(1e-2) | 43.2 | 16.56015 | 17 | 8.0(0.6) | 3.0(0.9) | 53(20) |
| $CH_3OCHO$ | 9(5, 5) − 8(5, 4) E | 110882.331(1e-2) | 43.2 | 16.55225 | 20 | 8.0(0.4) | 1.4(0.5) | 31(14) |
| $CH_3OCHO$ | 9(3, 7) − 8(3, 6) A | 110887.092(1e-2) | 32.6 | 21.25577 | 23 | 8.1(0.4) | 2.6(0.7) | 65(19) |
| $CH_3OCHO$ | 9(5, 4) − 8(5, 3) A | 110890.256(1e-2) | 43.2 | 16.56106 | 32 | 8.0(0.2) | 1.0(0.4) | 35(13) |
| $CH_3OCHO$ | 10(0, 10) − 9(0, 9) E | 111169.903(1e-2) | 30.2 | 26.18776 | 21 | 8.0(0.4) | 1.4(0.9) | 33(16) |
| $CH_3OCHO$ | 10(0, 10) − 9(0, 9) A | 111171.634(1e-2) | 30.2 | 26.19136 | 29 | 8.0(0.2) | 1.0(0.5) | 30(13) |
| $CH_3OCHO$ | 9(4, 6) − 8(4, 5) A | 111195.962(1e-2) | 37.2 | 19.21722 | 12 | 8.0(0.7) | 1.9(1.2) | 25(17) |
| $CH_3OH$, vt=0-2 | $7(2)^+ - 8(1)^+$, vt=0 | 111289.453(13e-3) | 102.7 | 9.3425 | 131 | 7.8(0.1) | 2.7(0.2) | 375(18) |
| $CH_3OCHO$ | 9(4, 5) − 8(4, 4) E | 111408.412(1e-2) | 37.3 | 18.18767 | 13 | 7.8(1.1) | 5.0(1.1) | 72(10) |
| $CH_3OCHO$ | 9(4, 5) − 8(4, 4) A | 111453.300(1e-2) | 37.2 | 19.21778 | 27 | 7.8(1.0) | 8.2(1.1) | 239(10) |
| $CH_3OCHO$ | 9(1, 8) − 8(1, 7) E | 111674.131(1e-2) | 28.1 | 23.18984 | 35 | 8.0(0.) | 2.6(0.6) | 97(17) |
| $CH_3OCHO$ | 9(1, 8) − 8(1, 7) A | 111682.189(1e-2) | 28.1 | 23.19587 | 33 | 8.0(0.2) | 1.8(0.3) | 64(12) |
| $CH_3OCHO$ | 10(1, 10) − 9(0, 9) E | 111734.002(1e-2) | 30.3 | 3.84434 | blended | − | − | − |
| $CH_3OCHO$ | 10(1, 10) − 9(0, 9) A | 111735.307(1e-2) | 30.3 | 3.84224 | 12 | 8.0(0.8) | 2.3(0.5) | 31(8) |
| $CH_3OCH_3$ | 19(3,16) − 19(2,17) AE | 111741.351(26e-3) | 187.5 | 123.39211 | 21 | 8.1(0.5) | 3.8(0.5) | 86(8) |
| $CH_3OCH_3$ | 9(3,16) − 19(2,17) EE | 111742.794(25e-3) | 187.5 | 329.06069 | 27 | 8.0(0.4) | 2.7(0.5) | 77(8) |
| $CH_3OCH_3$ | 19(3, 16) − 19(2, 17) AA | 111744.238(29e-3) | 187.5 | 205.6671 | 23 | 8.0(0.5) | 5.4(0.5) | 135(8) |
| $CH_3OCH_3$ | 7(0, 7) − 6(1, 6) AA | 111782.562(8e-3) | 25.2 | 53.86755 | 31 | 8.1(0.5) | 2.3(0.5) | 76(8) |
| $CH_3OCH_3$ | 7(0, 7) − 6(1, 6) EE | 111783.010(4e-2) | 25.3 | 86.2034 | blended | − | − | − |
| $CH_3OCH_3$ | 7(0, 7) − 6(1, 6) EA | 111783.647(7e-3) | 25.3 | 21.54865 | blended | − | − | − |

**Table A2.** (Continued)

| Species | Transitions | Rest Freq. (MHz) | $E_u$ (K) | $\mu^2S$ ($D^2$) | $T_{mb}$ (mK) | $V_{LSR}$ (km $s^{-1}$) | ΔV (km $s^{-1}$) | $\int T_{mb}$ dv (mK km $s^{-1}$) |
|---|---|---|---|---|---|---|---|---|
| $CH_3OCH_3$ | 7(0, 7) − 6(1, 6) AE | 111783.648(7e-3) | 25.3 | 32.32363 | blended | – | – | – |
| Hβ | H (48) β | 111885.070(0) | – | – | 311 | -1.8 | 25.3(0.3) | 8362(100) |
| $CH_3CHO$ | 6(1, 6) − 5(1, 5) A, vt=0 | 112248.716(3e-3) | 21.1 | 73.76807 | 31 | 8.5(0.7) | 3.0(1.3) | 99(42) |
| $CH_3CHO$ | 6(1, 6) − 5(1, 5) E, vt=0 | 112254.508(3e-3) | 21.2 | 73.79585 | 22 | 8.5(0.9) | 2.2(1.6) | 50(30) |
| $C^{17}O$ | 1 − 0 | 112359.284(1e-3) | 5.4 | 0.01217 | 149 | 8.5(0.2) | 3.4(0.5) | 537(65) |
| $CH_3OCH_3$ | 17(3, 14) − 17(2, 15) EA | 113057.427(19e-3) | 153.1 | 132.79 | 21 | 8.0(0.6) | 2.2(1.4) | 49(25) |
| $CH_3OCH_3$ | 17(3, 14) − 17(2, 15) AE | 113057.425(18e-3) | 153.1 | 88.525 | blended | – | – | – |
| $CH_3OCH_3$ | 17(3, 14) − 17(2, 15) EE | 113059.249(17e-3) | 153.1 | 354.12 | 31 | 8.1(0.4) | 2.7(1.1) | 88(27) |
| $CH_3OCH_3$ | 17(3, 14) − 17(2, 15) AA | 113061.072(22e-3) | 153.1 | 221.33 | 25 | 8.0(0.4) | 1.6(0.8) | 43(19) |
| CN | N= 1-0, J=1/2-1/2, F=1/2-1/2 | 113123.370(6e-3) | 5.4 | 0.15271 | 133 | 9.0(0.1) | 3.8(0.3) | 543(28) |
| CN | N= 1-0, J=1/2-1/2, F=1/2-3/2 | 113144.157(6e-3) | 5.4 | 1.2492 | 1069 | 9.0(0.1) | 3.4(0.1) | 3812(23) |
| CN | N= 1-0, J=1/2-1/2, F=3/2-1/2 | 113170.492(4e-3) | 5.4 | 1.2199 | 1093 | 9.0(0.) | 3.3(0.1) | 3880(22) |
| CN | N= 1-0, J=1/2-1/2, F=3/2-3/2 | 113191.279(3e-3) | 5.4 | 1.5836 | 1295 | 9.0(0.) | 3.4(0.1) | 4670(25) |
| CN | N= 1-0, J=3/2-1/2, F=3/2-1/2 | 113488.120(3e-3) | 5.4 | 1.5838 | 1143 | 9.0(0.5) | 3.8(0.5) | 4593(231) |
| CN | N= 1-0, J=3/2-1/2, F=5/2-3/2 | 113490.970(2e-3) | 5.4 | 4.205 | 3499 | 9.0(0.4) | 3.5(0.5) | 12867(231) |
| CN | N= 1-0, J=3/2-1/2, F=1/2-1/2 | 113499.644(3e-3) | 5.4 | 1.2491 | 800 | 9.0(0.5) | 3.9(0.5) | 3332(231) |
| CN | N= 1-0, J=3/2-1/2, F=3/2-3/2 | 113508.907(3e-3) | 5.4 | 1.2196 | 835 | 9.1(0.5) | 3.8(0.5) | 3414(231) |
| CN | N= 1-0, J=3/2-1/2, F=1/2-3/2 | 113520.432(4e-3) | 5.4 | 0.15263 | 103 | 9.1(0.3) | 6.4(0.5) | 709(231) |
| | | | | G232.62+00.99 | | | | |
| CCS | 8(9) − 7(8) | 106347.726(2e-2) | 25.0 | 74.425 | 54 | 18.0(0.1) | 2.8(0.3) | 159(14) |
| $^{34}SO$ | 3(2) − 2(1) | 106743.244(7e-2) | 20.9 | 3.557 | 39 | 16.3(0.1) | 2.4(0.4) | 100(12) |
| $CH_3OH$, vt=0-2 | $3(1)^+ − 4(0)^+$, vt=0 | 107013.831(1e-2) | 28.3 | 12.036 | 28 | 18.0(0.3) | 2.8(0.5) | 81(13) |
| $^{13}CN$ | 1(1, 0) − 0(1, 1), F = 1 − 2 | 108426.889(5e-2) | 5.2 | 1.267 | 12 | 16.1(0.5) | 4.3(1.2) | 56(13) |
| $^{13}CN$ | 1(1, 1) − 0(1, 0), F = 0 − 1 | 108631.121(5e-2) | 5.2 | 0.642 | 17 | 16.3(0.2) | 1.2(0.5) | 23(7) |
| $^{13}CN$ | 1(1, 1) − 0(1, 0), F = 1 − 1 | 108636.923(5e-2) | 5.2 | 1.932 | 99 | 16.4(0.7) | 5.0(1.5) | 53(15) |
| $^{13}CN$ | 1(2, 1) − 0(1, 1), F = 1 − 0 | 108638.212(5e-2) | 5.2 | 0.722 | 14 | 16.6(0.4) | 2.1(0.9) | 31(10) |
| $^{13}CN$ | 1(2, 1) − 0(1, 1), F = 2 − 1 | 108643.590(5e-2) | 5.2 | 0.856 | 12 | 16.2(0.7) | 5.5(1.4) | 71(16) |
| $^{13}CN$ | 1(2, 1) − 0(1, 1), F = 0 − 1 | 108644.346(5e-2) | 5.2 | 0.642 | blended | – | – | – |
| $^{13}CN$ | 1(2, 1) − 0(1, 1), F = 1 − 1 | 108645.064(5e-2) | 5.2 | 0.551 | blended | – | – | – |
| $^{13}CN$ | 1(1, 1) − 0(1, 0), F = 2 − 1 | 108651.297(5e-2) | 5.2 | 3.276 | 20 | 16.8(0.4) | 4.7(1.2) | 101(17) |
| $^{13}CN$ | 1(2, 1) − 0(1, 1), F = 2 − 2 | 108657.646(5e-2) | 5.2 | 2.420 | 28 | 17.1(0.2) | 2.5(0.4) | 74(10) |
| $^{13}CN$ | 1(2, 1) − 0(1, 1), F = 1 − 2 | 108658.948(5e-2) | 5.2 | 0.669 | blended | – | – | – |
| $^{13}CN$ | 1(2, 2) − 0(1, 1), F = 3 − 2 | 108780.201(5e-2) | 5.2 | 4.905 | 29 | 16.4(0.2) | 4.4(0.6) | 137(15) |
| $^{13}CN$ | 1(2, 2) − 0(1, 1), F = 2 − 1 | 108782.374(5e-2) | 5.2 | 2.586 | 35 | 16.6(0.1) | 1.8(0.2) | 66(9) |
| $^{13}CN$ | 1(2, 2) − 0(1, 1), F = 1 − 0 | 108786.982(5e-2) | 5.2 | 1.144 | 19 | 17.2(0.1) | 0.8(0.4) | 17(7) |
| $^{13}CN$ | 1(2, 2) − 0(1, 1), F = 1 − 1 | 108793.753(5e-2) | 5.2 | 0.894 | 11 | 16.8(0.4) | 2.3(0.8) | 27(9) |
| $^{13}CN$ | 1(2, 2) − 0(1, 1), F = 2 − 2 | 108796.400(5e-2) | 5.2 | 0.918 | 12 | 17.1(0.3) | 1.3(0.6) | 17(7) |
| $CH_3OH$, vt=0-2 | 0(0) − 1(-1) E2, vt=0 | 108893.945(12e-3) | 13.1 | 3.9134 | 81 | 18.1(0.1) | 4.9(0.2) | 423(17) |
| $HC_3N$ | 12 − 11 | 109173.634(1e-2) | 34.1 | 167.1 | 1244 | 17.0(0.) | 2.1(0.1) | 2834(25) |
| SO | 3(2) − 2(1) | 109252.220(1e-1) | 21.1 | 3.5585 | 558 | 17.1(0.) | 3.0(0.1) | 1803(19) |
| OCS | 9 − 8 | 109463.063(5e-3) | 26.3 | 4.6034 | 36 | 16.8(0.3) | 3.2(1.0) | 123(23) |
| $C^{18}O$ | 1 − 0 | 109782.173(6e-3) | 5.3 | 0.01221 | 1166 | 16.0(0.1) | 3.4(0.1) | 4251(6) |
| HNCO | 5(0, 5) − 4(0, 4) | 109905.749(7e-3) | 15.8 | 12.482 | 50 | 16.5(0.4) | 1.4(0.9) | 75(45) |
| $^{13}CO$ | 1 − 0 | 110201.35(0) | 5.3 | 0.01220 | 11589 | 16.2(0.1) | 4.3(0.1) | 53250(79) |
| $CH_3CN$ | 6(5, 0) − 5(5, 0) | 110330.345(0) | 197.1 | 56.399 | 27 | 17.2(0.5) | 3.9(0.5) | 112(11) |
| $CH_3CN$ | 6(4, 0) − 5(4, 0) | 110349.471(0) | 132.8 | 102.54 | 16 | 17.2(0.5) | 9.4(0.5) | 160(11) |
| $CH_3CN$ | 6(3, 0) − 5(-3, 0) | 110364.354(0) | 82.8 | 138.45 | 36 | 17.1(0.5) | 3.0(0.5) | 115(11) |
| $CH_3CN$ | 6(-3, 0) − 5(3, 0) | 110364.354(0) | 82.8 | 138.45 | blended | – | – | – |
| $CH_3CN$ | 6(2, 0) − 5(2, 0) | 110374.989(0) | 47.1 | 164.06 | 43 | 17.2(0.5) | 6.2(0.5) | 280(11) |
| $CH_3CN$ | 6(1, 0) − 5(1, 0) | 110381.372(0) | 25.7 | 179.45 | 88 | 17.2(0.4) | 3.5(0.5) | 329(11) |
| $CH_3CN$ | 6(0, 0) − 5(0, 0) | 110383.500(0) | 18.5 | 184.58 | 119 | 17.2(0.5) | 2.7(0.5) | 345(11) |
| $C^{17}O$ | 1 − 0 | 112359.284(1e-3) | 5.4 | 0.01217 | 129 | 15.8(0.9) | 2.6(1.7) | 356(197) |
| CN | N= 1-0, J=1/2-1/2, F=1/2-1/2 | 113123.370(6e-3) | 5.4 | 0.15271 | 167 | 17.0(0.5) | 2.8(0.5) | 501(75) |
| CN | N= 1-0, J=1/2-1/2, F=1/2-3/2 | 113144.157(6e-3) | 5.4 | 1.2492 | 759 | 17.1(0.5) | 3.6(0.5) | 2927(75) |
| CN | N= 1-0, J=1/2-1/2, F=3/2-1/2 | 113170.492(4e-3) | 5.4 | 1.2199 | 815 | 17.0(0.5) | 3.4(0.5) | 2932(75) |
| CN | N= 1-0, J=1/2-1/2, F=3/2-3/2 | 113191.279(3e-3) | 5.4 | 1.5836 | 889 | 17.1(0.5) | 3.4(0.5) | 3249(75) |
| CN | N= 1-0, J=3/2-1/2, F=3/2-1/2 | 113488.120(3e-3) | 5.4 | 1.5838 | 834 | 17.0(0.5) | 3.5(0.5) | 3121(163) |
| CN | N= 1-0, J=3/2-1/2, F=5/2-3/2 | 113490.970(2e-3) | 5.4 | 4.205 | 1721 | 17.0(0.5) | 4.1(0.5) | 7456(163) |
| CN | N= 1-0, J=3/2-1/2, F=1/2-1/2 | 113499.644(3e-3) | 5.4 | 1.2491 | 569 | 17.0(0.4) | 4.1(0.5) | 2476(163) |
| CN | N= 1-0, J=3/2-1/2, F=3/2-3/2 | 113508.907(3e-3) | 5.4 | 1.2196 | 701 | 17.0(0.5) | 3.4(0.5) | 2521(163) |
| CN | N= 1-0, J=3/2-1/2, F=1/2-3/2 | 113520.432(4e-3) | 5.4 | 0.15263 | 105 | 17.0(0.7) | 8.3(0.5) | 920(163) |

**Note.** (1): Molecule name; (2): Transition quantum numbers; (3): Rest frequency; (4): Upper state energy level (K); (5): Dipole-weighted transition dipole matrix elements; (6): Peak intensity; (7): centroid velocity; (8): FWHM, (9): Integrated intensity. "−" represents no values.
